# Supplementary material for: Bayesian Convolutional Deep Sets with Task-Dependent Stationary Prior
Source: arXiv:2210.12363 source file (2022-10-22)
Supplement: Supplementary file 1 [file 07-appendix-v01-chapter2-exp1-figure01-ablation.tex]

\begin{figure*}[htp!]
%\begin{figure*}[t]
\centering
\hspace{-2.5mm}
\subfloat[\label{fig:nd-multitask-a} rbf ]
{\includegraphics[width=0.235\linewidth,height=2.8cm]{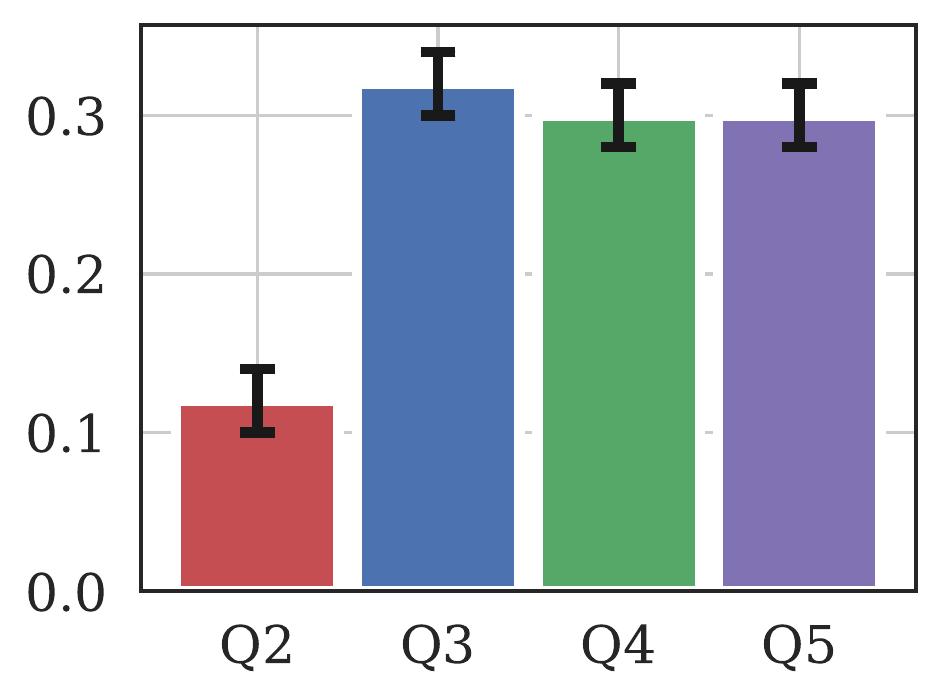}} \hspace{2mm}  
\subfloat[\label{fig:nd-multitask-b} matern-$\frac{5}{2}$]
{\includegraphics[width=0.235\linewidth,height=2.8cm]{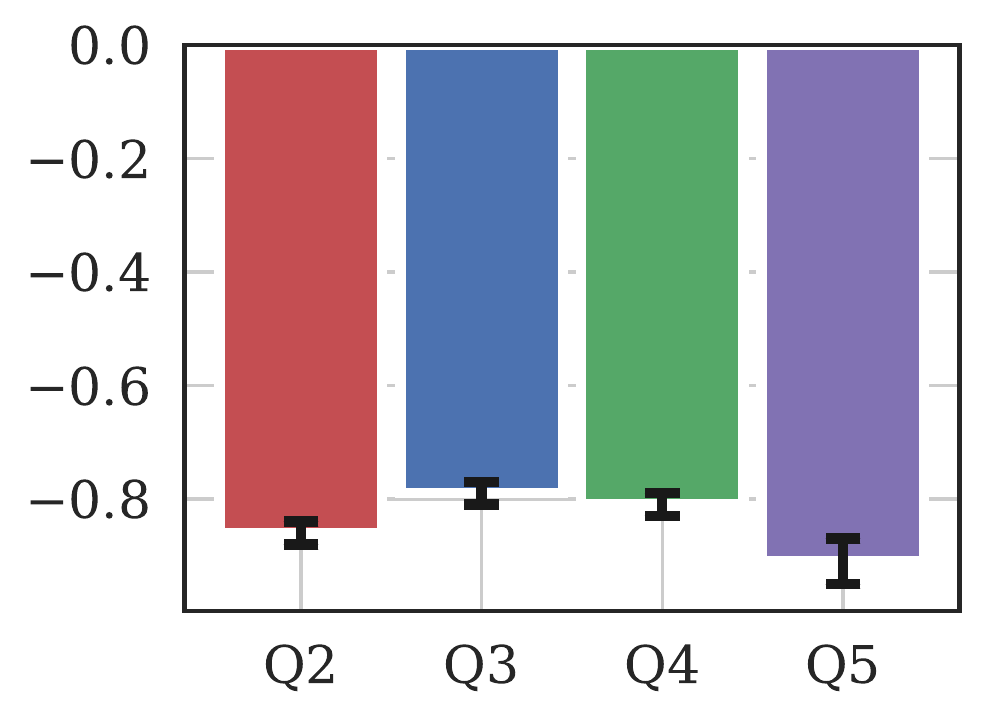}} \hspace{2mm} 
\subfloat[\label{fig:nd-multitask-c} weakly periodic]
{\includegraphics[width=0.235\linewidth,height=2.8cm]{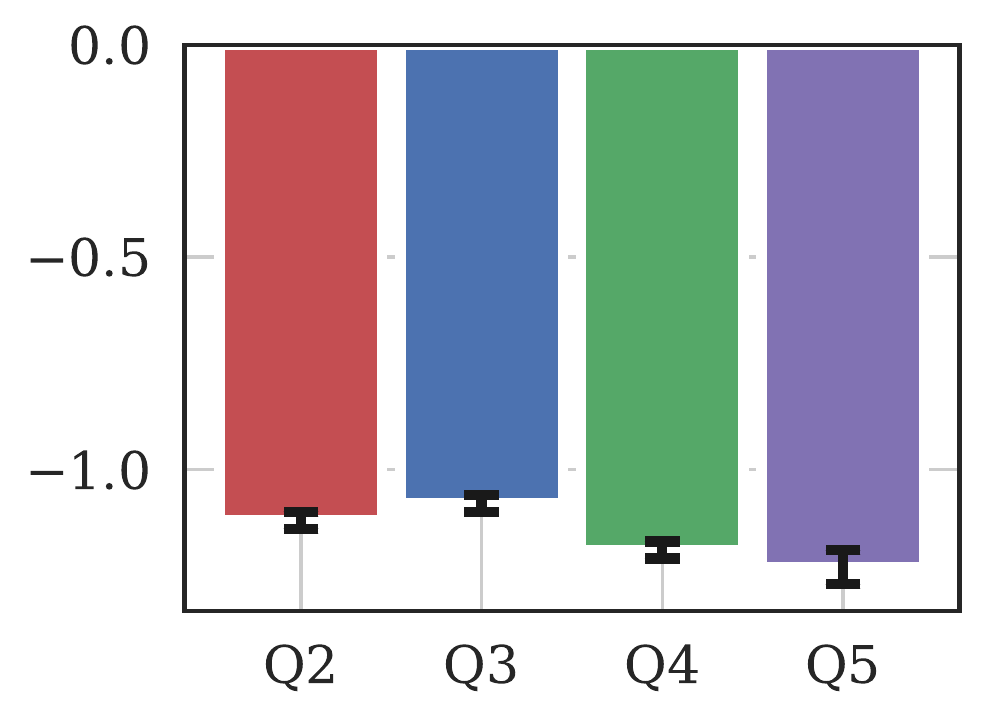}} \hspace{2mm}
\subfloat[\label{fig:nd-multitask-d} sawtooth]
{\includegraphics[width=0.235\linewidth,height=2.8cm]{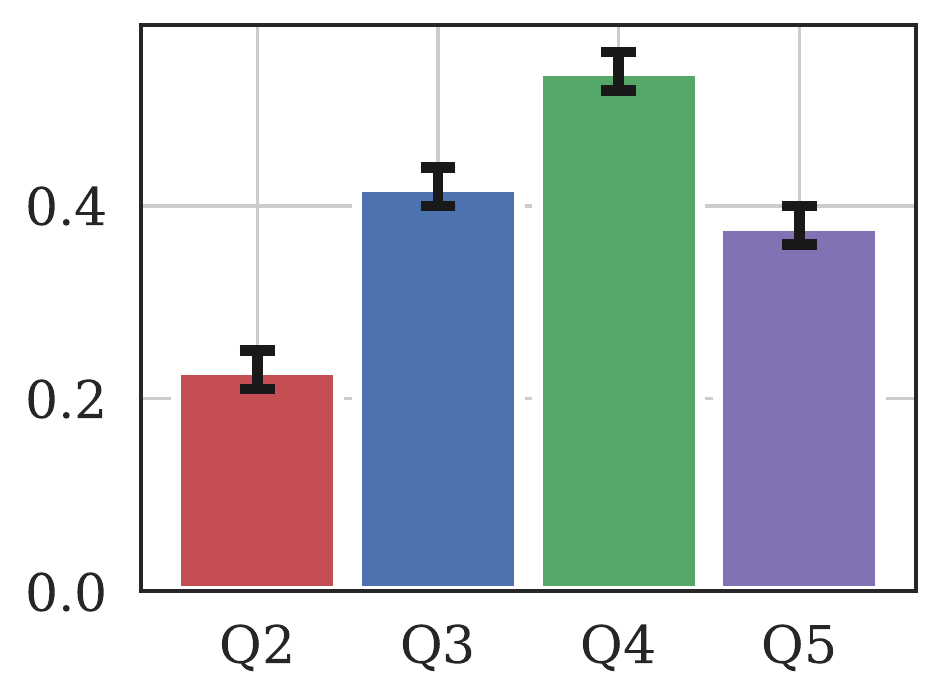}} \hspace{2mm}

\hspace{-2.5mm}
\subfloat[\label{fig:nd-multitask-a} rbf ]
{\includegraphics[width=0.235\linewidth,height=2.8cm]{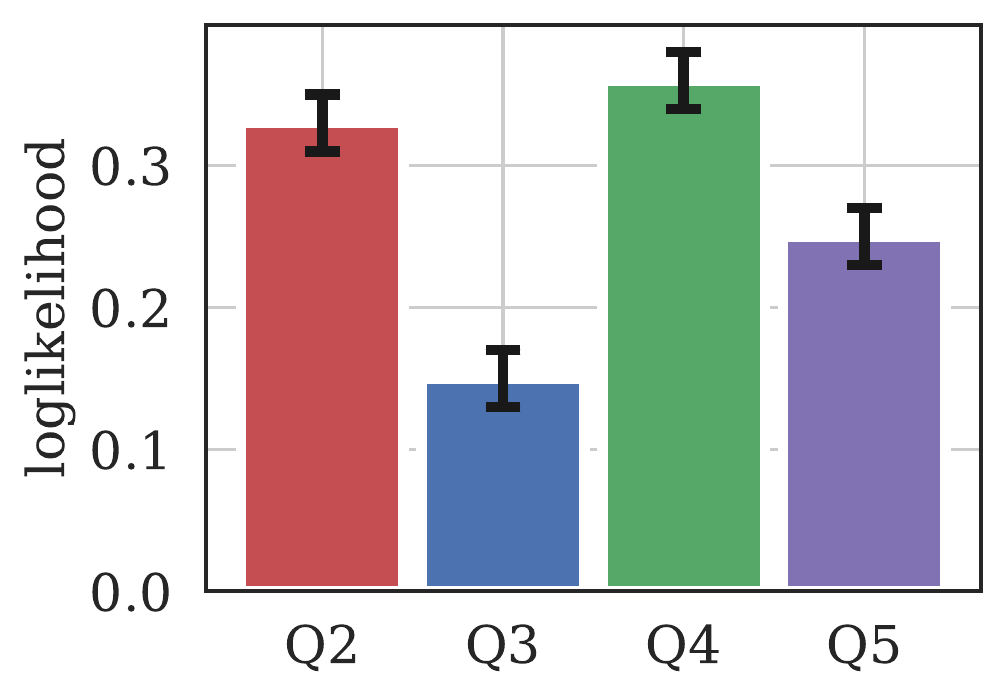}} \hspace{2mm}  
\subfloat[\label{fig:nd-multitask-b} matern-$\frac{5}{2}$]
{\includegraphics[width=0.235\linewidth,height=2.8cm]{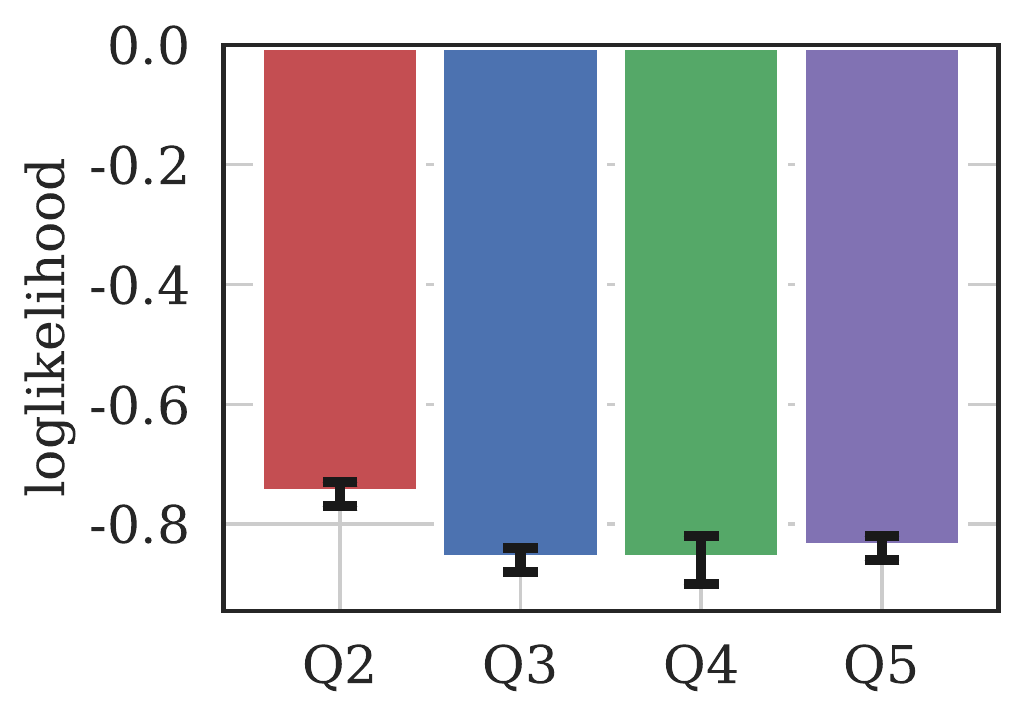}} \hspace{2mm} 
\subfloat[\label{fig:nd-multitask-c} weakly periodic]
{\includegraphics[width=0.235\linewidth,height=2.8cm]{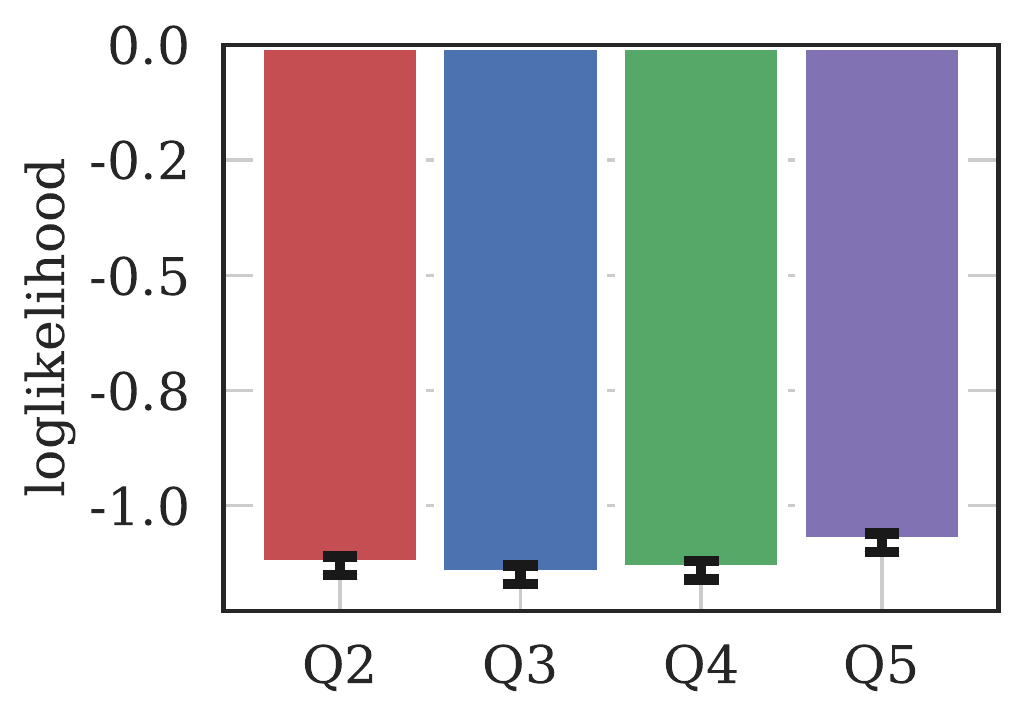}} \hspace{2mm}
\subfloat[\label{fig:nd-multitask-d} sawtooth]
{\includegraphics[width=0.235\linewidth,height=2.8cm]{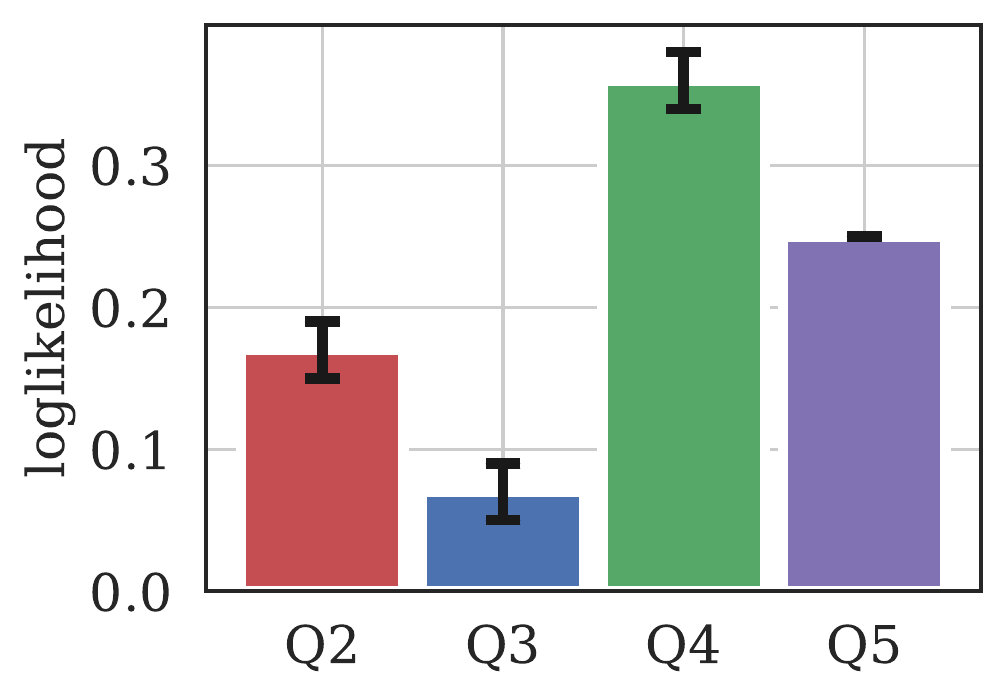}} \hspace{2mm}
\caption{Comparison over mixtures components $Q\in \{2,3,4,5\}$ for stationary basis kernel;
\\ \textr{ datav=1 :first columns=[0,5]Hz, second columns=[0,10]Hz }}
%\label{fig:nd-multitask-v1}
\end{figure*}

\begin{figure*}[htp!]
%\begin{figure*}[t]
\centering
\hspace{-2.5mm}
\subfloat[\label{fig:nd-multitask-a} rbf ]
{\includegraphics[width=0.235\linewidth,height=2.8cm]{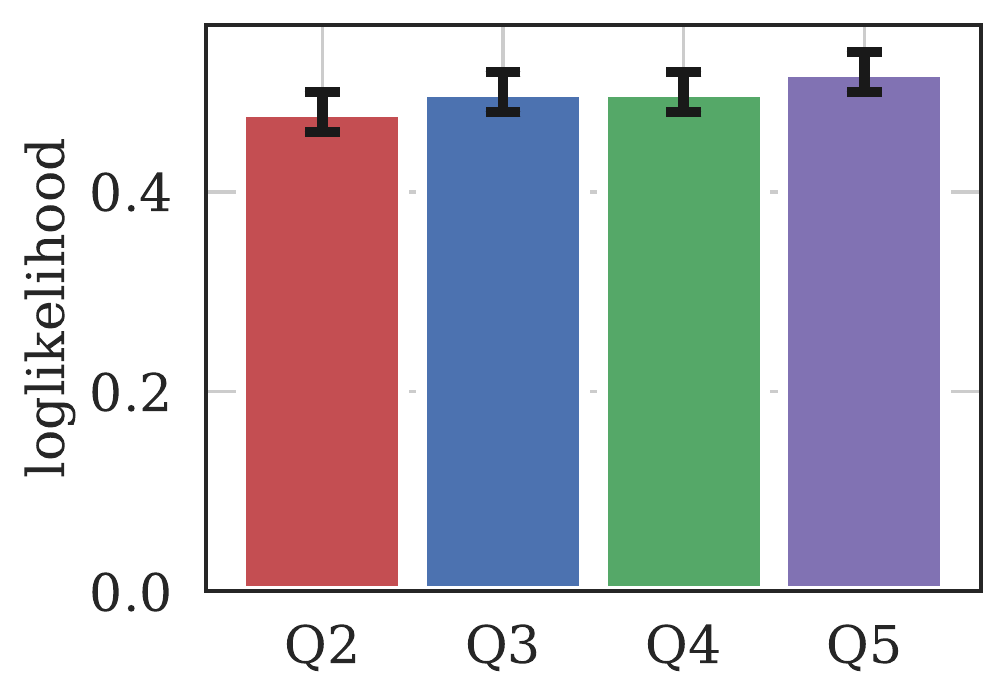}} \hspace{2mm}  
\subfloat[\label{fig:nd-multitask-b} matern-$\frac{5}{2}$]
{\includegraphics[width=0.235\linewidth,height=2.8cm]{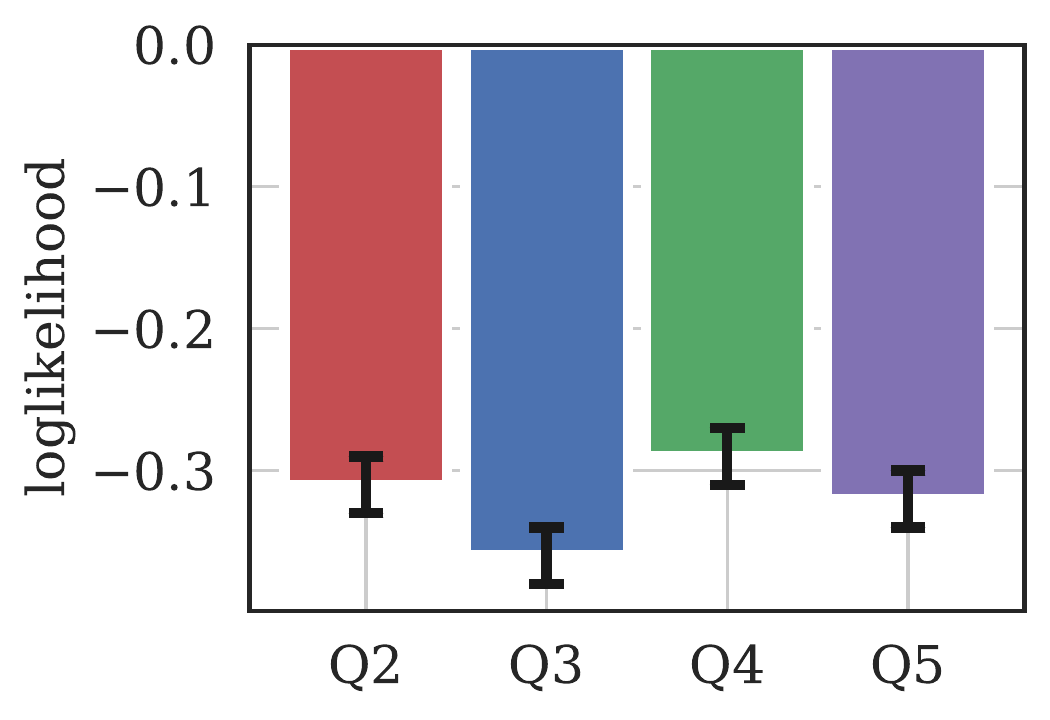}} \hspace{2mm} 
\subfloat[\label{fig:nd-multitask-c} weakly periodic]
{\includegraphics[width=0.235\linewidth,height=2.8cm]{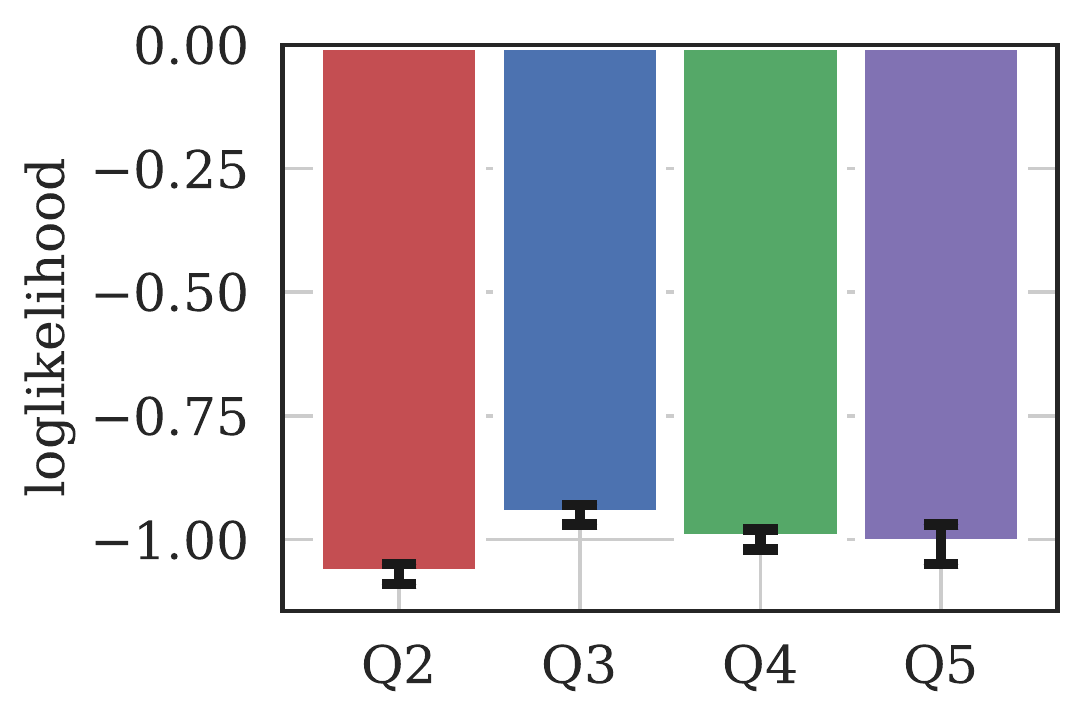}} \hspace{2mm}
\subfloat[\label{fig:nd-multitask-d} sawtooth]
{\includegraphics[width=0.235\linewidth,height=2.8cm]{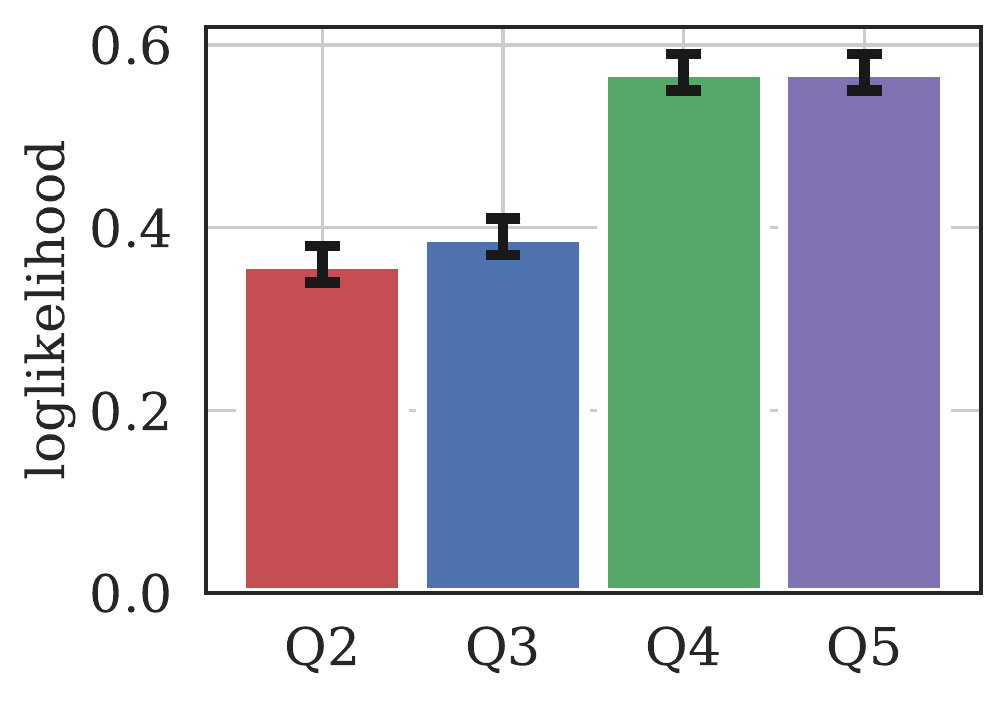}} \hspace{2mm}

\hspace{-2.5mm}
\subfloat[\label{fig:nd-multitask-a} rbf ]
{\includegraphics[width=0.235\linewidth,height=2.8cm]{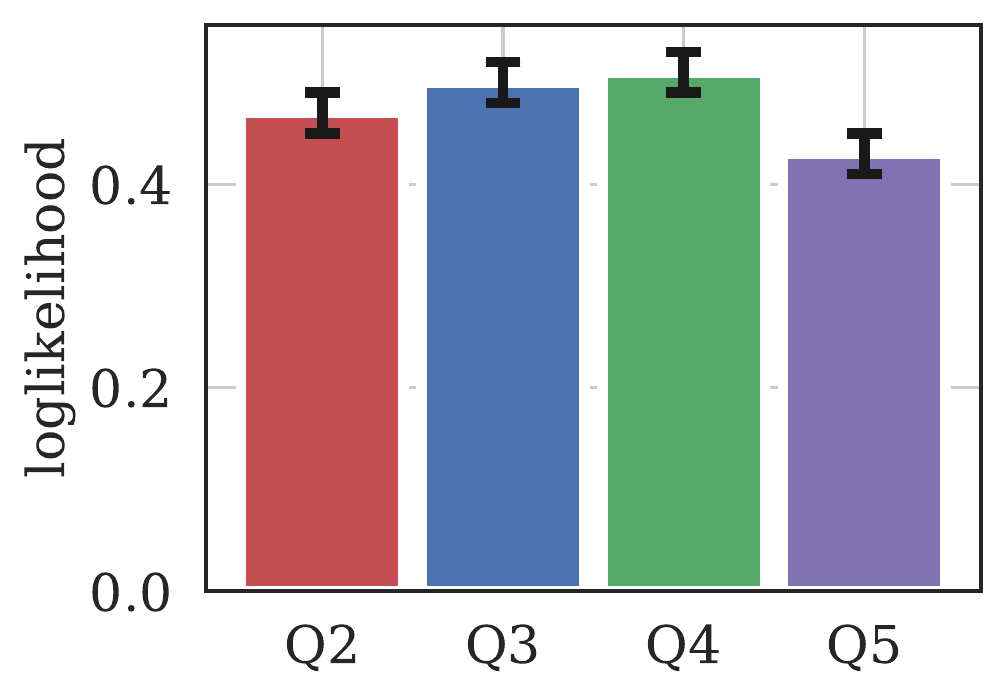}} \hspace{2mm}  
\subfloat[\label{fig:nd-multitask-b} matern-$\frac{5}{2}$]
{\includegraphics[width=0.235\linewidth,height=2.8cm]{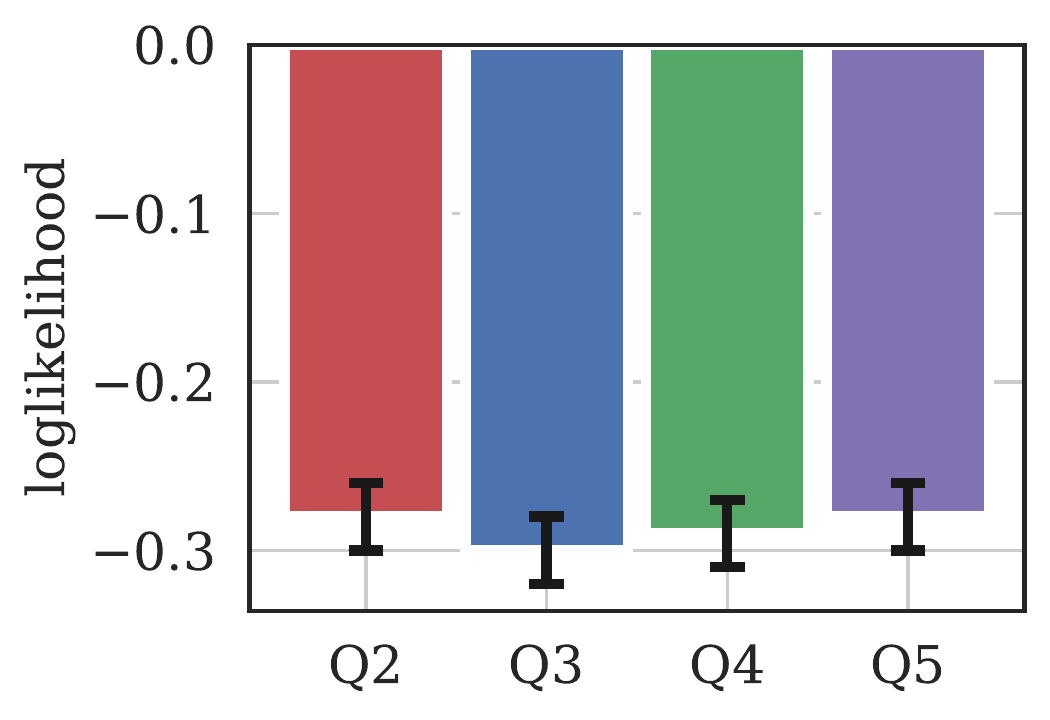}} \hspace{2mm} 
\subfloat[\label{fig:nd-multitask-c} weakly periodic]
{\includegraphics[width=0.235\linewidth,height=2.8cm]{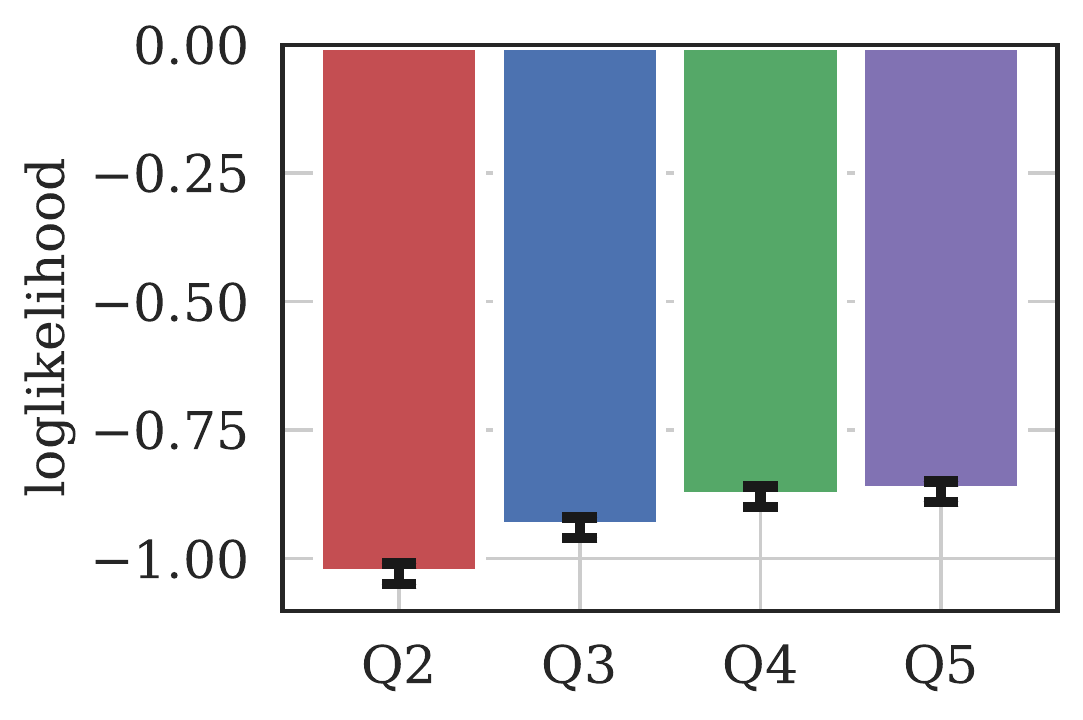}} \hspace{2mm}
\subfloat[\label{fig:nd-multitask-d} sawtooth]
{\includegraphics[width=0.235\linewidth,height=2.8cm]{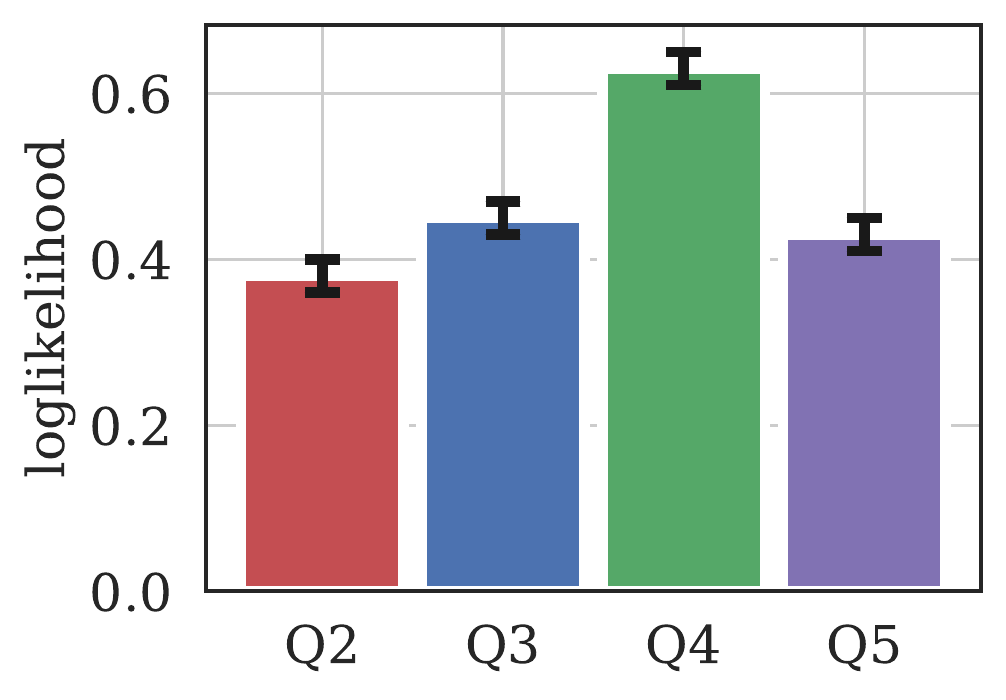}} \hspace{2mm}
\caption{Comparison over mixtures components $Q\in \{2,3,4,5\}$ for stationary basis kernel;
\\ 
\textr{ datav=2 :first columns=[0,5]Hz, second columns=[0,10]Hz }}
%\label{fig:nd-multitask-v1}
\end{figure*}
