# Supplementary material for: Bayesian Convolutional Deep Sets with Task-Dependent Stationary Prior
Source: arXiv:2210.12363 source file (2022-10-22)
Supplement: Supplementary file 2 [file 07-appendix-v01-chapter2-exp1-figure01.tex]

%\paragraph{small}

%\vfill

\begin{figure*}[htp!]
\centering
\subfloat[\label{fig:1d-a}  spectral density]
{\includegraphics[width=0.19\linewidth  ,height=2.40cm ]{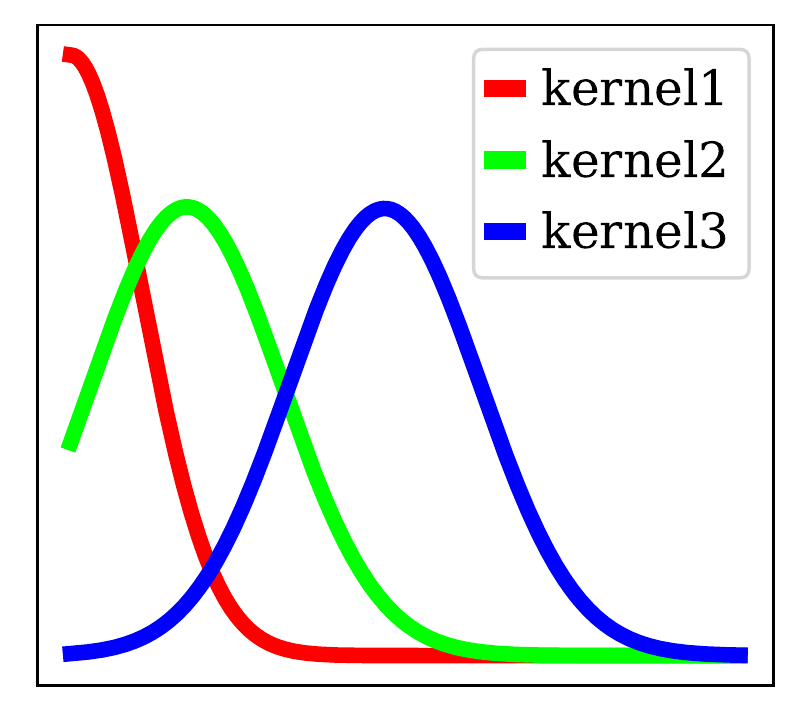}} \hspace{0.1mm}
\subfloat[\label{fig:1d-b} RBF]
{\includegraphics[width=0.19\linewidth ,height=2.40cm ]{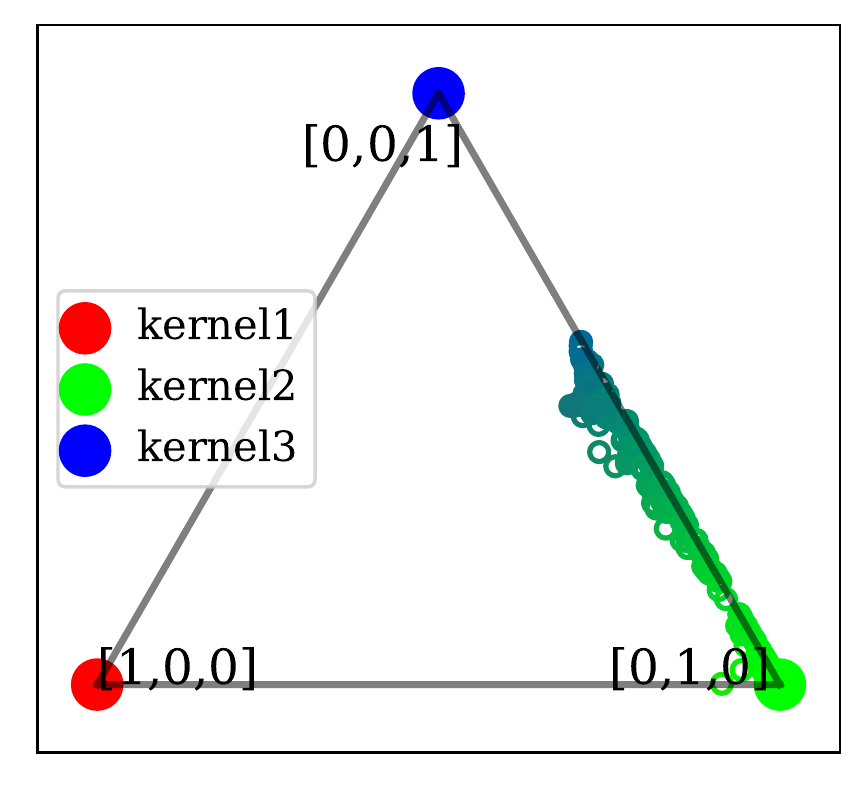}} \hspace{0.1mm}
\subfloat[\label{fig:1d-c} Matern-${\frac{5}{2}}$]
{\includegraphics[width=0.19\linewidth ,height=2.40cm ]{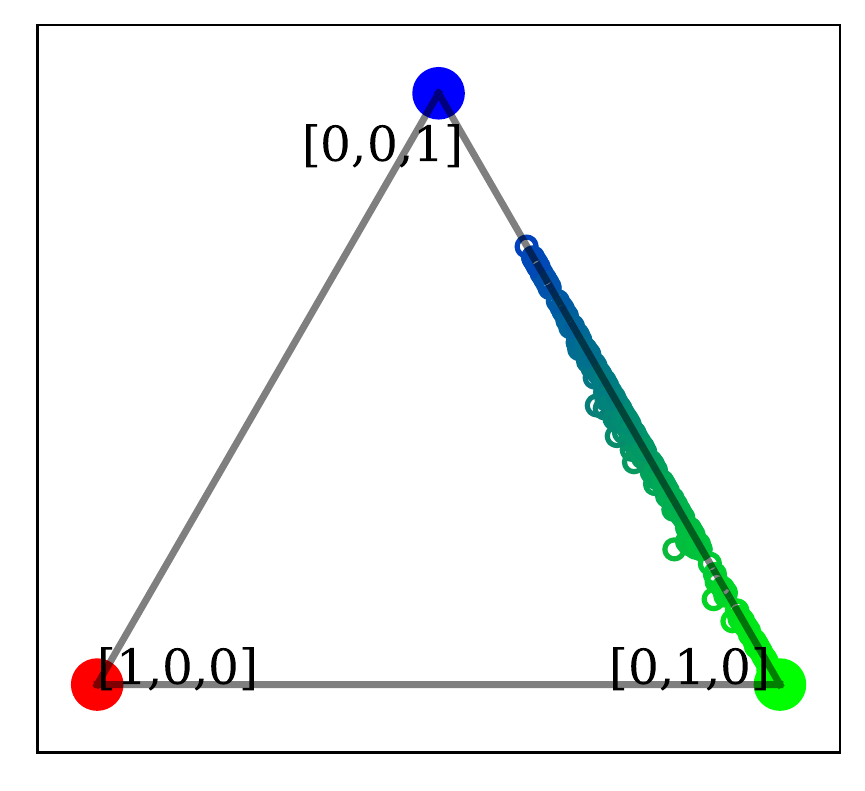}} \hspace{0.1mm}
\subfloat[\label{fig:1d-d} Weakly Periodic]
{\includegraphics[width=0.19\linewidth ,height=2.40cm ]{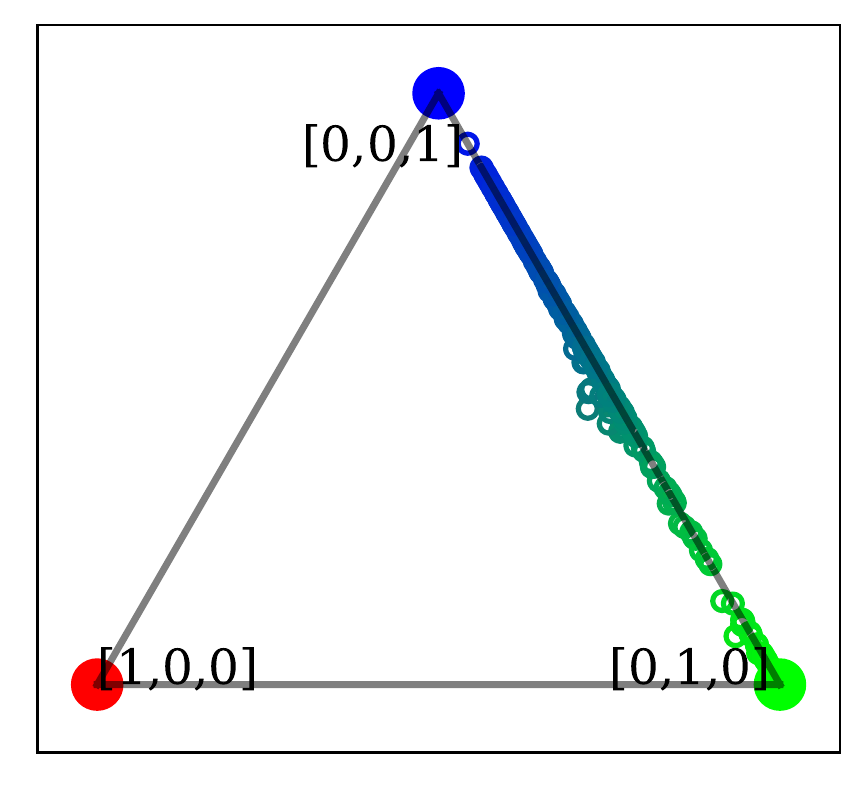}} \hspace{0.1mm}
\subfloat[\label{fig:1d-e} Sawtooth]
{\includegraphics[width=0.19\linewidth ,height=2.40cm ]{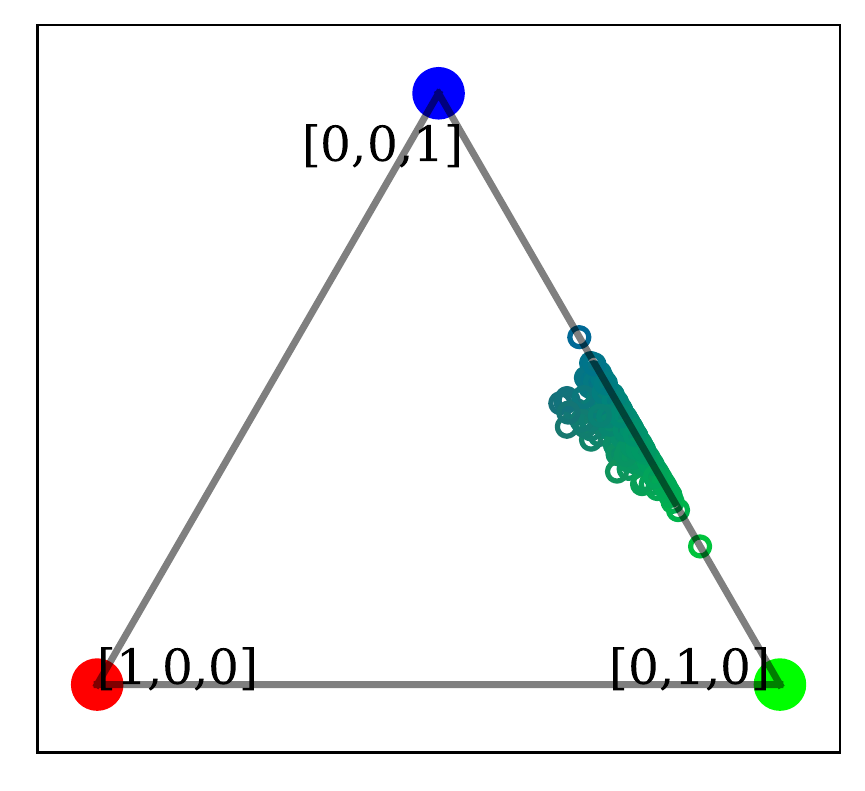}}  
%\caption{dsfasdklj}
\caption{\cref{fig:1d-a} denotes the spectral density of 3 basis kernels for proposed model; x-axis and y-axis denotes the frequency domain and the level of the density, respectively. \cref{fig:1d-b,fig:1d-c,fig:1d-d,fig:1d-e} show the outputs of $p_{\text{traninv-nn}}(X^{c},Y^{c})$ in \textb{Eq. (9)}  
$(X^{c},Y^{c}) \in \{(X^{c_n},Y^{c_n})\}_{n=1}^{256}$ for each process when the model is trained under the setting of \textb{the small number of context set ($\mathcal{U}([5,25])$)}}
\label{fig:1d-singletask_full-param-datav1}
\end{figure*}

\begin{figure*}[htp!]
\centering

\subfloat[\vspace{.0mm} \label{fig:v21} Functional representations of RBF ]
{\includegraphics[width=0.49\linewidth ,height=1.75cm ]{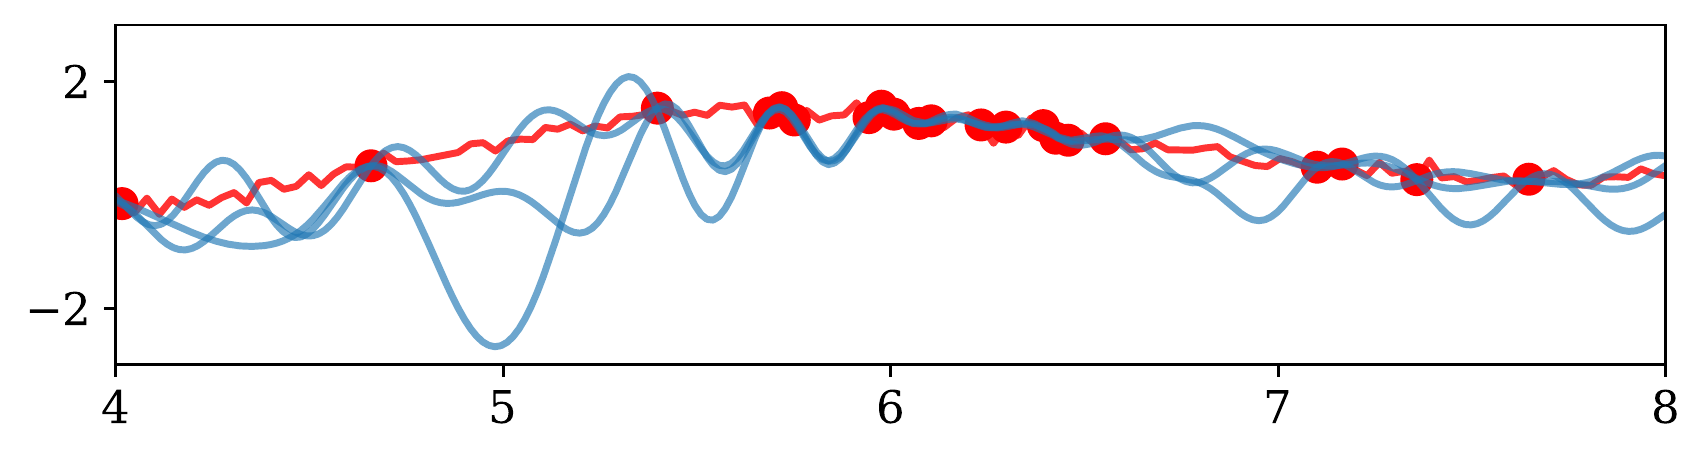}} 
\subfloat[\vspace{.0mm} \label{fig:v22} Functional representations of RBF ]
{\includegraphics[width=0.49\linewidth ,height=1.75cm ]{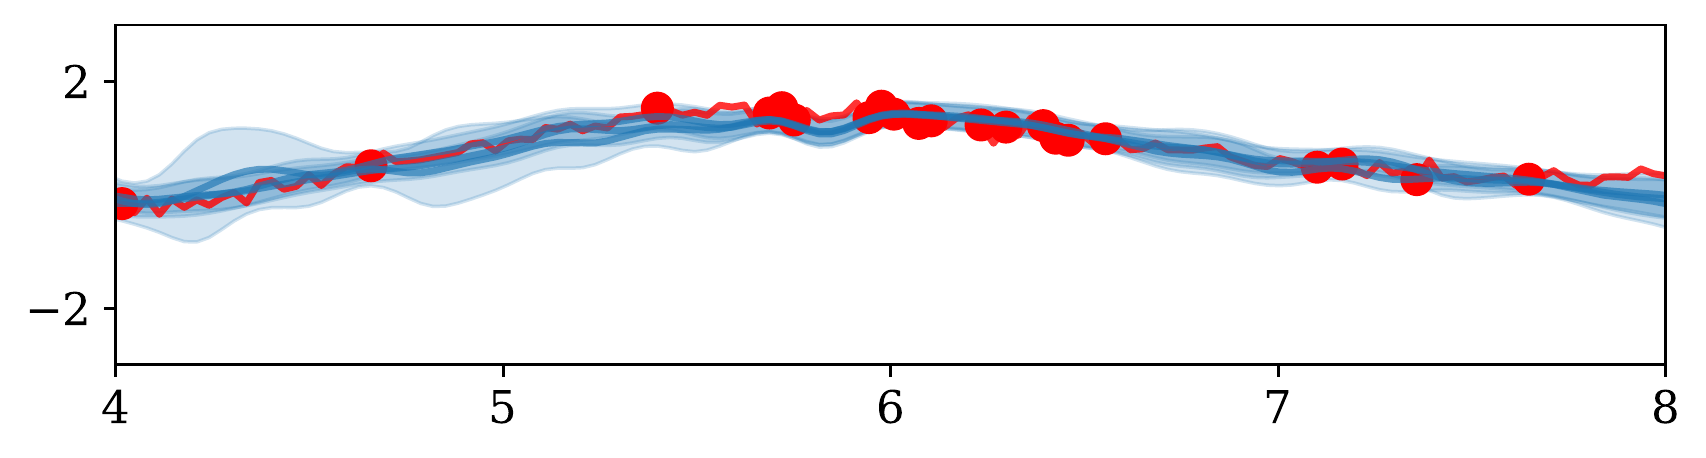}}

\subfloat[\vspace{.0mm} \label{fig:v23} Functional representations of Matern-$\frac{5}{2}$ ]
{\includegraphics[width=0.49\linewidth ,height=1.75cm ]{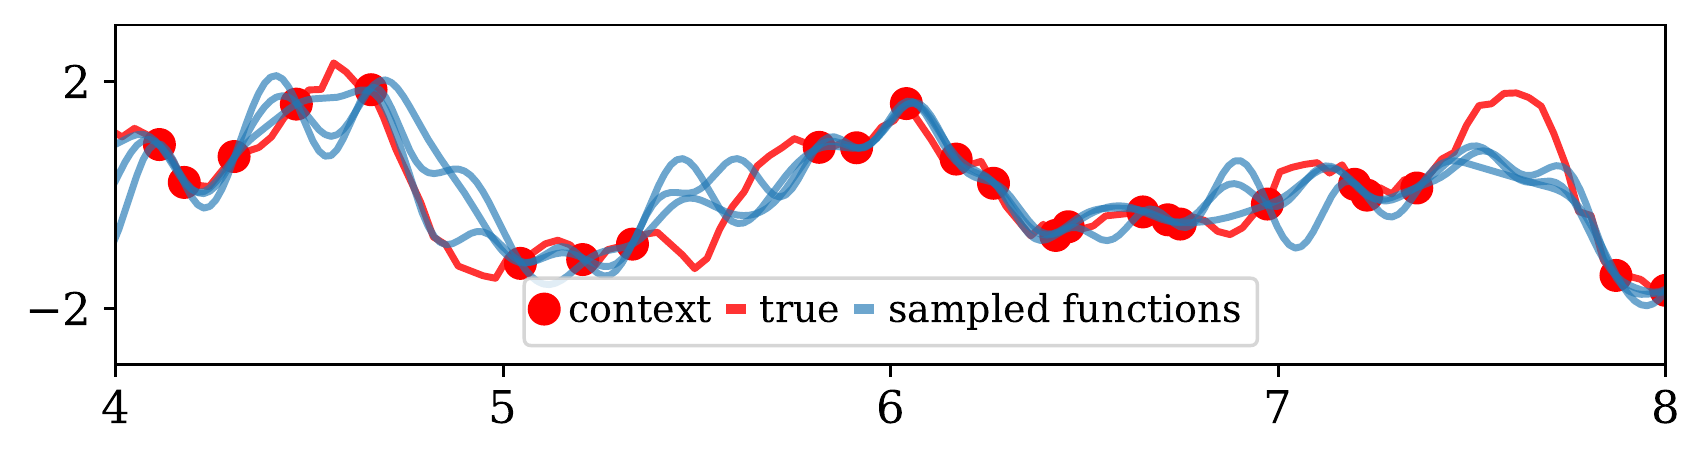}} 
\subfloat[\vspace{.0mm} \label{fig:v24} Functional representations of Matern-$\frac{5}{2}$ ]
{\includegraphics[width=0.49\linewidth ,height=1.75cm ]{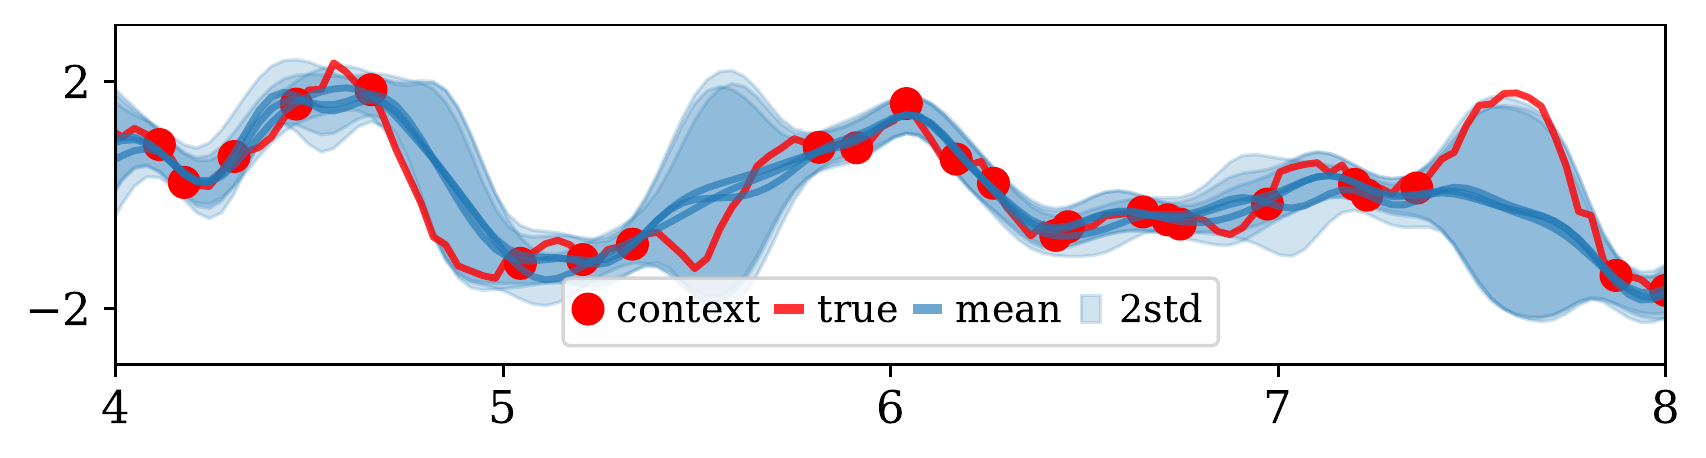}} 

\vspace{3mm}
\subfloat[\vspace{.0mm} \label{fig:v25} Functional representations of Weakly Periodic]
{\includegraphics[width=0.49\linewidth ,height=1.75cm ]{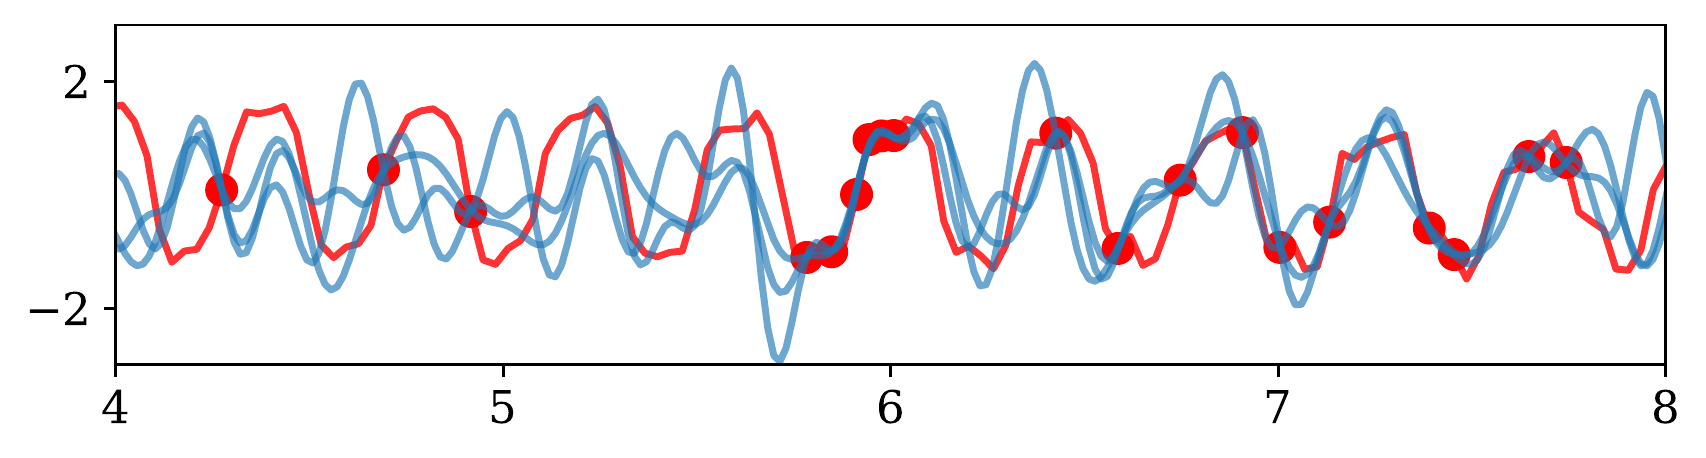}} 
\subfloat[\vspace{.0mm} \label{fig:v26} Functional representations of Weakly Periodic ]
{\includegraphics[width=0.49\linewidth ,height=1.75cm ]{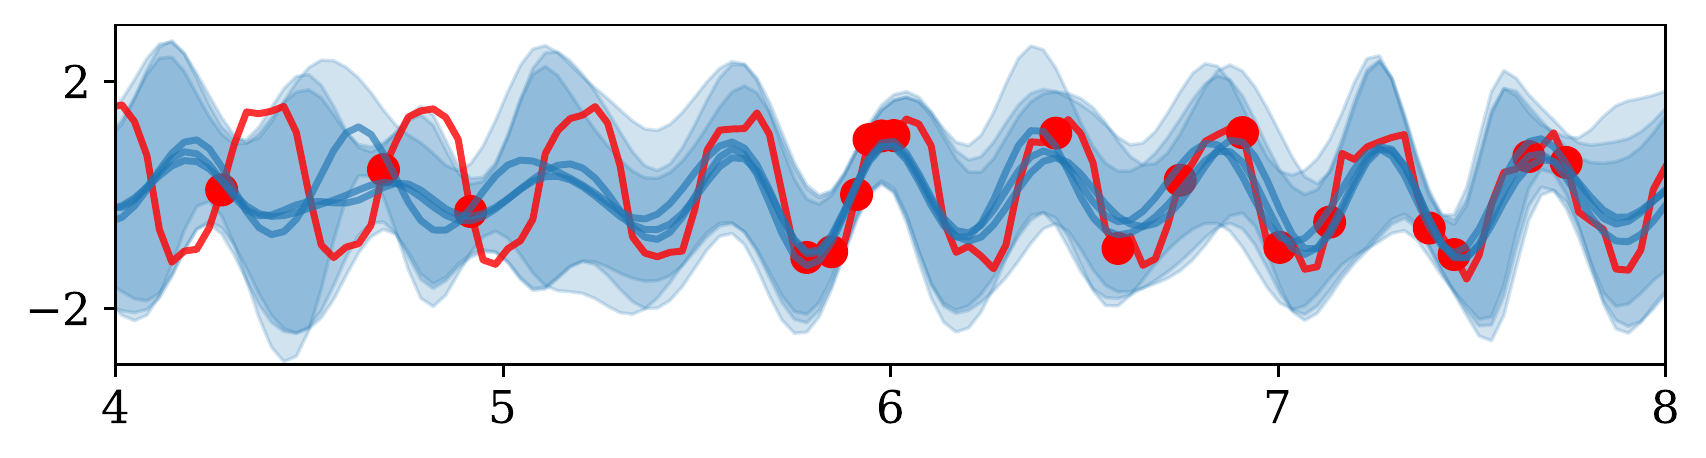}} 

\vspace{3mm}
\subfloat[\vspace{.0mm} \label{fig:v27} Functional representations of Sawtooth ]
{\includegraphics[width=0.49\linewidth ,height=1.75cm ]{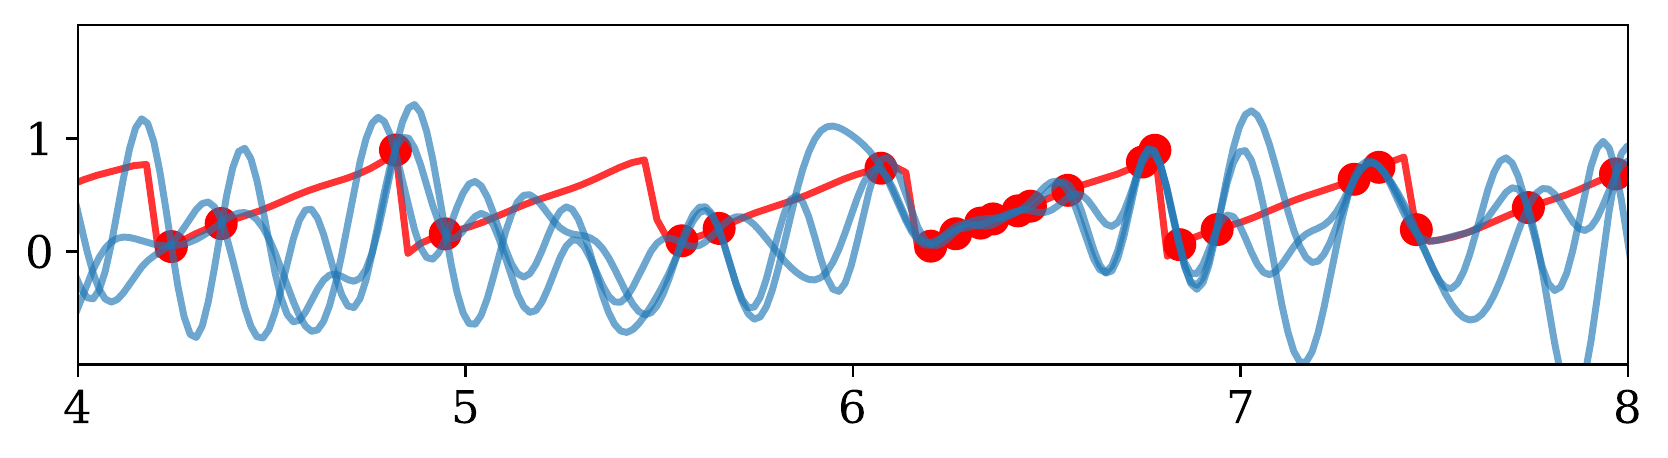}} 
\subfloat[\vspace{.0mm} \label{fig:v28} Functional representations of Sawtooth ]
{\includegraphics[width=0.49\linewidth ,height=1.75cm ]{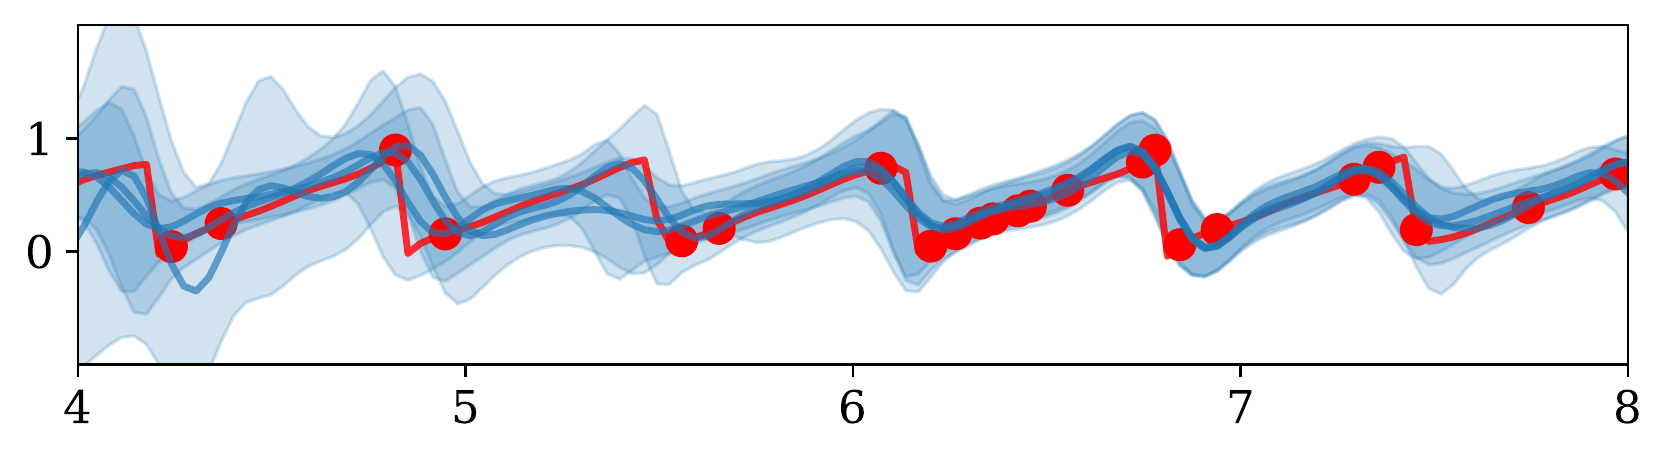}}

\caption{\cref{fig:v21,fig:v23,fig:v25,fig:v27} show 3 sampled functions of \textb{Eq. (9)} (main) for each processes by using context sets (outside training range). \cref{fig:v22,fig:v24,fig:v26,fig:v28}  show the corresponding 3 predictive distributions on target sets.}
\label{fig:1d-singletask-full-pred-datav1}
\end{figure*}
