# Supplementary material for: Bayesian Convolutional Deep Sets with Task-Dependent Stationary Prior
Source: arXiv:2210.12363 source file (2022-10-22)
Supplement: Supplementary file 4 [file 07-appendix-v01-chapter3-exp2-figure05.tex]

\clearpage

\begin{figure*}[htp!]
%\begin{figure*}[t]
\centering
\hspace{-2.5mm}
\subfloat[\label{fig:fig-a} \textb{sinusoidal}: spectral densities ]
{\includegraphics[width=0.37\linewidth,height=3.9cm]{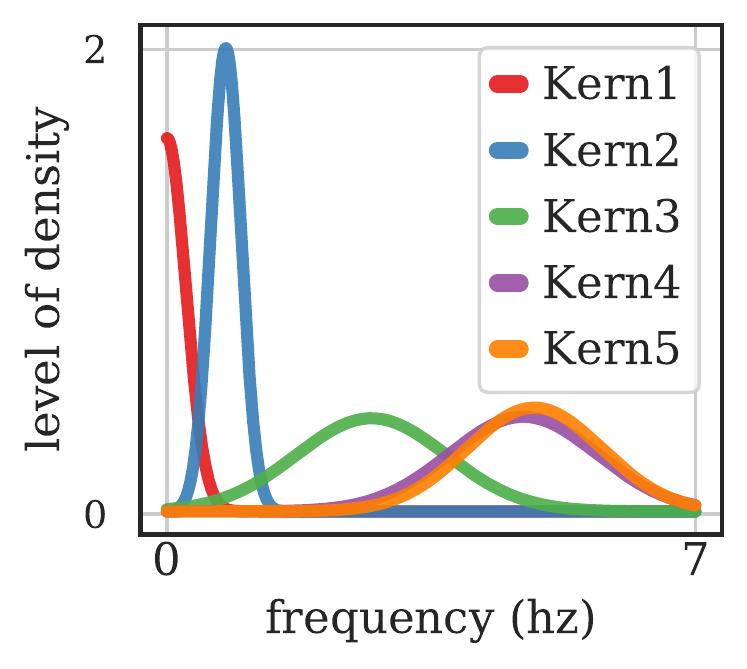}} 
\hspace{10mm}
\subfloat[\label{fig:fig-b} \textb{sinusoidal}: $p_{\text{traninv-nn}}(X_c,Y_c)$]   
{\includegraphics[width=0.39\linewidth,height=4.05cm]{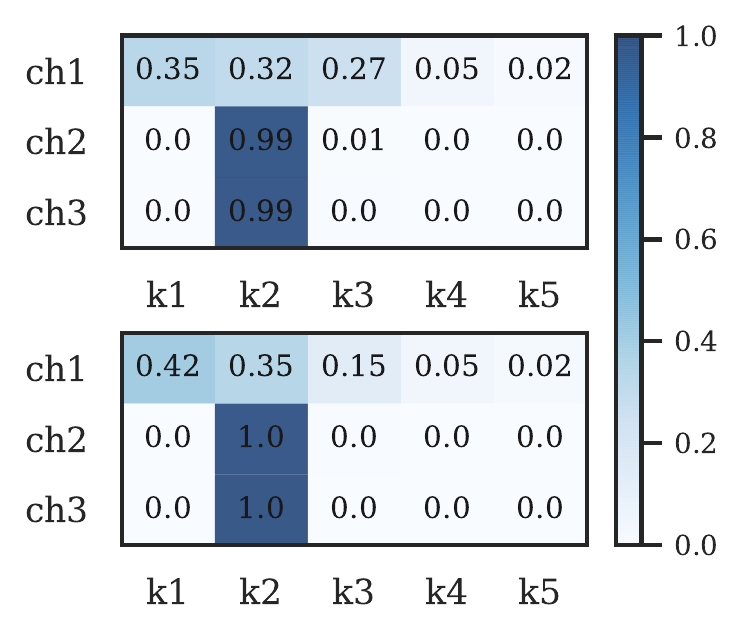}} 

\hspace{-2.5mm}
\subfloat[\label{fig:fig-c}  \textb{sinusoidal-varying}: spectral densities ]
{\includegraphics[width=0.37\linewidth,height=3.9cm]{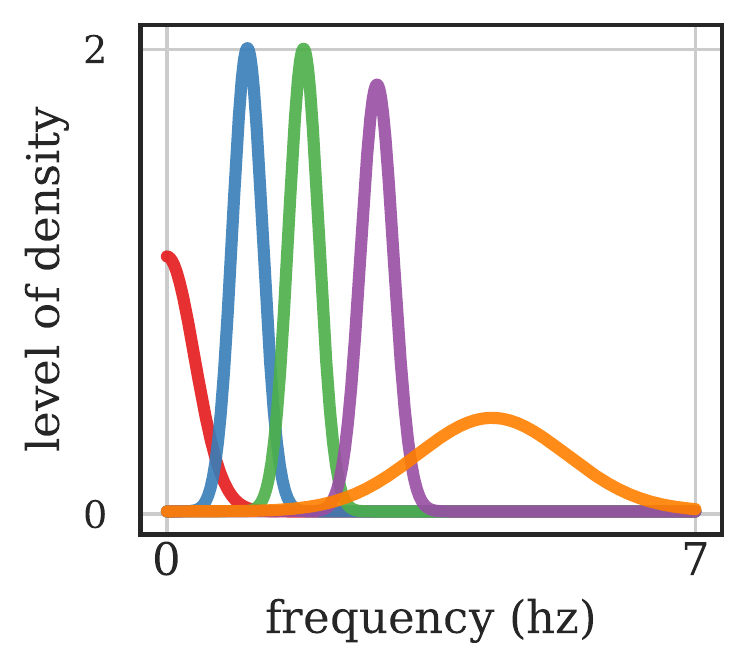}} 
\hspace{10mm}
\subfloat[\label{fig:fig-d} \textb{sinusoidal-varying}: $p_{\text{traninv-nn}}(X_c,Y_c)$ ]   
{\includegraphics[width=0.39\linewidth,height=4.05cm]{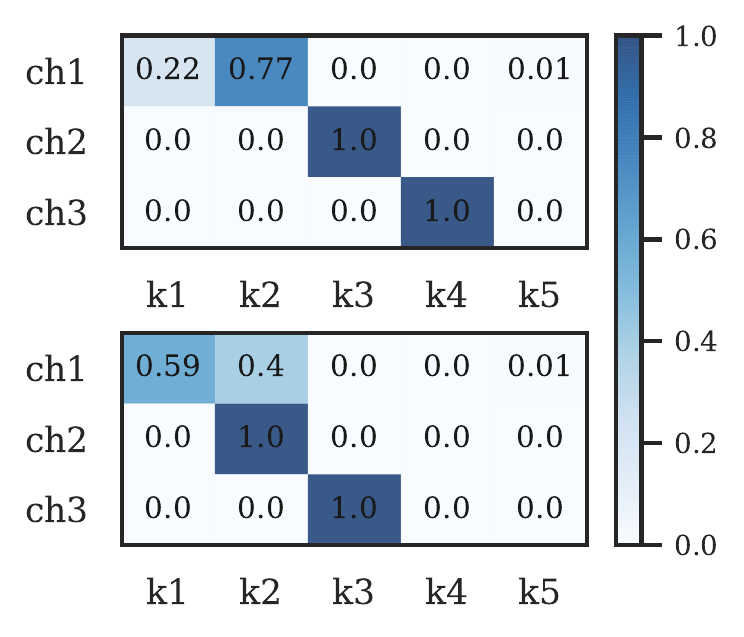}} 

\hspace{-2.5mm}
\subfloat[\label{fig:fig-e} \textb{mosm}: spectral densities ]
{\includegraphics[width=0.37\linewidth,height=3.9cm]{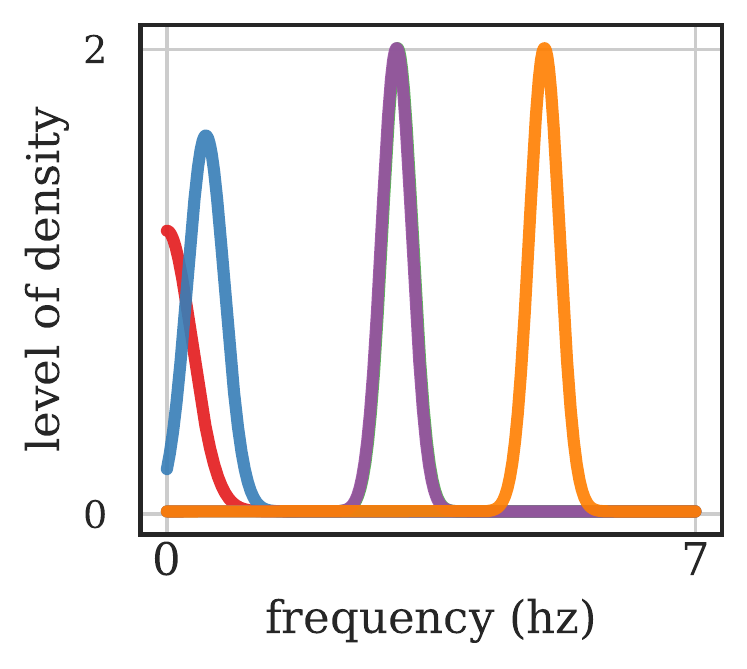}} 
\hspace{10mm}
\subfloat[\label{fig:fig-f} \textb{mosm}: $p_{\text{traninv-nn}}(X_c,Y_c)$ ]   
{\includegraphics[width=0.39\linewidth,height=4.05cm]{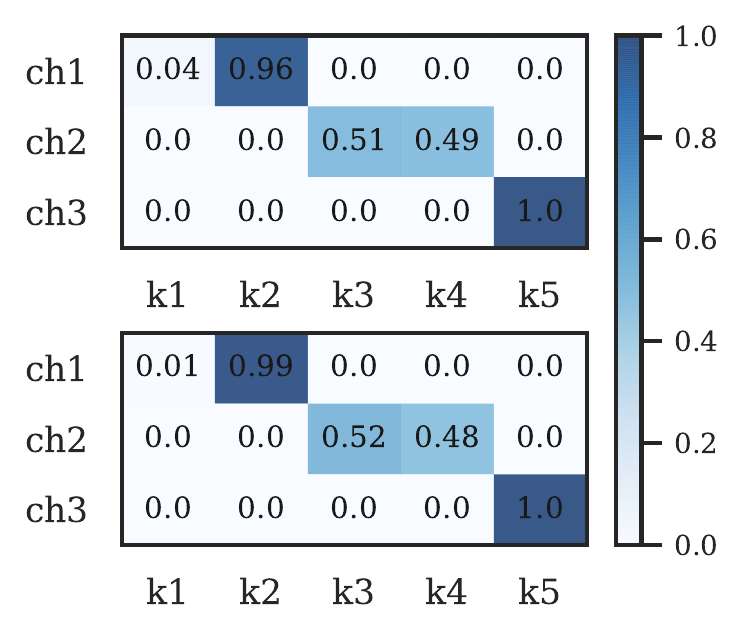}} 

\hspace{-2.5mm}
\subfloat[\label{fig:fig-g} \textb{mosm-varying}: spectral densities ]
{\includegraphics[width=0.37\linewidth,height=3.9cm]{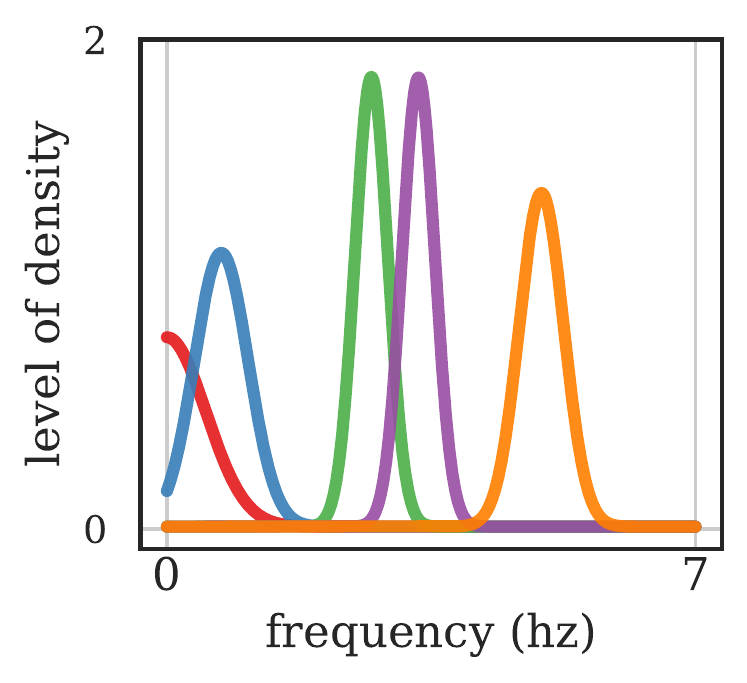}} 
\hspace{10mm}
\subfloat[\label{fig:fig-h} \textb{mosm-varying}: $p_{\text{traninv-nn}}(X_c,Y_c)$ ]   
{\includegraphics[width=0.39\linewidth,height=4.05cm]{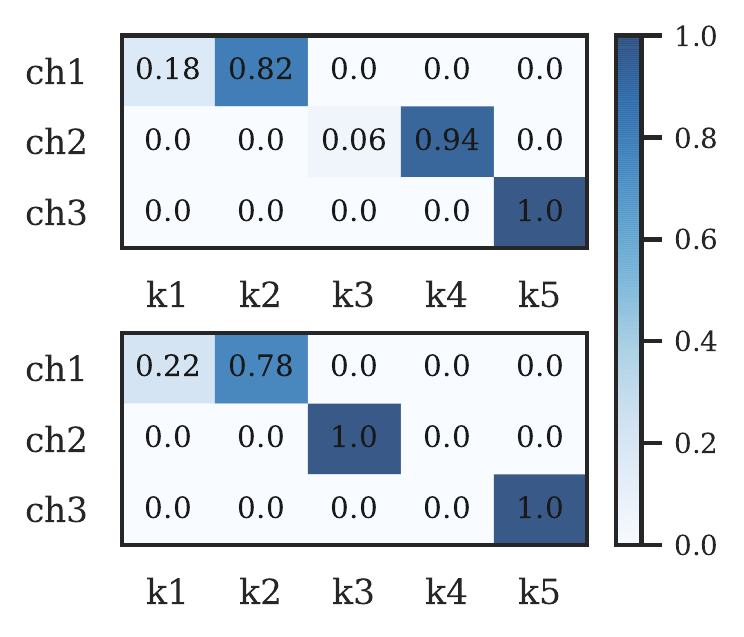}} 

%\caption{\textr{Prediction results} of multi-channel regression tasks over varying $N^{c}$ context data points.}
\caption{Qualitative analysis of task-dependent prior; \cref{fig:fig-a,fig:fig-b} show the estimated spectral densities of 5 basis stationary kernels $\{k_q\}_{q=1}^{Q}$ and parameters of categorical variable $p_{\text{traninv-nn}}(X_c,Y_c)$ obtained from \cref{fig:sin-d}, respectively. \cref{fig:fig-c,fig:fig-d} show the results corresponding to \cref{fig:sinvarying-d}. \cref{fig:fig-e,fig:fig-f} show the results corresponding to \cref{fig:mosm-d}. \cref{fig:fig-g,fig:fig-h} show the results corresponding to \cref{fig:mosmvarying-d}. These figures imply that when the model predicts the tasks having more diversity, the model use the task-dependent prior
as shown in \cref{fig:fig-d,fig:fig-h}.}

\label{fig:gpdep-weight}
\end{figure*}
