# Supplementary material for: Bayesian Convolutional Deep Sets with Task-Dependent Stationary Prior
Source: arXiv:2210.12363 source file (2022-10-22)
Supplement: Supplementary file 5 [file 07-appendix-v01.tex]

\clearpage

%\aistatstitle{Instructions for Paper Submissions to AISTATS 2023}
%\aistatstitle{Appendix}
%\aistatstitle{Bayesian Convolutional Neural Process with Task-Dependent Stationary Prior}

% \onecolumn
% \appendix

%\printbibliography[heading=none]

\clearpage
\appendix
\onecolumn

% \renewcommand\thefigure{\thesection\arabic{figure}}
% \setcounter{figure}{0}
% \renewcommand\theequation{\thesection\arabic{equation}}
% \setcounter{equation}{0}
% \renewcommand\thetable{\thesection\arabic{table}}
% \setcounter{table}{0}
% %\input{sections/appendix.tex}

% \linewidth\hsize \toptitlebar {\centering
% {\Large\bfseries \ourtitle\\ (Appendix) \par}}
%  \bottomtitlebar

% \makeatletter
% \renewcommand*\l@section{\@dottedtocline{1}{1.5em}{2.3em}}
% \makeatother

%\maketitle{D}
\aistatstitle{Appendix:\\
Bayesian Convolutional Deep Sets with Task-Dependent Stationary Prior}

\vspace{-3mm}
\setcounter{page}{1}
\counterwithin{figure}{section}
\counterwithin{equation}{section}

\addtocontents{toc}{\protect\setcounter{tocdepth}{2}}
\tableofcontents

\clearpage

%\section{Appendix}
% Optionally include extra information (complete proofs, additional experiments and plots) in the appendix.
% This section will often be part of the supplemental material.

\section{Further Details for the Proposed Methodology  }
\label{appendix:details-propose}

%\paragraph{Implementations.}
\subsection{Implementations}
\label{appendix:details-algorithm}

We explain how the proposed NP model outputs the predictive distributions on target sets in following algorithm. Our implementation is available at \url{https://anonymous.4open.science/r/multichannels-corrnp-7A1F/}. 
%----------------------------------------------------
% off-grid
%----------------------------------------------------
\begin{algorithm}[htp!]
\caption{Forward pass of the NP model via Bayesian ConvDeepsets (off-grid) }
\label{alg:BayesConvDeepsets}
    \begin{algorithmic}[1]
    %\Require $\rho = (\text{CNN}, \psi_\rho)$, $\psi$, and density $\zeta$ 
    \Require Model parameters: $\Theta$
    \Require The number of basis stationary kernels $Q$, the number of sampled spectral points $l$
    \Require Context set $D^{c}=\{(x^{c}_n, y^{c}_n)\}_{n=1}^{N^{c}}$, target inputs $X^{t}= \{x^{t}_n\}_{n=1}^{N^{t}}$ 
    \State Compute the discretized inputs $\{t_m\}_{m=1}^{M}$ by spacing inputs range $[\mathrm{min}\{X^{c},X^{t}\},\mathrm{max}\{X^{c},X^{t}\}]$ linearly.
    \State Select the task-dependent stationary prior as described in \textb{Eq. (11)}    
    \State Construct $N$ random functional representation $\{f_{(n)}(D^{c})(\bigcdot)\}_{n=1}^{N}$ on $\mathcal{I}$ as described in \textb{Eqs. (12-16)}.
    \State Construct $N$ random representations $\{\Phi^{\mathcal{B}}_{(n)}(D^{c})(\bigcdot)\}_{n=1}^{N}$ on finite grid points $\{t_m\}_{m=1}^{M}$ as described in \textb{Eq. (17)}.  
    \State Smooth $N$ random representations $\{\Phi^{\mathcal{B}}_{(n)}(D^{c})(\bigcdot)\}_{n=1}^{N}$ on target inputs $X^{t}$ by \textb{Eq. (6)}.  
    \State Generate $N$ predictive distributions $\{p \big( Y^{t} \ | \  X^{t},\Phi^{\mathcal{B}}_{(n)} \big) \}_{n=1}^{N}$ on target inputs $X^{t}$ by \textb{Eq. (20)}.
\end{algorithmic}
\end{algorithm}

%----------------------------------------------------
% on-grid
%----------------------------------------------------
\begin{algorithm}[htp!]
\caption{Forward pass of the NP model via Bayesian ConvDeepsets (on-grid) }
\label{alg:BayesConvDeepsets}
    \begin{algorithmic}[1]
    %\Require $\rho = (\text{CNN}, \psi_\rho)$, $\psi$, and density $\zeta$ 
    \Require Model parameters: $\Theta$
    \Require The number of basis stationary kernels $Q$, the number of sampled spectral points $l$
    \Require Context set $D^{c}=\{(x^{c}_n, y^{c}_n)\}_{n=1}^{N^{c}}$, target inputs $X^{t}= \{x^{t}_n\}_{n=1}^{N^{t}}$ on grid.
    \State Extract the context inputs $\sum_{n=1}^{N^{c}} \delta (\bigcdot -  x^{c}_n ) $
    and outputs  $\sum_{n=1}^{N^{c}} y^{c}_n   \delta (\bigcdot -  x^{c}_n ) $            on grid.
    \State Construct $N$ random functional representation $\{f_{(n)}(D^{c})(\bigcdot)\}_{n=1}^{N}$ on given grid as described in \textb{Eq. (12)}.
    \State Map $N$ random representations on grid where the $n$-th representation $f^M_{(n)}$ is computed as $$f^M_{(n)} = \mathrm{CNN}\left(\left[\sum_{n=1}^{N^{c}} \delta (\bigcdot -  x^{c}_n ) \ , \ \Phi^{\mathcal{B}}_{(n)}(D^{c})(\bigcdot) \right]\right).$$ \vspace{-1mm}  
    \State  Generate $N$ predictive distributions for target set with the $n$-th predictive mean $\mu^{t}_{(n)}$ and standard deviation $\sigma^{t}_{(n)}$,  \vspace{-1mm} $$\mu^{t}_{(n)}  \ , \ \sigma^{t}_{(n)} = f^M_{(n)} \circ  \left(\sum_{n=1}^{N^{t}} \delta (\bigcdot -  x^{t}_n ) \right).   $$ \vspace{-1mm}
\end{algorithmic}
\end{algorithm}

\clearpage
\subsection{Details for Proposed Methodology}
\subsubsection{Structure of Translation Invariant NN in \textb{Eq. (10) (main)}.}
\label{subsubsec:transinvnn}

% To maintain the translation equivariance for the induced functional representation of task-dependent stationary prior, we use the translation invariant neural network $p_{\mathrm{traninv-nn}}: (R^{N_c} {\times} d) \times (R^{N_c} {\times} d') \mapsto R^{Q}_{+}$, that satisfies $p_{\mathrm{traninv-nn}}(X^{c} {+} \tau,Y^{c}) = p_{\mathrm{traninv-nn}}(X^{c},Y^{c}) $ for modeling the parameter of categorical variables $Z=(z_1,..,z_Q)$. To this end, we construct $Q$ data representations of Convolutional Deep set by using $Q$ stationary kernels $\{k_q\}_{q=1}^{Q}$, and its $q$-th representation is defined as

% We construct the functional feature $ \textbf{h}_{\text{traninv}}(x^{c},y^{c})$ by evaluating $\{h_q(\bigcdot)\}_{q=1}^{Q}$ on $X^{c}$, and then concatenating it with the output $y^{c}$ as
In this work, we consider the following structure for the translation invariant network $\mathrm{p}_{\mathrm{nn}}(D^{c})$.
\vspace{-2mm}
\paragraph{Version 1 (without grid).}
With the $q$-th stationary kernel $k_q$, we construct the $q$-th representation $h_q(\bigcdot)=\sum_{n=1}^{N} y^{c}_n \ k_q(\bigcdot - x^{c}_n)$ for given context set  context set $D^c=\{(x^{c}_{n},y^{c}_{n})\}_{n=1}^{N^{c}}$, and map the concatenated representations via MLPs as follows:
\begin{align}
\mathrm{p}_{\mathrm{nn}}(D^{c}) \coloneqq 
\Phi_{\mathrm{MLP\text{-}2}}\bigg( \sum_{(x^{c},y^{c}) \in D^c} \Phi_{\mathrm{MLP\text{-}1}}\left(\Big[ h_1(x^{c}), \ h_2(x^{c}),.., \ h_Q(x^{c}), \ y^{c} \Big]\right)
\bigg).
\end{align}
This structure employs the structure of the kernel smoother and the Deepsets. Since $h_q(\bigcdot)$ function is invariant to the translation dataset $T_{\tau}(D^{c})$, this structure satisfies $\mathrm{p}_{nn}(T_{\tau}(D^{c})) = \mathrm{p}_{nn}(D^{c}) $ with $T_{\tau}(D^{c}) =\{(x^{c}_{n}+\tau,y^{c}_{n})\}_{n=1}^{N^{c}} $.

\paragraph{Version 2 (with grid).}
With the RBF kernel function $k_{\mathrm{RBF}}$, we use the data representation of ConvDeepsets on grid $\{t_m\}_{m=1}^{M}$, and map this representation to the parameters of the categorical distribution as follows:
\begin{align}
\mathrm{p}_{\mathrm{nn}}(D^{c}) \coloneqq 
\Phi_{\mathrm{MLP}}
\bigg( \sum_{  \hspace{1mm} \bigcdot \ \in \{t_m\}_{m=1}^{M}}
\mathrm{CNN}_{\mathrm{1D}}
    \left(
          \sum_{n=1}^{N}  \frac{y_n \ k_{\mathrm{RBF}}(\bigcdot - x_n)}{ \sum_{n=1}^{N}  k_{\mathrm{RBF}}(\bigcdot -  x_n)}  
    \right)
\bigg)
\end{align}
where $ \mathrm{CNN}_{\mathrm{1D}}$ denotes a stack of convolutional layer with ReLU activation. This structure employs the structure of the RBF kernel smoother used in ConvDeepsets and the Deepsets that ensures the set invariance. Since adding or averaging the representation of RBF smoother over the finite grid is invariant to the translation dataset $T_{\tau}(D^{c})$, this structure satisfies $\mathrm{p}_{\mathrm{nn}}(T_{\tau}(D^{c})) = \mathrm{p}_{\mathrm{nn}}(D^{c}) $ with $T_{\tau}(D^{c}) =\{(x^{c}_{n}+\tau,y^{c}_{n})\}_{n=1}^{N^{c}} $. 

Here, we use the representation of RBF smoother to obtain the parameter $\mathrm{p}_{\mathrm{nn}}(D^{c})$ of a latent Categorical distribution $\mathrm{Cat}(Z_{\mathrm{Cat}}|\mathrm{p}_{\mathrm{nn}}(D^{c}) )$ so that $\mathrm{p}_{\mathrm{nn}}(D^{c})$ assigns a task-dependent stationary prior. This approach is different to the use of ConvDeepsets in \citeb{gordon2019convolutional} that represents the data.

\paragraph{Version 3.} We extend \textbf{version 2} to obtain the parameter of Categorical distribution
for the image dataset $D^c$ as follows:
\begin{align}
\mathrm{p}_{\mathrm{nn}}(D^{c}) \coloneqq 
\Phi_{\mathrm{MLP}}
\bigg(
\mathrm{Pooling}
\bigg( \mathrm{CNN}_{\mathrm{2D}}
    \left(
          \sum_{n=1}^{N} y_n \ \delta(\bigcdot - x_n)   
    \right)
\bigg)
\bigg)
\end{align}
where $ \mathrm{CNN}_{\mathrm{2D}}$ denotes a stack of residual block.

\subsubsection{Structure of CNN $\rho$ in \textb{Eq. (17) (main)}.}
\label{subsubsec:cnnstructure}

\paragraph{Shallow and Deep CNN (1d).} For regression tasks with time-series dataset, we employ 5-layer CNN using ReLU activation function as a shallow network. All layers uses 16 channels except for the first layer (8 inchannels) and last layer (8 outchannels). We use kernels of size 5, stride 1, and zero.

For the structure of Deep CNN, we employ the 1D-Unet \citeb{ronneberger2015u}, which is used in \citeb{gordon2019convolutional}. 1D-Unet consists of 12-layer architecture with skip connections where the number of channels is doubled every layer for the first six layers, and halved every layer for the last six layers. The following describes which layers are concatenated, where $L_i \leftarrow \left[L_j, L_k \right]$ means that the input to layer $i$ is the concatenation of the activations of layers $j$ and $k$:
\begin{itemize}[leftmargin=5em]
    \vspace{-2mm}
    \item $L_8 \leftarrow \left[L_5, L_7 \right]$,
     \hspace{3mm} $L_9 \leftarrow \left[L_4, L_8 \right]$,
     \hspace{3mm} $L_{10} \leftarrow \left[L_3, L_9 \right]$,
     \hspace{3mm} $L_{11} \leftarrow \left[L_2, L_{10} \right]$,
     \hspace{3mm} $L_{12} \leftarrow \left[L_1, L_{11} \right]$.
\end{itemize}
We use ReLU activation function, kernels of size 5, stride 1, and zero padding for two units on all layers.

\paragraph{Shallow and Deep CNN (2d).} 
For image completion tasks, we use 3-layer of residual block as a shallow network and 6-layer of residual block as a deep network where each block uses 128 channel, and kernels of size 5, stride 1, and zero.

Further details of DNN structure used in this work can be checked in our implementations in \cref{appendix:details-algorithm}.

\clearpage

\clearpage
\subsection{Proofs}

% \clearpage
%\subsubsection{Random Functional representation in \textb{Eq. (12) (main)} } 
%\clearpage
\subsubsection{Proof of Proposition 2}

% Bayesian ConvDeepsets still holds the translation equivariance (TE) in the following proposition.
%\begin{proposition*} 
\begin{custom_pro}{2} 
\label{pro:te_probsense}
%\label{appendix_pro:Bayes_convdeepset}
Given dataset $D=\{(x_n,y_n)\}_{n=1}^{N}$, if the Bayesian ConvDeepsets $\Phi^{\mathcal{B}} (D) (\bigcdot)$ is defined on the finite grid points, $\Phi^{\mathcal{B}} (D) (\bigcdot)$ is still translation equivariant in distribution sense, i.e.,
\begin{align}
\Phi^{\mathcal{B}}  \circ (T_{\tau}(D)) \stackrel{d}{=}  T^{*}_{\tau} \circ (\Phi^{\mathcal{B}}(D)).
\label{eqn:te_probsense}
\vspace{-3mm}
\end{align}

\begin{proof}
 Let us first consider the left side of equation in \cref{eqn:te_probsense}. Then, for given dataset $D=\{(x_n,y_n)\}_{n=1}^{N}$, its $\tau$-translated dataset $T_{\tau}(D)=\{(x_n+\tau,y_n)\}_{n=1}^{N}$, and finite grid $\{t_m\}_{m=1}^{M}$, we can compute $\Phi^{\mathcal{B}}( T_{\tau}(D)  )(\bigcdot) $ as follows:
\begin{align}
\Phi^{\mathcal{B}}( T_{\tau}(D) )(\bigcdot)  = 
 \rho \circ
 \Big[  
 \underbrace{\sum_{n=1}^{N}  k_{\mathrm{RBF}}(\bigcdot -  (x_n  +\tau ) )}_{\mathrm{density}}  \hspace{2mm}  , \hspace{2mm} 
  \underbrace{\sum_{q=1}^{Q} \textb{ \sqrt{z_q^{\tau}} } \ \textb{ \phi_q^{\tau}(\bigcdot)} +
\sum_{n=1}^{N} \textb{v^{\tau}_{n}}  \ \textb{k(\bigcdot - x_{n} + \tau} )
}_{\mathrm{data \ representation}}
\Big].
\end{align}
where $z_q^{\tau}$, $\phi_q^{\tau}(\bigcdot)$, and $v^{\tau}_{n}$ denote the variation of $z_q$, $\phi_q(\bigcdot)$, and $v_{n}$ due to $\tau$-translated dataset $ T_{\tau}(D)$. The kernel function $k(\bigcdot - x_{n} + \tau)$ denotes the expectation of the latent kernel $\mathrm{E}_{q(Z_{\text{cat}} | D) }[k(\bigcdot - x_{n} ) \ | \ Z_{\text{cat}}]$ over $q(Z_{\text{cat}} | D)=\mathrm{Cat} \left( Z_{\text{cat}} \ ; \ \mathrm{p}_{\mathrm{nn}}(D) \right)$ with the translated invariant network $\mathrm{p}_{\mathrm{nn}}(D)$ that maps the set of dataset $D=\{(x_n,y_n)\}_{n=1}^{N}$ to the parameter of Categorical distribution. Since it has already been proven in \citeb{gordon2019convolutional} that mapping of density channel by CNN holds the TE property, we thus focus on validating that mapping of data representation by CNN holds the TE as well.
\vspace{-2mm}
\paragraph{Prior term.} For each term of data representation, we can check the following qualities:
\vspace{-2mm}
\begin{align}
(z_1^{\tau},..,z_Q^{\tau}) \ \stackrel{d}{=} \ (z_1,..,z_Q) 
\label{eqn:hold_latent}
\end{align}
where $(z_1^{\tau},..,z_Q^{\tau})\sim \mathrm{Cat}(Z;\mathrm{p}_{\mathrm{nn}}(T_{\tau}(D)))$, and  $(z_1,..,z_Q)\sim \mathrm{Cat}(Z;\mathrm{p}_{\mathrm{nn}}(D)$. The equality holds because the output of translated invariant network, i.e., the parameter of categorical distribution satisfies $\mathrm{p}_{\mathrm{nn}}(T_{\tau}(D))=\mathrm{p}_{\mathrm{nn}}(D)$. 

For the stationary prior term, each $q$-th random stationary function $\textb{ \phi_q^{\tau}(\bigcdot)}$ denotes a sample function of $GP(f;0,k_q)$ obtained by random Fourier Feature; the $q$-th kernel $k_q(\tau)$ is set to be  $k_q(\tau)=\int e^{i 2\pi   s^{T} \tau}p_q(s) ds $. Since each stationary function is not dependent on the translated dataset $T_{\tau}(D)$, thus it is trivial that $\textb{ \phi_q^{\tau}(\bigcdot)}=\textb{ \phi_q(\bigcdot)}$ for $q=1,..,Q$.

These results imply that task-dependent prior function $\sum_{q=1}^{Q} \textb{ \sqrt{z_q^{\tau}}} \textb{ \phi_q^{\tau}(\bigcdot)} $ is set consistently up to $T_{\tau}(D)=\{(x_n+\tau,y_n)\}_{n=1}^{N}$.

\vspace{-2mm}
\paragraph{Update term of data.} 
For the data update term, the expected kernel holds as follow:
\vspace{-1mm}
\begin{align}
\mathrm{E}_{q(Z_{\text{cat}}| T_{\tau}(D) ) }[ \ k( \bigcdot ) \ | \ Z_{\text{cat}} \ ]
&=
\mathrm{E}_{q(Z_{\text{cat}}| T_{\tau}(D) ) }[ z_1 k_1(\bigcdot )  \hspace{2mm} +  \hspace{2mm} \cdots  \hspace{2mm}  + \hspace{2mm} z_Q k_Q(\bigcdot ) ]  \nonumber \\
&= \mathrm{p}_{\mathrm{nn}}( T_{\tau}(D) )_{(1)} k_1(\bigcdot ) 
\hspace{2mm} +  \hspace{2mm} \cdots  \hspace{2mm}  + \mathrm{p}_{\mathrm{nn}}( T_{\tau}(D) )_{(Q)} k_Q(\bigcdot )   \\
&= \mathrm{p}_{\mathrm{nn}}( D )_{(1)} k_1(\bigcdot ) 
\hspace{2mm} +  \hspace{2mm} \cdots  \hspace{2mm}  + \mathrm{p}_{\mathrm{nn}}( D )_{(Q)} k_Q(\bigcdot )  \\
&= \mathrm{E}_{q(Z_{\text{cat}}| D ) }[ \ k(\bigcdot  ) \ | \ Z_{\text{cat}} \ ] \label{eqn:hold_latentkernel}, 
\end{align}
where the third equality holds due to the property of the translated invariant network  $\mathrm{p}_{\mathrm{nn}}(T_{\tau}(D))=\mathrm{p}_{\mathrm{nn}}(D)$. 

Also, we can confirm that the smoothing weight $v^{\tau}_n$ holds as follows:
\begin{align}
v^{\tau}_n \coloneqq [ \ K(X_{\tau},X_{\tau}) {+} \sigma^{2}_{\epsilon}I  ) {}^{-1}
          \left(Y^{c} - \Psi(X_{\tau}) \right) \ ]_{n}  = 
[ \ K(X,X) {+} \sigma^{2}_{\epsilon}I  ) {}^{-1}
          \left(Y^{c} - \Psi(X) \right) \ ]_n = v_n
          \label{eqn:hold_weight}, 
\end{align}
where $X_{\tau}=\{x_n+\tau \}_{n=1}^{N}$ and $X=\{x_n \}_{n=1}^{N}$. The first equality holds because the expected kernel $k(\bigcdot)$ is set to be consistent up the translated inputs as described in \cref{eqn:hold_latentkernel}, the expected kernel is stationary kernel, and the random stationary function $\Psi(X_{\tau})$ is set to be consistent up the translated inputs as described in \textbf{Prior term}.

Using the above results, we show that if $\Phi^{\mathcal{B}}  \circ (T_{\tau}(D))$ and $  T^{*}_{\tau} \circ (\Phi^{\mathcal{B}}(D))$ are evaluated on finite grid points $\{t_{m}\}_{m=1}^{M}$ respectively, then $\Phi^{\mathcal{B}}  \circ (T_{\tau}(D)) \stackrel{d}{=}  T^{*}_{\tau} \circ (\Phi^{\mathcal{B}}(D))$ holds as follows:
\begin{align}
\Phi^{\mathcal{B}}( T_{\tau}(D) )(\bigcdot)  &= 
 \rho \circ
 \Big[  
 \sum_{n=1}^{N}  k_{\mathrm{RBF}}(\bigcdot -  (x_n  +\tau ) ) \ , \  
\sum_{q=1}^{Q} \textb{ \sqrt{z_q^{\tau}} } \ \textb{ \phi_q^{\tau}(\bigcdot)} +
\sum_{n=1}^{N} \textb{v^{\tau}_{n}}  \ \textb{k(\bigcdot - (x_{n} + \tau) } )
\Big] \\
& \stackrel{d}{=} 
 \rho \circ
 \Big[  
 \sum_{n=1}^{N}  k_{\mathrm{RBF}}(\bigcdot -  (x_n  +\tau ) ) \ , \  
\sum_{q=1}^{Q} \textb{ \sqrt{z_q} } \ \textb{ \phi_q(\bigcdot)} +
\sum_{n=1}^{N} \textb{v_{n}}  \ \textb{k(\bigcdot - (x_{n} + \tau) } )
\Big]  \label{eqn:step2} \\
& \stackrel{d}{=} 
 \rho \circ
 \Big[  
 \sum_{n=1}^{N}  k_{\mathrm{RBF}}(\bigcdot -  (x_n  +\tau ) ) \ , \  
\sum_{q=1}^{Q} \textb{ \sqrt{z_q} } \ \textb{ \phi_q(\bigcdot - \tau)} +
\sum_{n=1}^{N} \textb{v_{n}}  \ \textb{k(\bigcdot - (x_{n} + \tau) } )
\Big] \label{eqn:step3}\\
& = 
\bigg( 
\underbrace{
 \rho \circ
 \Big[  
 \sum_{n=1}^{N}  k_{\mathrm{RBF}}(\bigcdot -  x_n   ) \ , \  
\sum_{q=1}^{Q} \textb{ \sqrt{z_q} } \ \textb{ \phi_q(\bigcdot)} +
\sum_{n=1}^{N} \textb{v_{n}}  \ \textb{k(\bigcdot - x_{n} } )
\Big]
}_{\Phi^{\mathcal{B}}(D)}
\bigg) (\bigcdot - \tau) 
= T^{*}_{\tau} \circ (\Phi^{\mathcal{B}}(D)).
\end{align}
The equality in \cref{eqn:step2} holds in distribution sense as explained in \cref{eqn:hold_latent,eqn:hold_latentkernel,eqn:hold_weight}.

%$\phi_q(\bigcdot ) \sim N(0; \Phi_q(G)\Phi_q(G)^{T})$ 
The equality in \cref{eqn:step3} holds because each $q$-th stationary random prior function $\phi_q(\bigcdot )$ evaluated on finite grid $G=\{t_{m}\}_{m=1}^{M}$ follows the Gaussian distribution as 
\begin{align}
\phi_q(\bigcdot ) \sim N(0; \Phi_q(G)\Phi_q(G)^{T}), \hspace{3mm} \Phi_q(G)\Phi_q(G)^{T} \approx K_q(G,G)
\end{align}
where $\Phi_q(G) = [\phi_q(t_{1} ),..,\phi_q(t_{M} )] \in R^{M \times f}$, with the number of sampled spectral points $f$, denotes the random feature matrix obtained by applying the random Fourier feature to $q$-th stationary kernel $k_q$, and $ \Phi_q(G)\Phi_q(G)^{T}$ approximate the Gram matrix $K_q(G,G) \in R^{M \times M}$. The $\tau$-translated function $\phi_q(\bigcdot - \tau)$ follows the same distribution as well:
\begin{align}
\phi_q(\bigcdot - \tau ) \sim N(0; \Phi_q(G)\Phi_q(G)^{T}).
\end{align}
This is because $\phi_q(\bigcdot)$ is a instance of the stationary process evaluated on finite points $G$, and its translated function still follows the same stationary process as well.

Therefore, we prove the representation of Bayesian ConvDeepsets holds the TE in distribution sense as stated in \cref{pro:te_probsense}.

\end{proof}
\vspace{-2mm}
%\end{proposition*}
\end{custom_pro}

\clearpage
%\paragraph{Training objective in \textb{Eq. (17)} (main).} 
\subsubsection{Proof of Training objective in \textb{Eq. (21) (main)}} 

%In this section, we explain how our training objective is 

Let $\Theta = \{\theta_{\mathrm{kernels}}, \theta_{\mathrm{p_{\mathrm{nn}}}}, \theta_{\rho},\theta_{\mathrm{pred}}\}$ be the learnable parameters for kernels, the translate invariant network, the CNN, and the network for prediction. To train the model parameters, we optimize following objective w.r.t $\Theta$ :
\begin{align}
 \mathbb{E}_{D^{c},D^{t} \sim p(\mathcal{T})} 
 \bigl[
 \mathcal{L}_{\text{ll}}(\Theta ; D^{c}, D^{t})  - \beta \hspace{.2mm} \mathcal{L}_{\text{reg}}( \Theta ;D^{c}, D^{t}) 
 \bigr]
\label{eqn:tr_objective}
\end{align}
where $\mathcal{L}_{\text{ll}}(\Theta ; D^{c}, D^{t})$ denotes the log likelihood, and $\mathcal{L}_{\text{reg}}(\Theta;D^{c}, D^{t})$ denotes the regularizer that induces the output of network $\mathrm{p}_{\mathrm{nn}}(D^c)$ to assign the reasonable stationary prior depending on context set $D^c$. In the following, we explain how the log likelihood $\mathcal{L}_{\text{ll}}(\Theta ; D^{c}, D^{t})$ and the regulaizer $\mathcal{L}_{\text{reg}}( \Theta ;D^{c}, D^{t})$ are derived:

%$\mathcal{L}_{\text{ll}}(\Theta ; D^{c}, D^{t})$
\paragraph{Likelihood.}  For each task of the context set $D^c=\{(x^{c}_{n},y^{c}_{n})\}_{n=1}^{N^{c}}$ and target set $D^t=\{(x^{t}_{n},y^{t}_{n})\}_{n=1}^{N^{t}}$ that are sampled from the distribution of the task $p(\mathcal{T})$, the multi-sampled log likelihood estimator $\mathcal{L}_{\text{ll}}(\Theta ; D^{c}, D^{t})$ is derived as  
\begin{align}
\log{p(Y^{t}| X^{t}, D^{c} )}  
&=
\log{
\int p(Y^{t}| X^{t}, \Phi^{\mathcal{B}}  ) 
p(\Phi^{\mathcal{B}} | Z_{\text{Cat}},D^{c} )
\ p(Z_{\text{Cat}}| D^{c}  ) 
\ 
d \Phi^{\mathcal{B}}
d Z_{\text{Cat}} 
} \\
&\approx 
\log{
\left(
\frac{1}{N} \sum_{n=1}^{N} p(Y^{t}| X^{t}, \Phi^{\mathcal{B}}_{(n)}  )
\right)
},  \hspace{2mm} \   Z_{(n)} \sim q(Z_{\mathrm{Cat}} | \mathrm{p}_{\mathrm{nn}}(D^{c}) ), \ \Phi^{\mathcal{B}}_{(n)} \sim p(\Phi^{\mathrm{B}}(D^{c})) | Z_{\mathrm{Cat}} = Z_{(n)} )
\nonumber \\
&=
\log{
\left(
\frac{1}{N} \sum_{n=1}^{N} \left( \prod_{i=1}^{N^{t}} p(y^{t}_{i}| x^{t}_{i}, \Phi^{\mathcal{B}}_{(n)}  ) \right)
\right)
}  \label{eqn:condiindep} \\
&= \log{
\left(
 \frac{1}{N} 
 \sum_{n=1}^{N} \exp{ \left(  \sum_{i=1}^{N^{t}} \log{p \left(  y^{t}_{i}| x^{t}_{i}, \Phi^{\mathcal{B}}_{(n)}  \right)}  \right) }
 \right)  }  = \coloneq   \mathcal{L}_{\text{ll}}(\Theta ; D^{c}, D^{t})
\end{align}

where $ Z_{(n)}$ denotes the $n$-th random sample of $q(Z_{\mathrm{Cat}} | D^{c}) = \mathrm{Cat}(Z_{\mathrm{Cat}}; \mathrm{p}_{\mathrm{nn}}(D^{c}))$, and $\Phi^{\mathcal{B}}_{(n)}$ denote the $n$-th sampled representation of Bayesian ConvDeepsets on finite grid $\{t_m\}_{m=1}^{M}$. In \cref{eqn:condiindep}, the conditional independence assumption for given $ \Phi^{\mathcal{B}}_{(n)} $ is used for the $n$-th likelihood, i.e.,  $p(Y^{t} | X^{t},\Phi^{\mathcal{B}}_{(n)})=\prod_{i=1}^{N^{t}} p(y^{t}_{i}| x^{t}_{i},\Phi^{\mathcal{B}}_{(n)})  $, and the likelihood of each observation $p(y^{t}_{i}| x^{t}_{i},\Phi^{\mathcal{B}}_{(n)})$ is modeled as Gaussian distribution, i.e.,
\begin{align}
p(y^{t}_{i}| x^{t}_{i},\Phi^{\mathcal{B}}_{(n)}) = 
N(y^{t}_{i}; \mu_{\mathrm{nn}} (x^{t}_{i},\Phi^{\mathcal{B}}_{(n)}) , \sigma^{2}_{\mathrm{nn}} (x^{t}_{i},\Phi^{\mathcal{B}}_{(n)}) ),
\end{align}
where $\mu_{\mathrm{nn}} (x^{t}_{i},\Phi^{\mathcal{B}}_{(n)})$ and $\sigma_{\mathrm{nn}} (x^{t}_{i},\Phi^{\mathcal{B}}_{(n)})$ denote the predictive mean and standard deviation on $x^{t}_{i}$, and both are parameterized by neural network. In this work, we smooth the representation $\Phi^{\mathcal{B}}_{(n)}$ on target input $x^{t}_{i}$ as described in \textb{Eq. (6) (main)}, and forward the smoothed representation by MLP layers to obtain the parameters of the predictive distribution.

% To assign the task-dependent stationary prior depending on context set $D^{c}$, we introduce the amortized latent variable of which is modeled by the categorical distribution parameterized by the translate invariant neural network $\mathrm{p}_{\mathrm{nn}}(D)$. Based on the fact the optimal variational distribution of $Z_{\mathrm{Cat}}$ is ,

\paragraph{Regularizer.} We consider the regulaizer $\mathcal{L}_{\text{reg}}( \Theta ;D^{c}, D^{t})$ to allow the output of  $\mathrm{p}_{\mathrm{nn}}(D^{c})$ to assign the proper stationary prior for given task. To this end, we employ the result of variational inference for the regulaizer: the optimal distribution of $Z_{\mathrm{Cat}}$ is proportional to the posterior of $Z^{c}$.
That is, let $\tilde{q} \left( Z_{\mathrm{Cat}} \right)$ be a variational distribution in a class of categorical distribution. Then the lower bound of log marginal likelihood is represented as 
\begin{align}
\log{p(Y^{t}|X^{t},D^{c})} \geq  
\int \log{ \left( \frac{p(Y^{t},Z_{\mathrm{Cat}}|X^{t},D^{c})}{\tilde{q} \left( Z_{\mathrm{Cat}}  \right) }   \right)}  
\tilde{q} \left( Z_{\mathrm{Cat}} \right) d Z_{\mathrm{Cat}}.
\end{align}
The equality holds when the variational distribution $ \tilde{q} \left ( Z_{\mathrm{Cat}} \right)$ is a posterior distribution of $Z_{\mathrm{Cat}}$ within a class of categorical distribution, i.e., $\tilde{q} \left( Z_{\mathrm{Cat}} \right)=p(Z_{\mathrm{Cat}} | D^c, D^{t}) =  \mathrm{Cat}(Z_{\text{cat}};\mathrm{p}_{\mathrm{posterior}}) $. Using the fact that the posterior distribution is proportional as
\begin{align}
p (Z_{\text{cat}} = \underbrace{(0,..,1,...0)}_{\mathrm{q\text{-}th \ indicator} } \ | \  D^{c}, D^{t}  ) 
&= \frac{p ( D^{t}, Z_{\text{cat}} = (0,..,1,...0) \ | \  D^{c}  ) }
        {p (  D^{t} \ | \  D^{c} ) }\\
&\propto  p ( D^{t}, Z_{\text{cat}} = (0,..,1,...0) \ | \  D^{c}  ) \\
&= p ( D^{t} | Z_{\text{cat}} = (0,..,1,...0), D^{c}  ) \
   p ( Z_{\text{cat}} = (0,..,1,...0) \ | \  D^{c}  ) \\
&\propto  p ( Y^{t} | X^{t}, Z_{\text{cat}} = (0,..,1,...0), D^{c}  ) \  p ( Y^{c} | X^{c}, Z_{\text{cat}} = (0,..,1,...0) ) \\ 
&\propto  p ( Y^{t} | X^{t}, Z_{\text{cat}} = (0,..,1,...0), D^{c}  ) ,
\end{align}
we set the parameter of posterior distribution $\mathrm{p}_{\mathrm{posterior}}$ such that $q$-th entry of $\mathrm{p}_{\mathrm{posterior}}$ is represented as 
\begin{align}
(\mathrm{p}_{\mathrm{posterior}})_{(q)} = 
\frac{\mathrm{exp} \left( \log{p(Y^{t} | X^{t}, D^{c}, k_q)} \ / \  \tau_{0} \right)}
{\sum_{q=1}^{Q} \mathrm{exp} \left( \log{p(Y^{t} | X^{t}, D^{c}, k_q)} \ /\  \tau_{0} \right)}
\end{align}
where $\tau_{0}$ denotes the temperature hyperparameters. For $\log{p(Y^{t} | X^{t}, D^{c}, k_q)}$, we compute the likelihood via empirical distribution as follows:
\begin{align}
\hspace{-2.2mm}
p(Y^{t} | X^{t},D^{c}, k_q) = N( Y^{t} ;\hat{\mu}_{q}(X^{t}),\mathrm{Diag}(\hat{\Sigma}_{q}(X^{t})) ),
\label{eqn:emp-gpposterior}
\end{align}
which can be computed efficiently. The empirical predictive mean $\hat{\mu}_{q}(X^{t}) \in R^{N_t}$ and diagonal covariance $\mathrm{Diag}(\hat{\Sigma}_{q}(X^{t})) \in R^{N_t}$ are computed by using the sample functions of GP posterior in \textb{Eq. (12) (main)}.

As a result, we consider the regulaizer $\mathcal{L}_{\text{reg}}( \Theta ;D^{c}, D^{t})$ via the KL divergence between categorical distribution, i.e,
\begin{align}
\mathcal{L}_{\text{reg}}( \Theta ;D^{c}, D^{t}) \coloneqq \mathrm{KL} \left( q(Z_{\text{cat}} \ | \  D^{c} )  \ || \  p (Z_{\text{cat}} \ | \  D^{c}, D^{t}  )  \right)
\label{eqn:appendix_reg}.
\end{align}

% , and compute the likelihood as
% \begin{align}
% \hspace{-2.2mm}
% p(Y^{t} | X^{t},D^{c}, k_q) = N( Y^{t} ;\hat{\mu}_{q}(X^{t}),\mathrm{Diag}(\hat{\Sigma}_{q}(X^{t})) ) 
% \label{eqn:emp-gpposterior}
% \end{align}
% where $\hat{\mu}_{q}(X^{t}) \in R^{N_t}$ and $\mathrm{Diag}(\hat{\Sigma}_{q}(X^{t})) \in R^{N_t}$ denote the empirical predictive mean and diagonal covariance of the GP posterior distribution on target set $X^{t}$. The sample functions of GP posterior, described in \cref{eqn:randomfunctionalfeature}, are used. The derivation of training loss is explained in Appendix A.3.

% these sample functions are obtained in forward procedure.
% the GP posterior distribution on target set $X^{t}$

% The $ p (Z_{\text{cat}} \ | \  D^{c}, D^{t}  )= \mathrm{Cat}(Z_{\text{cat}};\mathrm{p}_{\mathrm{prior}}  ) $ is computed with the parameter $\mathrm{p} \in {\Delta}^{Q-1} $ of which the $q$-th element $\mathrm{p}_{q} $ is defined as follows: 

% \begin{align}
% p (Z_{\text{cat}} = \underbrace{(0,..,1,...0)}_{\mathrm{q{-}th \ indicator}} \ | \  D^{c}, D^{t}  ) 
% &= p (Z_{\text{cat}} = (0,..,1,...0) \ | \  D^{c}, D^{t}  ) \\
% %\propto  p ( Y^{t}, Z_{\text{cat}} \ | \  X^{t}, D^{c},   )
% \end{align}

%\mathcal{L}
%\paragraph{Comparison the proposed training objective with the ELBO of variational inference.} 
\paragraph{Comparison the proposed training objective with the conventional ELBO.} 
As we consider the conventional ELBO estimator $\mathcal{L}_{N}$ of meta-learning framework, represented as,
\begin{align}
& \hspace{4.75mm} \mathbb{E}_{D^{c},D^{t} \sim p(\mathcal{T})} 
 \bigg[
 \int \log p \left( Y^{t}|X^{t},D^{c},\Phi^{\mathcal{B}},Z_{\mathrm{Cat}} \right) q(\Phi^{\mathcal{B}},Z_{\mathrm{Cat}}) \ d  \Phi^{\mathcal{B}} \ d Z_{\mathrm{Cat}}
 -
 \mathrm{KL}( q(\Phi^{\mathcal{B}},Z_{\mathrm{Cat}}) || p(\Phi^{\mathcal{B}},Z_{\mathrm{Cat}}) )  
 \bigg] \nonumber \\
&\approx \mathbb{E}_{D^{c},D^{t} \sim p(\mathcal{T})} 
\bigg[
\underbrace{\frac{1}{N} \sum_{n=1}^{N}\log p \left( Y^{t}|X^{t},D^{c},\Phi^{\mathcal{B}}_{(n)} \right) }_{\mathrm{likelihood}}
-
\underbrace{
\bigg(
\mathrm{KL}( q(\Phi^{\mathcal{B}}) || p(\Phi^{\mathcal{B}}) )  
+
\mathrm{KL}( q(Z_{\mathrm{Cat}}) || p(Z_{\mathrm{Cat}}) )  
\bigg)
}_{\mathrm{regulaizer}}
\bigg] \coloneqq \mathcal{L}_{N}
\label{eqn:appendix_reg_naive}
\end{align}
the proposed objective employs the multi-sampled log likelihood estimator, used in \citeb{burda2016importance,foong2020meta}, which is known to be tighter than the likelihood term of $\mathcal{L}_{N}$. In addition, the proposed objective focuses on regularizing $Z_{\mathrm{Cat}}$, and use the posterior distribution $p(Z_{\mathrm{cat}} | D^t,D^{c} )$ in \cref{eqn:appendix_reg} for training $q(Z_{\mathrm{Cat}})$ instead of the prior distribution $p(Z_{\mathrm{cat}} )$ as shown in \cref{eqn:appendix_reg_naive}.

\clearpage

%\subsection{Further Details for the 1d Regression Task}
\section{Further Details for 1d Regression Task}

\label{appendix:1d-regression-task}

% data --> model --> training -- additional results
\subsection{Details for Datasets}

To train the NP models, we employ the meta-learning framework; for every task, when the given finite observations, referred as context sets and target sets are assumed to be finite samples of the function sampled from stochastic process, the NP models first construct the functional representation of the context sets and then generate the predictive distribution on the target sets.

We consider 4 stationary stochastic processes: RBF,  Matern-$\frac{5}{2}$, Weakly periodic, and Sawtooth, which are used in \citeb{gordon2019convolutional}, to prepare the context and target sets. We describe the each process as follows:
\begin{itemize}[leftmargin=1em]
    \item \textbf{RBF (large lengthscale)}: The context and target sets are constructed by randomly choosing $N_{c}$ data points and $N_{t}$ data points from the function sampled from Gaussian Process (GP) with the following kernel function $k$ with the random lengthscale $l \sim \mathcal{U}([1.1,2.1])$, that is randomly sampled per each task:
    $$k(x, x') = e^{-\frac{1}{2}(\frac{x-x'}{l})^2}.$$
    \item \textbf{Matern-$\frac{5}{2}$ (small lengthscale)}: The context and target sets are constructed by randomly $N_{c}$ data points and $N_{t}$ data points from the function sampled from GP with the following kernel function $k$ with $d = |\frac{x - x'}{l}|$ and random lengthscale $l \sim \mathcal{U}([0.19,0.21])$, that is randomly sampled per each task:
    $$k(x, x') = (1 + \sqrt{5} d  + \frac{5}{3} d^2) e^{-\sqrt{5} d}.$$
    \item \textbf{Weakly periodic}: The context and target sets are constructed by randomly choosing $N_{c}$ data points and $N_{t}$ data points from the function sampled from GP with the following kernel function $k$ with $g_1(x) = \cos(2 \pi f x )$, $g_2(x) = \sin(2\pi f x )$, and random frequency parameter $f \sim \mathcal{U}([2.0,3.0])$, that is randomly sampled per each task:
    $$k(x, x') = e^{ \left( -\frac12 (g_1(x) - g_1(x'))^2 -\frac12 (g_2(x) - g_2(x'))^2 - \frac{1}{32} (x-x')^2 \right)}.$$
    \item \textbf{Sawtooth}: The context and target sets are constructed by randomly choosing $N_{c}$ data points and $N_{t}$ data points from the sampled function $y_{\text{sawtooth}}(t)$ represented as
    $$y_{\text{sawtooth}}(t) = \frac{A}{2} - \frac{A}{\pi}\sum_{k=1}^\infty (-1)^k \frac{\sin(2\pi k f (t+\tau))}{k},$$
    where $A$ denotes the amplitude, $f$ denotes the frequency, $\tau$ denotes the shift, and $t$ denotes time. We use truncate the series at an integer $K$. We consider the random amplitude $A \sim \mathcal{U}([0.8,1.2])$, random frequency $f \sim \mathcal{U}([1,2])$, random truncation integer $K \sim \mathcal{U}([10,20])$, and random shift $\tau \sim \mathcal{U}([-1,1])$, which are randomly sampled for each task. 
\end{itemize}
%http://143.248.92.34:8888/lab/workspaces/auto-U/tree/UAI22_CCCNP_from108/dataset_singletask_1d.py

%\subsubsection{Details for Training, Validation, and Test}
\subsection{Details for Tasks of Training, Validation, and Test }
\label{subsubsec:prepare_sets}

In this experiment, we set the training range \textb{$[0,4]$} and test range \textb{$[4,8]$} (outside of training range). For training, we construct the context sets and target sets by sampling the data points on training range. Then, we evaluate the trained models with context sets and target sets, that are sampled on test range. These test sets are used to check whether trained NP models holds translation equivariance.

We consider the following number of data points for training, validation, and test:
\begin{itemize}[leftmargin=1em]
    \vspace{-2mm}
    \item \textbf{Small number of context data points:} For training, we randomly sample \textb{$N_c \sim \mathcal{U}([5,25])$} as the number of context data points, and randomly sample \textb{$N_t \sim \mathcal{U}([N_c,50])$} as the number of target data points for each task. We use \textb{$500{\times}50{\times}16$} tasks for training through 500 batches. For validation, we set $N_c$ context data points and $N_t$ target data points as done in training, and use \textb{$128{\times}16$} tasks for validation to choose the parameters of the trained models. For test, we also set $N_c$ context data points and $N_t$ target data points for each processes (RBF, Matern-$\frac{5}{2}$, Weakly periodic, and Sawtooth), as done in training, and use \textb{$128{\times}16$} tasks per the process to evaluate the trained models using the chosen parameters in validation.
    \vspace{-1mm}
    \item \textbf{Large number of context data points:} For training, we randomly sample \textb{$N_c \sim \mathcal{U}([10,50])$} as the number of context data points, and randomly sample \textb{$N_t \sim \mathcal{U}([N_c,50])$} as the number of target data points for each task. For validation and test, we use \textb{$128{\times}16$} tasks. For test set, we use \textb{$128{\times}16$} tasks per the process, as done in the case of \textbf{the small number of context data points}.
\end{itemize}

Additionally, we consider the same number of tasks per each stochastic process so that the NP models does not fit particular stochastic process only during training

\subsection{Details for Hyperparameters.}

\paragraph{Hyperparameters of Kernels.}

% For the hyperparameter of RBF kernels used for ConvCNP and ConvLNP, we conduct the experiment with  $l\in\{0.1,0.5,1.0\}$, and set the lengthscale $l=0.1$ for both models because it obtains the best performance out of those candidates.

% For the hyperparameter of RBF kernels used for GPConvCNP-RBF, we conduct the experiment with  $l\in\{0.1,0.5,1.0\}$, and set the lengthscale  $l=1.0$ obtaining the best performance out of those candidates.

% For the hyperparameter of SM kernels ($Q=1$) used for GPConvCNP-SM, we set $\mu$ randomly by sampling $\mu$ from $\mathcal{U}(0,5)$, and set $\Sigma=1.0$. 

% For the hyperparameter of basis kernels, we set $\mathrm{Hz}_{\mathrm{max}}=5$ and 3 basis stationary kernels ($Q=3$ ). Then, we set $\{\mu_q\}_{q=1}^{3}$ by randomly sampling $\mu_q \sim \mathcal{U}[0,\mathrm{Hz}_{\mathrm{max}}]$ with $\mu_1=0 \leq ..\leq \mu_3$, and set
% $\Sigma_q = 1.0$ for $q=1,..,3$. For the noise parameter $\sigma^{2}_{\epsilon}$, we set $\sigma_{\epsilon}=1e\text{-}{2}$.

For the hyperparameter of RBF kernels used for ConvCNP and ConvLNP, we conduct the experiment with  $l\in\{0,01,0.1,0.5\}$, and set the lengthscale $l=0.01$ for both models obtaining the best performance out of those candidates.

For the hyperparameter of GPConvCNP, we conduct the experiment with  $l\in\{0.1,0.5,1.0\}$, and set the lengthscale  $l=1.0$ obtaining the best performance out of those candidates.

For the hyperparameter of the proposed method, we use $Q\in\{3,4,5\}$ basis stationary kernels, and set $\mathrm{HZ}_{\mathrm{max}}=Q$. Then, we space the frequency range $[0,\mathrm{HZ}_{\mathrm{max}}]$ linearly, set each centered value as $\mu_q$ with $\mu_1=0 \leq ..\leq \mu_Q$, and set $\sigma_q = 0.5(\mu_{2} -\mu_{1})$ for $q=1,..,Q$. For the noise parameter $\sigma^{2}_{\epsilon}$, we set $\sigma_{\epsilon}=1e\text{-}{2}$.

For the number of spectral points, we use $l=10$ in \textb{Eq. (14)}.

For the number of sample function, we use $N=5$ in \textb{Eq. (19)}.

For training, we  use ADAM optimizer \citeb{kingma2014adam} with learning rate $5e\text{-}4$ and weight decay $1e\text{-}4$. 

For the regularizer hyperparameter $\beta$ in \textb{Eq. (21)}, we set $\beta=0.1$ for the proposed method.

% \paragraph{Hyperparameters of Kernel Approximation in \textb{Eq. (9)}.}
% For the number of spectral points ($l$ in \textb{Eq. (9)}) used for kernel approximation, we use 10 random Fourier features ($l=10$) per each basis stationary kernel, and thus use total $Q \times 10$ random Fourier features. For the multi-channel stochastic process, we use total $K \times (Q \times 10)$ random Fourier features with $K$ channels.

% \paragraph{Hyperparameters of Random Functional Representations in \textb{Eq. (10)}.}
% For the number of random functional representations ($N$ in \textb{Eq. (10)}), we use 10 functional representations ($N=10$). For multi-channel stochastic process, we use total $K \times 10$ representations with $K$ channels.

% \paragraph{Hyperparameters for Training.} We use ADAM optimizer \citeb{kingma2014adam} with learning rate $5e\text{-}4$ and weight decay $1e\text{-}4$. For the regularizer hyperparameter $\beta$ in \textb{Eq. (17)}, we set $\beta=0.5$.

\subsubsection{Baseline Implementations}
\label{subsubsec:baseline2}
For ANP, we employ the deterministic path of the model described by \citeb{kim2018attentive} for 1d regression experiment. For ConCNP, ConvLNP, and GPConvCNP, we employ the structure of Deep CNN 1d as described in \cref{subsubsec:cnnstructure}. For ANP and ConvCNP, we employ the implementation \footnotemark{\footnotetext[1]{\url{https://github.com/cambridge-mlg/convcnp}}}. For ConvLNP, we refer to the implementation \footnotemark{\footnotetext[2]{\url{https://github.com/YannDubs/Neural-Process-Family}}}.

\clearpage
\subsection{Additional Results}
%\vspace{-2mm}
\paragraph{Training with a small number of context sets.}
For the completeness of the experiment results, we report additional results of the training with a small number of context set $(N_c \sim \mathcal{U}([5,25]) )$. \cref{fig:exp5-1:small-a,fig:exp5-1:small-b,fig:exp5-1:small-c,fig:exp5-1:small-d}
 describes the mean and one-standard error of the log likelihood for $1024$ tasks (within training range). For evaluation, we set varying number of context data points $N^c \in \{5,10,15,20,25\}$ and target points $N^{t}=50$. \cref{fig:exp5-1:small-e,fig:exp5-1:small-f,fig:exp5-1:small-g,fig:exp5-1:small-h} corresponds to the results for tasks (beyond training range). We could not report the results of AttnCNP due to poor generalization performance.

\vspace{-3mm}
\begin{figure}[H]
%\begin{figure}[htp!]
\centering
\subfloat[ \label{fig:exp5-1:small-a} RBF (in-range)]
{\includegraphics[width=0.24\linewidth]{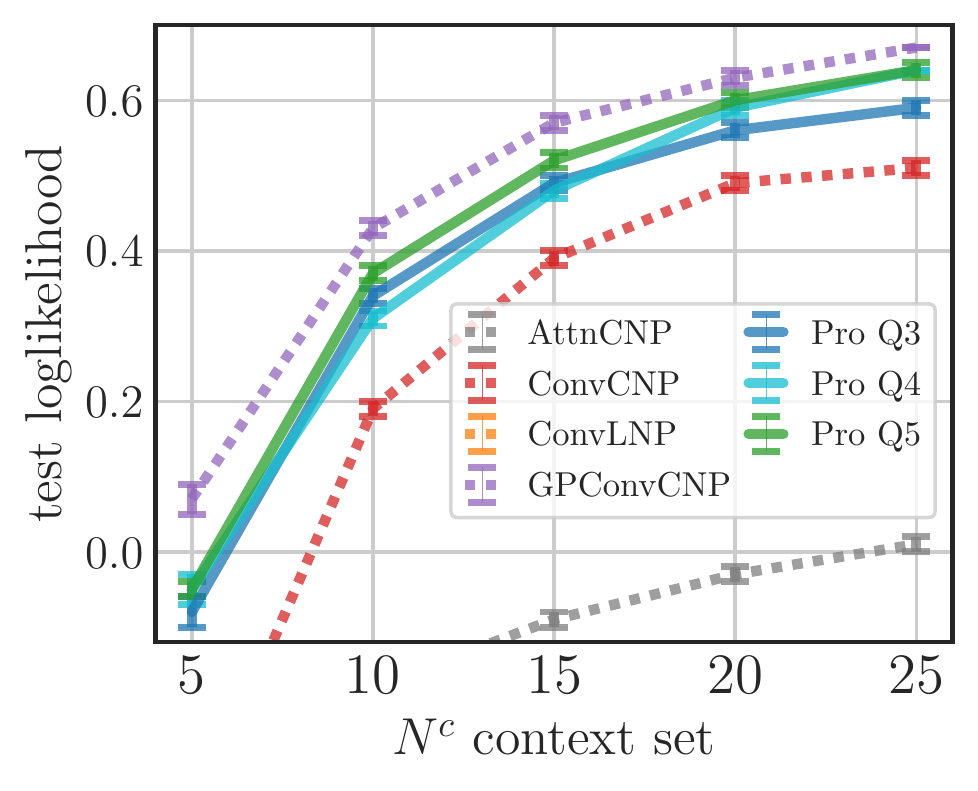}}   \hspace{0.5mm} 
\subfloat[ \label{fig:exp5-1:small-b} Matern-${\frac{5}{2}}$ (in-range)] 
{\includegraphics[width=0.24\linewidth]{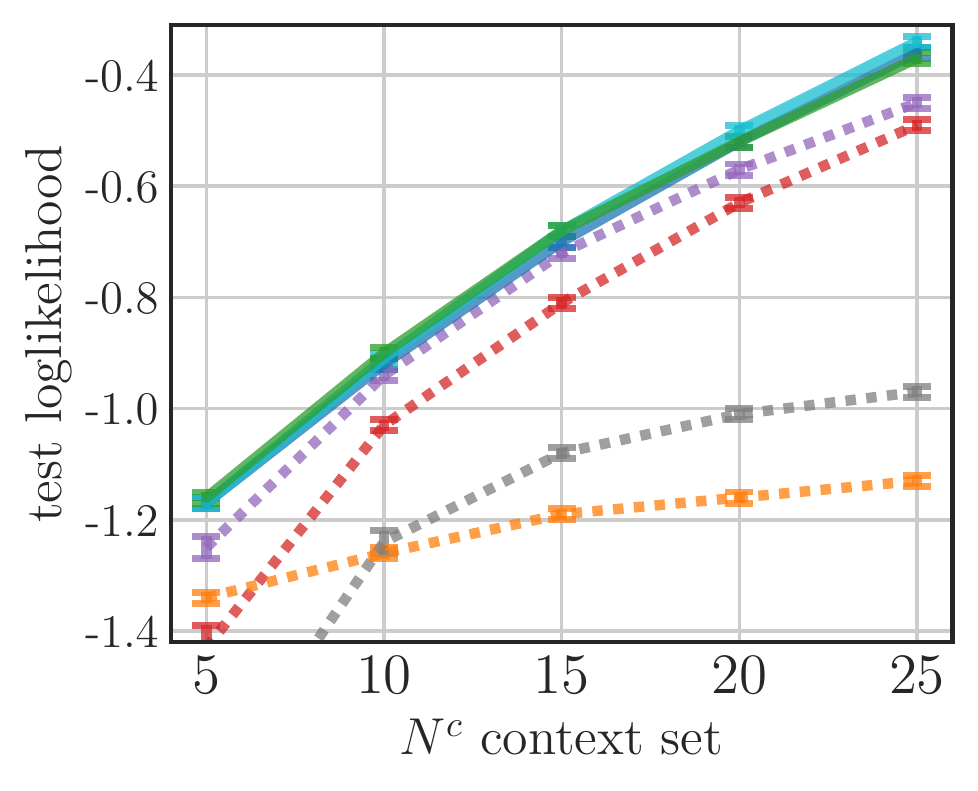}} \hspace{0.5mm}  
\subfloat[ \label{fig:exp5-1:small-c} Weakly periodic (in-range)]
{\includegraphics[width=0.24\linewidth]{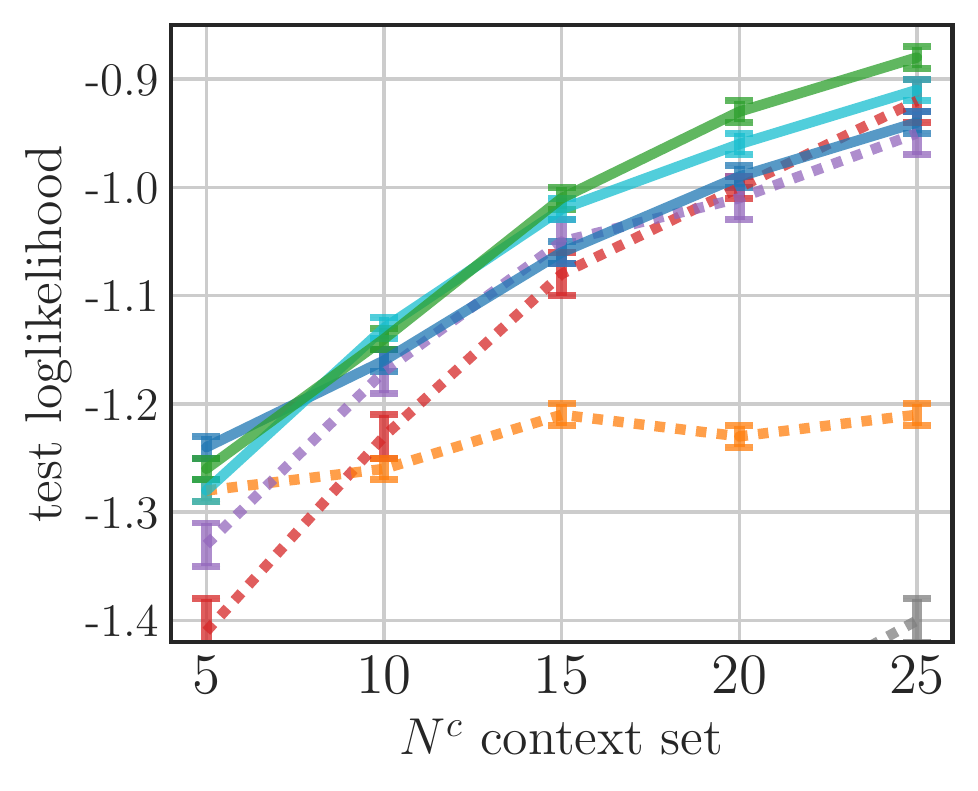}}  \hspace{0.5mm} 
\subfloat[ \label{fig:exp5-1:small-d}Sawtooth (in-range)]
{\includegraphics[width=0.24\linewidth]{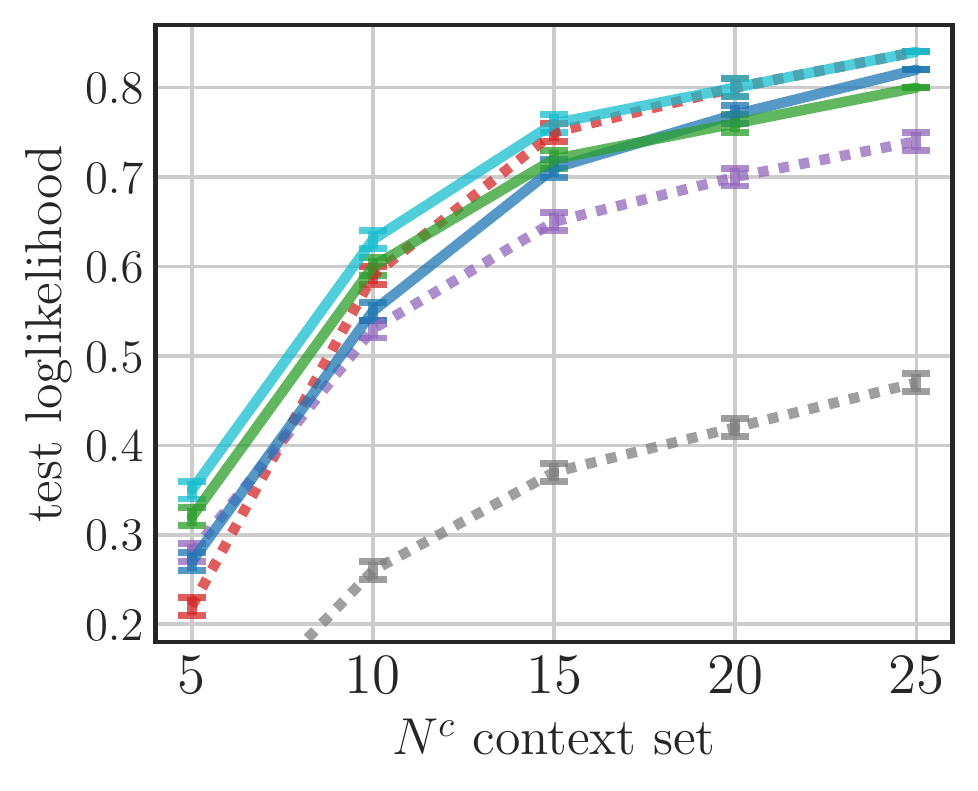}}   

\vspace{2mm}
\subfloat[ \label{fig:exp5-1:small-e} RBF (out-range)]
{\includegraphics[width=0.24\linewidth]{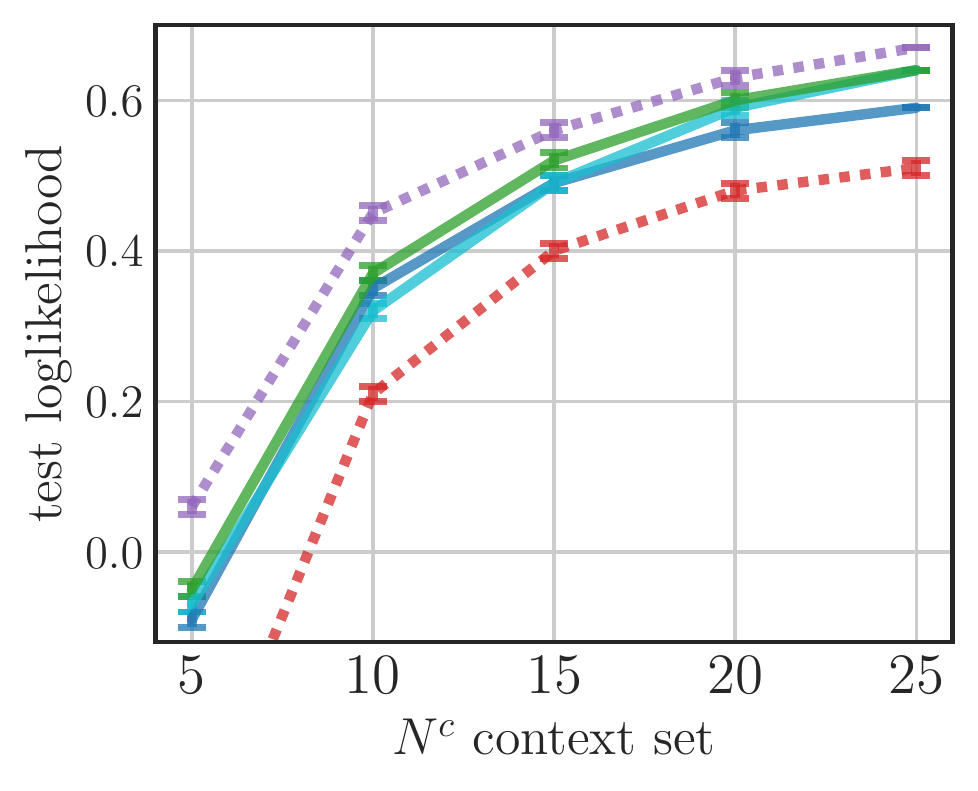}}   \hspace{0.5mm} 
\subfloat[ \label{fig:exp5-1:small-f} Matern-${\frac{5}{2}}$ (out-range)] 
{\includegraphics[width=0.24\linewidth]{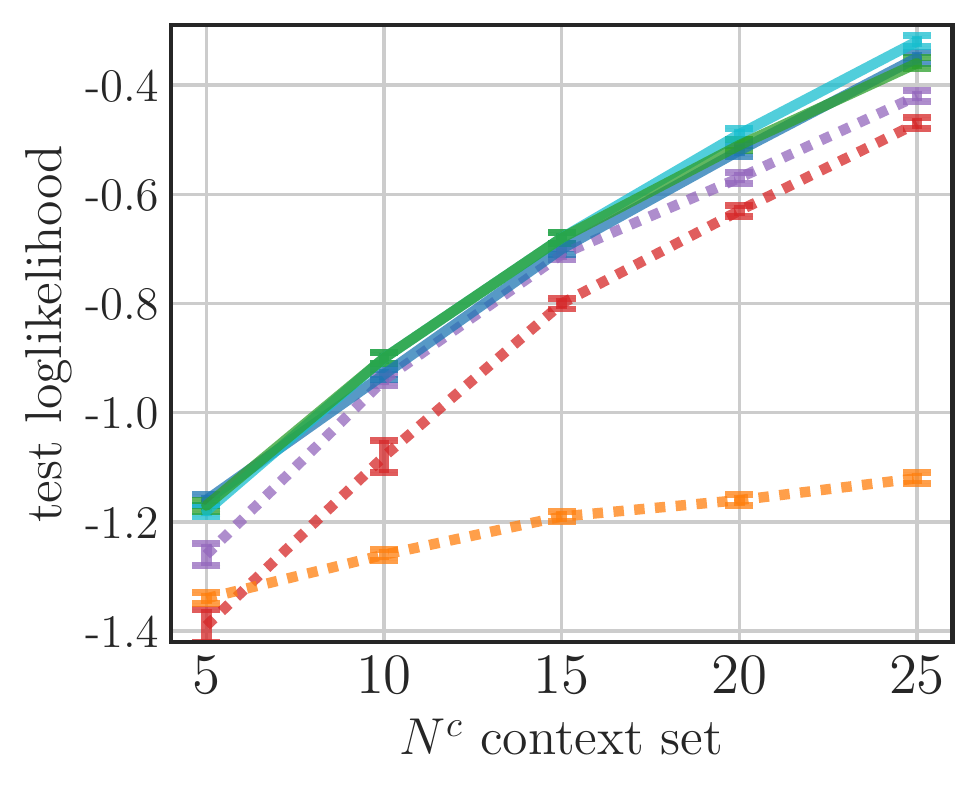}} \hspace{0.5mm}  
\subfloat[ \label{fig:exp5-1:small-g} Weakly periodic (out-range)]
{\includegraphics[width=0.24\linewidth]{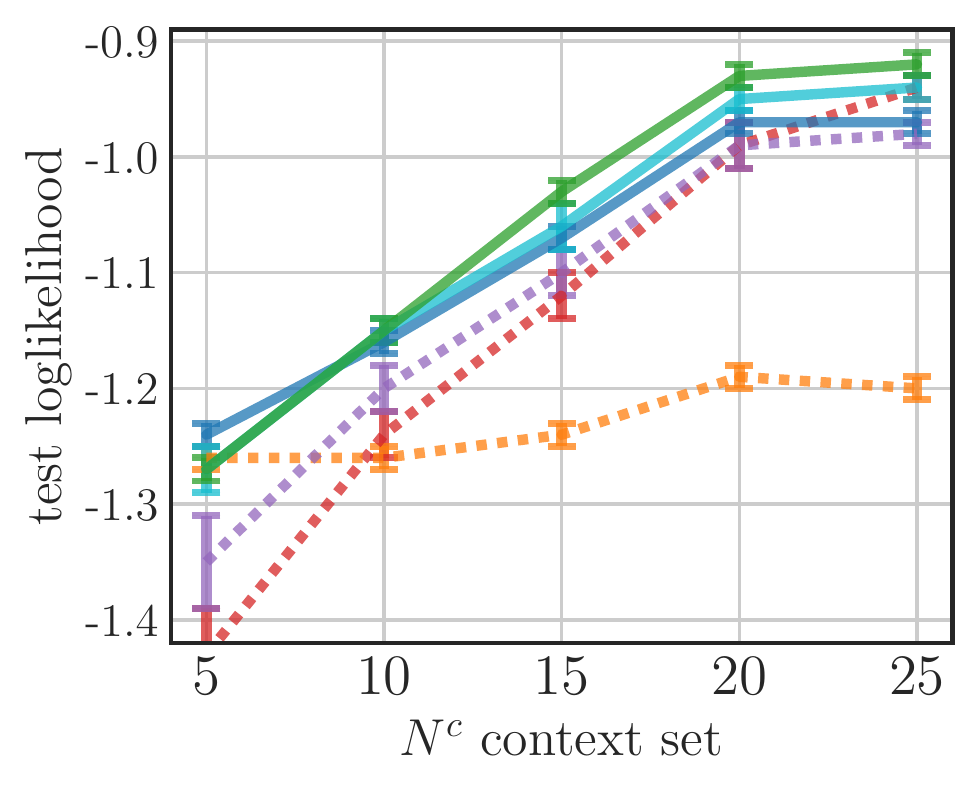}}  \hspace{0.5mm} 
\subfloat[ \label{fig:exp5-1:small-h} Sawtooth (out-range)]
{\includegraphics[width=0.24\linewidth]{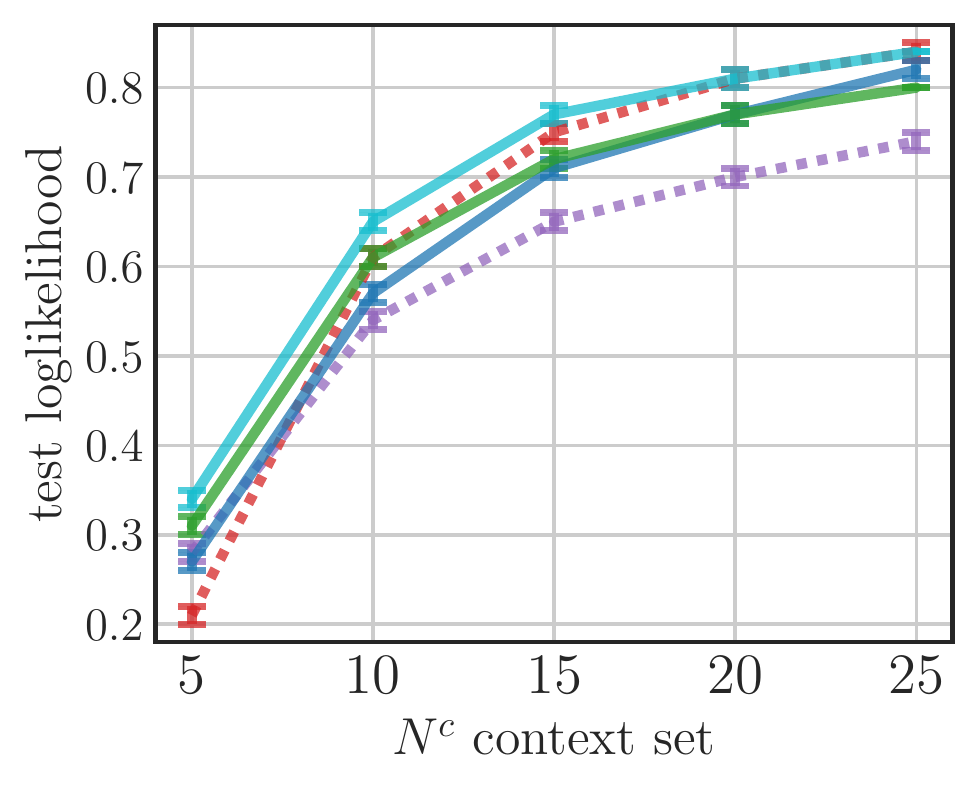}}   
\caption{Prediction result of each processes from training setting of \textb{small $N^{c}$} context points.}
\label{fig:exp5-1:smallset_comparison-supp}
\end{figure}

\vspace{-4mm}
\paragraph{Training with a large number of context sets.}
\vspace{-4mm}

Additionally, we report the results of the training with a large number of context set $(N_c \sim \mathcal{U}([10,50]) )$, and apply the same evaluation procedure with setting of a small number of context set. \cref{fig:exp5-1:small-a2,fig:exp5-1:small-b2,fig:exp5-1:small-c2,fig:exp5-1:small-d2}
 describes the mean and one-standard error of the log likelihood for $1024$ tasks (within training range). \cref{fig:exp5-1:small-e2,fig:exp5-1:small-f2,fig:exp5-1:small-g2,fig:exp5-1:small-h2} corresponds to the results for tasks (beyond training range).

\vspace{-3mm}
\begin{figure}[H]
%\begin{figure}[htp!]
\centering
\subfloat[\label{fig:exp5-1:small-a2} RBF (in-range)]
{\includegraphics[width=0.24\linewidth]{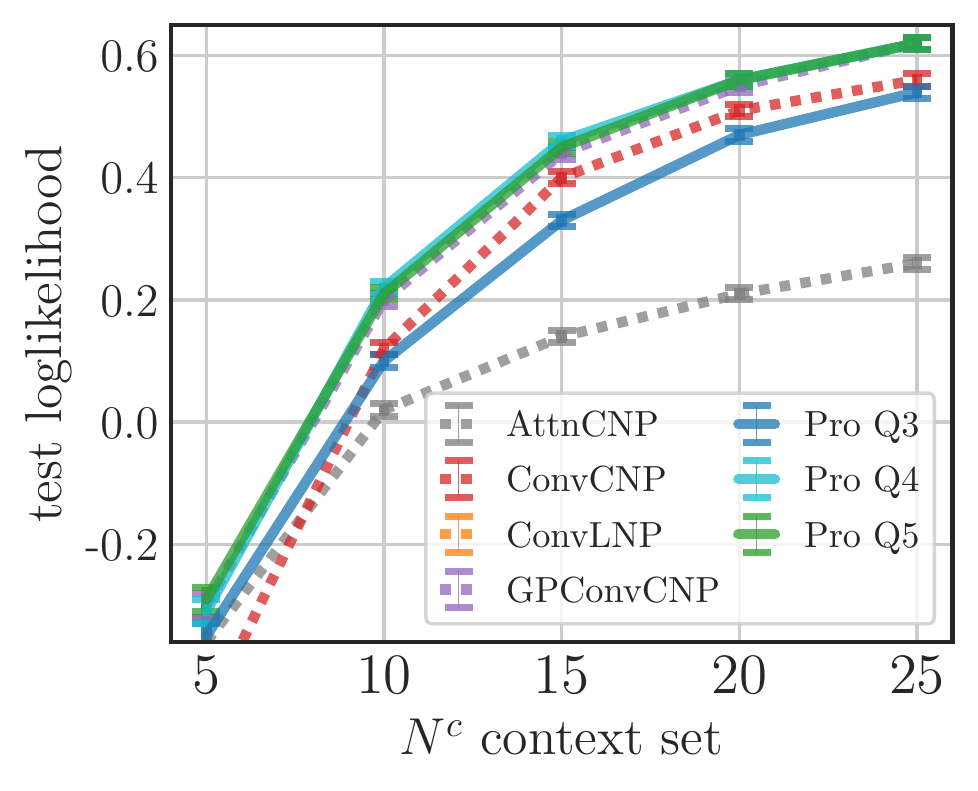}}   \hspace{0.5mm} 
\subfloat[\label{fig:exp5-1:small-b2} Matern-${\frac{5}{2}}$ (in-range)] 
{\includegraphics[width=0.24\linewidth]{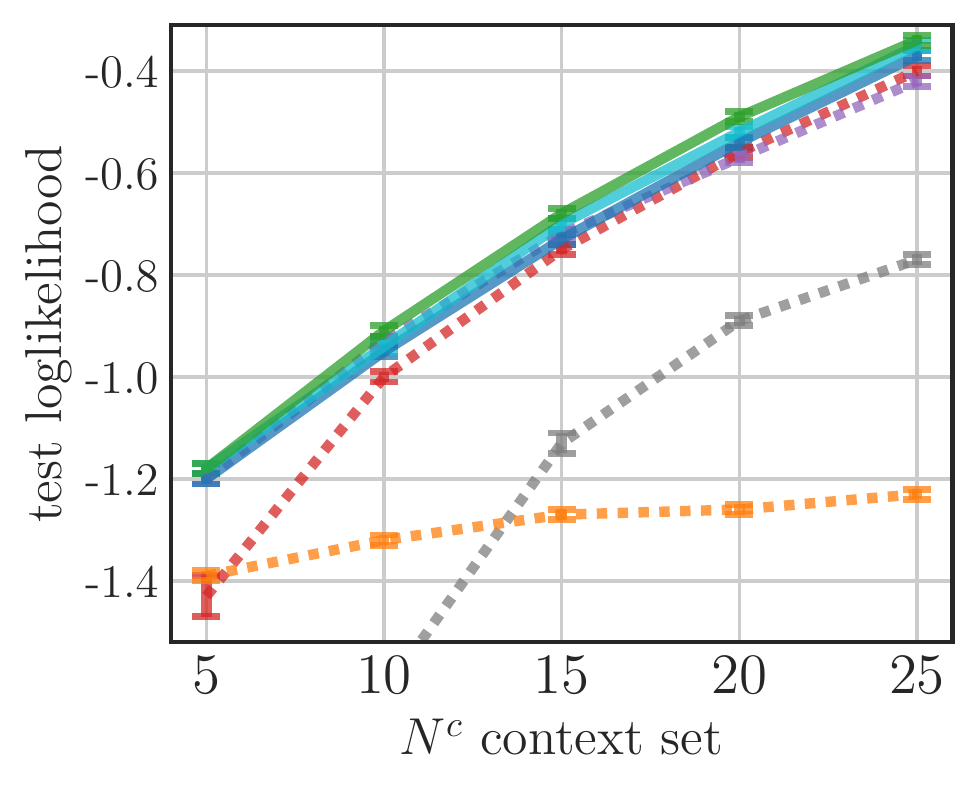}} \hspace{0.5mm}  
\subfloat[\label{fig:exp5-1:small-c2} Weakly periodic (in-range)]
{\includegraphics[width=0.24\linewidth]{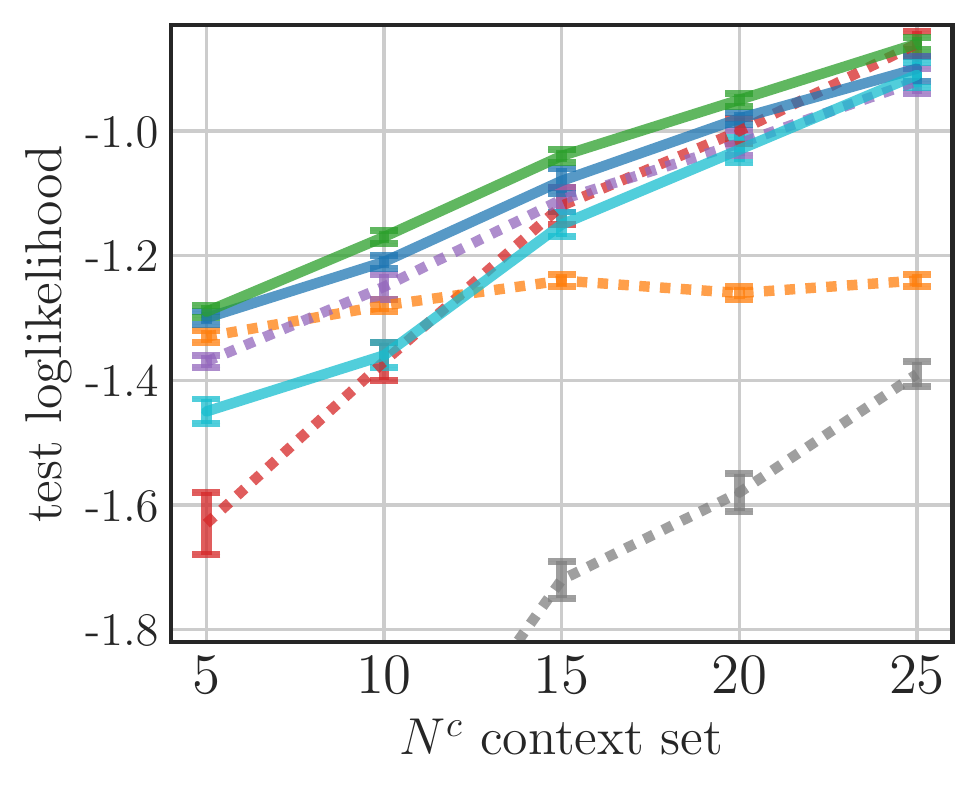}}  \hspace{0.5mm} 
\subfloat[\label{fig:exp5-1:small-d2} Sawtooth (in-range)]
{\includegraphics[width=0.24\linewidth]{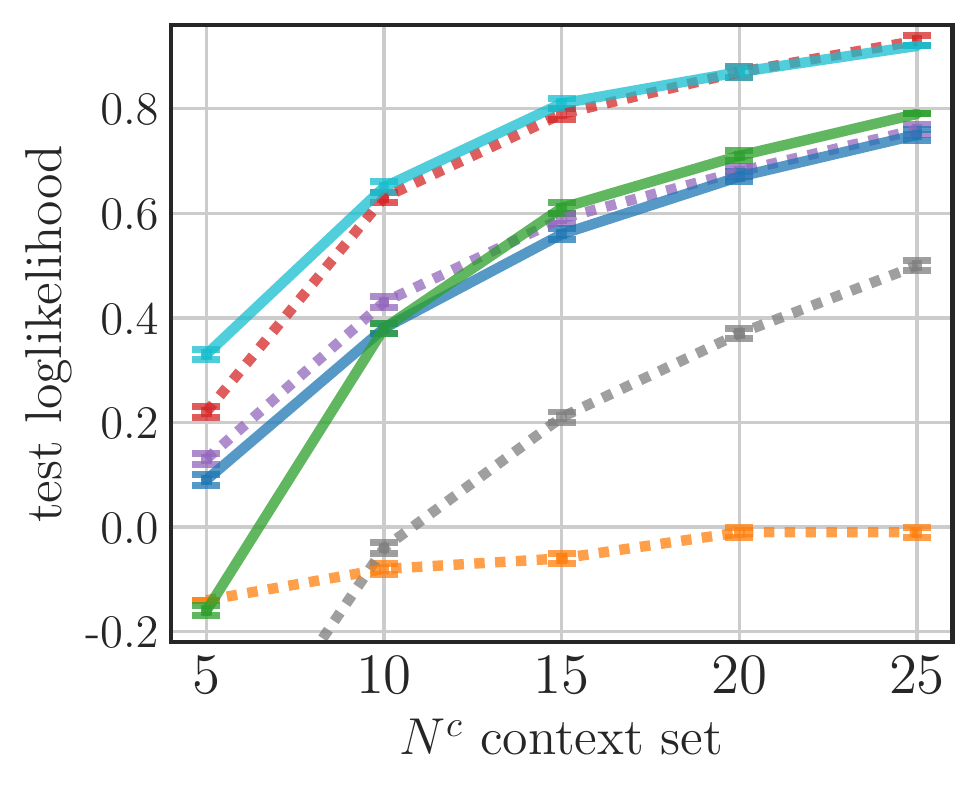}}   

\vspace{2mm}
\subfloat[\label{fig:exp5-1:small-e2} RBF (out-range)]
{\includegraphics[width=0.24\linewidth]{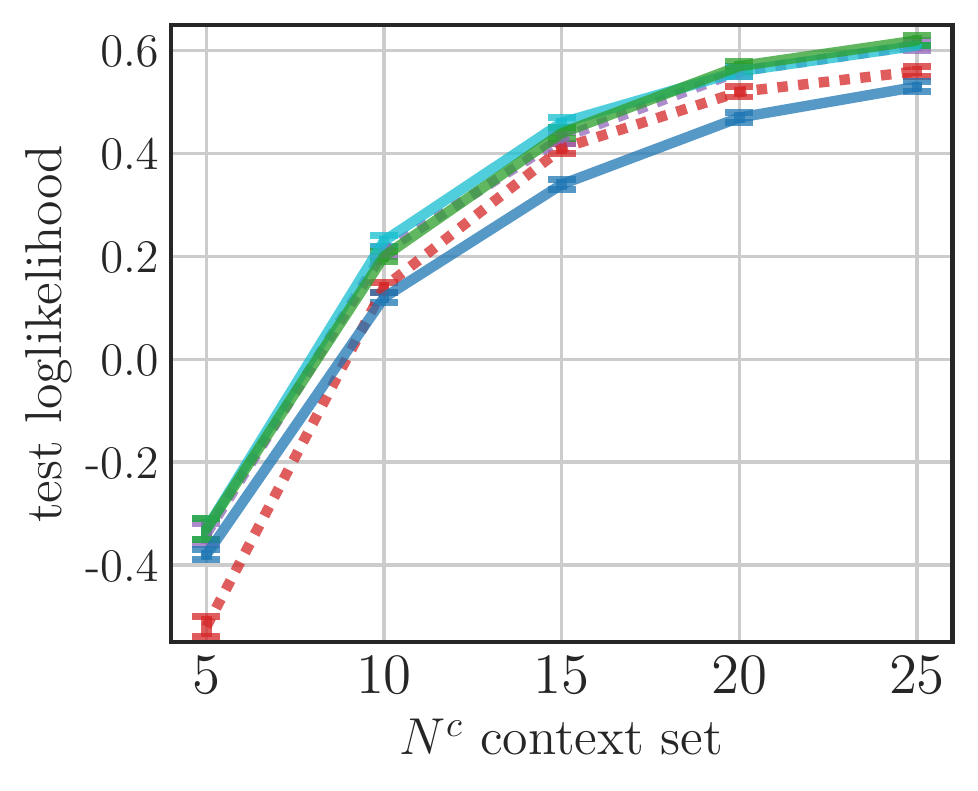}}   \hspace{0.5mm} 
\subfloat[\label{fig:exp5-1:small-f2}  Matern-${\frac{5}{2}}$ (out-range)] 
{\includegraphics[width=0.24\linewidth]{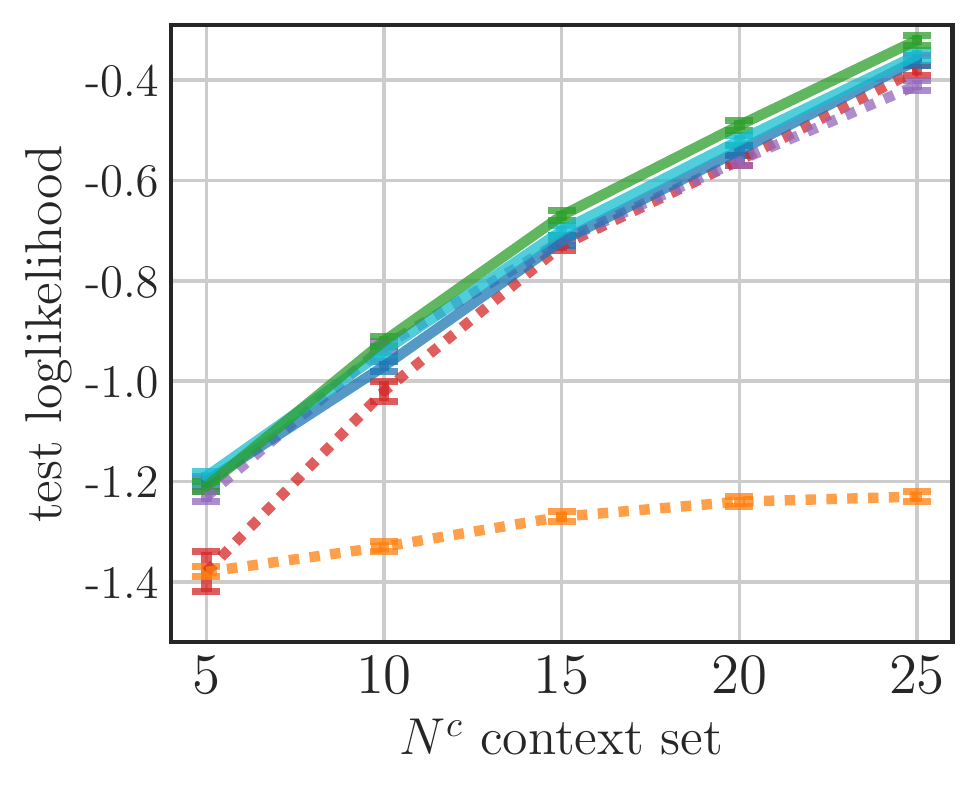}} \hspace{0.5mm}  
\subfloat[\label{fig:exp5-1:small-g2} Weakly periodic (out-range)]
{\includegraphics[width=0.24\linewidth]{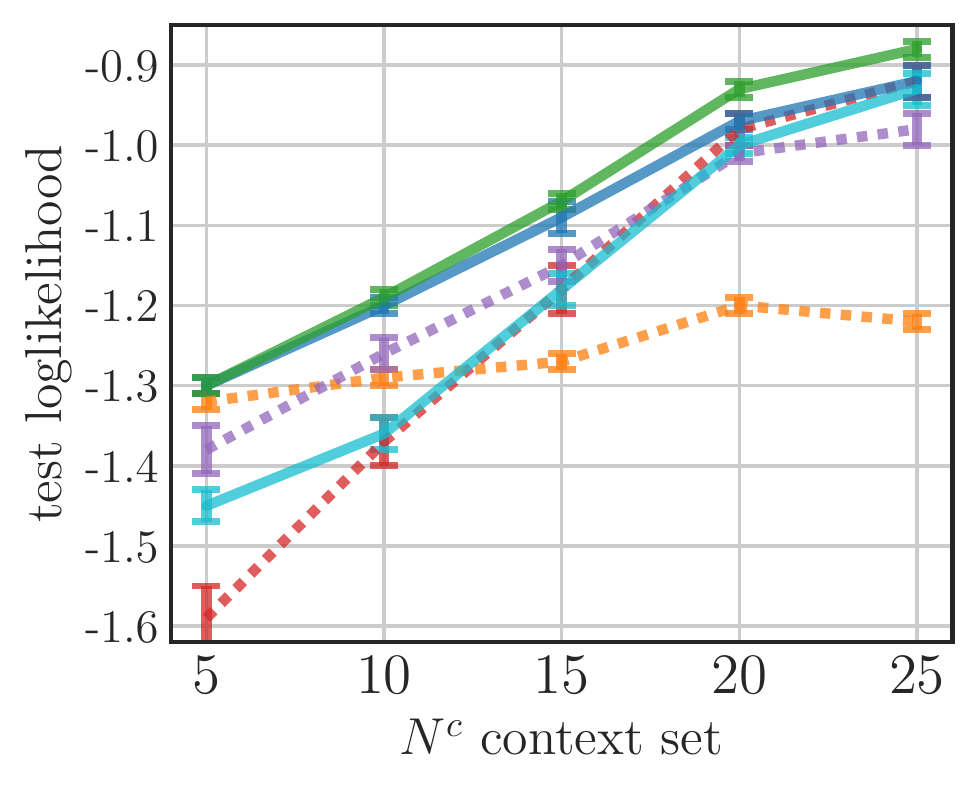}}  \hspace{0.5mm} 
\subfloat[\label{fig:exp5-1:small-h2} Sawtooth (out-range)]
{\includegraphics[width=0.24\linewidth]{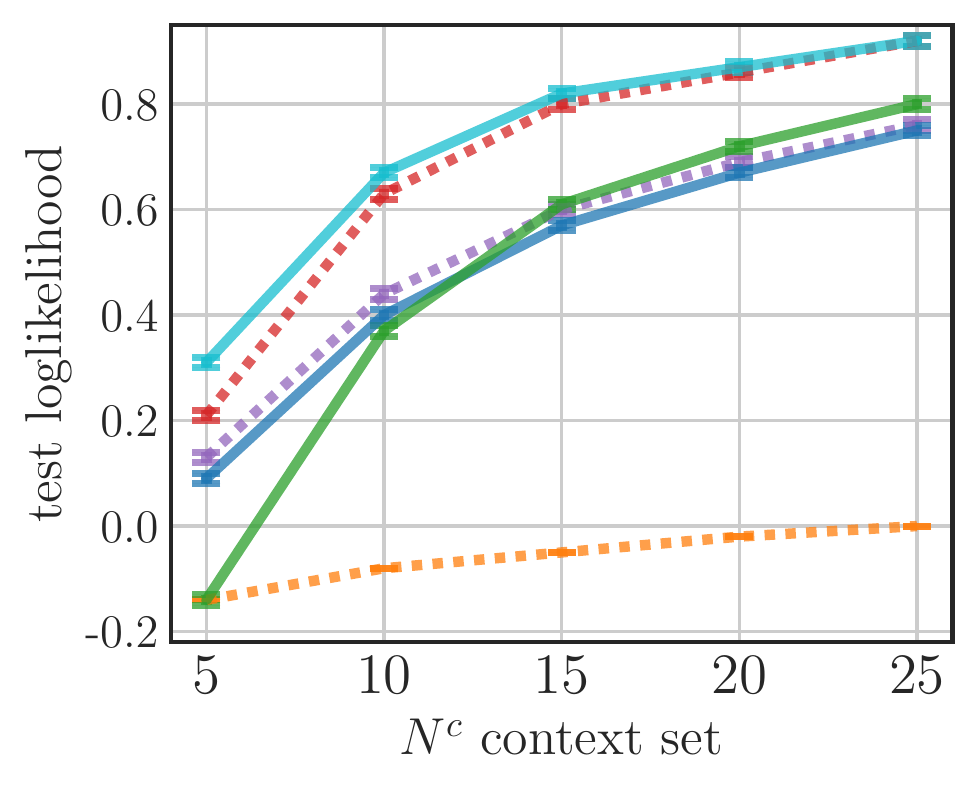}}   
\caption{Prediction result of each processes from training setting of \textb{large $N^{c}$} context points .   }
\label{fig:exp5-1:smallset_comparison}
\end{figure}
\vspace{-4mm}

\paragraph{Conclusion.} The proposed NP model ($Q=3,4,5$) using a Bayesian ConvDeepsets has shown superior prediction performances especially when training with a small number of context data points. When a more number of context points is allowed for training, the performance gap between ConvCNP and proposed method decreases as shown in \cref{fig:exp5-1:small-e,fig:exp5-1:small-e2} and \cref{fig:exp5-1:small-f,fig:exp5-1:small-f2}. 
%Also, when the number of data points 

%64 context set $\{D^{c}_{n}\}_{n=1}^{128}$ of each process

\paragraph{Prediction results for training a large number of context sets.}

Also, we report prediction results in \cref{fig:1d-singletask-prediction-large} and quantitative analysis of the trained parameters when the NP models are trained with the setting of a large number of context sets. We see that $\mathrm{p}_{\mathrm{nn}}(D^c)$ allocates the most of stationary priors as second spectral density (green) that overlaps most frequency region with the RBF prior (red). This results are quite different to the result of the setting of a small number of context sets (main). We believe that this implies why the RBF kernel smoother of ConvDeepsets could be effective when using a sufficient number of context set, and why the task-dependent stationary prior could be effective when using a small number of context set.

\begin{figure*}[h]
\subfloat[\label{fig:1d-singletask-a-large}  Spectral density]
{\includegraphics[width=0.19\linewidth  ,height=2.5cm ]{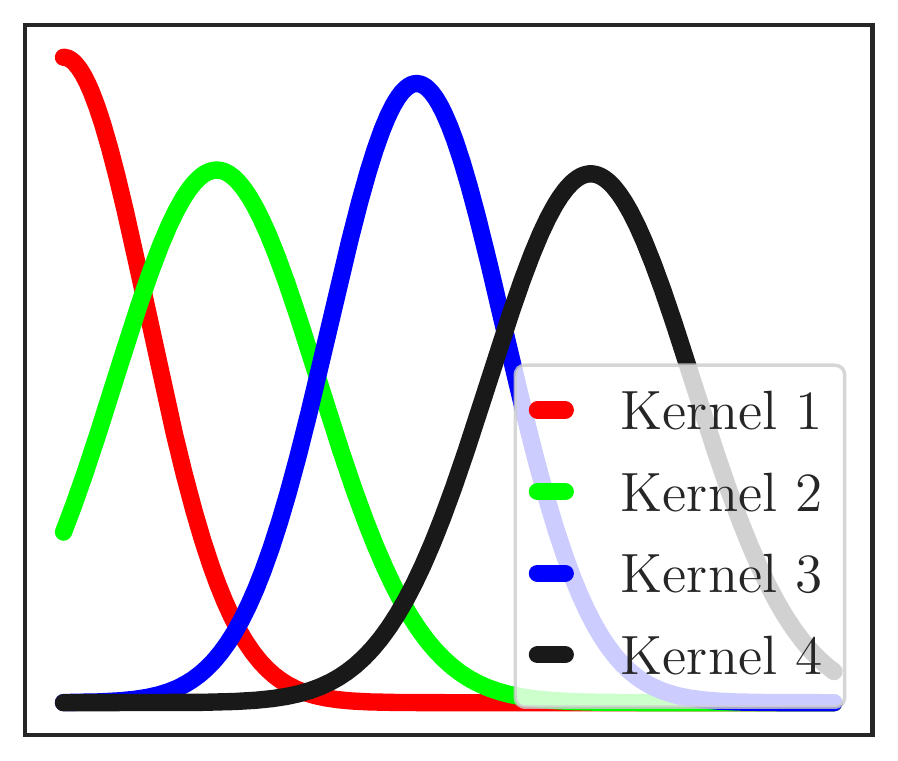}} \hspace{0.1mm}
\subfloat[\label{fig:1d-singletask-b-large} RBF]
{\includegraphics[width=0.19\linewidth ,height=2.5cm ]{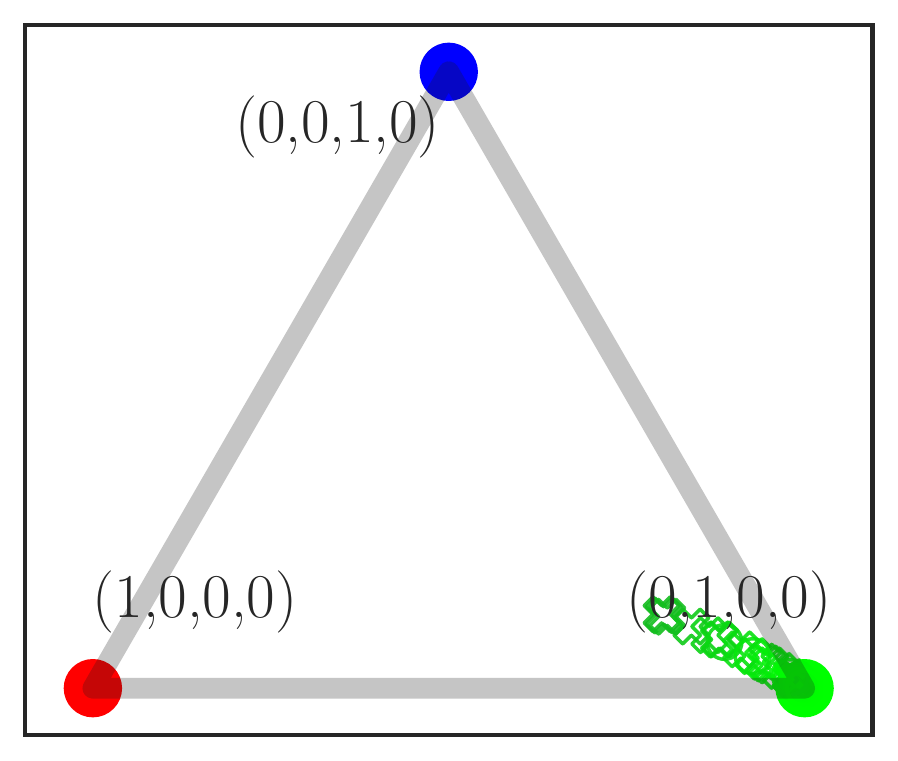}} \hspace{0.1mm}
\subfloat[\label{fig:1d-singletask-c-large} Matern-${\frac{5}{2}}$]
{\includegraphics[width=0.19\linewidth ,height=2.5cm ]{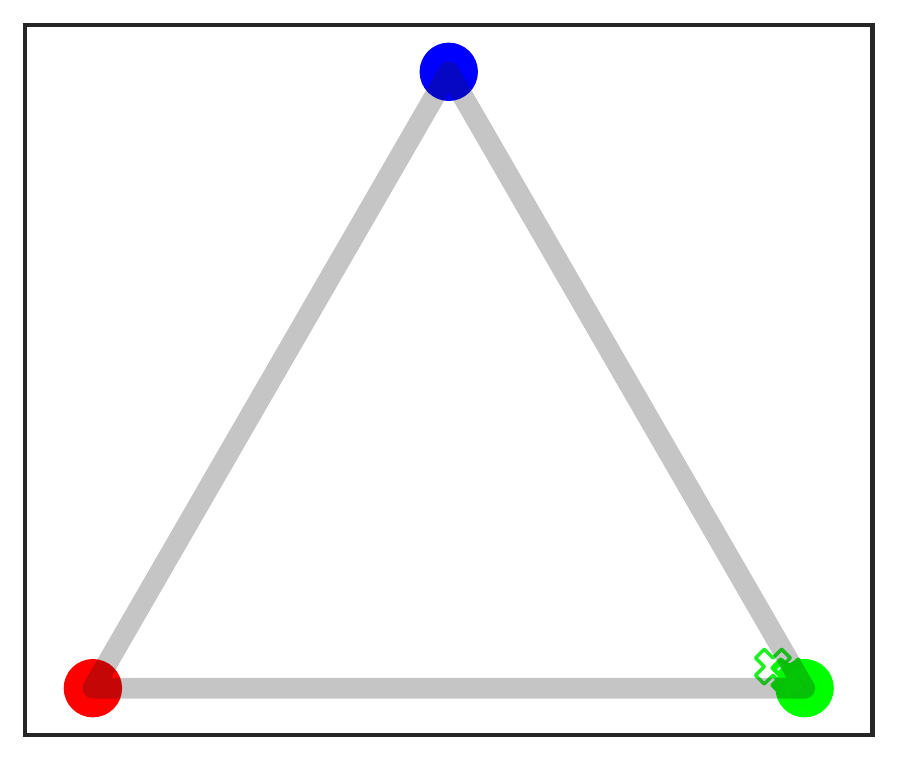}} \hspace{0.1mm}
\subfloat[\label{fig:1d-singletask-d-large} Weakly Periodic]
{\includegraphics[width=0.19\linewidth ,height=2.5cm ]{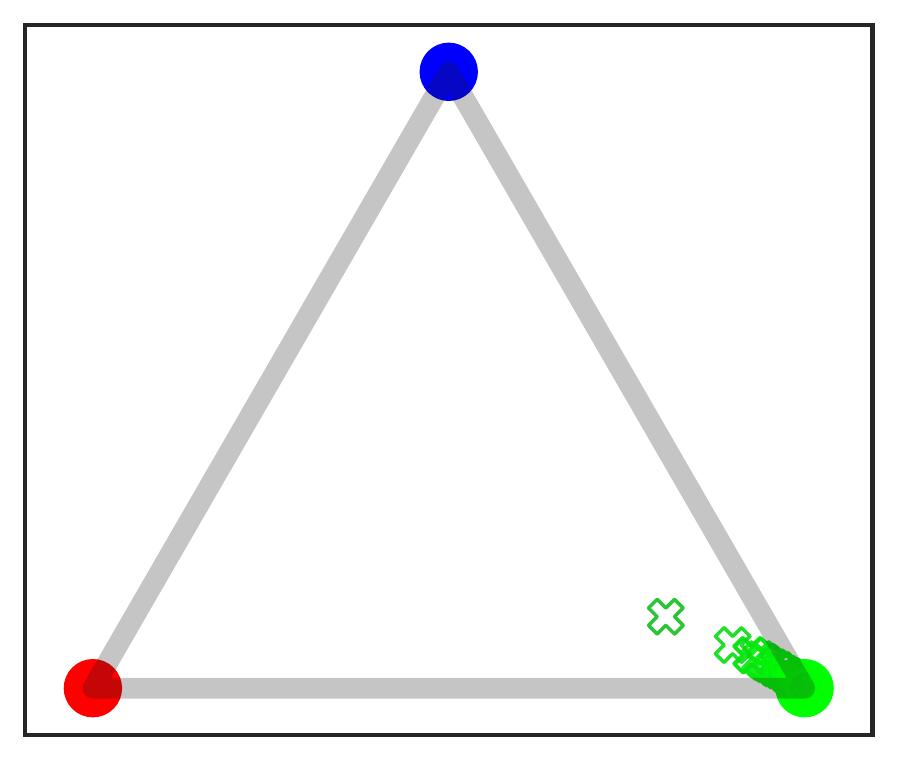}} \hspace{0.1mm}
\subfloat[\label{fig:1d-singletask-e-large} Sawtooth]
{\includegraphics[width=0.19\linewidth ,height=2.5cm ]{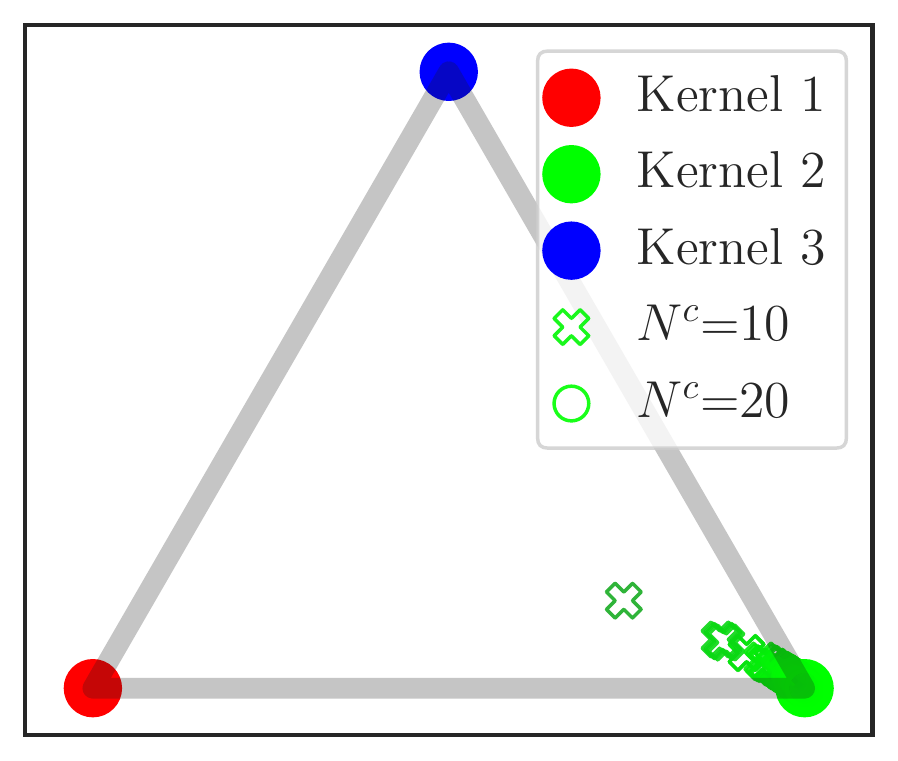}} 
\vspace{1mm}
\subfloat[\label{fig:1d-singletask-f-large} Predictive distribution of each baseline on each process ($N^c=15$) ]
{\includegraphics[width=0.99\linewidth  ]{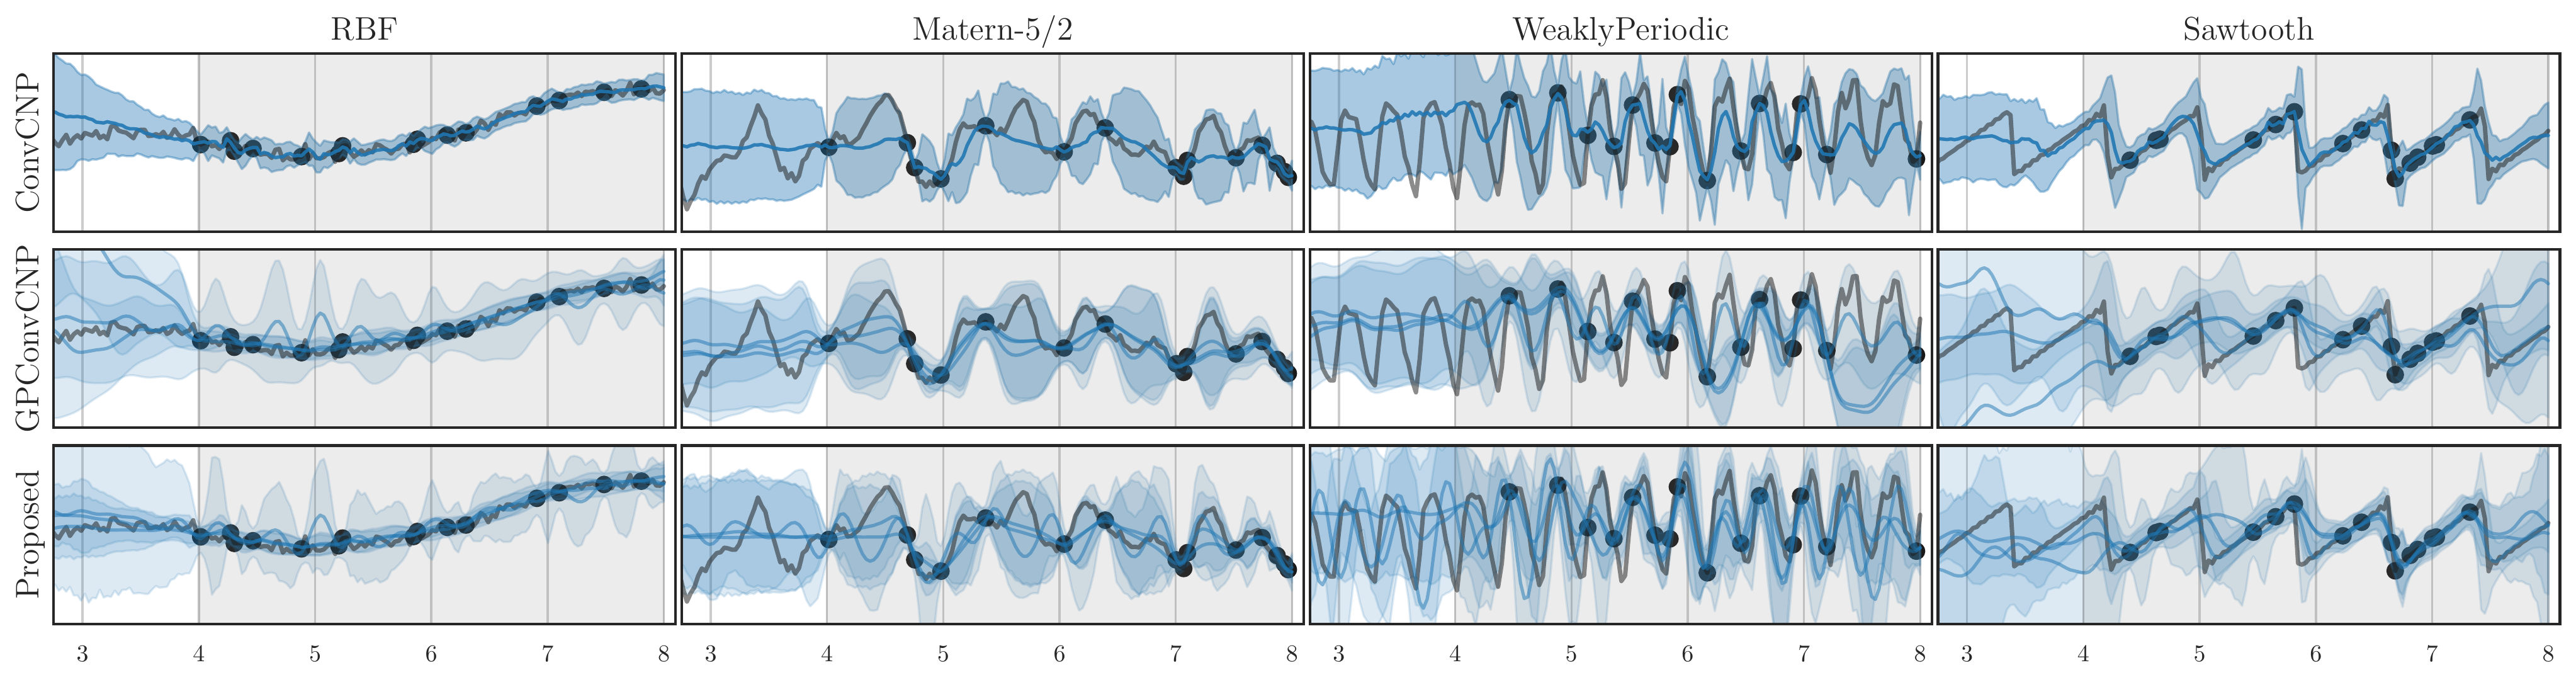}}
\caption{Stochastic processes modeling beyond training range (gray region $[4,8]$): \cref{fig:1d-singletask-a-large} denotes the trained spectral density with $Q=4$ kernels. \cref{fig:1d-singletask-b-large,fig:1d-singletask-c-large,fig:1d-singletask-d-large,fig:1d-singletask-e-large} denote the output of $\mathrm{p}_{\mathrm{nn}}(D^{c})$ for 128 context set $\{D^{c}_{n}\}_{n=1}^{128}$ of each process. \cref{fig:1d-singletask-f-large} shows the predictive distributions of the baselines on each process. 
}
\label{fig:1d-singletask-prediction-large}
\end{figure*}
\vspace{-3mm}

\paragraph{Validation error during training phase.} We report the averaged log likelihood evaluated on validation set during training; the validation set consists of $128\times 16$ tasks that have the equal number of task for each process.
\cref{fig:1d-singletask-val-small} and \cref{fig:1d-singletask-val-large} shows the validation metric over training epochs when using a small number of context set and large number of context set, respectively. In each epoch, we use $500 \times 16$ tasks for training. These figures imply that when the stationary priors are imposed well like $Q=4$, the propose model can achieve good performance while using the less number of training tasks.
\vspace{-3mm}
\begin{figure*}[h]
\centering
\subfloat[\label{fig:1d-singletask-val-small}  Small context set $N^{c}\sim U(5,25)$]
{\includegraphics[width=0.47\linewidth,height=4.5cm  ]{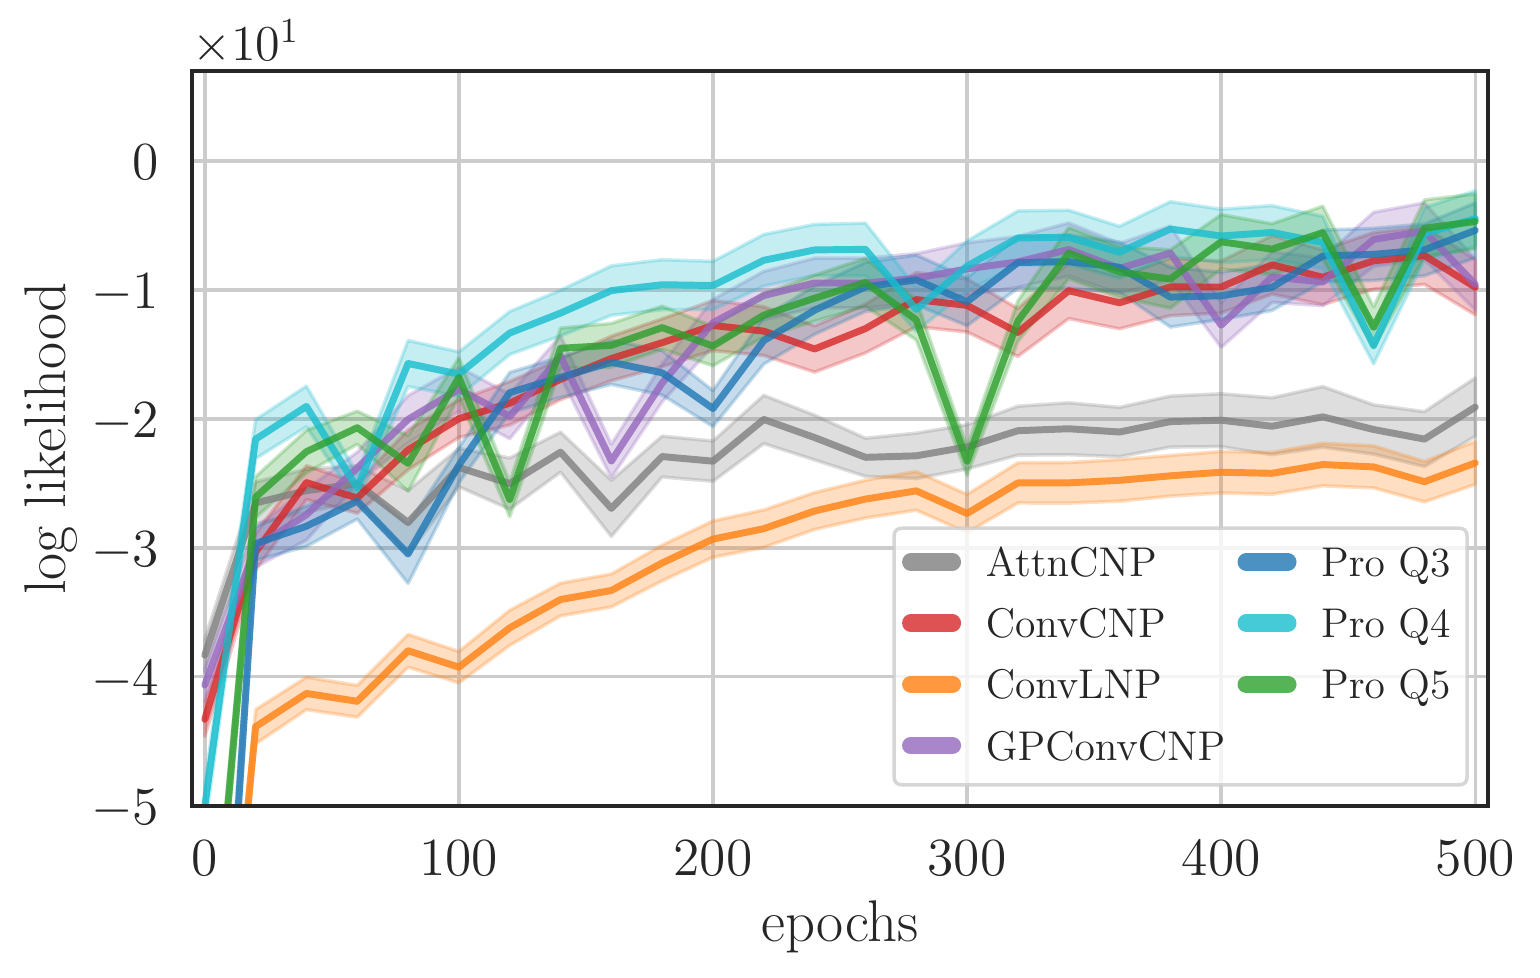}} \hspace{3mm}
\subfloat[\label{fig:1d-singletask-val-large} Large context set $N^{c}\sim U(10,50)$ ]
{\includegraphics[width=0.47\linewidth,height=4.5cm ]{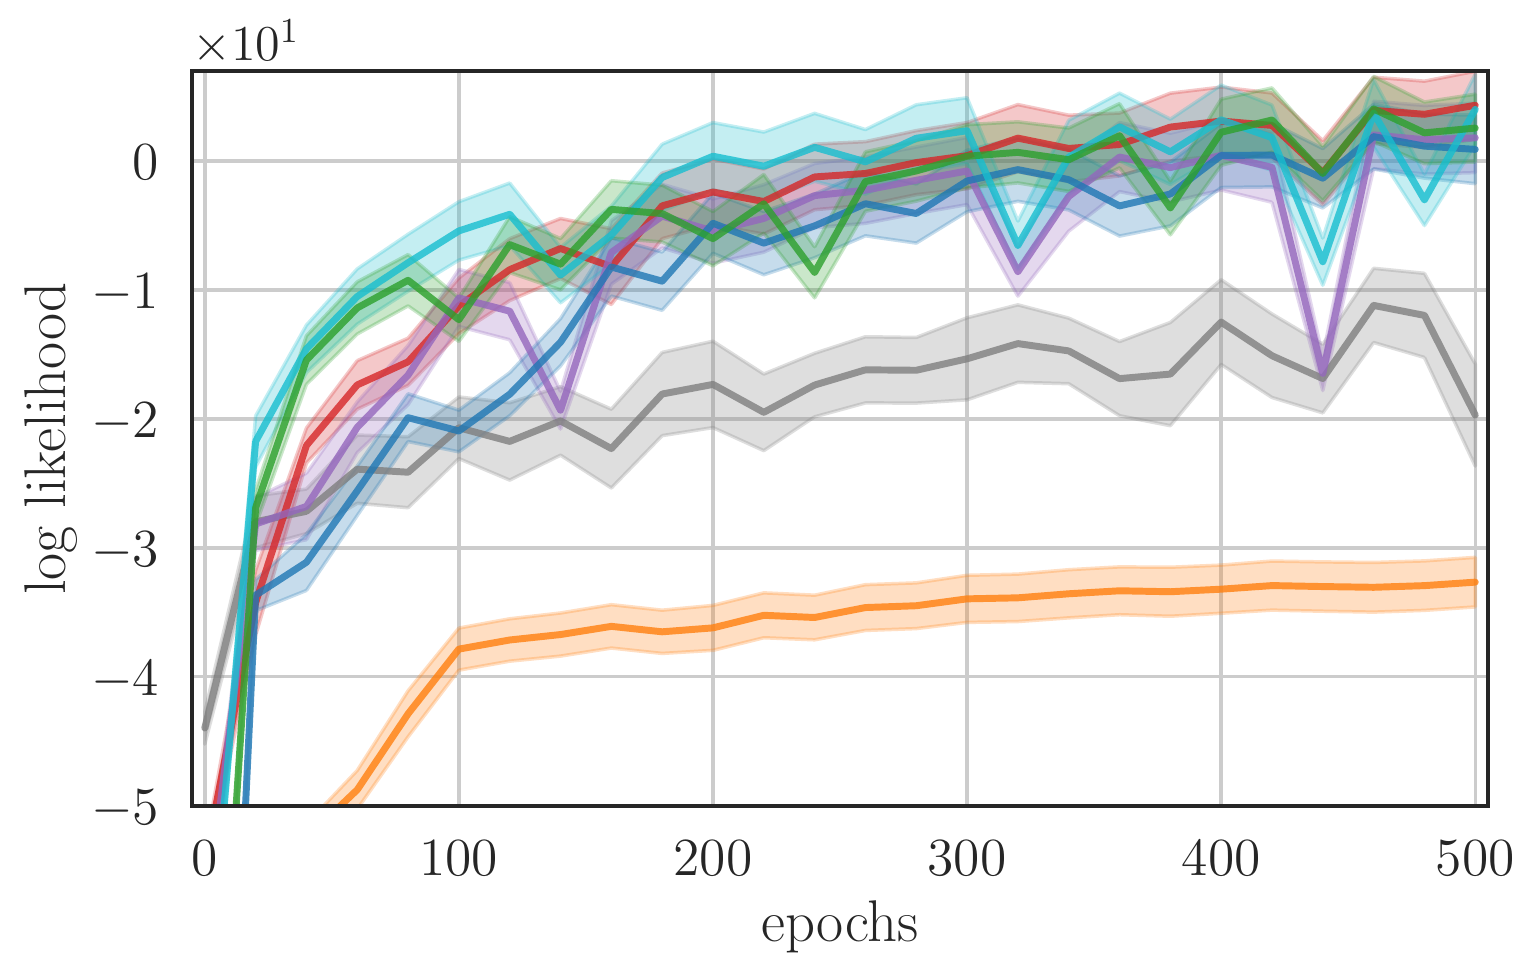}} 
\end{figure*}

\clearpage

\section{Further Details for Multi-Channel Regression Task}
\label{appendix:nd-regression-task}

% sine wave function $f_i$ has following function as \ 
%         \[
%             f_{i}(t) = \sin{(w_i + \theta_i) (t - \phi_i) } + \epsilon  \newline \\ 
%         \]

\subsection{Details for Datasets}

In this section, we consider two types of the multi-channel stationary process: (1) sinusoidal process and (2) GP using the Multi-output SM kernel (MOSM) \citeb{parra2017spectral}, that constructs the cross covariance function of two different processes based on Crammer theorem, i.e., a multi-channel extension of Bochner's theorem. Additionally, we consider two types of tasks for each process: (1) a simple task and a difficult task having more diversity to study how the task-dependent prior on functional representation affects the performance of the corresponding NP model depending on task diversity. We hypothesis that when the small number of data points is given for the task having more diversity, assigning a reasonable prior on functional representation could be helpful to solve the targeted tasks. Each process is described as follows:
\begin{itemize}[leftmargin=1em]
\item  \textbf{Sinusoidal-phase} : $i$-th channel context and target sets are constructed by randomly choosing $N^{(i)}_{c}$ data points and $N^{(i)}_{t}$ data points from the sampled function $f_i(t)$, that is represented as $$ f_{i}(t) = A_i\sin{ \left( 2\pi w_i (t - \phi_i) \right)} + \epsilon, \hspace{10mm}  i=1,2,3  \hspace{3mm}, $$ where $A_i$ denotes $i$-th channel amplitude parameter, $w_i$ denotes $i$-th channel frequency parameter, $ \phi_i$ denotes $i$-th channel phase parameters, and $\epsilon$ is random noise satisfying $\epsilon \sim N(0,0.1^2)$. For frequency parameters, we set $w_1 = 2.1, w_2 = 4.1$, and $w_3=6.1$. For the amplitude, we set $A_1=1 + a, A_2=2 + a$, and $A_3=3 + a$ by using a random amplitude $a \sim \mathcal{U}([-25,0.25])$. For the phase parameter, we consider random phase $\tau_{1} \sim \mathcal{U}([-1,1]), \tau_{2} \sim \mathcal{U}([-1.5,0.5])$, and $\tau_{3} \sim \mathcal{U}([-2,0])$. The random parameters for amplitude $a$ and phases $\{\tau_1,\tau_2,\tau_3\}$ are randomly sampled for each task.

\item  \textbf{Sinusoidal-all}  : $i$-th channel context and target sets are constructed by randomly choosing $N^{(i)}_{c}$ data points and $N^{(i)}_{t}$ data points from the sampled function $f_i(t)$, that is represented as  that is represented as $$ f_{i}(t) = A_i\sin{ \left( 2\pi (w_i + \theta_i) (t - \phi_i) \right)} + \epsilon  \hspace{10mm}  i=1,2,3, $$ where $\theta_i$ denotes $i$-th channel random frequency parameter. In this generation procedure, we consider random frequency parameters additionally; we first sample $\theta \sim \mathcal{U}([0,5])$, and set $\theta_1 = \theta, \theta_2 = 2\theta$, and $\theta_3 = 3\theta$. This is intended to let the task of this process have more diversity. For other parameters $\{A_i,w_i,\phi_i\}_{i=1}^{3}$, we set the same setting as described in \textbf{Sinusoidal}.

% k_{i j}(\tau) = \displaystyle\sum_{q=1}^{Q} \alpha_{ij}^{(q)} \exp \left ( - \frac{1}{2} (\tau + \theta_{ij}^{(q)})^{\top} \Sigma_{ij}^{(q)} (\tau + \theta_{ij}^{(q)}) \right ) \cos \left((\tau + \theta_{ij}^{(q)})^{\top} \mu_{ij}^{(q)} + \phi_{ij}^{(q)}  \right) 
% where $\alpha_{ij}^{(q)} = w_{ij}^{(q)} (2\pi)^{\frac{n}{2}} | \Sigma_{ij}^{(q)} |^{1/2}  $ and the superindex $(\cdot)^{(q)}$ denotes the parameter of the $q^\text{th}$ component of the spectral mixture. 

%$\Sigma_1=\mathrm{Diag}([0.5])$, $\Sigma_2=0.5$, $\Sigma_3=\mathrm{Diag}([0.5])$ for covarinace parameters
%http://143.248.92.34:8888/lab/workspaces/auto-K/tree/UAI22_CCCNP_from108/dataset_multitask_1d.py
\item  \textbf{MOSM}: : $i$-th channel context and target sets are constructed by randomly choosing $N^{(i)}_{c}$ data points and $N^{(i)}_{t}$ data points from $i$-th channel function of the multi-output function sampled from Gaussian Process (GP) with the following kernel function $\{k_{ij}\}_{i,j=1}^{3}$ of which the cross kernel $k_{ij}$ between $i$-th channel and $j$-th channel is represented as $$k_{ij}(x, x') = \exp \left ( - \frac{1}{2} ( x-x' + \theta_{ij})^{\top} \Sigma_{ij} (x-x' + \theta_{ij}) \right ) \cos \left( 2\pi(x-x' + \theta_{ij})^{\top} \mu_{ij} + \phi_{ij}  \right), $$
where $\mu_{i j}  =  (\Sigma_{i} + \Sigma_{j})^{-1} (\Sigma_{i} \mu_{j} + \Sigma_{j} \mu_{i})$, $\Sigma_{ij}  = 2\Sigma_{i}(\Sigma_{i} + \Sigma_{j})^{-1} \Sigma_{j}$, $\phi_{ij} = \phi_i - \phi_j$, and $\phi_{ij} = \phi_i - \phi_j$ when $\mu_{i}$ denote $i$-th channel mean parameter, $\Sigma_{i}$ denotes $i$-th channel covariance parameter, $\theta_{i}$ denotes $i$-th channel delay parameter, and $\phi_i$ denotes $i$-th channel phase parameter, respectively. In this experiment, we set 
$\mu_1=0.1$, $\mu_2=3.0$, $\mu_3=5.0$ for mean parameters and $\Sigma_1=0.1$, $\Sigma_2=0.1$, $\Sigma_3=0.1$ for covariance parameters. We set $\theta_i=1$ with $i=1,2,3$ for delay parameters and $\phi_i=0$ with $i=1,2,3$ for phase parameters. We employ the following implementation \citeb{mogptk} \footnotemark{\footnotetext[3]{\url{https://github.com/GAMES-UChile/mogptk}}}.

\item  \textbf{MOSM-varying}: $i$-th channel context and target sets are constructed by randomly choosing $N^{(i)}_{c}$ data points and $N^{(i)}_{t}$ data points from $i$-th channel function of the multi-output function as described in $\textbf{MOSM}$ with different hyperparameter setting. We consider random mean parameters to generate the diverse tasks. We consider the random mean parameters; we first sample perturb noises $\{n_j\}_{j=1}^{3} \sim N(0,.5^{2}I)$ every task, and then set $\mu_1=0.1 + n_1$, $\mu_2=3.0 + n_2$, $\mu_3=5.0 + n_3$, which are reinitialized every task. Since this trick generates the data points observed from a new multi-output stationary process every task by considering the different cross correlation function between different two processes, the generated tasks are more diverse.

\end{itemize}

\subsection{Details for Tasks of Training, Validation, and Test }

In this experiment, we set the training range \textb{$[0,3]$} and test range \textb{$[3,6]$} (outside of training range). For training, we construct the context sets and target sets by sampling the data points on training range. Then, we evaluate the trained models with context sets and target sets, that are sampled on test range as described in \cref{subsubsec:prepare_sets}.

We consider the following number of data points for training, validation, and test: 
\begin{itemize}[leftmargin=1em]
    \vspace{-2mm}
    \item For training, we randomly sample \textb{$N_c \sim \mathcal{U}([5,25])$} as the number of context data points, and randomly sample \textb{$N_t \sim \mathcal{U}([N_c,50])$} as the number of target data points for each task. We use \textb{$500{\times}50{\times}16$} tasks for training through 500 batches. For validation, we set $N_c$ context data points and $N_t$ target data points as done in training, and use \textb{$64{\times}16$} tasks for validation to choose the parameters of the trained models. For test, we consider the varying \textb{$N_c \in \{5,10,15,20,25,30\}$} context data points and $N_t=50$ target data points per a task, and use \textb{$64{\times}16$} tasks per given $N_c$ context points to study how the number of context data points affects the predictive performance of the trained models using the parameters obtained in validation procedure.  
\end{itemize}

\subsection{Details for Hyperparameters.}

%\paragraph{Hyperparameters of Kernels.}

% For stationary kernels, we set $\mu_{1}=[0.0,0.0]$ and $\sigma_{1}=[0.5,0.5]$ for $Q=1$.

% For $Q=2$, we set $\mu_{1}=[0.0,0.0],\mu_{2}=[2.0,0.0],\mu_{3}=[0.0,2.0],$ and $\mu_{4}=[2.0,2.0]$ and $\sigma_{q}=[0.5,0.5]$ for $q=1,..,4$.

% For the number of spectral points, we use $l=10$ in \textb{Eq. (14)}.

% For the number of sample function, we use $N=4$ in \textb{Eq. (19)}.

% For the prior hyperparameter of approximate scheme $\alpha$, we use $\alpha \in \{.05,0.1\}$.

% For training, we  use ADAM optimizer \citeb{kingma2014adam} with learning rate $5e\text{-}4$ and weight decay $1e\text{-}4$. 

% For the regularizer hyperparameter $\beta$ in \textb{Eq. (21)}, we set $\beta=0.1$ for the proposed method.

For the hyperparameter of RBF kernels used for ConvCNP and ConvLNP, we conduct the experiment with  $l\in\{0.1,0.5,1.0\}$, and set the lengthscale $l=0.1$ for both models obtaining the best performance out of those candidates.

For the hyperparameter of GPConvCNP, we set $l=1.0$ for each channel respectively. 

For the hyperparameter of the proposed method, we use $5$ basis stationary kernels ($Q=5$), and set $\mathrm{HZ}_{\mathrm{max}}=Q$. Then, we space the frequency range $[0,\mathrm{HZ}_{\mathrm{max}}]$ linearly, and set each centered value as $\mu_q$ with $\mu_1=0 \leq ..\leq \mu_5$, and set
$\sigma_q = 0.5(\mu_{2} -\mu_{1})$ for $q=1,..,5$. For the noise parameter $\sigma^{2}_{\epsilon}$, we set $\sigma_{\epsilon}=1e\text{-}{2}$.

For the number of spectral points, we use $l=10$ in \textb{Eq. (14)}.

For the number of sample function, we use $N=10$ in \textb{Eq. (19)}.

For training, we  use ADAM optimizer \citeb{kingma2014adam} with learning rate $5e\text{-}4$ and weight decay $1e\text{-}4$. 

For the regularizer hyperparameter $\beta$ in \textb{Eq. (21)}, we set $\beta=0.1$ for the proposed method.

\subsection{Additional Results}
%We report additional results obtained in experimental section 5.2 (main). 

\paragraph{Results of Sinusoidal dataset.}

For completeness of results, we report additional prediction results of other baseline on theh tasks of Sinusoidal-all as shown in \cref{fig:nd-multitask-f,fig:nd-multitask-g}.

\vspace{-2mm}
\paragraph{Results of MOSM dataset.} We report additional results on GP-MOSM dataset. 
\cref{fig:nd2-multitask-a,fig:nd2-multitask-b} describes the mean and one-standard error of the log likelihood for 1024 tasks (beyond training range); \cref{fig:nd2-multitask-a} shows the result of the less diversity task (varying phase), and \cref{fig:nd2-multitask-b} corresponds to that of the high diversity (varying amplitude, frequency, and phase). These figures show that the proposed method could model processes well on both less and more diverse tasks. 

\cref{fig:nd2-multitask-c} shows the trained spectral density of $\{k_{q}\}_{q=1}^{5}$ on high diversity task. \cref{fig:nd2-multitask-d,fig:nd2-multitask-e} denote the parameters $\mathrm{p}_{\mathrm{nn}}(D^{c})$ for two tasks (top and bottom), and THE corresponding predictions of the proposed method.  \cref{fig:nd2-multitask-f,fig:nd2-multitask-g} show the prediction results of ConvCNP and GPConvCNP, respectively.

\begin{figure*}[t]
\centering
\subfloat[\label{fig:nd-multitask-a} Sinusoidal-phase ]
{\includegraphics[width=0.23\linewidth]{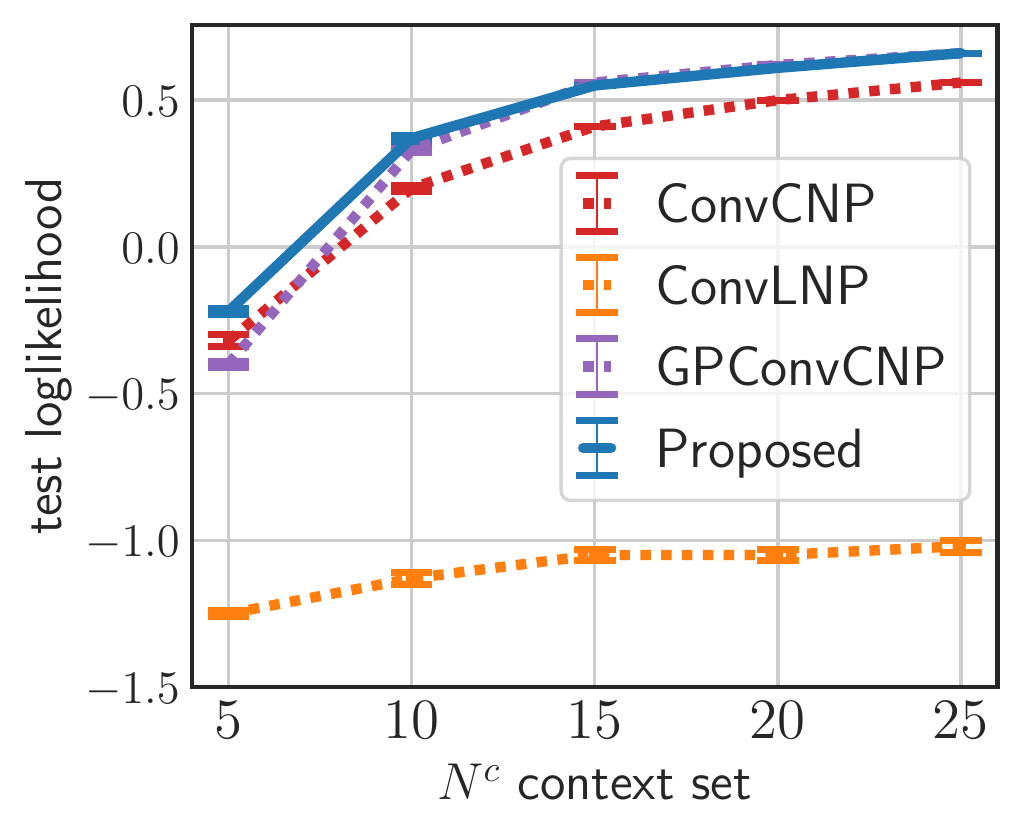}} 
\hspace{.1mm}
\subfloat[\label{fig:nd-multitask-b} Sinusoidal-all ]
{\includegraphics[width=0.23\linewidth]{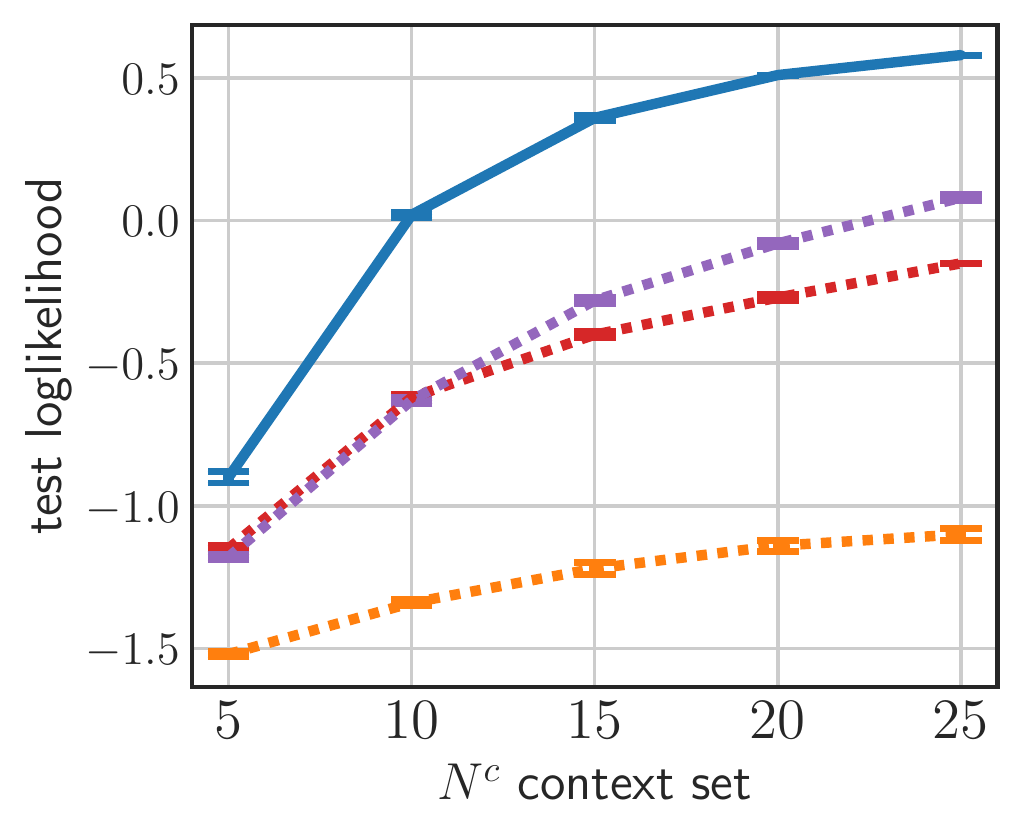}} 
\hspace{3mm}
\subfloat[\label{fig:nd-multitask-c} Spectral density]
{\includegraphics[width=0.23\linewidth]{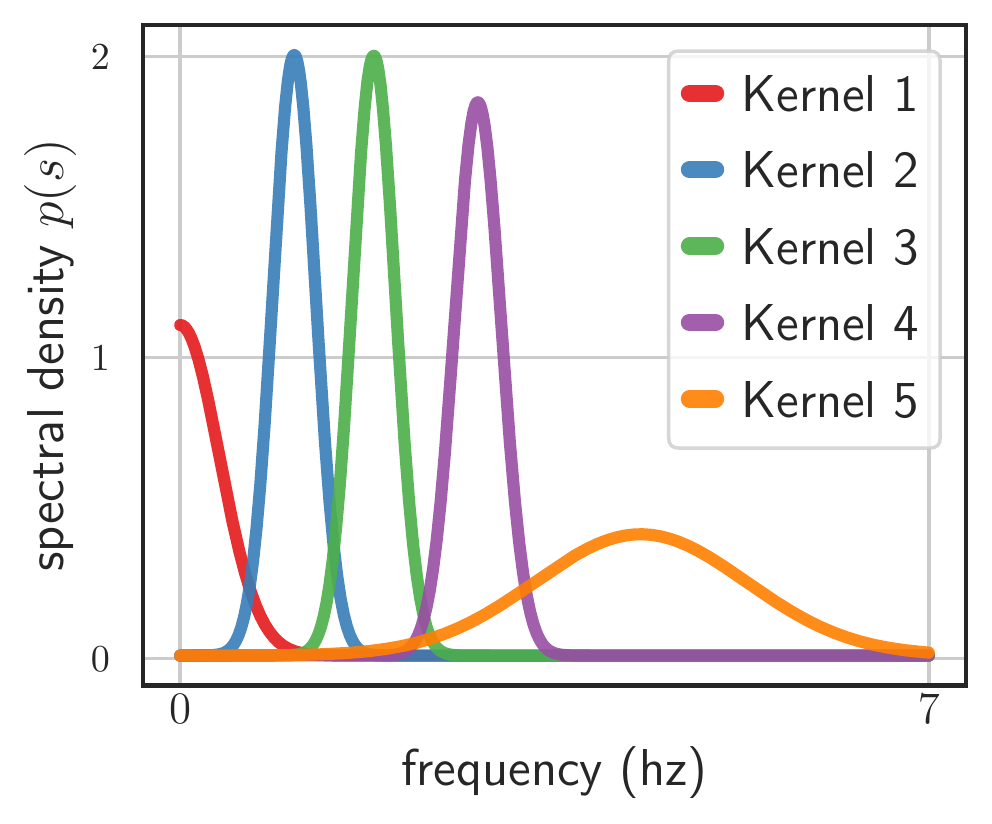}}
\hspace{.1mm}
\subfloat[\label{fig:nd-multitask-d} Task-dependent prior]
{\includegraphics[width=0.23\linewidth]{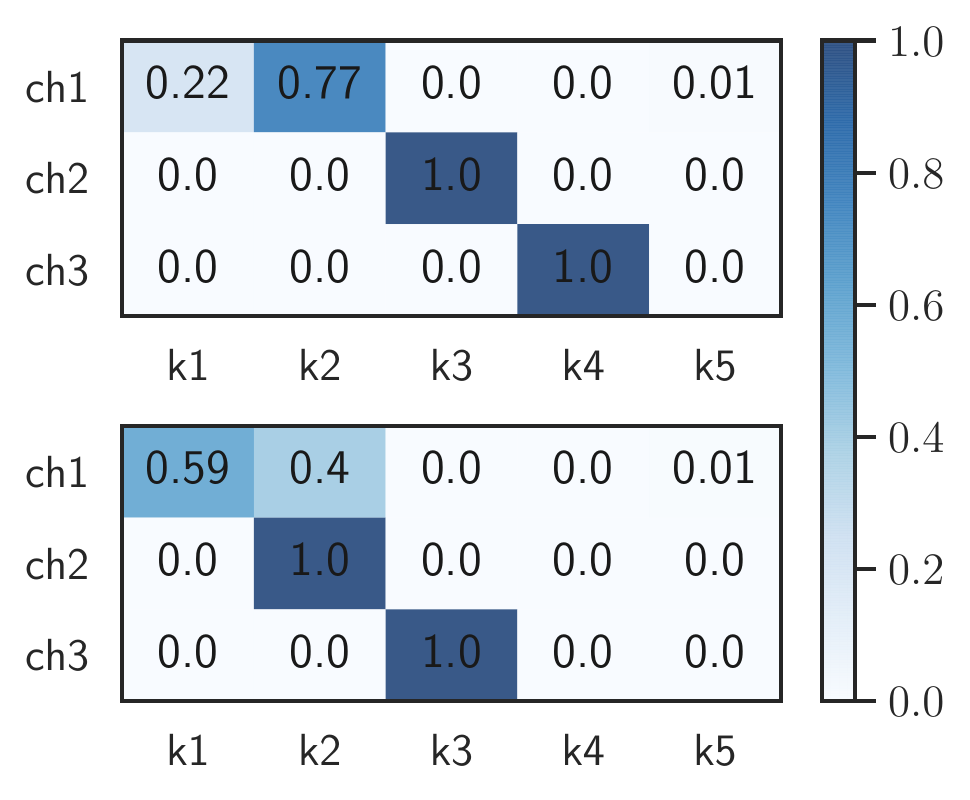}}
\vspace{4mm}
\subfloat[\label{fig:nd-multitask-e} Proposed: Prediction for 2 different tasks ($N^{c}=10$) of the Sinusoidal-all  ]
{\includegraphics[width=0.98\linewidth]{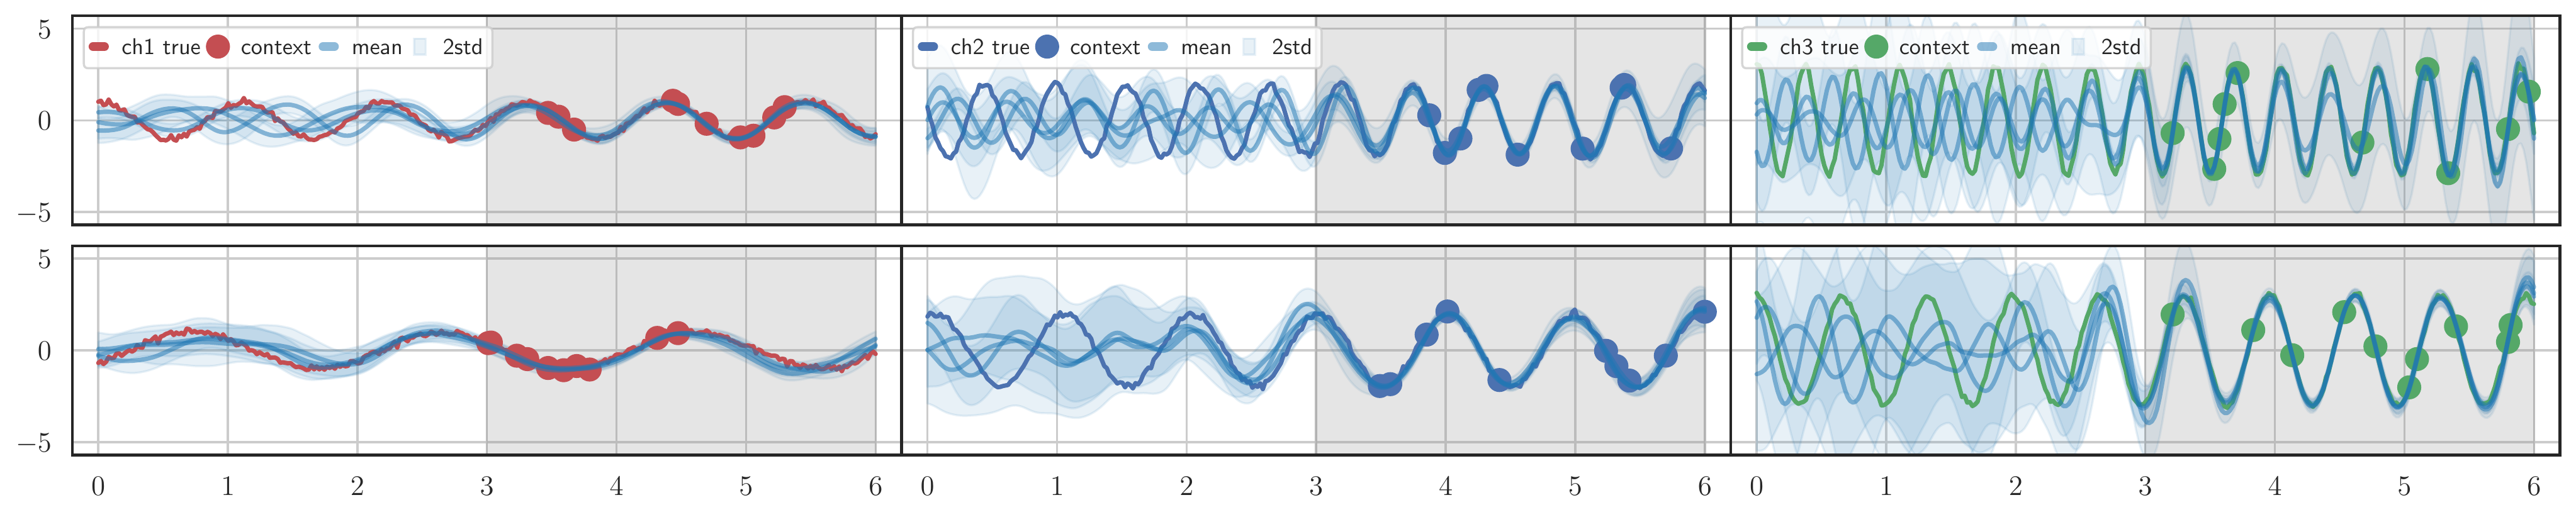}} 
\vspace{2mm}
\subfloat[\label{fig:nd-multitask-f} ConvCNP: Prediction for 2 different tasks ($N^{c}=10$) of the Sinusoidal-all  ]
{\includegraphics[width=0.98\linewidth]{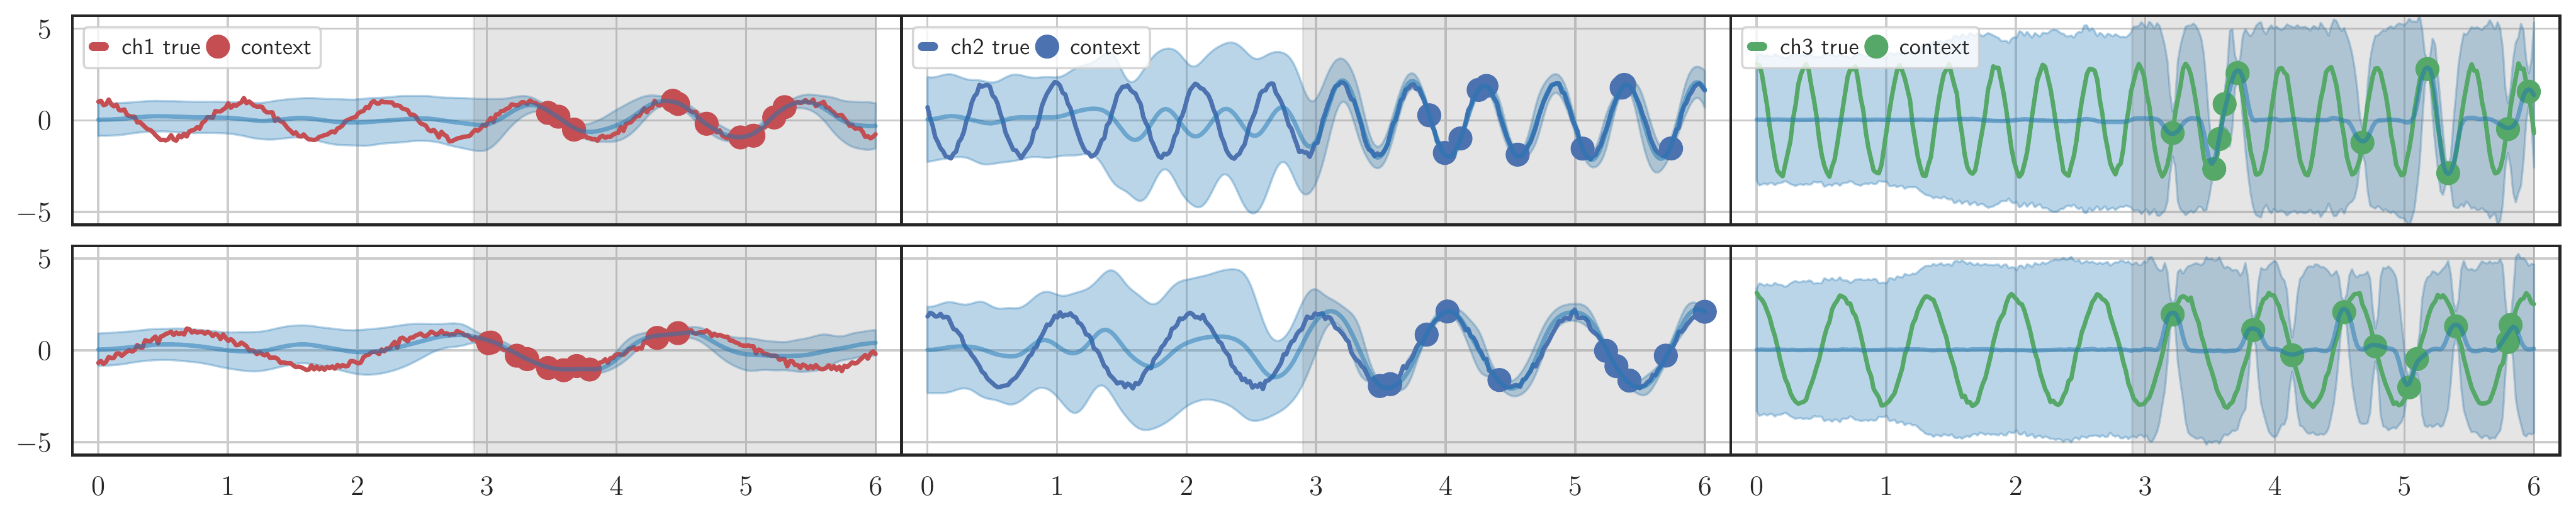}} 

\vspace{2mm}
\subfloat[\label{fig:nd-multitask-g} GPConvCNP: Prediction for 2 different tasks ($N^{c}=10$) of the Sinusoidal-all  ]
{\includegraphics[width=0.98\linewidth]{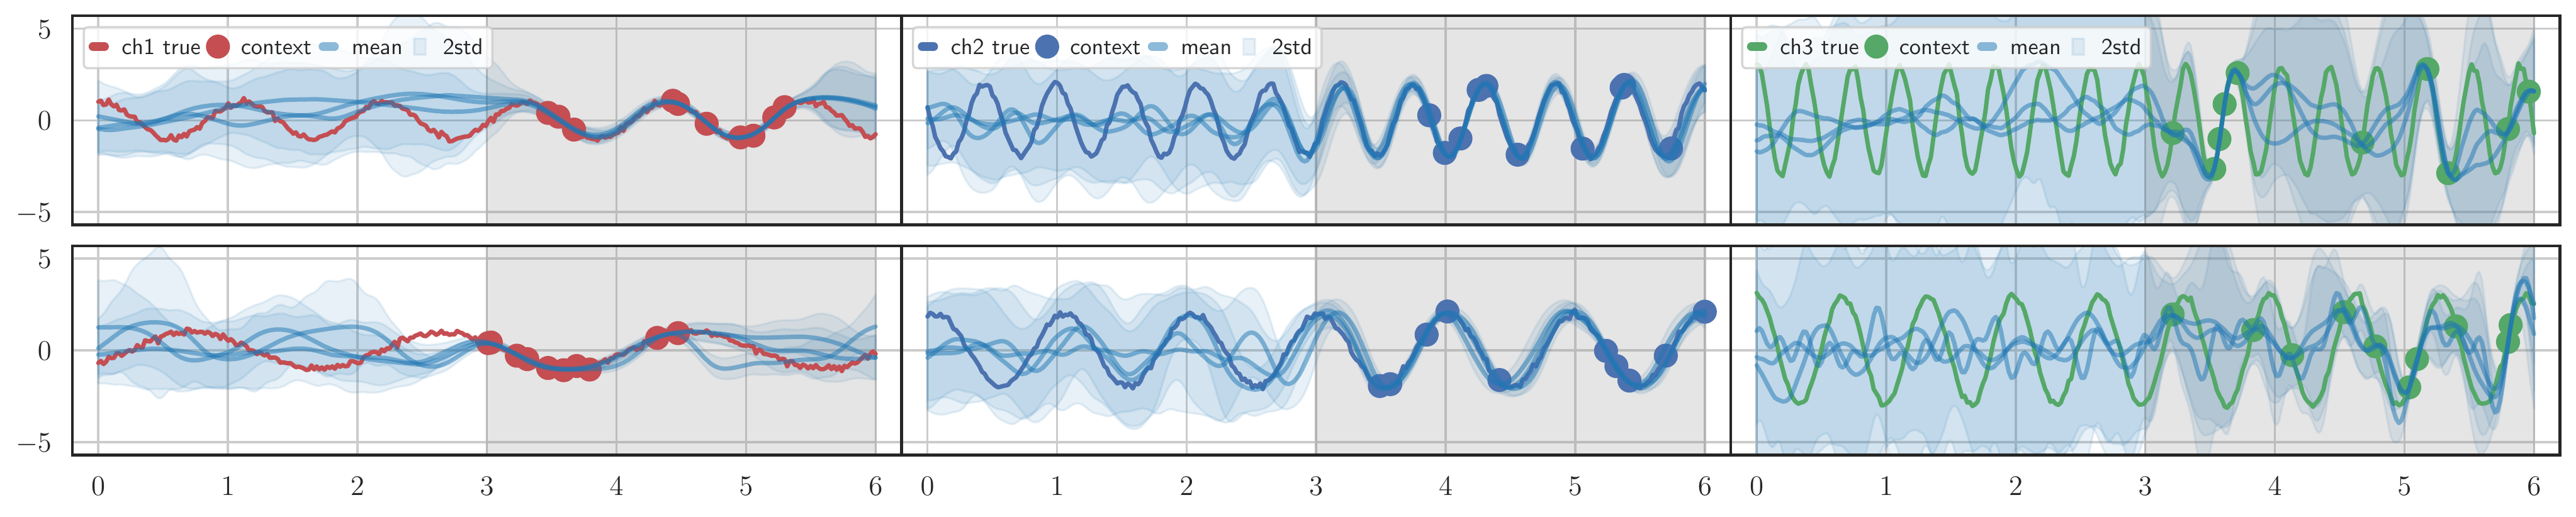}} 
\caption{3-channel sinusoidal processes modeling: \cref{fig:nd-multitask-a,fig:nd-multitask-b} denotes test likelihood on sinusoidal processes having different task diversity. \cref{fig:nd-multitask-c} denote the trained spectral density $\{p_q(s)\}_{q=1}^{5}$ for the Sinusoidal-all process, and \cref{fig:nd-multitask-d,fig:nd-multitask-e} show the chosen prior and corresponding prediction for 2 tasks; as the context sets having small frequency characteristics are given (from first to second row in \cref{fig:nd-multitask-e}), the stationary prior is imposed differently (from top to bottom in \cref{fig:nd-multitask-d}). \cref{fig:nd-multitask-f,fig:nd-multitask-g} show the prediction results using the same context set with \cref{fig:nd-multitask-e}.
}
\label{fig:nd-multitask-pred}
\end{figure*}

\begin{figure*}[t]
\centering
\subfloat[\label{fig:nd2-multitask-a} MOSM ]
{\includegraphics[width=0.23\linewidth]{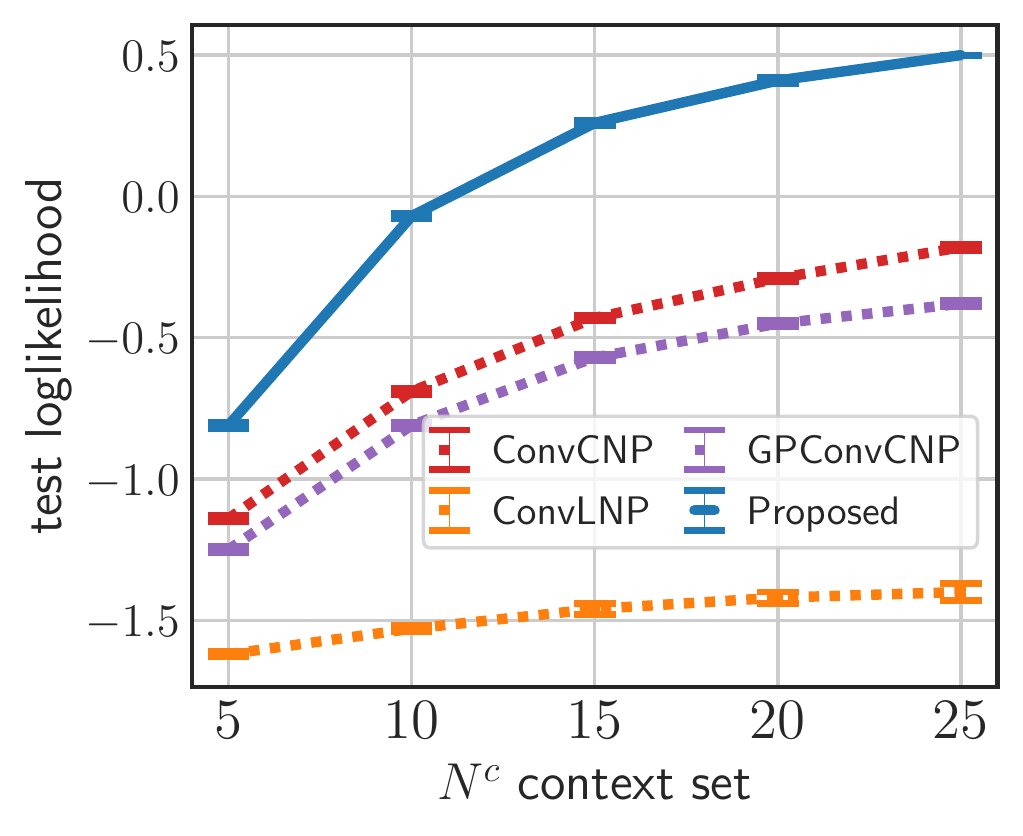}} 
\hspace{.1mm}
\subfloat[\label{fig:nd2-multitask-b} MOSM-varying ]
{\includegraphics[width=0.23\linewidth]{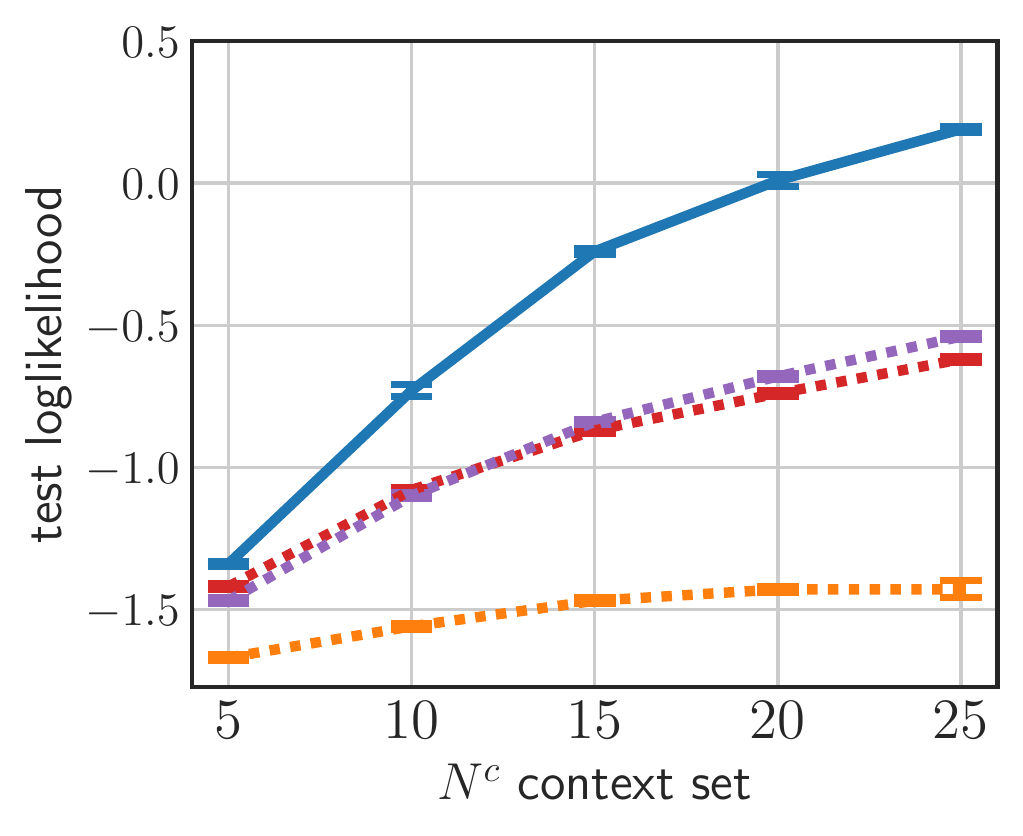}} 
\hspace{3mm}
\subfloat[\label{fig:nd2-multitask-c} Spectral density]
{\includegraphics[width=0.23\linewidth]{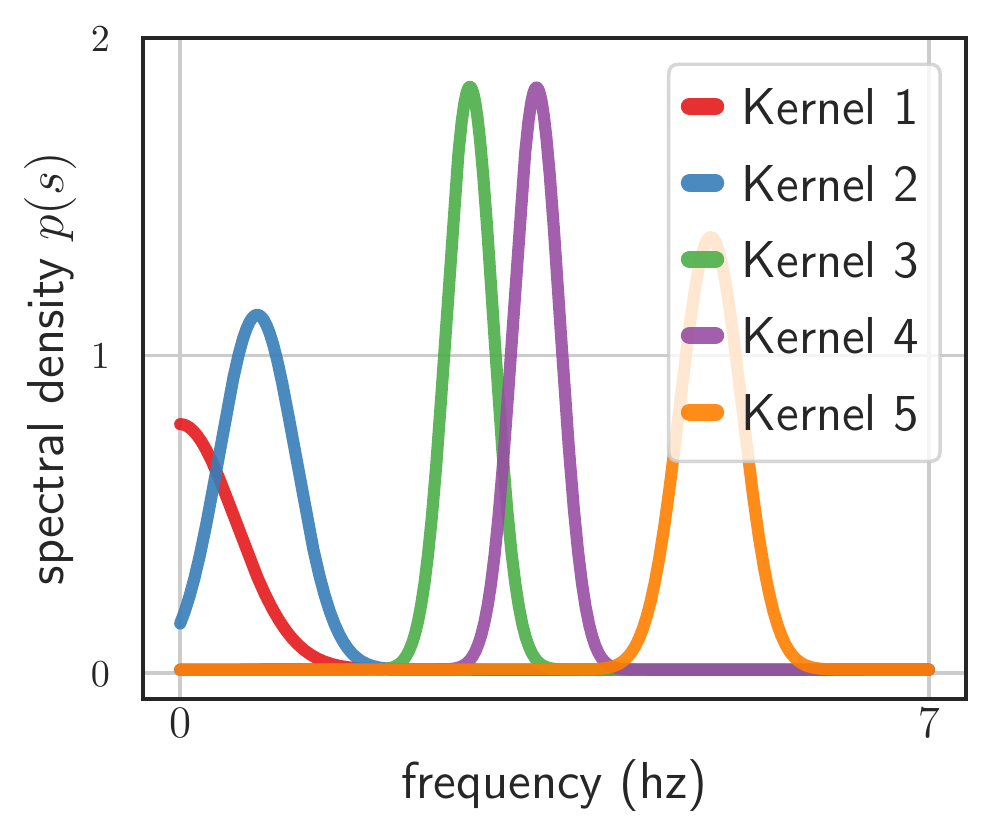}} 
\hspace{.1mm}
\subfloat[\label{fig:nd2-multitask-d} Task-dependent prior]
{\includegraphics[width=0.23\linewidth]{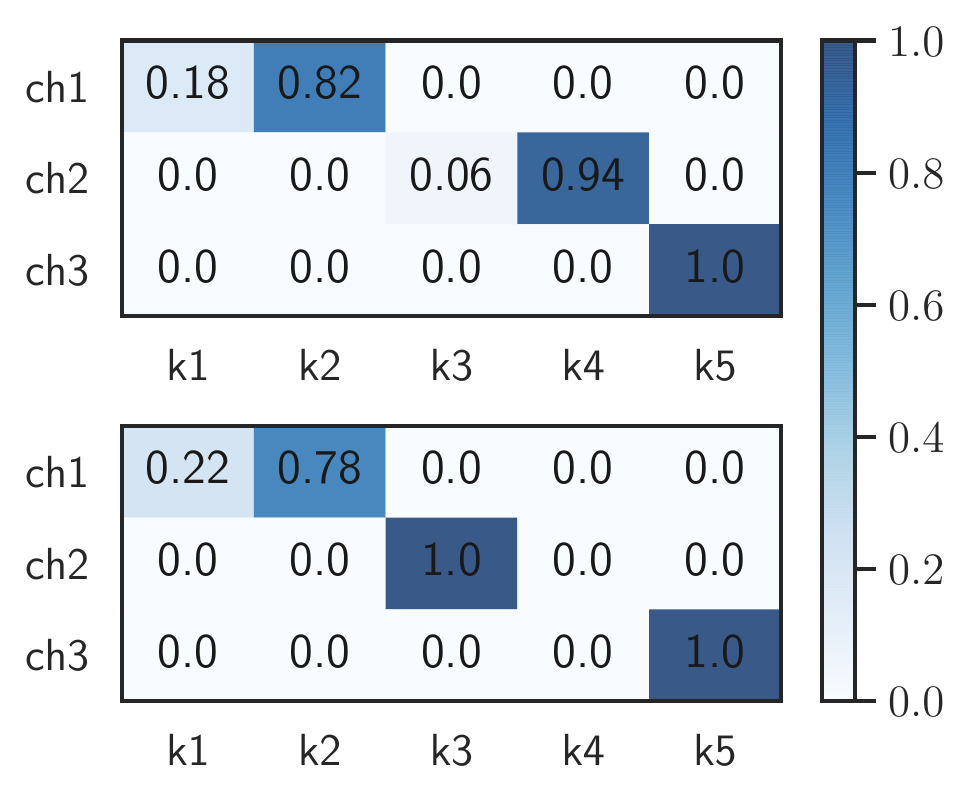}} 

\vspace{4mm}
\subfloat[\label{fig:nd2-multitask-e} Proposed: Prediction for 2 different tasks ($N^{c}=10$) of the MOSM-varying  ]
{\includegraphics[width=0.98\linewidth]{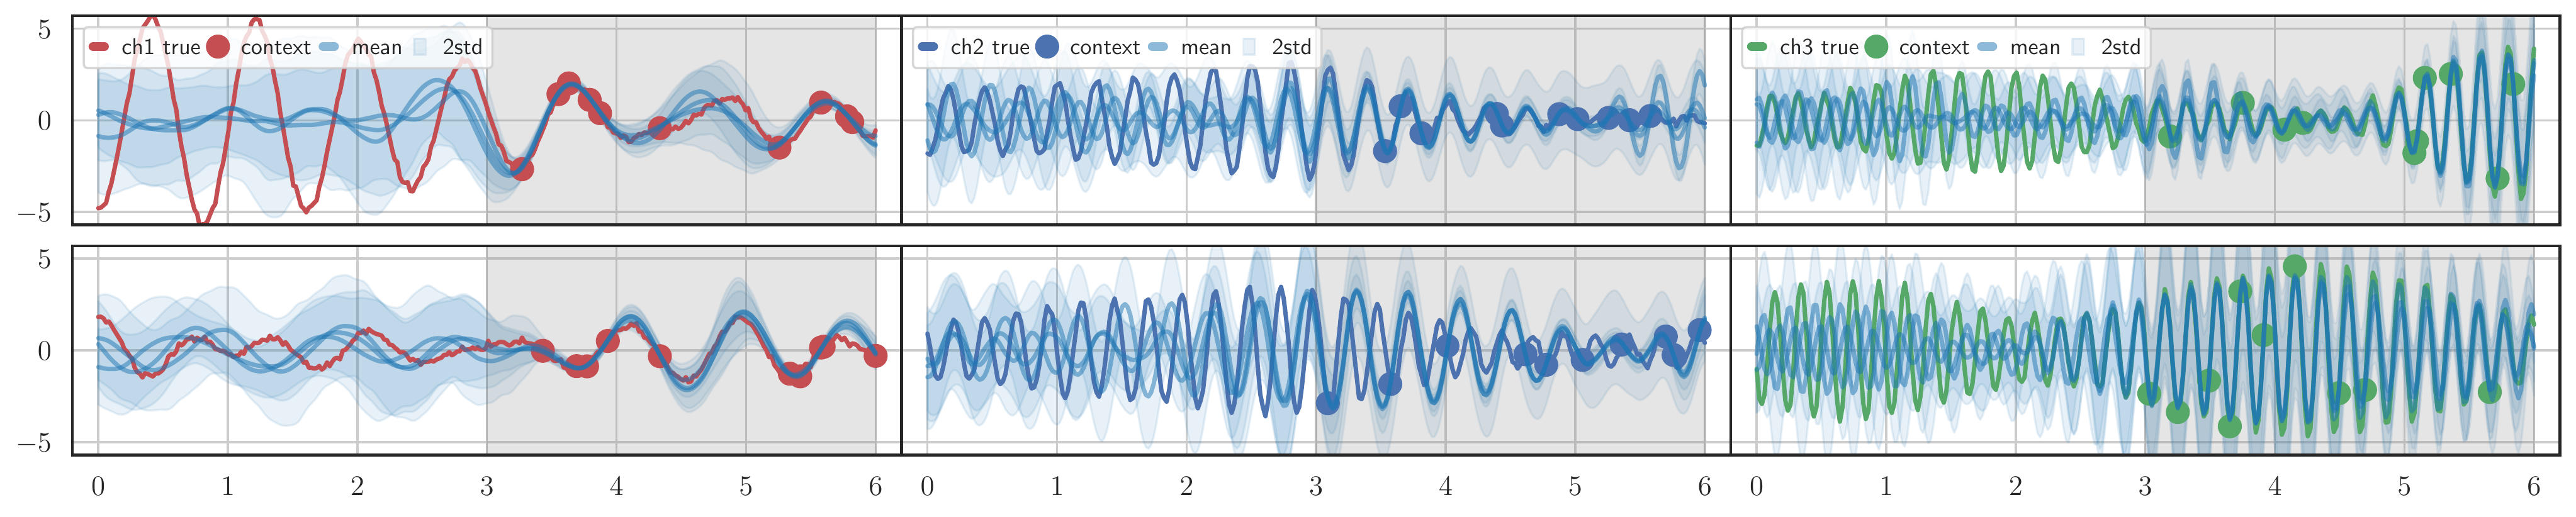}} 
\vspace{2mm}
\subfloat[\label{fig:nd2-multitask-f} ConvCNP:  Prediction for 2 different tasks ($N^{c}=10$) of the MOSM-varying  ]
{\includegraphics[width=0.98\linewidth]{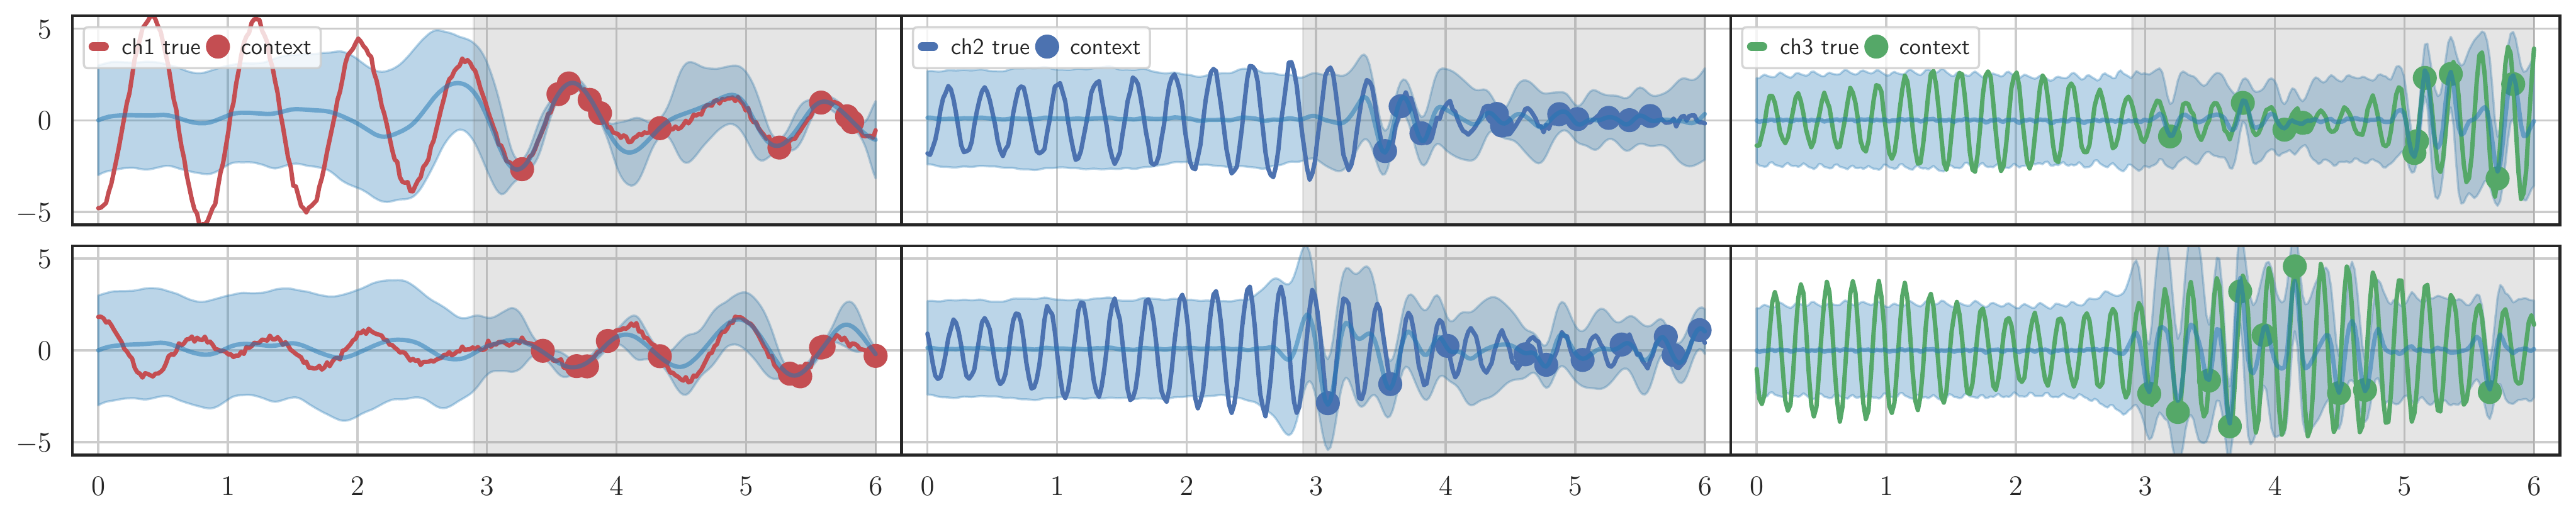}} 
\vspace{2mm}
\subfloat[\label{fig:nd2-multitask-g} GPConvCNP: Prediction for 2 different tasks ($N^{c}=10$) of the MOSM-varying  ]
{\includegraphics[width=0.98\linewidth]{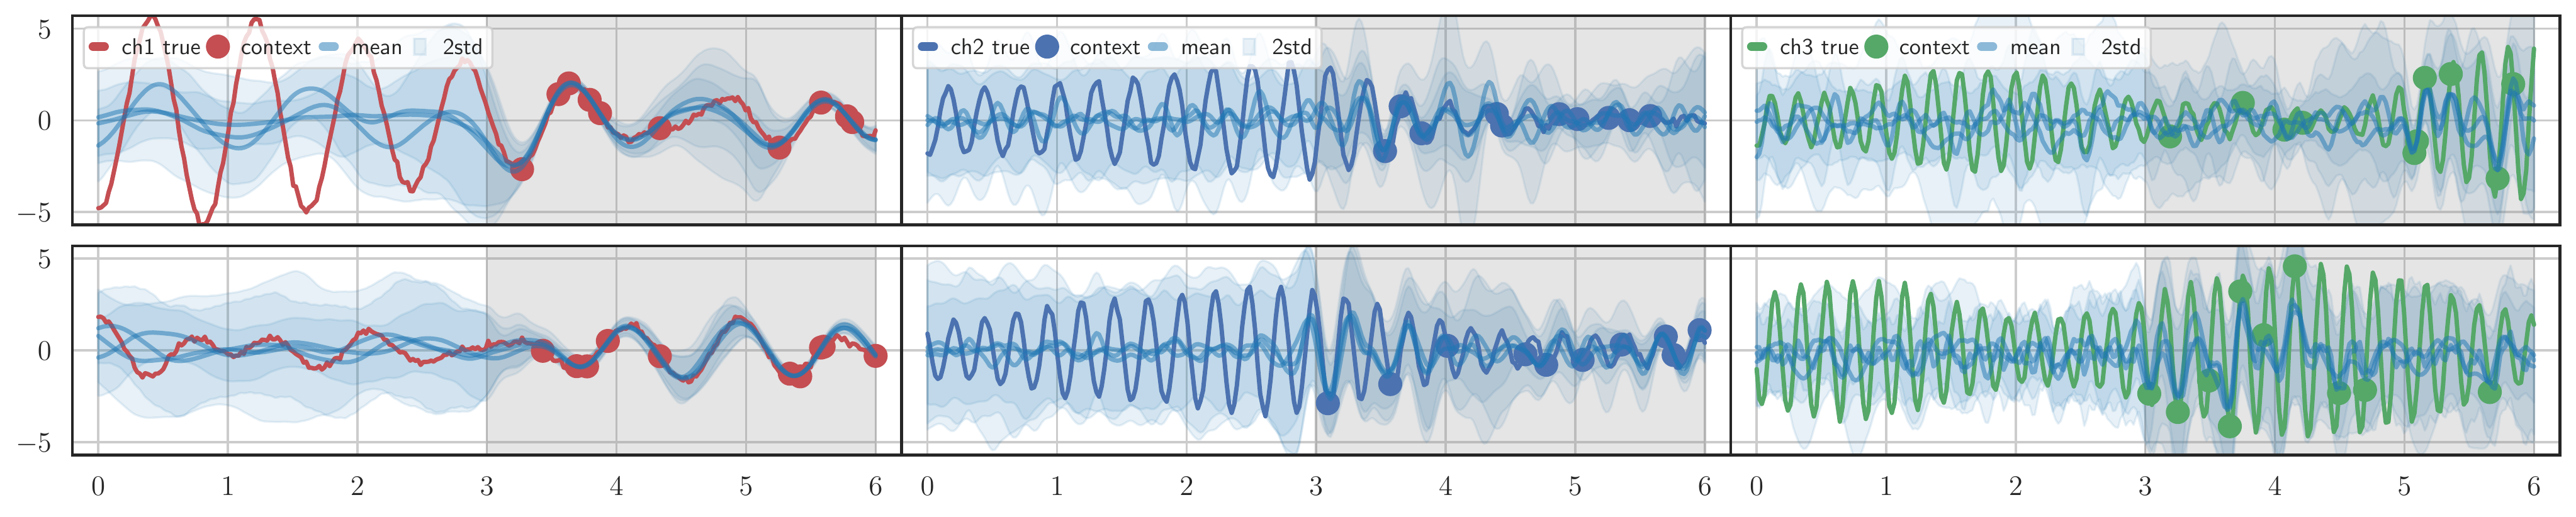}} 
\caption{3-channel GP-MOSM processes modeling: \cref{fig:nd2-multitask-a,fig:nd2-multitask-b} denotes test likelihood having different task diversity. \cref{fig:nd2-multitask-c} denote the trained spectral density for the MOSM-varying process, and \cref{fig:nd2-multitask-d,fig:nd2-multitask-e} show the chosen prior and corresponding prediction for 2 tasks; check that the stationary prior is imposed differently (from top to bottom in \cref{fig:nd2-multitask-d}), when context are given differently (from first to second row in \cref{fig:nd2-multitask-e}). \cref{fig:nd2-multitask-f,fig:nd2-multitask-g} show the prediction results using the same context set with \cref{fig:nd2-multitask-e}.
}
\label{fig:nd-multitask-pred}
\end{figure*}

\clearpage

%\subsection{Additional Experimental Results}

%\subsection{Further Details for the Predator-Pray model}
\section{Further Details for Image Completion Task}

\subsection{Details for Datasets}
For image completion task, each task is defined to predict the randomly chosen pixel values of image when using given partial pixel values as context set. To do this, we use a subset of monthly land surface temperature set used in \citeb{remes2017non}. We use the surface temperature of North America ($53{\times}115{\times}3$) and Europe ($78{\times}102{\times}3$).

% For each task, we set that $N^c$ context points and $N^{t}$ target points is proportional to the size of image by choosing a small context rate $p \in \{.01,.05,.10,.20\}$ randomly with probability $[4/10,3/10,2/10,1/10]$. This is indented to investigate how NP models predict the image of temperature when NP models are trained with each context set $D^{c}$ having the the small number $N^{c}$ of context points.

\subsection{Details for Tasks of Training, Validation, and Test }

We use the datasets (2018 - 2020) for the training, and datasets (2021) for the test. 

For training, we randomly sample the context and target set by choosing a small context rate $p \in \{.01,.05,.10,.20\}$ randomly with probability \textb{$[4/10,3/10,2/10,1/10]$}. We use \textb{$2500 \times 5$} tasks for training, and \textb{$256 \times 4$ } tasks as validation set.

For test, we set the varying context rate \textb{$p \in \{.01,.05,.10,.20\}$} as done in training phase, and set target set by choosing a target rate \textb{$p=.5$} We use each \textb{$256$ } tasks per context rate \textb{$p \in \{.01,.05,.10,.20\}$} to evaluate the trained models.

\subsection{Details for Hyperparameters.}

%\paragraph{Hyperparameters of proposed method.}

For stationary kernels, we set $\mu_{1}=[0.0,0.0]$ and $\sigma_{1}=[0.5,0.5]$ for $Q=1$.

For $Q=4$, we set $\mu_{1}=[0.0,0.0],\mu_{2}=[2.0,0.0],\mu_{3}=[0.0,2.0],$ and $\mu_{4}=[2.0,2.0]$ and $\sigma_{q}=[0.5,0.5]$ for $q=1,..,4$.

For the number of spectral points, we use $l=10$ in \textb{Eq. (14)}.

For the number of sample function, we use $N=4$ in \textb{Eq. (19)}.

For the prior hyperparameter of approximate scheme $\alpha$, we use $\alpha \in \{.05,0.1\}$.

For training, we  use ADAM optimizer \citeb{kingma2014adam} with learning rate $5e\text{-}4$ and weight decay $1e\text{-}4$. 

For the regularizer hyperparameter $\beta$ in \textb{Eq. (21)}, we set $\beta=0.1$ for the proposed method.

% \paragraph{Hyperparameters for Training.} We use ADAM optimizer \citeb{kingma2014adam} with learning rate $5e\text{-}4$ and weight decay $1e\text{-}4$. For the regularizer hyperparameter $\beta$ in \textb{Eq. (21)}, we set $\beta=0.1$.

% \subsection{Baseline Implementations}
% For ConvCNP and the proposed model, we use the shallow 2d CNN described in \cref{subsubsec:cnnstructure} for all models

\subsection{Additional Results}
%fig:predator-pray-70

We report additional prediction results for image completion tasks of North America dataset in \cref{fig:image_completion-usa-a}.
\begin{figure*}[h]
\centering
% {\includegraphics[width=0.975\linewidth,height=5cm]{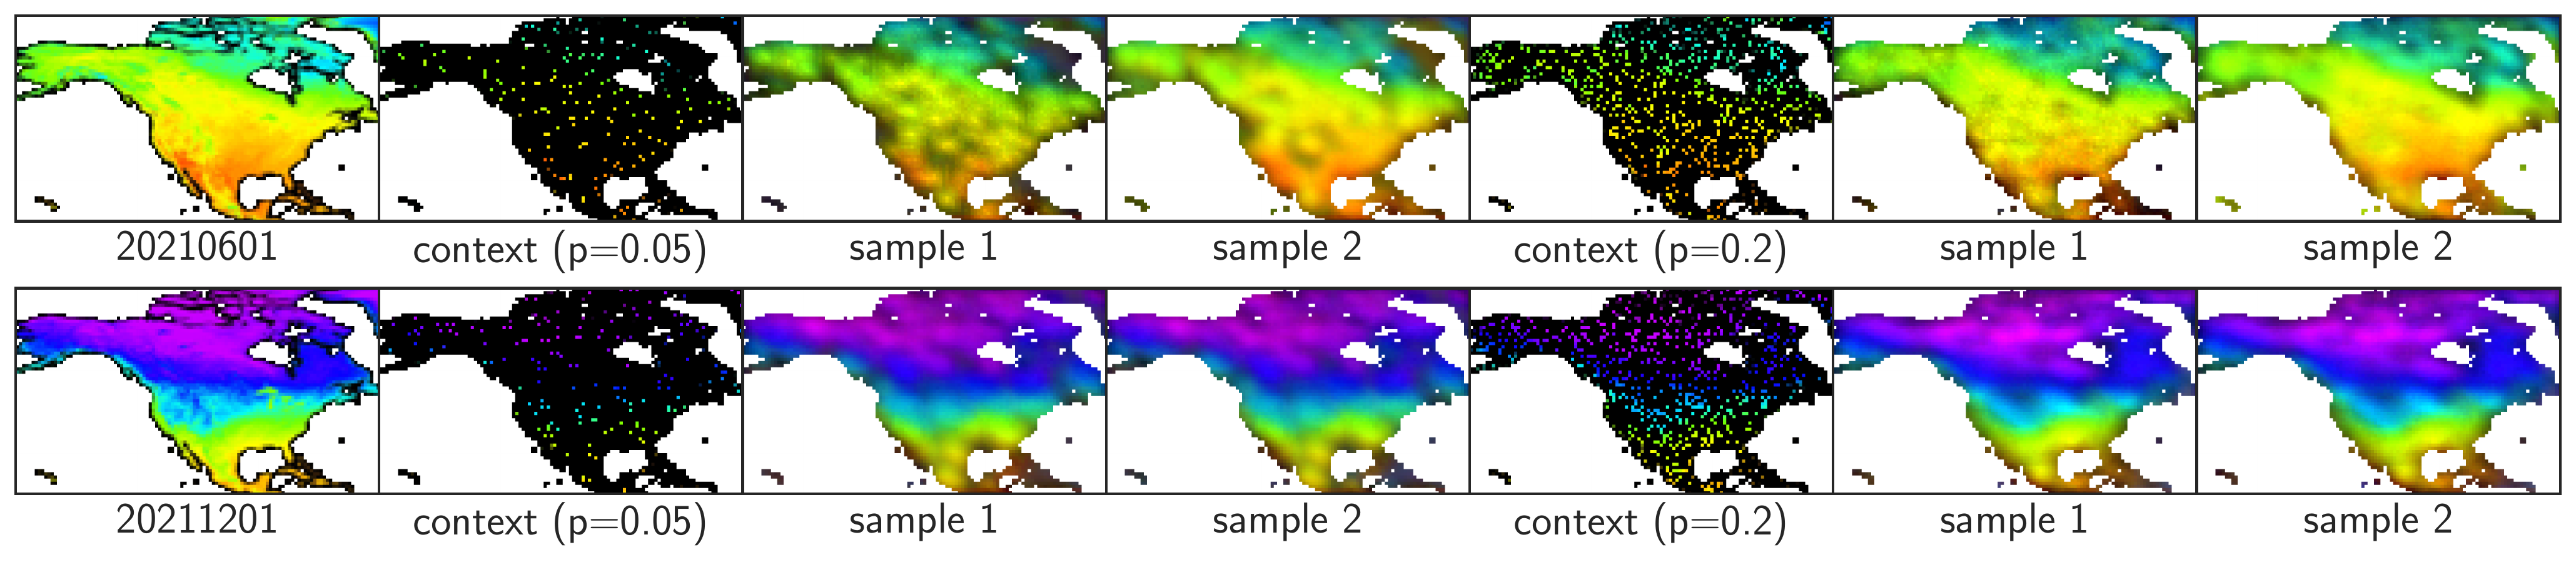}}  
{\includegraphics[width=0.95\linewidth,height=4.5cm]{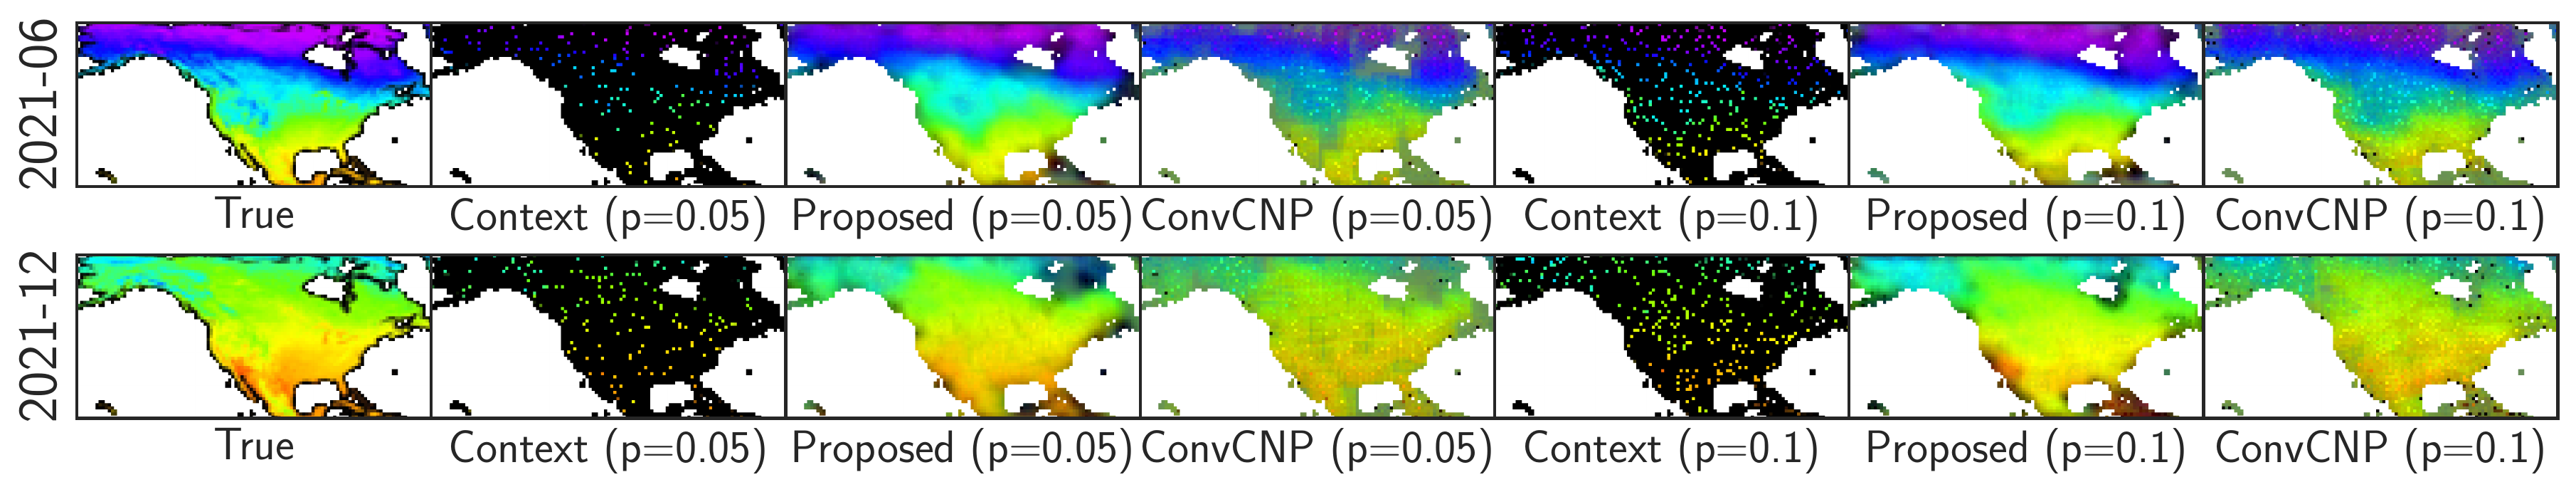}}  
\caption{Prediction results for North America temperatures (June 2021 and December 2021) that are out of training sets.}
\label{fig:image_completion-usa-a}
\end{figure*}

Additionally, we report the progress of the test log likelihood during training phase in \cref{fig:exp5-3:smallset-usa-progress,fig:exp5-3:smallset-eu-progress}. These figures compare the prediction improvement of the models depending on the number of used training tasks.

\cref{fig:exp5-3:small-a,fig:exp5-3:small-b,fig:exp5-3:small-c,fig:exp5-3:small-d} shows the test log likelihood on the dataset of North America (2018-2020) over varying training tasks $\{2500,5000,7500,10000\}$. \cref{fig:exp5-3:small-e,fig:exp5-3:small-f,fig:exp5-3:small-g,fig:exp5-3:small-h} shows the corresponding results on the dataset of North America (2021).

With the same protocol of North America experiment results,  \cref{fig:exp5-3:small-a2,fig:exp5-3:small-b2,fig:exp5-3:small-c2,fig:exp5-3:small-d2} shows the corresponding results on Europe temperature (2018-2020), and \cref{fig:exp5-3:small-e2,fig:exp5-3:small-f2,fig:exp5-3:small-g2,fig:exp5-3:small-h2} shows the corresponding results on Europe temperature (2018-2020),

\vspace{-3mm}
\begin{figure}[H]
%\begin{figure}[htp!]
\centering
\subfloat[ \label{fig:exp5-3:small-a}  2500 tasks (in-train)]
{\includegraphics[width=0.24\linewidth]{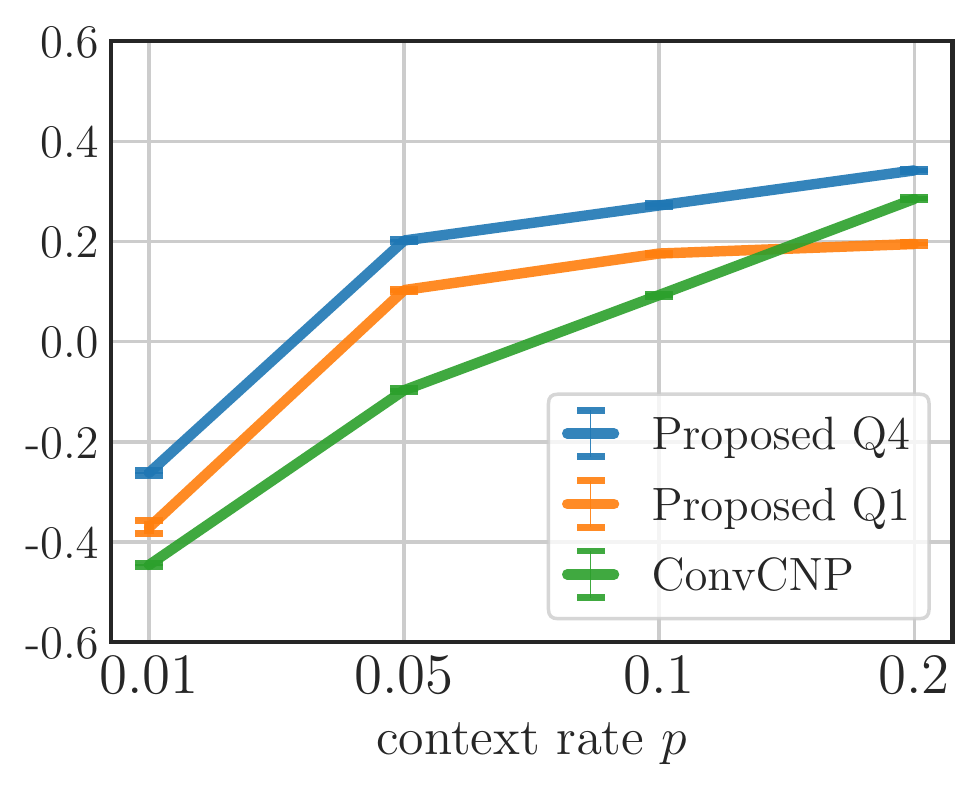}}   \hspace{0.5mm} 
\subfloat[ \label{fig:exp5-3:small-b} 5000 tasks (in-train)] 
{\includegraphics[width=0.24\linewidth]{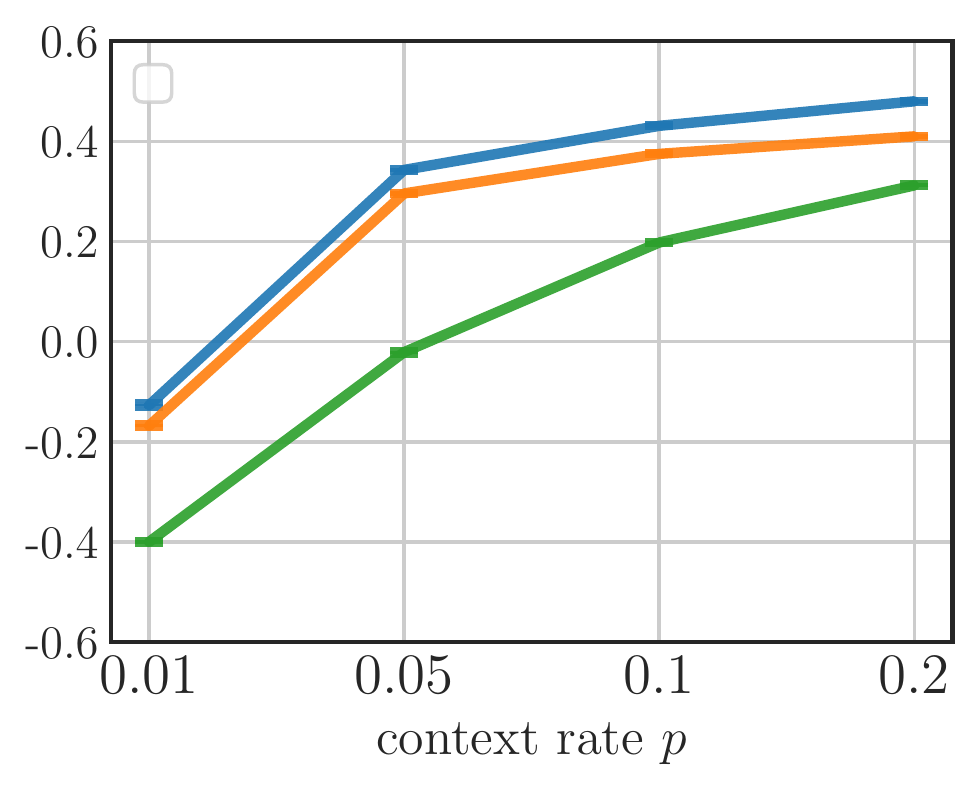}}   \hspace{0.5mm} 
\subfloat[ \label{fig:exp5-3:small-c} 7500 tasks (in-train) ]
{\includegraphics[width=0.24\linewidth]{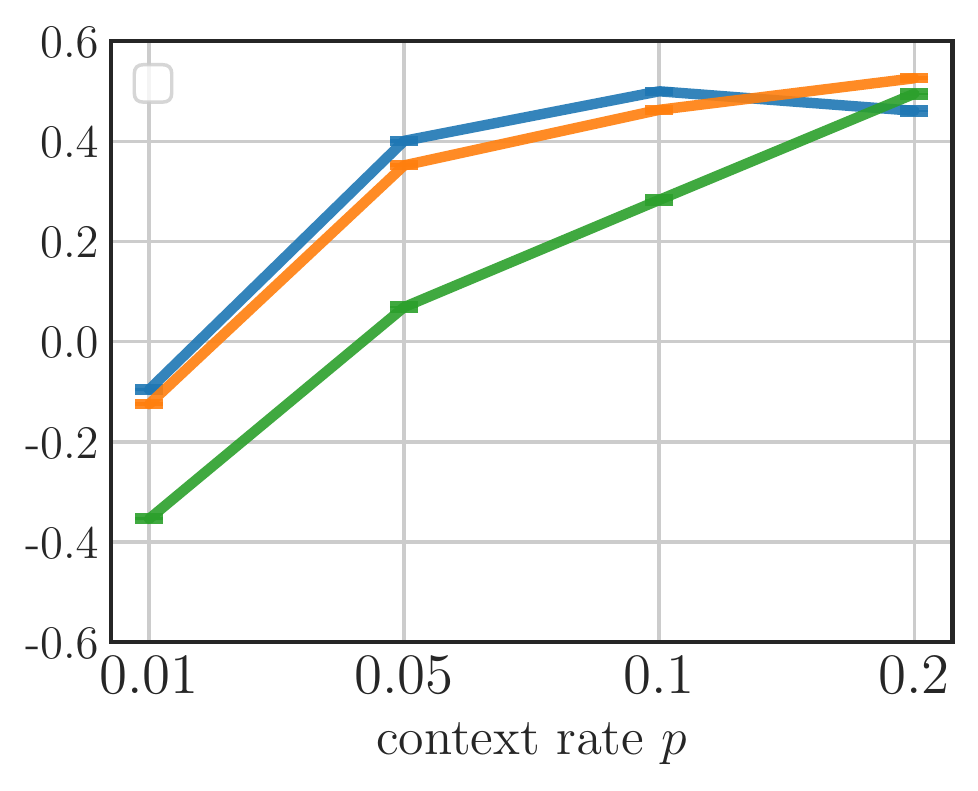}}  \hspace{0.5mm} 
\subfloat[ \label{fig:exp5-3:small-d} 10000 tasks (in-train) ]
{\includegraphics[width=0.24\linewidth]{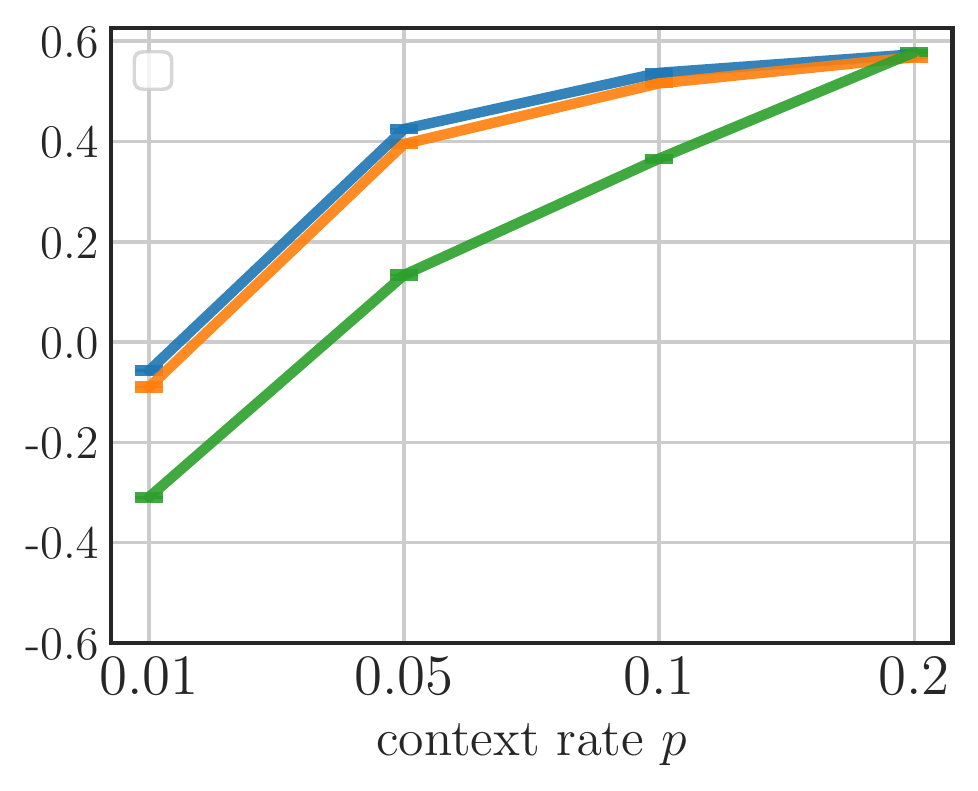}}

\vspace{2mm}
\subfloat[ \label{fig:exp5-3:small-e}  2500 tasks (out-train)]
{\includegraphics[width=0.24\linewidth]{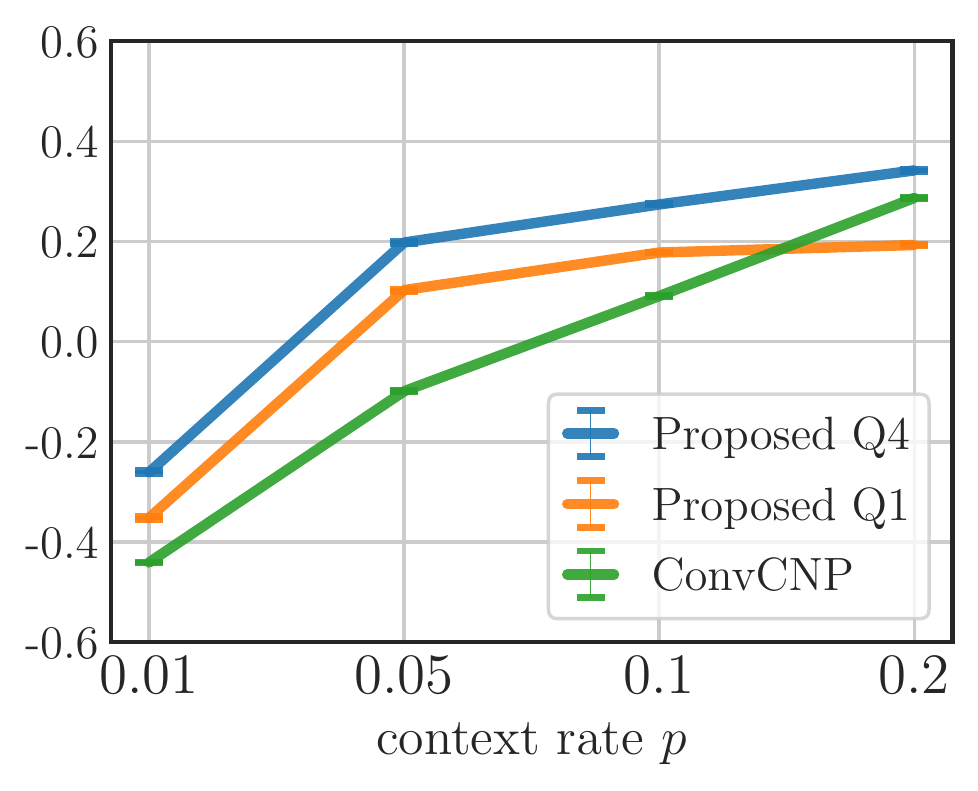}}   \hspace{0.5mm} 
\subfloat[ \label{fig:exp5-3:small-f} 5000 tasks (out-train)] 
{\includegraphics[width=0.24\linewidth]{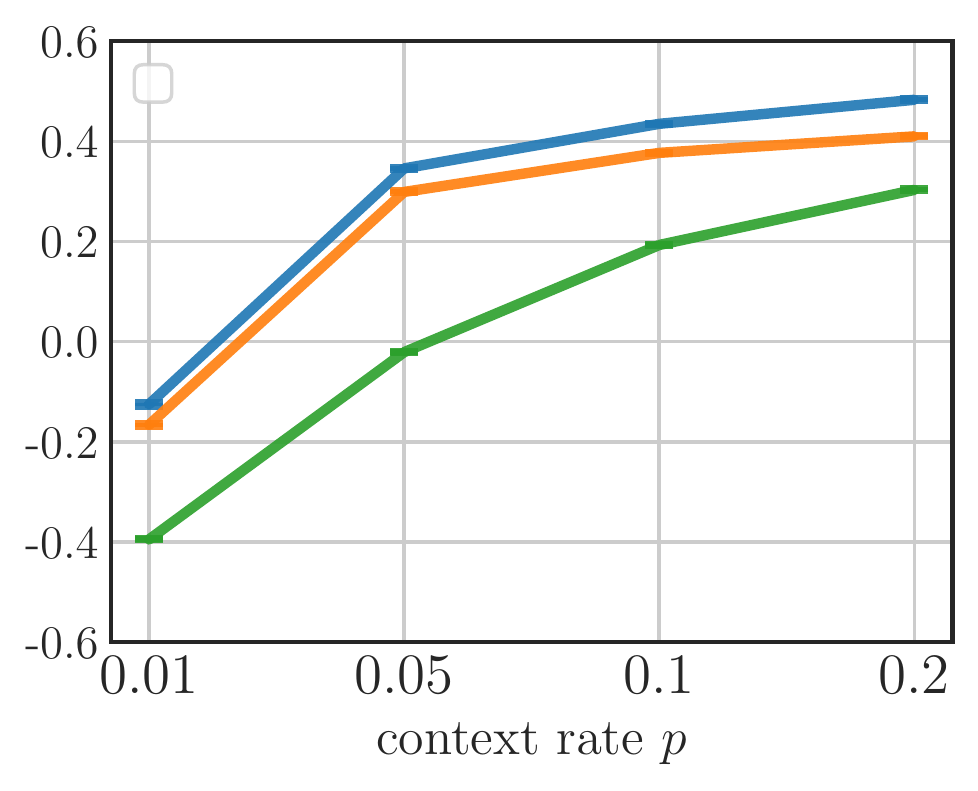}}   \hspace{0.5mm} 
\subfloat[ \label{fig:exp5-3:small-g} 7500 tasks (out-train) ]
{\includegraphics[width=0.24\linewidth]{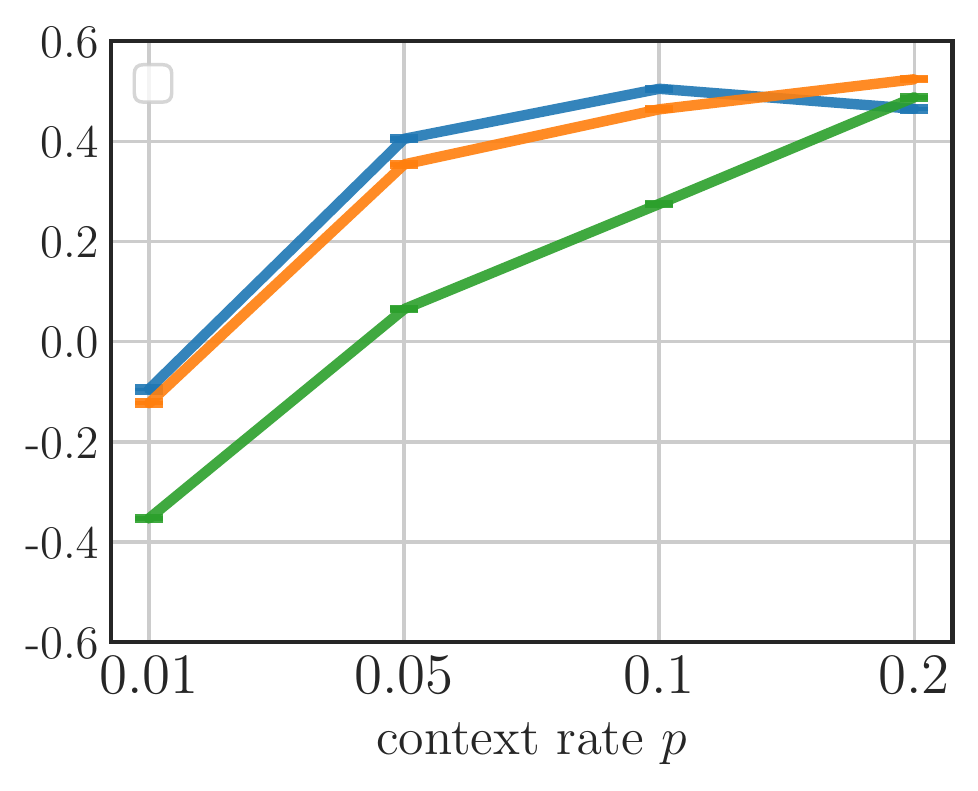}}  \hspace{0.5mm} 
\subfloat[ \label{fig:exp5-3:small-h} 10000 tasks (out-train) ]
{\includegraphics[width=0.24\linewidth]{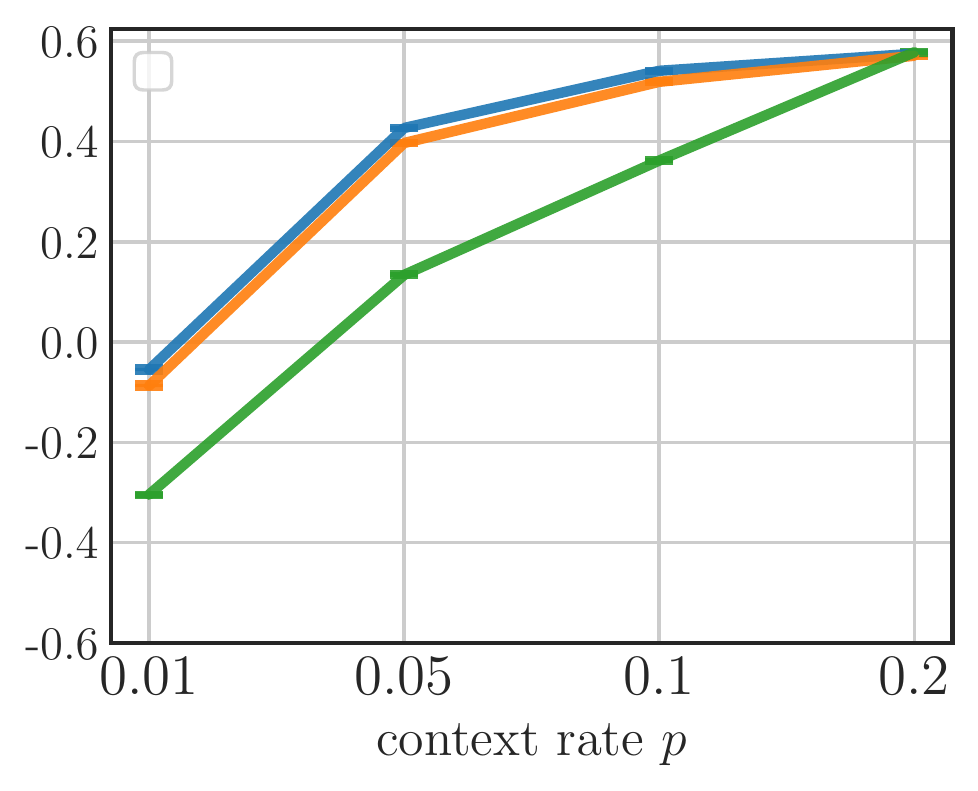}}
\caption{Test log likelihood of \textb{North America} dataset over the varying number of training tasks.}
\label{fig:exp5-3:smallset-usa-progress}
\end{figure}

\vspace{3mm}
\begin{figure}[H]
%\begin{figure}[htp!]
\centering
\subfloat[ \label{fig:exp5-3:small-a2}  2500 tasks (in-train)]
{\includegraphics[width=0.24\linewidth]{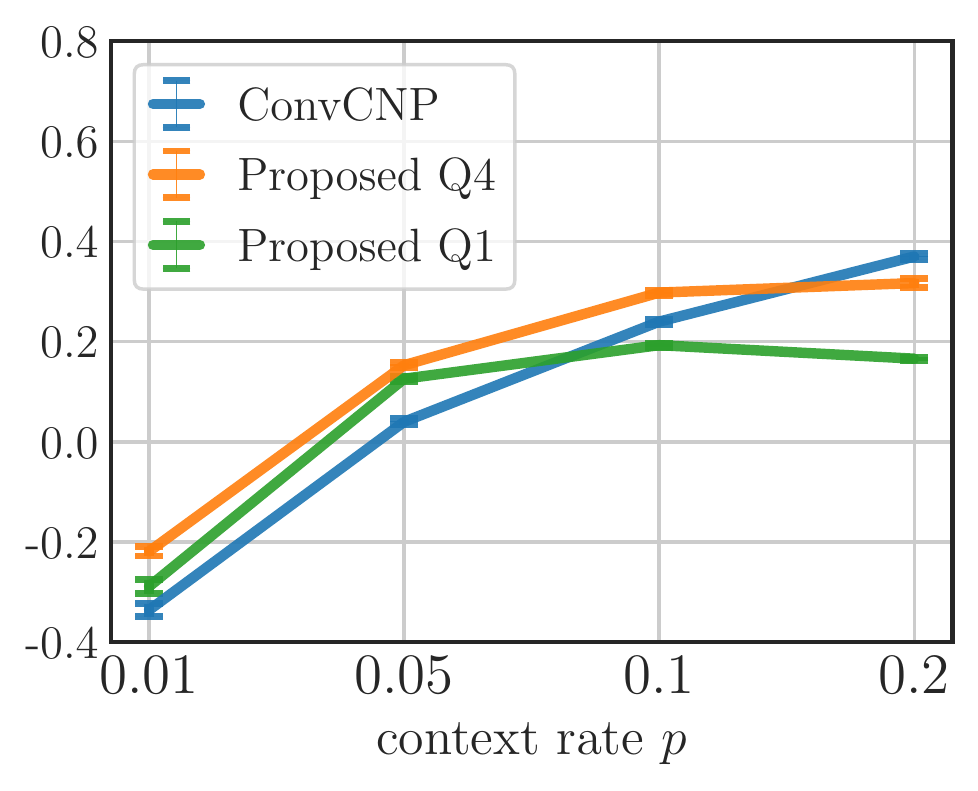}}   \hspace{0.5mm} 
\subfloat[ \label{fig:exp5-3:small-b2} 5000 tasks (in-train)] 
{\includegraphics[width=0.24\linewidth]{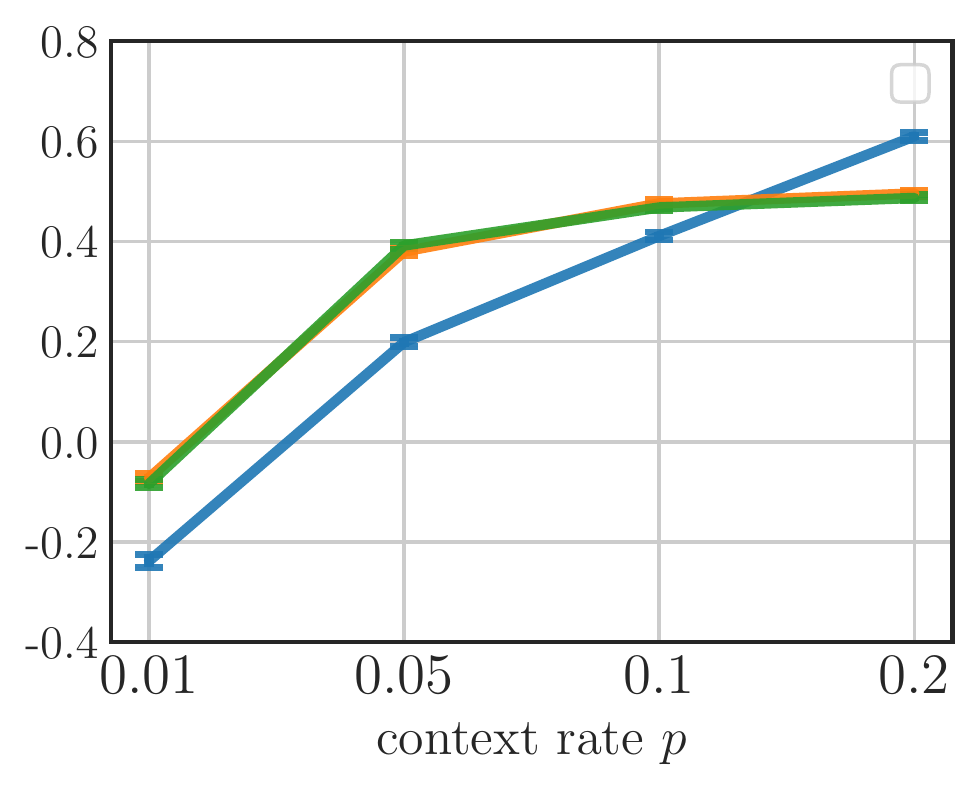}}   \hspace{0.5mm} 
\subfloat[ \label{fig:exp5-3:small-c2} 7500 tasks (in-train) ]
{\includegraphics[width=0.24\linewidth]{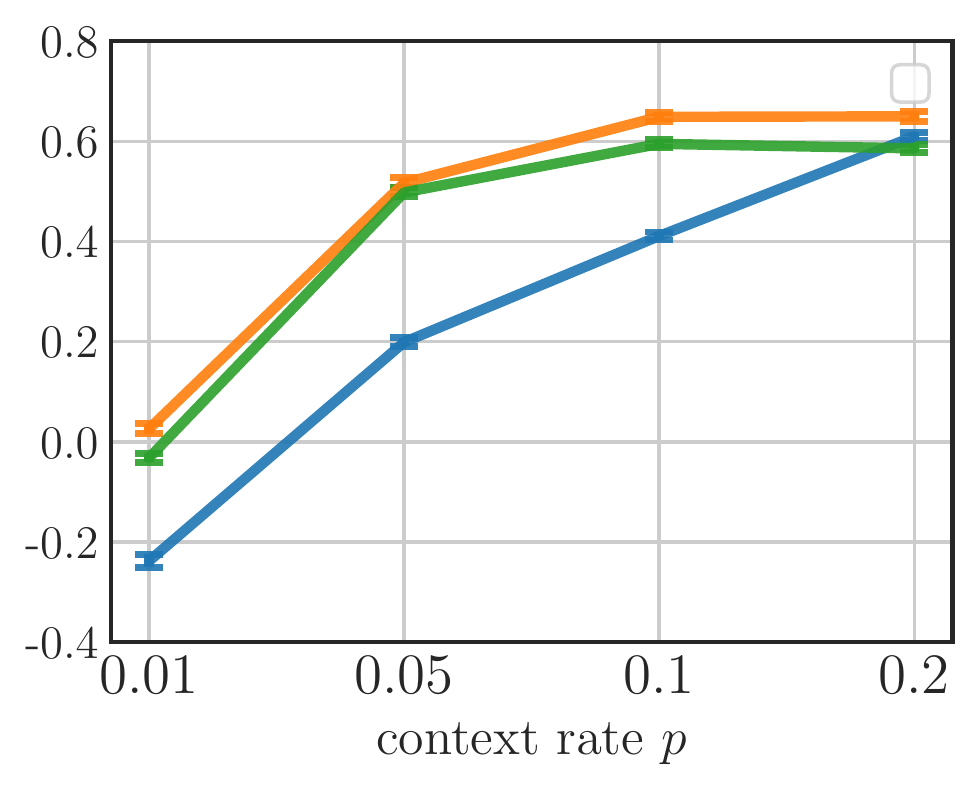}}  \hspace{0.5mm} 
\subfloat[ \label{fig:exp5-3:small-d2} 10000 tasks (in-train) ]
{\includegraphics[width=0.24\linewidth]{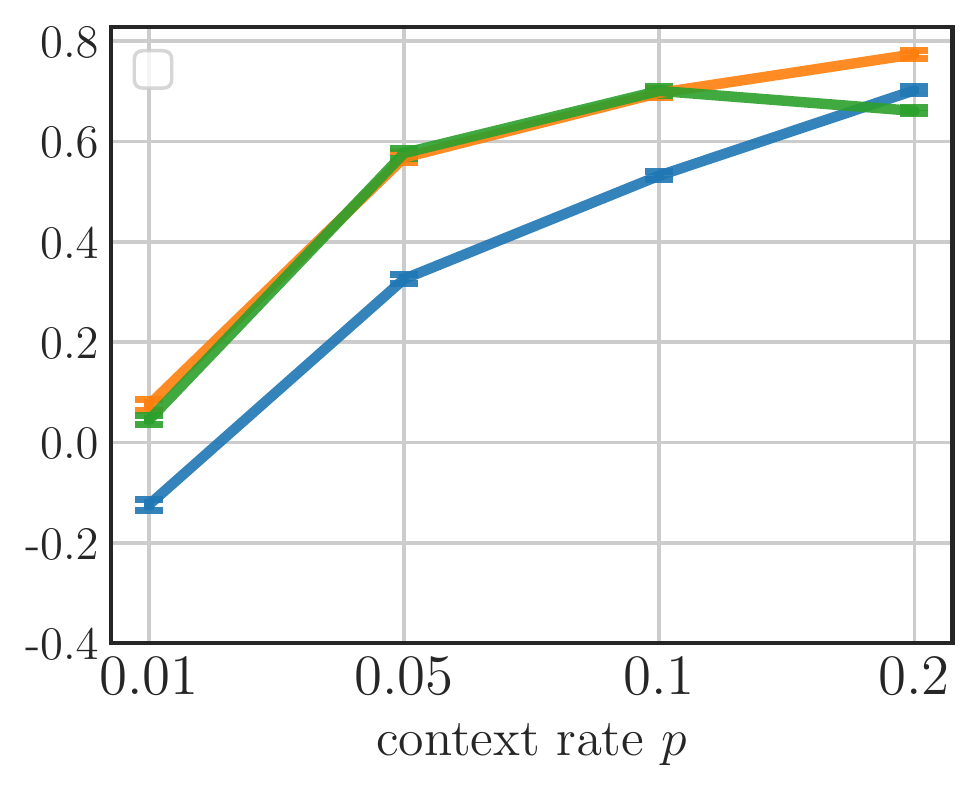}}

\vspace{2mm}
\subfloat[ \label{fig:exp5-3:small-e2}  2500 tasks (out-train)]
{\includegraphics[width=0.24\linewidth]{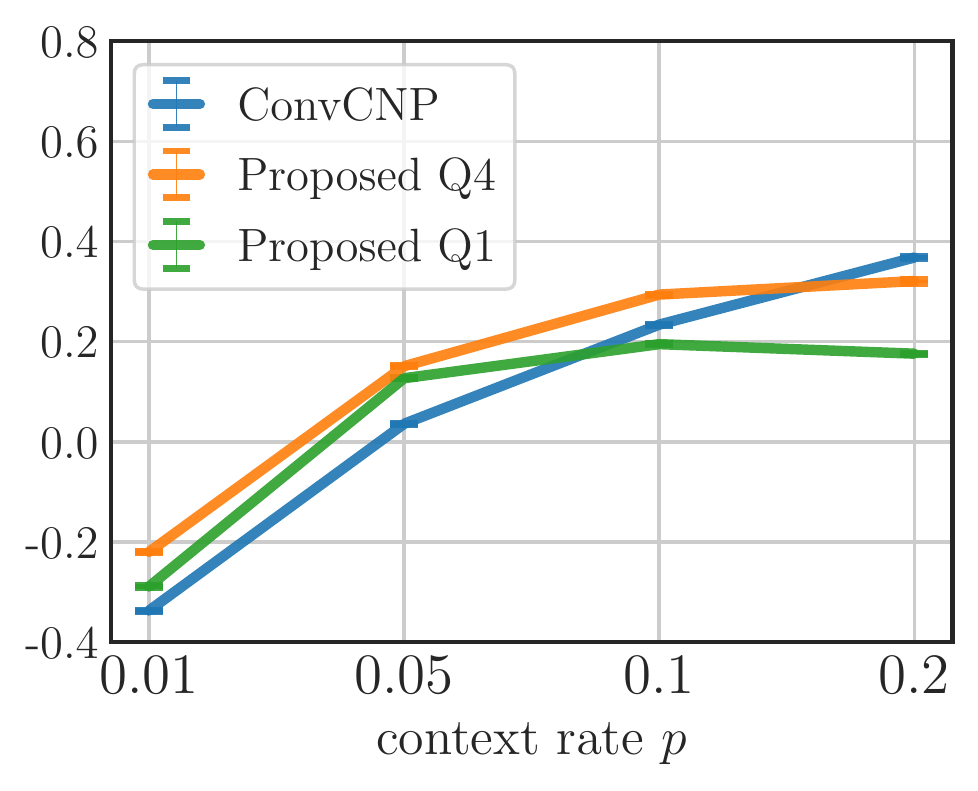}}   \hspace{0.5mm} 
\subfloat[ \label{fig:exp5-3:small-f2} 5000 tasks (out-train)] 
{\includegraphics[width=0.24\linewidth]{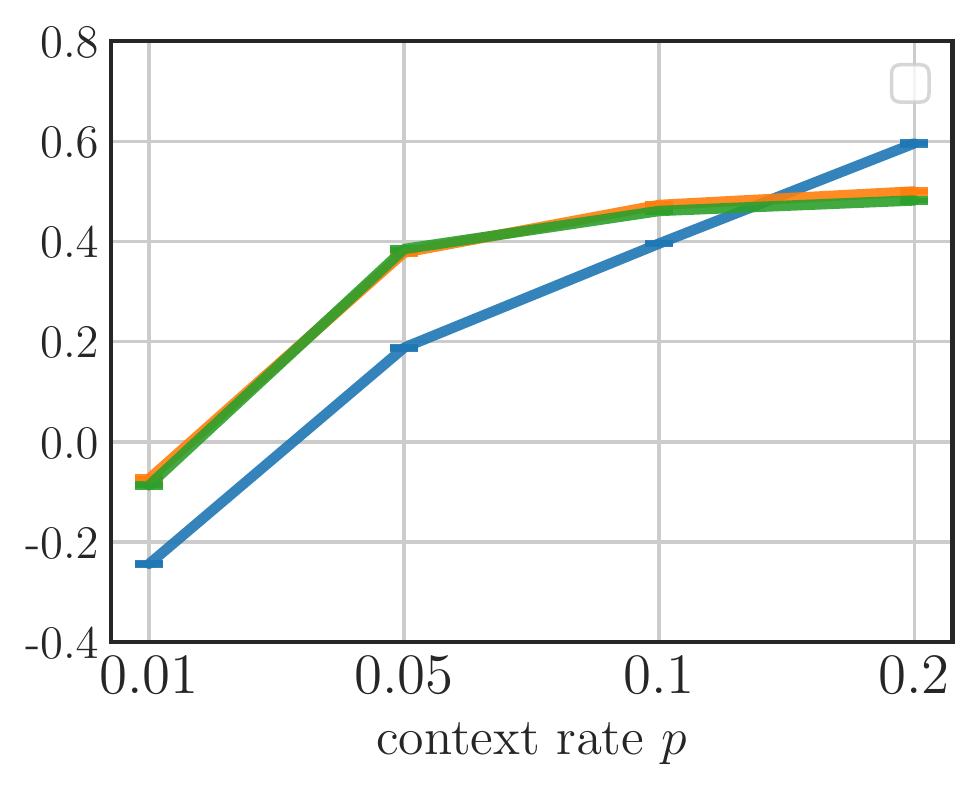}}   \hspace{0.5mm} 
\subfloat[ \label{fig:exp5-3:small-g2} 7500 tasks (out-train) ]
{\includegraphics[width=0.24\linewidth]{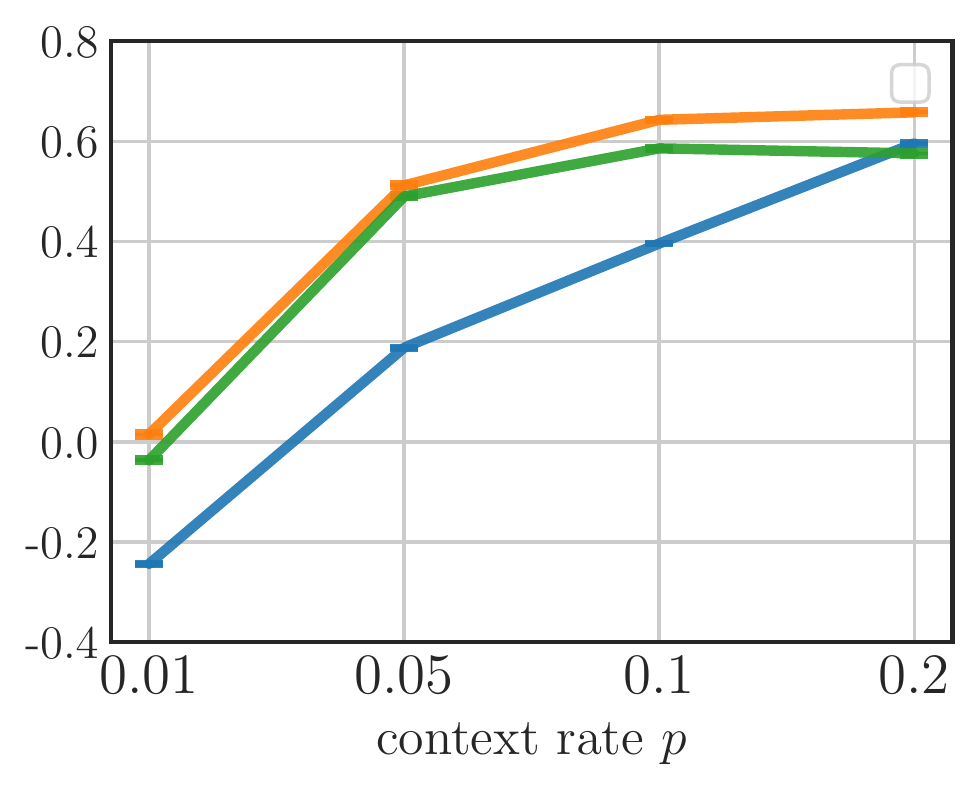}}  \hspace{0.5mm} 
\subfloat[ \label{fig:exp5-3:small-h2} 10000 tasks (out-train) ]
{\includegraphics[width=0.24\linewidth]{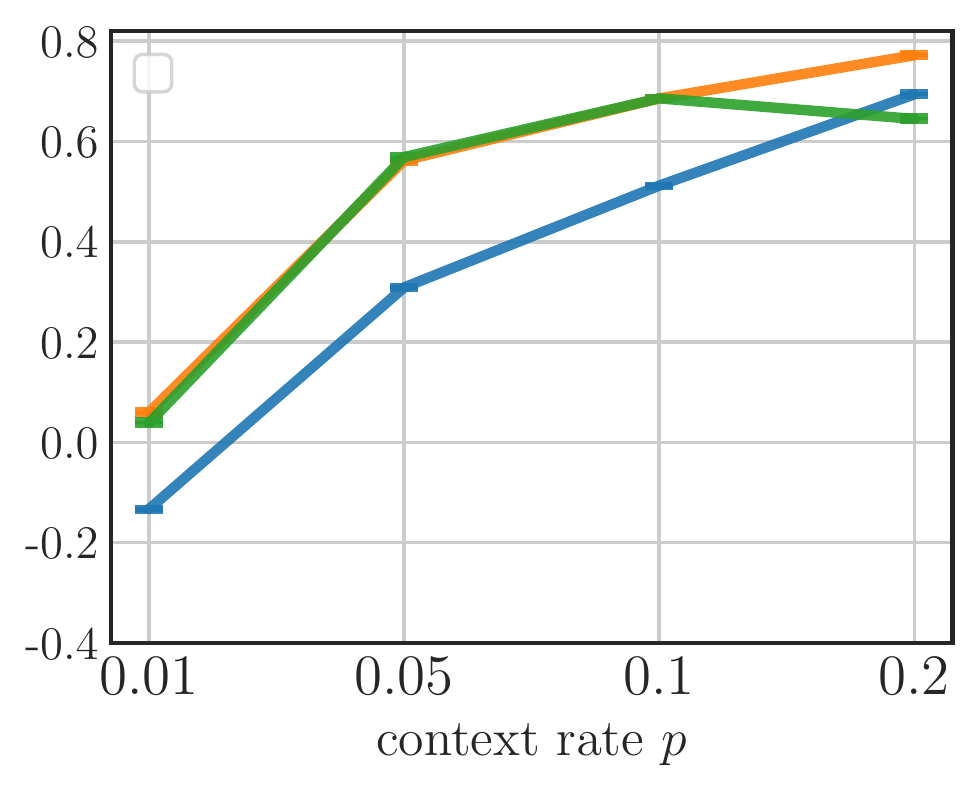}}
\caption{Test log likelihood of \textb{Europe} dataset over the varying number of training tasks.}
\label{fig:exp5-3:smallset-eu-progress}
\end{figure}

% \vspace{5mm}

% \input{07-appendix-v01-chapter4-exp3-figure01}
% \input{07-appendix-v01-chapter4-exp3-figure02}
% \input{07-appendix-v01-chapter4-exp3-figure03}
\clearpage

%\subsection{Further Details for the Predator-Pray model}
%\section{Further Details for the Predator-Pray model}
\section{Further Details for Simulation to Real (Predator-Pray model)}

\subsection{Details for Datasets}

In this experiment, we use synthetic dataset simulated by a Lotka-Volterra differential equation \citeb{lotka2002contribution} for training, and then predicts the real-world dataset (Hudson’s Bay hare-lynx data) for test. We employ the following implementation \citeb{lee2020bootstrapping} \footnotemark{\footnotetext[4]{\url{https://github.com/juho-lee/bnp/blob/master/regression/data/lotka_volterra.py}}}.

\subsection{Details for Tasks of Training, Validation, and Test }
We consider the following number of data points for training, validation, and test: 
\begin{itemize}[leftmargin=1em]
    \vspace{-2mm}
    \item \textbf{Simulated dataset:}
    For training, we randomly sample total data point \textb{$N \sim \mathcal{U}([100{-}15,100])$}, and set $N_t=N$ as the number of target data points for each task. Out of the sampled total points, we sample \textb{$N_c \sim \mathcal{U}([15,30{-}15])$} data points randomly, and use them as context data points. We use \textb{$100{\times}32{\times}32$} tasks for training through 100 batches. For validation, we set $N_c$ context data points and $N_t$ target data points as done in training, and use \textb{$128{\times}32$} tasks for validation to choose the parameters of the trained models.
    For test, we consider $N_t$ target data points per a task as described in training, and use \textb{$N_c \in \{10,20,30,40,50,70,80\}$} context data points, that are chosen randomly from the $N_t$ target data points for each task. We use \textb{$64{\times}16$} tasks per given $N_c$ context points to study how the number of context data points affects the predictive performance of the trained models using the parameters obtained in validation procedure.
    \item \textbf{Real dataset:} For evaluation on real dataset, we consider $N_t=91$ target data points, and use \textb{$N_c \in \{10,20,30,40,50,70,80\}$} context data points, that are chosen randomly from $N_t$ target data points for each task. We use \textb{$64{\times}16$} tasks per given $N_c$ context points to evaluate the trained model with Simulated dataset.
\end{itemize}

\subsection{Details for Hyperparameters.}

For the hyperparameter of RBF kernels used for ConvCNP, we conduct the experiment with  $l\in\{0.01,0.1\}$, and set the lengthscale $l=0.01$ for each channel because it obtains the best performance for both models out of those candidates.

For the hyperparameter used for GPConvCNP, we use RBF kernel $(Q=1)$ for each channel, and set $\Sigma=0.1$ for each channel. 

For the hyperparameter of basis kernels, we set $\mathrm{Hz}_{\mathrm{max}}=5$ and 4 basis stationary kernels ($Q=4$). Then, we set $\{\mu_q\}_{q=1}^{4}$ by randomly sampling $\mu_q \sim \mathcal{U}[0,\mathrm{Hz}_{\mathrm{max}}]$ with $\mu_1=0 \leq ..\leq \mu_4$, and set
$\Sigma_q = 0.1$ for $q=1,..,4$. For the noise parameter $\sigma^{2}_{\epsilon}$, we set $\sigma_{\epsilon}=1e\text{-}{2}$.

For the number of spectral points, we use $l=10$ in \textb{Eq. (14)}.

For the number of sample function, we use $N=5$ in \textb{Eq. (19)}.

For the prior hyperparameter of approximate scheme $\alpha$, we use $\alpha \in \{.05,0.1\}$.

For training, we  use ADAM optimizer \citeb{kingma2014adam} with learning rate $1e\text{-}3$ and weight decay $1e\text{-}4$. 

For the regularizer hyperparameter $\beta$ in \textb{Eq. (21)}, we set $\beta=0.5$ for the proposed method.

\clearpage
\subsection{Additional Results}
%fig:predator-pray-70

%We report additional prediction results obtained in experimental section 5.3 (main). 

We conduct the predator-pray benchmark experiment conducted in \citeb{gordon2019convolutional,petersen2021gp,lee2020bootstrapping}; the NP models are first trained on the synthetic dataset simulated by a Lotka-Volterra differential equation \citeb{lotka2002contribution}, and then predict the real-world dataset (Hudson’s Bay hare-lynx data). 

%Further details of settings and additional results are reported in \textb{Appendix A.4}.

%{\includegraphics[width=0.48\linewidth,height=2.75cm]
\begin{figure}[H]
\subfloat[\label{fig:predpray-a} simulated set]
{\includegraphics[width=0.24\linewidth]{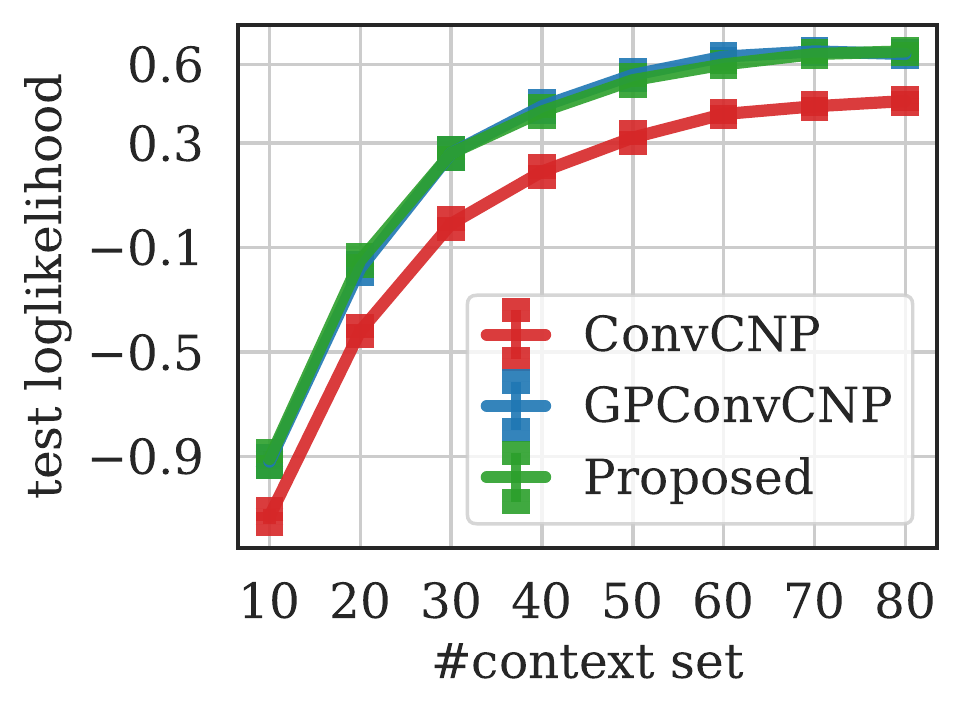}} \hspace{1mm}  
\subfloat[\label{fig:predpray-b} real set]
{\includegraphics[width=0.24\linewidth]{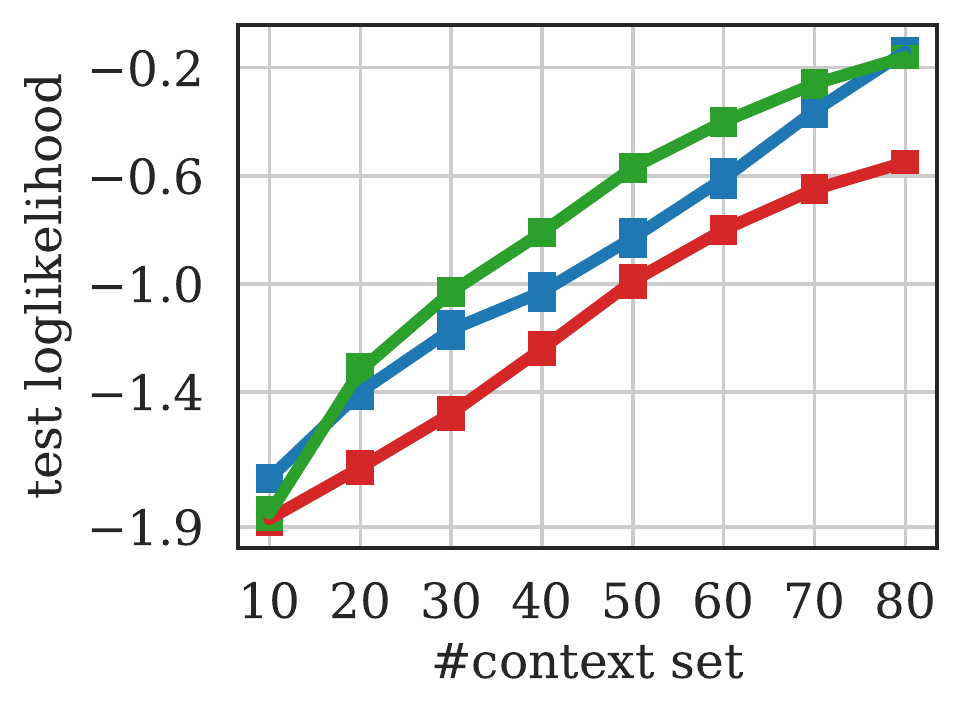}}  
\subfloat[\label{fig:predpray-c} real set]
{\includegraphics[width=0.235\linewidth]{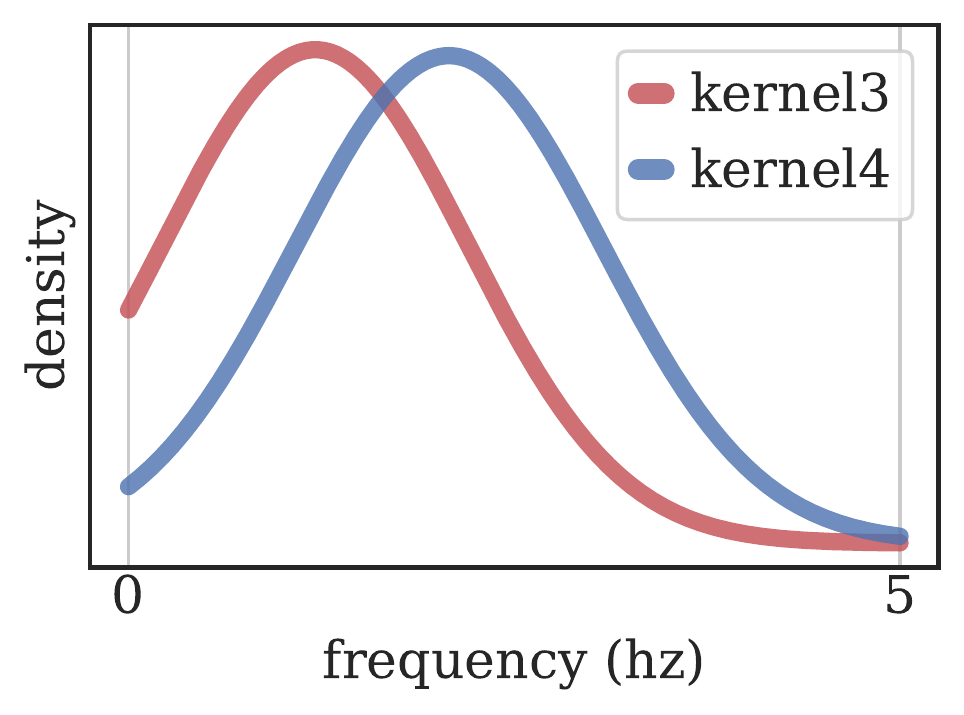}}  
\subfloat[\label{fig:predpray-d} real set]
{\includegraphics[width=0.25\linewidth]{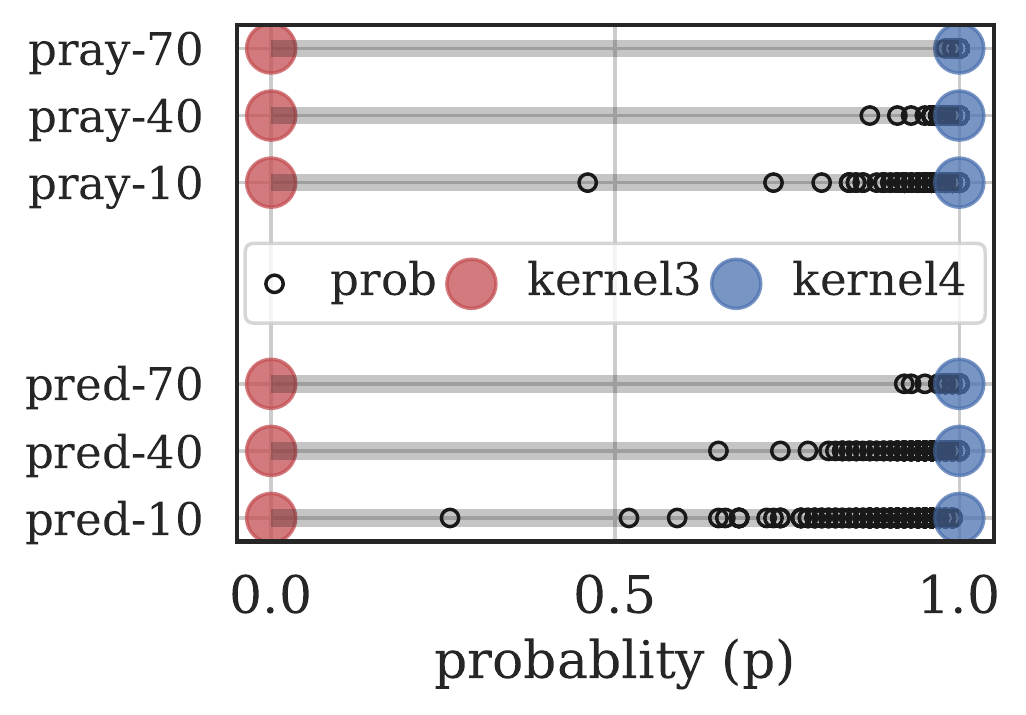}}  
\caption{{Prediction Results on simulated and real dataset;}}
\end{figure}

\cref{fig:predpray-a,fig:predpray-b} describes the mean and one-standard error of the test log likelihood for 1024 tasks of simulated and real datasets, respectively; we consider $N^{c}\in \{10,...,80\}$ context points. These figures imply that for small $N^{c}\in \{20,..,70\}$ context data points, task-dependent prior could help improve the prediction performance by using the different prior depending on $N^{c}$ context data points.

\cref{fig:predator-pray-10,fig:predator-pray-40,fig:predator-pray-70} show the prediction results of ConvCNP, GPConvCNP, and the proposed model for 2 different tasks of \textb{real dataset}, respectively.\cref{fig:predator-pray-10} shows the results using 10 context data points ($n^{c}=10$).  \cref{fig:predator-pray-40} and \cref{fig:predator-pray-70} correspond to results of $n^{c}=40$ and $n^{c}=70$, respectively. GPConvCNP and the proposed model generate 5 predictive distributions on target set respectively by using 5 random functional representations. 

\cref{fig:predator-pray-10} reveals that how the random functional representations using prior affect the prediction on target sets when the small number of context data points is given. \cref{fig:predator-pray-40} reveals that the task-dependent prior enables more robust predictions as shown in \cref{fig:pray-40e,fig:pray-40f} compared to GPConvCNP as shown in \cref{fig:pray-40c,fig:pray-40d}. \cref{fig:predator-pray-70} reveals that all models obtain similar predictive distribution on target sets when the large number of context data points is given.

\vspace{5mm}

\vspace{-5mm}
\begin{figure*}[htp!]

% \subfloat[\label{fig:fig-h} \textb{mosm-varying}: $p_{\text{traninv-nn}}(X_c,Y_c)$ ]   
% {\includegraphics[width=0.41\linewidth,height=4.85cm]{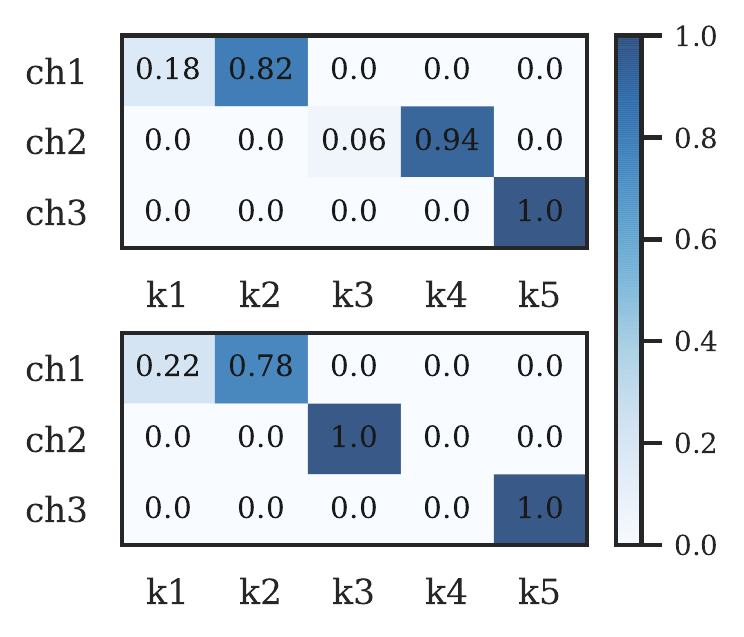}} 
\centering
\subfloat[ \label{fig:pray-10a} ConvCNP with Task1 ($N^c=10$)]{
 \includegraphics[width=0.49\linewidth]{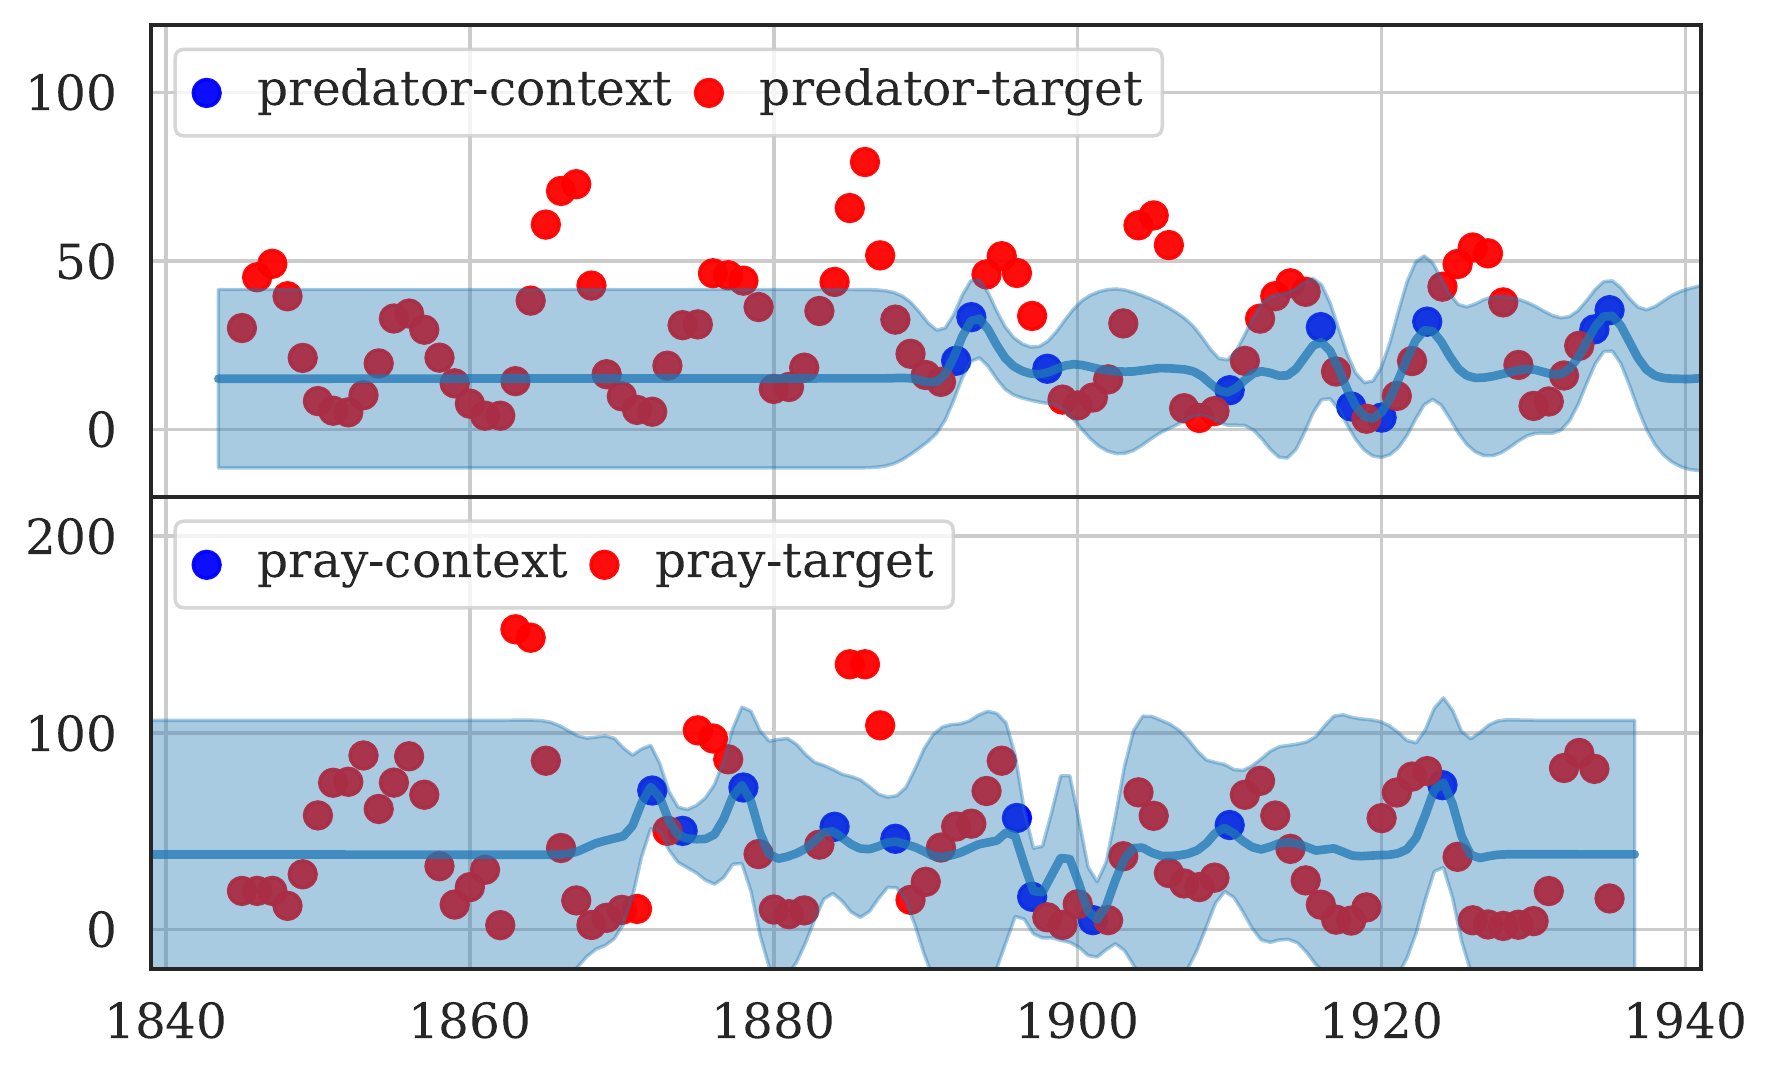}}
\subfloat[ \label{fig:pray-10b} ConvCNP with Task2 ($N^c=10$)]{\includegraphics[width=0.49\linewidth]{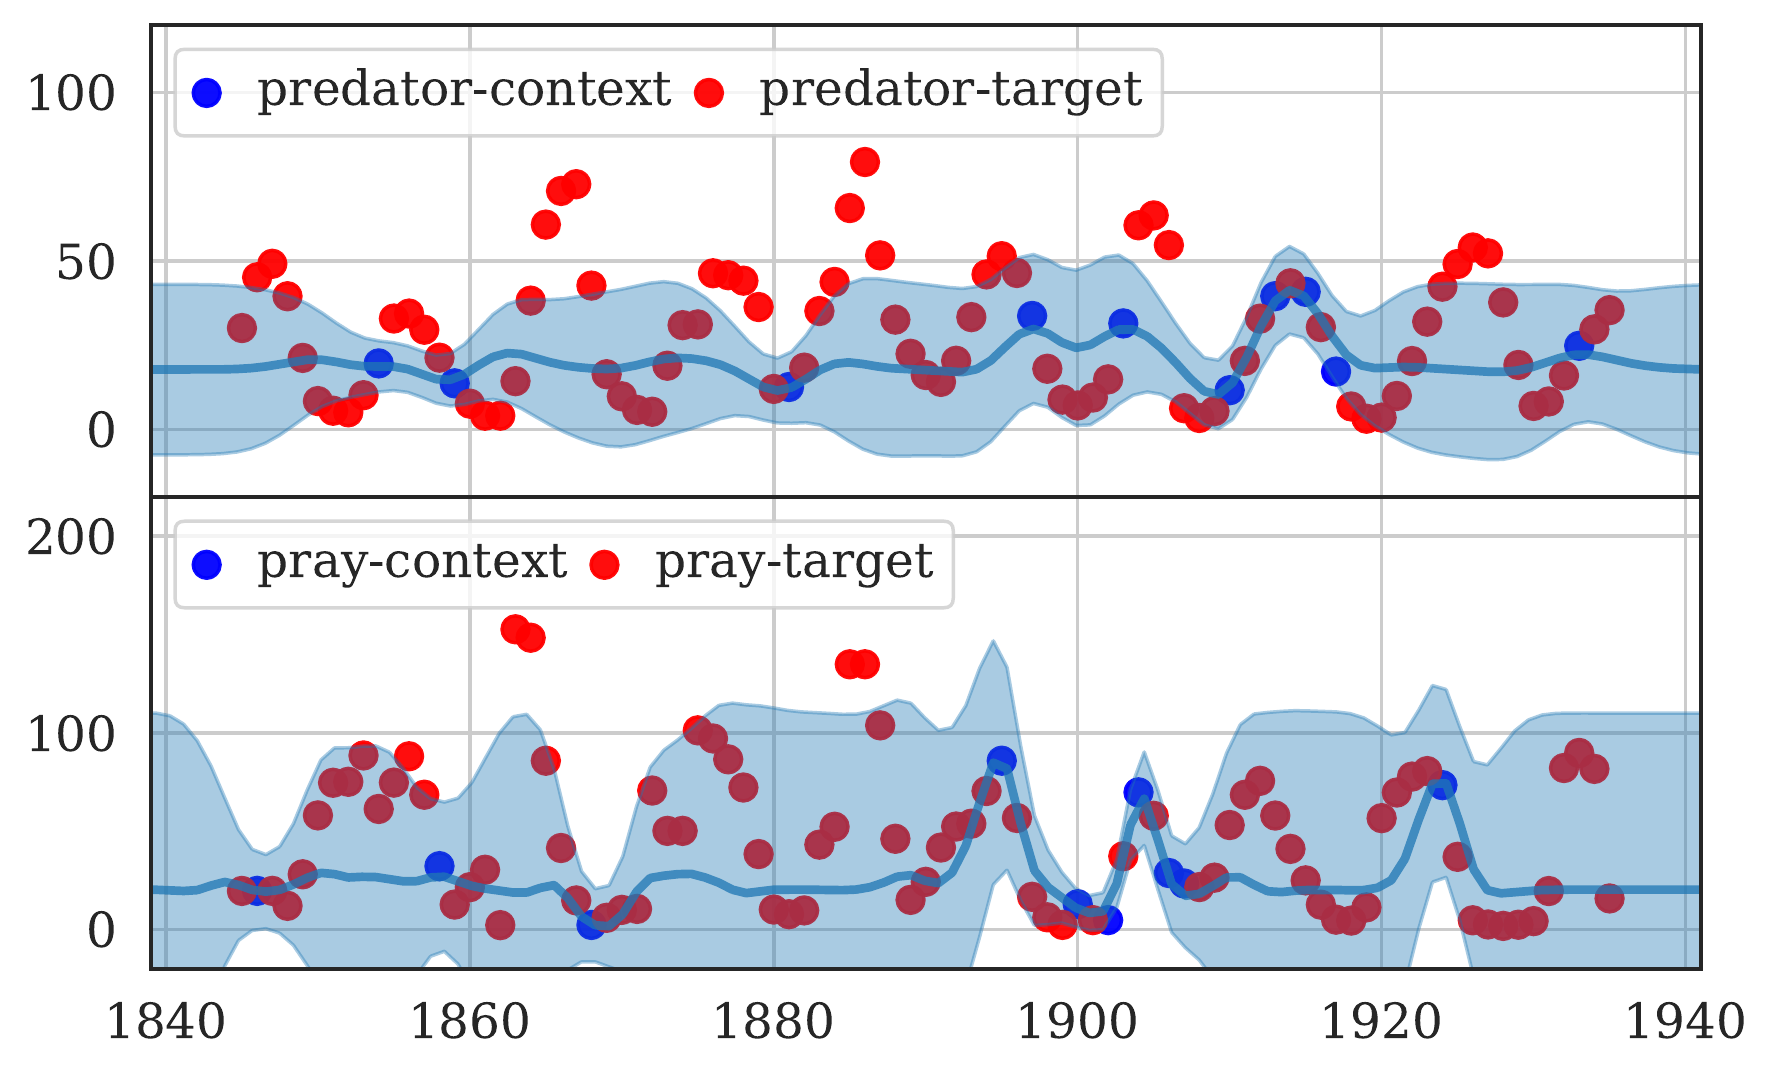}}

 \vspace{4mm}
\subfloat[ \label{fig:pray-10c} GPConvCNP with Task1 ($N^c=10$)]{
 \includegraphics[width=0.49\linewidth]{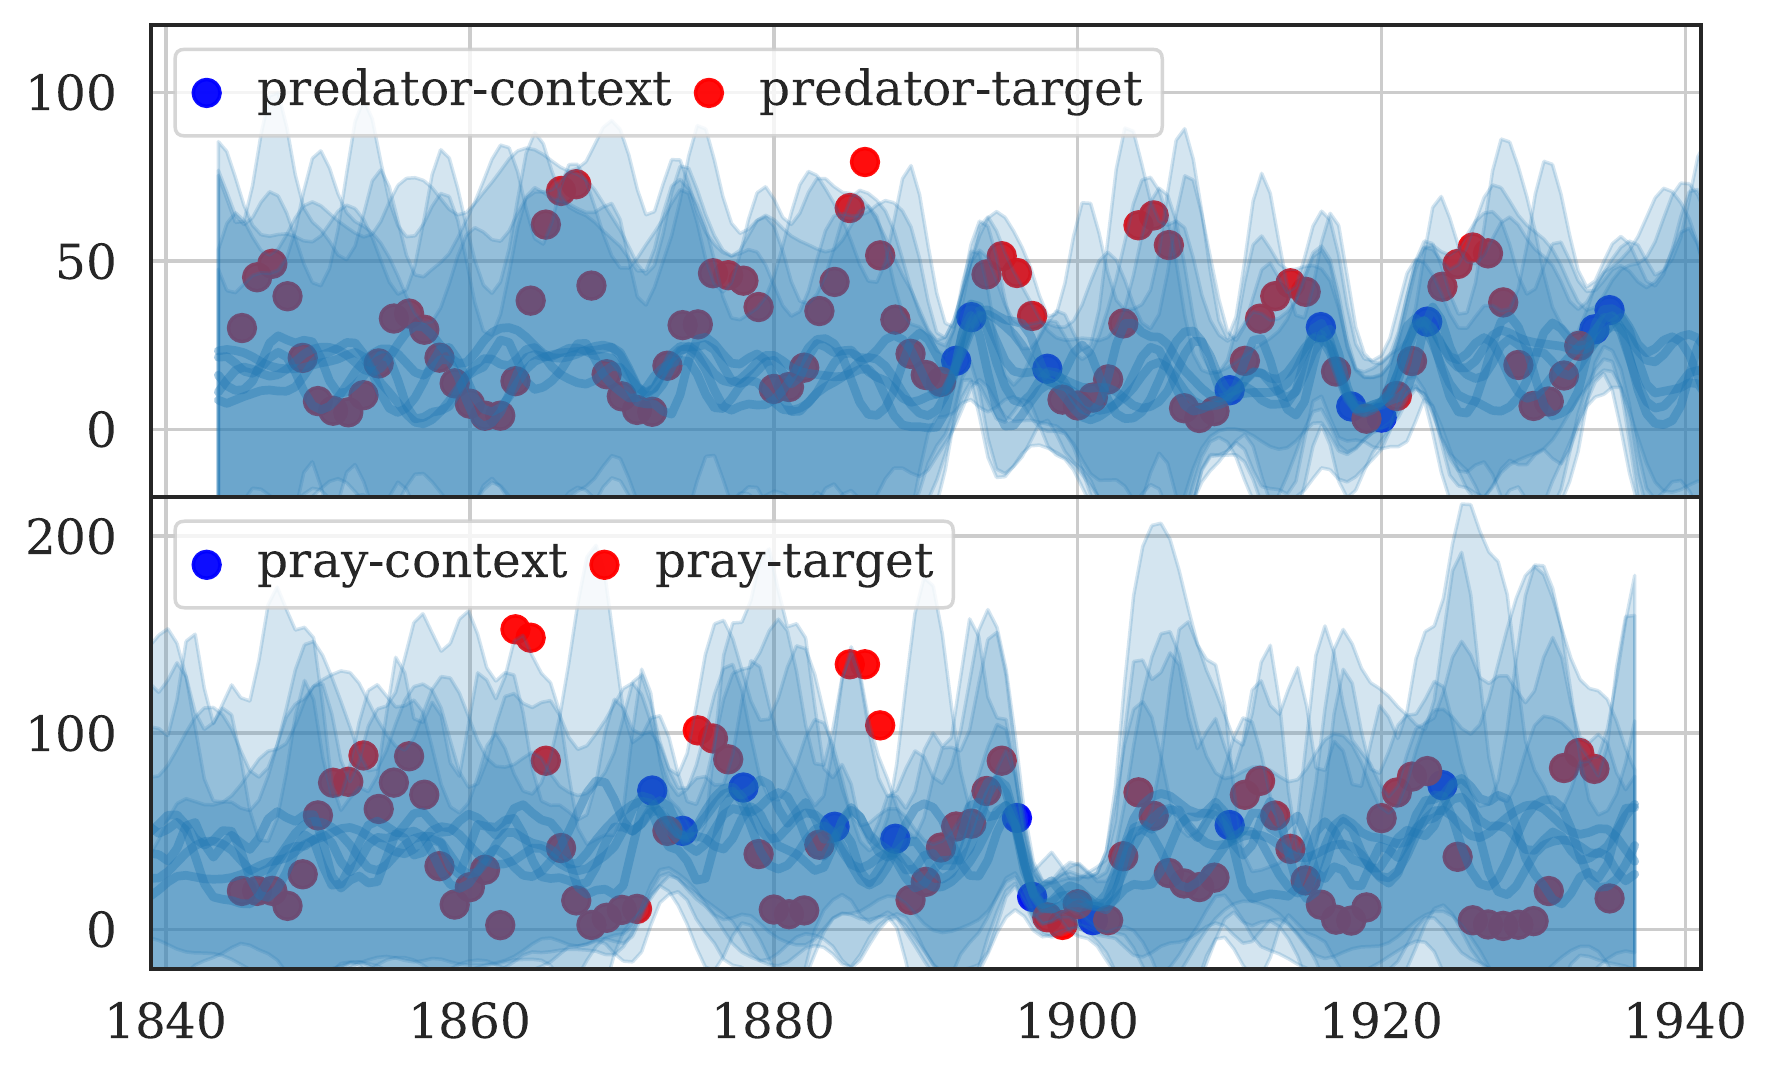}}
\subfloat[\label{fig:pray-10d} GPConvCNP with Task2 ($N^c=10$)]{
 \includegraphics[width=0.49\linewidth]{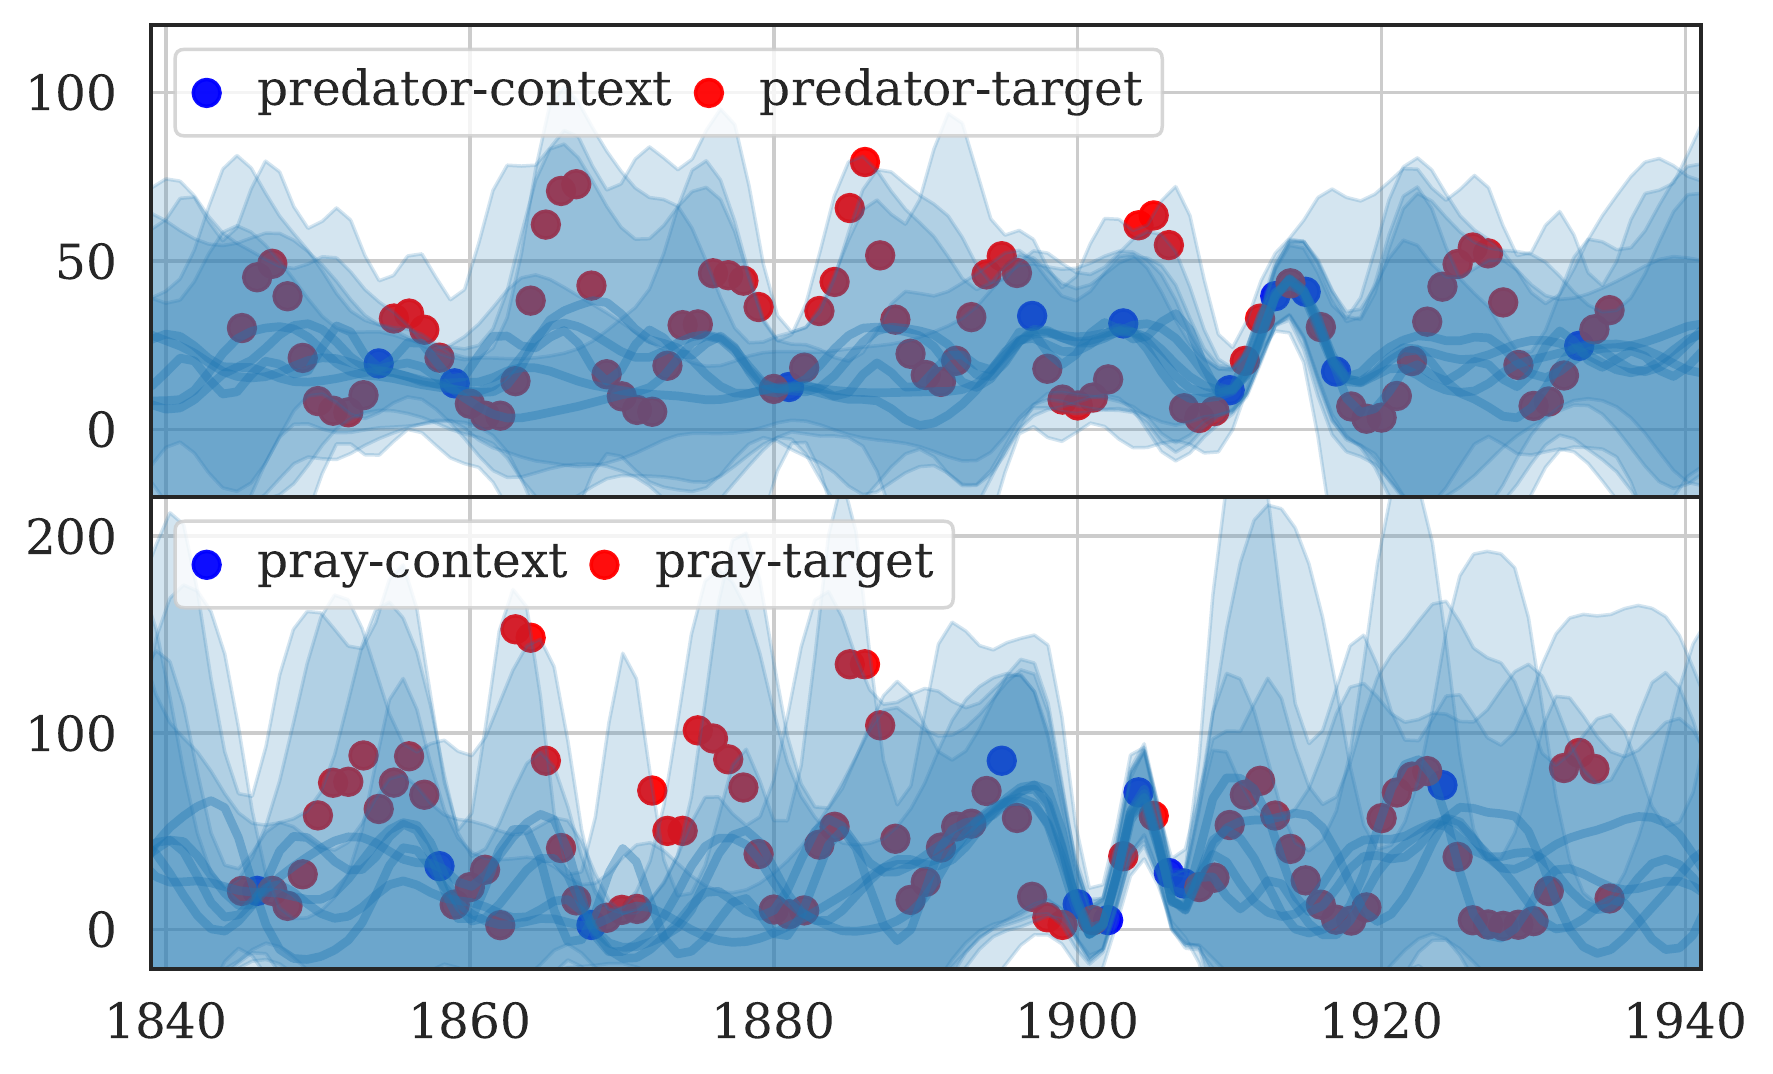}}
 
 \vspace{4mm}
\subfloat[\label{fig:pray-10e} Proposed Model with Task1 ($N^c=10$)]{
 \includegraphics[width=0.49\linewidth]{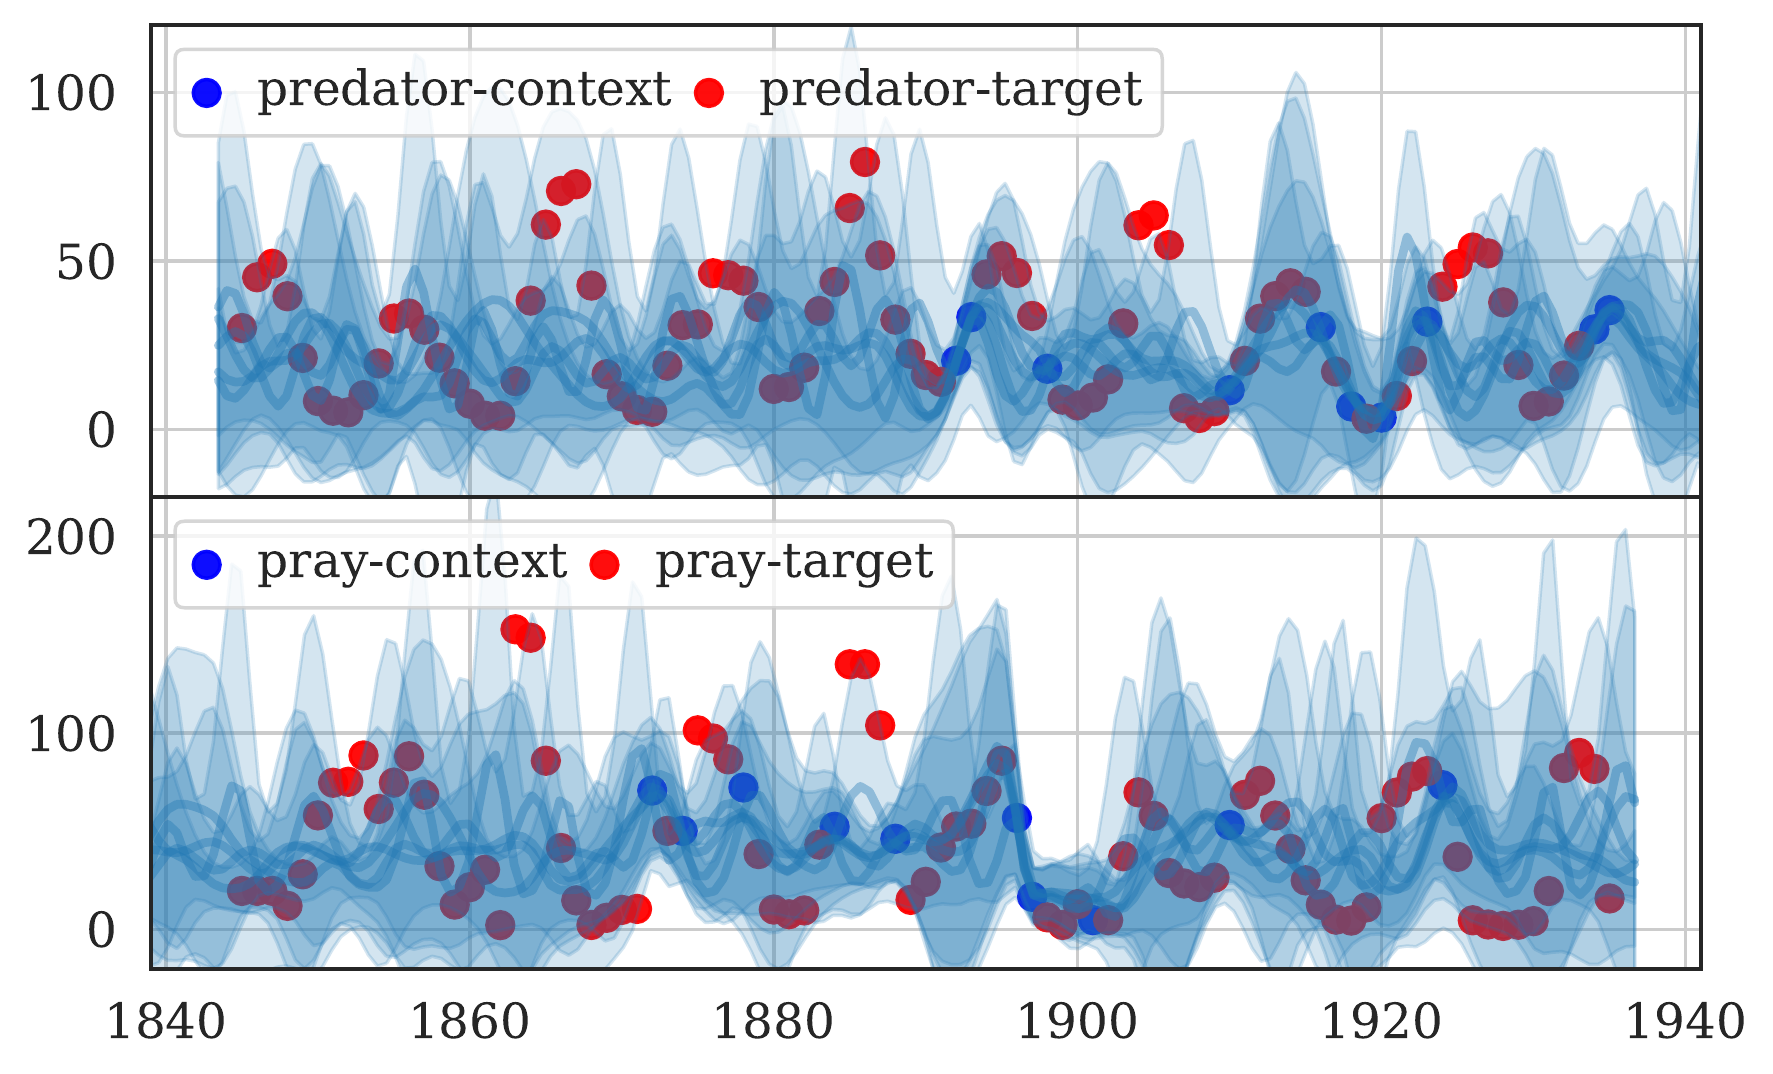}}
\subfloat[\label{fig:pray-10f}Proposed Model with Task2 ($N^c=10$)]{
 \includegraphics[width=0.49\linewidth]{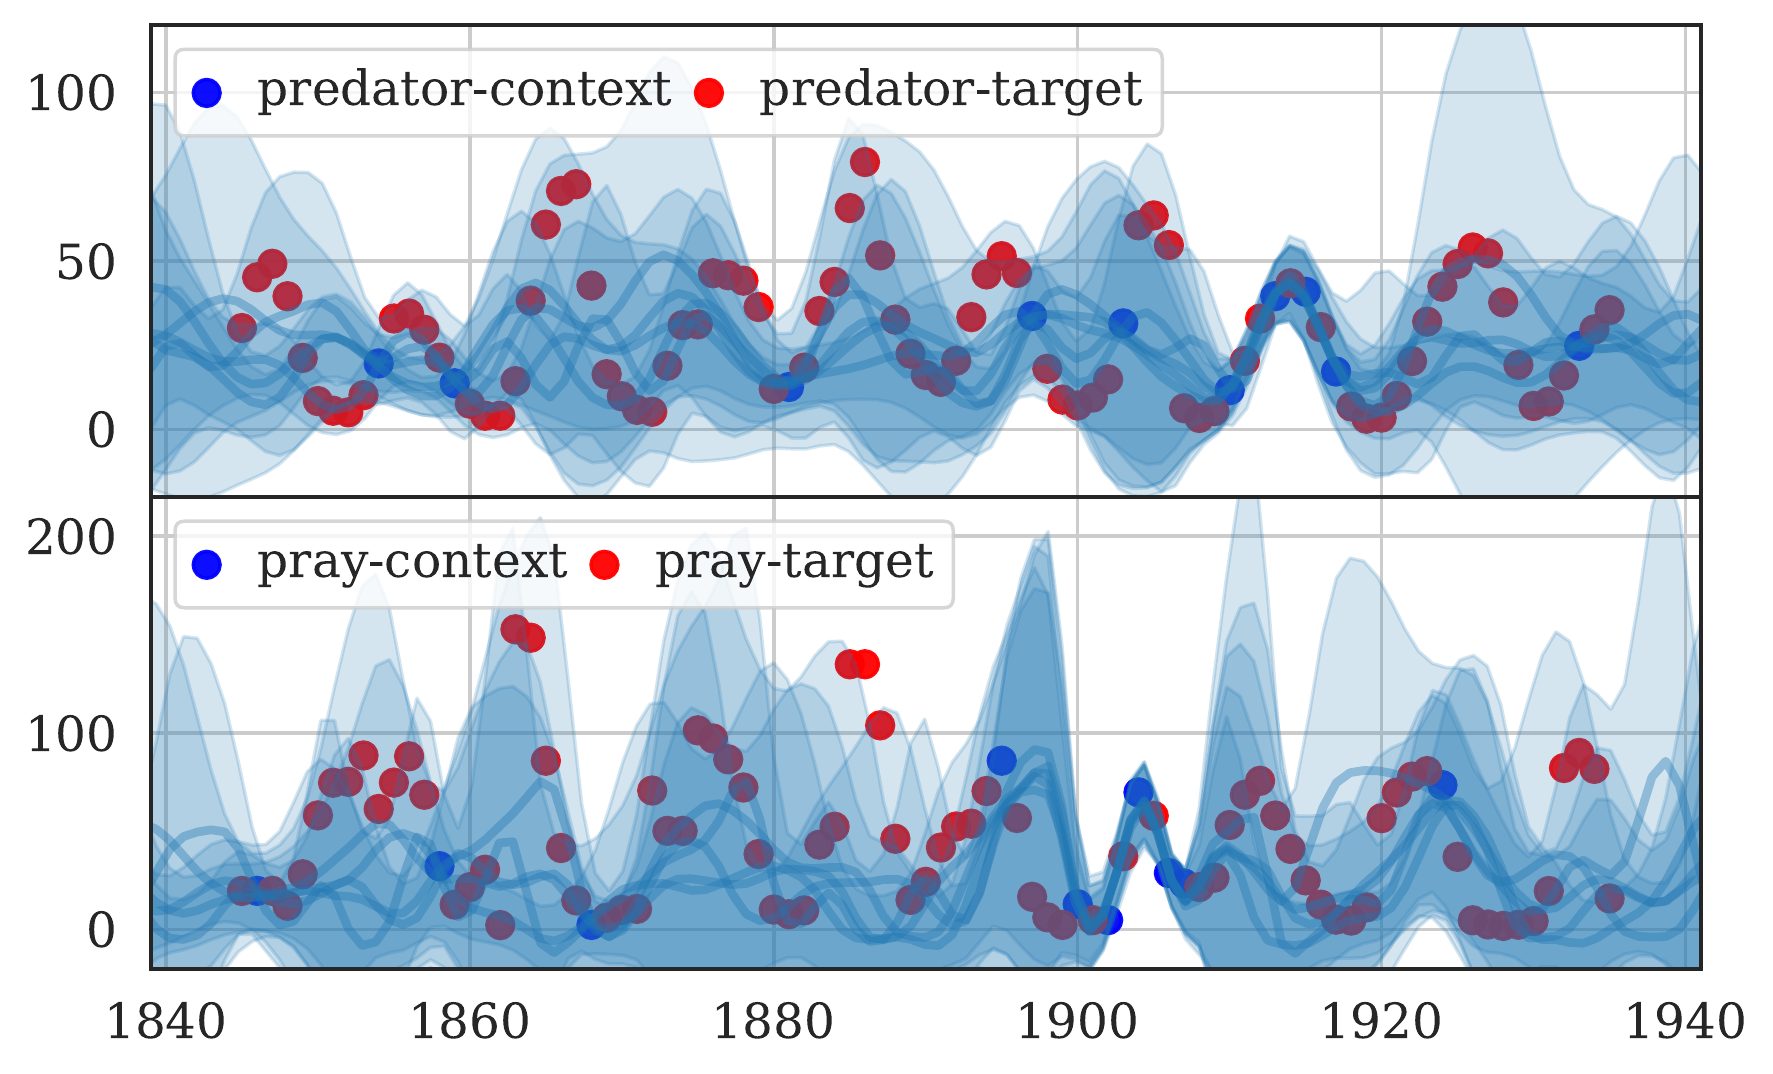}}

\caption{ Prediction results of \textb{Predator-Pray model with 10 context data points ($N^{c}=10$)}; \cref{fig:pray-10a,fig:pray-10b} shows the prediction results of 2 different tasks, respectively. \cref{fig:pray-10c,fig:pray-10d} correspond to the prediction results of GPConvCNP using 5 random functional representations. \cref{fig:pray-10e,fig:pray-10f} correspond to the prediction results of the proposed model using 5 random functional representations. These figures imply that how the random functional representations using prior affect the prediction on target sets when the small number of context data points is given}
\label{fig:predator-pray-10}
\end{figure*}

\vspace{-5mm}
\begin{figure*}[htp!]

% \subfloat[\label{fig:fig-h} \textb{mosm-varying}: $p_{\text{traninv-nn}}(X_c,Y_c)$ ]   
% {\includegraphics[width=0.41\linewidth,height=4.85cm]{Figures/07-appendix-exp2/mosm-varying/mosmvarying_datav11_deptrue_gpdep_weight.pdf}} 
\centering
\subfloat[\label{fig:pray-40a}ConvCNP with Task1 ($N^c=40$)]{
 \includegraphics[width=0.49\linewidth]{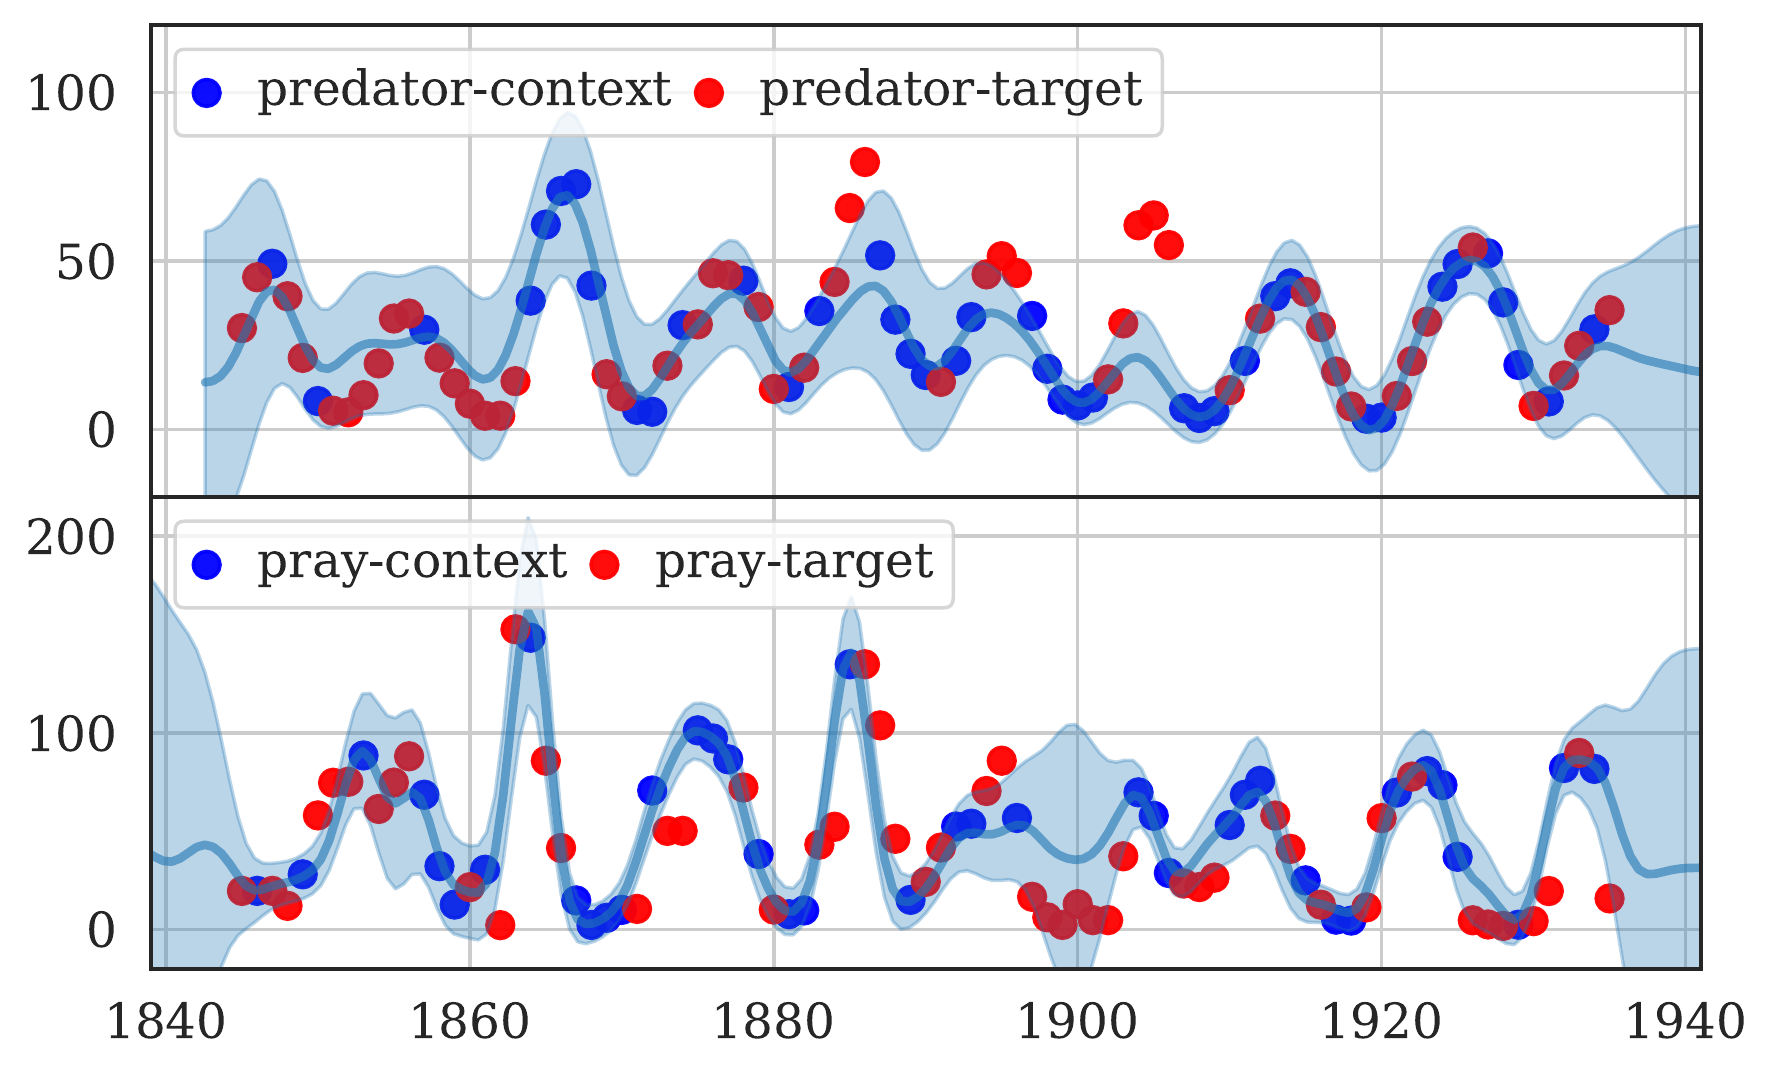}}
\subfloat[\label{fig:pray-40b}ConvCNP with Task2 ($N^c=40$)]{\includegraphics[width=0.49\linewidth]{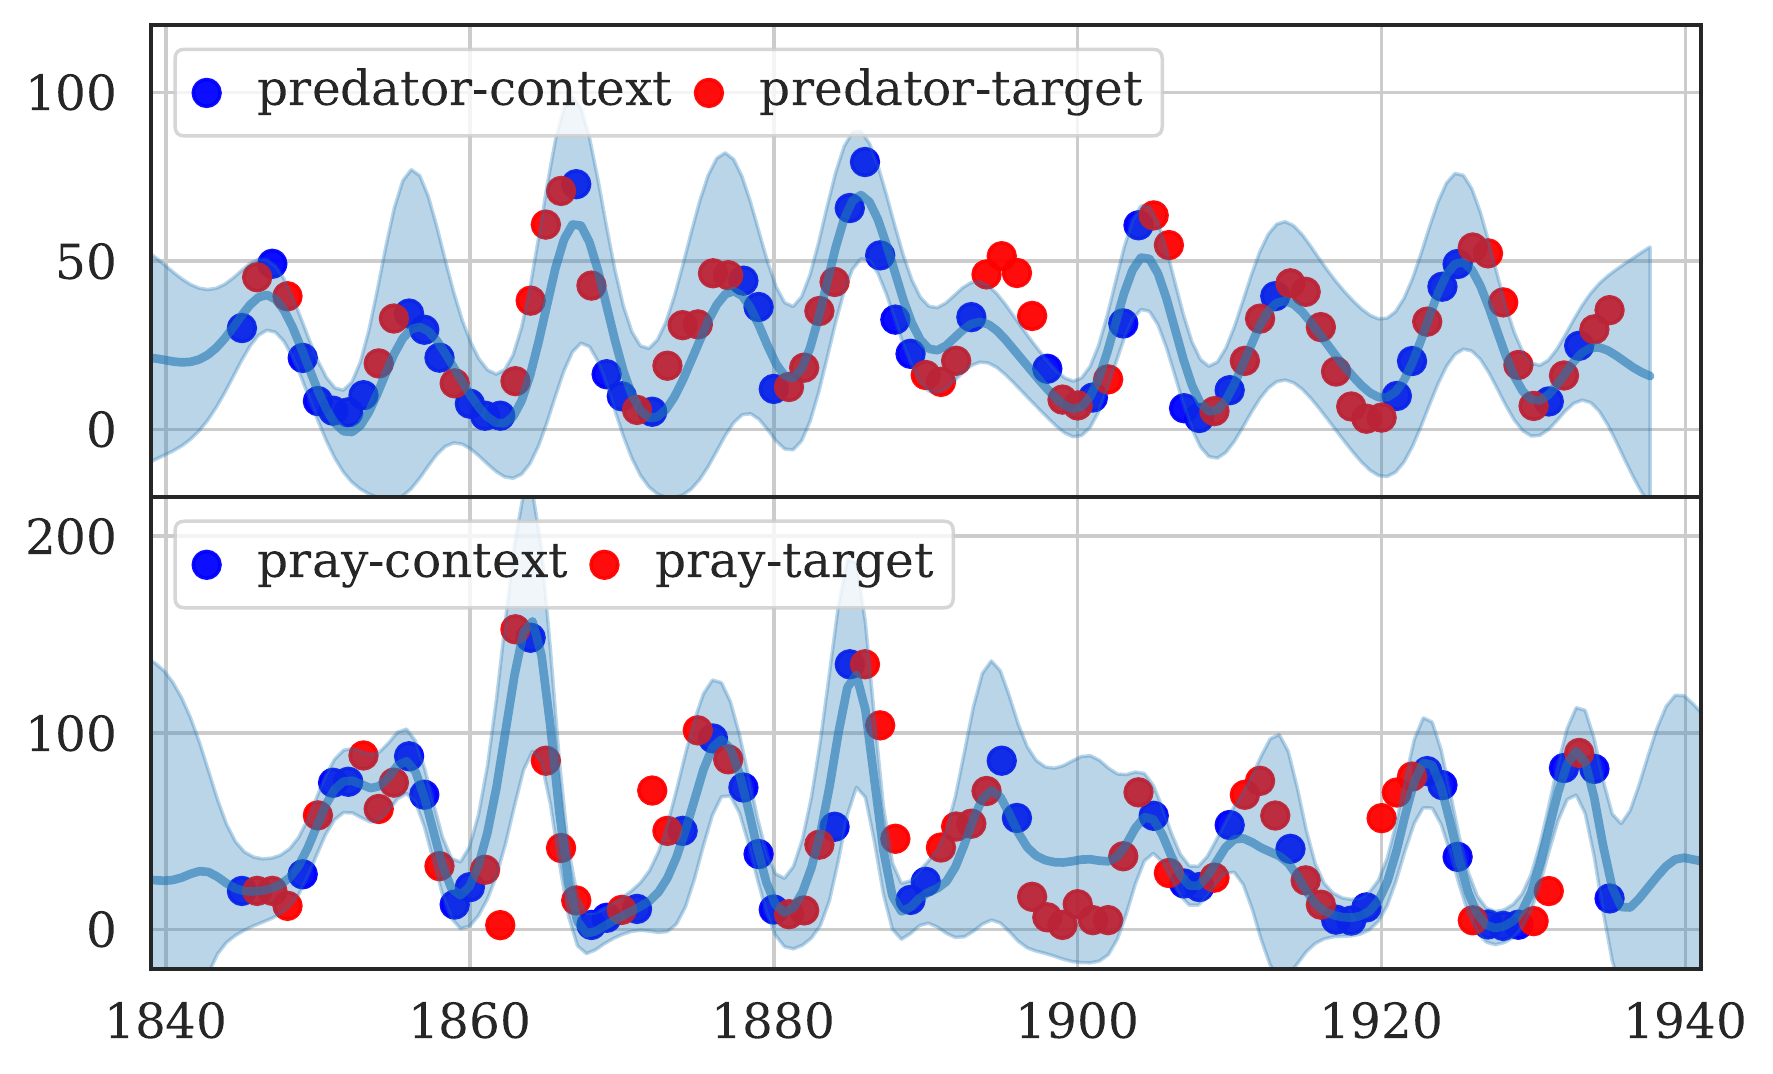}}

 \vspace{4mm}
\subfloat[\label{fig:pray-40c}GPConvCNP with Task1 ($N^c=40$)]{
 \includegraphics[width=0.49\linewidth]{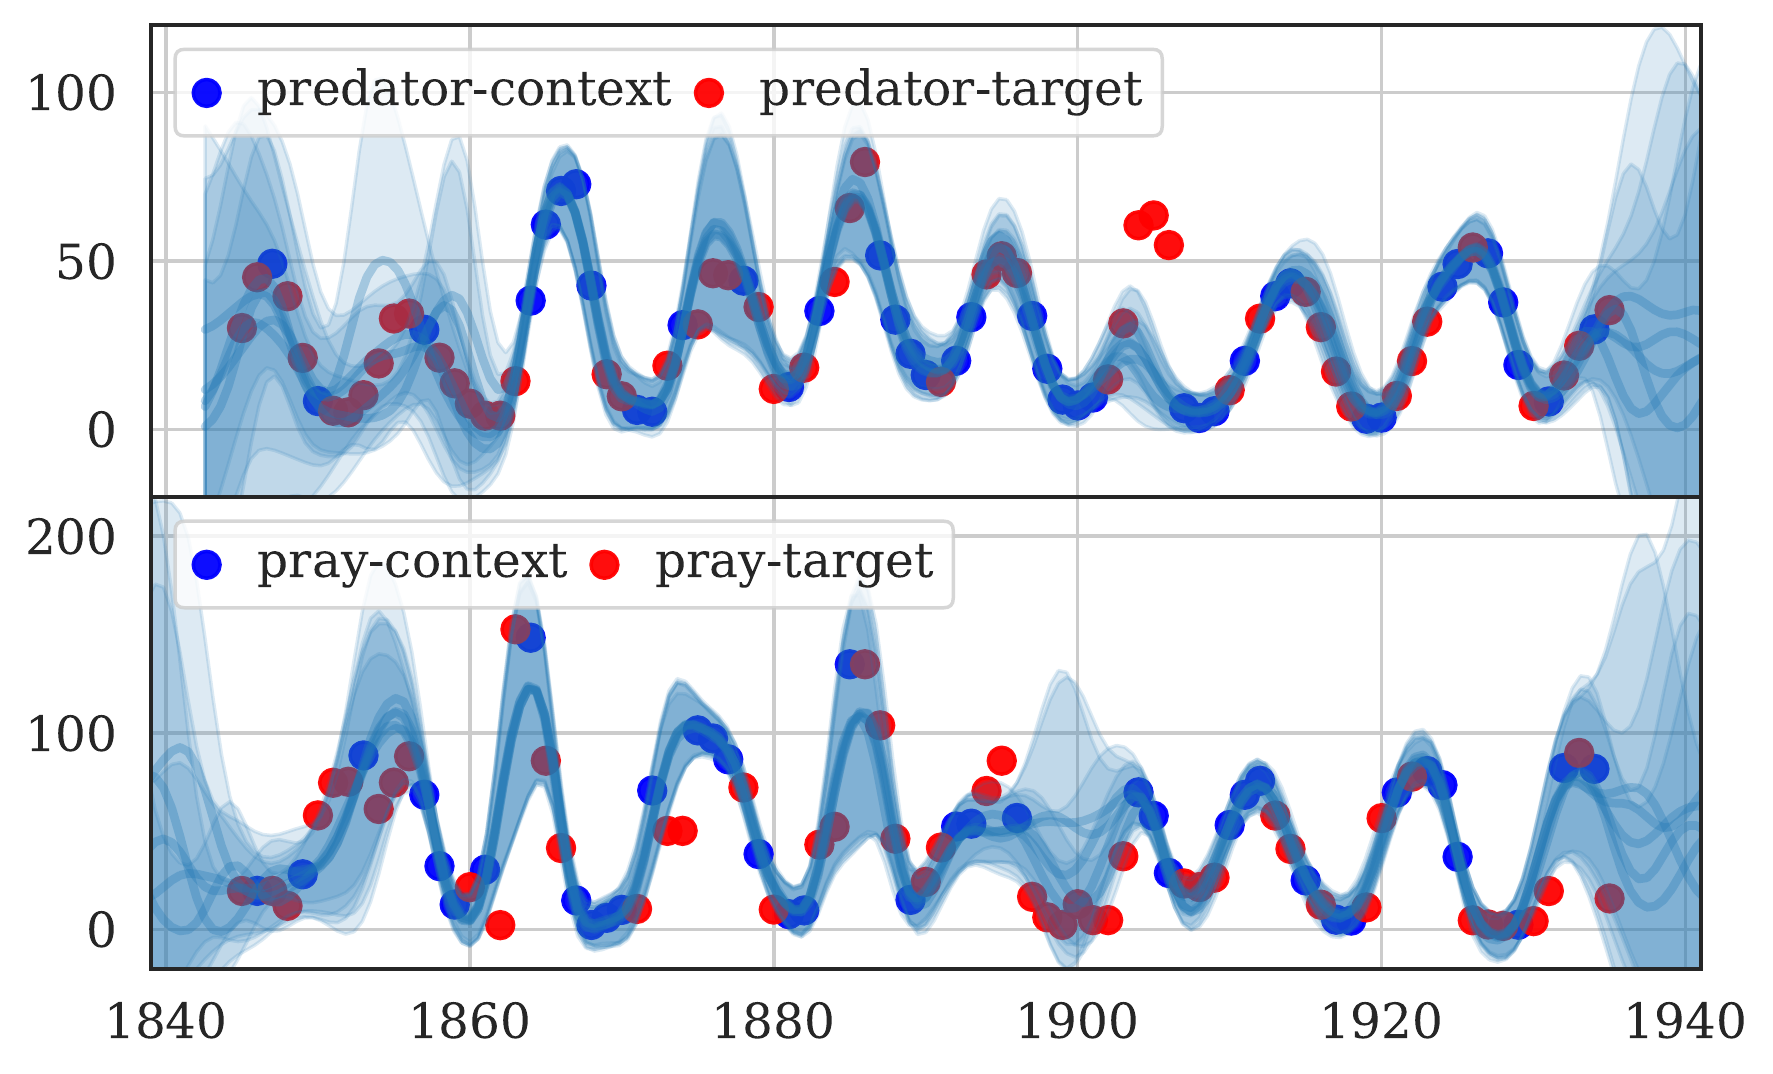}}
\subfloat[\label{fig:pray-40d}GPConvCNP with Task2 ($N^c=40$)]{
 \includegraphics[width=0.49\linewidth]{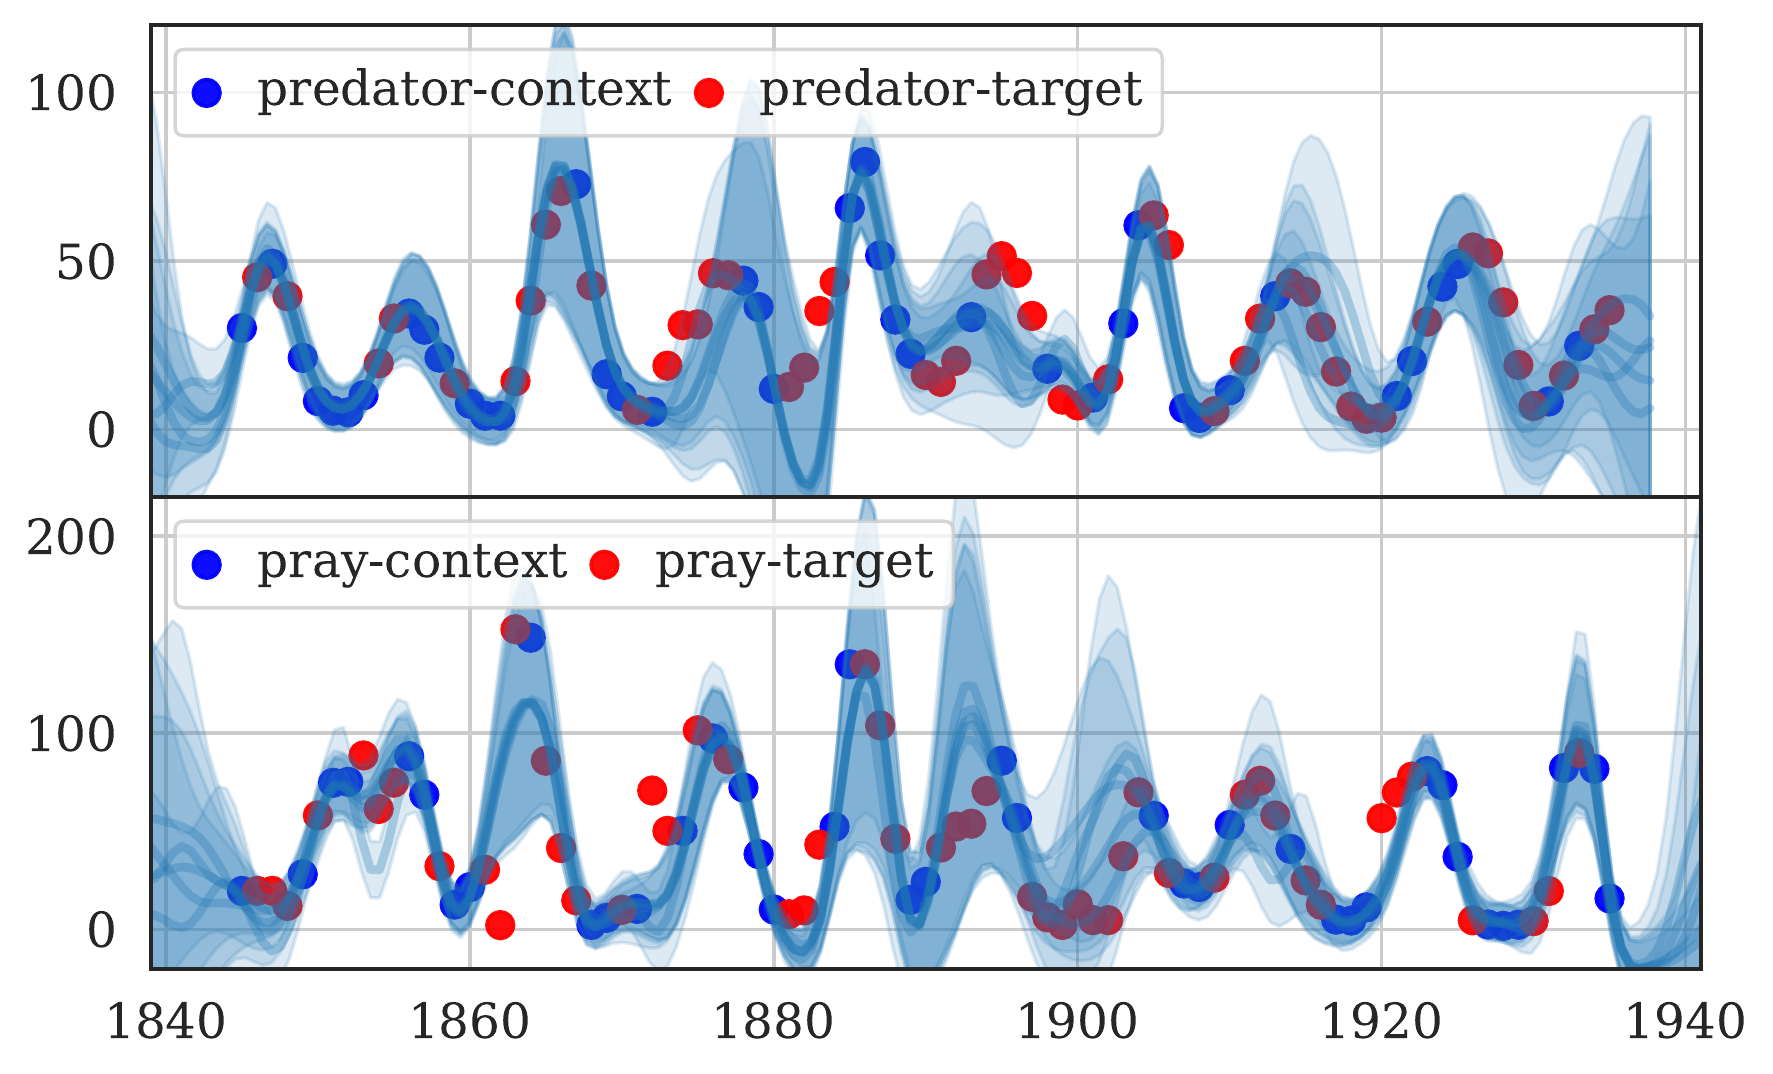}}
 
 \vspace{4mm}
\subfloat[\label{fig:pray-40e}Proposed Model with Task1 ($N^c=40$)]{
 \includegraphics[width=0.49\linewidth]{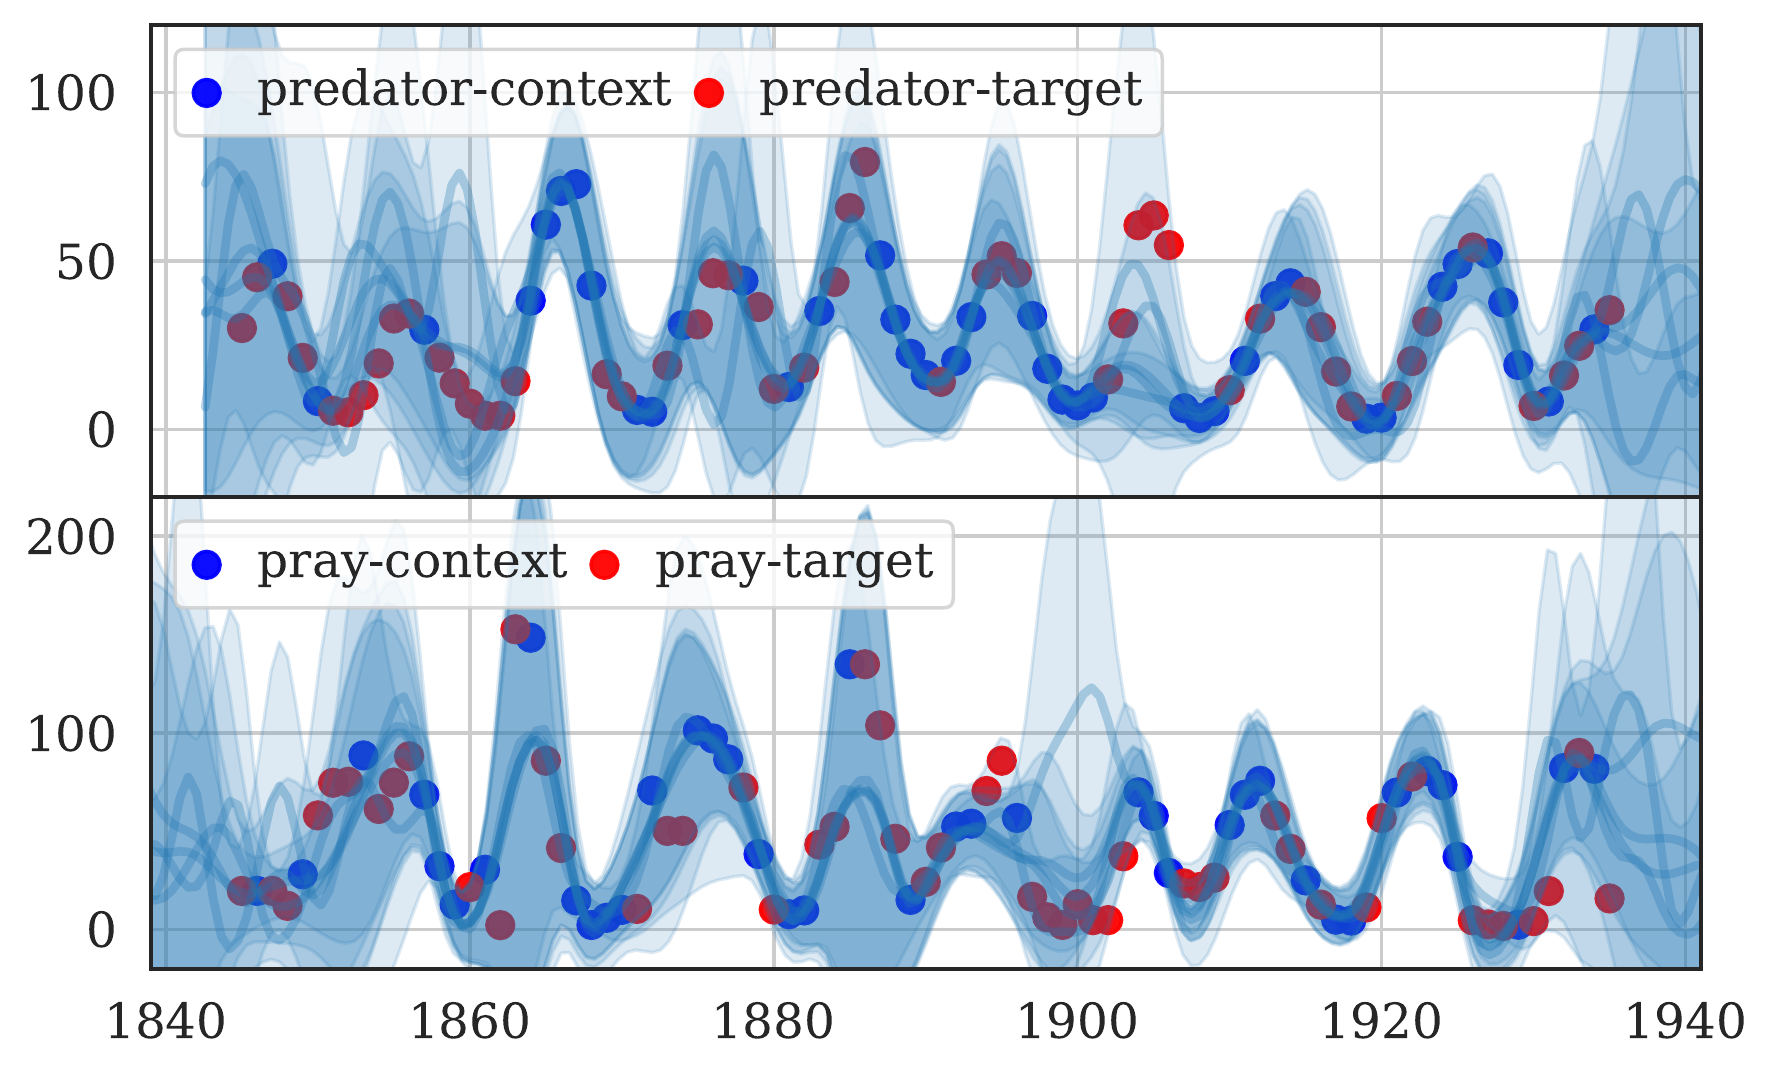}}
\subfloat[\label{fig:pray-40f}Proposed Model with Task2 ($N^c=40$)]{
 \includegraphics[width=0.49\linewidth]{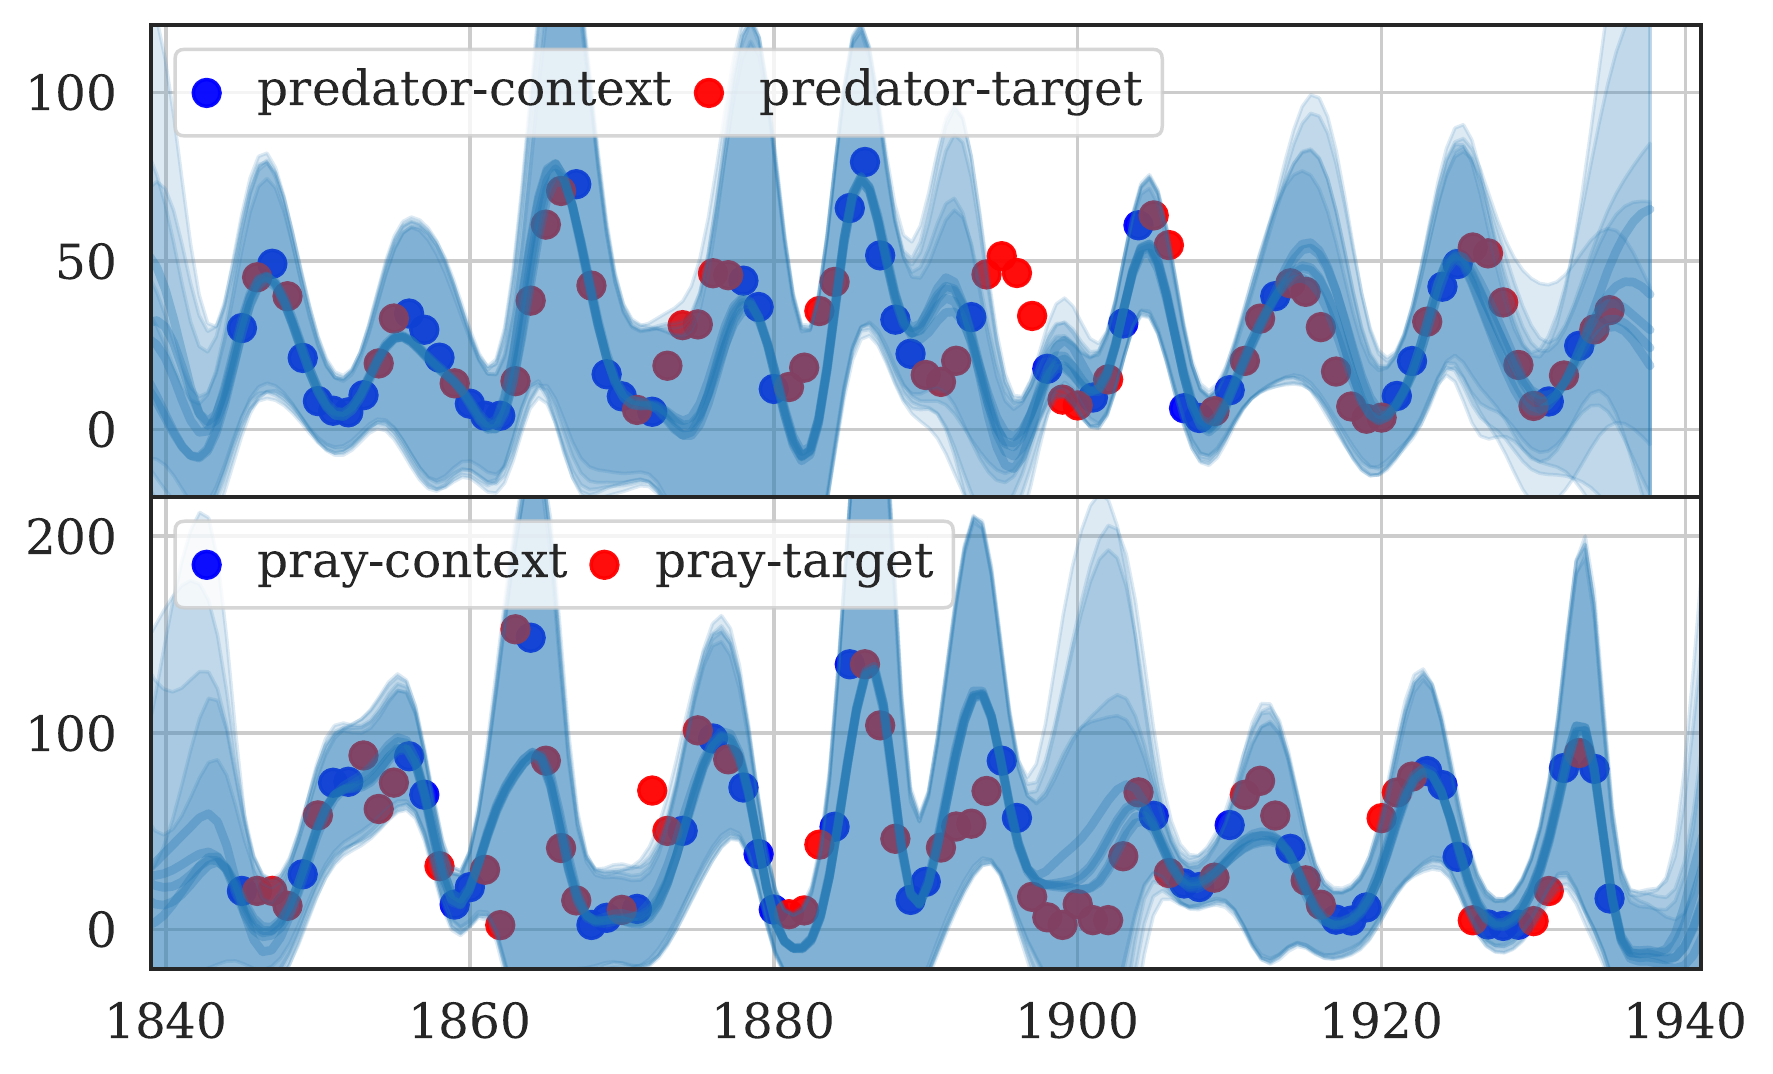}}

\caption{ Prediction results of \textb{Predator-Pray model with 40 context data points ($N^{c}=40$)}; \cref{fig:pray-40a,fig:pray-40b} shows the prediction results of 2 different tasks, respectively. \cref{fig:pray-40c,fig:pray-40d} correspond to the prediction results of GPConvCNP using 5 random functional representations. \cref{fig:pray-40e,fig:pray-40f} correspond to the prediction results of the proposed model using 5 random functional representations. These figures imply the task-dependent prior enables more robust predictions as shown in \cref{fig:pray-40e,fig:pray-40f} compared to GPConvCNP as shown in \cref{fig:pray-40c,fig:pray-40d}}
\label{fig:predator-pray-40}
\end{figure*}

\vspace{-5mm}
\begin{figure*}[htp!]

% \subfloat[\label{fig:fig-h} \textb{mosm-varying}: $p_{\text{traninv-nn}}(X_c,Y_c)$ ]   
% {\includegraphics[width=0.41\linewidth,height=4.85cm]{Figures/07-appendix-exp2/mosm-varying/mosmvarying_datav11_deptrue_gpdep_weight.pdf}} 
\centering
\subfloat[\label{fig:pray-70a} ConvCNP with Task1 ($N^c=70$)]{
 \includegraphics[width=0.49\linewidth]{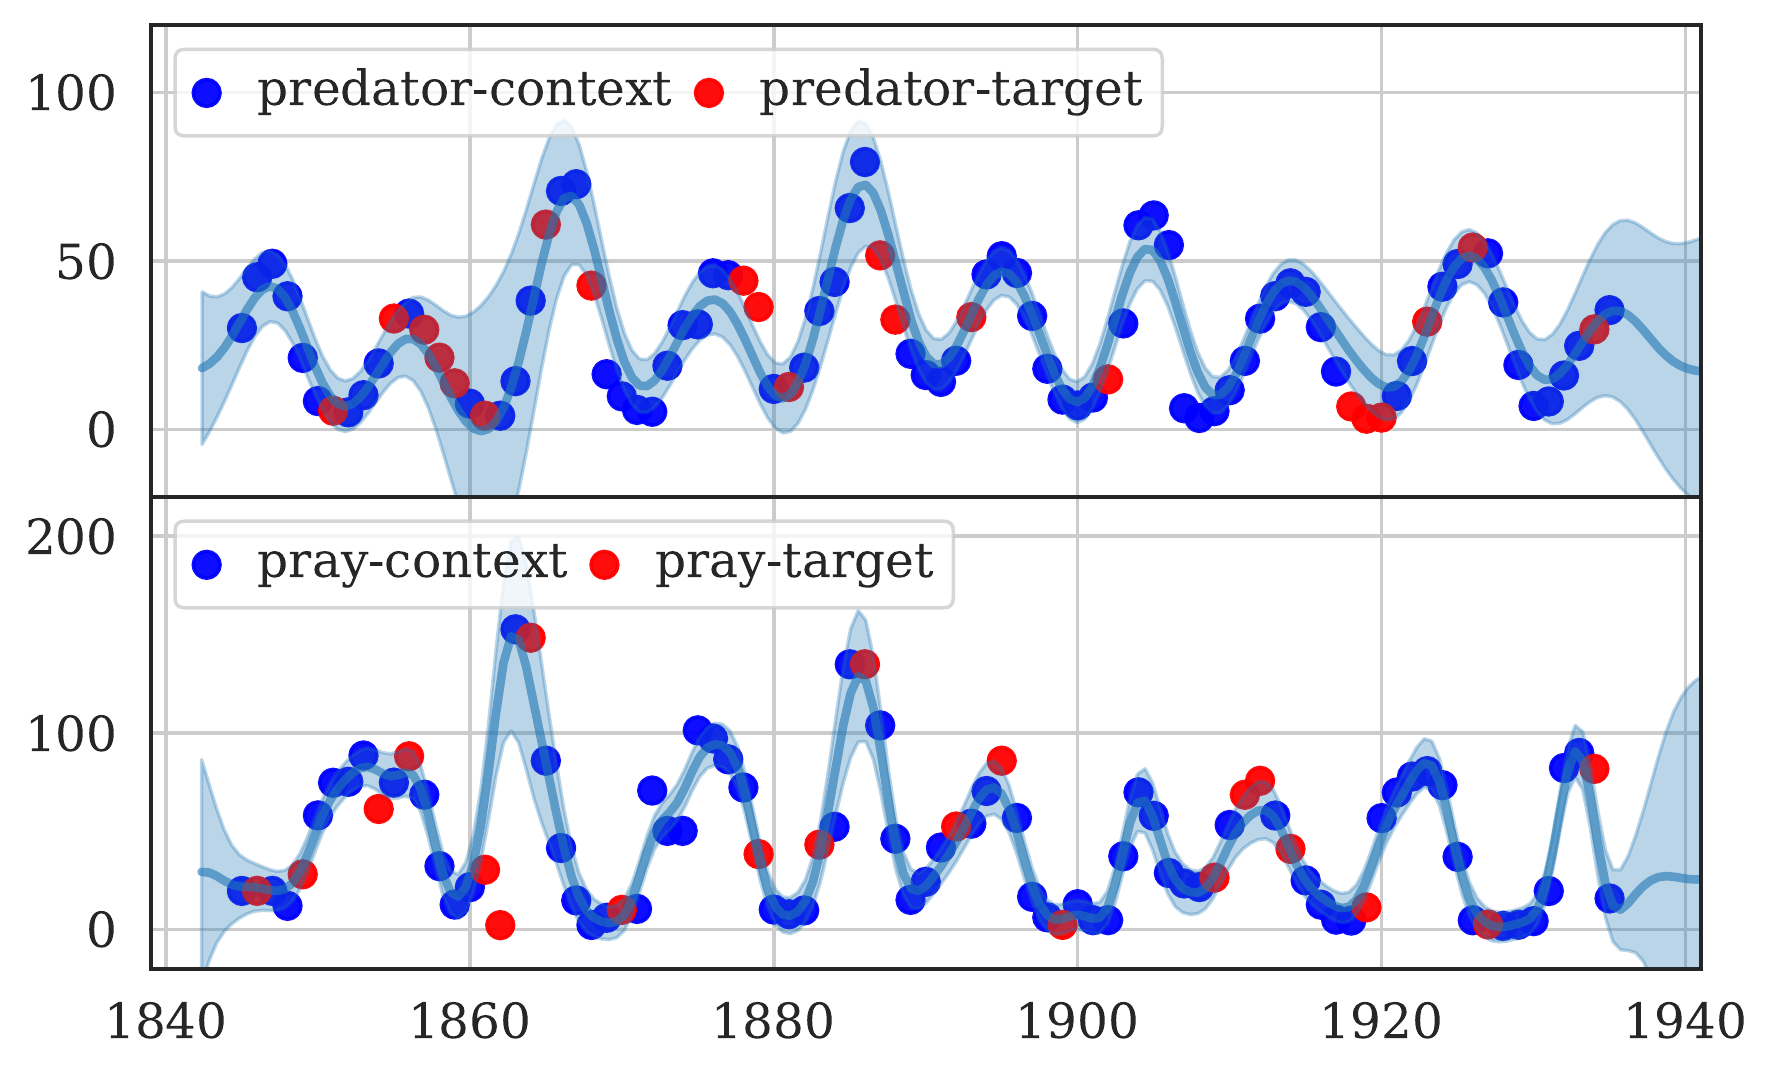}}
\subfloat[\label{fig:pray-70b} ConvCNP with Task2 ($N^c=70$)]{\includegraphics[width=0.49\linewidth]{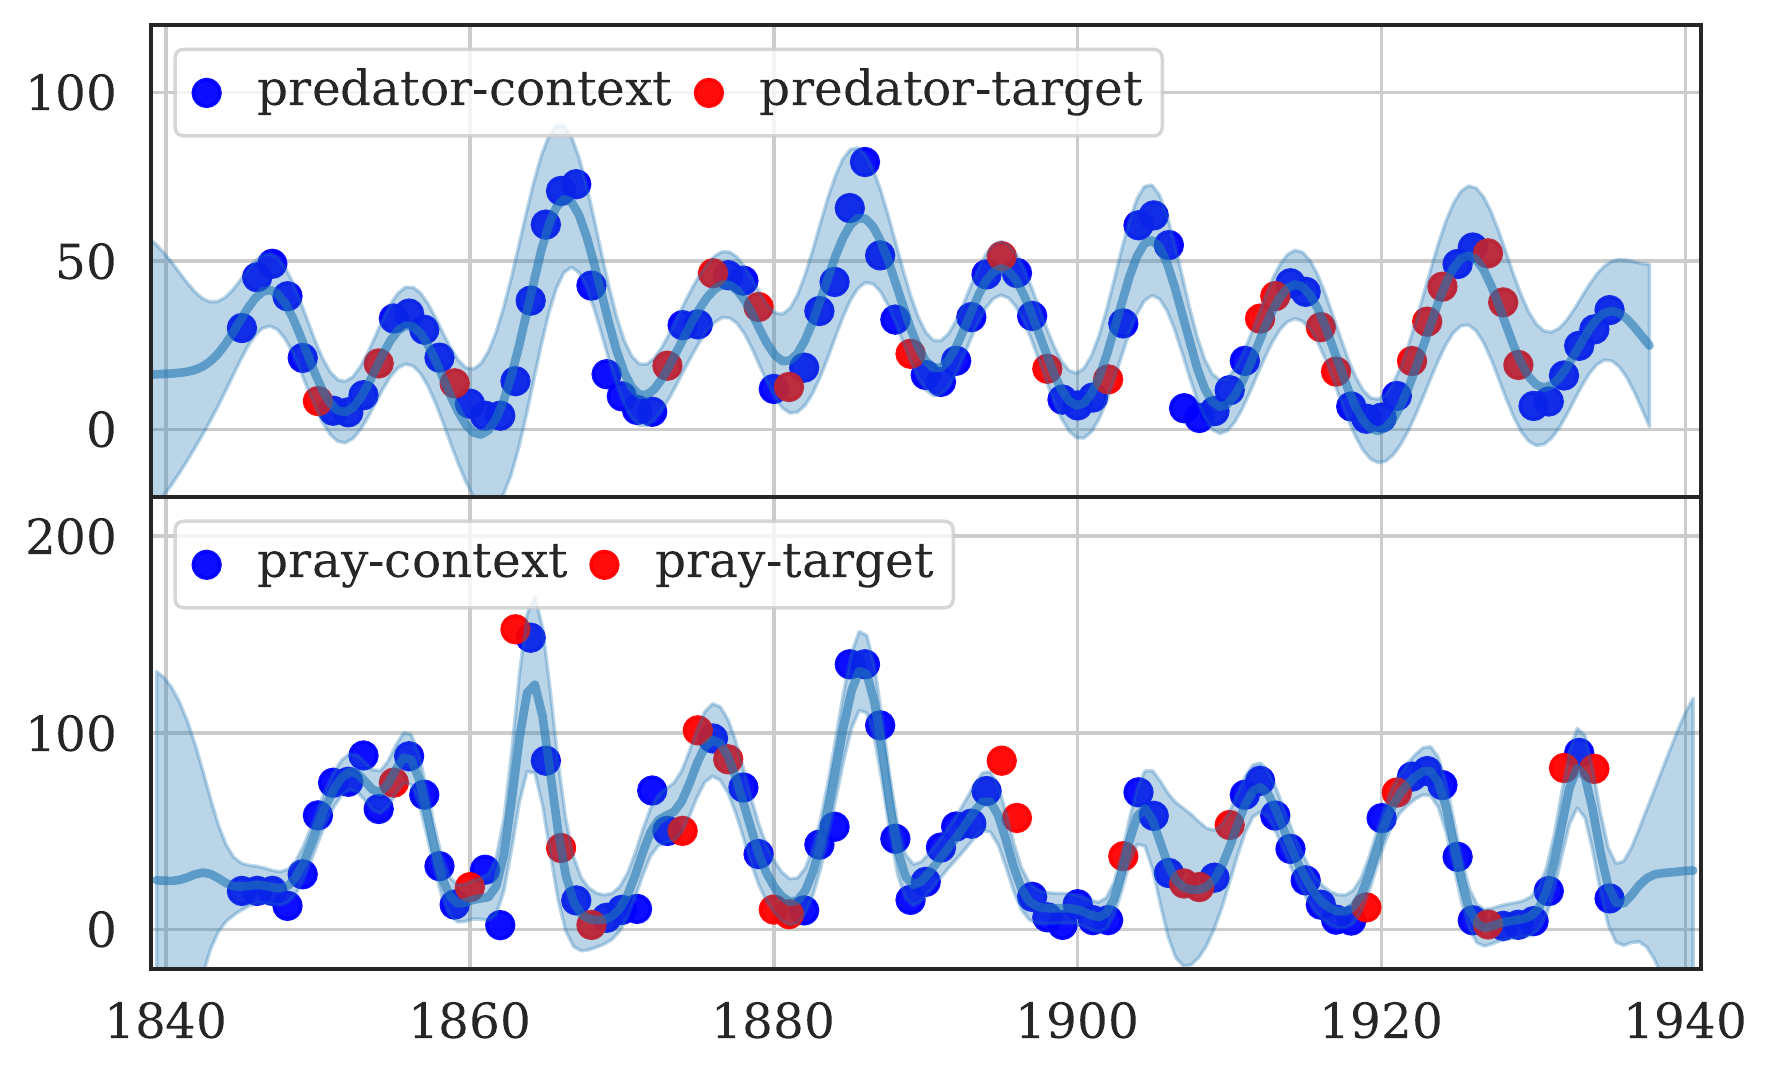}}

 \vspace{4mm}
\subfloat[\label{fig:pray-70c} GPConvCNP with Task1 ($N^c=70$)]{
 \includegraphics[width=0.49\linewidth]{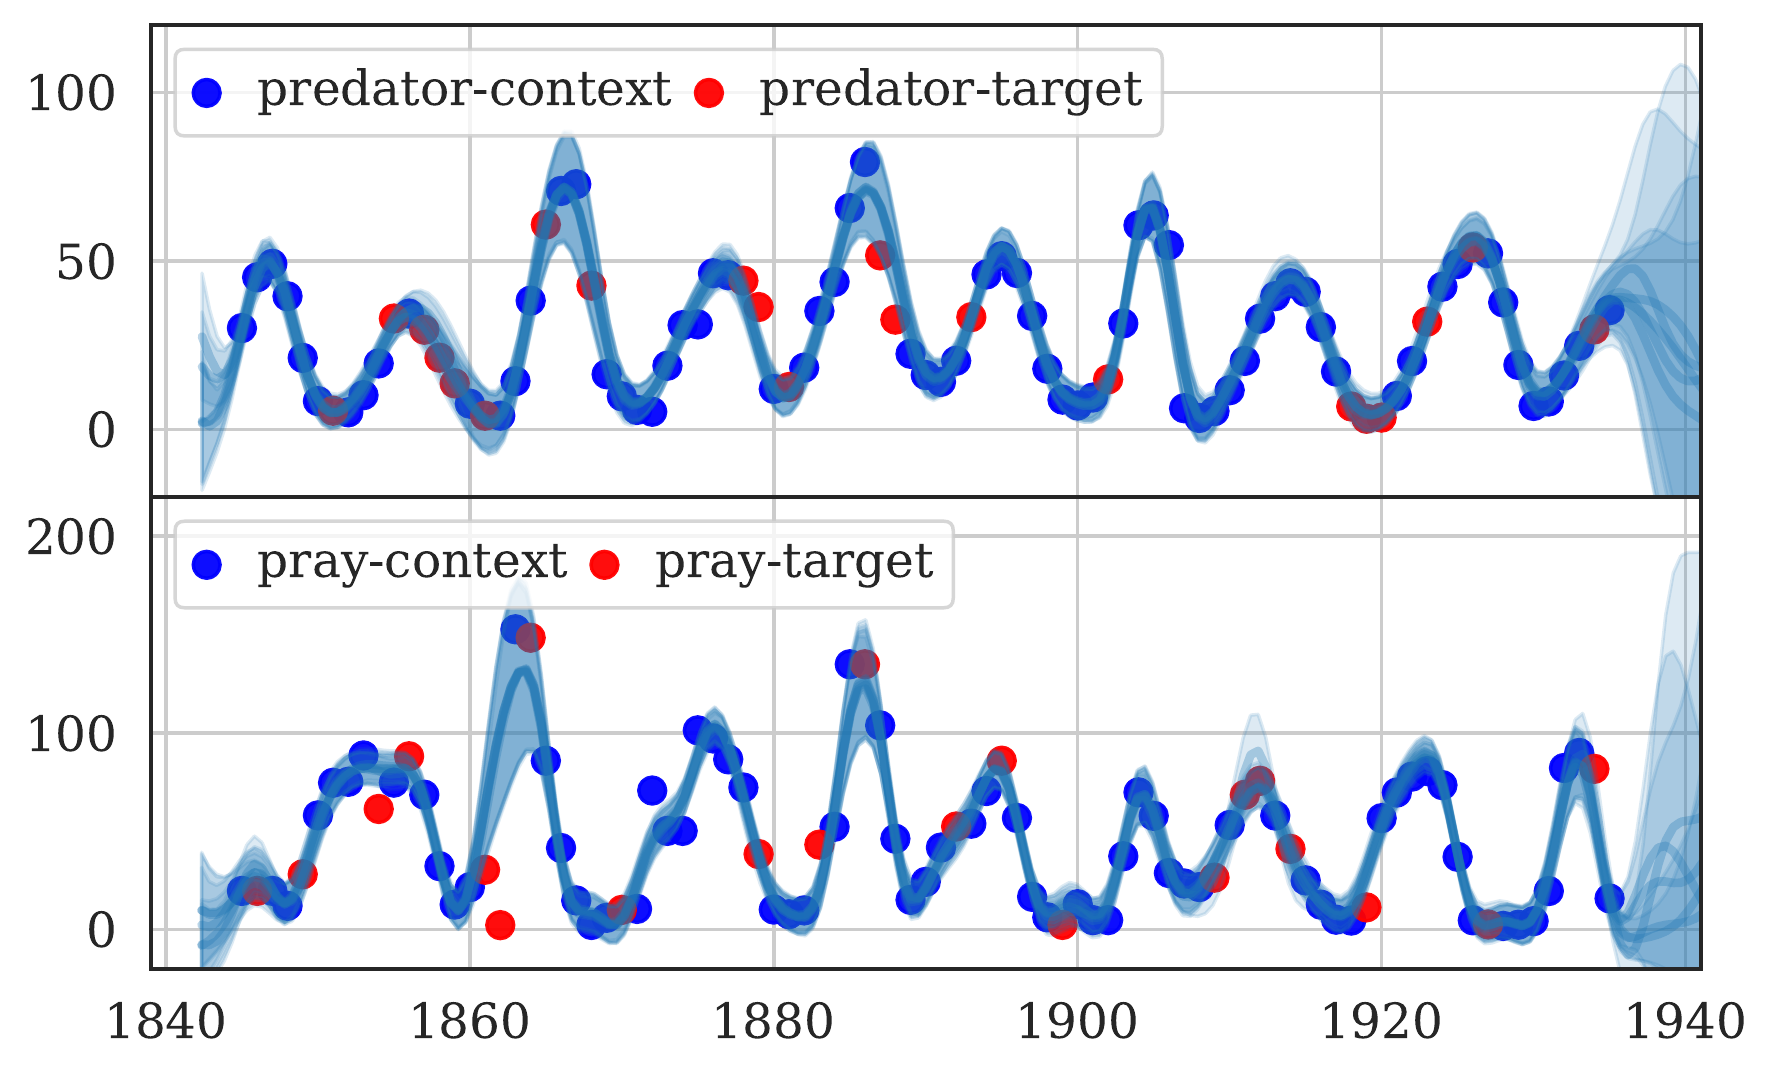}}
\subfloat[\label{fig:pray-70d} GPConvCNP with Task2 ($N^c=70$)]{
 \includegraphics[width=0.49\linewidth]{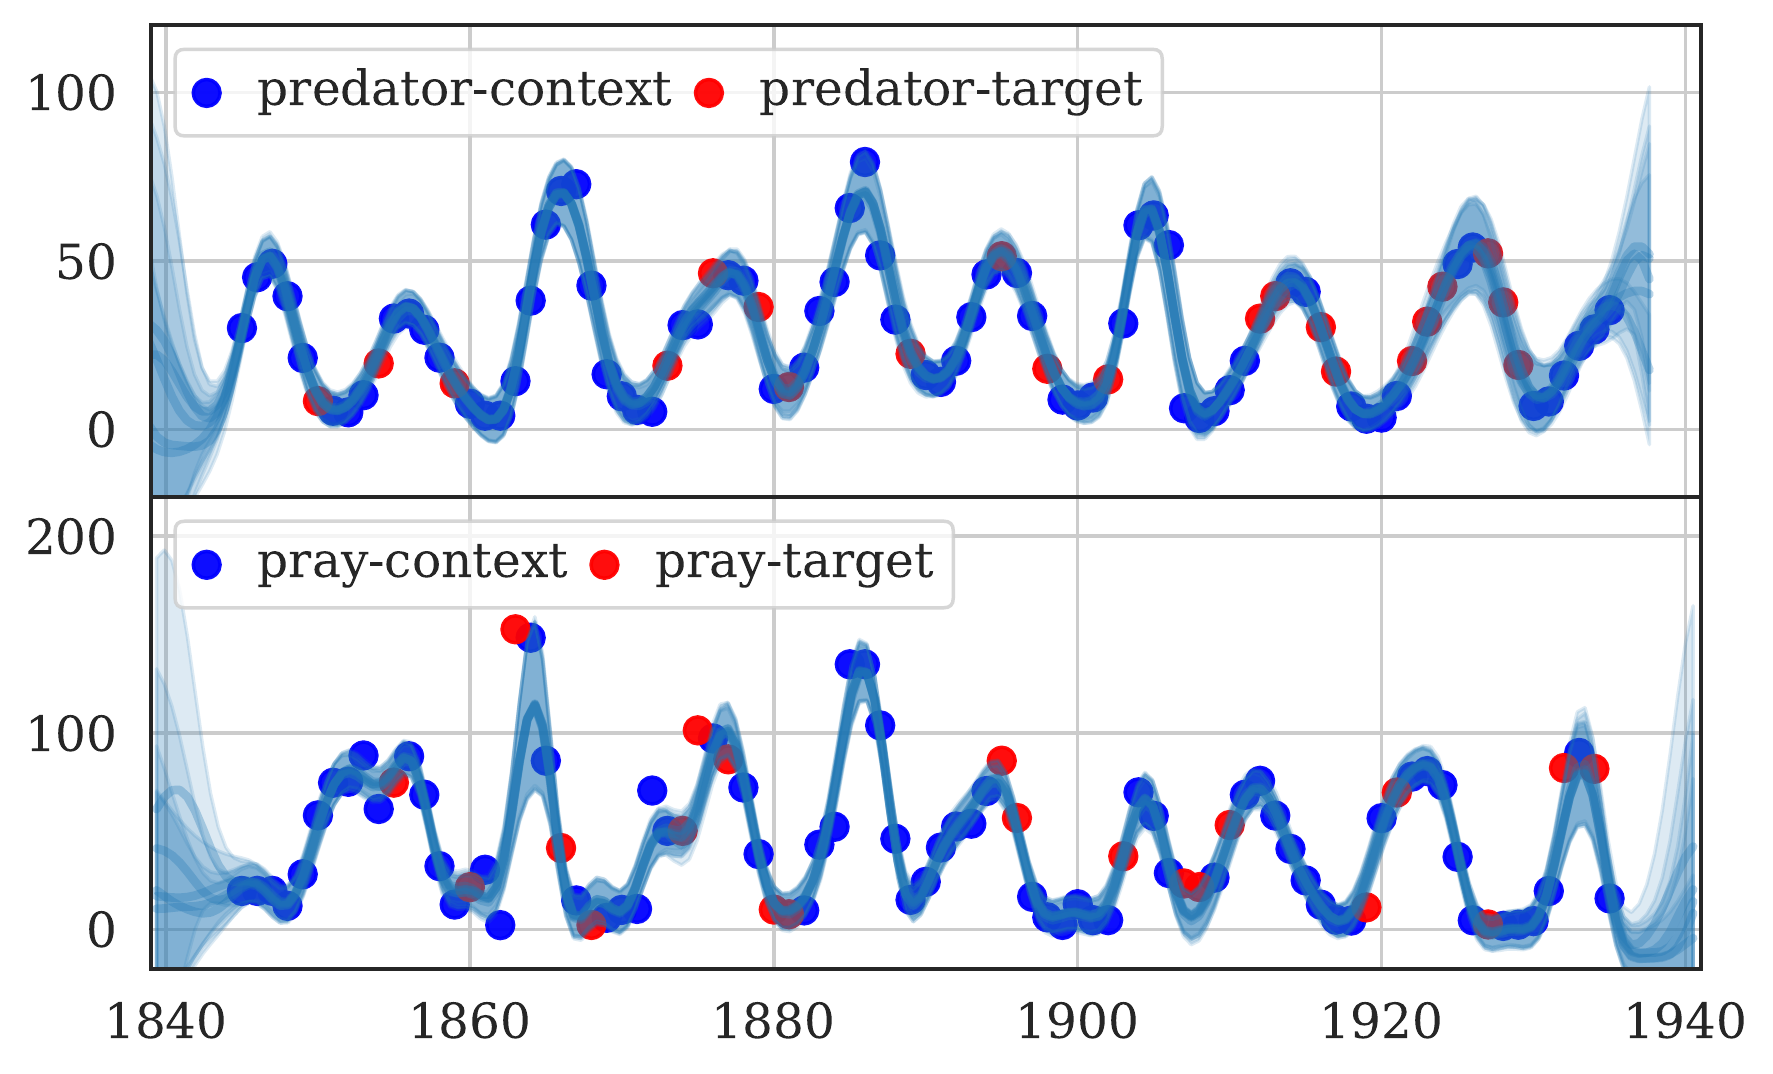}}
 
 \vspace{4mm}
\subfloat[\label{fig:pray-70e}Proposed Model with Task1 ($N^c=70$)]{
 \includegraphics[width=0.49\linewidth]{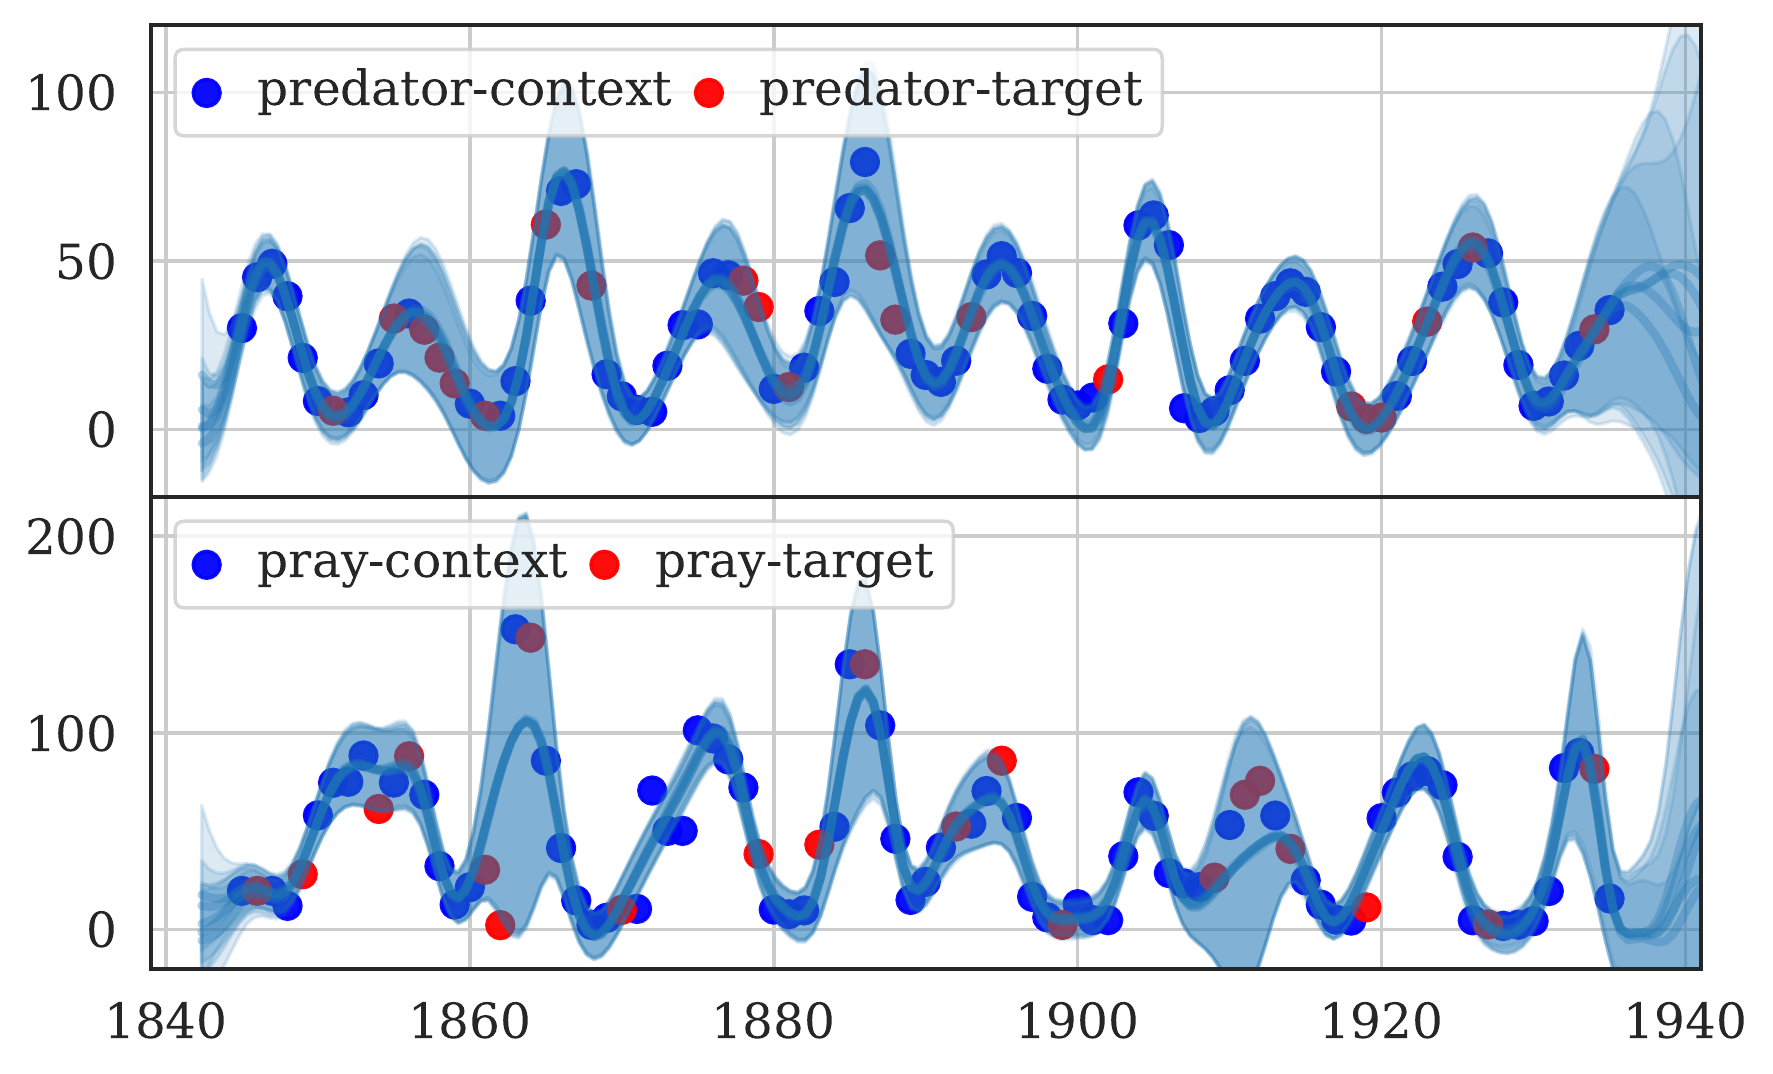}}
\subfloat[\label{fig:pray-70f}Proposed Model with Task2 ($N^c=70$)]{
 \includegraphics[width=0.49\linewidth]{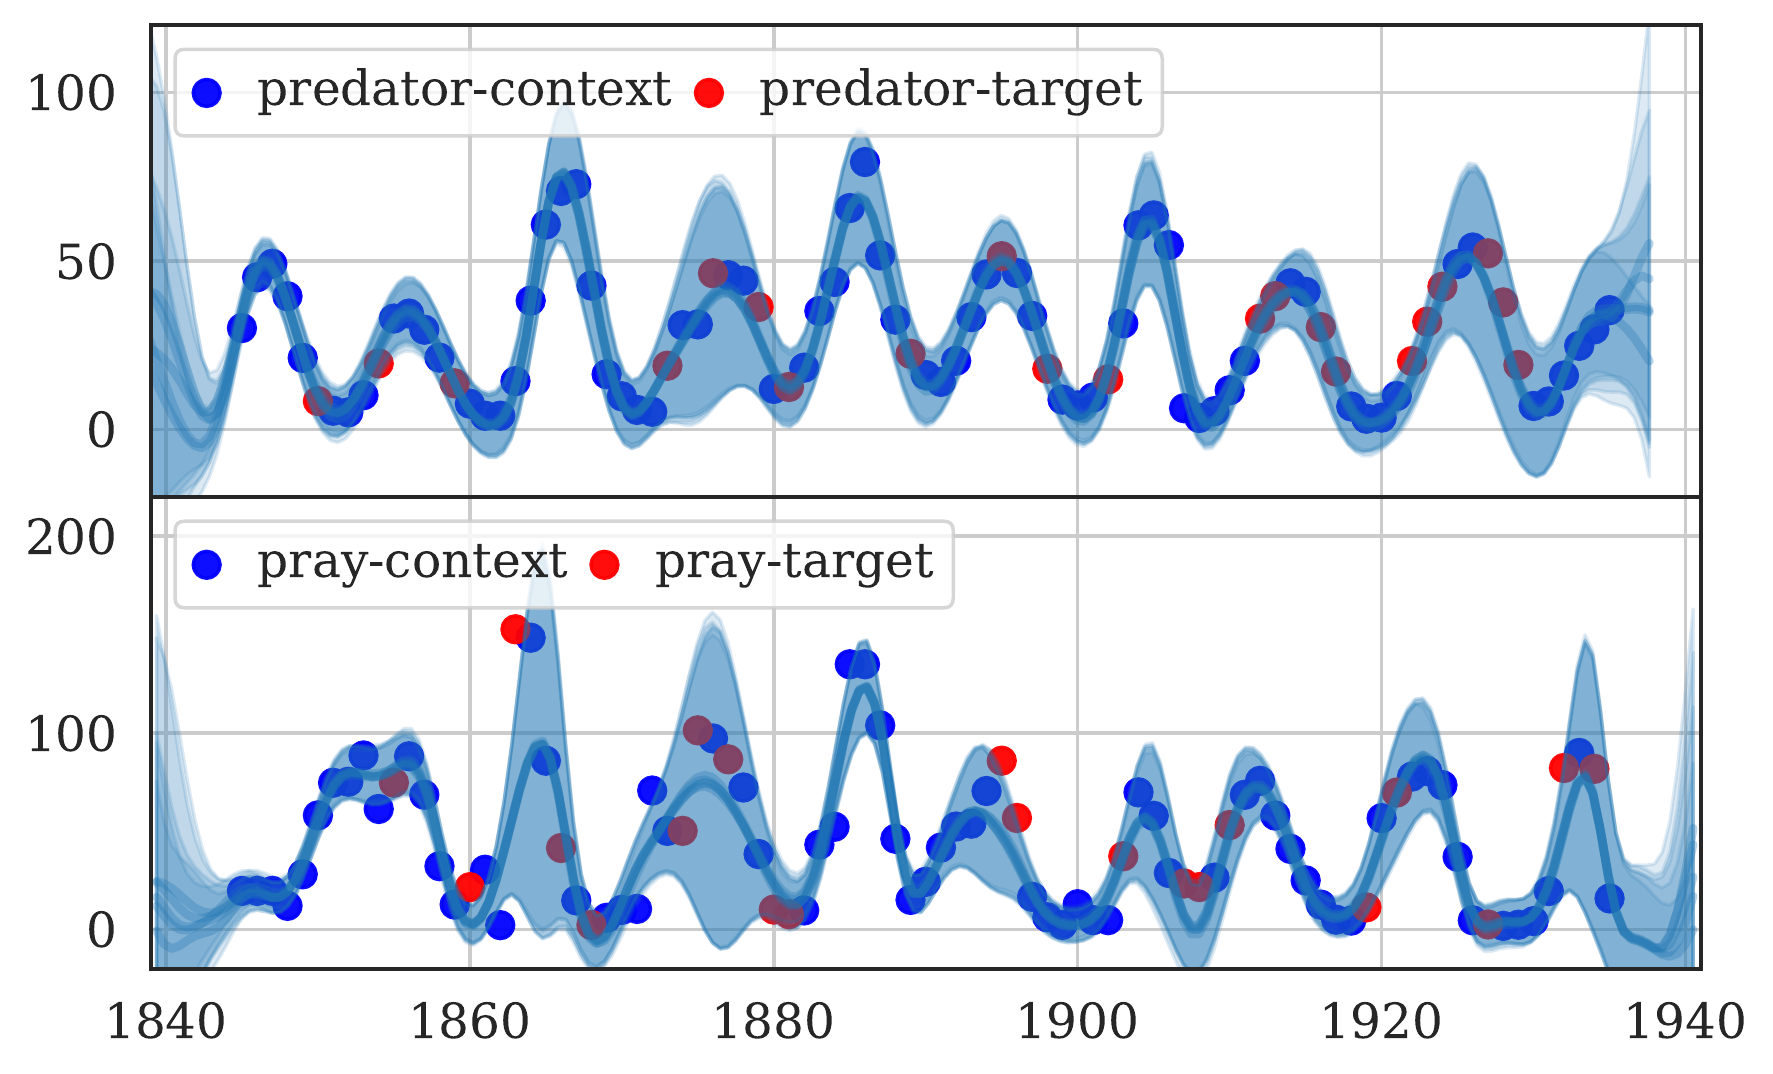}}

\caption{Prediction results of \textb{Predator-Pray model with 70 context data points ($N^{c}=70$)}; \cref{fig:pray-70a,fig:pray-70b} shows the prediction results of 2 different tasks, respectively. \cref{fig:pray-70c,fig:pray-70d} correspond to the prediction results of GPConvCNP using 5 random functional representations. \cref{fig:pray-70e,fig:pray-70f} correspond to the prediction results of the proposed model using 5 random functional representations. These figures imply  that all models obtain similar predictive distribution on target sets when the large number of context data points is given.}
\label{fig:predator-pray-70}
\end{figure*}
\clearpage

% \input{07-appendix-v01-chapter5-expelse}
% \clearpage
