# Supplementary material for: Bayesian Convolutional Deep Sets with Task-Dependent Stationary Prior
Source: arXiv:2210.12363 source file (2022-10-22)
Supplement: Supplementary file 6 [file 07-appendix-v01-algorithm-01.tex]

%----------------------------------------------------
% off-grid
%----------------------------------------------------
\begin{algorithm}[htp!]
\caption{Forward pass of the NP model via Bayesian ConvDeepsets (off-grid) }
\label{alg:BayesConvDeepsets}
    \begin{algorithmic}[1]
    %\Require $\rho = (\text{CNN}, \psi_\rho)$, $\psi$, and density $\zeta$ 
    \Require Model parameters: $\Theta$
    \Require The number of basis stationary kernels $Q$, the number of sampled spectral points $l$
    \Require Context set $D^{c}=\{(x^{c}_n, y^{c}_n)\}_{n=1}^{N^{c}}$, target inputs $X^{t}= \{x^{t}_n\}_{n=1}^{N^{t}}$ 
    \State Compute the discretized inputs $\{t_m\}_{m=1}^{M}$ by spacing inputs range $[\mathrm{min}\{X^{c},X^{t}\},\mathrm{max}\{X^{c},X^{t}\}]$ linearly.
    \State Select the task-dependent stationary prior as described in \textb{Eq. (11)}    
    \State Construct $N$ random functional representation $\{f_{(n)}(D^{c})(\bigcdot)\}_{n=1}^{N}$ on $\mathcal{I}$ as described in \textb{Eqs. (12-16)}.
    \State Construct $N$ random representations $\{\Phi^{\mathcal{B}}_{(n)}(D^{c})(\bigcdot)\}_{n=1}^{N}$ on finite grid points $\{t_m\}_{m=1}^{M}$ as described in \textb{Eq. (17)}.  
    \State Smooth $N$ random representations $\{\Phi^{\mathcal{B}}_{(n)}(D^{c})(\bigcdot)\}_{n=1}^{N}$ on target inputs $X^{t}$ by \textb{Eq. (6)}.  
    \State Generate $N$ predictive distributions $\{p \big( Y^{t} \ | \  X^{t},\Phi^{\mathcal{B}}_{(n)} \big) \}_{n=1}^{N}$ on target inputs $X^{t}$ by \textb{Eq. (20)}.
\end{algorithmic}
\end{algorithm}

%----------------------------------------------------
% on-grid
%----------------------------------------------------
\begin{algorithm}[htp!]
\caption{Forward pass of the NP model via Bayesian ConvDeepsets (on-grid) }
\label{alg:BayesConvDeepsets}
    \begin{algorithmic}[1]
    %\Require $\rho = (\text{CNN}, \psi_\rho)$, $\psi$, and density $\zeta$ 
    \Require Model parameters: $\Theta$
    \Require The number of basis stationary kernels $Q$, the number of sampled spectral points $l$
    \Require Context set $D^{c}=\{(x^{c}_n, y^{c}_n)\}_{n=1}^{N^{c}}$, target inputs $X^{t}= \{x^{t}_n\}_{n=1}^{N^{t}}$ on grid.
    \State Extract the context inputs $\sum_{n=1}^{N^{c}} \delta (\bigcdot -  x^{c}_n ) $
    and outputs  $\sum_{n=1}^{N^{c}} y^{c}_n   \delta (\bigcdot -  x^{c}_n ) $            on grid.
    \State Construct $N$ random functional representation $\{f_{(n)}(D^{c})(\bigcdot)\}_{n=1}^{N}$ on given grid as described in \textb{Eq. (12)}.
    \State Map $N$ random representations on grid where the $n$-th representation $f^M_{(n)}$ is computed as $$f^M_{(n)} = \mathrm{CNN}\left(\left[\sum_{n=1}^{N^{c}} \delta (\bigcdot -  x^{c}_n ) \ , \ \Phi^{\mathcal{B}}_{(n)}(D^{c})(\bigcdot) \right]\right).$$ \vspace{-1mm}  
    \State  Generate $N$ predictive distributions for target set with the $n$-th predictive mean $\mu^{t}_{(n)}$ and standard deviation $\sigma^{t}_{(n)}$,  \vspace{-1mm} $$\mu^{t}_{(n)}  \ , \ \sigma^{t}_{(n)} = f^M_{(n)} \circ  \left(\sum_{n=1}^{N^{t}} \delta (\bigcdot -  x^{t}_n ) \right).   $$ \vspace{-1mm}
\end{algorithmic}
\end{algorithm}
