# Supplementary material for: Bayesian Convolutional Deep Sets with Task-Dependent Stationary Prior
Source: arXiv:2210.12363 source file (2022-10-22)
Supplement: Supplementary file 7 [file 07-appendix-v01-chapter1-method.tex]

\section{Further Details for the Proposed Methodology  }
\label{appendix:details-propose}

%\paragraph{Implementations.}
\subsection{Implementations}
\label{appendix:details-algorithm}

We explain how the proposed NP model outputs the predictive distributions on target sets in following algorithm. Our implementation is available at \url{https://anonymous.4open.science/r/multichannels-corrnp-7A1F/}. 
%----------------------------------------------------
% off-grid
%----------------------------------------------------
\begin{algorithm}[htp!]
\caption{Forward pass of the NP model via Bayesian ConvDeepsets (off-grid) }
\label{alg:BayesConvDeepsets}
    \begin{algorithmic}[1]
    %\Require $\rho = (\text{CNN}, \psi_\rho)$, $\psi$, and density $\zeta$ 
    \Require Model parameters: $\Theta$
    \Require The number of basis stationary kernels $Q$, the number of sampled spectral points $l$
    \Require Context set $D^{c}=\{(x^{c}_n, y^{c}_n)\}_{n=1}^{N^{c}}$, target inputs $X^{t}= \{x^{t}_n\}_{n=1}^{N^{t}}$ 
    \State Compute the discretized inputs $\{t_m\}_{m=1}^{M}$ by spacing inputs range $[\mathrm{min}\{X^{c},X^{t}\},\mathrm{max}\{X^{c},X^{t}\}]$ linearly.
    \State Select the task-dependent stationary prior as described in \textb{Eq. (11)}    
    \State Construct $N$ random functional representation $\{f_{(n)}(D^{c})(\bigcdot)\}_{n=1}^{N}$ on $\mathcal{I}$ as described in \textb{Eqs. (12-16)}.
    \State Construct $N$ random representations $\{\Phi^{\mathcal{B}}_{(n)}(D^{c})(\bigcdot)\}_{n=1}^{N}$ on finite grid points $\{t_m\}_{m=1}^{M}$ as described in \textb{Eq. (17)}.  
    \State Smooth $N$ random representations $\{\Phi^{\mathcal{B}}_{(n)}(D^{c})(\bigcdot)\}_{n=1}^{N}$ on target inputs $X^{t}$ by \textb{Eq. (6)}.  
    \State Generate $N$ predictive distributions $\{p \big( Y^{t} \ | \  X^{t},\Phi^{\mathcal{B}}_{(n)} \big) \}_{n=1}^{N}$ on target inputs $X^{t}$ by \textb{Eq. (20)}.
\end{algorithmic}
\end{algorithm}

%----------------------------------------------------
% on-grid
%----------------------------------------------------
\begin{algorithm}[htp!]
\caption{Forward pass of the NP model via Bayesian ConvDeepsets (on-grid) }
\label{alg:BayesConvDeepsets}
    \begin{algorithmic}[1]
    %\Require $\rho = (\text{CNN}, \psi_\rho)$, $\psi$, and density $\zeta$ 
    \Require Model parameters: $\Theta$
    \Require The number of basis stationary kernels $Q$, the number of sampled spectral points $l$
    \Require Context set $D^{c}=\{(x^{c}_n, y^{c}_n)\}_{n=1}^{N^{c}}$, target inputs $X^{t}= \{x^{t}_n\}_{n=1}^{N^{t}}$ on grid.
    \State Extract the context inputs $\sum_{n=1}^{N^{c}} \delta (\bigcdot -  x^{c}_n ) $
    and outputs  $\sum_{n=1}^{N^{c}} y^{c}_n   \delta (\bigcdot -  x^{c}_n ) $            on grid.
    \State Construct $N$ random functional representation $\{f_{(n)}(D^{c})(\bigcdot)\}_{n=1}^{N}$ on given grid as described in \textb{Eq. (12)}.
    \State Map $N$ random representations on grid where the $n$-th representation $f^M_{(n)}$ is computed as $$f^M_{(n)} = \mathrm{CNN}\left(\left[\sum_{n=1}^{N^{c}} \delta (\bigcdot -  x^{c}_n ) \ , \ \Phi^{\mathcal{B}}_{(n)}(D^{c})(\bigcdot) \right]\right).$$ \vspace{-1mm}  
    \State  Generate $N$ predictive distributions for target set with the $n$-th predictive mean $\mu^{t}_{(n)}$ and standard deviation $\sigma^{t}_{(n)}$,  \vspace{-1mm} $$\mu^{t}_{(n)}  \ , \ \sigma^{t}_{(n)} = f^M_{(n)} \circ  \left(\sum_{n=1}^{N^{t}} \delta (\bigcdot -  x^{t}_n ) \right).   $$ \vspace{-1mm}
\end{algorithmic}
\end{algorithm}

\clearpage
\subsection{Details for Proposed Methodology}
\subsubsection{Structure of Translation Invariant NN in \textb{Eq. (10) (main)}.}
\label{subsubsec:transinvnn}

% To maintain the translation equivariance for the induced functional representation of task-dependent stationary prior, we use the translation invariant neural network $p_{\mathrm{traninv-nn}}: (R^{N_c} {\times} d) \times (R^{N_c} {\times} d') \mapsto R^{Q}_{+}$, that satisfies $p_{\mathrm{traninv-nn}}(X^{c} {+} \tau,Y^{c}) = p_{\mathrm{traninv-nn}}(X^{c},Y^{c}) $ for modeling the parameter of categorical variables $Z=(z_1,..,z_Q)$. To this end, we construct $Q$ data representations of Convolutional Deep set by using $Q$ stationary kernels $\{k_q\}_{q=1}^{Q}$, and its $q$-th representation is defined as

% We construct the functional feature $ \textbf{h}_{\text{traninv}}(x^{c},y^{c})$ by evaluating $\{h_q(\bigcdot)\}_{q=1}^{Q}$ on $X^{c}$, and then concatenating it with the output $y^{c}$ as
In this work, we consider the following structure for the translation invariant network $\mathrm{p}_{\mathrm{nn}}(D^{c})$.
\vspace{-2mm}
\paragraph{Version 1 (without grid).}
With the $q$-th stationary kernel $k_q$, we construct the $q$-th representation $h_q(\bigcdot)=\sum_{n=1}^{N} y^{c}_n \ k_q(\bigcdot - x^{c}_n)$ for given context set  context set $D^c=\{(x^{c}_{n},y^{c}_{n})\}_{n=1}^{N^{c}}$, and map the concatenated representations via MLPs as follows:
\begin{align}
\mathrm{p}_{\mathrm{nn}}(D^{c}) \coloneqq 
\Phi_{\mathrm{MLP\text{-}2}}\bigg( \sum_{(x^{c},y^{c}) \in D^c} \Phi_{\mathrm{MLP\text{-}1}}\left(\Big[ h_1(x^{c}), \ h_2(x^{c}),.., \ h_Q(x^{c}), \ y^{c} \Big]\right)
\bigg).
\end{align}
This structure employs the structure of the kernel smoother and the Deepsets. Since $h_q(\bigcdot)$ function is invariant to the translation dataset $T_{\tau}(D^{c})$, this structure satisfies $\mathrm{p}_{nn}(T_{\tau}(D^{c})) = \mathrm{p}_{nn}(D^{c}) $ with $T_{\tau}(D^{c}) =\{(x^{c}_{n}+\tau,y^{c}_{n})\}_{n=1}^{N^{c}} $.

\paragraph{Version 2 (with grid).}
With the RBF kernel function $k_{\mathrm{RBF}}$, we use the data representation of ConvDeepsets on grid $\{t_m\}_{m=1}^{M}$, and map this representation to the parameters of the categorical distribution as follows:
\begin{align}
\mathrm{p}_{\mathrm{nn}}(D^{c}) \coloneqq 
\Phi_{\mathrm{MLP}}
\bigg( \sum_{  \hspace{1mm} \bigcdot \ \in \{t_m\}_{m=1}^{M}}
\mathrm{CNN}_{\mathrm{1D}}
    \left(
          \sum_{n=1}^{N}  \frac{y_n \ k_{\mathrm{RBF}}(\bigcdot - x_n)}{ \sum_{n=1}^{N}  k_{\mathrm{RBF}}(\bigcdot -  x_n)}  
    \right)
\bigg)
\end{align}
where $ \mathrm{CNN}_{\mathrm{1D}}$ denotes a stack of convolutional layer with ReLU activation. This structure employs the structure of the RBF kernel smoother used in ConvDeepsets and the Deepsets that ensures the set invariance. Since adding or averaging the representation of RBF smoother over the finite grid is invariant to the translation dataset $T_{\tau}(D^{c})$, this structure satisfies $\mathrm{p}_{\mathrm{nn}}(T_{\tau}(D^{c})) = \mathrm{p}_{\mathrm{nn}}(D^{c}) $ with $T_{\tau}(D^{c}) =\{(x^{c}_{n}+\tau,y^{c}_{n})\}_{n=1}^{N^{c}} $. 

Here, we use the representation of RBF smoother to obtain the parameter $\mathrm{p}_{\mathrm{nn}}(D^{c})$ of a latent Categorical distribution $\mathrm{Cat}(Z_{\mathrm{Cat}}|\mathrm{p}_{\mathrm{nn}}(D^{c}) )$ so that $\mathrm{p}_{\mathrm{nn}}(D^{c})$ assigns a task-dependent stationary prior. This approach is different to the use of ConvDeepsets in \citeb{gordon2019convolutional} that represents the data.

\paragraph{Version 3.} We extend \textbf{version 2} to obtain the parameter of Categorical distribution
for the image dataset $D^c$ as follows:
\begin{align}
\mathrm{p}_{\mathrm{nn}}(D^{c}) \coloneqq 
\Phi_{\mathrm{MLP}}
\bigg(
\mathrm{Pooling}
\bigg( \mathrm{CNN}_{\mathrm{2D}}
    \left(
          \sum_{n=1}^{N} y_n \ \delta(\bigcdot - x_n)   
    \right)
\bigg)
\bigg)
\end{align}
where $ \mathrm{CNN}_{\mathrm{2D}}$ denotes a stack of residual block.

\subsubsection{Structure of CNN $\rho$ in \textb{Eq. (17) (main)}.}
\label{subsubsec:cnnstructure}

\paragraph{Shallow and Deep CNN (1d).} For regression tasks with time-series dataset, we employ 5-layer CNN using ReLU activation function as a shallow network. All layers uses 16 channels except for the first layer (8 inchannels) and last layer (8 outchannels). We use kernels of size 5, stride 1, and zero.

For the structure of Deep CNN, we employ the 1D-Unet \citeb{ronneberger2015u}, which is used in \citeb{gordon2019convolutional}. 1D-Unet consists of 12-layer architecture with skip connections where the number of channels is doubled every layer for the first six layers, and halved every layer for the last six layers. The following describes which layers are concatenated, where $L_i \leftarrow \left[L_j, L_k \right]$ means that the input to layer $i$ is the concatenation of the activations of layers $j$ and $k$:
\begin{itemize}[leftmargin=5em]
    \vspace{-2mm}
    \item $L_8 \leftarrow \left[L_5, L_7 \right]$,
     \hspace{3mm} $L_9 \leftarrow \left[L_4, L_8 \right]$,
     \hspace{3mm} $L_{10} \leftarrow \left[L_3, L_9 \right]$,
     \hspace{3mm} $L_{11} \leftarrow \left[L_2, L_{10} \right]$,
     \hspace{3mm} $L_{12} \leftarrow \left[L_1, L_{11} \right]$.
\end{itemize}
We use ReLU activation function, kernels of size 5, stride 1, and zero padding for two units on all layers.

\paragraph{Shallow and Deep CNN (2d).} 
For image completion tasks, we use 3-layer of residual block as a shallow network and 6-layer of residual block as a deep network where each block uses 128 channel, and kernels of size 5, stride 1, and zero.

Further details of DNN structure used in this work can be checked in our implementations in \cref{appendix:details-algorithm}.

\clearpage

\clearpage
\subsection{Proofs}

% \clearpage
%\subsubsection{Random Functional representation in \textb{Eq. (12) (main)} } 
%\clearpage
\subsubsection{Proof of Proposition 2}

% Bayesian ConvDeepsets still holds the translation equivariance (TE) in the following proposition.
%\begin{proposition*} 
\begin{custom_pro}{2} 
\label{pro:te_probsense}
%\label{appendix_pro:Bayes_convdeepset}
Given dataset $D=\{(x_n,y_n)\}_{n=1}^{N}$, if the Bayesian ConvDeepsets $\Phi^{\mathcal{B}} (D) (\bigcdot)$ is defined on the finite grid points, $\Phi^{\mathcal{B}} (D) (\bigcdot)$ is still translation equivariant in distribution sense, i.e.,
\begin{align}
\Phi^{\mathcal{B}}  \circ (T_{\tau}(D)) \stackrel{d}{=}  T^{*}_{\tau} \circ (\Phi^{\mathcal{B}}(D)).
\label{eqn:te_probsense}
\vspace{-3mm}
\end{align}

\begin{proof}
 Let us first consider the left side of equation in \cref{eqn:te_probsense}. Then, for given dataset $D=\{(x_n,y_n)\}_{n=1}^{N}$, its $\tau$-translated dataset $T_{\tau}(D)=\{(x_n+\tau,y_n)\}_{n=1}^{N}$, and finite grid $\{t_m\}_{m=1}^{M}$, we can compute $\Phi^{\mathcal{B}}( T_{\tau}(D)  )(\bigcdot) $ as follows:
\begin{align}
\Phi^{\mathcal{B}}( T_{\tau}(D) )(\bigcdot)  = 
 \rho \circ
 \Big[  
 \underbrace{\sum_{n=1}^{N}  k_{\mathrm{RBF}}(\bigcdot -  (x_n  +\tau ) )}_{\mathrm{density}}  \hspace{2mm}  , \hspace{2mm} 
  \underbrace{\sum_{q=1}^{Q} \textb{ \sqrt{z_q^{\tau}} } \ \textb{ \phi_q^{\tau}(\bigcdot)} +
\sum_{n=1}^{N} \textb{v^{\tau}_{n}}  \ \textb{k(\bigcdot - x_{n} + \tau} )
}_{\mathrm{data \ representation}}
\Big].
\end{align}
where $z_q^{\tau}$, $\phi_q^{\tau}(\bigcdot)$, and $v^{\tau}_{n}$ denote the variation of $z_q$, $\phi_q(\bigcdot)$, and $v_{n}$ due to $\tau$-translated dataset $ T_{\tau}(D)$. The kernel function $k(\bigcdot - x_{n} + \tau)$ denotes the expectation of the latent kernel $\mathrm{E}_{q(Z_{\text{cat}} | D) }[k(\bigcdot - x_{n} ) \ | \ Z_{\text{cat}}]$ over $q(Z_{\text{cat}} | D)=\mathrm{Cat} \left( Z_{\text{cat}} \ ; \ \mathrm{p}_{\mathrm{nn}}(D) \right)$ with the translated invariant network $\mathrm{p}_{\mathrm{nn}}(D)$ that maps the set of dataset $D=\{(x_n,y_n)\}_{n=1}^{N}$ to the parameter of Categorical distribution. Since it has already been proven in \citeb{gordon2019convolutional} that mapping of density channel by CNN holds the TE property, we thus focus on validating that mapping of data representation by CNN holds the TE as well.
\vspace{-2mm}
\paragraph{Prior term.} For each term of data representation, we can check the following qualities:
\vspace{-2mm}
\begin{align}
(z_1^{\tau},..,z_Q^{\tau}) \ \stackrel{d}{=} \ (z_1,..,z_Q) 
\label{eqn:hold_latent}
\end{align}
where $(z_1^{\tau},..,z_Q^{\tau})\sim \mathrm{Cat}(Z;\mathrm{p}_{\mathrm{nn}}(T_{\tau}(D)))$, and  $(z_1,..,z_Q)\sim \mathrm{Cat}(Z;\mathrm{p}_{\mathrm{nn}}(D)$. The equality holds because the output of translated invariant network, i.e., the parameter of categorical distribution satisfies $\mathrm{p}_{\mathrm{nn}}(T_{\tau}(D))=\mathrm{p}_{\mathrm{nn}}(D)$. 

For the stationary prior term, each $q$-th random stationary function $\textb{ \phi_q^{\tau}(\bigcdot)}$ denotes a sample function of $GP(f;0,k_q)$ obtained by random Fourier Feature; the $q$-th kernel $k_q(\tau)$ is set to be  $k_q(\tau)=\int e^{i 2\pi   s^{T} \tau}p_q(s) ds $. Since each stationary function is not dependent on the translated dataset $T_{\tau}(D)$, thus it is trivial that $\textb{ \phi_q^{\tau}(\bigcdot)}=\textb{ \phi_q(\bigcdot)}$ for $q=1,..,Q$.

These results imply that task-dependent prior function $\sum_{q=1}^{Q} \textb{ \sqrt{z_q^{\tau}}} \textb{ \phi_q^{\tau}(\bigcdot)} $ is set consistently up to $T_{\tau}(D)=\{(x_n+\tau,y_n)\}_{n=1}^{N}$.

\vspace{-2mm}
\paragraph{Update term of data.} 
For the data update term, the expected kernel holds as follow:
\vspace{-1mm}
\begin{align}
\mathrm{E}_{q(Z_{\text{cat}}| T_{\tau}(D) ) }[ \ k( \bigcdot ) \ | \ Z_{\text{cat}} \ ]
&=
\mathrm{E}_{q(Z_{\text{cat}}| T_{\tau}(D) ) }[ z_1 k_1(\bigcdot )  \hspace{2mm} +  \hspace{2mm} \cdots  \hspace{2mm}  + \hspace{2mm} z_Q k_Q(\bigcdot ) ]  \nonumber \\
&= \mathrm{p}_{\mathrm{nn}}( T_{\tau}(D) )_{(1)} k_1(\bigcdot ) 
\hspace{2mm} +  \hspace{2mm} \cdots  \hspace{2mm}  + \mathrm{p}_{\mathrm{nn}}( T_{\tau}(D) )_{(Q)} k_Q(\bigcdot )   \\
&= \mathrm{p}_{\mathrm{nn}}( D )_{(1)} k_1(\bigcdot ) 
\hspace{2mm} +  \hspace{2mm} \cdots  \hspace{2mm}  + \mathrm{p}_{\mathrm{nn}}( D )_{(Q)} k_Q(\bigcdot )  \\
&= \mathrm{E}_{q(Z_{\text{cat}}| D ) }[ \ k(\bigcdot  ) \ | \ Z_{\text{cat}} \ ] \label{eqn:hold_latentkernel}, 
\end{align}
where the third equality holds due to the property of the translated invariant network  $\mathrm{p}_{\mathrm{nn}}(T_{\tau}(D))=\mathrm{p}_{\mathrm{nn}}(D)$. 

Also, we can confirm that the smoothing weight $v^{\tau}_n$ holds as follows:
\begin{align}
v^{\tau}_n \coloneqq [ \ K(X_{\tau},X_{\tau}) {+} \sigma^{2}_{\epsilon}I  ) {}^{-1}
          \left(Y^{c} - \Psi(X_{\tau}) \right) \ ]_{n}  = 
[ \ K(X,X) {+} \sigma^{2}_{\epsilon}I  ) {}^{-1}
          \left(Y^{c} - \Psi(X) \right) \ ]_n = v_n
          \label{eqn:hold_weight}, 
\end{align}
where $X_{\tau}=\{x_n+\tau \}_{n=1}^{N}$ and $X=\{x_n \}_{n=1}^{N}$. The first equality holds because the expected kernel $k(\bigcdot)$ is set to be consistent up the translated inputs as described in \cref{eqn:hold_latentkernel}, the expected kernel is stationary kernel, and the random stationary function $\Psi(X_{\tau})$ is set to be consistent up the translated inputs as described in \textbf{Prior term}.

Using the above results, we show that if $\Phi^{\mathcal{B}}  \circ (T_{\tau}(D))$ and $  T^{*}_{\tau} \circ (\Phi^{\mathcal{B}}(D))$ are evaluated on finite grid points $\{t_{m}\}_{m=1}^{M}$ respectively, then $\Phi^{\mathcal{B}}  \circ (T_{\tau}(D)) \stackrel{d}{=}  T^{*}_{\tau} \circ (\Phi^{\mathcal{B}}(D))$ holds as follows:
\begin{align}
\Phi^{\mathcal{B}}( T_{\tau}(D) )(\bigcdot)  &= 
 \rho \circ
 \Big[  
 \sum_{n=1}^{N}  k_{\mathrm{RBF}}(\bigcdot -  (x_n  +\tau ) ) \ , \  
\sum_{q=1}^{Q} \textb{ \sqrt{z_q^{\tau}} } \ \textb{ \phi_q^{\tau}(\bigcdot)} +
\sum_{n=1}^{N} \textb{v^{\tau}_{n}}  \ \textb{k(\bigcdot - (x_{n} + \tau) } )
\Big] \\
& \stackrel{d}{=} 
 \rho \circ
 \Big[  
 \sum_{n=1}^{N}  k_{\mathrm{RBF}}(\bigcdot -  (x_n  +\tau ) ) \ , \  
\sum_{q=1}^{Q} \textb{ \sqrt{z_q} } \ \textb{ \phi_q(\bigcdot)} +
\sum_{n=1}^{N} \textb{v_{n}}  \ \textb{k(\bigcdot - (x_{n} + \tau) } )
\Big]  \label{eqn:step2} \\
& \stackrel{d}{=} 
 \rho \circ
 \Big[  
 \sum_{n=1}^{N}  k_{\mathrm{RBF}}(\bigcdot -  (x_n  +\tau ) ) \ , \  
\sum_{q=1}^{Q} \textb{ \sqrt{z_q} } \ \textb{ \phi_q(\bigcdot - \tau)} +
\sum_{n=1}^{N} \textb{v_{n}}  \ \textb{k(\bigcdot - (x_{n} + \tau) } )
\Big] \label{eqn:step3}\\
& = 
\bigg( 
\underbrace{
 \rho \circ
 \Big[  
 \sum_{n=1}^{N}  k_{\mathrm{RBF}}(\bigcdot -  x_n   ) \ , \  
\sum_{q=1}^{Q} \textb{ \sqrt{z_q} } \ \textb{ \phi_q(\bigcdot)} +
\sum_{n=1}^{N} \textb{v_{n}}  \ \textb{k(\bigcdot - x_{n} } )
\Big]
}_{\Phi^{\mathcal{B}}(D)}
\bigg) (\bigcdot - \tau) 
= T^{*}_{\tau} \circ (\Phi^{\mathcal{B}}(D)).
\end{align}
The equality in \cref{eqn:step2} holds in distribution sense as explained in \cref{eqn:hold_latent,eqn:hold_latentkernel,eqn:hold_weight}.

%$\phi_q(\bigcdot ) \sim N(0; \Phi_q(G)\Phi_q(G)^{T})$ 
The equality in \cref{eqn:step3} holds because each $q$-th stationary random prior function $\phi_q(\bigcdot )$ evaluated on finite grid $G=\{t_{m}\}_{m=1}^{M}$ follows the Gaussian distribution as 
\begin{align}
\phi_q(\bigcdot ) \sim N(0; \Phi_q(G)\Phi_q(G)^{T}), \hspace{3mm} \Phi_q(G)\Phi_q(G)^{T} \approx K_q(G,G)
\end{align}
where $\Phi_q(G) = [\phi_q(t_{1} ),..,\phi_q(t_{M} )] \in R^{M \times f}$, with the number of sampled spectral points $f$, denotes the random feature matrix obtained by applying the random Fourier feature to $q$-th stationary kernel $k_q$, and $ \Phi_q(G)\Phi_q(G)^{T}$ approximate the Gram matrix $K_q(G,G) \in R^{M \times M}$. The $\tau$-translated function $\phi_q(\bigcdot - \tau)$ follows the same distribution as well:
\begin{align}
\phi_q(\bigcdot - \tau ) \sim N(0; \Phi_q(G)\Phi_q(G)^{T}).
\end{align}
This is because $\phi_q(\bigcdot)$ is a instance of the stationary process evaluated on finite points $G$, and its translated function still follows the same stationary process as well.

Therefore, we prove the representation of Bayesian ConvDeepsets holds the TE in distribution sense as stated in \cref{pro:te_probsense}.

\end{proof}
\vspace{-2mm}
%\end{proposition*}
\end{custom_pro}

\clearpage
%\paragraph{Training objective in \textb{Eq. (17)} (main).} 
\subsubsection{Proof of Training objective in \textb{Eq. (21) (main)}} 

%In this section, we explain how our training objective is 

Let $\Theta = \{\theta_{\mathrm{kernels}}, \theta_{\mathrm{p_{\mathrm{nn}}}}, \theta_{\rho},\theta_{\mathrm{pred}}\}$ be the learnable parameters for kernels, the translate invariant network, the CNN, and the network for prediction. To train the model parameters, we optimize following objective w.r.t $\Theta$ :
\begin{align}
 \mathbb{E}_{D^{c},D^{t} \sim p(\mathcal{T})} 
 \bigl[
 \mathcal{L}_{\text{ll}}(\Theta ; D^{c}, D^{t})  - \beta \hspace{.2mm} \mathcal{L}_{\text{reg}}( \Theta ;D^{c}, D^{t}) 
 \bigr]
\label{eqn:tr_objective}
\end{align}
where $\mathcal{L}_{\text{ll}}(\Theta ; D^{c}, D^{t})$ denotes the log likelihood, and $\mathcal{L}_{\text{reg}}(\Theta;D^{c}, D^{t})$ denotes the regularizer that induces the output of network $\mathrm{p}_{\mathrm{nn}}(D^c)$ to assign the reasonable stationary prior depending on context set $D^c$. In the following, we explain how the log likelihood $\mathcal{L}_{\text{ll}}(\Theta ; D^{c}, D^{t})$ and the regulaizer $\mathcal{L}_{\text{reg}}( \Theta ;D^{c}, D^{t})$ are derived:

%$\mathcal{L}_{\text{ll}}(\Theta ; D^{c}, D^{t})$
\paragraph{Likelihood.}  For each task of the context set $D^c=\{(x^{c}_{n},y^{c}_{n})\}_{n=1}^{N^{c}}$ and target set $D^t=\{(x^{t}_{n},y^{t}_{n})\}_{n=1}^{N^{t}}$ that are sampled from the distribution of the task $p(\mathcal{T})$, the multi-sampled log likelihood estimator $\mathcal{L}_{\text{ll}}(\Theta ; D^{c}, D^{t})$ is derived as  
\begin{align}
\log{p(Y^{t}| X^{t}, D^{c} )}  
&=
\log{
\int p(Y^{t}| X^{t}, \Phi^{\mathcal{B}}  ) 
p(\Phi^{\mathcal{B}} | Z_{\text{Cat}},D^{c} )
\ p(Z_{\text{Cat}}| D^{c}  ) 
\ 
d \Phi^{\mathcal{B}}
d Z_{\text{Cat}} 
} \\
&\approx 
\log{
\left(
\frac{1}{N} \sum_{n=1}^{N} p(Y^{t}| X^{t}, \Phi^{\mathcal{B}}_{(n)}  )
\right)
},  \hspace{2mm} \   Z_{(n)} \sim q(Z_{\mathrm{Cat}} | \mathrm{p}_{\mathrm{nn}}(D^{c}) ), \ \Phi^{\mathcal{B}}_{(n)} \sim p(\Phi^{\mathrm{B}}(D^{c})) | Z_{\mathrm{Cat}} = Z_{(n)} )
\nonumber \\
&=
\log{
\left(
\frac{1}{N} \sum_{n=1}^{N} \left( \prod_{i=1}^{N^{t}} p(y^{t}_{i}| x^{t}_{i}, \Phi^{\mathcal{B}}_{(n)}  ) \right)
\right)
}  \label{eqn:condiindep} \\
&= \log{
\left(
 \frac{1}{N} 
 \sum_{n=1}^{N} \exp{ \left(  \sum_{i=1}^{N^{t}} \log{p \left(  y^{t}_{i}| x^{t}_{i}, \Phi^{\mathcal{B}}_{(n)}  \right)}  \right) }
 \right)  }  = \coloneq   \mathcal{L}_{\text{ll}}(\Theta ; D^{c}, D^{t})
\end{align}

where $ Z_{(n)}$ denotes the $n$-th random sample of $q(Z_{\mathrm{Cat}} | D^{c}) = \mathrm{Cat}(Z_{\mathrm{Cat}}; \mathrm{p}_{\mathrm{nn}}(D^{c}))$, and $\Phi^{\mathcal{B}}_{(n)}$ denote the $n$-th sampled representation of Bayesian ConvDeepsets on finite grid $\{t_m\}_{m=1}^{M}$. In \cref{eqn:condiindep}, the conditional independence assumption for given $ \Phi^{\mathcal{B}}_{(n)} $ is used for the $n$-th likelihood, i.e.,  $p(Y^{t} | X^{t},\Phi^{\mathcal{B}}_{(n)})=\prod_{i=1}^{N^{t}} p(y^{t}_{i}| x^{t}_{i},\Phi^{\mathcal{B}}_{(n)})  $, and the likelihood of each observation $p(y^{t}_{i}| x^{t}_{i},\Phi^{\mathcal{B}}_{(n)})$ is modeled as Gaussian distribution, i.e.,
\begin{align}
p(y^{t}_{i}| x^{t}_{i},\Phi^{\mathcal{B}}_{(n)}) = 
N(y^{t}_{i}; \mu_{\mathrm{nn}} (x^{t}_{i},\Phi^{\mathcal{B}}_{(n)}) , \sigma^{2}_{\mathrm{nn}} (x^{t}_{i},\Phi^{\mathcal{B}}_{(n)}) ),
\end{align}
where $\mu_{\mathrm{nn}} (x^{t}_{i},\Phi^{\mathcal{B}}_{(n)})$ and $\sigma_{\mathrm{nn}} (x^{t}_{i},\Phi^{\mathcal{B}}_{(n)})$ denote the predictive mean and standard deviation on $x^{t}_{i}$, and both are parameterized by neural network. In this work, we smooth the representation $\Phi^{\mathcal{B}}_{(n)}$ on target input $x^{t}_{i}$ as described in \textb{Eq. (6) (main)}, and forward the smoothed representation by MLP layers to obtain the parameters of the predictive distribution.

% To assign the task-dependent stationary prior depending on context set $D^{c}$, we introduce the amortized latent variable of which is modeled by the categorical distribution parameterized by the translate invariant neural network $\mathrm{p}_{\mathrm{nn}}(D)$. Based on the fact the optimal variational distribution of $Z_{\mathrm{Cat}}$ is ,

\paragraph{Regularizer.} We consider the regulaizer $\mathcal{L}_{\text{reg}}( \Theta ;D^{c}, D^{t})$ to allow the output of  $\mathrm{p}_{\mathrm{nn}}(D^{c})$ to assign the proper stationary prior for given task. To this end, we employ the result of variational inference for the regulaizer: the optimal distribution of $Z_{\mathrm{Cat}}$ is proportional to the posterior of $Z^{c}$.
That is, let $\tilde{q} \left( Z_{\mathrm{Cat}} \right)$ be a variational distribution in a class of categorical distribution. Then the lower bound of log marginal likelihood is represented as 
\begin{align}
\log{p(Y^{t}|X^{t},D^{c})} \geq  
\int \log{ \left( \frac{p(Y^{t},Z_{\mathrm{Cat}}|X^{t},D^{c})}{\tilde{q} \left( Z_{\mathrm{Cat}}  \right) }   \right)}  
\tilde{q} \left( Z_{\mathrm{Cat}} \right) d Z_{\mathrm{Cat}}.
\end{align}
The equality holds when the variational distribution $ \tilde{q} \left ( Z_{\mathrm{Cat}} \right)$ is a posterior distribution of $Z_{\mathrm{Cat}}$ within a class of categorical distribution, i.e., $\tilde{q} \left( Z_{\mathrm{Cat}} \right)=p(Z_{\mathrm{Cat}} | D^c, D^{t}) =  \mathrm{Cat}(Z_{\text{cat}};\mathrm{p}_{\mathrm{posterior}}) $. Using the fact that the posterior distribution is proportional as
\begin{align}
p (Z_{\text{cat}} = \underbrace{(0,..,1,...0)}_{\mathrm{q\text{-}th \ indicator} } \ | \  D^{c}, D^{t}  ) 
&= \frac{p ( D^{t}, Z_{\text{cat}} = (0,..,1,...0) \ | \  D^{c}  ) }
        {p (  D^{t} \ | \  D^{c} ) }\\
&\propto  p ( D^{t}, Z_{\text{cat}} = (0,..,1,...0) \ | \  D^{c}  ) \\
&= p ( D^{t} | Z_{\text{cat}} = (0,..,1,...0), D^{c}  ) \
   p ( Z_{\text{cat}} = (0,..,1,...0) \ | \  D^{c}  ) \\
&\propto  p ( Y^{t} | X^{t}, Z_{\text{cat}} = (0,..,1,...0), D^{c}  ) \  p ( Y^{c} | X^{c}, Z_{\text{cat}} = (0,..,1,...0) ) \\ 
&\propto  p ( Y^{t} | X^{t}, Z_{\text{cat}} = (0,..,1,...0), D^{c}  ) ,
\end{align}
we set the parameter of posterior distribution $\mathrm{p}_{\mathrm{posterior}}$ such that $q$-th entry of $\mathrm{p}_{\mathrm{posterior}}$ is represented as 
\begin{align}
(\mathrm{p}_{\mathrm{posterior}})_{(q)} = 
\frac{\mathrm{exp} \left( \log{p(Y^{t} | X^{t}, D^{c}, k_q)} \ / \  \tau_{0} \right)}
{\sum_{q=1}^{Q} \mathrm{exp} \left( \log{p(Y^{t} | X^{t}, D^{c}, k_q)} \ /\  \tau_{0} \right)}
\end{align}
where $\tau_{0}$ denotes the temperature hyperparameters. For $\log{p(Y^{t} | X^{t}, D^{c}, k_q)}$, we compute the likelihood via empirical distribution as follows:
\begin{align}
\hspace{-2.2mm}
p(Y^{t} | X^{t},D^{c}, k_q) = N( Y^{t} ;\hat{\mu}_{q}(X^{t}),\mathrm{Diag}(\hat{\Sigma}_{q}(X^{t})) ),
\label{eqn:emp-gpposterior}
\end{align}
which can be computed efficiently. The empirical predictive mean $\hat{\mu}_{q}(X^{t}) \in R^{N_t}$ and diagonal covariance $\mathrm{Diag}(\hat{\Sigma}_{q}(X^{t})) \in R^{N_t}$ are computed by using the sample functions of GP posterior in \textb{Eq. (12) (main)}.

As a result, we consider the regulaizer $\mathcal{L}_{\text{reg}}( \Theta ;D^{c}, D^{t})$ via the KL divergence between categorical distribution, i.e,
\begin{align}
\mathcal{L}_{\text{reg}}( \Theta ;D^{c}, D^{t}) \coloneqq \mathrm{KL} \left( q(Z_{\text{cat}} \ | \  D^{c} )  \ || \  p (Z_{\text{cat}} \ | \  D^{c}, D^{t}  )  \right)
\label{eqn:appendix_reg}.
\end{align}

% , and compute the likelihood as
% \begin{align}
% \hspace{-2.2mm}
% p(Y^{t} | X^{t},D^{c}, k_q) = N( Y^{t} ;\hat{\mu}_{q}(X^{t}),\mathrm{Diag}(\hat{\Sigma}_{q}(X^{t})) ) 
% \label{eqn:emp-gpposterior}
% \end{align}
% where $\hat{\mu}_{q}(X^{t}) \in R^{N_t}$ and $\mathrm{Diag}(\hat{\Sigma}_{q}(X^{t})) \in R^{N_t}$ denote the empirical predictive mean and diagonal covariance of the GP posterior distribution on target set $X^{t}$. The sample functions of GP posterior, described in \cref{eqn:randomfunctionalfeature}, are used. The derivation of training loss is explained in Appendix A.3.

% these sample functions are obtained in forward procedure.
% the GP posterior distribution on target set $X^{t}$

% The $ p (Z_{\text{cat}} \ | \  D^{c}, D^{t}  )= \mathrm{Cat}(Z_{\text{cat}};\mathrm{p}_{\mathrm{prior}}  ) $ is computed with the parameter $\mathrm{p} \in {\Delta}^{Q-1} $ of which the $q$-th element $\mathrm{p}_{q} $ is defined as follows: 

% \begin{align}
% p (Z_{\text{cat}} = \underbrace{(0,..,1,...0)}_{\mathrm{q{-}th \ indicator}} \ | \  D^{c}, D^{t}  ) 
% &= p (Z_{\text{cat}} = (0,..,1,...0) \ | \  D^{c}, D^{t}  ) \\
% %\propto  p ( Y^{t}, Z_{\text{cat}} \ | \  X^{t}, D^{c},   )
% \end{align}

%\mathcal{L}
%\paragraph{Comparison the proposed training objective with the ELBO of variational inference.} 
\paragraph{Comparison the proposed training objective with the conventional ELBO.} 
As we consider the conventional ELBO estimator $\mathcal{L}_{N}$ of meta-learning framework, represented as,
\begin{align}
& \hspace{4.75mm} \mathbb{E}_{D^{c},D^{t} \sim p(\mathcal{T})} 
 \bigg[
 \int \log p \left( Y^{t}|X^{t},D^{c},\Phi^{\mathcal{B}},Z_{\mathrm{Cat}} \right) q(\Phi^{\mathcal{B}},Z_{\mathrm{Cat}}) \ d  \Phi^{\mathcal{B}} \ d Z_{\mathrm{Cat}}
 -
 \mathrm{KL}( q(\Phi^{\mathcal{B}},Z_{\mathrm{Cat}}) || p(\Phi^{\mathcal{B}},Z_{\mathrm{Cat}}) )  
 \bigg] \nonumber \\
&\approx \mathbb{E}_{D^{c},D^{t} \sim p(\mathcal{T})} 
\bigg[
\underbrace{\frac{1}{N} \sum_{n=1}^{N}\log p \left( Y^{t}|X^{t},D^{c},\Phi^{\mathcal{B}}_{(n)} \right) }_{\mathrm{likelihood}}
-
\underbrace{
\bigg(
\mathrm{KL}( q(\Phi^{\mathcal{B}}) || p(\Phi^{\mathcal{B}}) )  
+
\mathrm{KL}( q(Z_{\mathrm{Cat}}) || p(Z_{\mathrm{Cat}}) )  
\bigg)
}_{\mathrm{regulaizer}}
\bigg] \coloneqq \mathcal{L}_{N}
\label{eqn:appendix_reg_naive}
\end{align}
the proposed objective employs the multi-sampled log likelihood estimator, used in \citeb{burda2016importance,foong2020meta}, which is known to be tighter than the likelihood term of $\mathcal{L}_{N}$. In addition, the proposed objective focuses on regularizing $Z_{\mathrm{Cat}}$, and use the posterior distribution $p(Z_{\mathrm{cat}} | D^t,D^{c} )$ in \cref{eqn:appendix_reg} for training $q(Z_{\mathrm{Cat}})$ instead of the prior distribution $p(Z_{\mathrm{cat}} )$ as shown in \cref{eqn:appendix_reg_naive}.
