# Supplementary material for: Bayesian Convolutional Deep Sets with Task-Dependent Stationary Prior
Source: arXiv:2210.12363 source file (2022-10-22)
Supplement: Supplementary file 9 [file 07-appendix-v01-chapter2-exp1.tex]

%\subsection{Further Details for the 1d Regression Task}
\section{Further Details for 1d Regression Task}

\label{appendix:1d-regression-task}

% data --> model --> training -- additional results
\subsection{Details for Datasets}

To train the NP models, we employ the meta-learning framework; for every task, when the given finite observations, referred as context sets and target sets are assumed to be finite samples of the function sampled from stochastic process, the NP models first construct the functional representation of the context sets and then generate the predictive distribution on the target sets.

We consider 4 stationary stochastic processes: RBF,  Matern-$\frac{5}{2}$, Weakly periodic, and Sawtooth, which are used in \citeb{gordon2019convolutional}, to prepare the context and target sets. We describe the each process as follows:
\begin{itemize}[leftmargin=1em]
    \item \textbf{RBF (large lengthscale)}: The context and target sets are constructed by randomly choosing $N_{c}$ data points and $N_{t}$ data points from the function sampled from Gaussian Process (GP) with the following kernel function $k$ with the random lengthscale $l \sim \mathcal{U}([1.1,2.1])$, that is randomly sampled per each task:
    $$k(x, x') = e^{-\frac{1}{2}(\frac{x-x'}{l})^2}.$$
    \item \textbf{Matern-$\frac{5}{2}$ (small lengthscale)}: The context and target sets are constructed by randomly $N_{c}$ data points and $N_{t}$ data points from the function sampled from GP with the following kernel function $k$ with $d = |\frac{x - x'}{l}|$ and random lengthscale $l \sim \mathcal{U}([0.19,0.21])$, that is randomly sampled per each task:
    $$k(x, x') = (1 + \sqrt{5} d  + \frac{5}{3} d^2) e^{-\sqrt{5} d}.$$
    \item \textbf{Weakly periodic}: The context and target sets are constructed by randomly choosing $N_{c}$ data points and $N_{t}$ data points from the function sampled from GP with the following kernel function $k$ with $g_1(x) = \cos(2 \pi f x )$, $g_2(x) = \sin(2\pi f x )$, and random frequency parameter $f \sim \mathcal{U}([2.0,3.0])$, that is randomly sampled per each task:
    $$k(x, x') = e^{ \left( -\frac12 (g_1(x) - g_1(x'))^2 -\frac12 (g_2(x) - g_2(x'))^2 - \frac{1}{32} (x-x')^2 \right)}.$$
    \item \textbf{Sawtooth}: The context and target sets are constructed by randomly choosing $N_{c}$ data points and $N_{t}$ data points from the sampled function $y_{\text{sawtooth}}(t)$ represented as
    $$y_{\text{sawtooth}}(t) = \frac{A}{2} - \frac{A}{\pi}\sum_{k=1}^\infty (-1)^k \frac{\sin(2\pi k f (t+\tau))}{k},$$
    where $A$ denotes the amplitude, $f$ denotes the frequency, $\tau$ denotes the shift, and $t$ denotes time. We use truncate the series at an integer $K$. We consider the random amplitude $A \sim \mathcal{U}([0.8,1.2])$, random frequency $f \sim \mathcal{U}([1,2])$, random truncation integer $K \sim \mathcal{U}([10,20])$, and random shift $\tau \sim \mathcal{U}([-1,1])$, which are randomly sampled for each task. 
\end{itemize}
%http://143.248.92.34:8888/lab/workspaces/auto-U/tree/UAI22_CCCNP_from108/dataset_singletask_1d.py

%\subsubsection{Details for Training, Validation, and Test}
\subsection{Details for Tasks of Training, Validation, and Test }
\label{subsubsec:prepare_sets}

In this experiment, we set the training range \textb{$[0,4]$} and test range \textb{$[4,8]$} (outside of training range). For training, we construct the context sets and target sets by sampling the data points on training range. Then, we evaluate the trained models with context sets and target sets, that are sampled on test range. These test sets are used to check whether trained NP models holds translation equivariance.

We consider the following number of data points for training, validation, and test:
\begin{itemize}[leftmargin=1em]
    \vspace{-2mm}
    \item \textbf{Small number of context data points:} For training, we randomly sample \textb{$N_c \sim \mathcal{U}([5,25])$} as the number of context data points, and randomly sample \textb{$N_t \sim \mathcal{U}([N_c,50])$} as the number of target data points for each task. We use \textb{$500{\times}50{\times}16$} tasks for training through 500 batches. For validation, we set $N_c$ context data points and $N_t$ target data points as done in training, and use \textb{$128{\times}16$} tasks for validation to choose the parameters of the trained models. For test, we also set $N_c$ context data points and $N_t$ target data points for each processes (RBF, Matern-$\frac{5}{2}$, Weakly periodic, and Sawtooth), as done in training, and use \textb{$128{\times}16$} tasks per the process to evaluate the trained models using the chosen parameters in validation.
    \vspace{-1mm}
    \item \textbf{Large number of context data points:} For training, we randomly sample \textb{$N_c \sim \mathcal{U}([10,50])$} as the number of context data points, and randomly sample \textb{$N_t \sim \mathcal{U}([N_c,50])$} as the number of target data points for each task. For validation and test, we use \textb{$128{\times}16$} tasks. For test set, we use \textb{$128{\times}16$} tasks per the process, as done in the case of \textbf{the small number of context data points}.
\end{itemize}

Additionally, we consider the same number of tasks per each stochastic process so that the NP models does not fit particular stochastic process only during training

\subsection{Details for Hyperparameters.}

\paragraph{Hyperparameters of Kernels.}

% For the hyperparameter of RBF kernels used for ConvCNP and ConvLNP, we conduct the experiment with  $l\in\{0.1,0.5,1.0\}$, and set the lengthscale $l=0.1$ for both models because it obtains the best performance out of those candidates.

% For the hyperparameter of RBF kernels used for GPConvCNP-RBF, we conduct the experiment with  $l\in\{0.1,0.5,1.0\}$, and set the lengthscale  $l=1.0$ obtaining the best performance out of those candidates.

% For the hyperparameter of SM kernels ($Q=1$) used for GPConvCNP-SM, we set $\mu$ randomly by sampling $\mu$ from $\mathcal{U}(0,5)$, and set $\Sigma=1.0$. 

% For the hyperparameter of basis kernels, we set $\mathrm{Hz}_{\mathrm{max}}=5$ and 3 basis stationary kernels ($Q=3$ ). Then, we set $\{\mu_q\}_{q=1}^{3}$ by randomly sampling $\mu_q \sim \mathcal{U}[0,\mathrm{Hz}_{\mathrm{max}}]$ with $\mu_1=0 \leq ..\leq \mu_3$, and set
% $\Sigma_q = 1.0$ for $q=1,..,3$. For the noise parameter $\sigma^{2}_{\epsilon}$, we set $\sigma_{\epsilon}=1e\text{-}{2}$.

For the hyperparameter of RBF kernels used for ConvCNP and ConvLNP, we conduct the experiment with  $l\in\{0,01,0.1,0.5\}$, and set the lengthscale $l=0.01$ for both models obtaining the best performance out of those candidates.

For the hyperparameter of GPConvCNP, we conduct the experiment with  $l\in\{0.1,0.5,1.0\}$, and set the lengthscale  $l=1.0$ obtaining the best performance out of those candidates.

For the hyperparameter of the proposed method, we use $Q\in\{3,4,5\}$ basis stationary kernels, and set $\mathrm{HZ}_{\mathrm{max}}=Q$. Then, we space the frequency range $[0,\mathrm{HZ}_{\mathrm{max}}]$ linearly, set each centered value as $\mu_q$ with $\mu_1=0 \leq ..\leq \mu_Q$, and set $\sigma_q = 0.5(\mu_{2} -\mu_{1})$ for $q=1,..,Q$. For the noise parameter $\sigma^{2}_{\epsilon}$, we set $\sigma_{\epsilon}=1e\text{-}{2}$.

For the number of spectral points, we use $l=10$ in \textb{Eq. (14)}.

For the number of sample function, we use $N=5$ in \textb{Eq. (19)}.

For training, we  use ADAM optimizer \citeb{kingma2014adam} with learning rate $5e\text{-}4$ and weight decay $1e\text{-}4$. 

For the regularizer hyperparameter $\beta$ in \textb{Eq. (21)}, we set $\beta=0.1$ for the proposed method.

% \paragraph{Hyperparameters of Kernel Approximation in \textb{Eq. (9)}.}
% For the number of spectral points ($l$ in \textb{Eq. (9)}) used for kernel approximation, we use 10 random Fourier features ($l=10$) per each basis stationary kernel, and thus use total $Q \times 10$ random Fourier features. For the multi-channel stochastic process, we use total $K \times (Q \times 10)$ random Fourier features with $K$ channels.

% \paragraph{Hyperparameters of Random Functional Representations in \textb{Eq. (10)}.}
% For the number of random functional representations ($N$ in \textb{Eq. (10)}), we use 10 functional representations ($N=10$). For multi-channel stochastic process, we use total $K \times 10$ representations with $K$ channels.

% \paragraph{Hyperparameters for Training.} We use ADAM optimizer \citeb{kingma2014adam} with learning rate $5e\text{-}4$ and weight decay $1e\text{-}4$. For the regularizer hyperparameter $\beta$ in \textb{Eq. (17)}, we set $\beta=0.5$.

\subsubsection{Baseline Implementations}
\label{subsubsec:baseline2}
For ANP, we employ the deterministic path of the model described by \citeb{kim2018attentive} for 1d regression experiment. For ConCNP, ConvLNP, and GPConvCNP, we employ the structure of Deep CNN 1d as described in \cref{subsubsec:cnnstructure}. For ANP and ConvCNP, we employ the implementation \footnotemark{\footnotetext[1]{\url{https://github.com/cambridge-mlg/convcnp}}}. For ConvLNP, we refer to the implementation \footnotemark{\footnotetext[2]{\url{https://github.com/YannDubs/Neural-Process-Family}}}.

\clearpage
\subsection{Additional Results}
%\vspace{-2mm}
\paragraph{Training with a small number of context sets.}
For the completeness of the experiment results, we report additional results of the training with a small number of context set $(N_c \sim \mathcal{U}([5,25]) )$. \cref{fig:exp5-1:small-a,fig:exp5-1:small-b,fig:exp5-1:small-c,fig:exp5-1:small-d}
 describes the mean and one-standard error of the log likelihood for $1024$ tasks (within training range). For evaluation, we set varying number of context data points $N^c \in \{5,10,15,20,25\}$ and target points $N^{t}=50$. \cref{fig:exp5-1:small-e,fig:exp5-1:small-f,fig:exp5-1:small-g,fig:exp5-1:small-h} corresponds to the results for tasks (beyond training range). We could not report the results of AttnCNP due to poor generalization performance.

\vspace{-3mm}
\begin{figure}[H]
%\begin{figure}[htp!]
\centering
\subfloat[ \label{fig:exp5-1:small-a} RBF (in-range)]
{\includegraphics[width=0.24\linewidth]{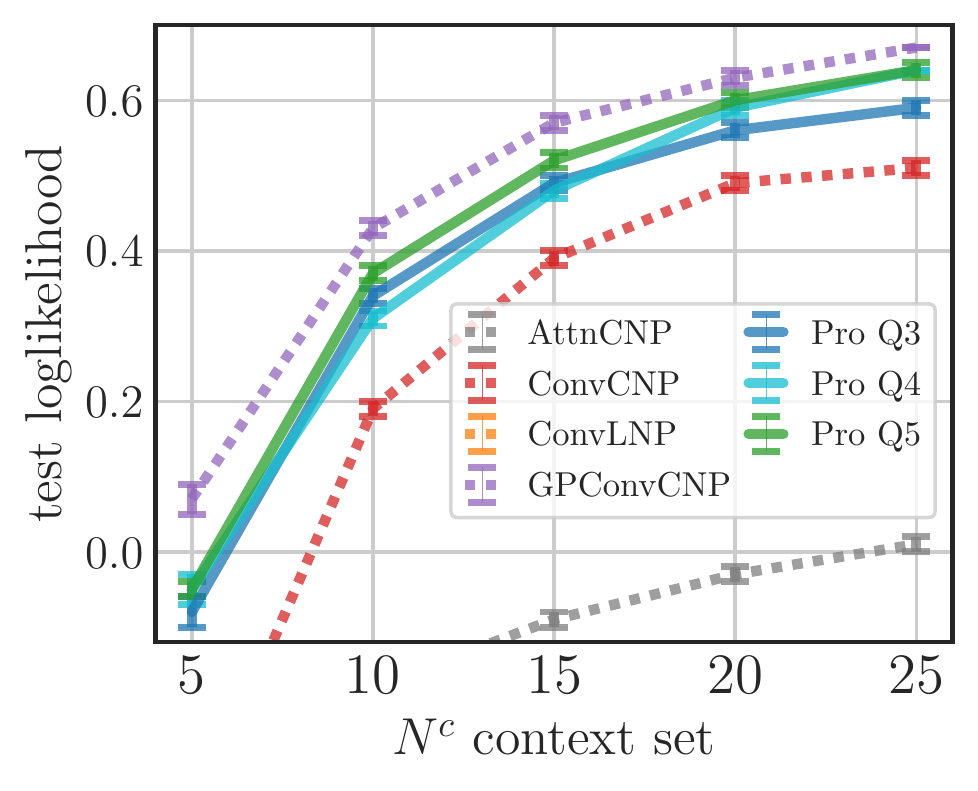}}   \hspace{0.5mm} 
\subfloat[ \label{fig:exp5-1:small-b} Matern-${\frac{5}{2}}$ (in-range)] 
{\includegraphics[width=0.24\linewidth]{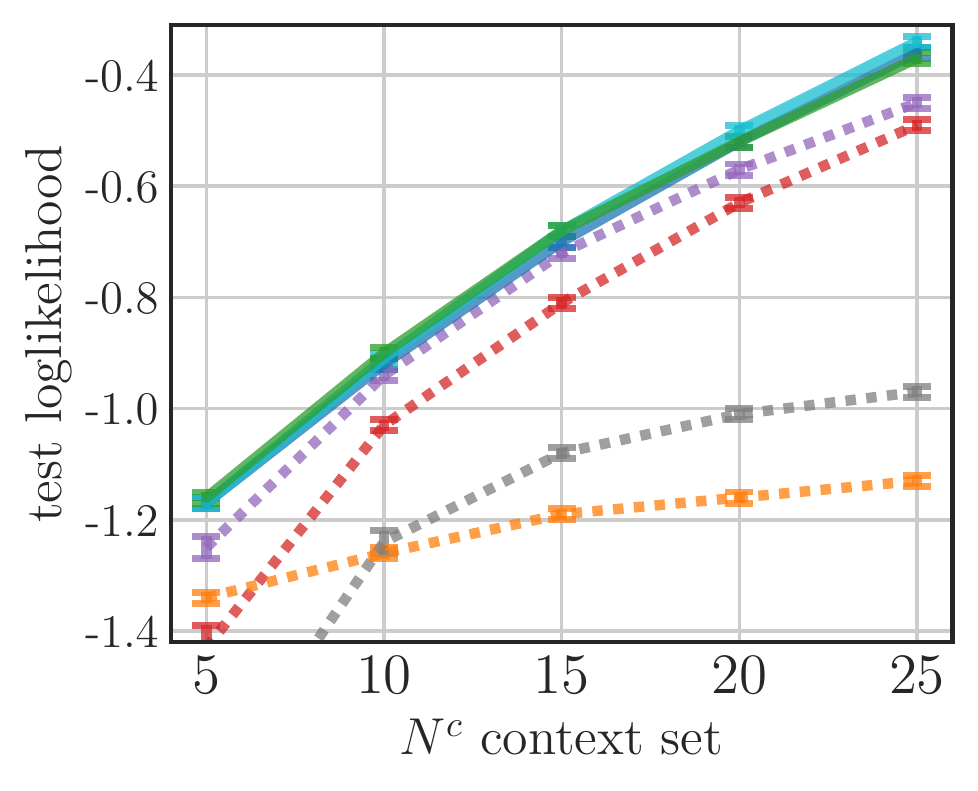}} \hspace{0.5mm}  
\subfloat[ \label{fig:exp5-1:small-c} Weakly periodic (in-range)]
{\includegraphics[width=0.24\linewidth]{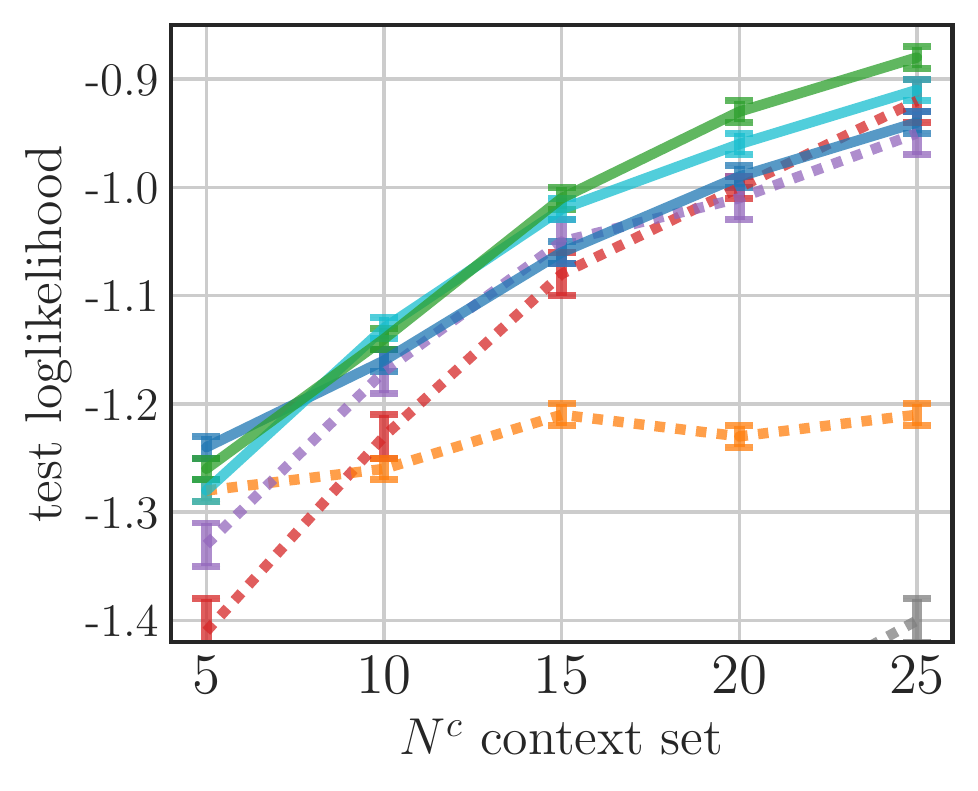}}  \hspace{0.5mm} 
\subfloat[ \label{fig:exp5-1:small-d}Sawtooth (in-range)]
{\includegraphics[width=0.24\linewidth]{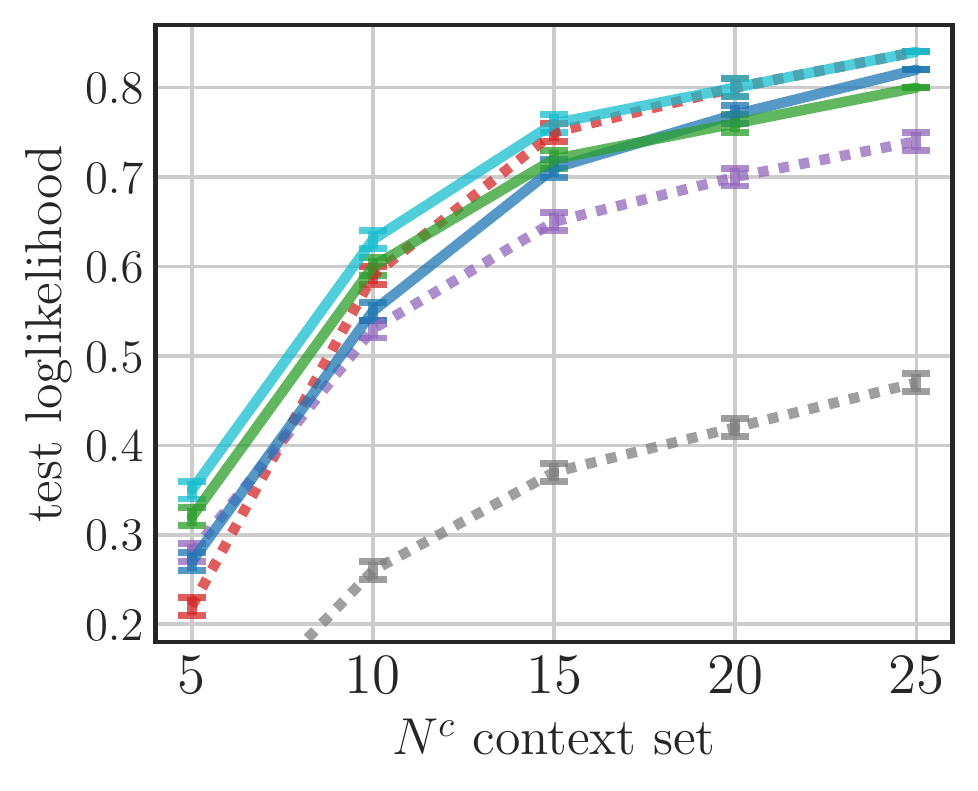}}   

\vspace{2mm}
\subfloat[ \label{fig:exp5-1:small-e} RBF (out-range)]
{\includegraphics[width=0.24\linewidth]{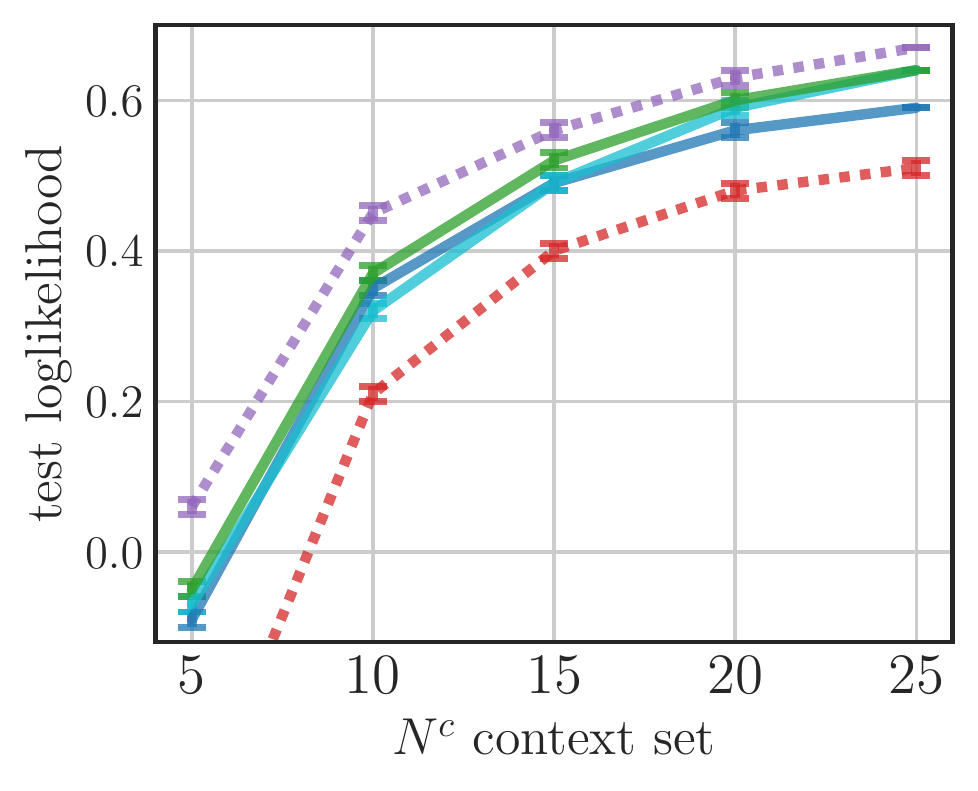}}   \hspace{0.5mm} 
\subfloat[ \label{fig:exp5-1:small-f} Matern-${\frac{5}{2}}$ (out-range)] 
{\includegraphics[width=0.24\linewidth]{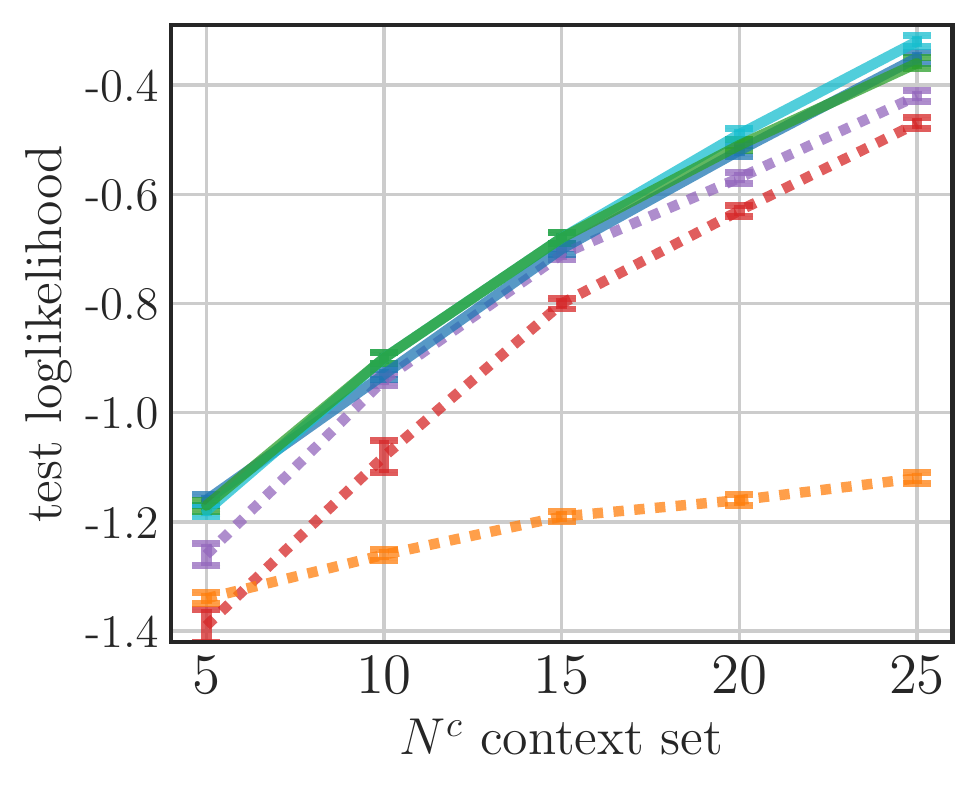}} \hspace{0.5mm}  
\subfloat[ \label{fig:exp5-1:small-g} Weakly periodic (out-range)]
{\includegraphics[width=0.24\linewidth]{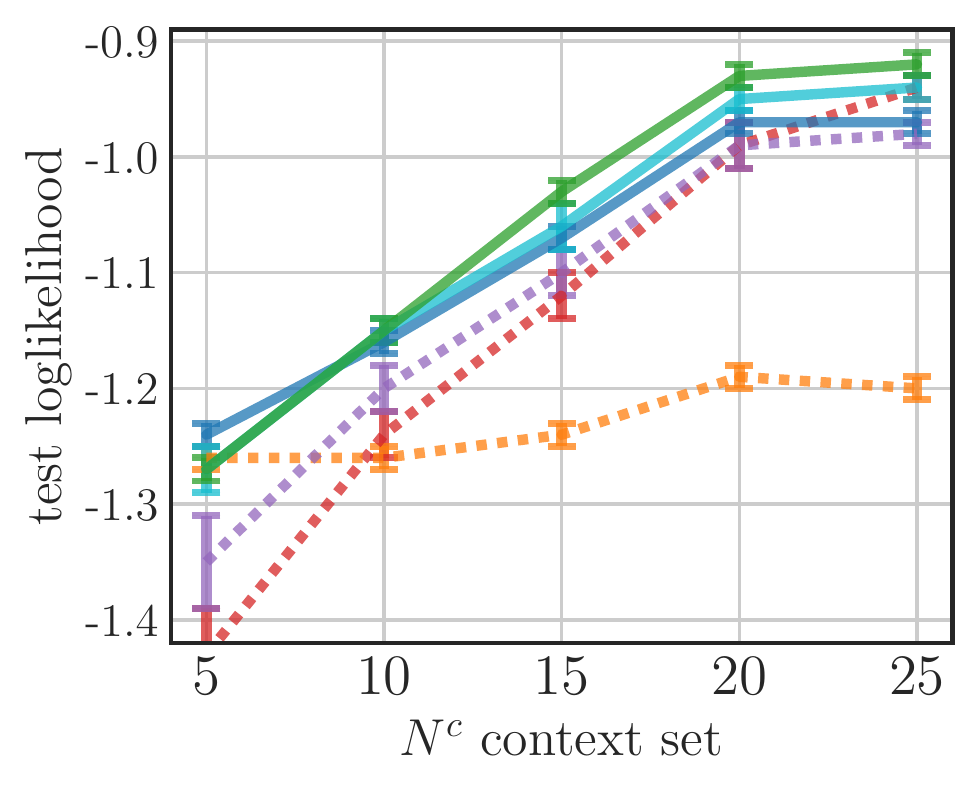}}  \hspace{0.5mm} 
\subfloat[ \label{fig:exp5-1:small-h} Sawtooth (out-range)]
{\includegraphics[width=0.24\linewidth]{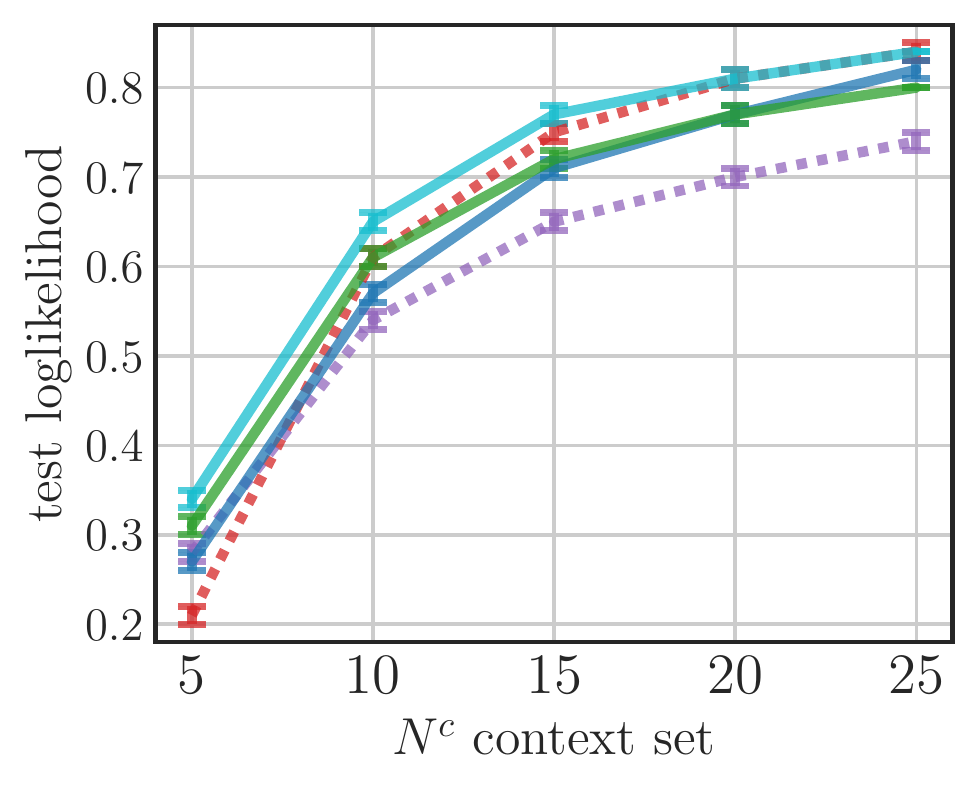}}   
\caption{Prediction result of each processes from training setting of \textb{small $N^{c}$} context points.}
\label{fig:exp5-1:smallset_comparison-supp}
\end{figure}

\vspace{-4mm}
\paragraph{Training with a large number of context sets.}
\vspace{-4mm}

Additionally, we report the results of the training with a large number of context set $(N_c \sim \mathcal{U}([10,50]) )$, and apply the same evaluation procedure with setting of a small number of context set. \cref{fig:exp5-1:small-a2,fig:exp5-1:small-b2,fig:exp5-1:small-c2,fig:exp5-1:small-d2}
 describes the mean and one-standard error of the log likelihood for $1024$ tasks (within training range). \cref{fig:exp5-1:small-e2,fig:exp5-1:small-f2,fig:exp5-1:small-g2,fig:exp5-1:small-h2} corresponds to the results for tasks (beyond training range).

\vspace{-3mm}
\begin{figure}[H]
%\begin{figure}[htp!]
\centering
\subfloat[\label{fig:exp5-1:small-a2} RBF (in-range)]
{\includegraphics[width=0.24\linewidth]{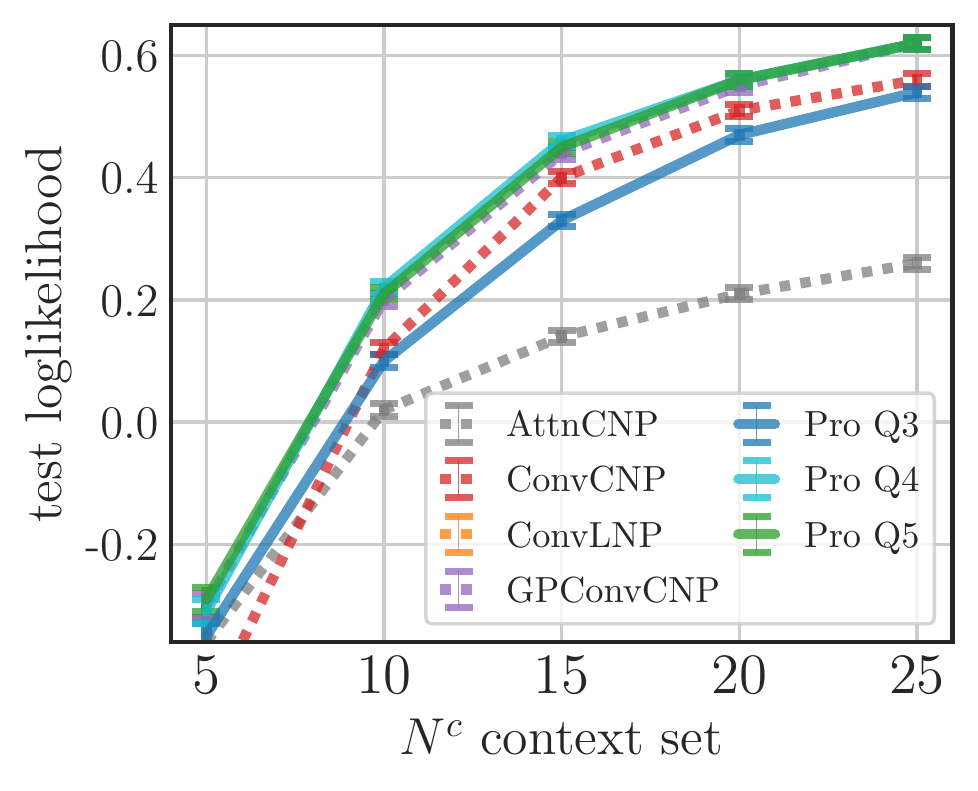}}   \hspace{0.5mm} 
\subfloat[\label{fig:exp5-1:small-b2} Matern-${\frac{5}{2}}$ (in-range)] 
{\includegraphics[width=0.24\linewidth]{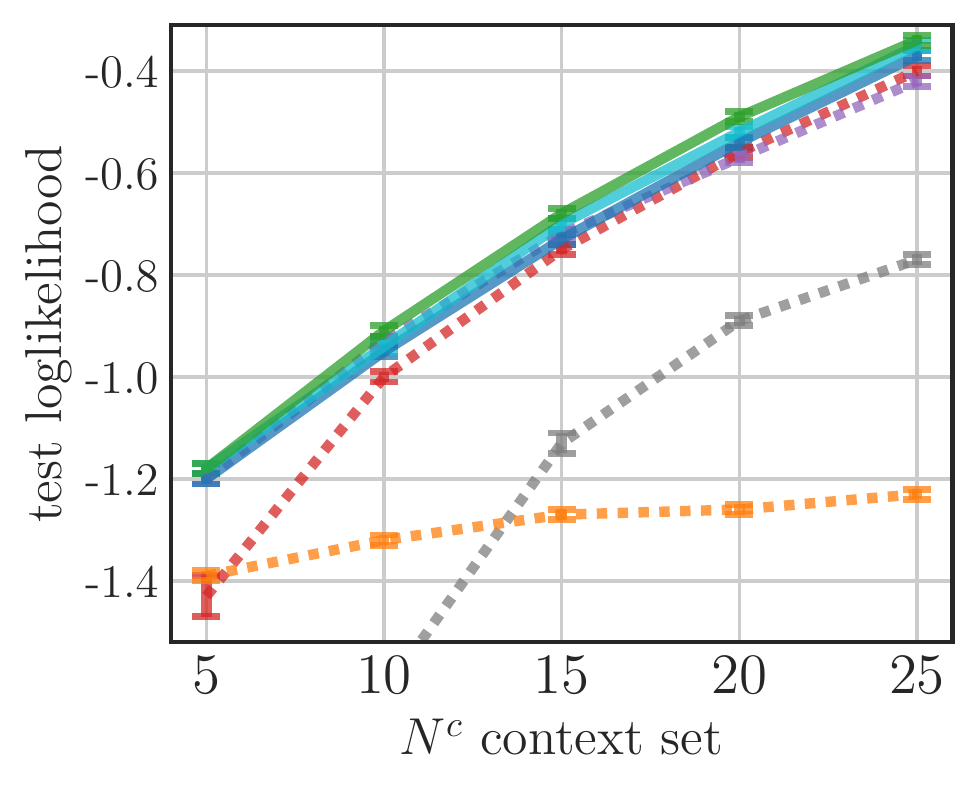}} \hspace{0.5mm}  
\subfloat[\label{fig:exp5-1:small-c2} Weakly periodic (in-range)]
{\includegraphics[width=0.24\linewidth]{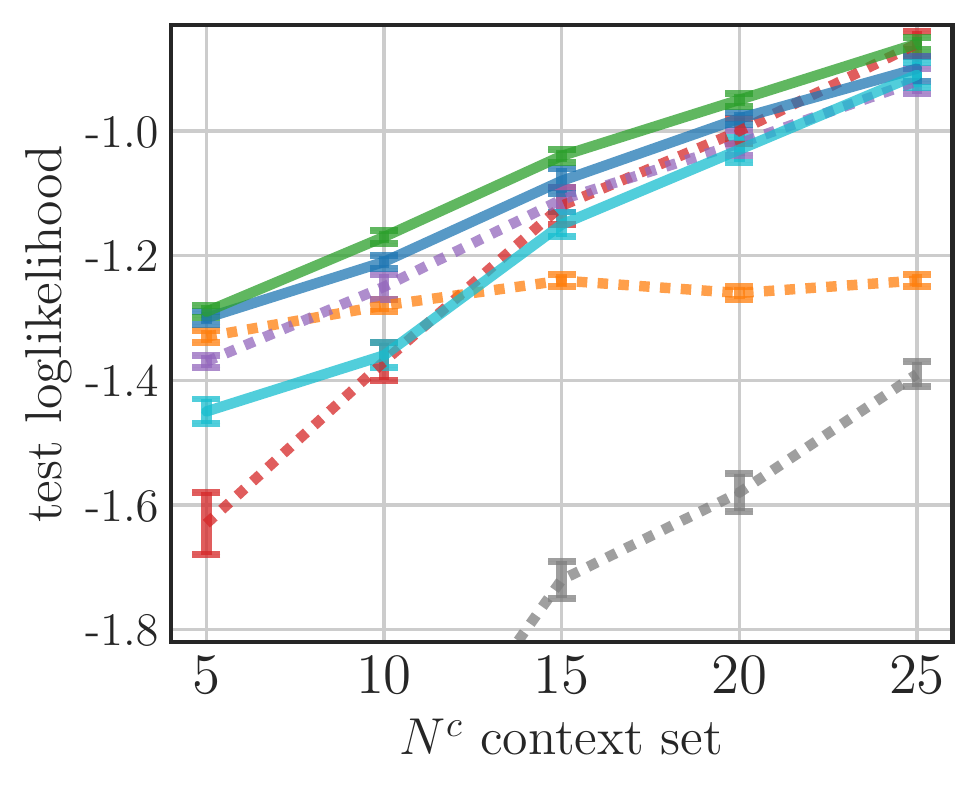}}  \hspace{0.5mm} 
\subfloat[\label{fig:exp5-1:small-d2} Sawtooth (in-range)]
{\includegraphics[width=0.24\linewidth]{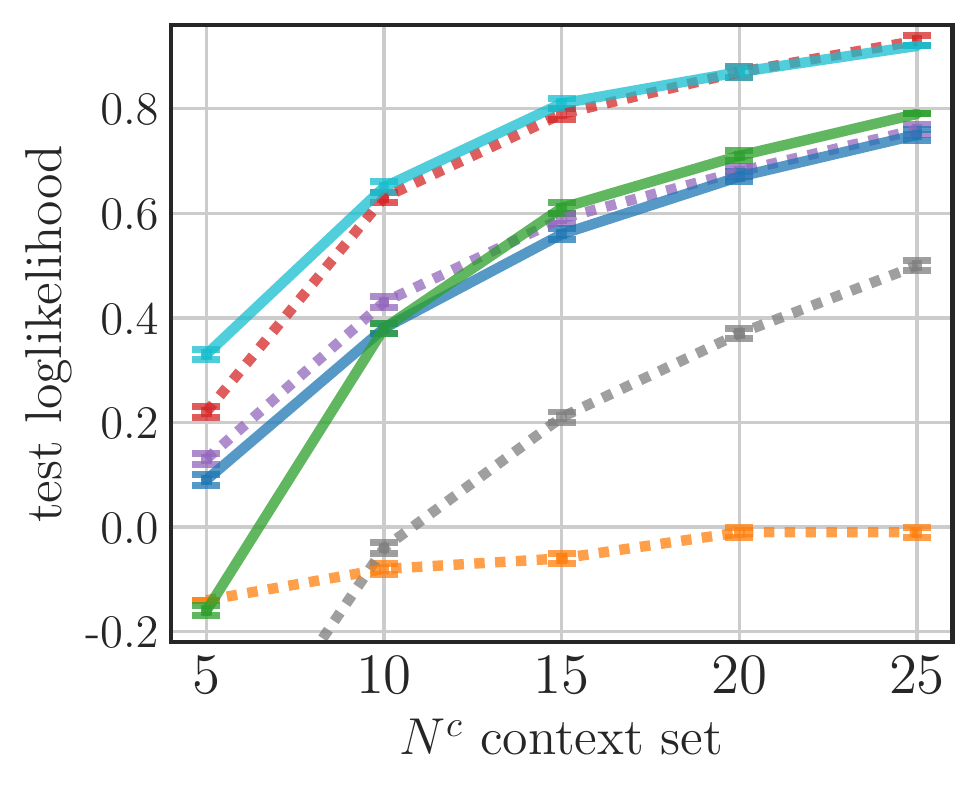}}   

\vspace{2mm}
\subfloat[\label{fig:exp5-1:small-e2} RBF (out-range)]
{\includegraphics[width=0.24\linewidth]{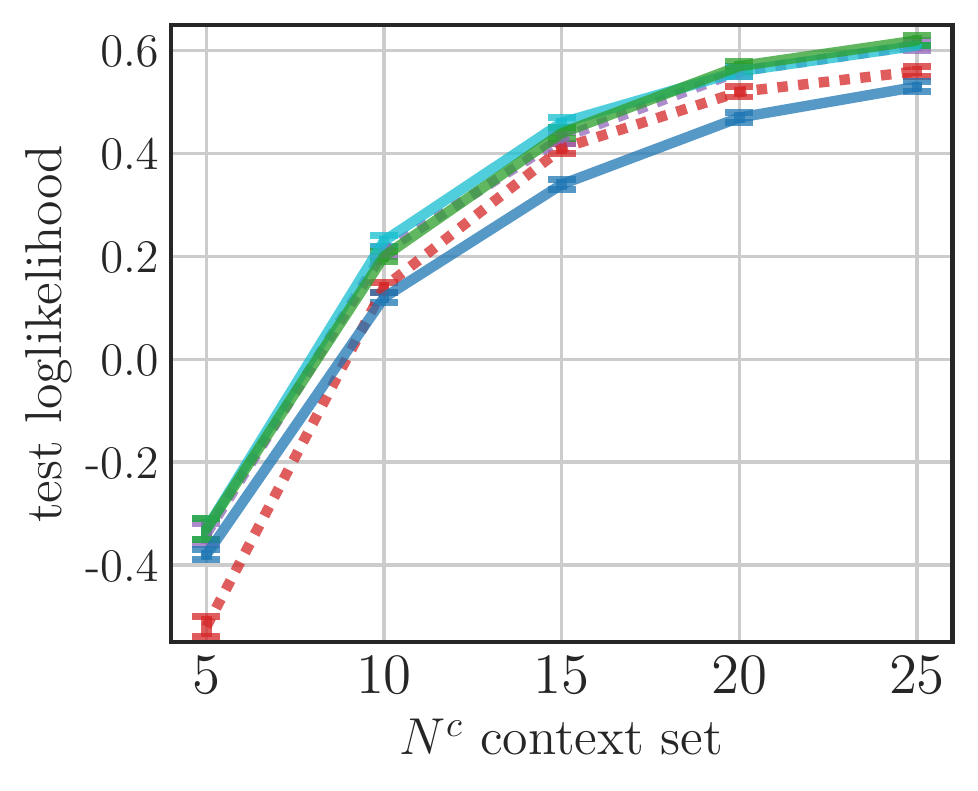}}   \hspace{0.5mm} 
\subfloat[\label{fig:exp5-1:small-f2}  Matern-${\frac{5}{2}}$ (out-range)] 
{\includegraphics[width=0.24\linewidth]{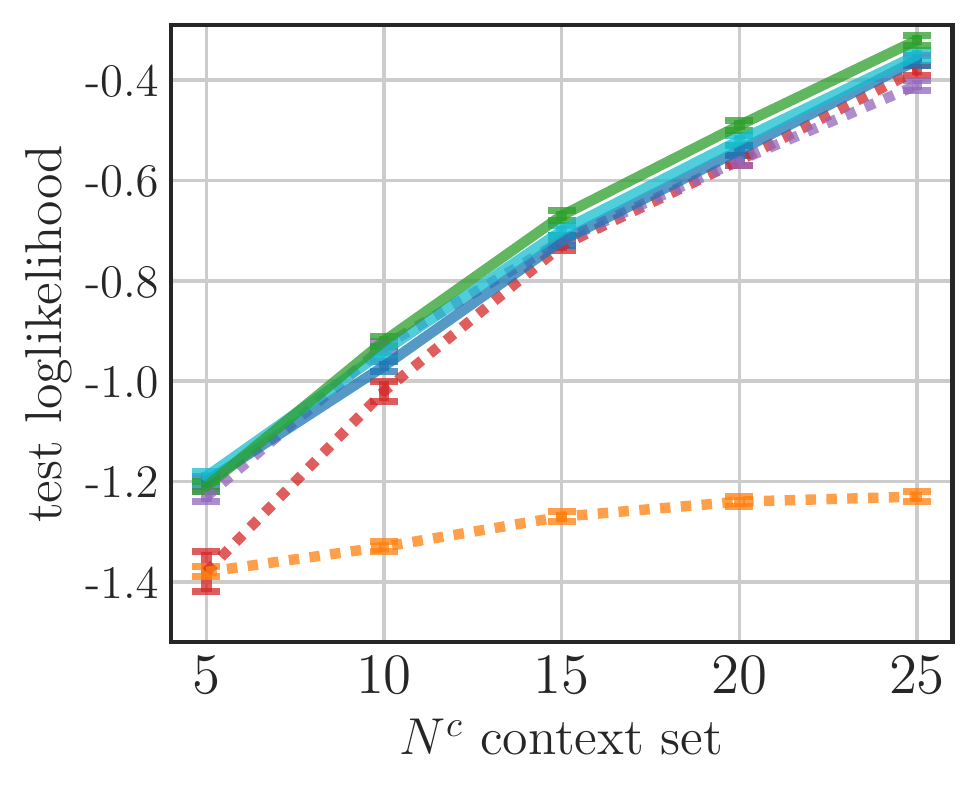}} \hspace{0.5mm}  
\subfloat[\label{fig:exp5-1:small-g2} Weakly periodic (out-range)]
{\includegraphics[width=0.24\linewidth]{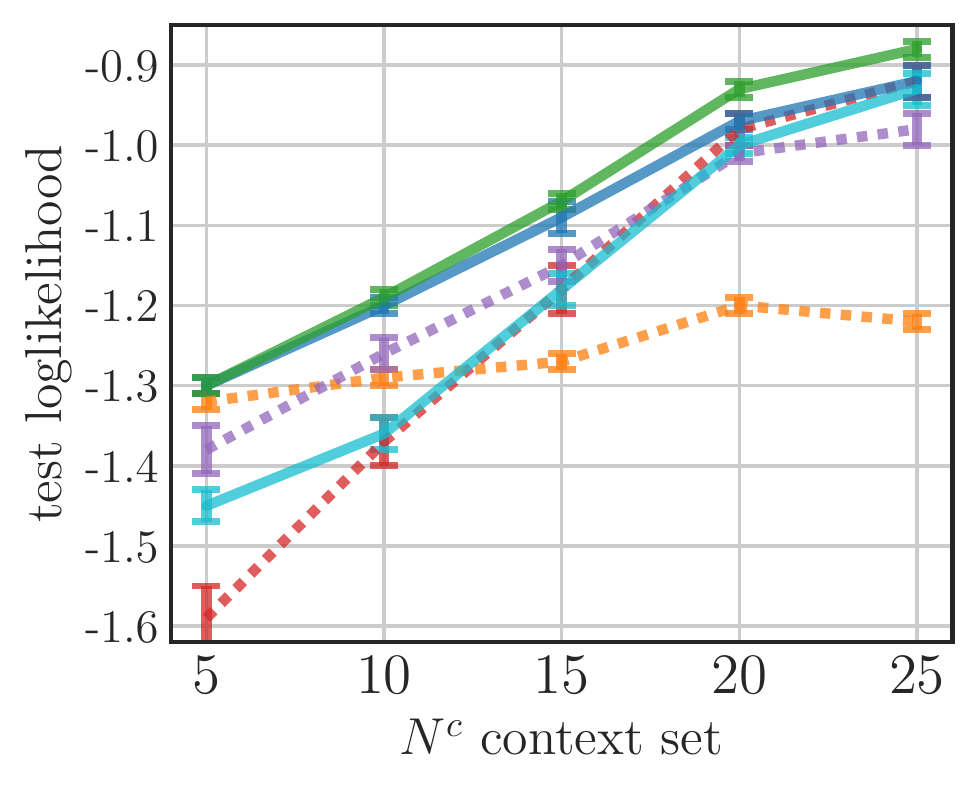}}  \hspace{0.5mm} 
\subfloat[\label{fig:exp5-1:small-h2} Sawtooth (out-range)]
{\includegraphics[width=0.24\linewidth]{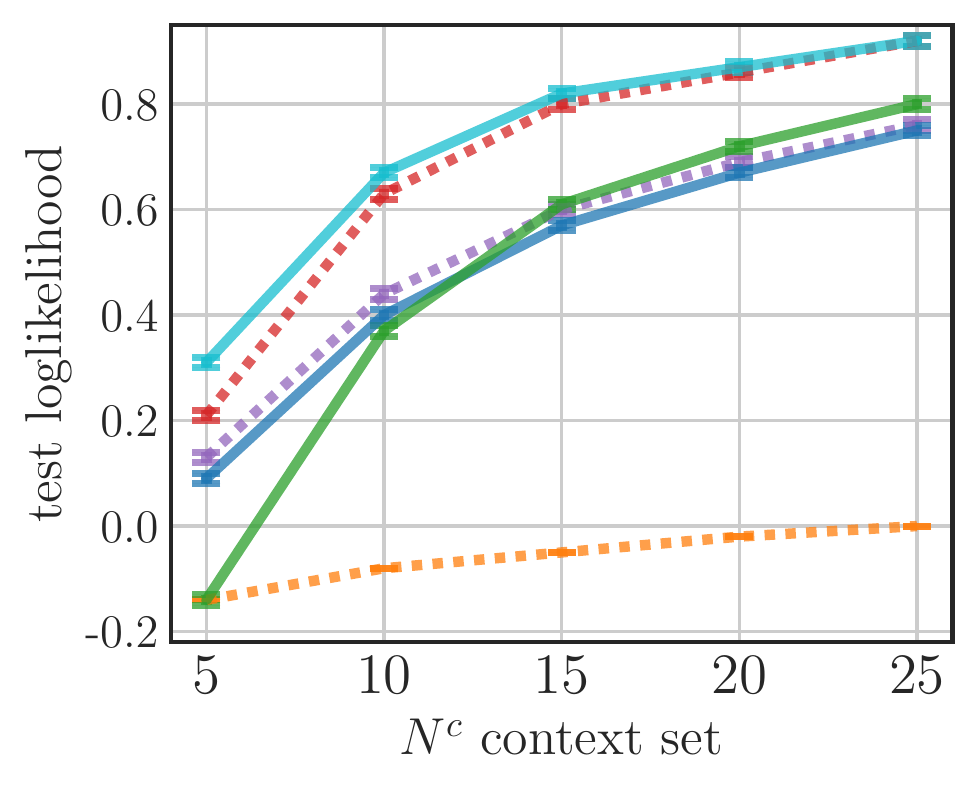}}   
\caption{Prediction result of each processes from training setting of \textb{large $N^{c}$} context points .   }
\label{fig:exp5-1:smallset_comparison}
\end{figure}
\vspace{-4mm}

\paragraph{Conclusion.} The proposed NP model ($Q=3,4,5$) using a Bayesian ConvDeepsets has shown superior prediction performances especially when training with a small number of context data points. When a more number of context points is allowed for training, the performance gap between ConvCNP and proposed method decreases as shown in \cref{fig:exp5-1:small-e,fig:exp5-1:small-e2} and \cref{fig:exp5-1:small-f,fig:exp5-1:small-f2}. 
%Also, when the number of data points 

%64 context set $\{D^{c}_{n}\}_{n=1}^{128}$ of each process

\paragraph{Prediction results for training a large number of context sets.}

Also, we report prediction results in \cref{fig:1d-singletask-prediction-large} and quantitative analysis of the trained parameters when the NP models are trained with the setting of a large number of context sets. We see that $\mathrm{p}_{\mathrm{nn}}(D^c)$ allocates the most of stationary priors as second spectral density (green) that overlaps most frequency region with the RBF prior (red). This results are quite different to the result of the setting of a small number of context sets (main). We believe that this implies why the RBF kernel smoother of ConvDeepsets could be effective when using a sufficient number of context set, and why the task-dependent stationary prior could be effective when using a small number of context set.

\begin{figure*}[h]
\subfloat[\label{fig:1d-singletask-a-large}  Spectral density]
{\includegraphics[width=0.19\linewidth  ,height=2.5cm ]{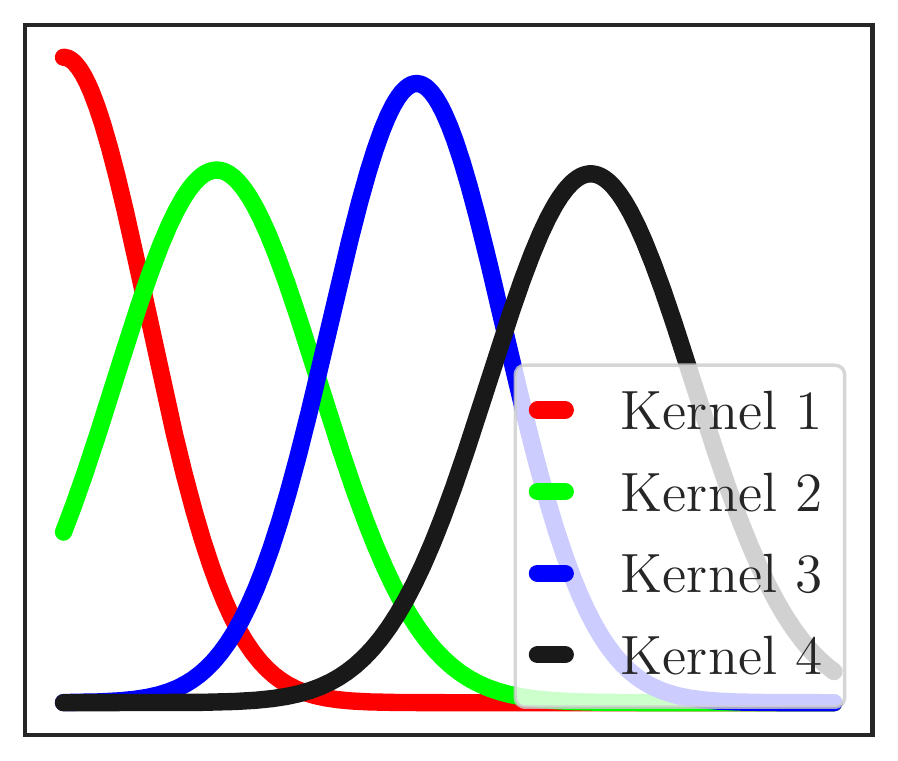}} \hspace{0.1mm}
\subfloat[\label{fig:1d-singletask-b-large} RBF]
{\includegraphics[width=0.19\linewidth ,height=2.5cm ]{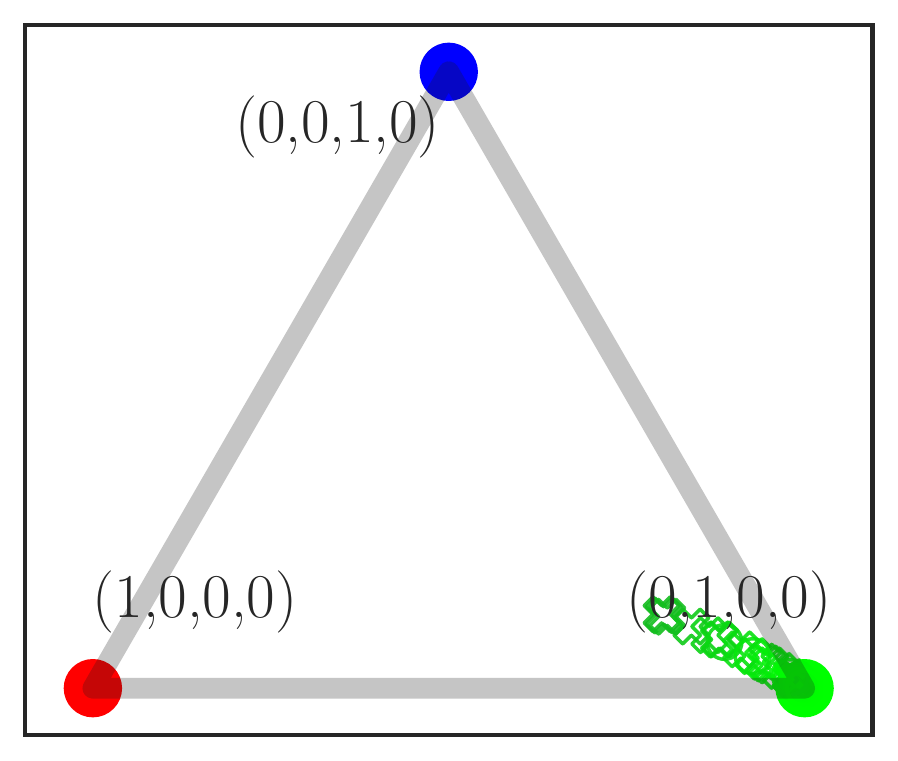}} \hspace{0.1mm}
\subfloat[\label{fig:1d-singletask-c-large} Matern-${\frac{5}{2}}$]
{\includegraphics[width=0.19\linewidth ,height=2.5cm ]{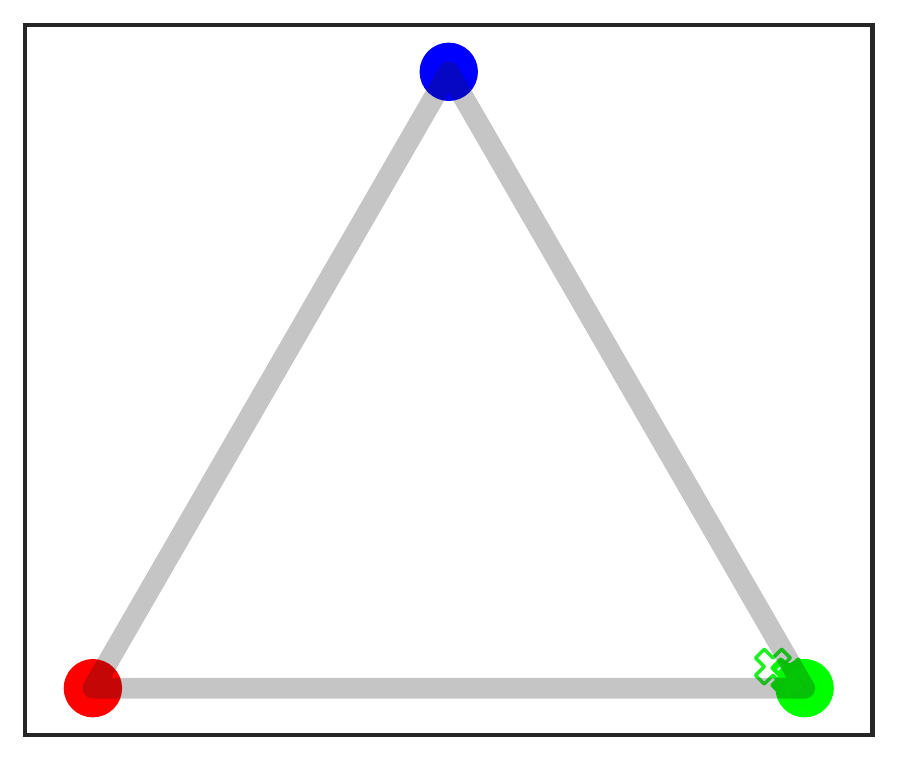}} \hspace{0.1mm}
\subfloat[\label{fig:1d-singletask-d-large} Weakly Periodic]
{\includegraphics[width=0.19\linewidth ,height=2.5cm ]{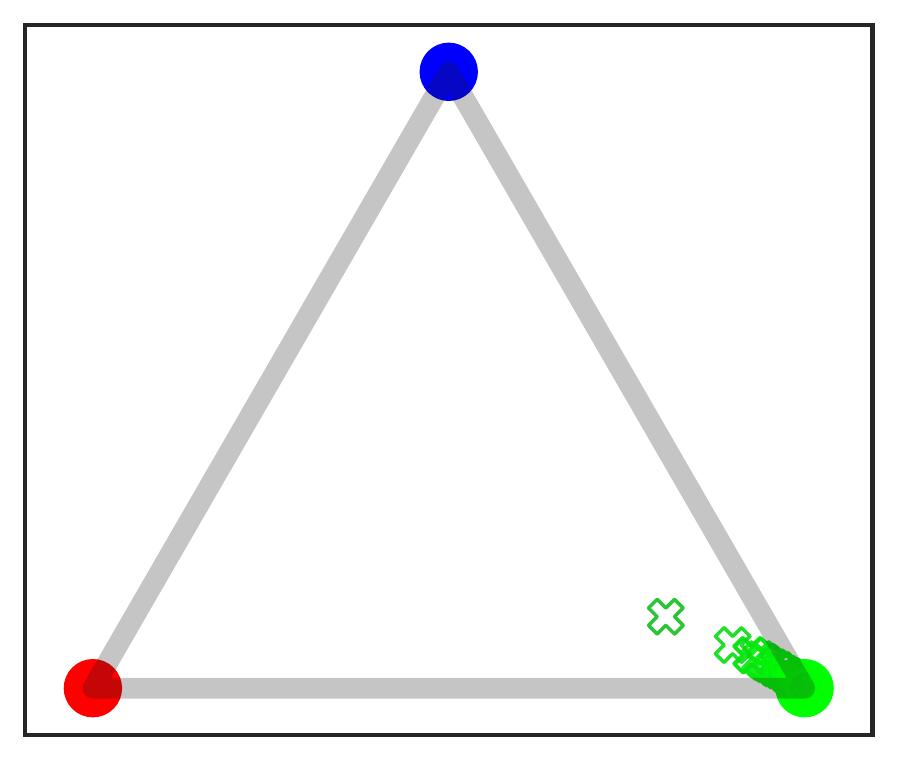}} \hspace{0.1mm}
\subfloat[\label{fig:1d-singletask-e-large} Sawtooth]
{\includegraphics[width=0.19\linewidth ,height=2.5cm ]{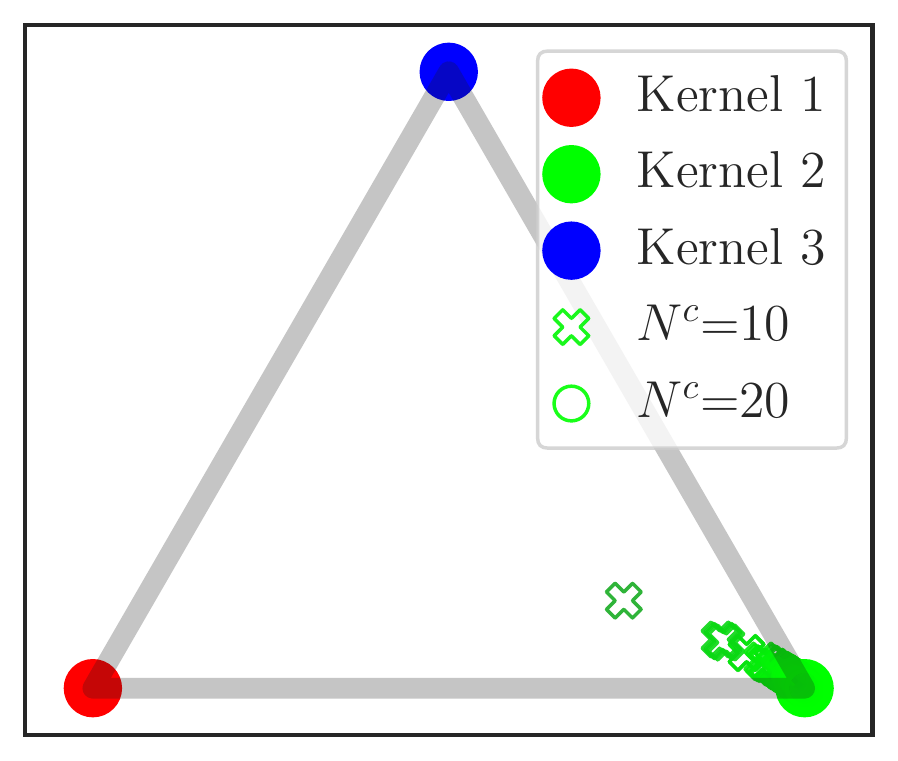}} 
\vspace{1mm}
\subfloat[\label{fig:1d-singletask-f-large} Predictive distribution of each baseline on each process ($N^c=15$) ]
{\includegraphics[width=0.99\linewidth  ]{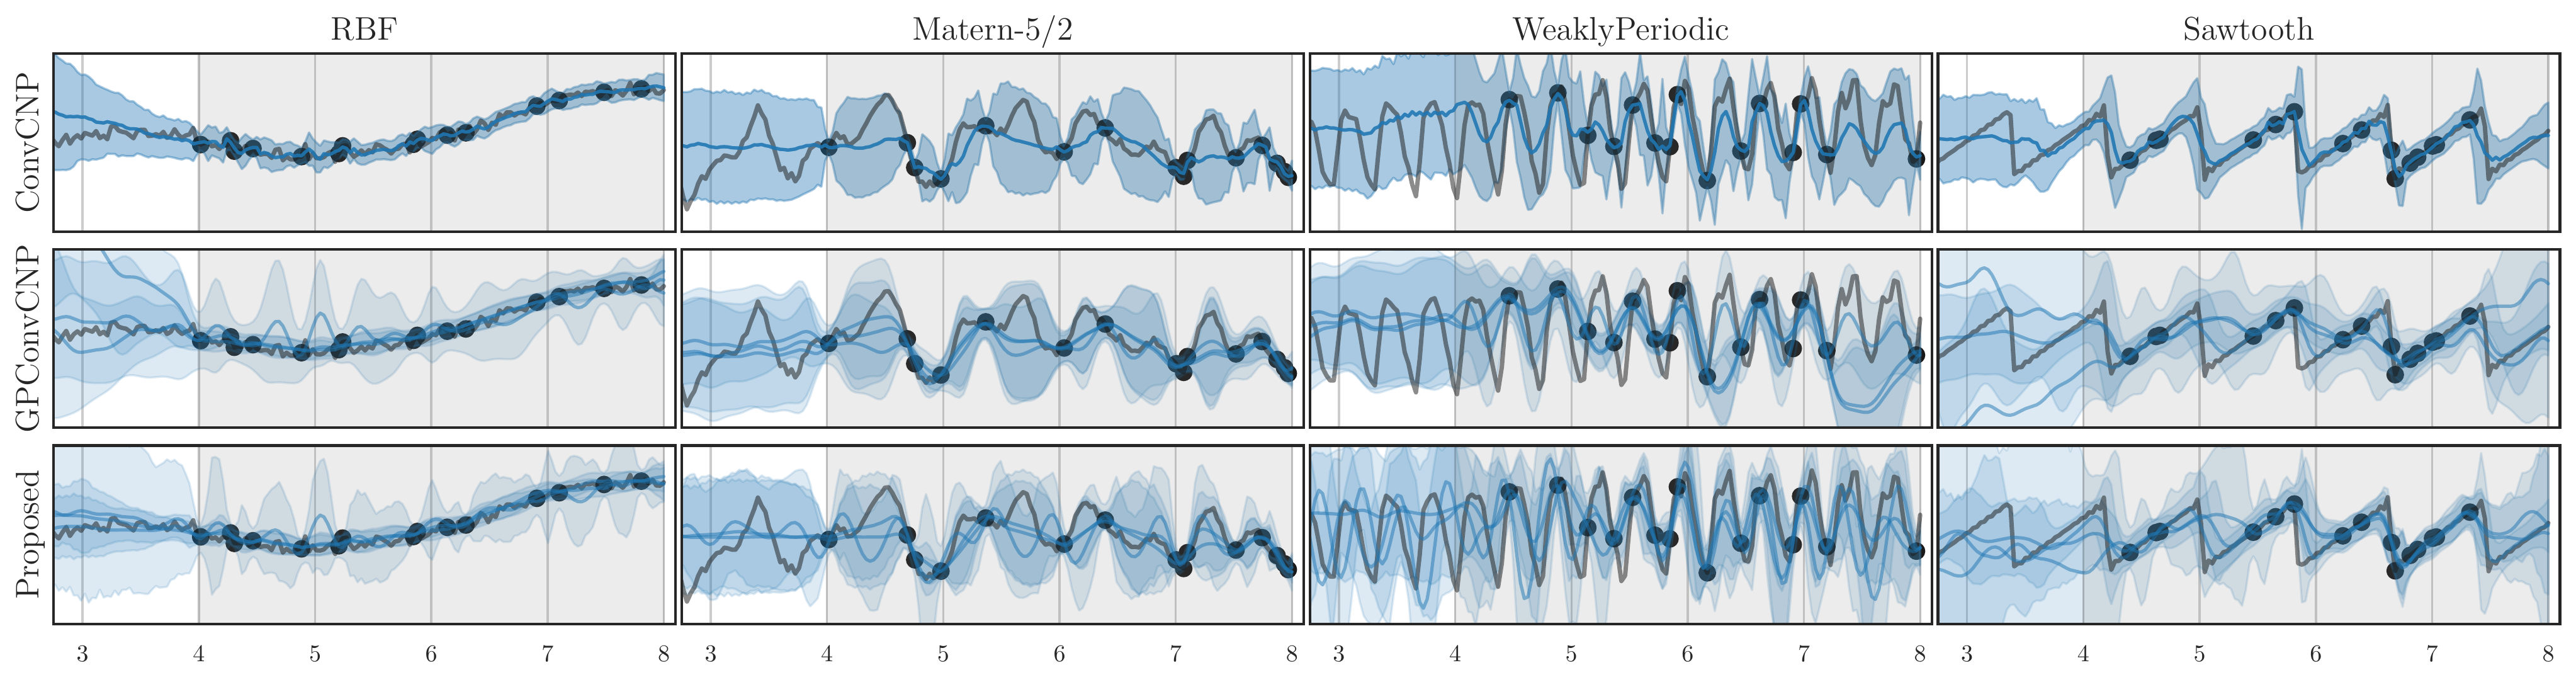}}
\caption{Stochastic processes modeling beyond training range (gray region $[4,8]$): \cref{fig:1d-singletask-a-large} denotes the trained spectral density with $Q=4$ kernels. \cref{fig:1d-singletask-b-large,fig:1d-singletask-c-large,fig:1d-singletask-d-large,fig:1d-singletask-e-large} denote the output of $\mathrm{p}_{\mathrm{nn}}(D^{c})$ for 128 context set $\{D^{c}_{n}\}_{n=1}^{128}$ of each process. \cref{fig:1d-singletask-f-large} shows the predictive distributions of the baselines on each process. 
}
\label{fig:1d-singletask-prediction-large}
\end{figure*}
\vspace{-3mm}

\paragraph{Validation error during training phase.} We report the averaged log likelihood evaluated on validation set during training; the validation set consists of $128\times 16$ tasks that have the equal number of task for each process.
\cref{fig:1d-singletask-val-small} and \cref{fig:1d-singletask-val-large} shows the validation metric over training epochs when using a small number of context set and large number of context set, respectively. In each epoch, we use $500 \times 16$ tasks for training. These figures imply that when the stationary priors are imposed well like $Q=4$, the propose model can achieve good performance while using the less number of training tasks.
\vspace{-3mm}
\begin{figure*}[h]
\centering
\subfloat[\label{fig:1d-singletask-val-small}  Small context set $N^{c}\sim U(5,25)$]
{\includegraphics[width=0.47\linewidth,height=4.5cm  ]{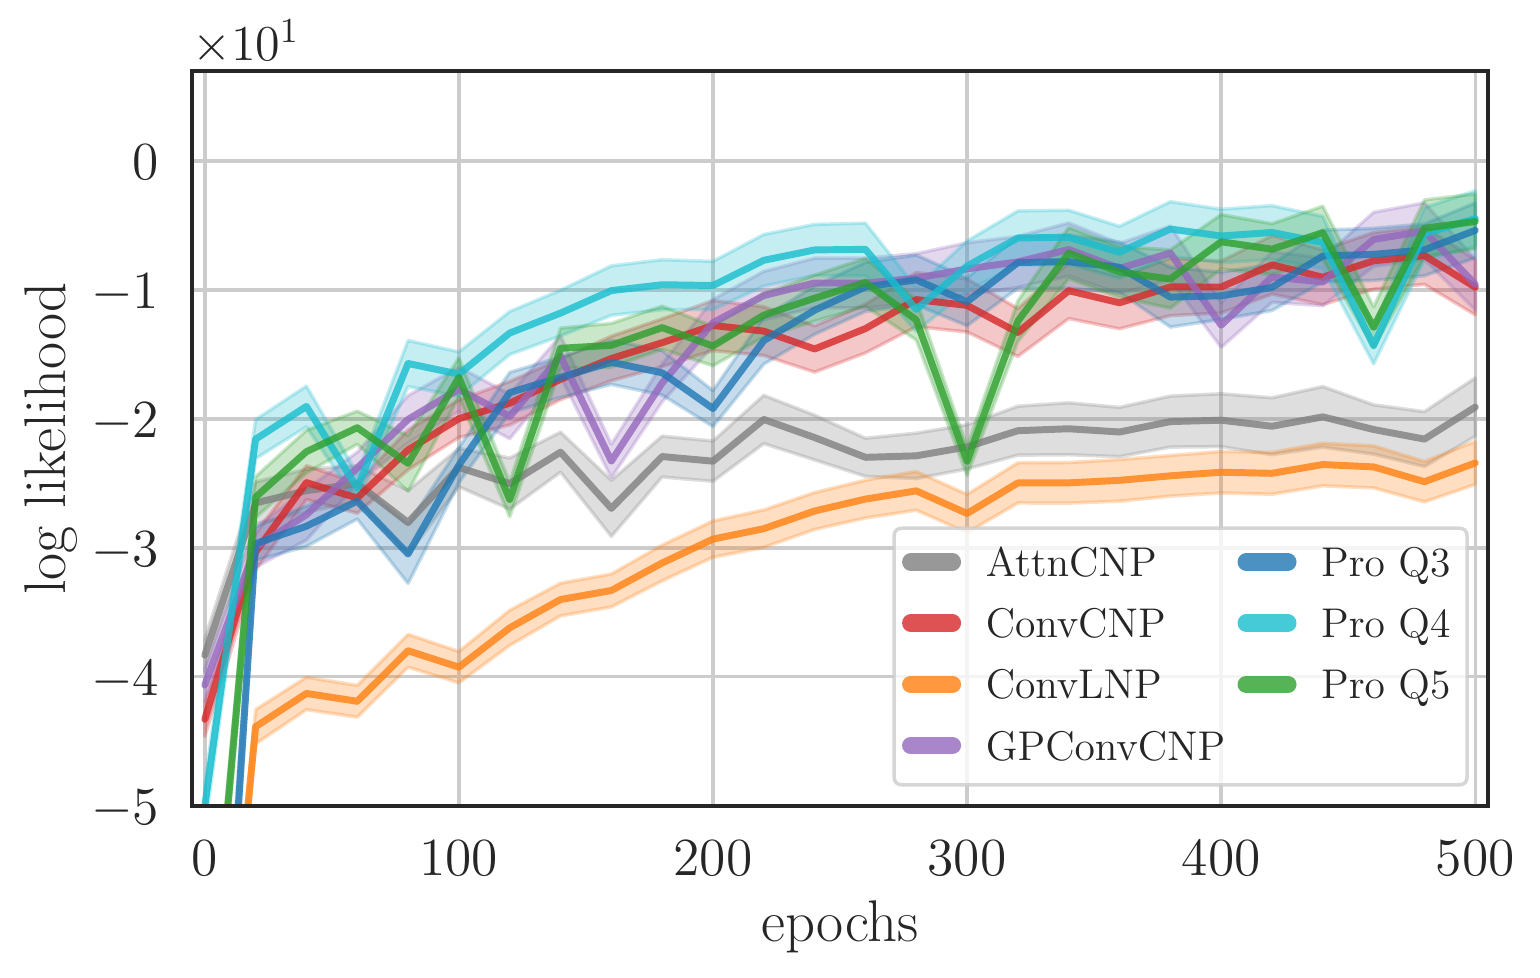}} \hspace{3mm}
\subfloat[\label{fig:1d-singletask-val-large} Large context set $N^{c}\sim U(10,50)$ ]
{\includegraphics[width=0.47\linewidth,height=4.5cm ]{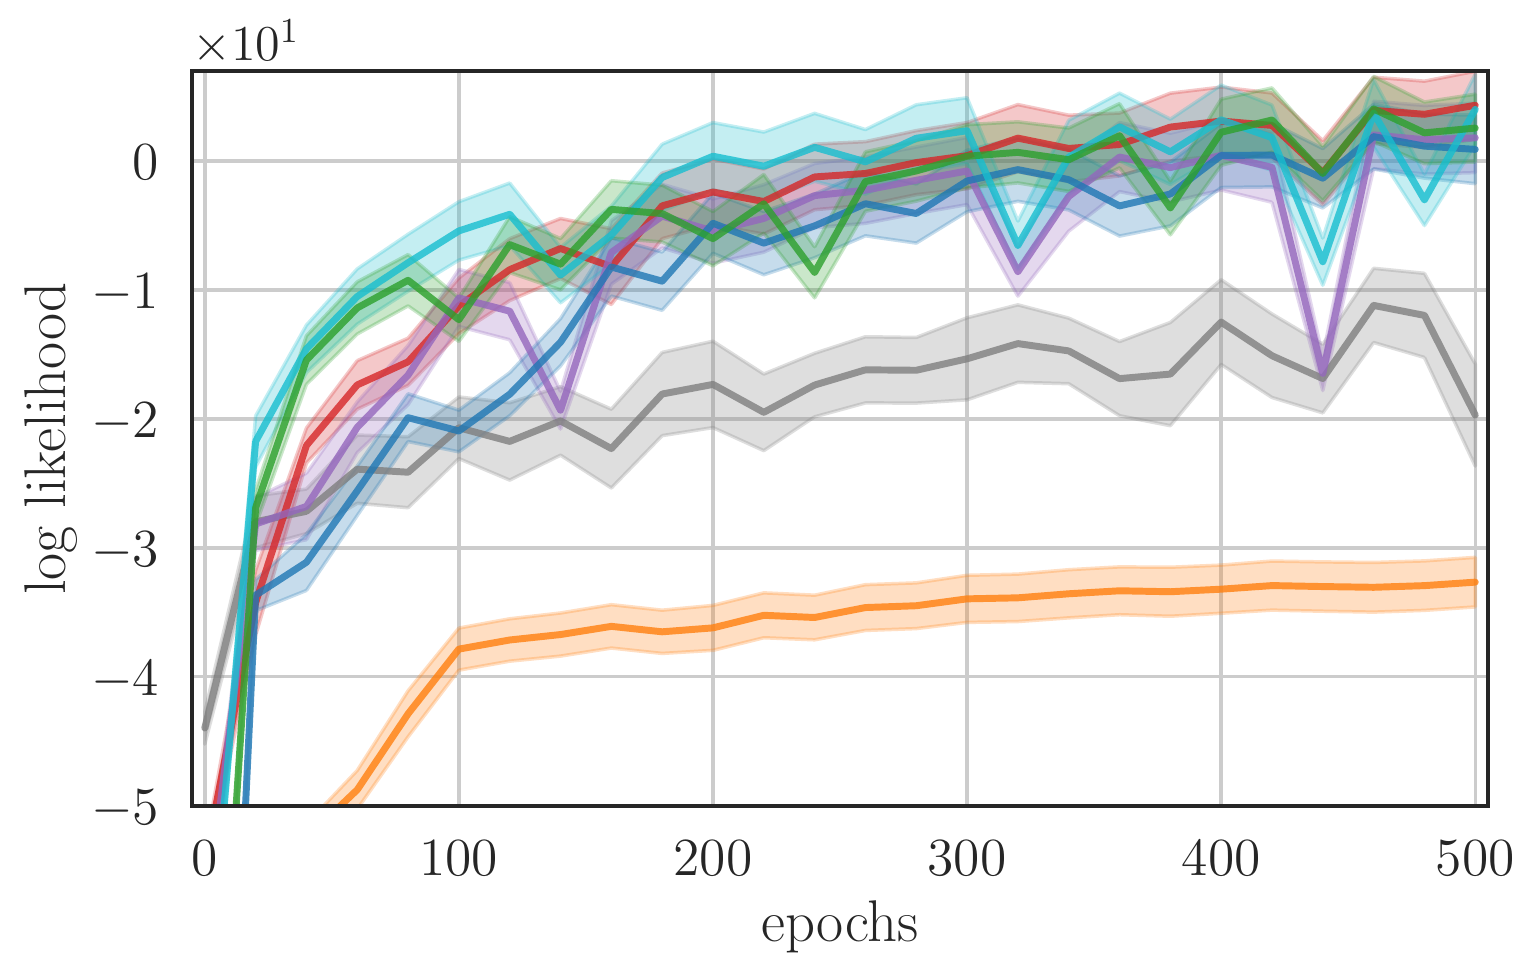}} 
\end{figure*}
