# Supplementary material for: Bayesian Convolutional Deep Sets with Task-Dependent Stationary Prior
Source: arXiv:2210.12363 source file (2022-10-22)
Supplement: Supplementary file 10 [file 07-appendix-v01-chapter3-exp2-figure01.tex]

%\clearpage

\begin{figure*}[htp!]

\centering

 \includegraphics[width=0.98\linewidth,height=1.8cm]{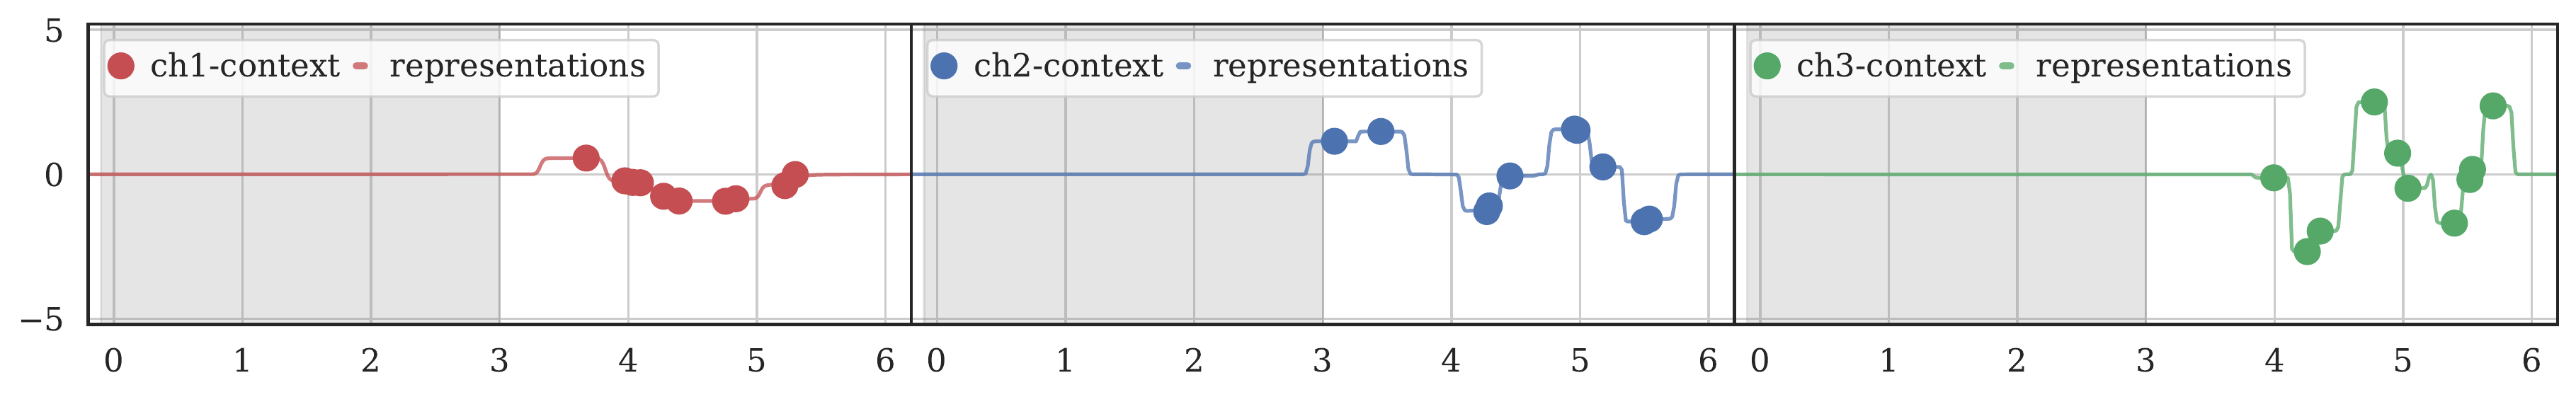}
 \vspace{-1mm}
 \includegraphics[width=0.98\linewidth,height=1.8cm]{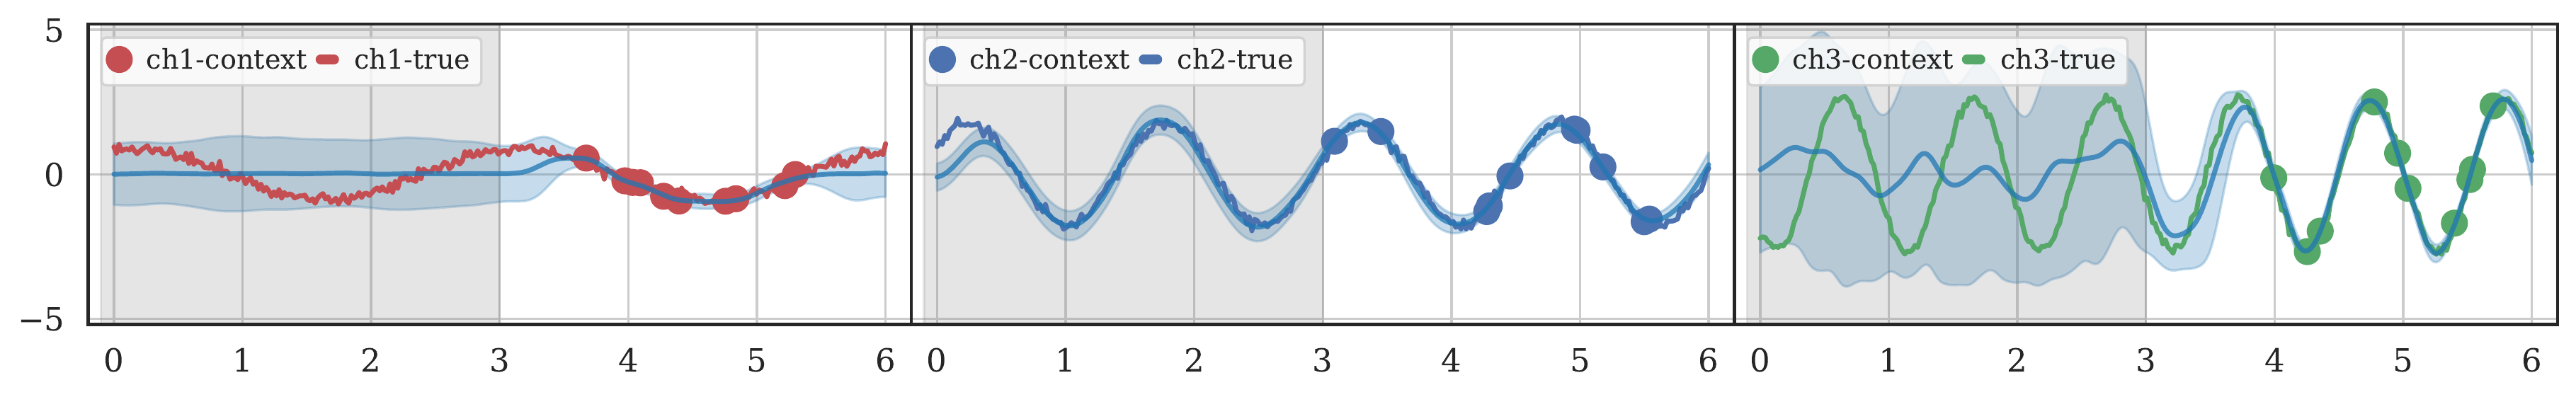}
 
\vspace{5mm}
\includegraphics[width=0.98\linewidth,height=1.8cm]{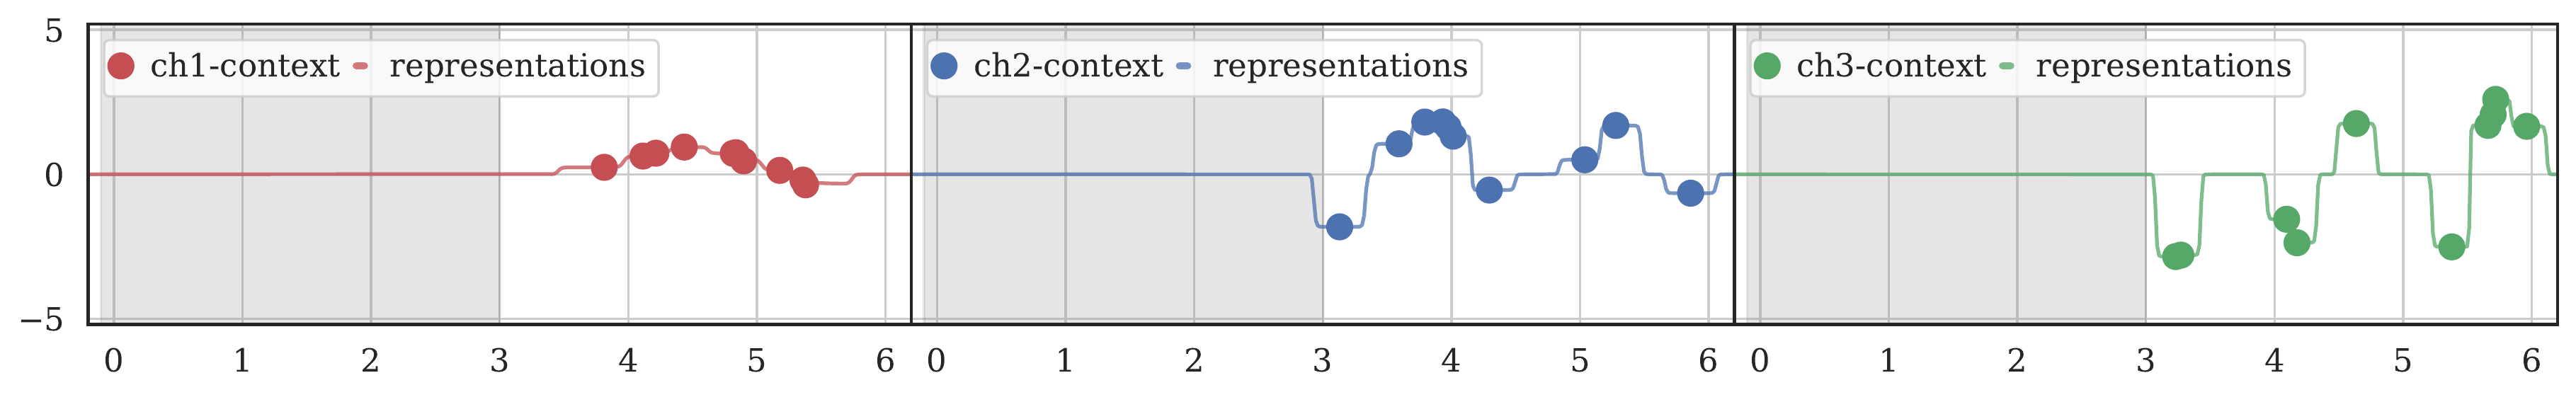}
\vspace{-1mm}
 \includegraphics[width=0.98\linewidth,height=1.8cm]{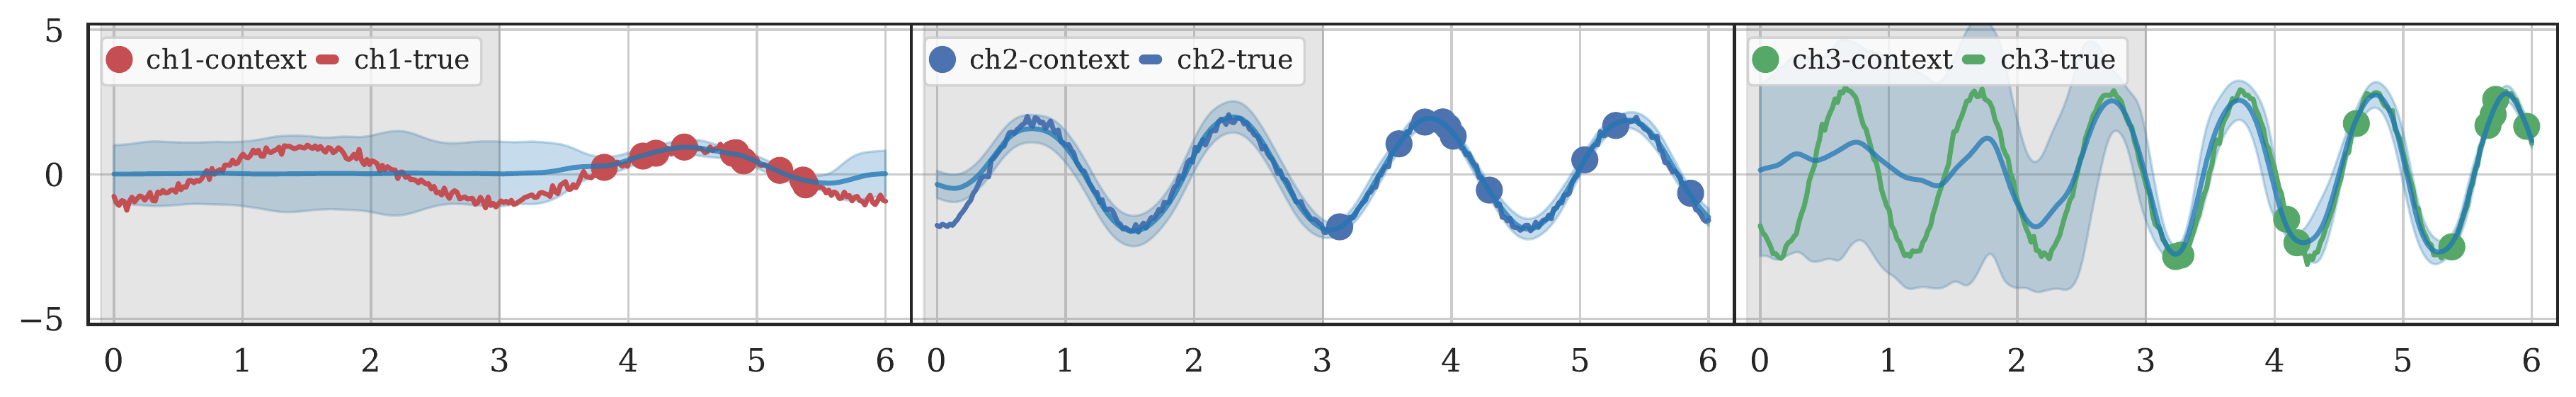}

\caption{ \textb{ConvCNP} prediction results of \textb{Sinusoidal Process}; 10 context data points ($N^{c}=10$) per channel observed outside training range $[3,6]$ are used. The first row shows the functional representation, and the second row denotes its prediction results. The third row and fourth row correspond to the functional representation of the different task, and its prediction result, respectively.}
\label{fig:sin-a}
\end{figure*}

\vspace{10mm}

\begin{figure*}[htp!]

\centering

 \includegraphics[width=0.98\linewidth,height=1.8cm]{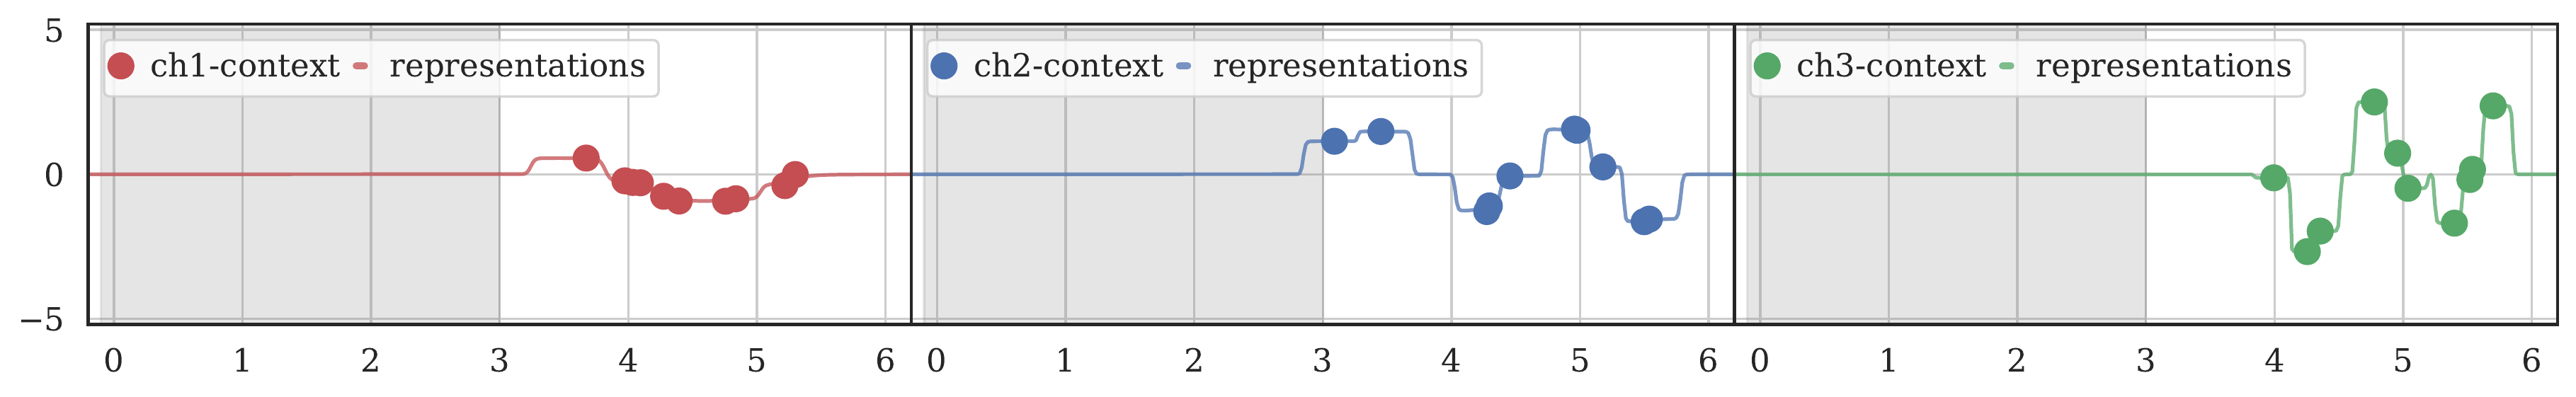}
 \vspace{-1mm}
 \includegraphics[width=0.98\linewidth,height=1.8cm]{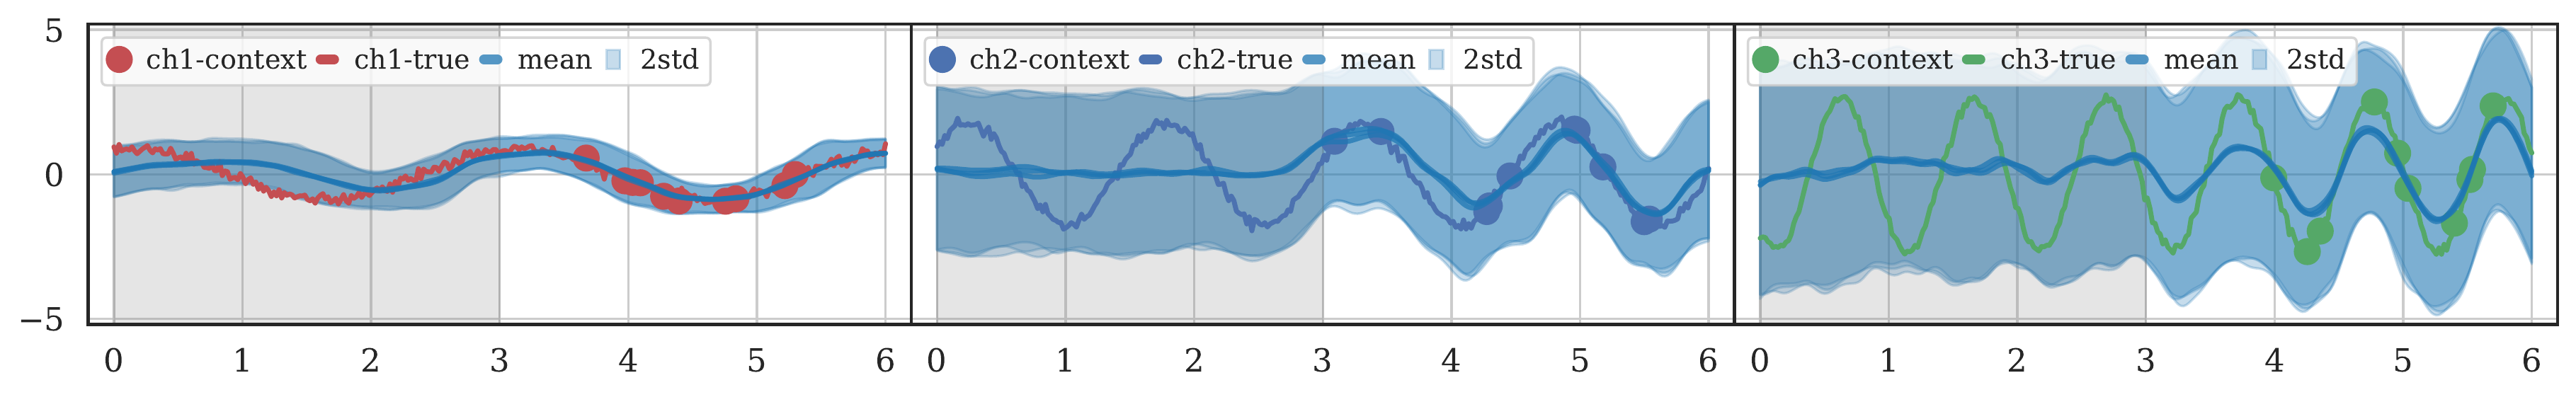}
 
\vspace{5mm}
\includegraphics[width=0.98\linewidth,height=1.8cm]{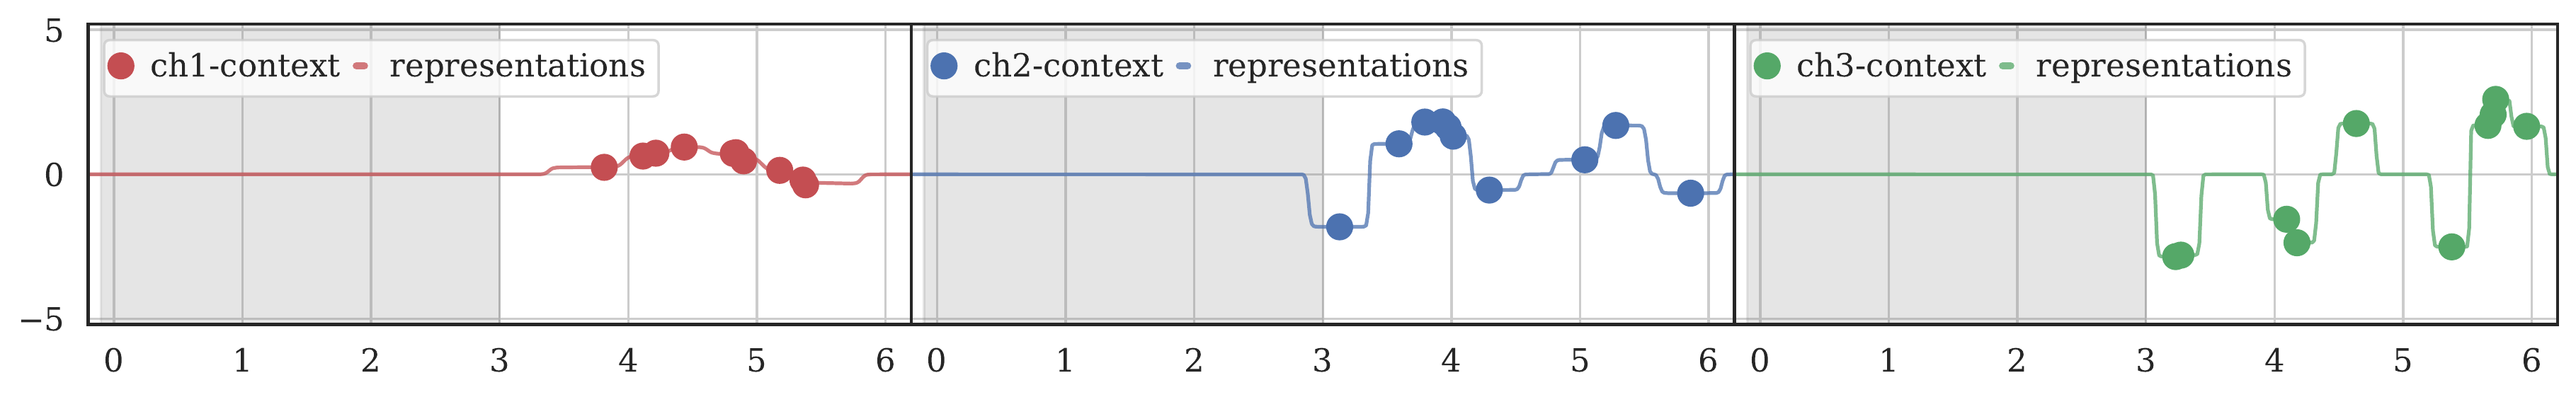}
\vspace{-1mm}
 \includegraphics[width=0.98\linewidth,height=1.8cm]{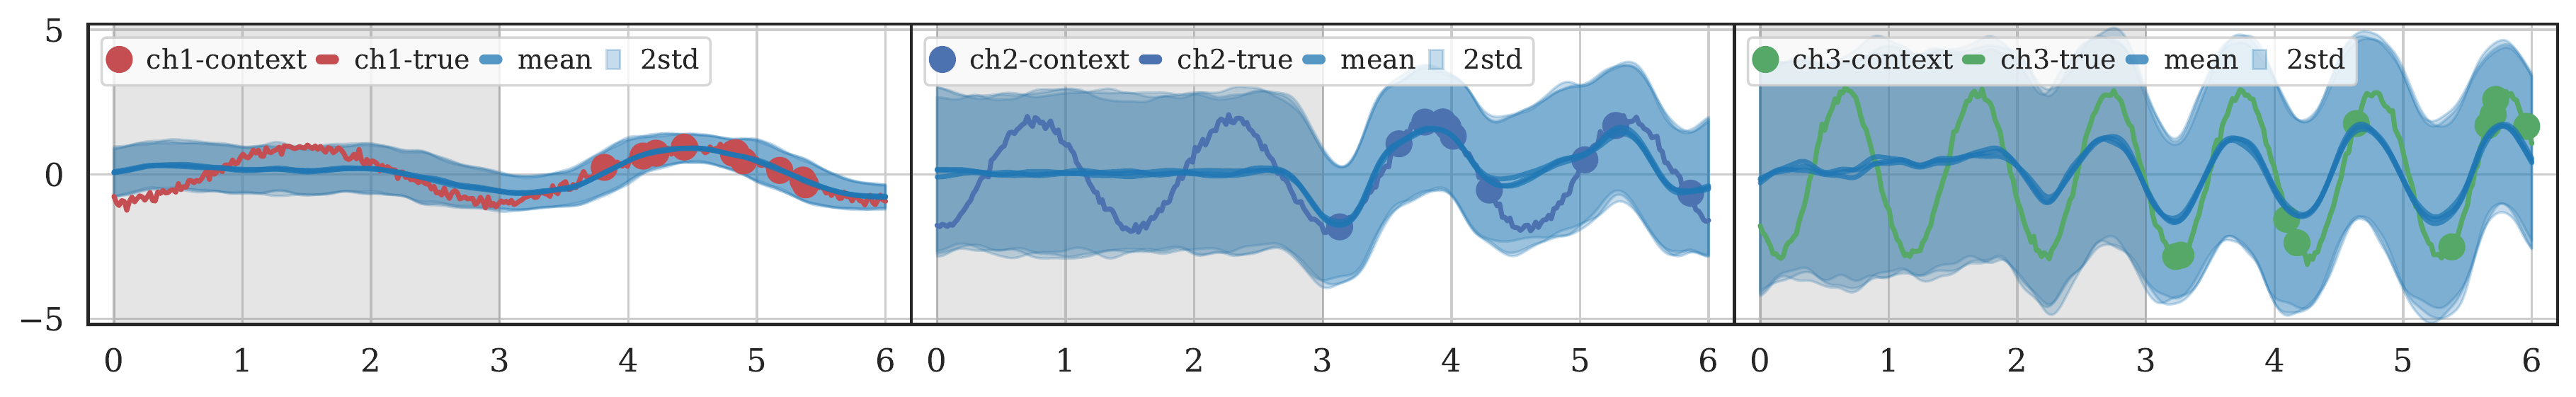}

\caption{ \textb{ConvLNP} prediction results of \textb{Sinusoidal Process}; 10 context data points ($N^{c}=10$) per channel observed outside training range $[3,6]$ are used. The first row shows 4 functional representations, and the second row denotes its prediction results. The third row and fourth row correspond to 4 functional representations of the different task, and its prediction result, respectively.}
\label{fig:sin-b}
\end{figure*}

\clearpage
\begin{figure*}[htp!]

\centering

 \includegraphics[width=0.98\linewidth,height=1.8cm]{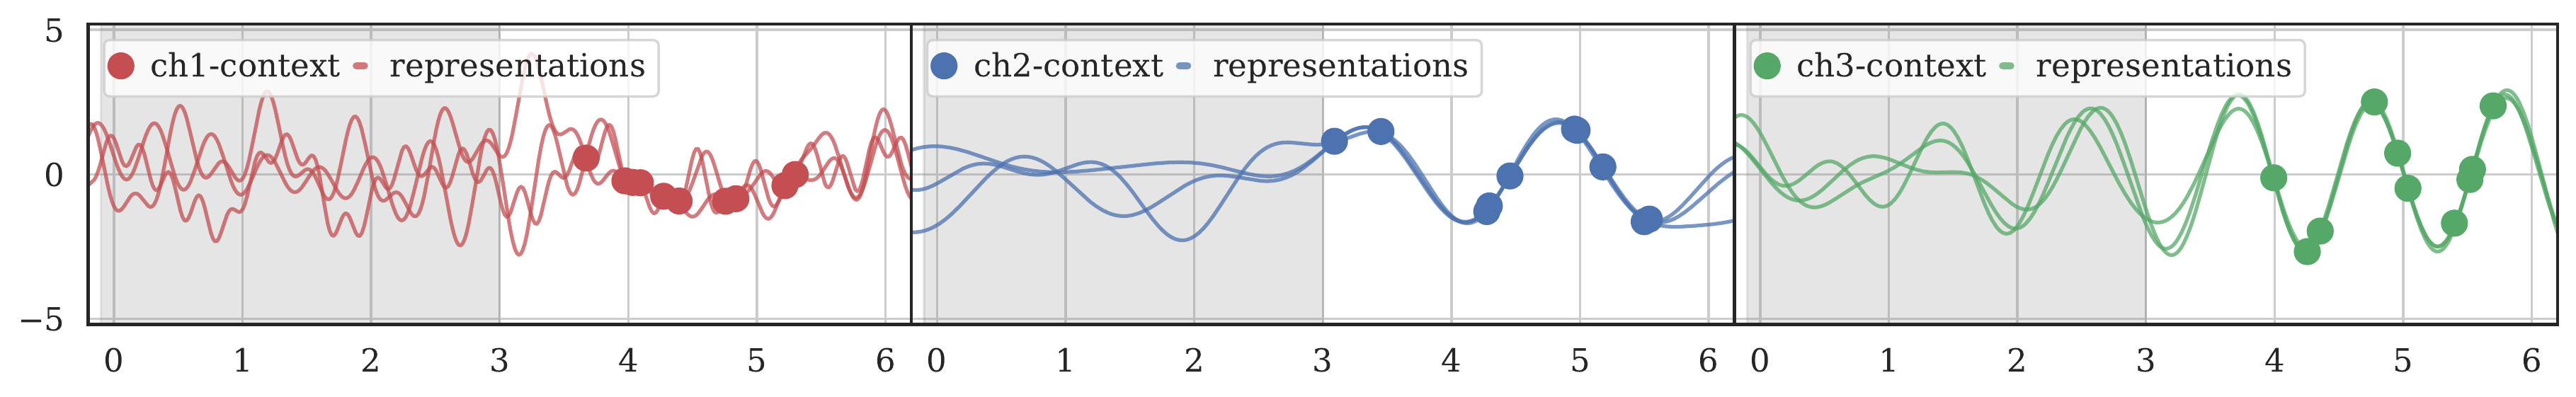}
 \vspace{-1mm}
 \includegraphics[width=0.98\linewidth,height=1.8cm]{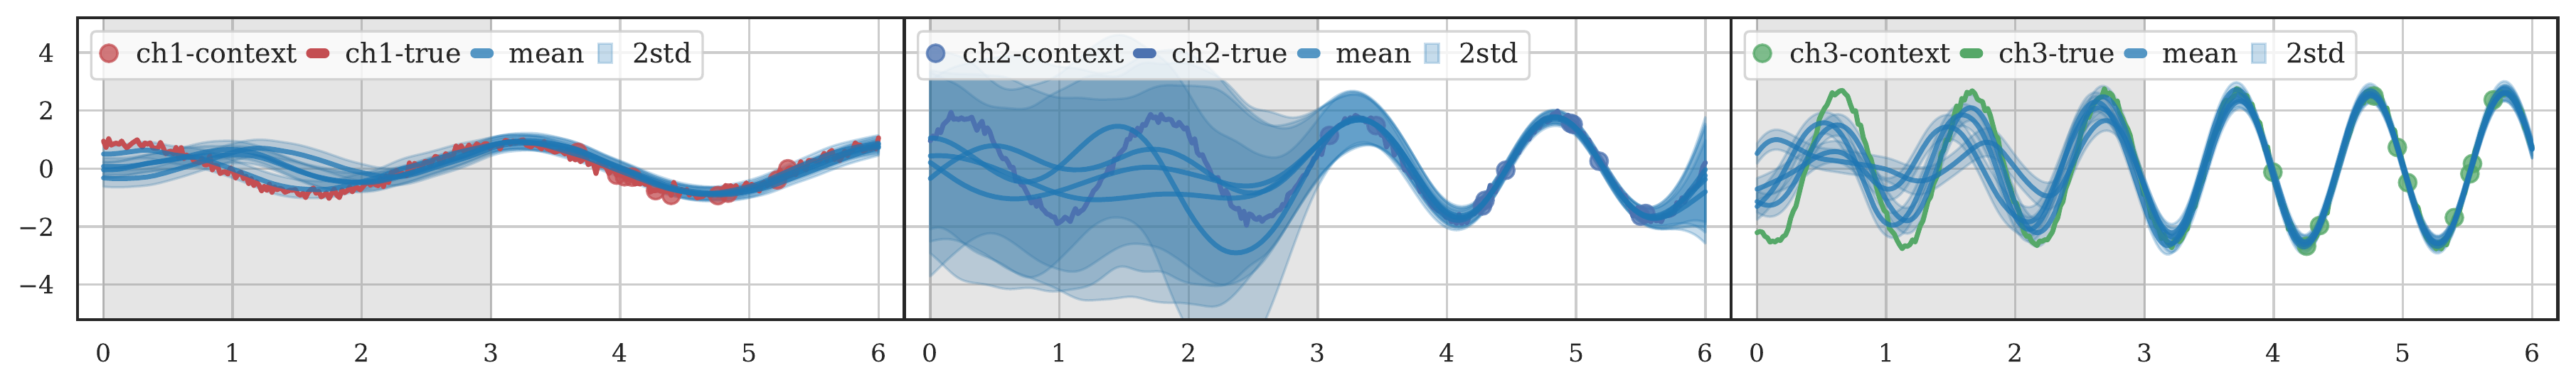}
 
\vspace{5mm}
\includegraphics[width=0.98\linewidth,height=1.8cm]{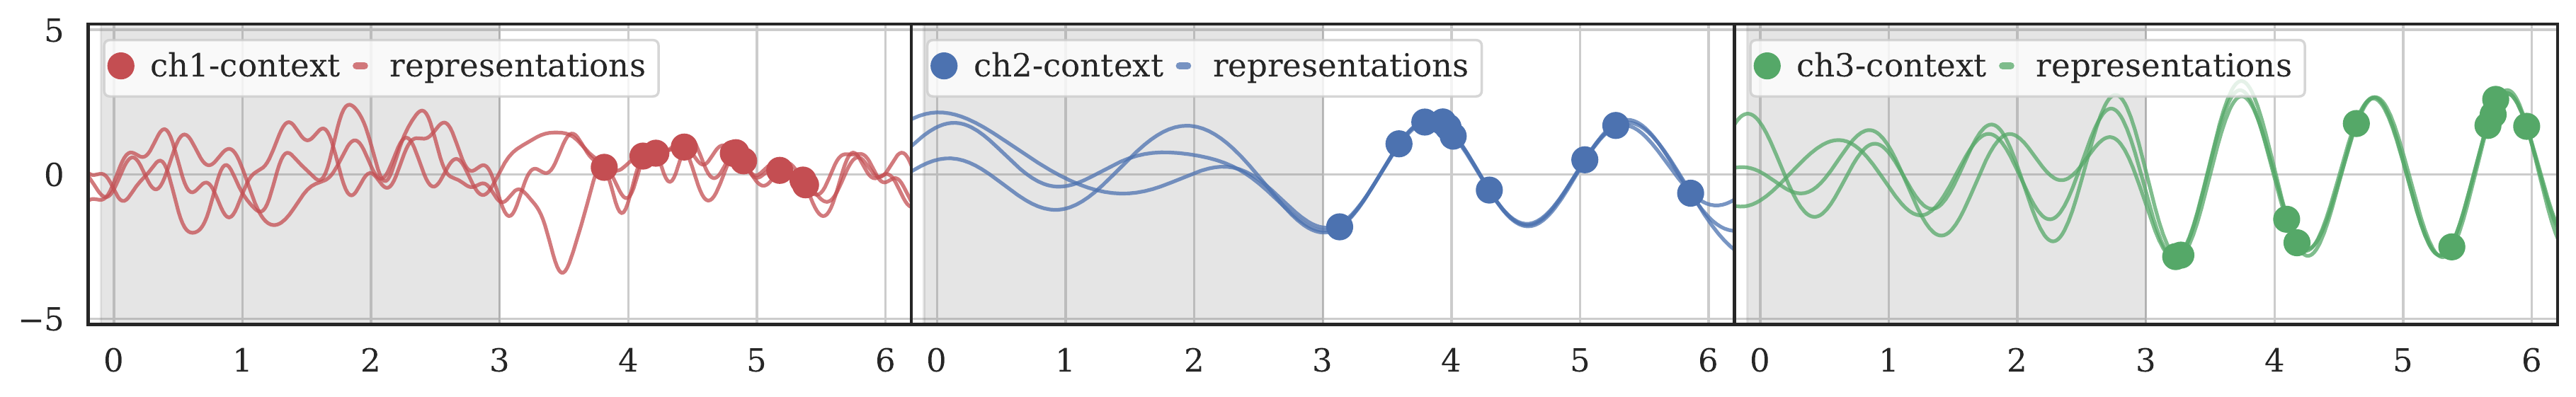}
\vspace{-1mm}
 \includegraphics[width=0.98\linewidth,height=1.8cm]{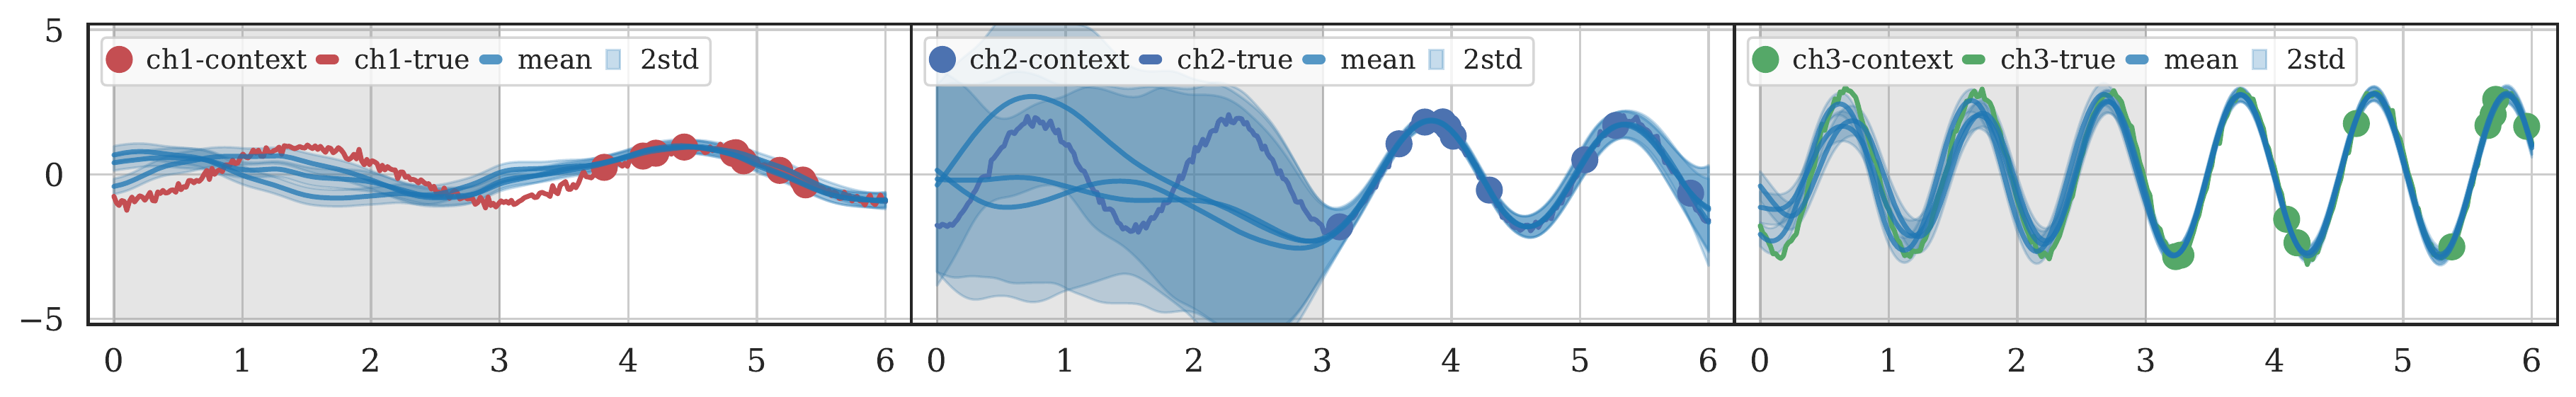}

\caption{ \textb{GPConvCNP} prediction results of \textb{Sinusoidal Process}; 10 context data points ($N^{c}=10$) per channel observed outside training range $[3,6]$ are used. The first row shows 4 functional representations, and the second row denotes its prediction results. The third row and fourth row correspond to 4 functional representations of the different task, and its prediction result, respectively.}
\label{fig:sin-c}
\end{figure*}

\vspace{10mm}
\begin{figure*}[htp!]

\centering

 \includegraphics[width=0.98\linewidth,height=1.8cm]{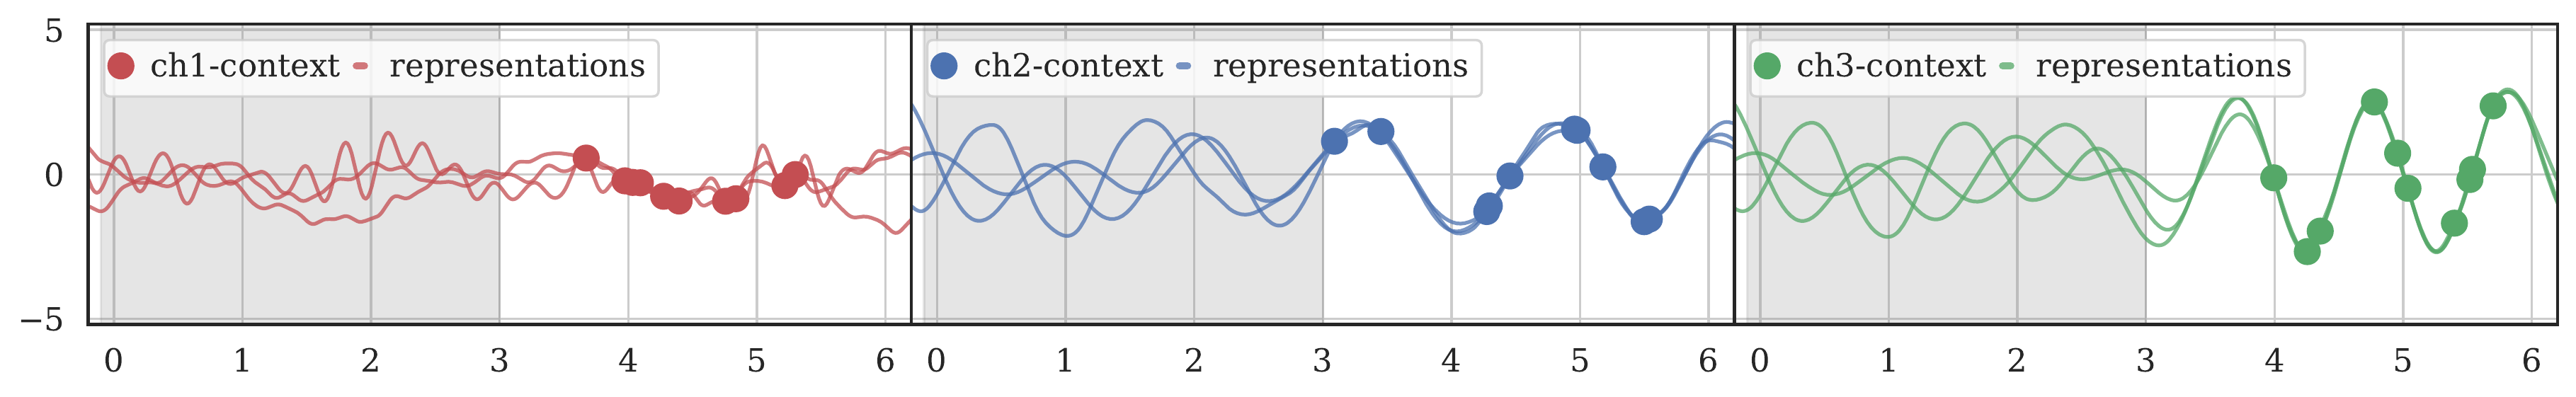}
 \vspace{-1mm}
 \includegraphics[width=0.98\linewidth,height=1.8cm]{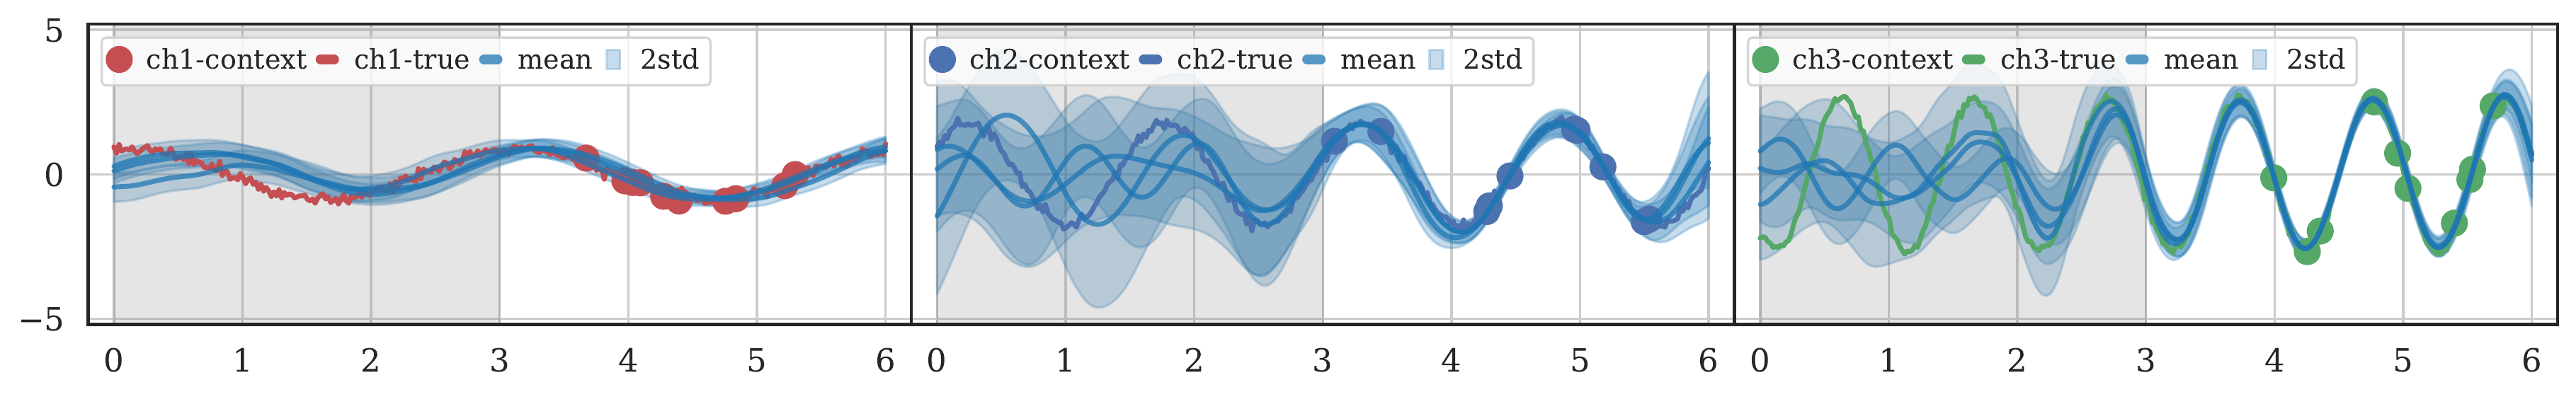}
 
\vspace{5mm}
\includegraphics[width=0.98\linewidth,height=1.8cm]{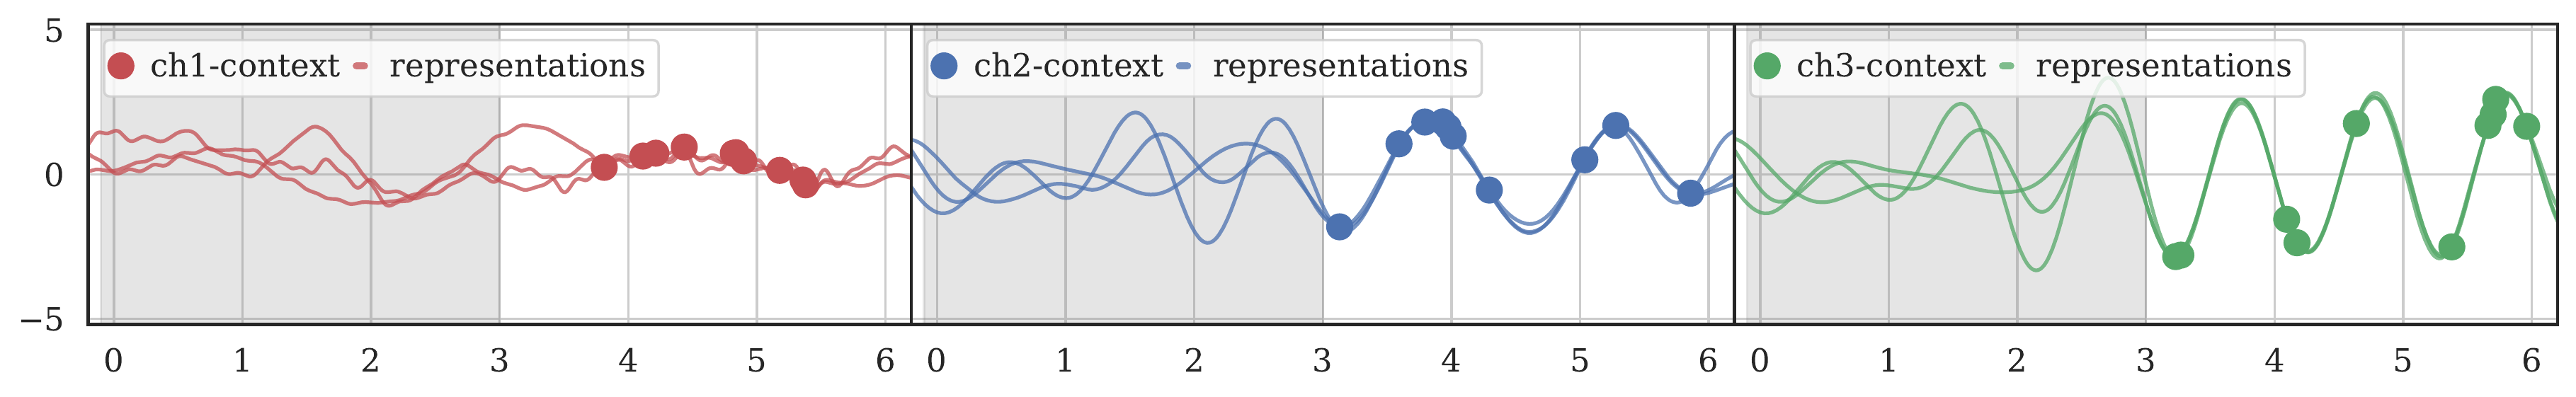}
\vspace{-1mm}
 \includegraphics[width=0.98\linewidth,height=1.8cm]{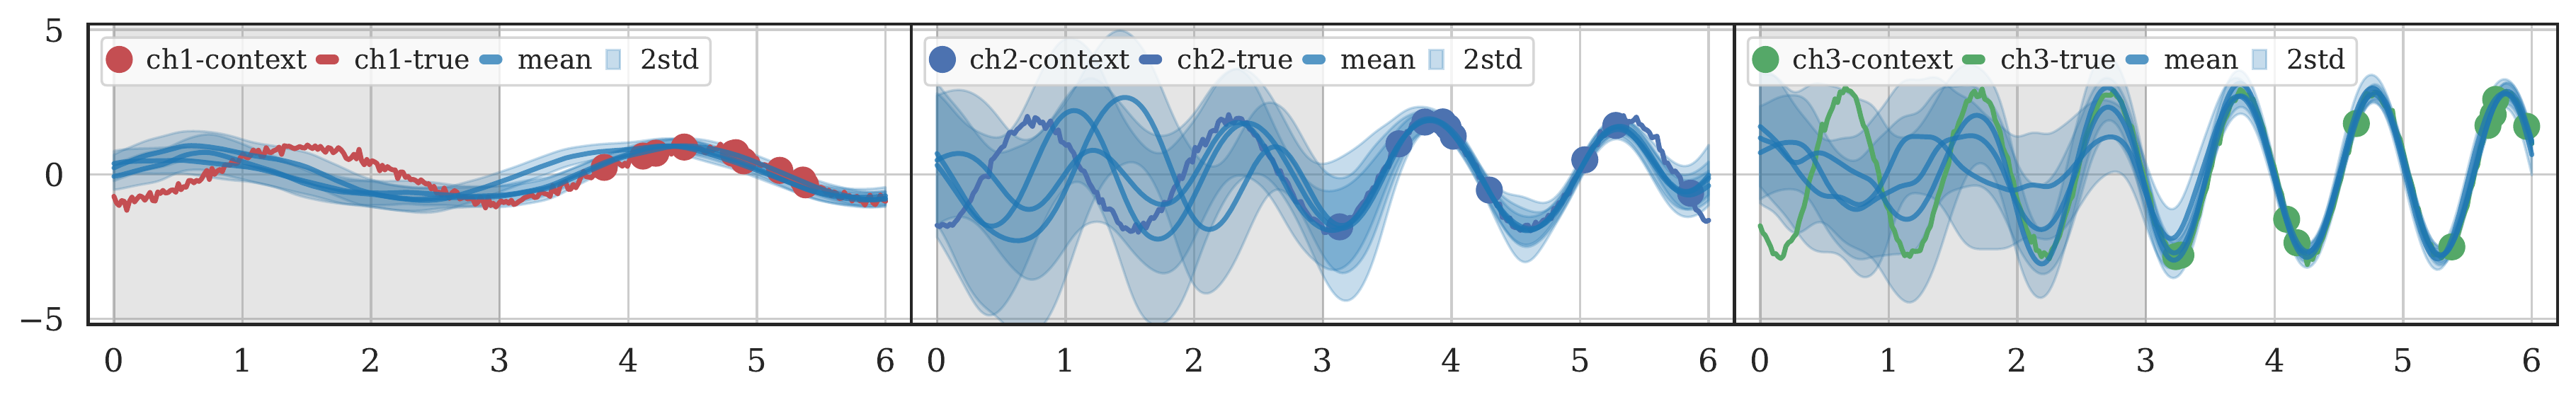}

\caption{ \textb{Proposed model} prediction results of \textb{Sinusoidal Process}; 10 context data points ($N^{c}=10$) per channel observed outside training range $[3,6]$ are used. The first row shows 3 functional representations, and the second row denotes its prediction results. The third row and fourth row correspond to 3 functional representations of the different task, and its prediction result, respectively.}
\label{fig:sin-d}
\end{figure*}
