# Supplementary material for: Bayesian Convolutional Deep Sets with Task-Dependent Stationary Prior
Source: arXiv:2210.12363 source file (2022-10-22)
Supplement: Supplementary file 13 [file 07-appendix-v01-chapter3-exp2.tex]

\section{Further Details for Multi-Channel Regression Task}
\label{appendix:nd-regression-task}

% sine wave function $f_i$ has following function as \ 
%         \[
%             f_{i}(t) = \sin{(w_i + \theta_i) (t - \phi_i) } + \epsilon  \newline \\ 
%         \]

\subsection{Details for Datasets}

In this section, we consider two types of the multi-channel stationary process: (1) sinusoidal process and (2) GP using the Multi-output SM kernel (MOSM) \citeb{parra2017spectral}, that constructs the cross covariance function of two different processes based on Crammer theorem, i.e., a multi-channel extension of Bochner's theorem. Additionally, we consider two types of tasks for each process: (1) a simple task and a difficult task having more diversity to study how the task-dependent prior on functional representation affects the performance of the corresponding NP model depending on task diversity. We hypothesis that when the small number of data points is given for the task having more diversity, assigning a reasonable prior on functional representation could be helpful to solve the targeted tasks. Each process is described as follows:
\begin{itemize}[leftmargin=1em]
\item  \textbf{Sinusoidal-phase} : $i$-th channel context and target sets are constructed by randomly choosing $N^{(i)}_{c}$ data points and $N^{(i)}_{t}$ data points from the sampled function $f_i(t)$, that is represented as $$ f_{i}(t) = A_i\sin{ \left( 2\pi w_i (t - \phi_i) \right)} + \epsilon, \hspace{10mm}  i=1,2,3  \hspace{3mm}, $$ where $A_i$ denotes $i$-th channel amplitude parameter, $w_i$ denotes $i$-th channel frequency parameter, $ \phi_i$ denotes $i$-th channel phase parameters, and $\epsilon$ is random noise satisfying $\epsilon \sim N(0,0.1^2)$. For frequency parameters, we set $w_1 = 2.1, w_2 = 4.1$, and $w_3=6.1$. For the amplitude, we set $A_1=1 + a, A_2=2 + a$, and $A_3=3 + a$ by using a random amplitude $a \sim \mathcal{U}([-25,0.25])$. For the phase parameter, we consider random phase $\tau_{1} \sim \mathcal{U}([-1,1]), \tau_{2} \sim \mathcal{U}([-1.5,0.5])$, and $\tau_{3} \sim \mathcal{U}([-2,0])$. The random parameters for amplitude $a$ and phases $\{\tau_1,\tau_2,\tau_3\}$ are randomly sampled for each task.

\item  \textbf{Sinusoidal-all}  : $i$-th channel context and target sets are constructed by randomly choosing $N^{(i)}_{c}$ data points and $N^{(i)}_{t}$ data points from the sampled function $f_i(t)$, that is represented as  that is represented as $$ f_{i}(t) = A_i\sin{ \left( 2\pi (w_i + \theta_i) (t - \phi_i) \right)} + \epsilon  \hspace{10mm}  i=1,2,3, $$ where $\theta_i$ denotes $i$-th channel random frequency parameter. In this generation procedure, we consider random frequency parameters additionally; we first sample $\theta \sim \mathcal{U}([0,5])$, and set $\theta_1 = \theta, \theta_2 = 2\theta$, and $\theta_3 = 3\theta$. This is intended to let the task of this process have more diversity. For other parameters $\{A_i,w_i,\phi_i\}_{i=1}^{3}$, we set the same setting as described in \textbf{Sinusoidal}.

% k_{i j}(\tau) = \displaystyle\sum_{q=1}^{Q} \alpha_{ij}^{(q)} \exp \left ( - \frac{1}{2} (\tau + \theta_{ij}^{(q)})^{\top} \Sigma_{ij}^{(q)} (\tau + \theta_{ij}^{(q)}) \right ) \cos \left((\tau + \theta_{ij}^{(q)})^{\top} \mu_{ij}^{(q)} + \phi_{ij}^{(q)}  \right) 
% where $\alpha_{ij}^{(q)} = w_{ij}^{(q)} (2\pi)^{\frac{n}{2}} | \Sigma_{ij}^{(q)} |^{1/2}  $ and the superindex $(\cdot)^{(q)}$ denotes the parameter of the $q^\text{th}$ component of the spectral mixture. 

%$\Sigma_1=\mathrm{Diag}([0.5])$, $\Sigma_2=0.5$, $\Sigma_3=\mathrm{Diag}([0.5])$ for covarinace parameters
%http://143.248.92.34:8888/lab/workspaces/auto-K/tree/UAI22_CCCNP_from108/dataset_multitask_1d.py
\item  \textbf{MOSM}: : $i$-th channel context and target sets are constructed by randomly choosing $N^{(i)}_{c}$ data points and $N^{(i)}_{t}$ data points from $i$-th channel function of the multi-output function sampled from Gaussian Process (GP) with the following kernel function $\{k_{ij}\}_{i,j=1}^{3}$ of which the cross kernel $k_{ij}$ between $i$-th channel and $j$-th channel is represented as $$k_{ij}(x, x') = \exp \left ( - \frac{1}{2} ( x-x' + \theta_{ij})^{\top} \Sigma_{ij} (x-x' + \theta_{ij}) \right ) \cos \left( 2\pi(x-x' + \theta_{ij})^{\top} \mu_{ij} + \phi_{ij}  \right), $$
where $\mu_{i j}  =  (\Sigma_{i} + \Sigma_{j})^{-1} (\Sigma_{i} \mu_{j} + \Sigma_{j} \mu_{i})$, $\Sigma_{ij}  = 2\Sigma_{i}(\Sigma_{i} + \Sigma_{j})^{-1} \Sigma_{j}$, $\phi_{ij} = \phi_i - \phi_j$, and $\phi_{ij} = \phi_i - \phi_j$ when $\mu_{i}$ denote $i$-th channel mean parameter, $\Sigma_{i}$ denotes $i$-th channel covariance parameter, $\theta_{i}$ denotes $i$-th channel delay parameter, and $\phi_i$ denotes $i$-th channel phase parameter, respectively. In this experiment, we set 
$\mu_1=0.1$, $\mu_2=3.0$, $\mu_3=5.0$ for mean parameters and $\Sigma_1=0.1$, $\Sigma_2=0.1$, $\Sigma_3=0.1$ for covariance parameters. We set $\theta_i=1$ with $i=1,2,3$ for delay parameters and $\phi_i=0$ with $i=1,2,3$ for phase parameters. We employ the following implementation \citeb{mogptk} \footnotemark{\footnotetext[3]{\url{https://github.com/GAMES-UChile/mogptk}}}.

\item  \textbf{MOSM-varying}: $i$-th channel context and target sets are constructed by randomly choosing $N^{(i)}_{c}$ data points and $N^{(i)}_{t}$ data points from $i$-th channel function of the multi-output function as described in $\textbf{MOSM}$ with different hyperparameter setting. We consider random mean parameters to generate the diverse tasks. We consider the random mean parameters; we first sample perturb noises $\{n_j\}_{j=1}^{3} \sim N(0,.5^{2}I)$ every task, and then set $\mu_1=0.1 + n_1$, $\mu_2=3.0 + n_2$, $\mu_3=5.0 + n_3$, which are reinitialized every task. Since this trick generates the data points observed from a new multi-output stationary process every task by considering the different cross correlation function between different two processes, the generated tasks are more diverse.

\end{itemize}

\subsection{Details for Tasks of Training, Validation, and Test }

In this experiment, we set the training range \textb{$[0,3]$} and test range \textb{$[3,6]$} (outside of training range). For training, we construct the context sets and target sets by sampling the data points on training range. Then, we evaluate the trained models with context sets and target sets, that are sampled on test range as described in \cref{subsubsec:prepare_sets}.

We consider the following number of data points for training, validation, and test: 
\begin{itemize}[leftmargin=1em]
    \vspace{-2mm}
    \item For training, we randomly sample \textb{$N_c \sim \mathcal{U}([5,25])$} as the number of context data points, and randomly sample \textb{$N_t \sim \mathcal{U}([N_c,50])$} as the number of target data points for each task. We use \textb{$500{\times}50{\times}16$} tasks for training through 500 batches. For validation, we set $N_c$ context data points and $N_t$ target data points as done in training, and use \textb{$64{\times}16$} tasks for validation to choose the parameters of the trained models. For test, we consider the varying \textb{$N_c \in \{5,10,15,20,25,30\}$} context data points and $N_t=50$ target data points per a task, and use \textb{$64{\times}16$} tasks per given $N_c$ context points to study how the number of context data points affects the predictive performance of the trained models using the parameters obtained in validation procedure.  
\end{itemize}

\subsection{Details for Hyperparameters.}

%\paragraph{Hyperparameters of Kernels.}

% For stationary kernels, we set $\mu_{1}=[0.0,0.0]$ and $\sigma_{1}=[0.5,0.5]$ for $Q=1$.

% For $Q=2$, we set $\mu_{1}=[0.0,0.0],\mu_{2}=[2.0,0.0],\mu_{3}=[0.0,2.0],$ and $\mu_{4}=[2.0,2.0]$ and $\sigma_{q}=[0.5,0.5]$ for $q=1,..,4$.

% For the number of spectral points, we use $l=10$ in \textb{Eq. (14)}.

% For the number of sample function, we use $N=4$ in \textb{Eq. (19)}.

% For the prior hyperparameter of approximate scheme $\alpha$, we use $\alpha \in \{.05,0.1\}$.

% For training, we  use ADAM optimizer \citeb{kingma2014adam} with learning rate $5e\text{-}4$ and weight decay $1e\text{-}4$. 

% For the regularizer hyperparameter $\beta$ in \textb{Eq. (21)}, we set $\beta=0.1$ for the proposed method.

For the hyperparameter of RBF kernels used for ConvCNP and ConvLNP, we conduct the experiment with  $l\in\{0.1,0.5,1.0\}$, and set the lengthscale $l=0.1$ for both models obtaining the best performance out of those candidates.

For the hyperparameter of GPConvCNP, we set $l=1.0$ for each channel respectively. 

For the hyperparameter of the proposed method, we use $5$ basis stationary kernels ($Q=5$), and set $\mathrm{HZ}_{\mathrm{max}}=Q$. Then, we space the frequency range $[0,\mathrm{HZ}_{\mathrm{max}}]$ linearly, and set each centered value as $\mu_q$ with $\mu_1=0 \leq ..\leq \mu_5$, and set
$\sigma_q = 0.5(\mu_{2} -\mu_{1})$ for $q=1,..,5$. For the noise parameter $\sigma^{2}_{\epsilon}$, we set $\sigma_{\epsilon}=1e\text{-}{2}$.

For the number of spectral points, we use $l=10$ in \textb{Eq. (14)}.

For the number of sample function, we use $N=10$ in \textb{Eq. (19)}.

For training, we  use ADAM optimizer \citeb{kingma2014adam} with learning rate $5e\text{-}4$ and weight decay $1e\text{-}4$. 

For the regularizer hyperparameter $\beta$ in \textb{Eq. (21)}, we set $\beta=0.1$ for the proposed method.

\subsection{Additional Results}
%We report additional results obtained in experimental section 5.2 (main). 

\paragraph{Results of Sinusoidal dataset.}

For completeness of results, we report additional prediction results of other baseline on theh tasks of Sinusoidal-all as shown in \cref{fig:nd-multitask-f,fig:nd-multitask-g}.

\vspace{-2mm}
\paragraph{Results of MOSM dataset.} We report additional results on GP-MOSM dataset. 
\cref{fig:nd2-multitask-a,fig:nd2-multitask-b} describes the mean and one-standard error of the log likelihood for 1024 tasks (beyond training range); \cref{fig:nd2-multitask-a} shows the result of the less diversity task (varying phase), and \cref{fig:nd2-multitask-b} corresponds to that of the high diversity (varying amplitude, frequency, and phase). These figures show that the proposed method could model processes well on both less and more diverse tasks. 

\cref{fig:nd2-multitask-c} shows the trained spectral density of $\{k_{q}\}_{q=1}^{5}$ on high diversity task. \cref{fig:nd2-multitask-d,fig:nd2-multitask-e} denote the parameters $\mathrm{p}_{\mathrm{nn}}(D^{c})$ for two tasks (top and bottom), and THE corresponding predictions of the proposed method.  \cref{fig:nd2-multitask-f,fig:nd2-multitask-g} show the prediction results of ConvCNP and GPConvCNP, respectively.

\begin{figure*}[t]
\centering
\subfloat[\label{fig:nd-multitask-a} Sinusoidal-phase ]
{\includegraphics[width=0.23\linewidth]{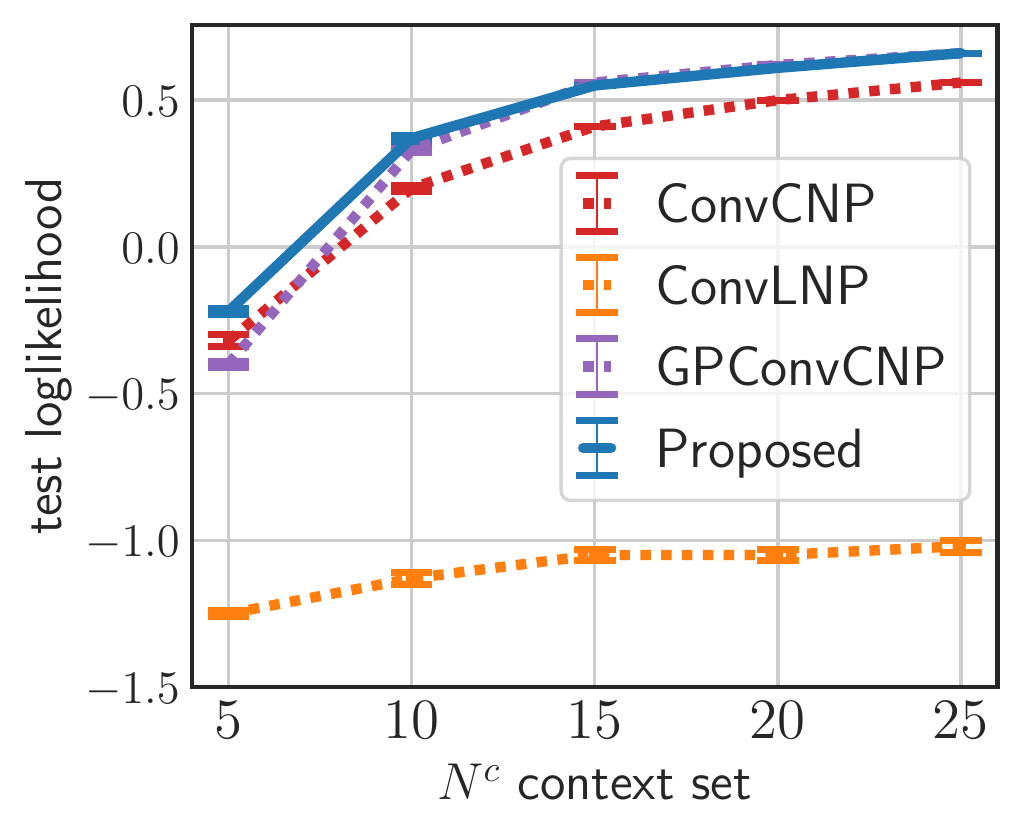}} 
\hspace{.1mm}
\subfloat[\label{fig:nd-multitask-b} Sinusoidal-all ]
{\includegraphics[width=0.23\linewidth]{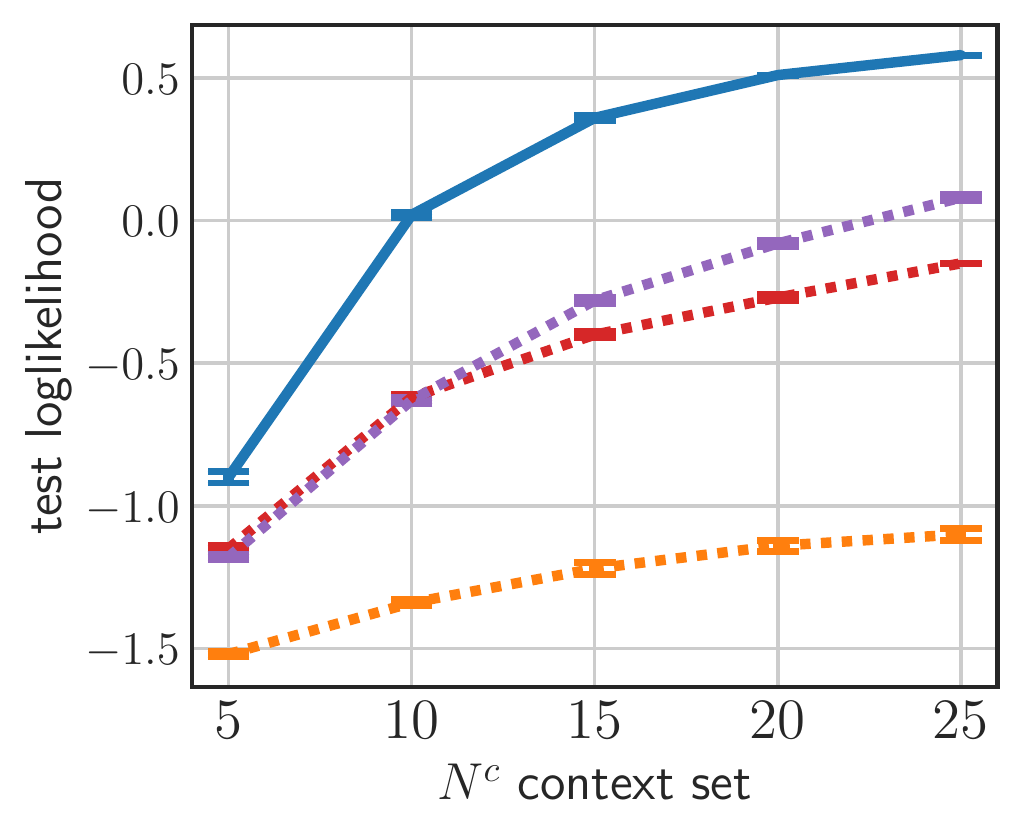}} 
\hspace{3mm}
\subfloat[\label{fig:nd-multitask-c} Spectral density]
{\includegraphics[width=0.23\linewidth]{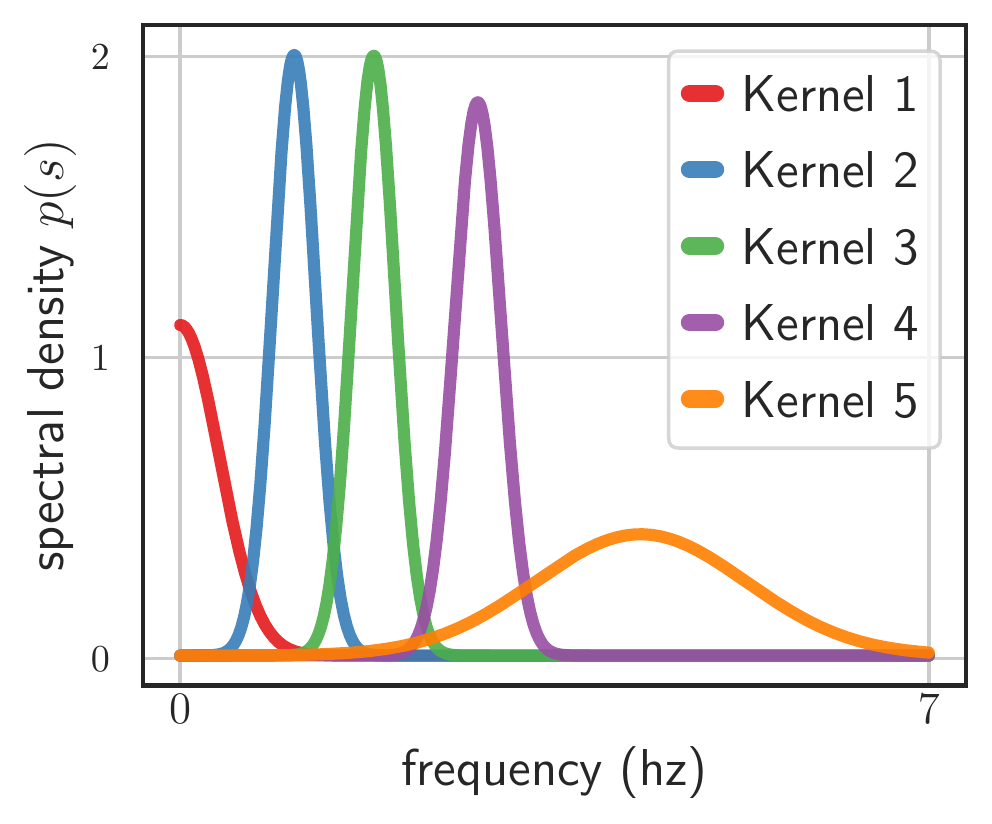}}
\hspace{.1mm}
\subfloat[\label{fig:nd-multitask-d} Task-dependent prior]
{\includegraphics[width=0.23\linewidth]{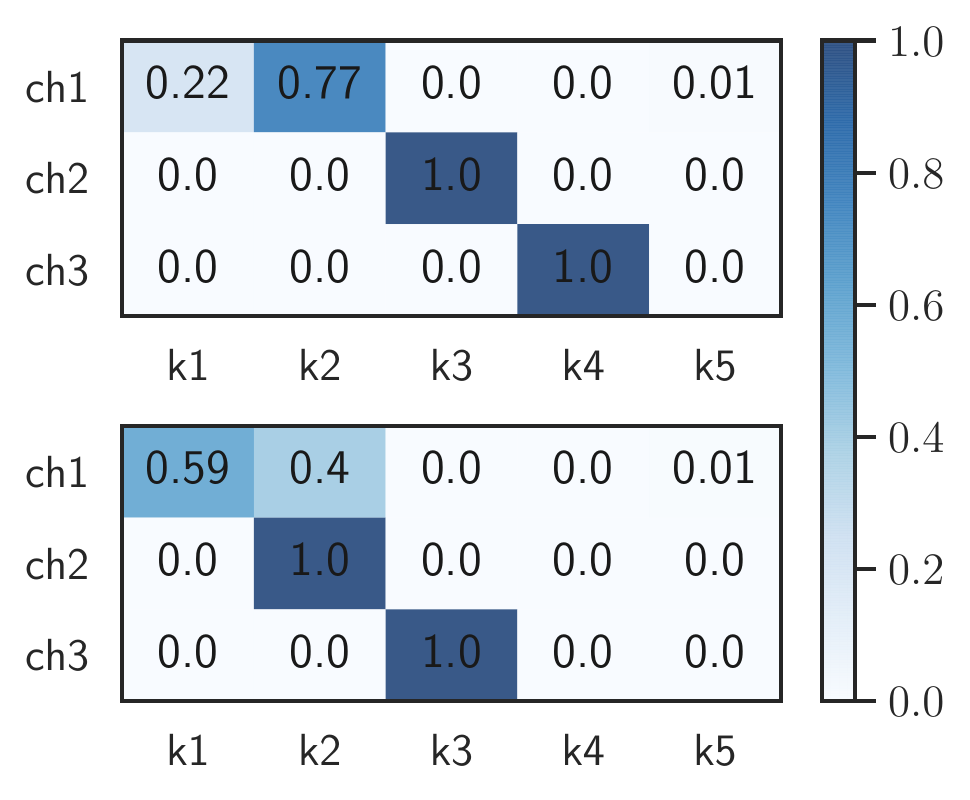}}
\vspace{4mm}
\subfloat[\label{fig:nd-multitask-e} Proposed: Prediction for 2 different tasks ($N^{c}=10$) of the Sinusoidal-all  ]
{\includegraphics[width=0.98\linewidth]{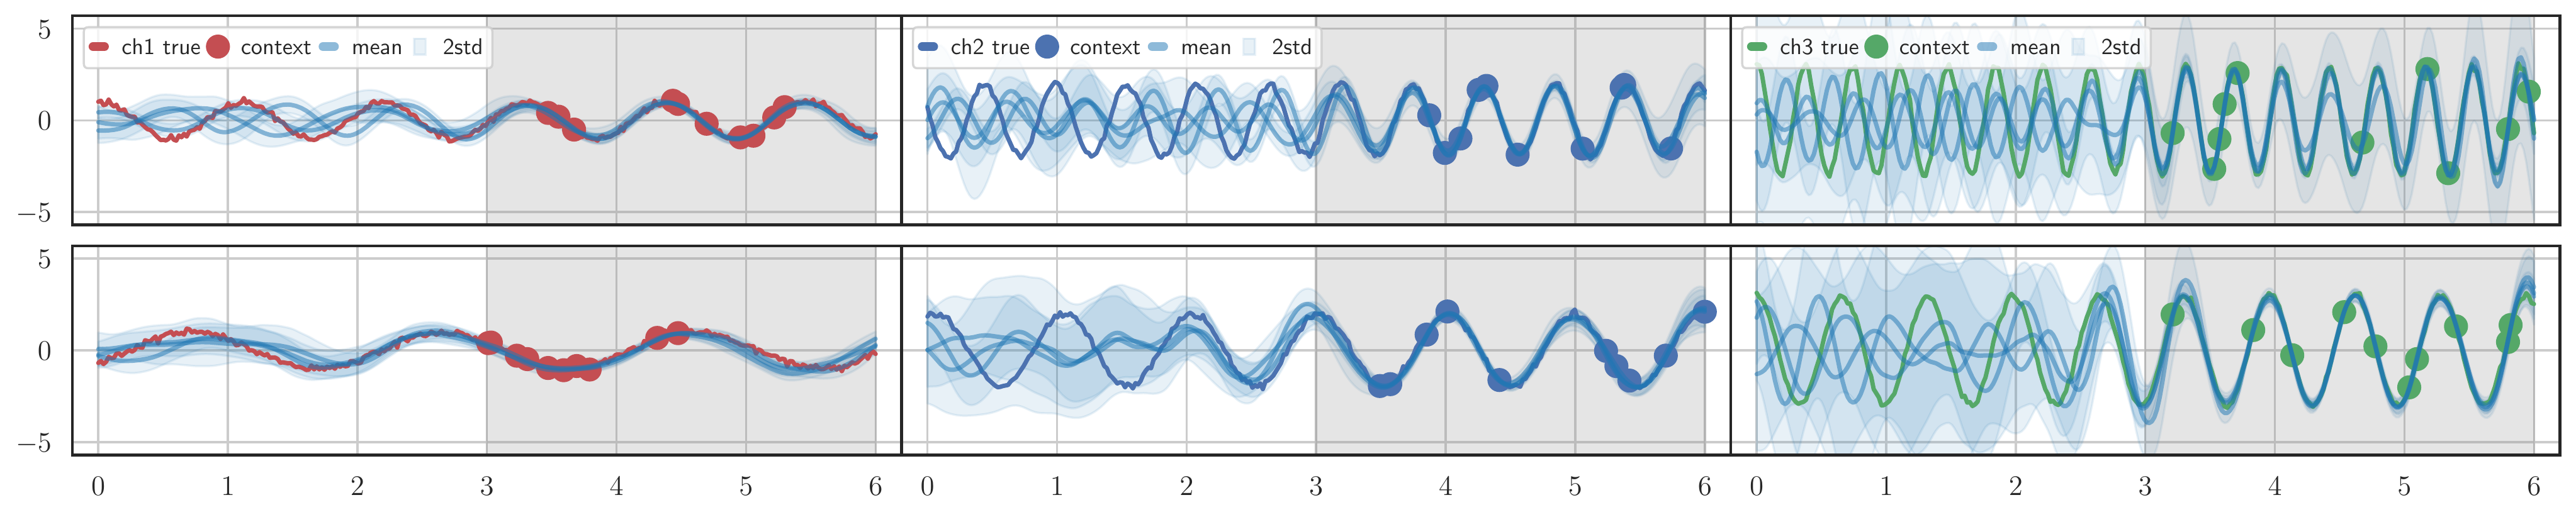}} 
\vspace{2mm}
\subfloat[\label{fig:nd-multitask-f} ConvCNP: Prediction for 2 different tasks ($N^{c}=10$) of the Sinusoidal-all  ]
{\includegraphics[width=0.98\linewidth]{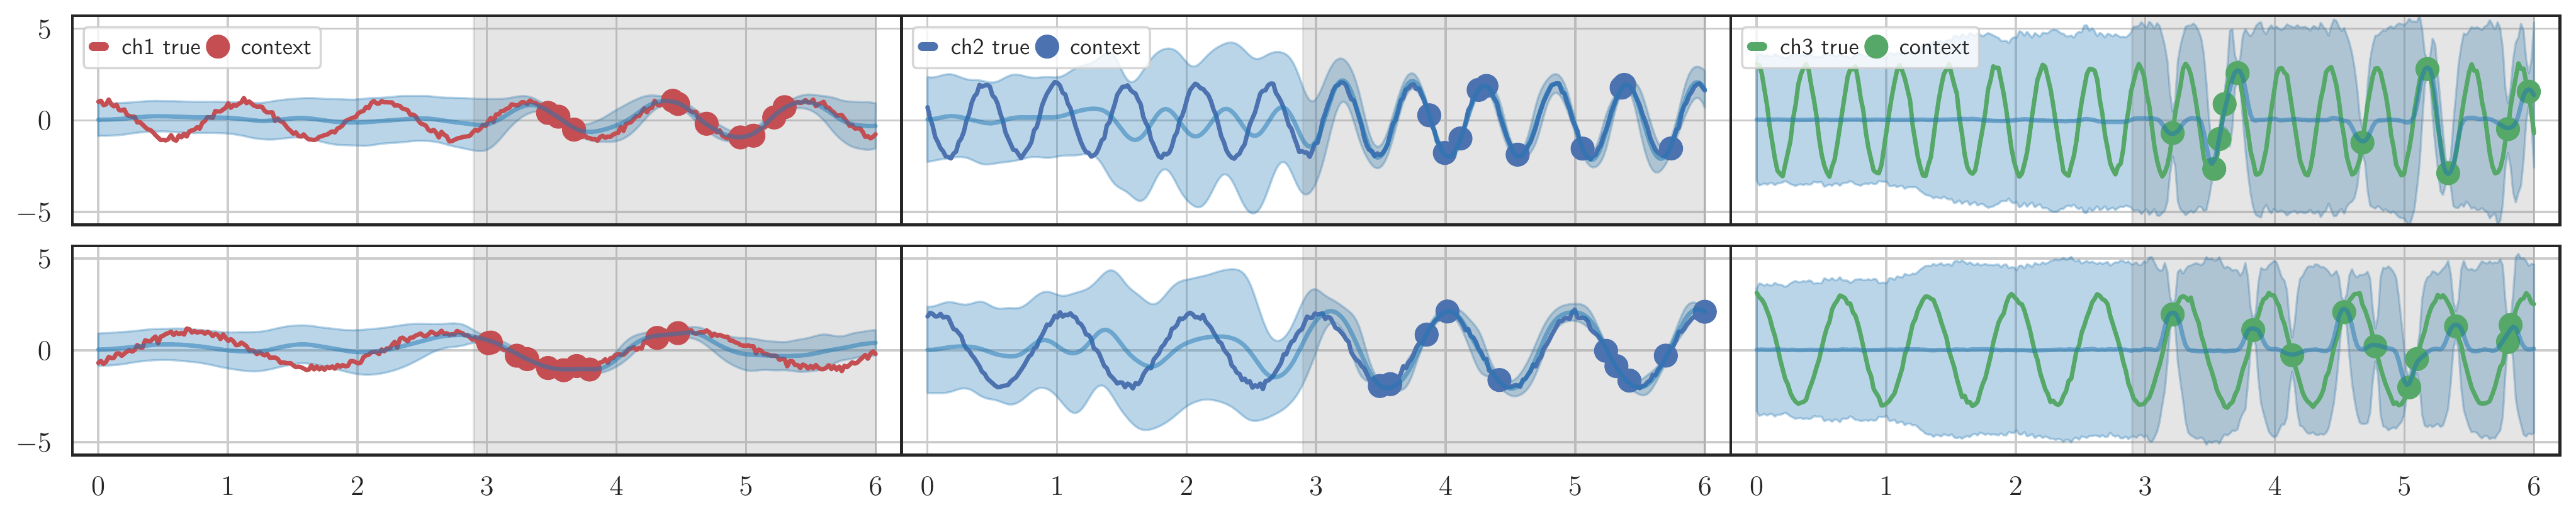}} 

\vspace{2mm}
\subfloat[\label{fig:nd-multitask-g} GPConvCNP: Prediction for 2 different tasks ($N^{c}=10$) of the Sinusoidal-all  ]
{\includegraphics[width=0.98\linewidth]{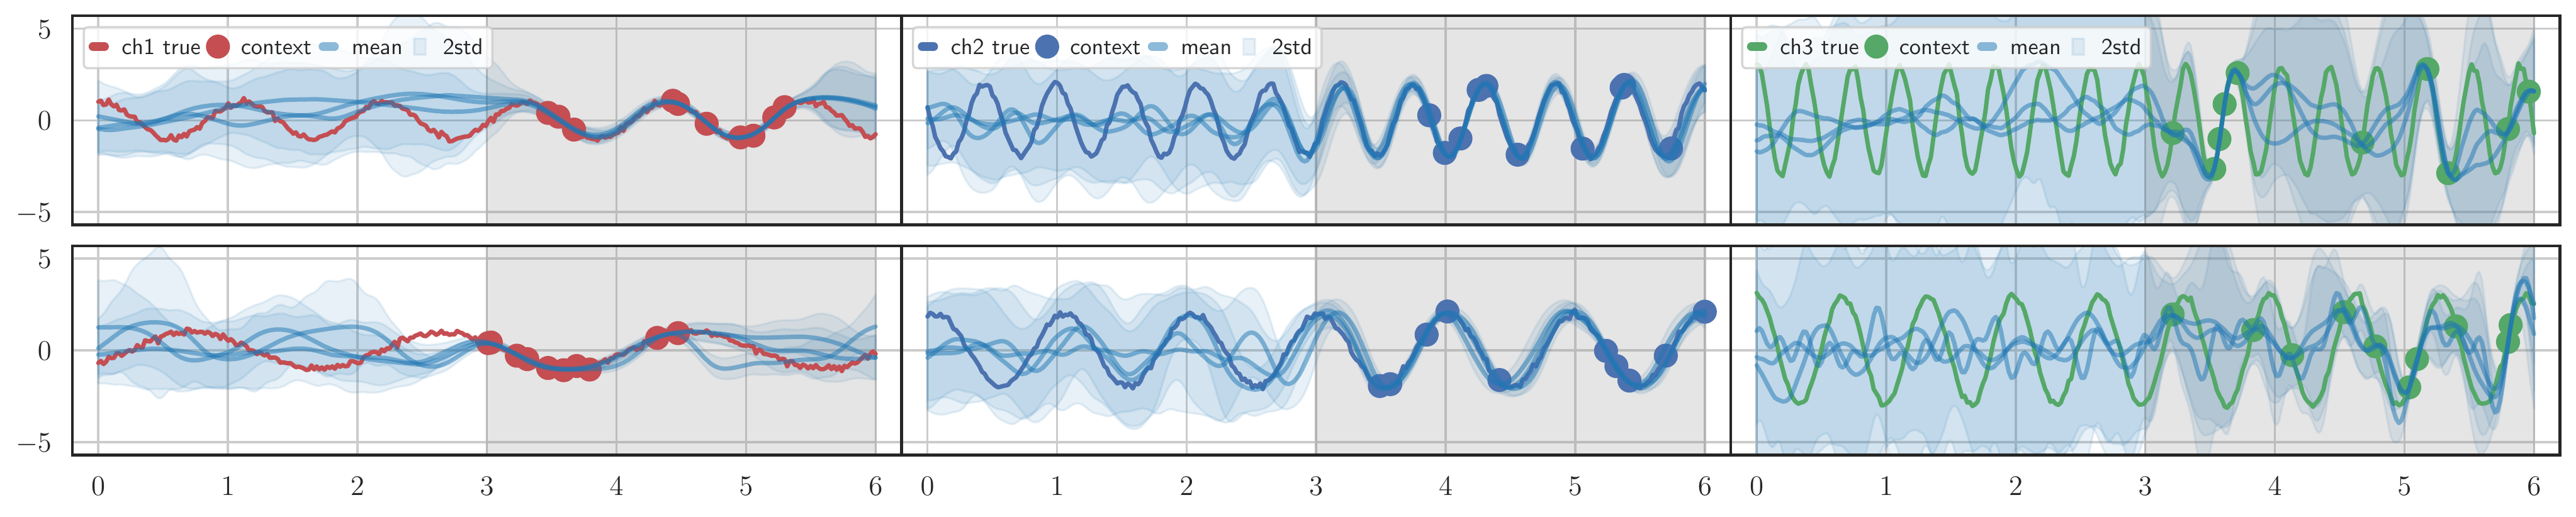}} 
\caption{3-channel sinusoidal processes modeling: \cref{fig:nd-multitask-a,fig:nd-multitask-b} denotes test likelihood on sinusoidal processes having different task diversity. \cref{fig:nd-multitask-c} denote the trained spectral density $\{p_q(s)\}_{q=1}^{5}$ for the Sinusoidal-all process, and \cref{fig:nd-multitask-d,fig:nd-multitask-e} show the chosen prior and corresponding prediction for 2 tasks; as the context sets having small frequency characteristics are given (from first to second row in \cref{fig:nd-multitask-e}), the stationary prior is imposed differently (from top to bottom in \cref{fig:nd-multitask-d}). \cref{fig:nd-multitask-f,fig:nd-multitask-g} show the prediction results using the same context set with \cref{fig:nd-multitask-e}.
}
\label{fig:nd-multitask-pred}
\end{figure*}

\begin{figure*}[t]
\centering
\subfloat[\label{fig:nd2-multitask-a} MOSM ]
{\includegraphics[width=0.23\linewidth]{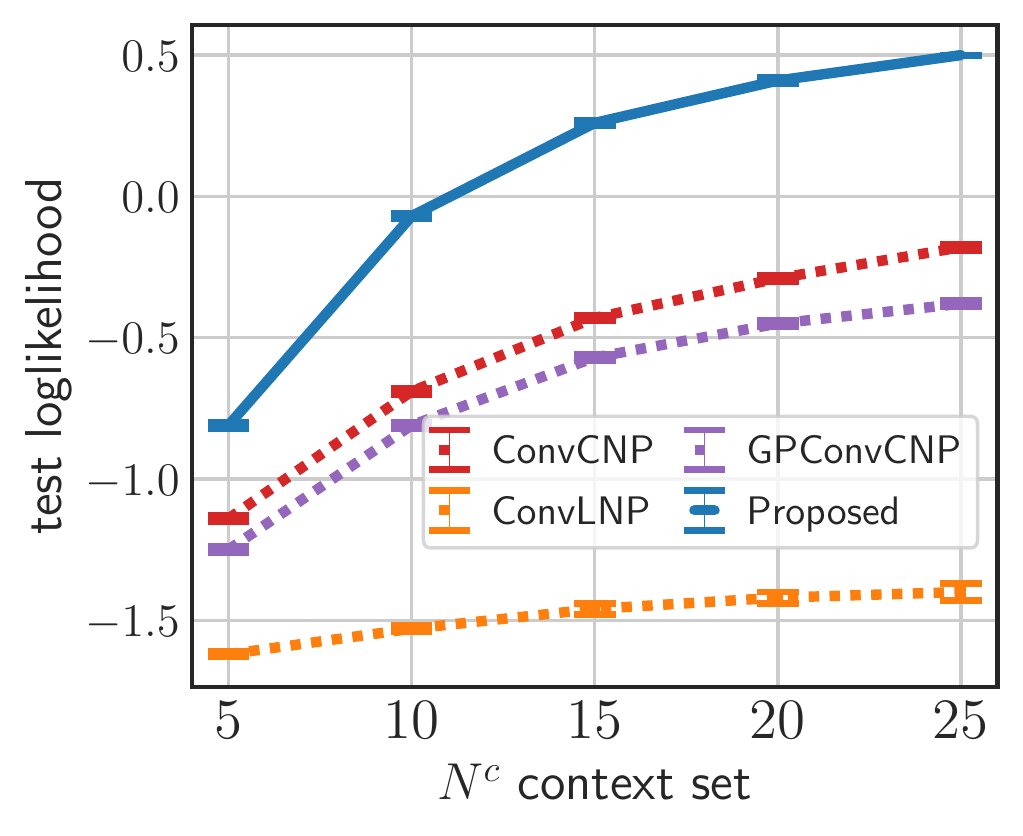}} 
\hspace{.1mm}
\subfloat[\label{fig:nd2-multitask-b} MOSM-varying ]
{\includegraphics[width=0.23\linewidth]{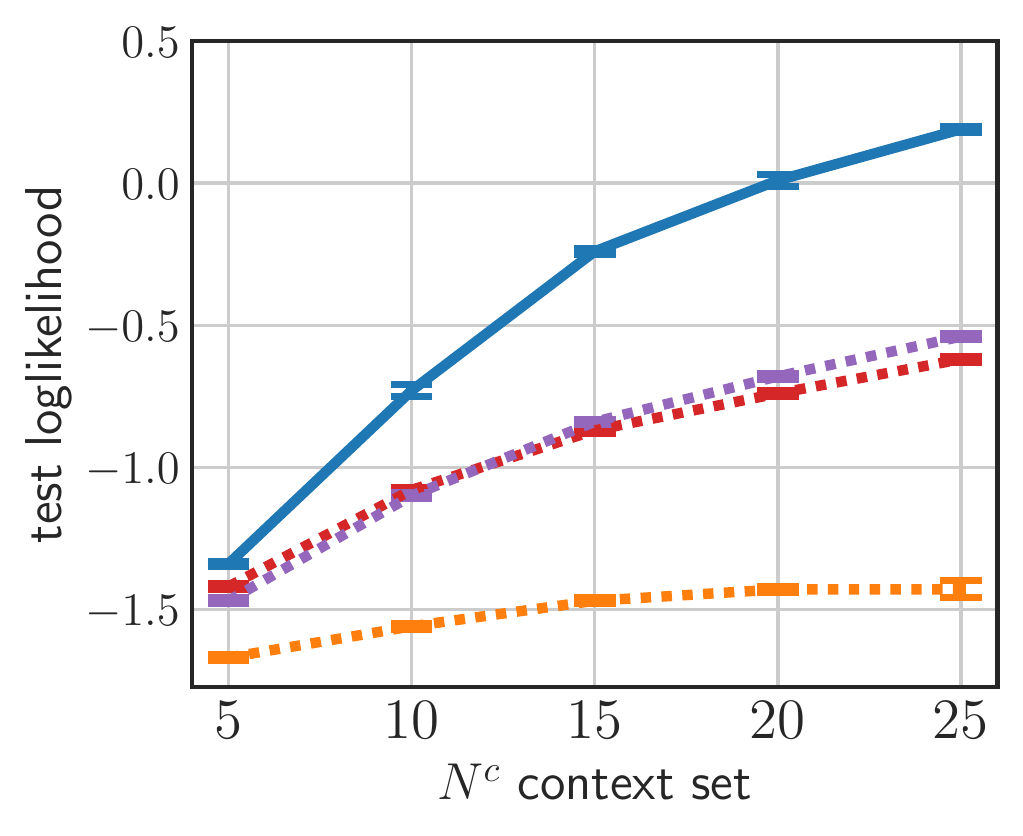}} 
\hspace{3mm}
\subfloat[\label{fig:nd2-multitask-c} Spectral density]
{\includegraphics[width=0.23\linewidth]{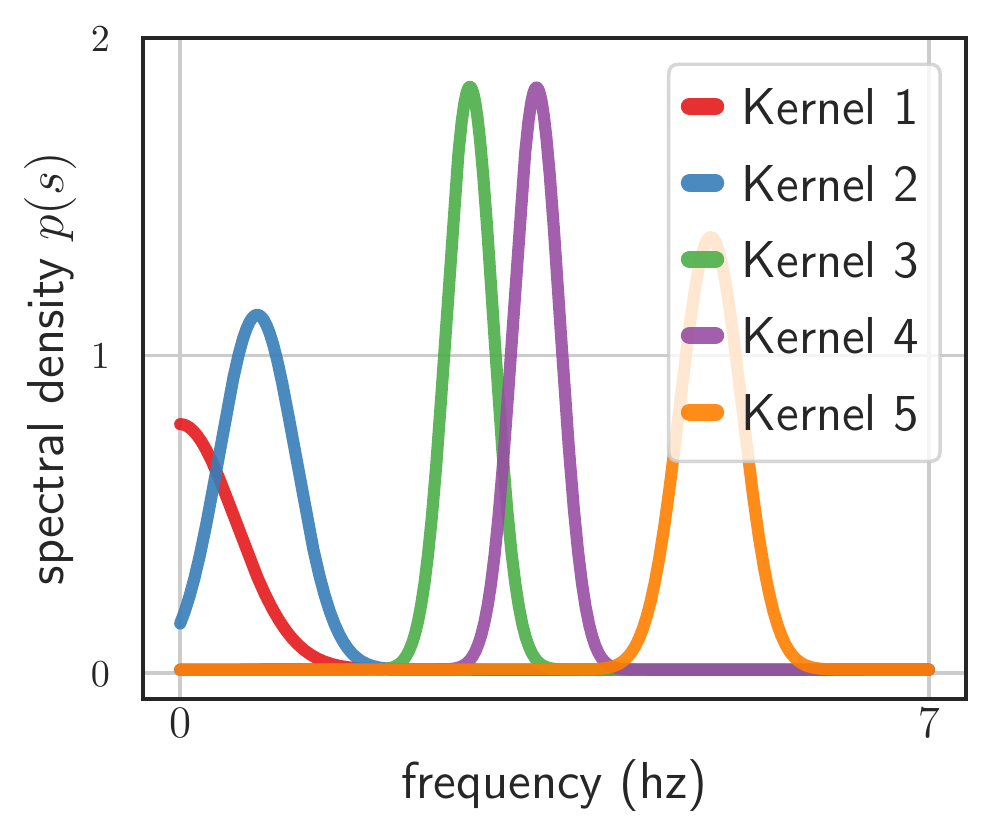}} 
\hspace{.1mm}
\subfloat[\label{fig:nd2-multitask-d} Task-dependent prior]
{\includegraphics[width=0.23\linewidth]{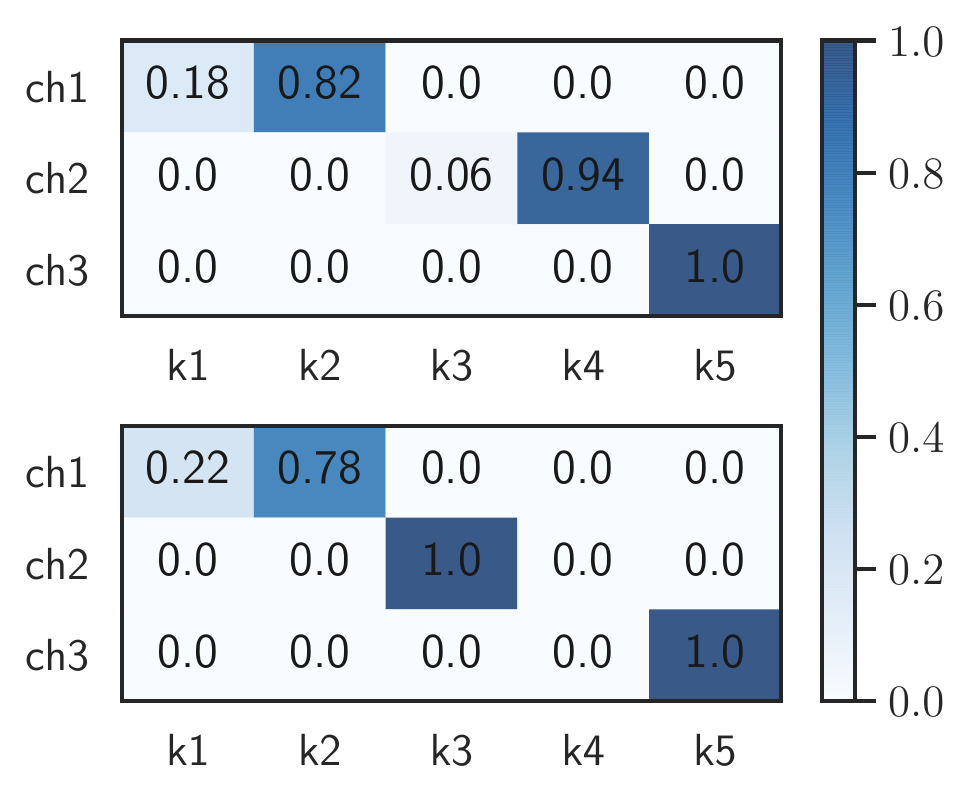}} 

\vspace{4mm}
\subfloat[\label{fig:nd2-multitask-e} Proposed: Prediction for 2 different tasks ($N^{c}=10$) of the MOSM-varying  ]
{\includegraphics[width=0.98\linewidth]{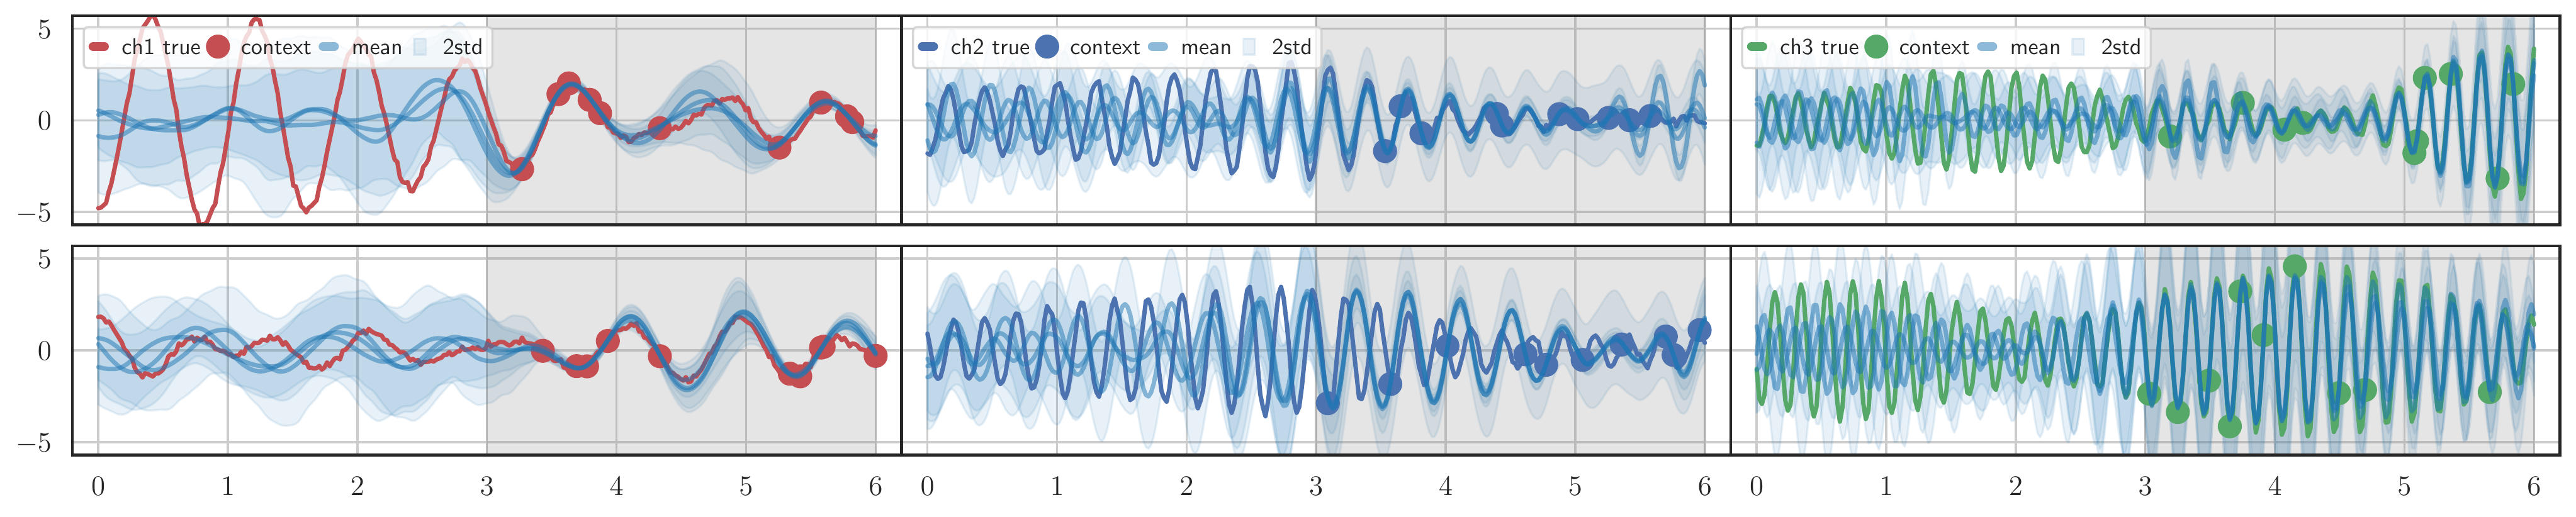}} 
\vspace{2mm}
\subfloat[\label{fig:nd2-multitask-f} ConvCNP:  Prediction for 2 different tasks ($N^{c}=10$) of the MOSM-varying  ]
{\includegraphics[width=0.98\linewidth]{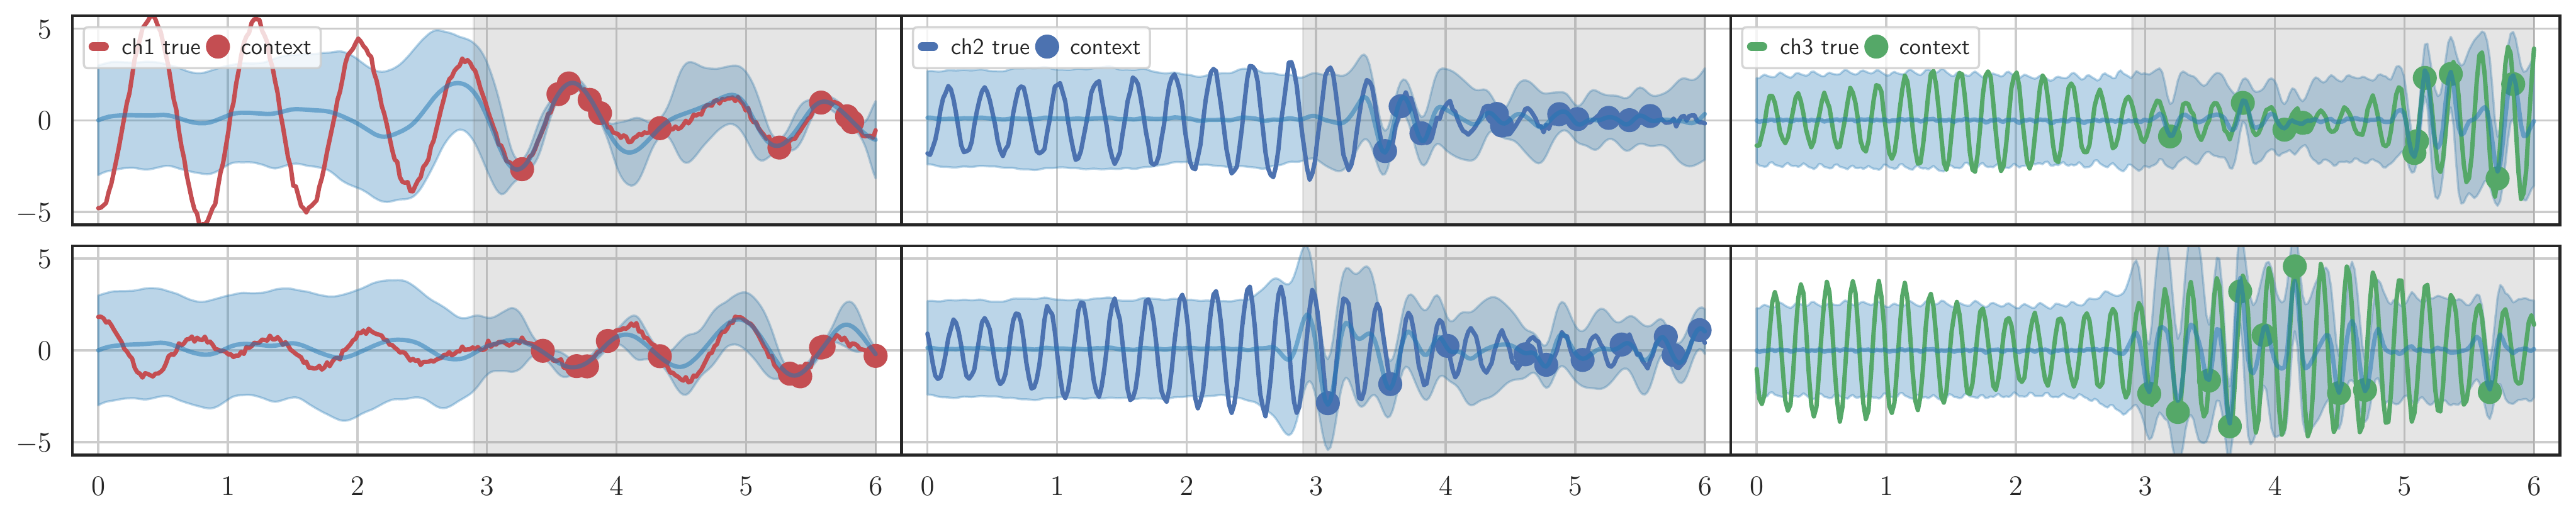}} 
\vspace{2mm}
\subfloat[\label{fig:nd2-multitask-g} GPConvCNP: Prediction for 2 different tasks ($N^{c}=10$) of the MOSM-varying  ]
{\includegraphics[width=0.98\linewidth]{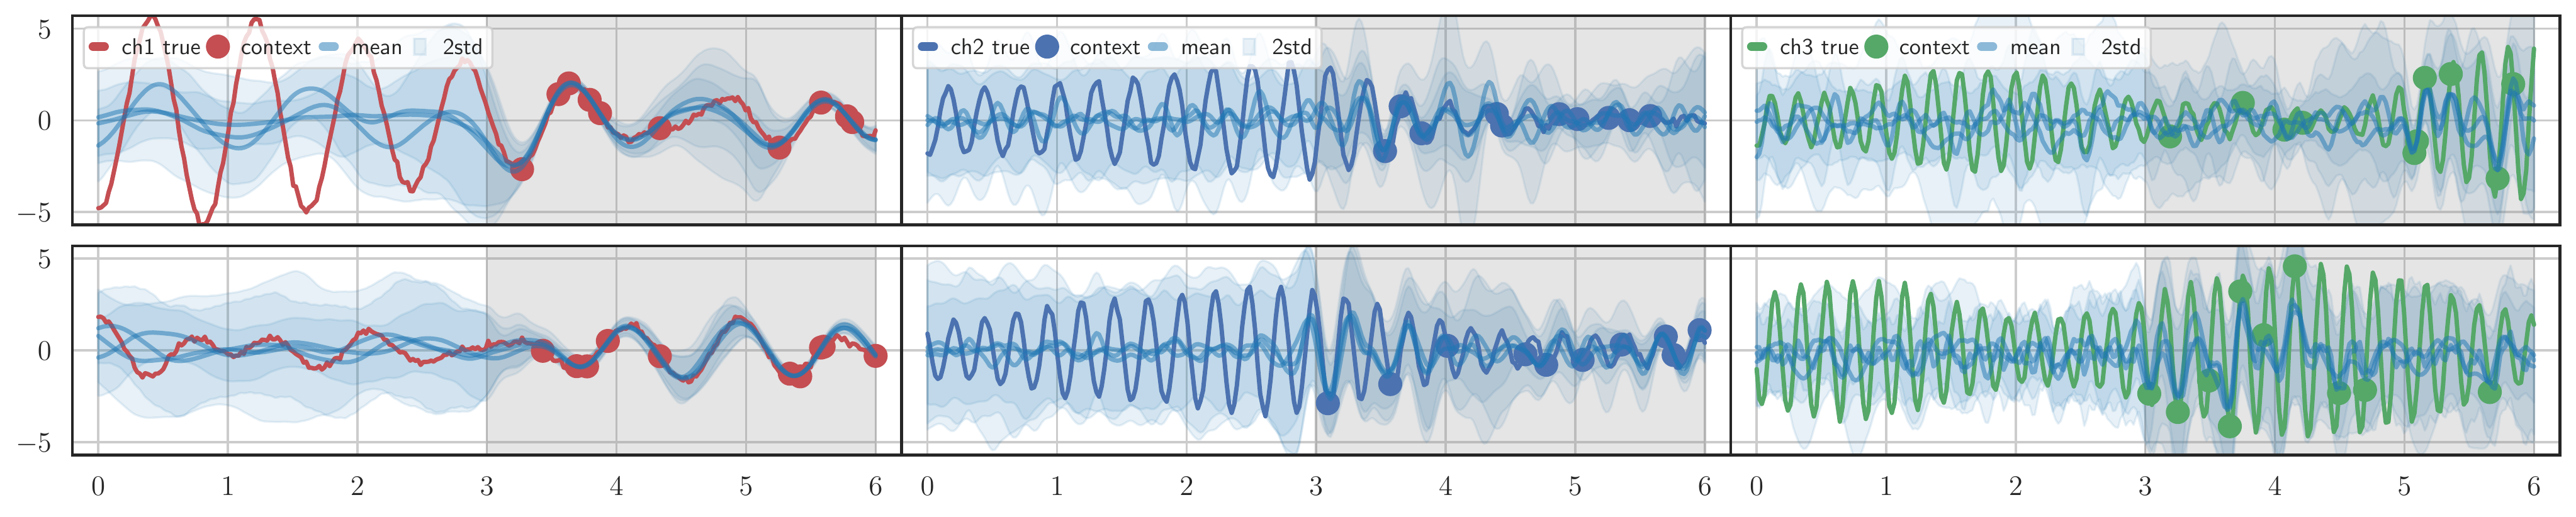}} 
\caption{3-channel GP-MOSM processes modeling: \cref{fig:nd2-multitask-a,fig:nd2-multitask-b} denotes test likelihood having different task diversity. \cref{fig:nd2-multitask-c} denote the trained spectral density for the MOSM-varying process, and \cref{fig:nd2-multitask-d,fig:nd2-multitask-e} show the chosen prior and corresponding prediction for 2 tasks; check that the stationary prior is imposed differently (from top to bottom in \cref{fig:nd2-multitask-d}), when context are given differently (from first to second row in \cref{fig:nd2-multitask-e}). \cref{fig:nd2-multitask-f,fig:nd2-multitask-g} show the prediction results using the same context set with \cref{fig:nd2-multitask-e}.
}
\label{fig:nd-multitask-pred}
\end{figure*}
