# Supplementary material for: Bayesian Convolutional Deep Sets with Task-Dependent Stationary Prior
Source: arXiv:2210.12363 source file (2022-10-22)
Supplement: Supplementary file 14 [file 07-appendix-v01-chapter4-exp3-figure01.tex]

\vspace{-5mm}
\begin{figure*}[htp!]

% \subfloat[\label{fig:fig-h} \textb{mosm-varying}: $p_{\text{traninv-nn}}(X_c,Y_c)$ ]   
% {\includegraphics[width=0.41\linewidth,height=4.85cm]{Figures/07-appendix-exp2/mosm-varying/mosmvarying_datav11_deptrue_gpdep_weight.pdf}} 
\centering
\subfloat[ \label{fig:pray-10a} ConvCNP with Task1 ($N^c=10$)]{
 \includegraphics[width=0.49\linewidth]{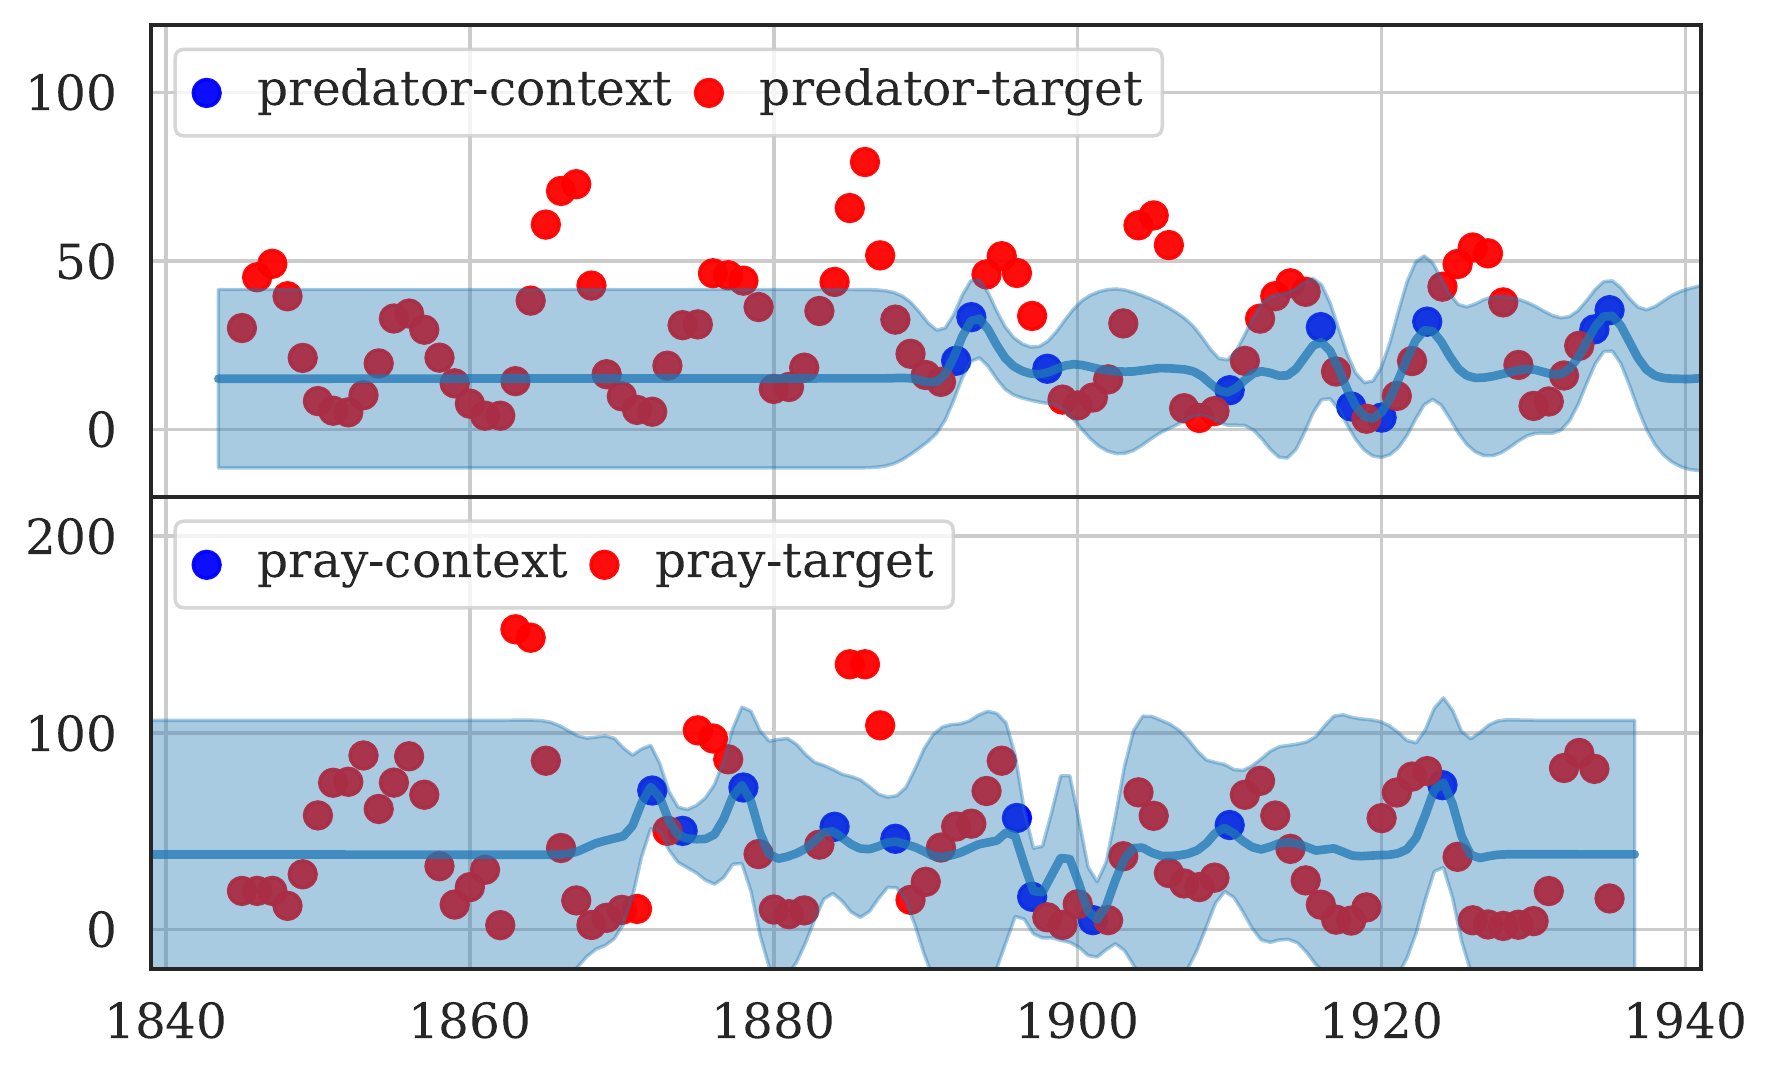}}
\subfloat[ \label{fig:pray-10b} ConvCNP with Task2 ($N^c=10$)]{\includegraphics[width=0.49\linewidth]{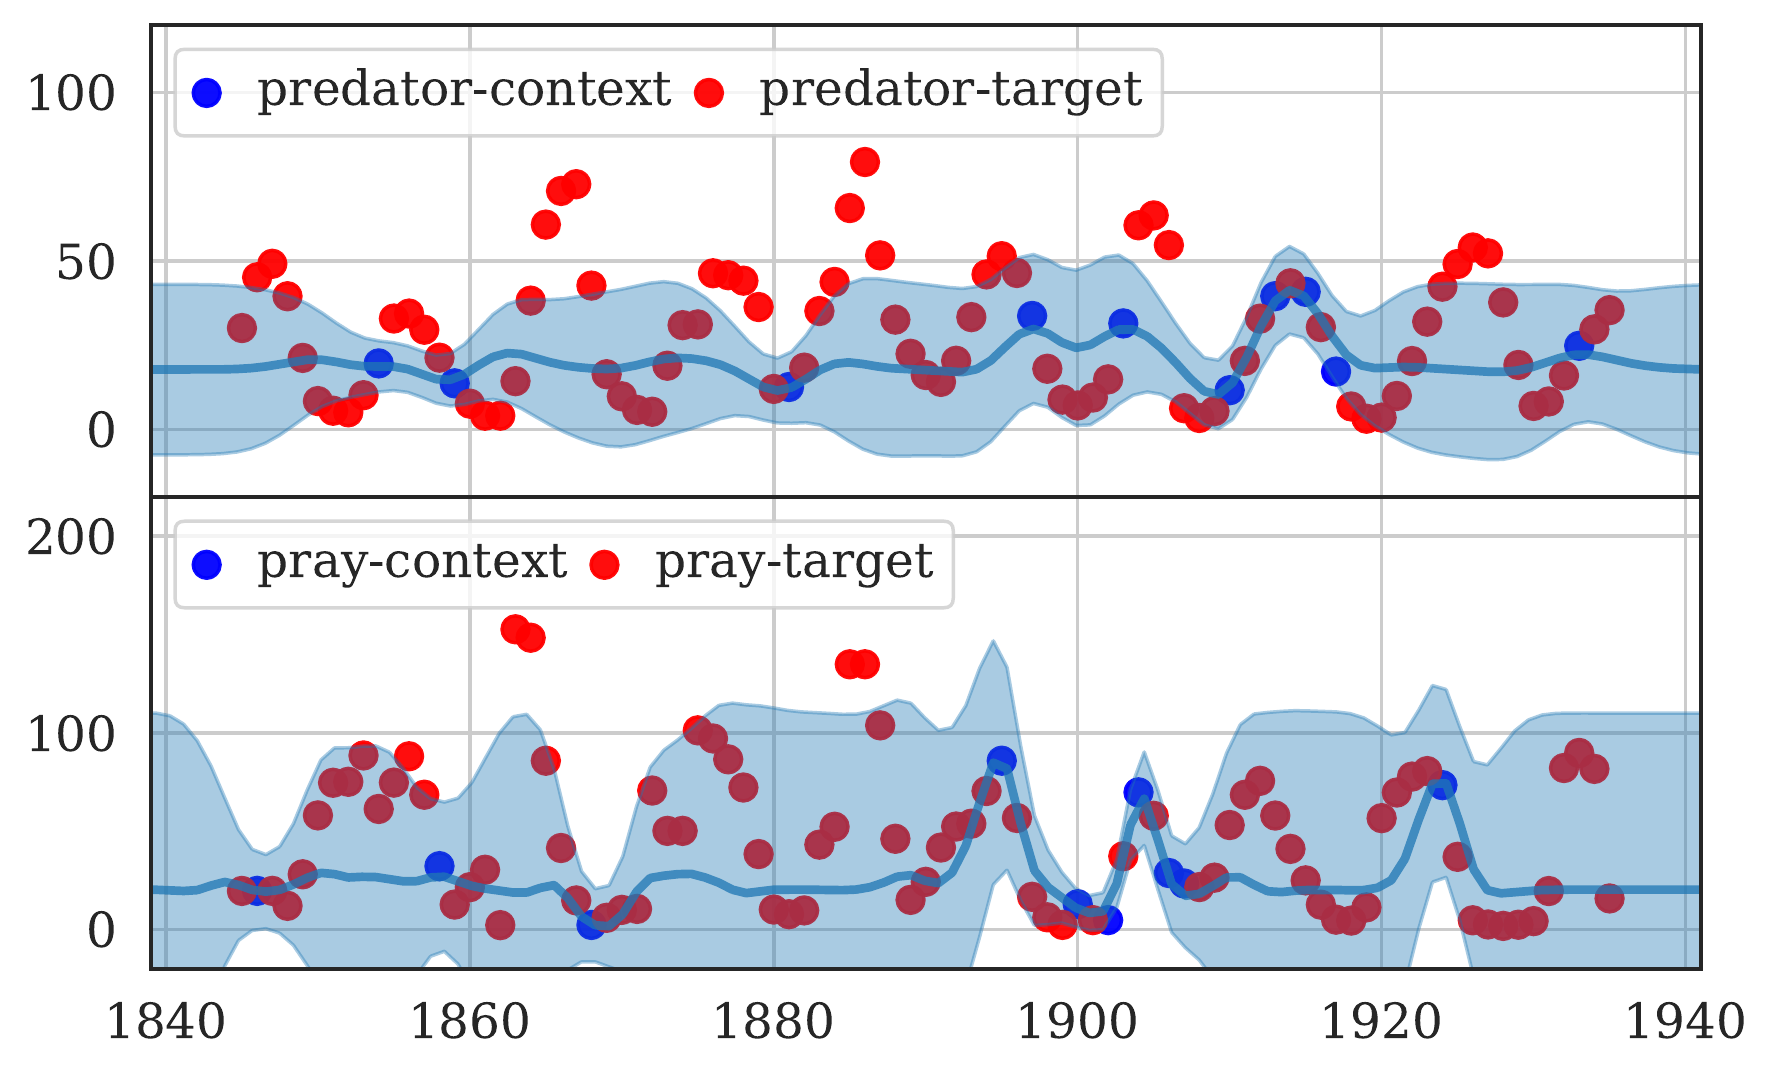}}

 \vspace{4mm}
\subfloat[ \label{fig:pray-10c} GPConvCNP with Task1 ($N^c=10$)]{
 \includegraphics[width=0.49\linewidth]{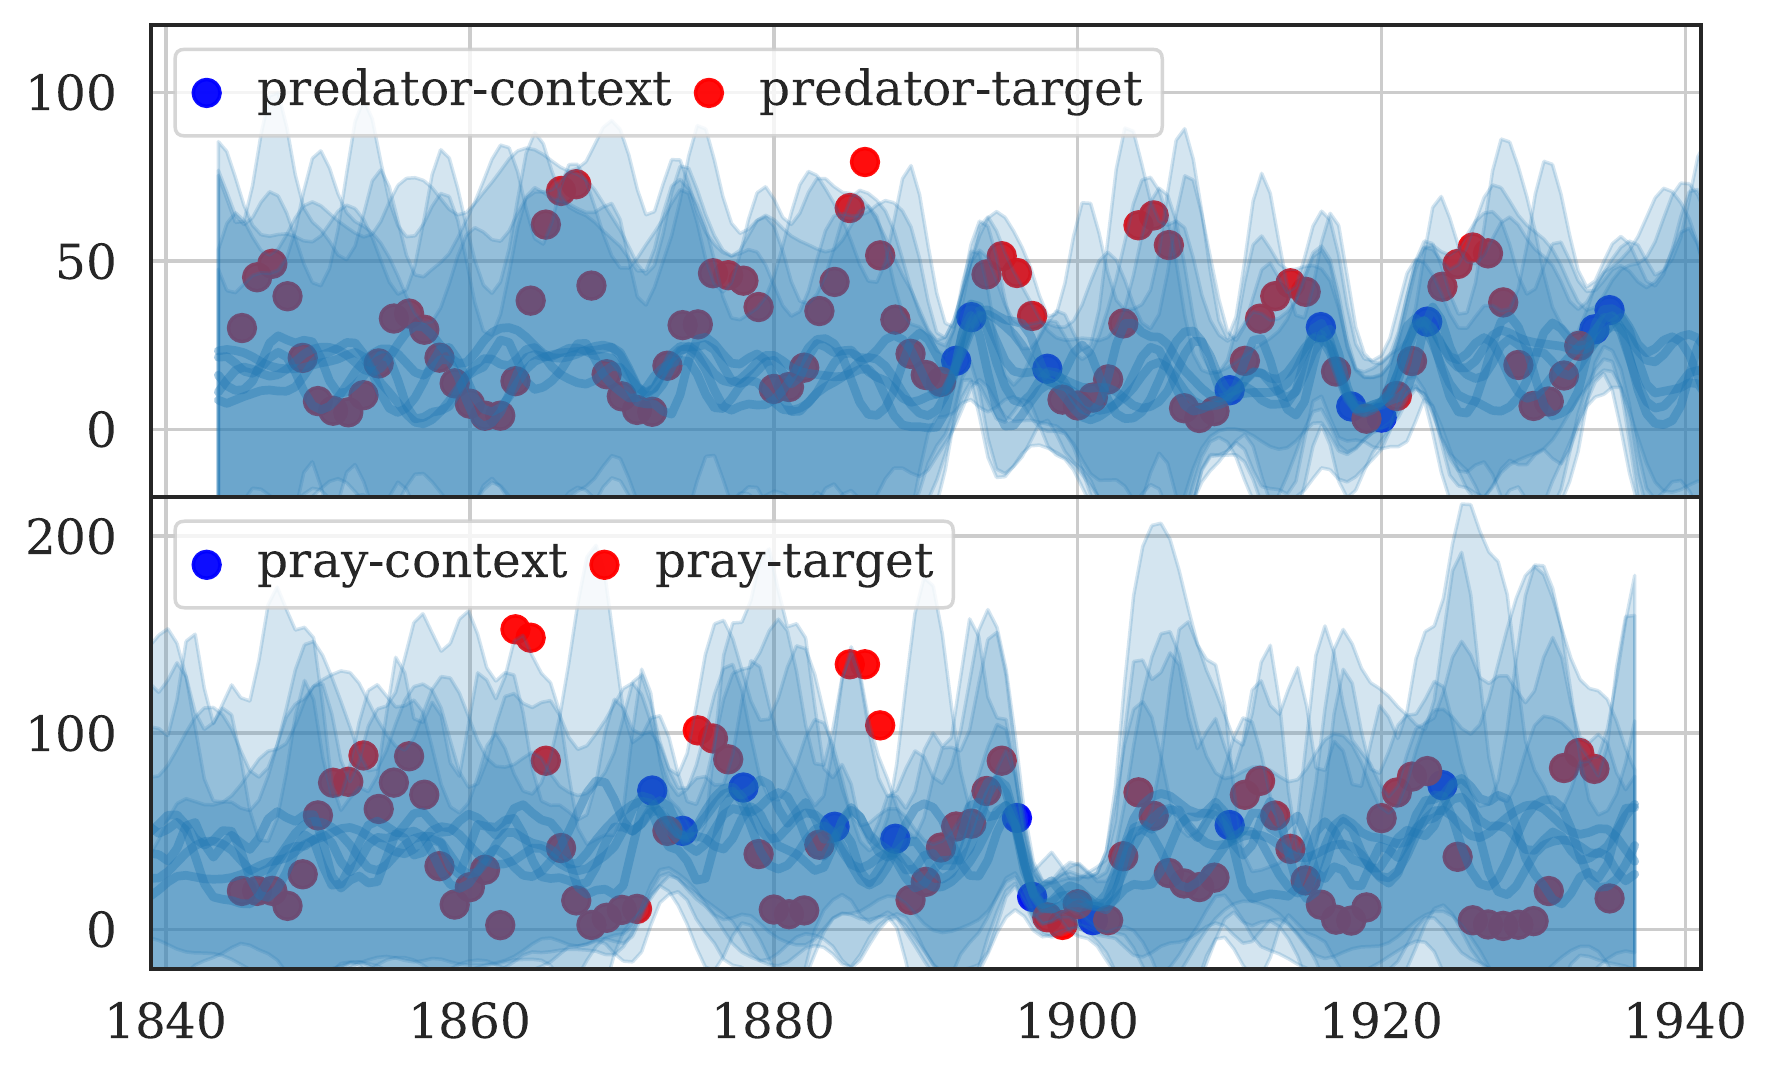}}
\subfloat[\label{fig:pray-10d} GPConvCNP with Task2 ($N^c=10$)]{
 \includegraphics[width=0.49\linewidth]{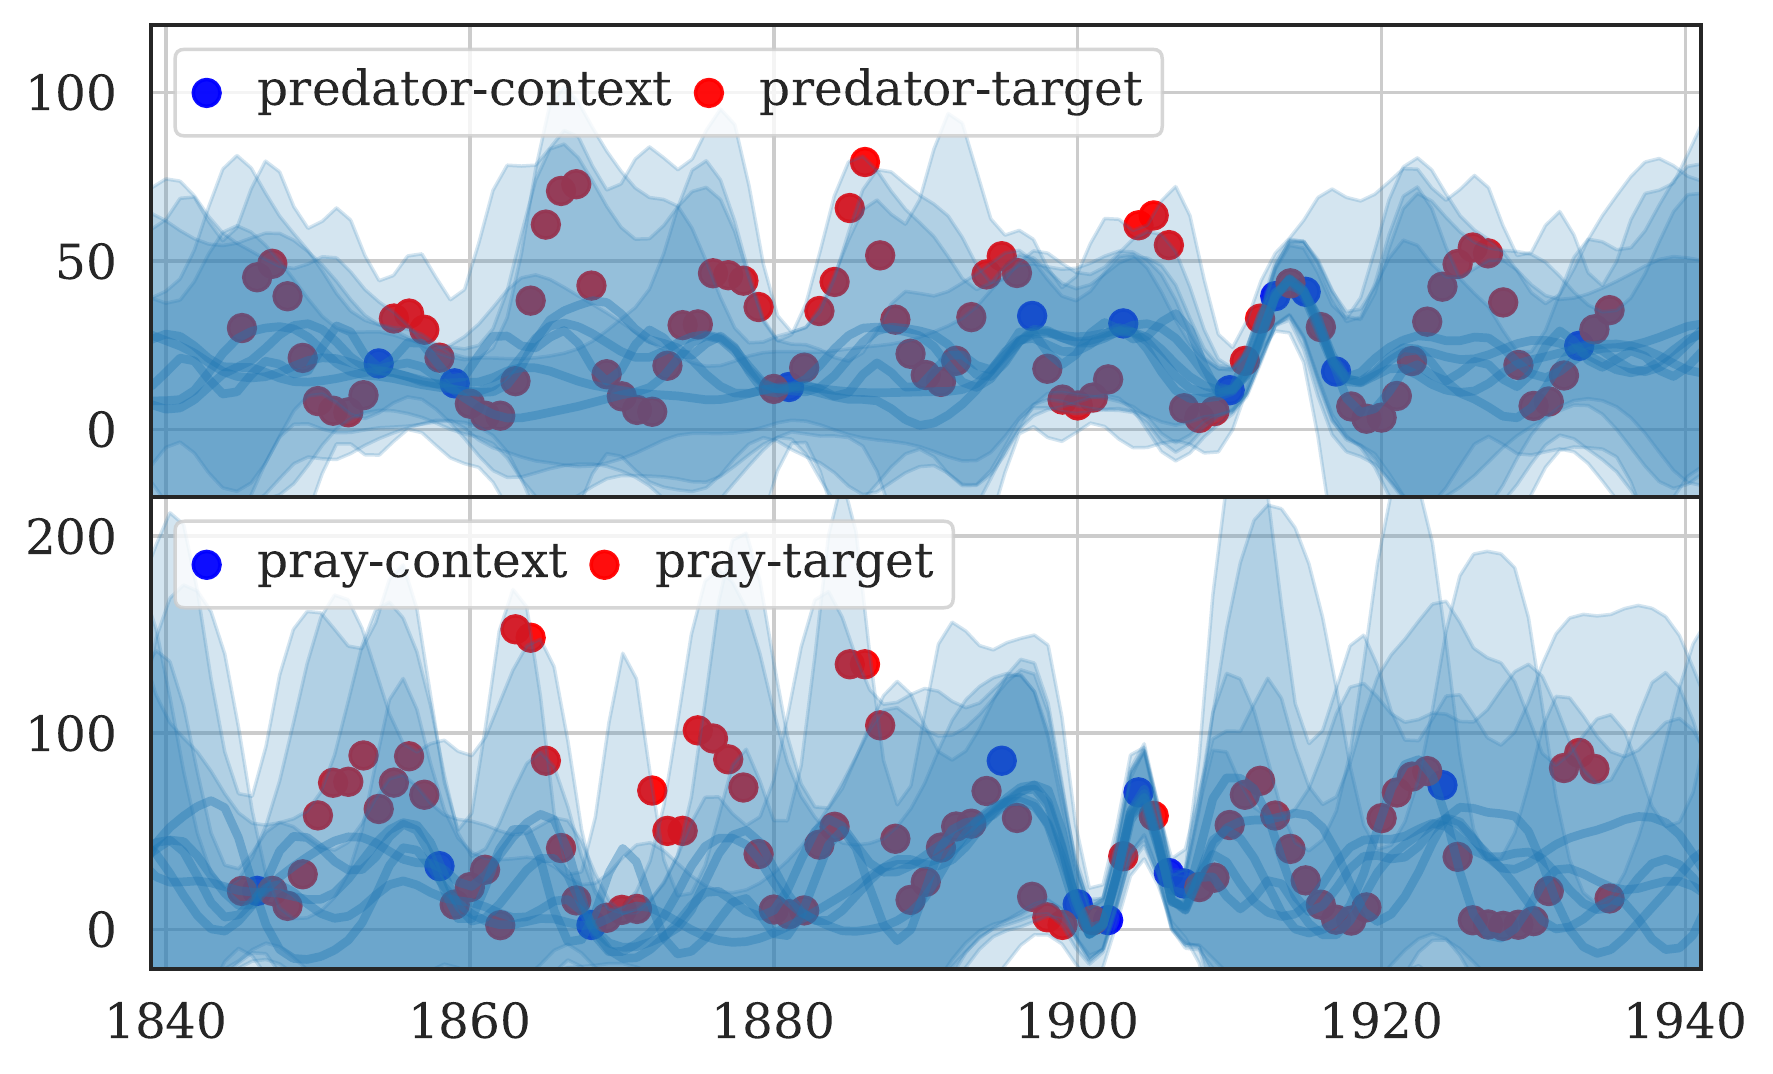}}
 
 \vspace{4mm}
\subfloat[\label{fig:pray-10e} Proposed Model with Task1 ($N^c=10$)]{
 \includegraphics[width=0.49\linewidth]{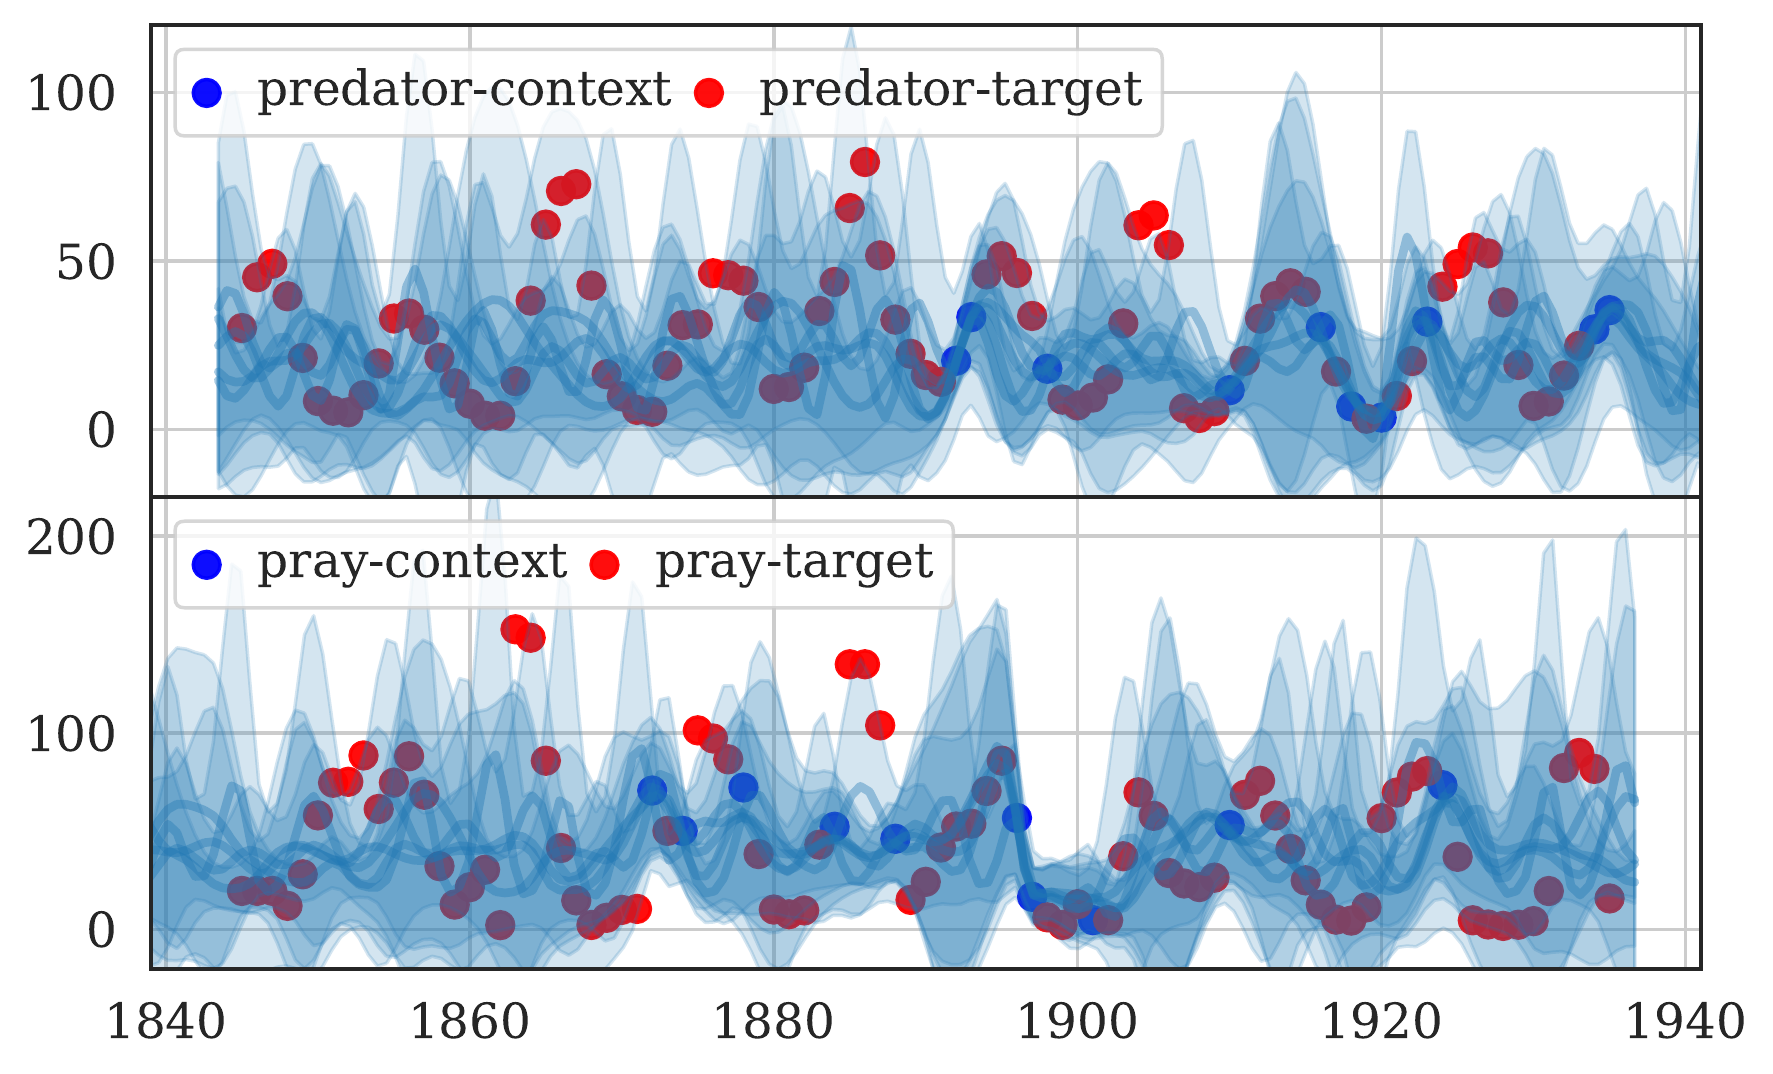}}
\subfloat[\label{fig:pray-10f}Proposed Model with Task2 ($N^c=10$)]{
 \includegraphics[width=0.49\linewidth]{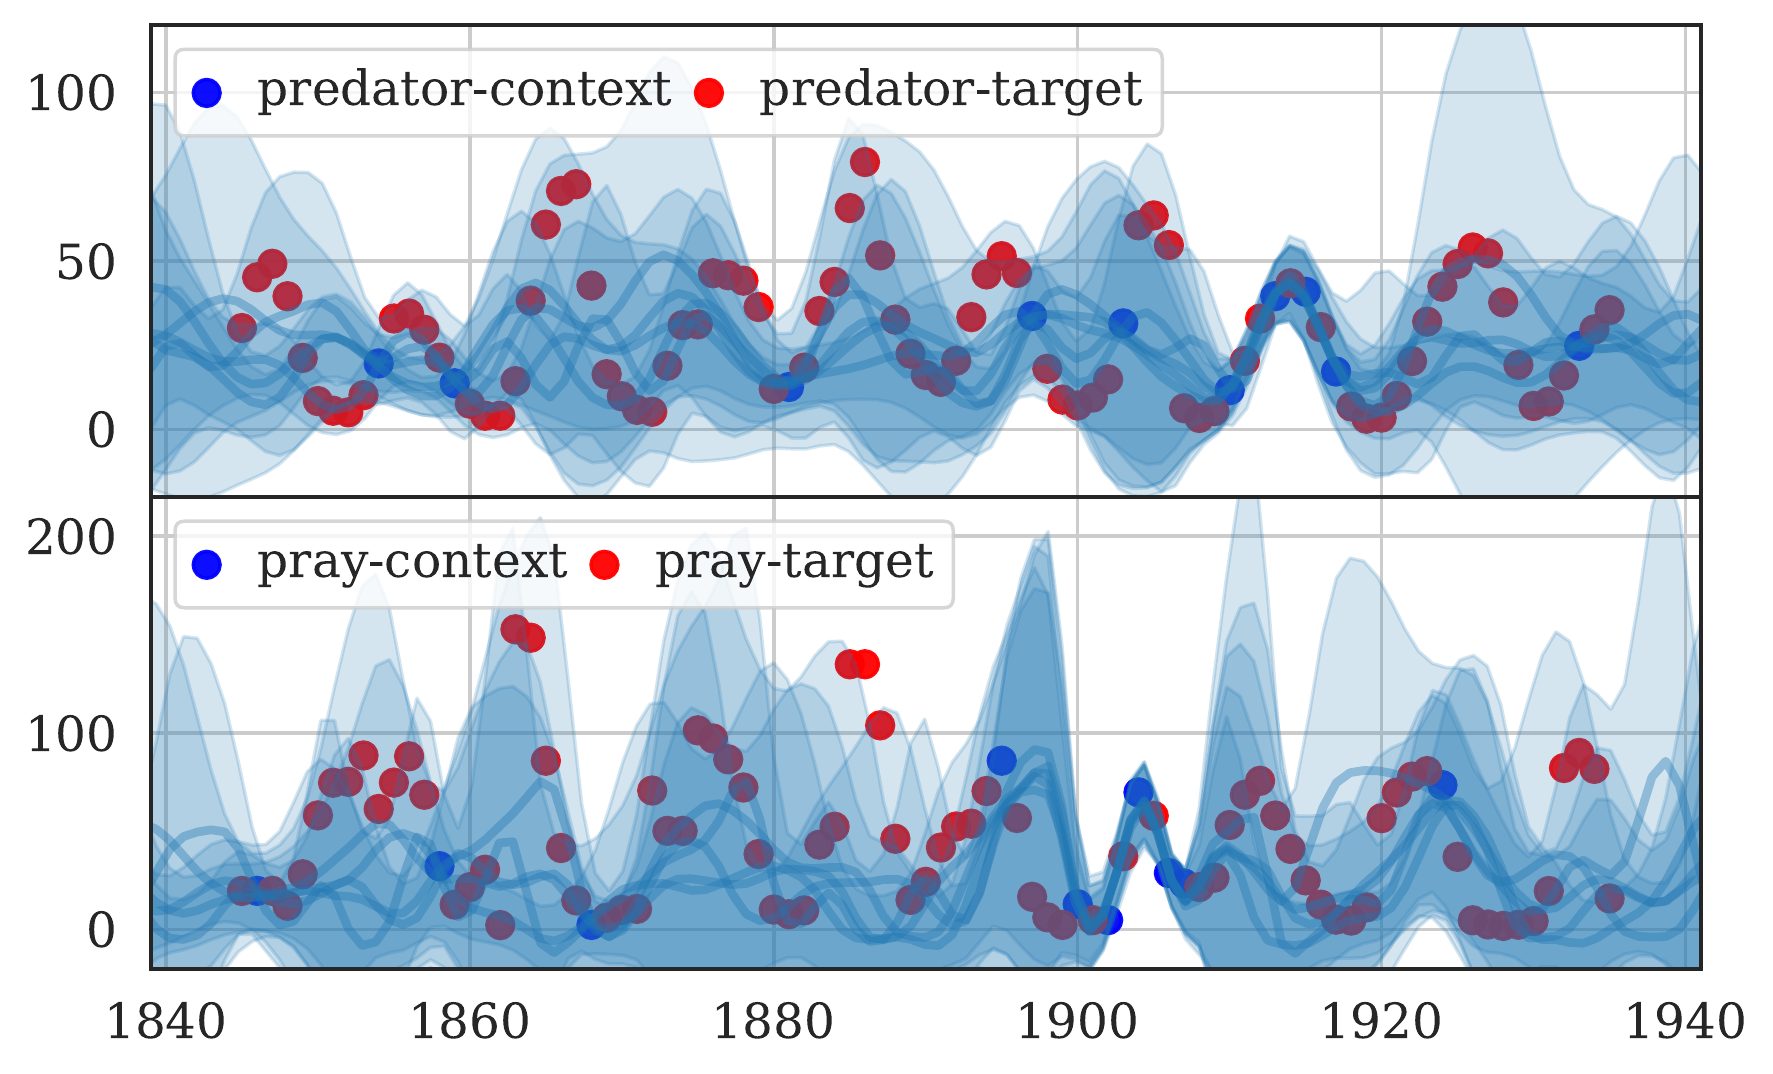}}

\caption{ Prediction results of \textb{Predator-Pray model with 10 context data points ($N^{c}=10$)}; \cref{fig:pray-10a,fig:pray-10b} shows the prediction results of 2 different tasks, respectively. \cref{fig:pray-10c,fig:pray-10d} correspond to the prediction results of GPConvCNP using 5 random functional representations. \cref{fig:pray-10e,fig:pray-10f} correspond to the prediction results of the proposed model using 5 random functional representations. These figures imply that how the random functional representations using prior affect the prediction on target sets when the small number of context data points is given}
\label{fig:predator-pray-10}
\end{figure*}
