# Supplementary material for: Bayesian Convolutional Deep Sets with Task-Dependent Stationary Prior
Source: arXiv:2210.12363 source file (2022-10-22)
Supplement: Supplementary file 15 [file 07-appendix-v01-chapter4-exp3-figure02.tex]

\vspace{-5mm}
\begin{figure*}[htp!]

% \subfloat[\label{fig:fig-h} \textb{mosm-varying}: $p_{\text{traninv-nn}}(X_c,Y_c)$ ]   
% {\includegraphics[width=0.41\linewidth,height=4.85cm]{Figures/07-appendix-exp2/mosm-varying/mosmvarying_datav11_deptrue_gpdep_weight.pdf}} 
\centering
\subfloat[\label{fig:pray-40a}ConvCNP with Task1 ($N^c=40$)]{
 \includegraphics[width=0.49\linewidth]{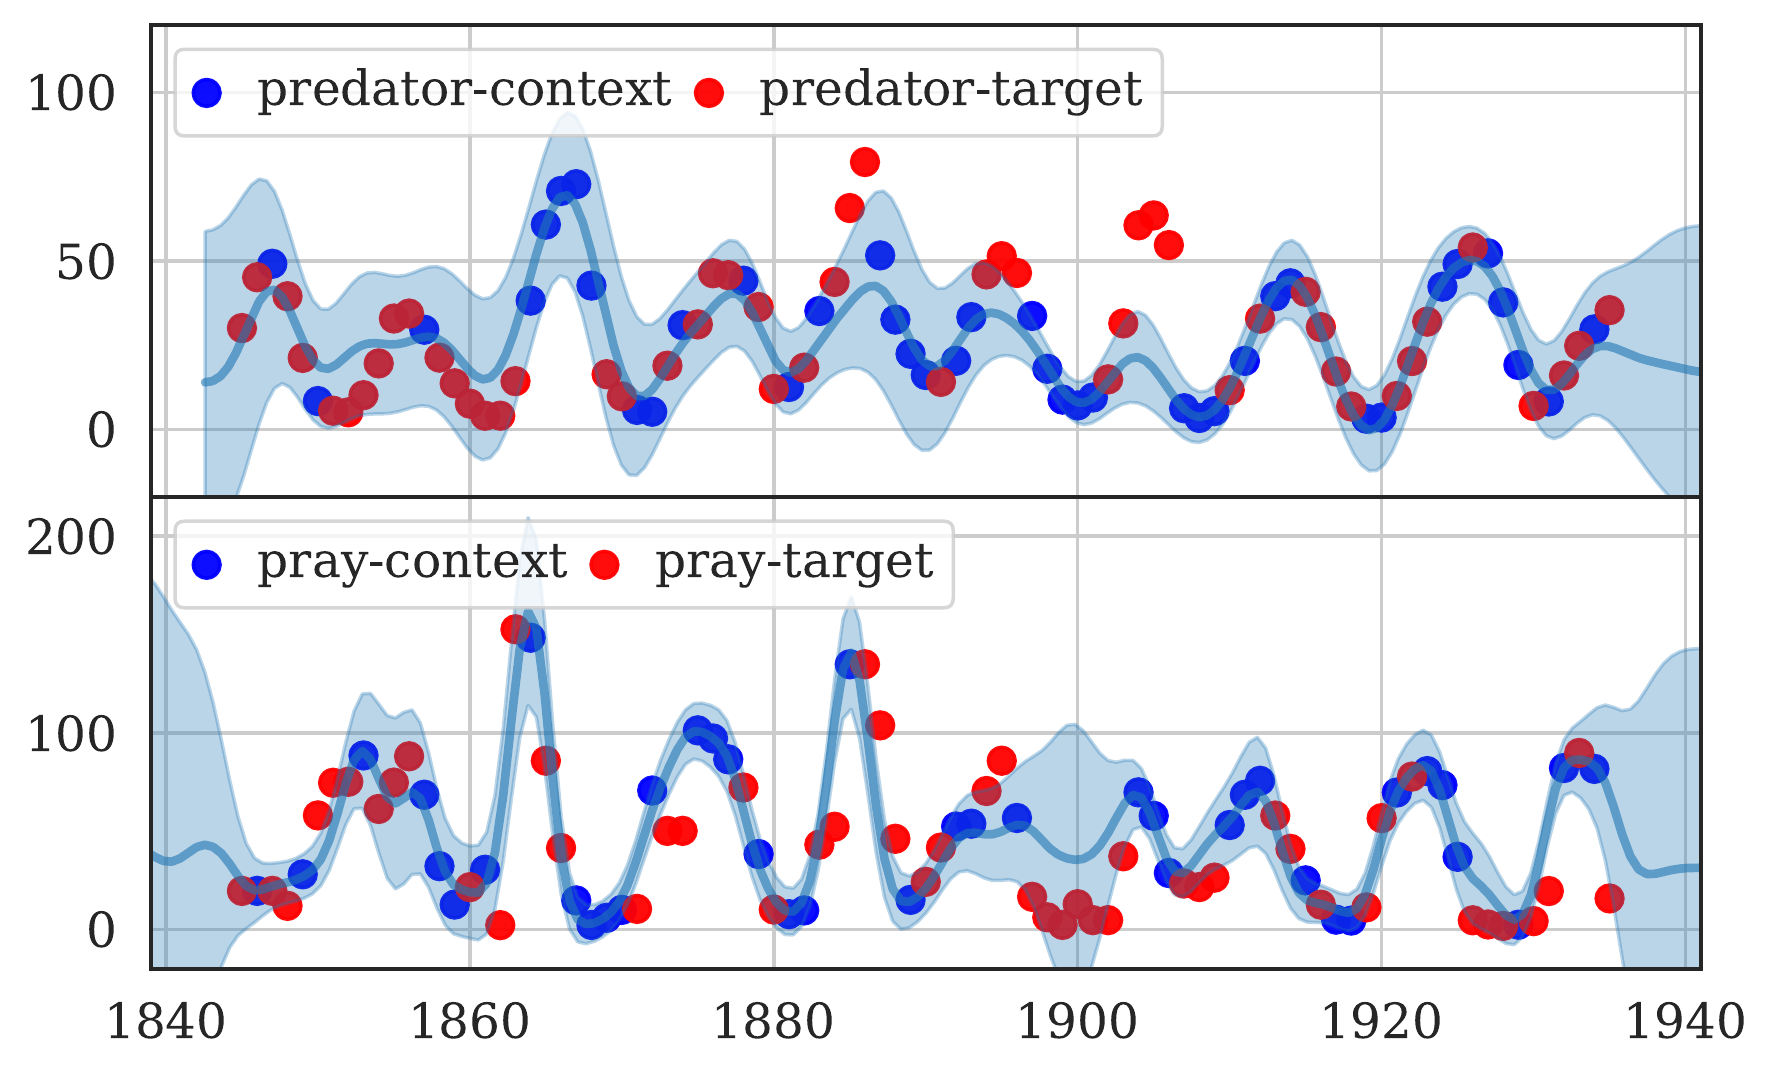}}
\subfloat[\label{fig:pray-40b}ConvCNP with Task2 ($N^c=40$)]{\includegraphics[width=0.49\linewidth]{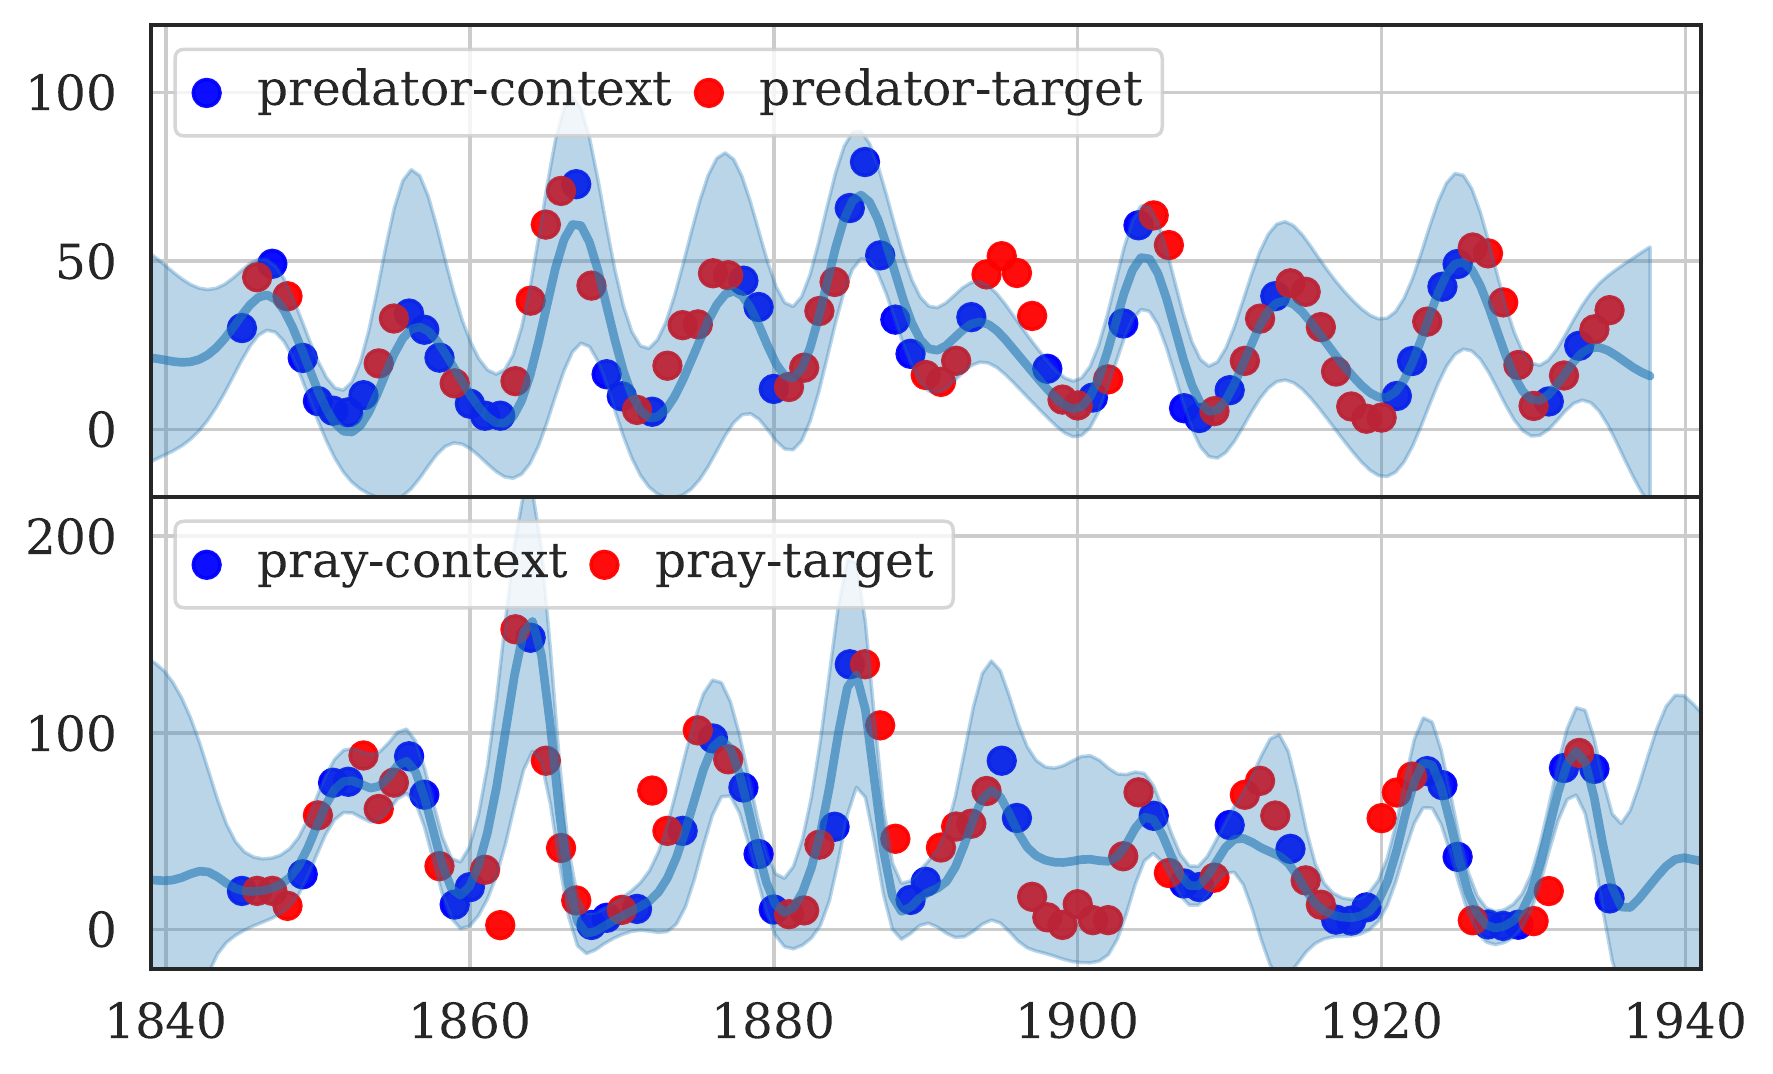}}

 \vspace{4mm}
\subfloat[\label{fig:pray-40c}GPConvCNP with Task1 ($N^c=40$)]{
 \includegraphics[width=0.49\linewidth]{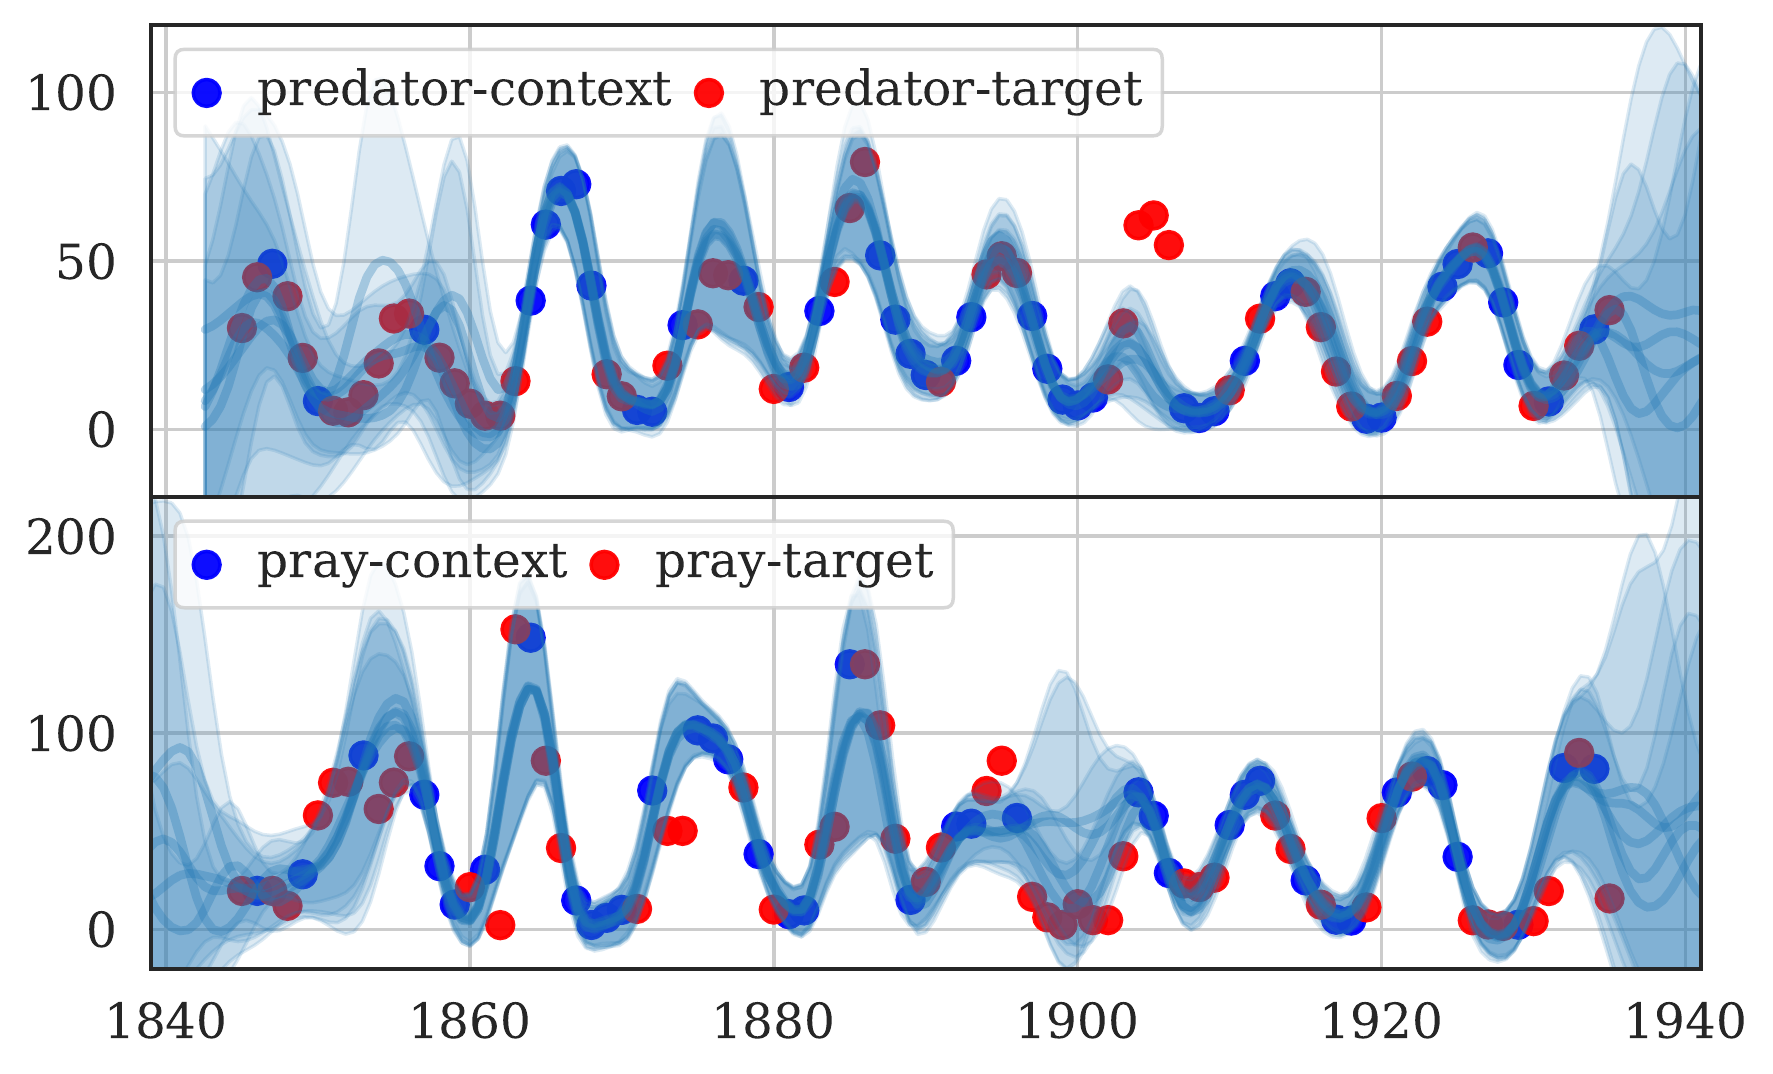}}
\subfloat[\label{fig:pray-40d}GPConvCNP with Task2 ($N^c=40$)]{
 \includegraphics[width=0.49\linewidth]{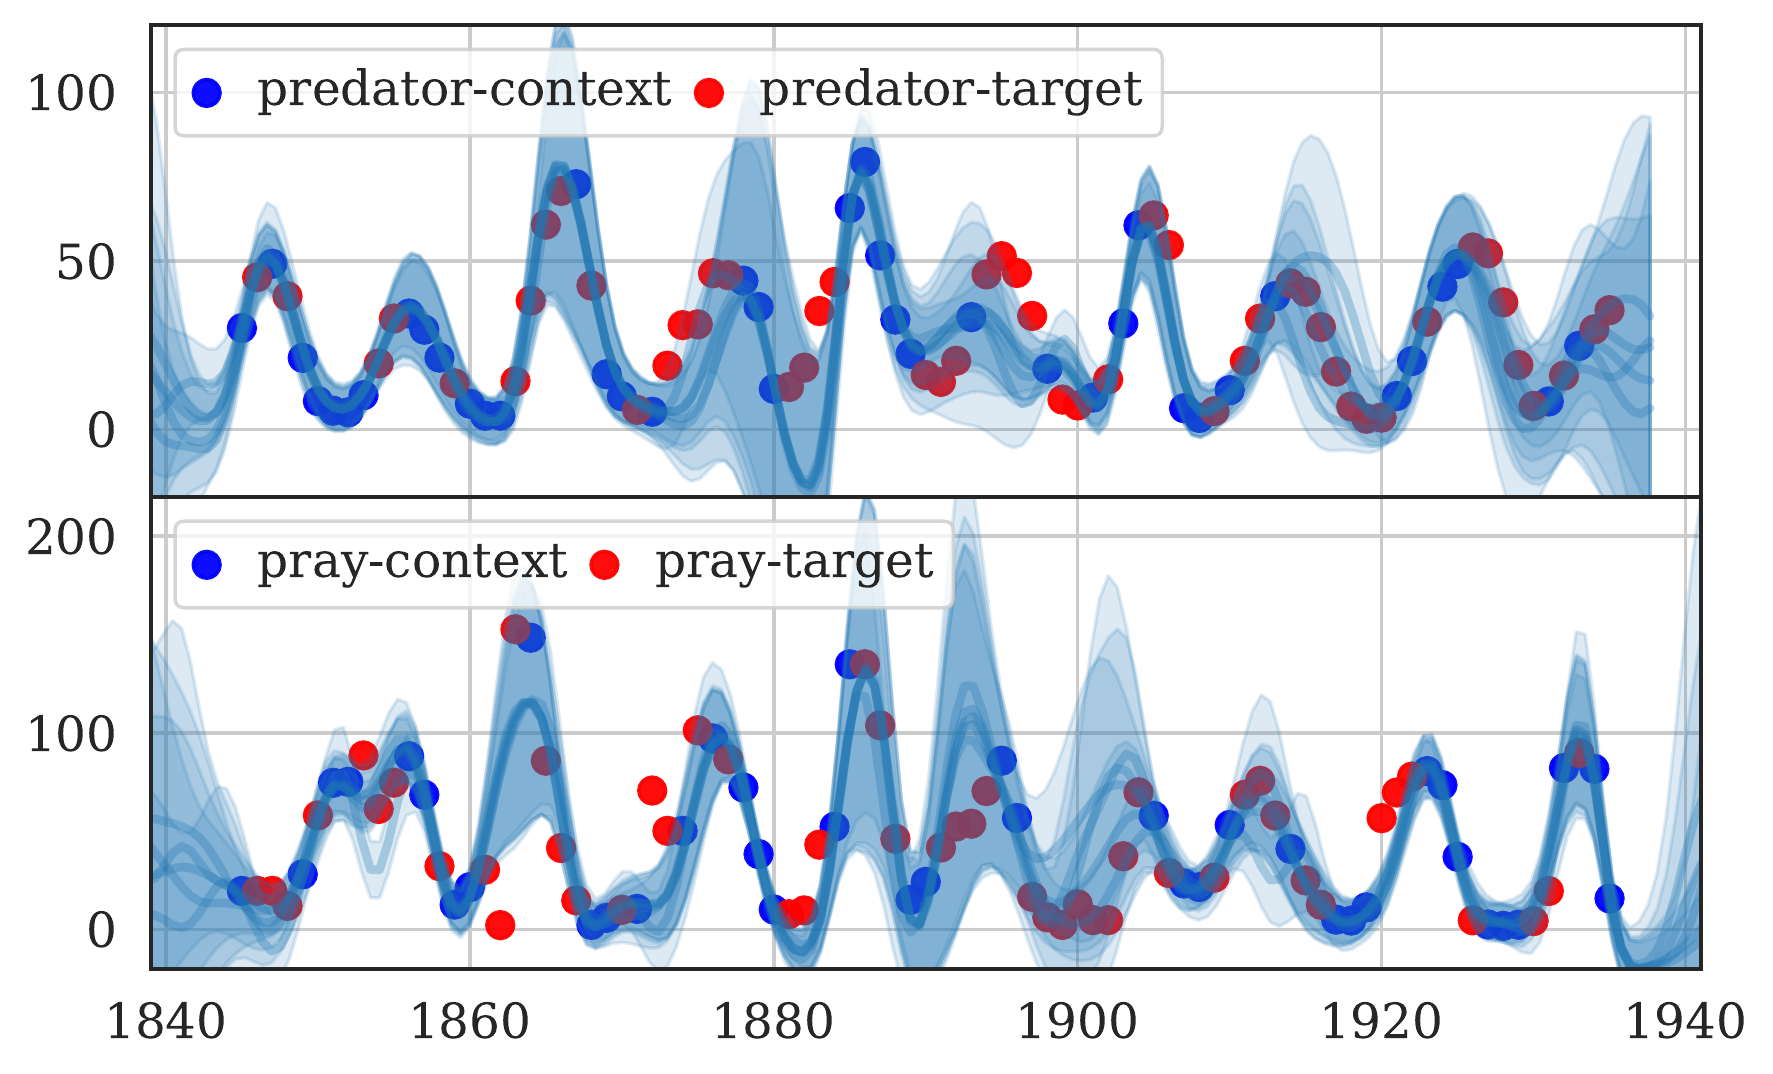}}
 
 \vspace{4mm}
\subfloat[\label{fig:pray-40e}Proposed Model with Task1 ($N^c=40$)]{
 \includegraphics[width=0.49\linewidth]{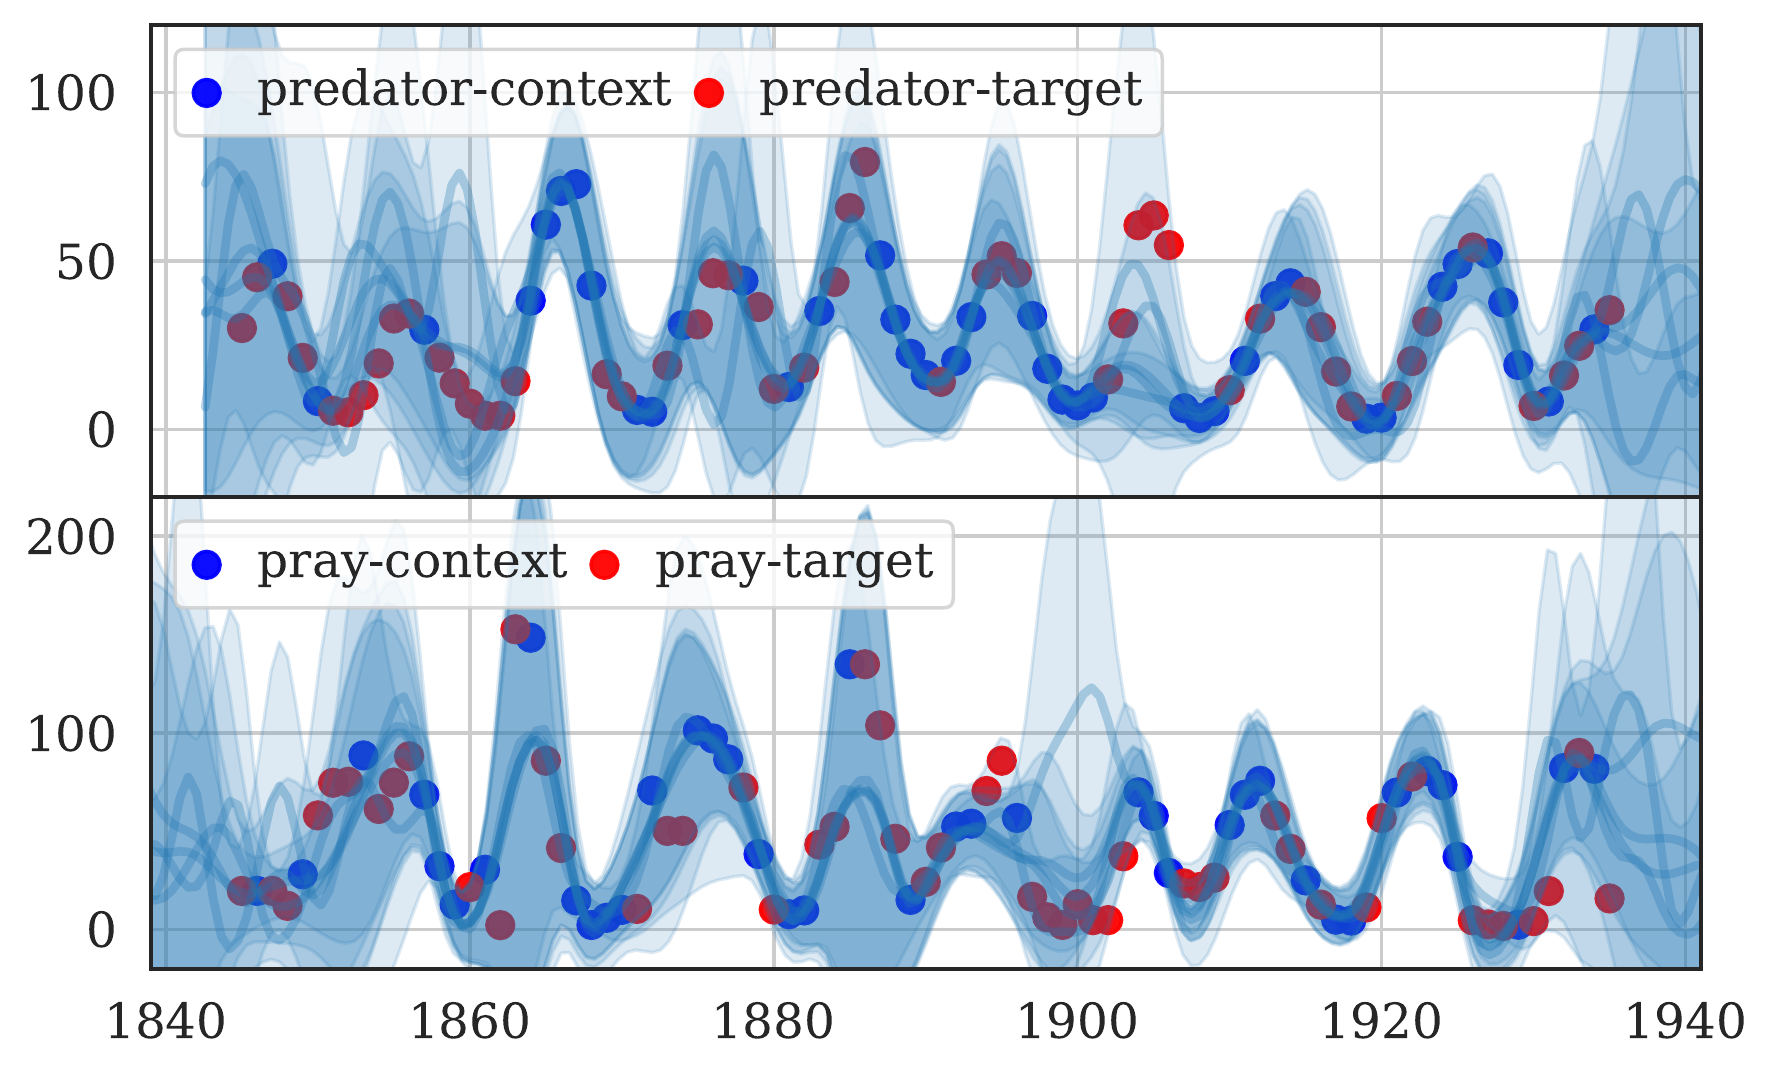}}
\subfloat[\label{fig:pray-40f}Proposed Model with Task2 ($N^c=40$)]{
 \includegraphics[width=0.49\linewidth]{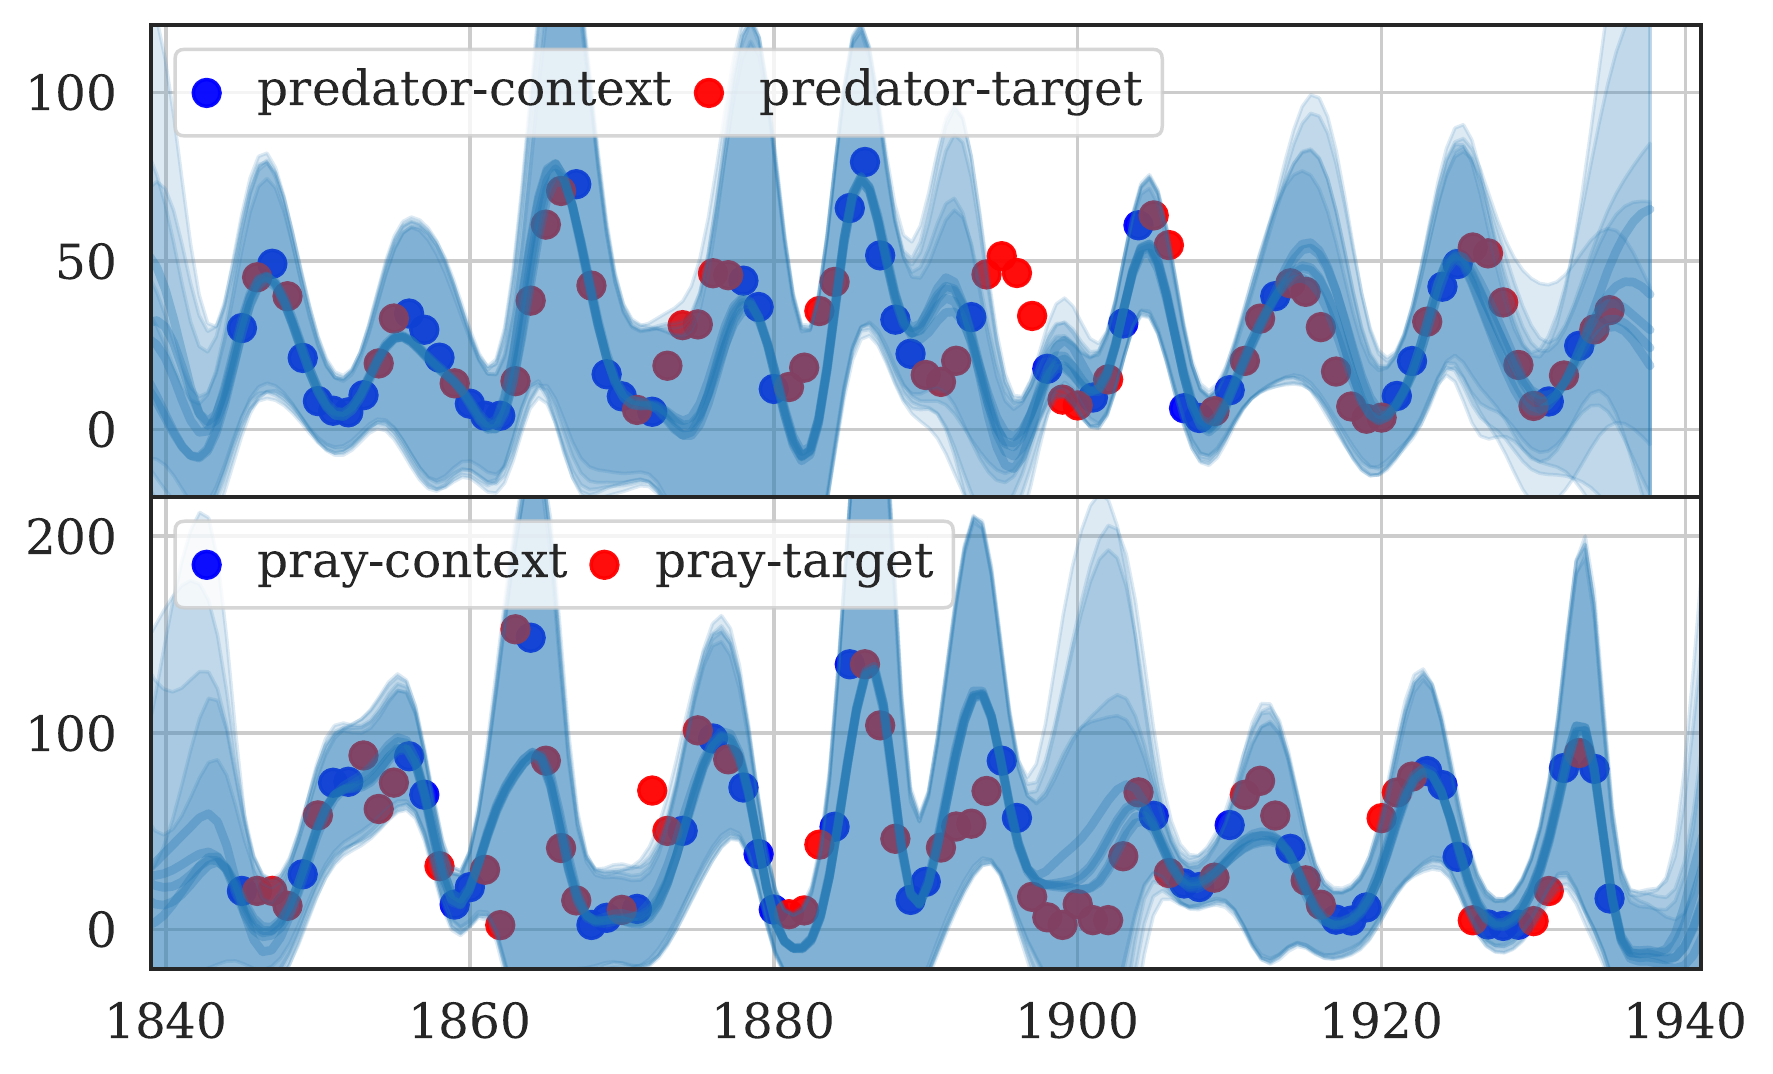}}

\caption{ Prediction results of \textb{Predator-Pray model with 40 context data points ($N^{c}=40$)}; \cref{fig:pray-40a,fig:pray-40b} shows the prediction results of 2 different tasks, respectively. \cref{fig:pray-40c,fig:pray-40d} correspond to the prediction results of GPConvCNP using 5 random functional representations. \cref{fig:pray-40e,fig:pray-40f} correspond to the prediction results of the proposed model using 5 random functional representations. These figures imply the task-dependent prior enables more robust predictions as shown in \cref{fig:pray-40e,fig:pray-40f} compared to GPConvCNP as shown in \cref{fig:pray-40c,fig:pray-40d}}
\label{fig:predator-pray-40}
\end{figure*}
