# Supplementary material for: Bayesian Convolutional Deep Sets with Task-Dependent Stationary Prior
Source: arXiv:2210.12363 source file (2022-10-22)
Supplement: Supplementary file 16 [file 07-appendix-v01-chapter4-exp3-figure03.tex]

\vspace{-5mm}
\begin{figure*}[htp!]

% \subfloat[\label{fig:fig-h} \textb{mosm-varying}: $p_{\text{traninv-nn}}(X_c,Y_c)$ ]   
% {\includegraphics[width=0.41\linewidth,height=4.85cm]{Figures/07-appendix-exp2/mosm-varying/mosmvarying_datav11_deptrue_gpdep_weight.pdf}} 
\centering
\subfloat[\label{fig:pray-70a} ConvCNP with Task1 ($N^c=70$)]{
 \includegraphics[width=0.49\linewidth]{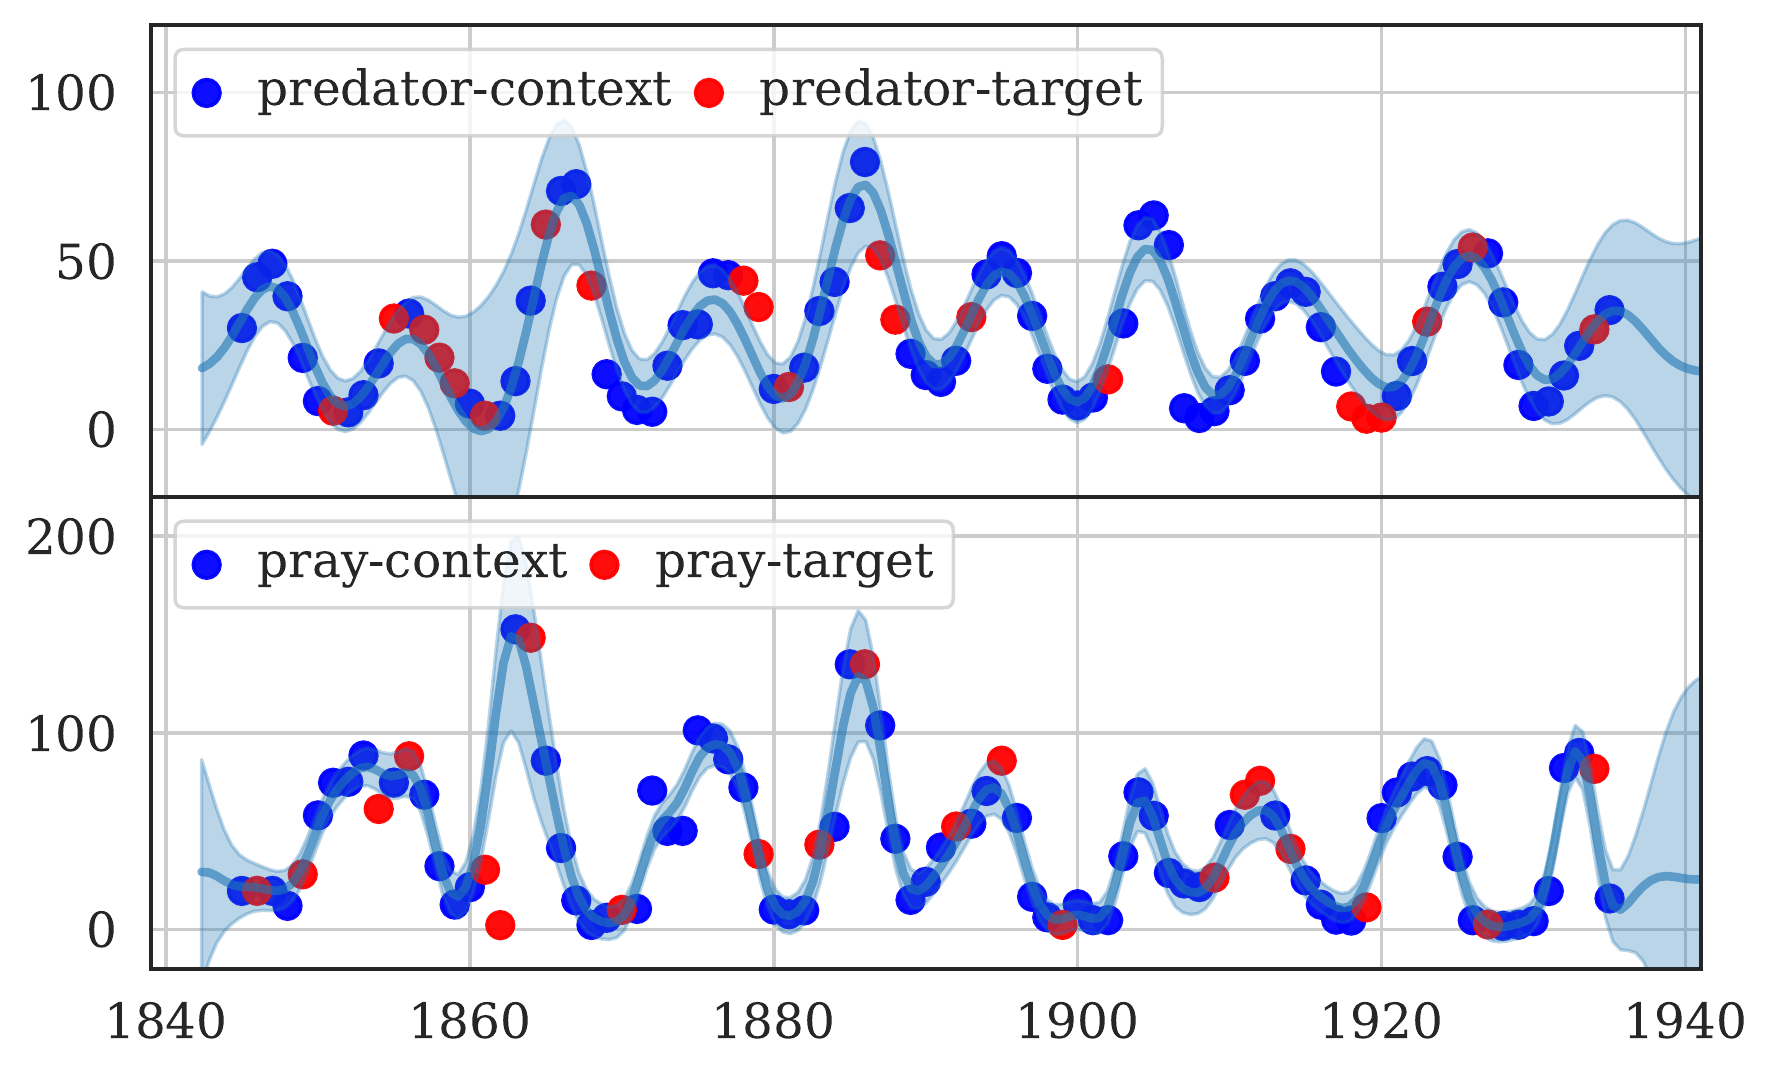}}
\subfloat[\label{fig:pray-70b} ConvCNP with Task2 ($N^c=70$)]{\includegraphics[width=0.49\linewidth]{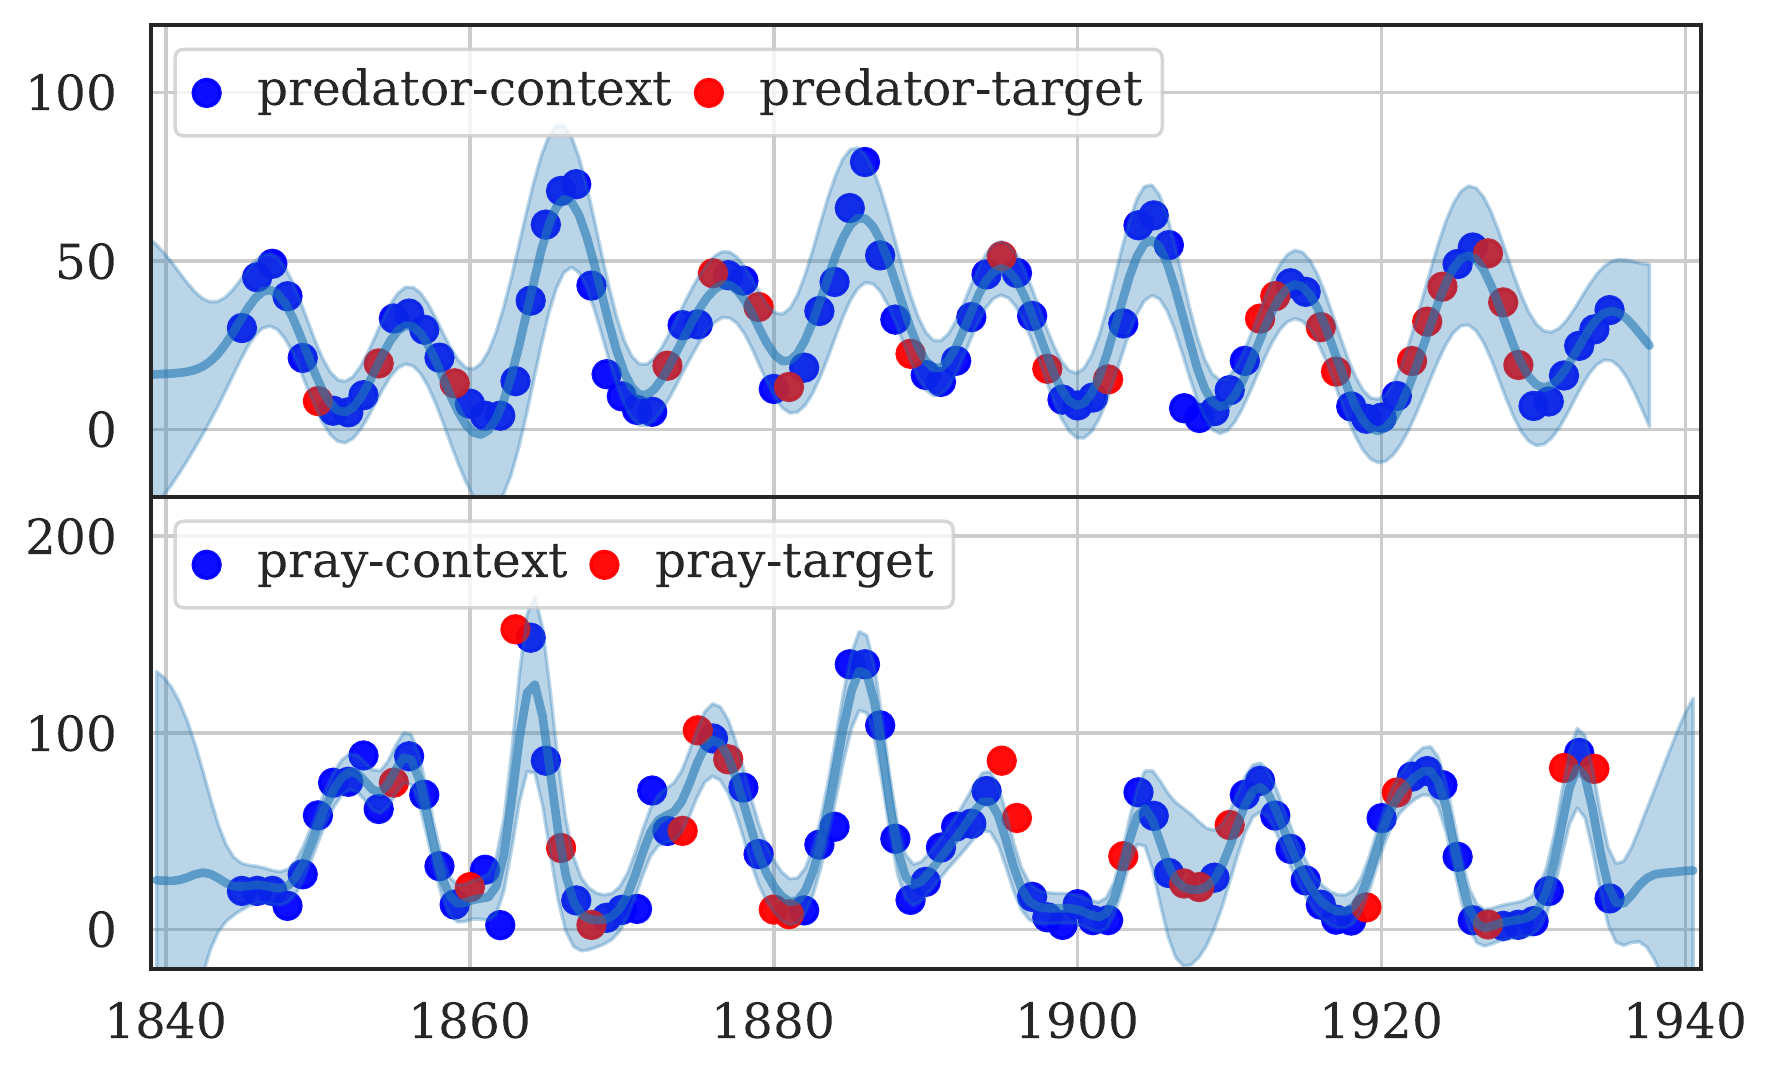}}

 \vspace{4mm}
\subfloat[\label{fig:pray-70c} GPConvCNP with Task1 ($N^c=70$)]{
 \includegraphics[width=0.49\linewidth]{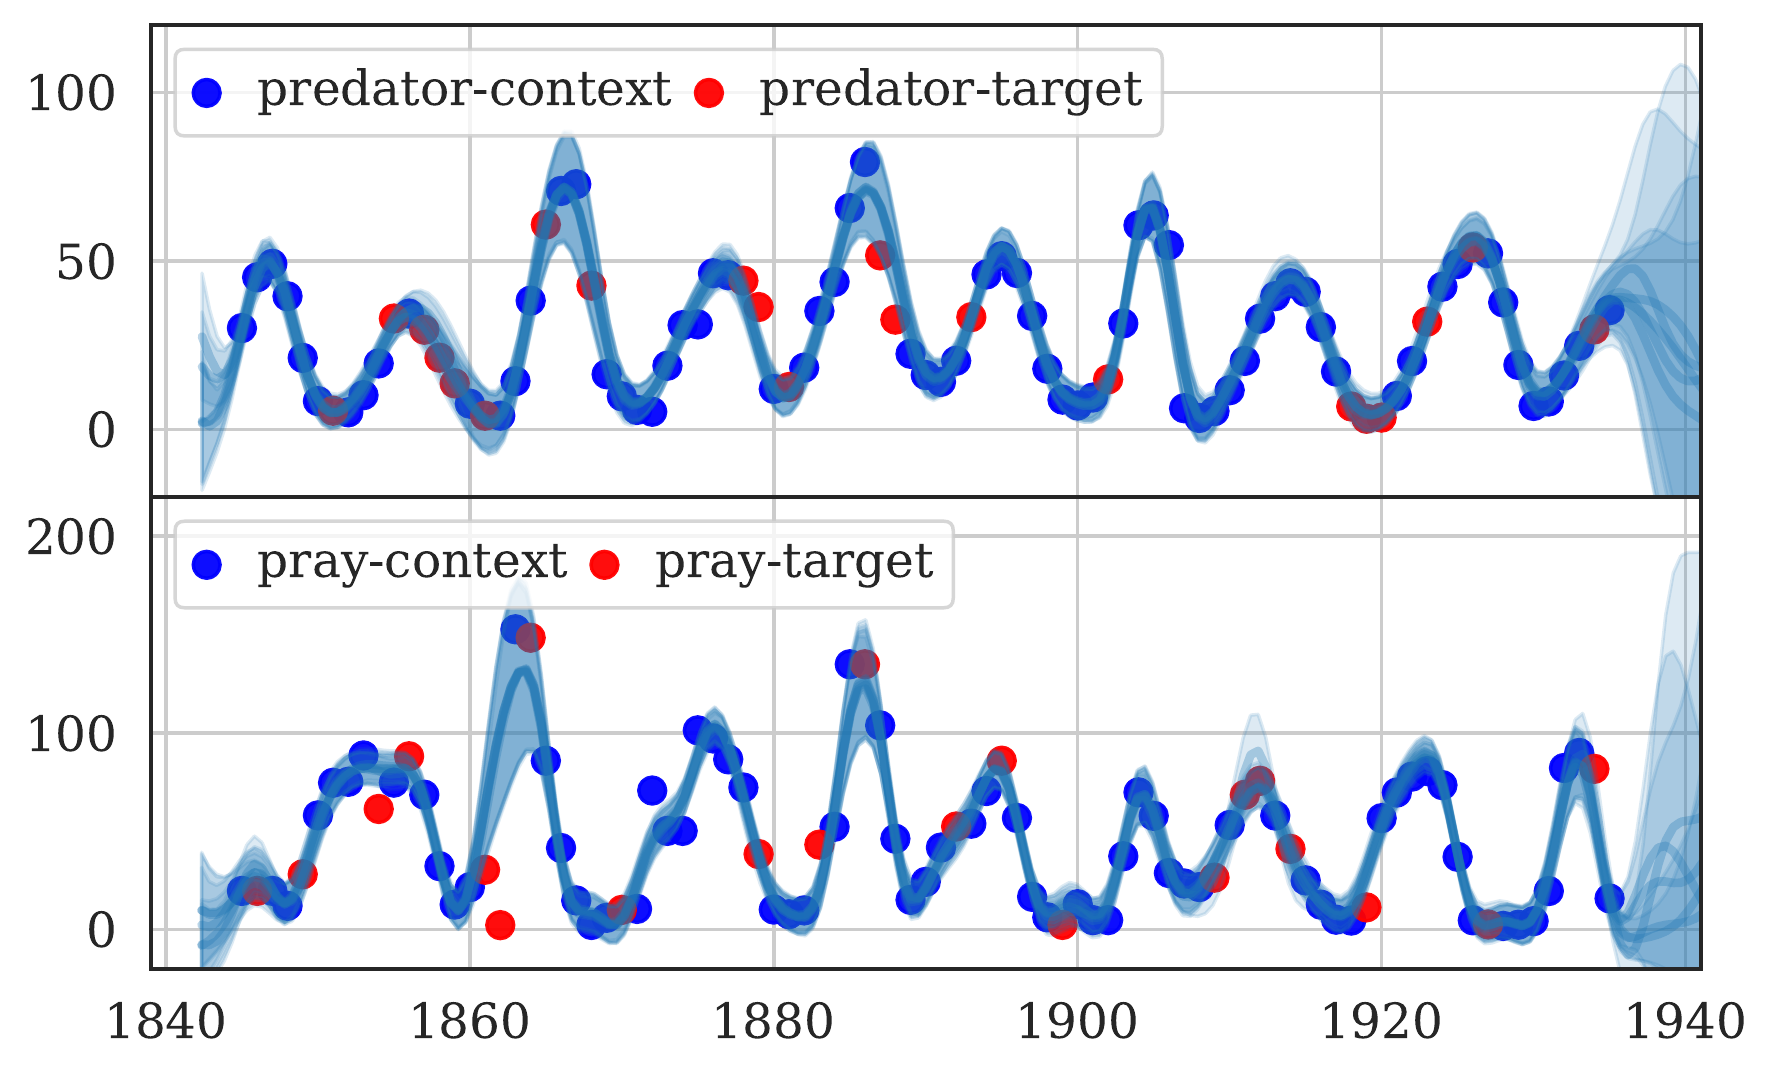}}
\subfloat[\label{fig:pray-70d} GPConvCNP with Task2 ($N^c=70$)]{
 \includegraphics[width=0.49\linewidth]{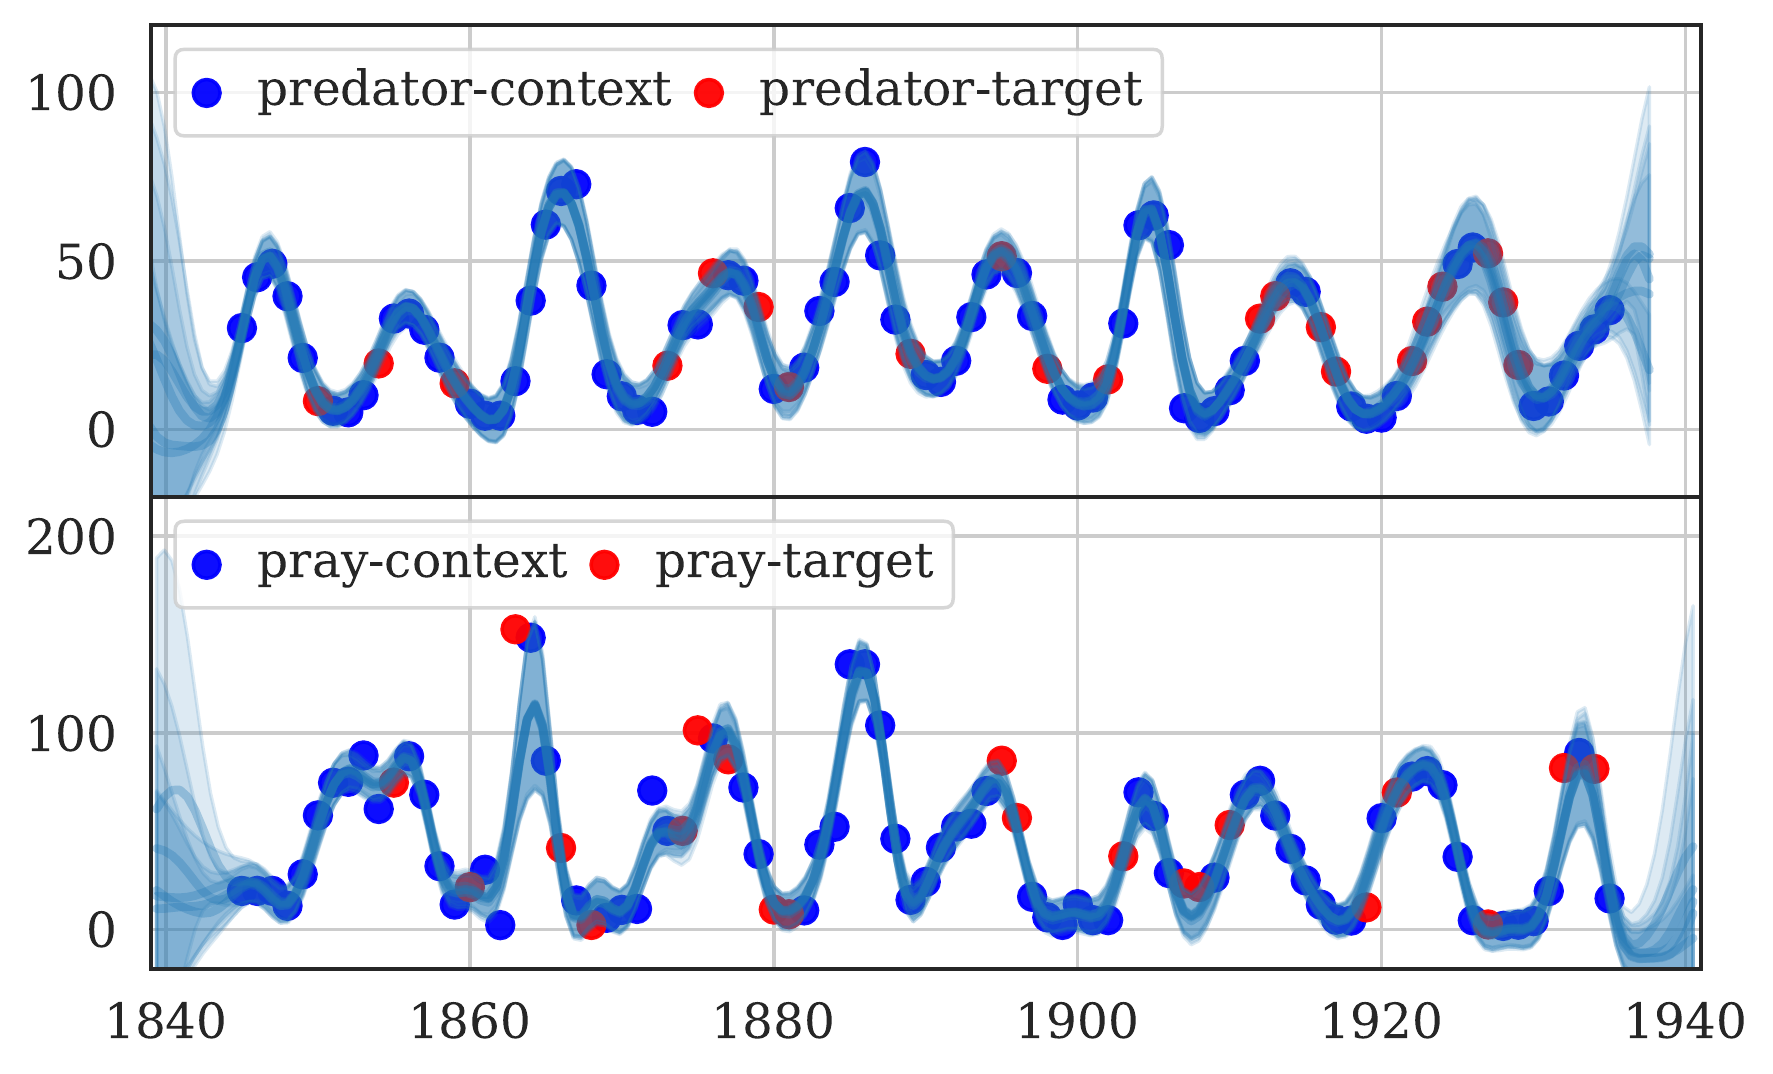}}
 
 \vspace{4mm}
\subfloat[\label{fig:pray-70e}Proposed Model with Task1 ($N^c=70$)]{
 \includegraphics[width=0.49\linewidth]{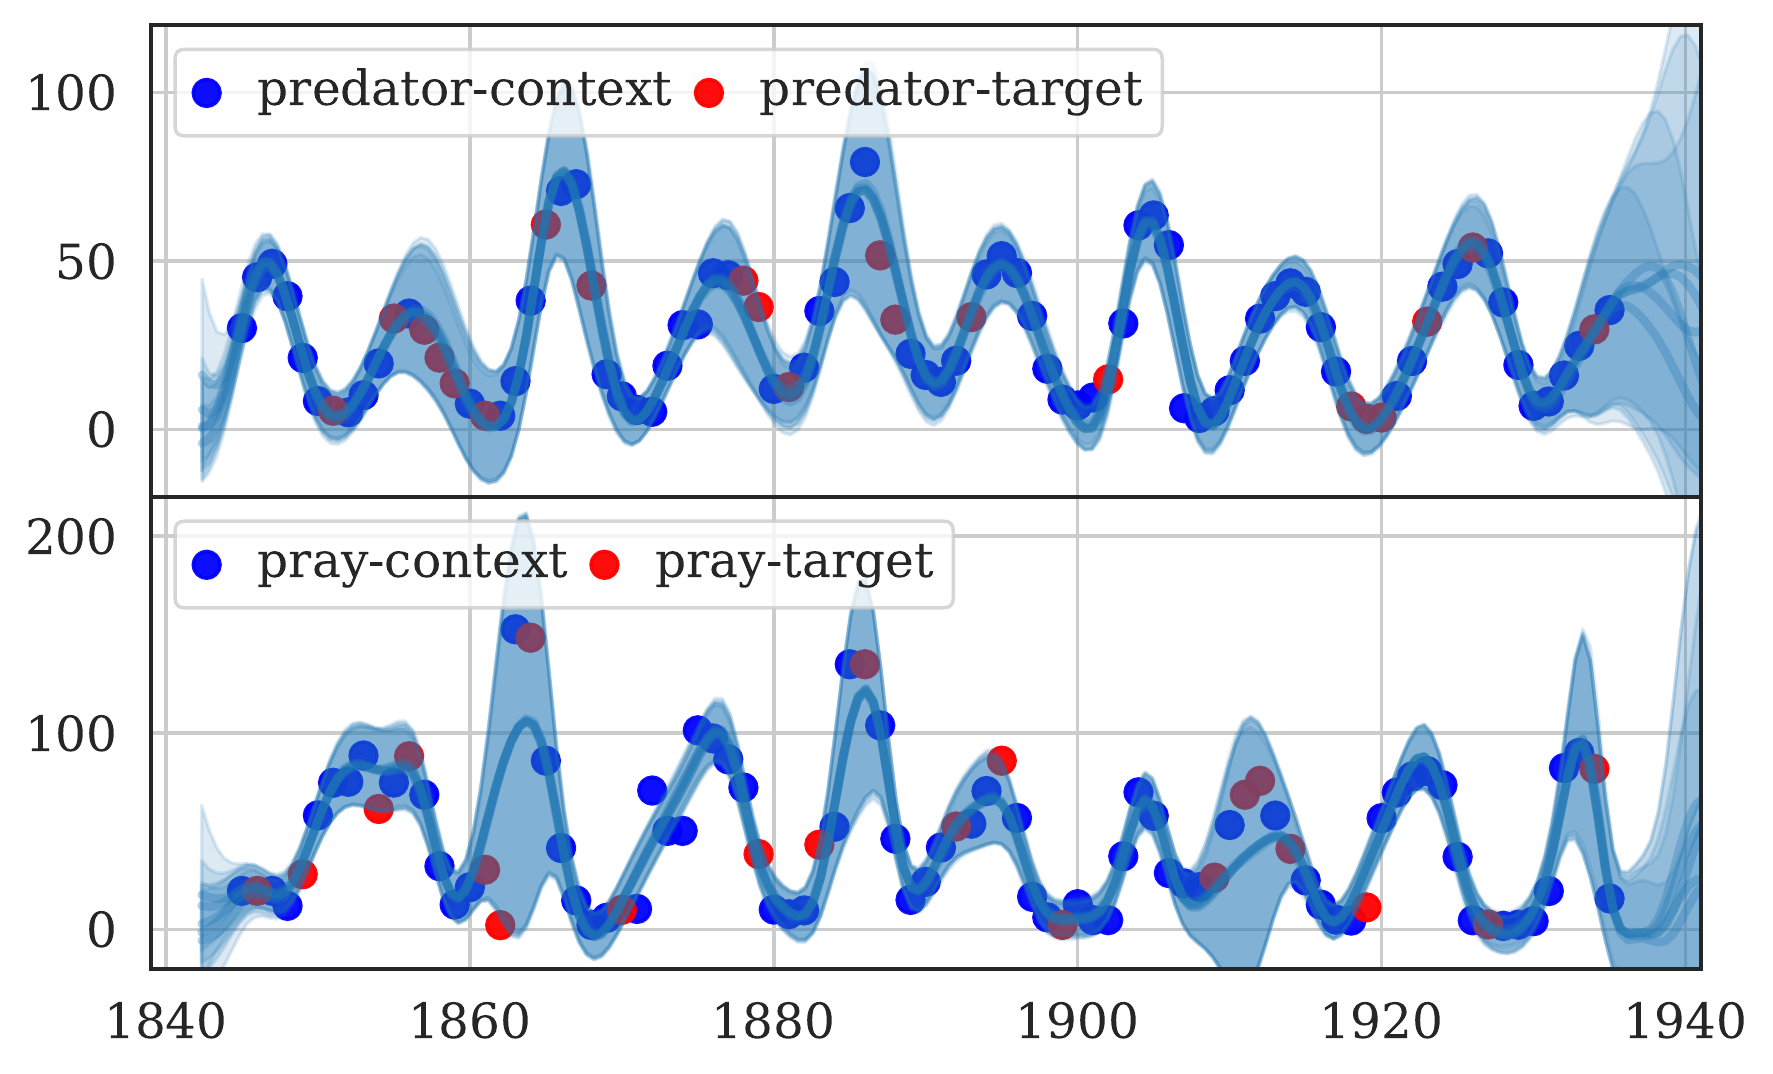}}
\subfloat[\label{fig:pray-70f}Proposed Model with Task2 ($N^c=70$)]{
 \includegraphics[width=0.49\linewidth]{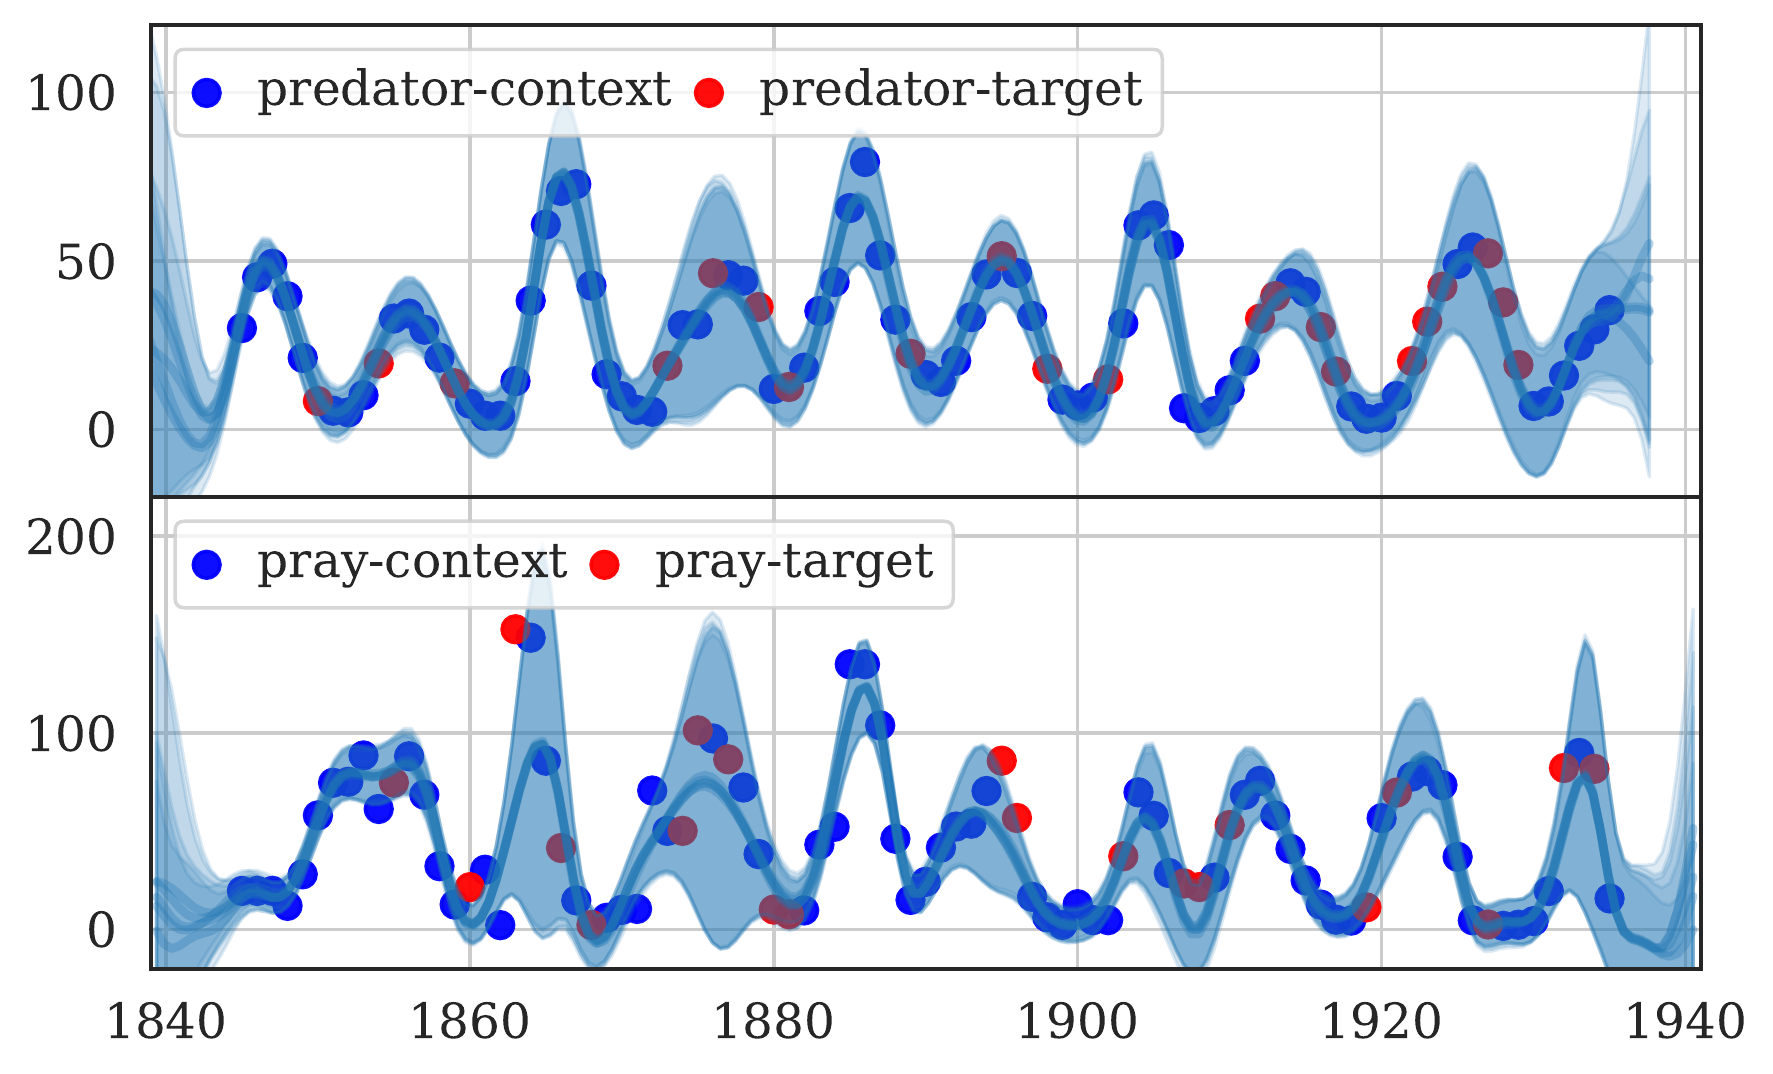}}

\caption{Prediction results of \textb{Predator-Pray model with 70 context data points ($N^{c}=70$)}; \cref{fig:pray-70a,fig:pray-70b} shows the prediction results of 2 different tasks, respectively. \cref{fig:pray-70c,fig:pray-70d} correspond to the prediction results of GPConvCNP using 5 random functional representations. \cref{fig:pray-70e,fig:pray-70f} correspond to the prediction results of the proposed model using 5 random functional representations. These figures imply  that all models obtain similar predictive distribution on target sets when the large number of context data points is given.}
\label{fig:predator-pray-70}
\end{figure*}
