# Supplementary material for: Bayesian Convolutional Deep Sets with Task-Dependent Stationary Prior
Source: arXiv:2210.12363 source file (2022-10-22)
Supplement: Supplementary file 17 [file 07-appendix-v01-chapter4-exp3.tex]

%\subsection{Further Details for the Predator-Pray model}
%\section{Further Details for the Predator-Pray model}
\section{Further Details for Simulation to Real (Predator-Pray model)}

\subsection{Details for Datasets}

In this experiment, we use synthetic dataset simulated by a Lotka-Volterra differential equation \citeb{lotka2002contribution} for training, and then predicts the real-world dataset (Hudson’s Bay hare-lynx data) for test. We employ the following implementation \citeb{lee2020bootstrapping} \footnotemark{\footnotetext[4]{\url{https://github.com/juho-lee/bnp/blob/master/regression/data/lotka_volterra.py}}}.

\subsection{Details for Tasks of Training, Validation, and Test }
We consider the following number of data points for training, validation, and test: 
\begin{itemize}[leftmargin=1em]
    \vspace{-2mm}
    \item \textbf{Simulated dataset:}
    For training, we randomly sample total data point \textb{$N \sim \mathcal{U}([100{-}15,100])$}, and set $N_t=N$ as the number of target data points for each task. Out of the sampled total points, we sample \textb{$N_c \sim \mathcal{U}([15,30{-}15])$} data points randomly, and use them as context data points. We use \textb{$100{\times}32{\times}32$} tasks for training through 100 batches. For validation, we set $N_c$ context data points and $N_t$ target data points as done in training, and use \textb{$128{\times}32$} tasks for validation to choose the parameters of the trained models.
    For test, we consider $N_t$ target data points per a task as described in training, and use \textb{$N_c \in \{10,20,30,40,50,70,80\}$} context data points, that are chosen randomly from the $N_t$ target data points for each task. We use \textb{$64{\times}16$} tasks per given $N_c$ context points to study how the number of context data points affects the predictive performance of the trained models using the parameters obtained in validation procedure.
    \item \textbf{Real dataset:} For evaluation on real dataset, we consider $N_t=91$ target data points, and use \textb{$N_c \in \{10,20,30,40,50,70,80\}$} context data points, that are chosen randomly from $N_t$ target data points for each task. We use \textb{$64{\times}16$} tasks per given $N_c$ context points to evaluate the trained model with Simulated dataset.
\end{itemize}

\subsection{Details for Hyperparameters.}

For the hyperparameter of RBF kernels used for ConvCNP, we conduct the experiment with  $l\in\{0.01,0.1\}$, and set the lengthscale $l=0.01$ for each channel because it obtains the best performance for both models out of those candidates.

For the hyperparameter used for GPConvCNP, we use RBF kernel $(Q=1)$ for each channel, and set $\Sigma=0.1$ for each channel. 

For the hyperparameter of basis kernels, we set $\mathrm{Hz}_{\mathrm{max}}=5$ and 4 basis stationary kernels ($Q=4$). Then, we set $\{\mu_q\}_{q=1}^{4}$ by randomly sampling $\mu_q \sim \mathcal{U}[0,\mathrm{Hz}_{\mathrm{max}}]$ with $\mu_1=0 \leq ..\leq \mu_4$, and set
$\Sigma_q = 0.1$ for $q=1,..,4$. For the noise parameter $\sigma^{2}_{\epsilon}$, we set $\sigma_{\epsilon}=1e\text{-}{2}$.

For the number of spectral points, we use $l=10$ in \textb{Eq. (14)}.

For the number of sample function, we use $N=5$ in \textb{Eq. (19)}.

For the prior hyperparameter of approximate scheme $\alpha$, we use $\alpha \in \{.05,0.1\}$.

For training, we  use ADAM optimizer \citeb{kingma2014adam} with learning rate $1e\text{-}3$ and weight decay $1e\text{-}4$. 

For the regularizer hyperparameter $\beta$ in \textb{Eq. (21)}, we set $\beta=0.5$ for the proposed method.

\clearpage
\subsection{Additional Results}
%fig:predator-pray-70

%We report additional prediction results obtained in experimental section 5.3 (main). 

We conduct the predator-pray benchmark experiment conducted in \citeb{gordon2019convolutional,petersen2021gp,lee2020bootstrapping}; the NP models are first trained on the synthetic dataset simulated by a Lotka-Volterra differential equation \citeb{lotka2002contribution}, and then predict the real-world dataset (Hudson’s Bay hare-lynx data). 

%Further details of settings and additional results are reported in \textb{Appendix A.4}.

%{\includegraphics[width=0.48\linewidth,height=2.75cm]
\begin{figure}[H]
\subfloat[\label{fig:predpray-a} simulated set]
{\includegraphics[width=0.24\linewidth]{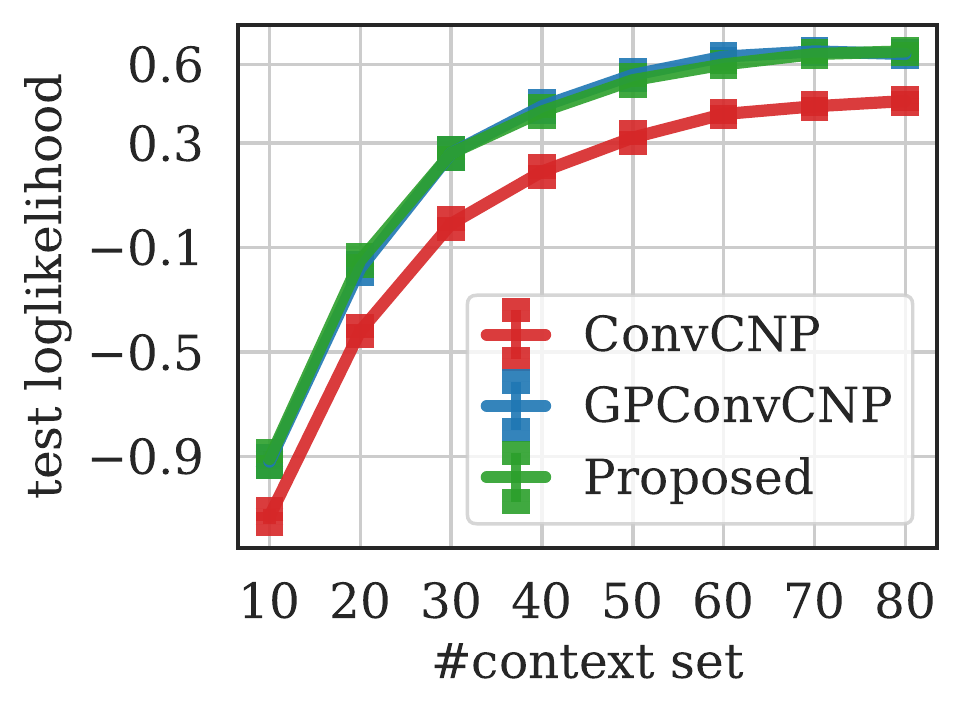}} \hspace{1mm}  
\subfloat[\label{fig:predpray-b} real set]
{\includegraphics[width=0.24\linewidth]{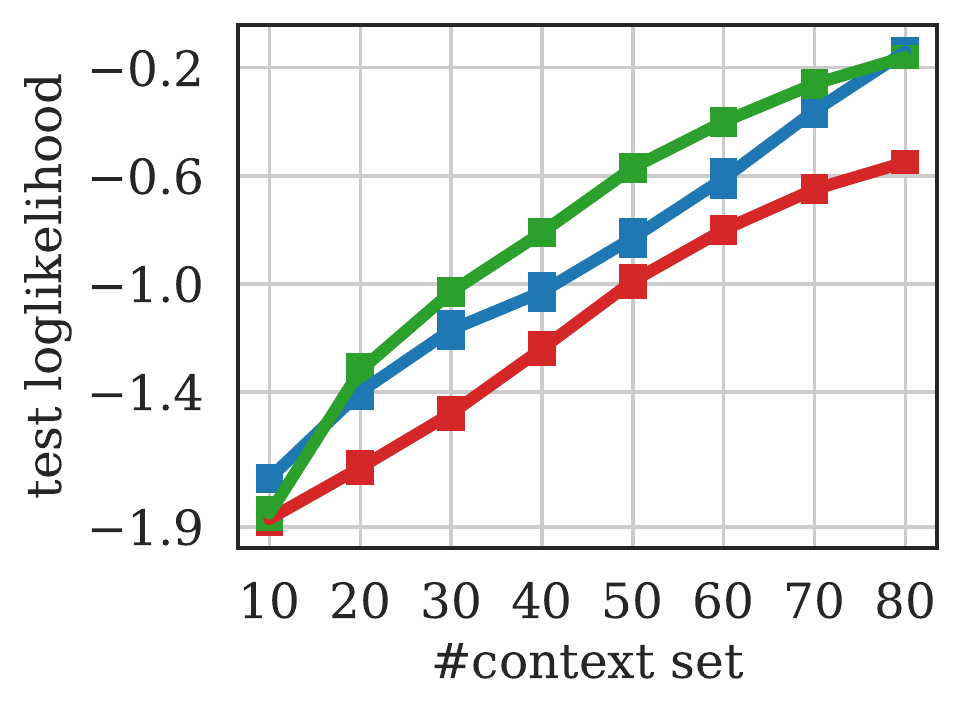}}  
\subfloat[\label{fig:predpray-c} real set]
{\includegraphics[width=0.235\linewidth]{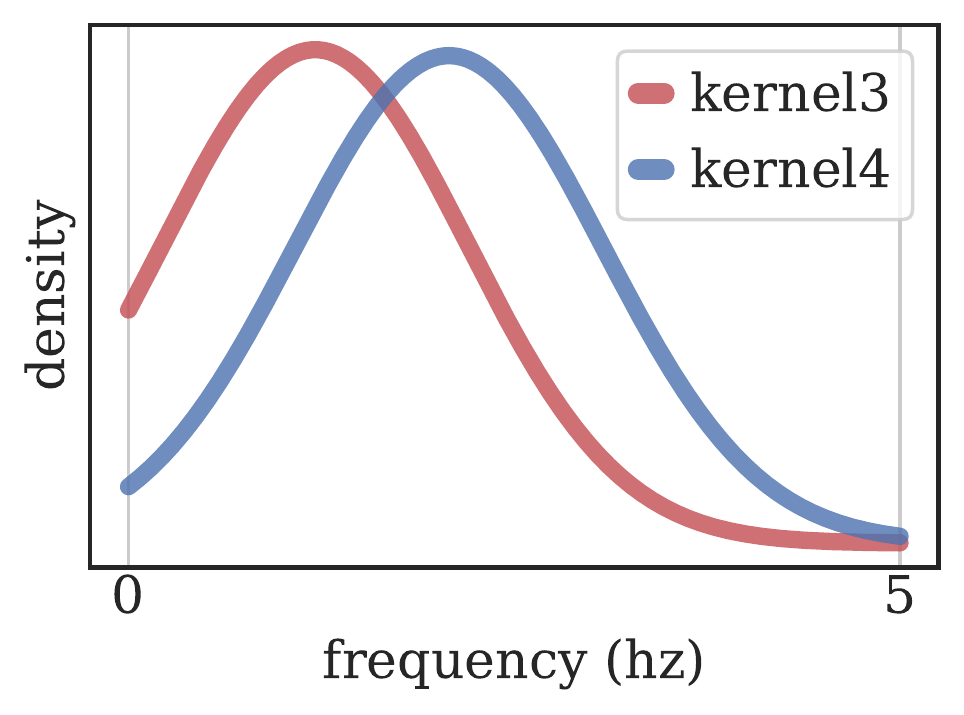}}  
\subfloat[\label{fig:predpray-d} real set]
{\includegraphics[width=0.25\linewidth]{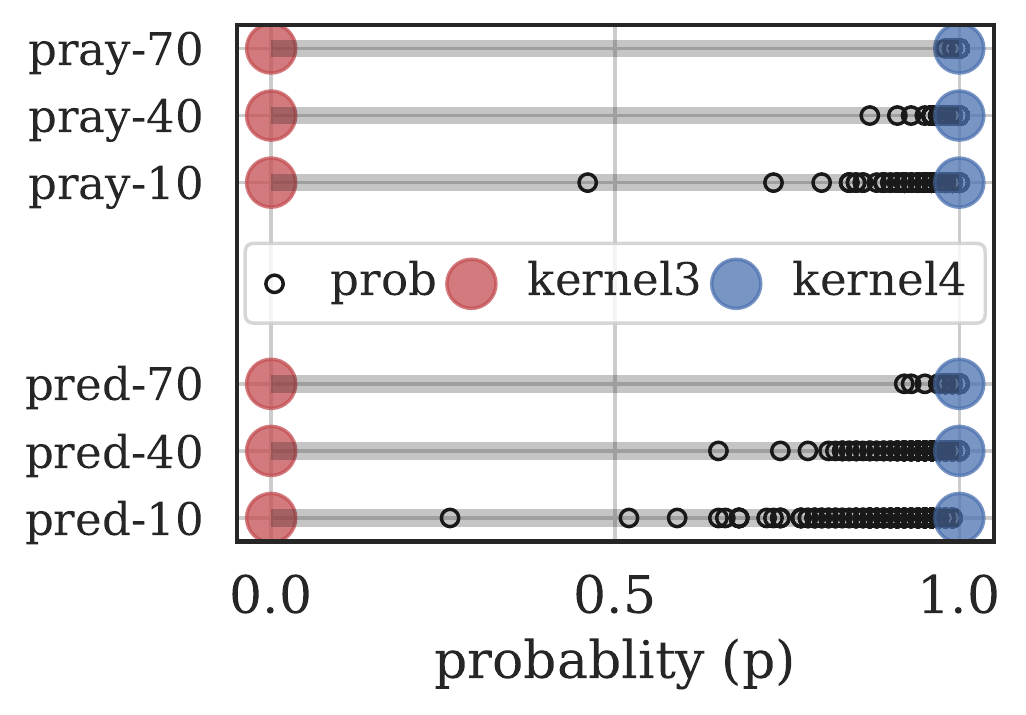}}  
\caption{{Prediction Results on simulated and real dataset;}}
\end{figure}

\cref{fig:predpray-a,fig:predpray-b} describes the mean and one-standard error of the test log likelihood for 1024 tasks of simulated and real datasets, respectively; we consider $N^{c}\in \{10,...,80\}$ context points. These figures imply that for small $N^{c}\in \{20,..,70\}$ context data points, task-dependent prior could help improve the prediction performance by using the different prior depending on $N^{c}$ context data points.

\cref{fig:predator-pray-10,fig:predator-pray-40,fig:predator-pray-70} show the prediction results of ConvCNP, GPConvCNP, and the proposed model for 2 different tasks of \textb{real dataset}, respectively.\cref{fig:predator-pray-10} shows the results using 10 context data points ($n^{c}=10$).  \cref{fig:predator-pray-40} and \cref{fig:predator-pray-70} correspond to results of $n^{c}=40$ and $n^{c}=70$, respectively. GPConvCNP and the proposed model generate 5 predictive distributions on target set respectively by using 5 random functional representations. 

\cref{fig:predator-pray-10} reveals that how the random functional representations using prior affect the prediction on target sets when the small number of context data points is given. \cref{fig:predator-pray-40} reveals that the task-dependent prior enables more robust predictions as shown in \cref{fig:pray-40e,fig:pray-40f} compared to GPConvCNP as shown in \cref{fig:pray-40c,fig:pray-40d}. \cref{fig:predator-pray-70} reveals that all models obtain similar predictive distribution on target sets when the large number of context data points is given.

\vspace{5mm}

\vspace{-5mm}
\begin{figure*}[htp!]

% \subfloat[\label{fig:fig-h} \textb{mosm-varying}: $p_{\text{traninv-nn}}(X_c,Y_c)$ ]   
% {\includegraphics[width=0.41\linewidth,height=4.85cm]{Figures/07-appendix-exp2/mosm-varying/mosmvarying_datav11_deptrue_gpdep_weight.pdf}} 
\centering
\subfloat[ \label{fig:pray-10a} ConvCNP with Task1 ($N^c=10$)]{
 \includegraphics[width=0.49\linewidth]{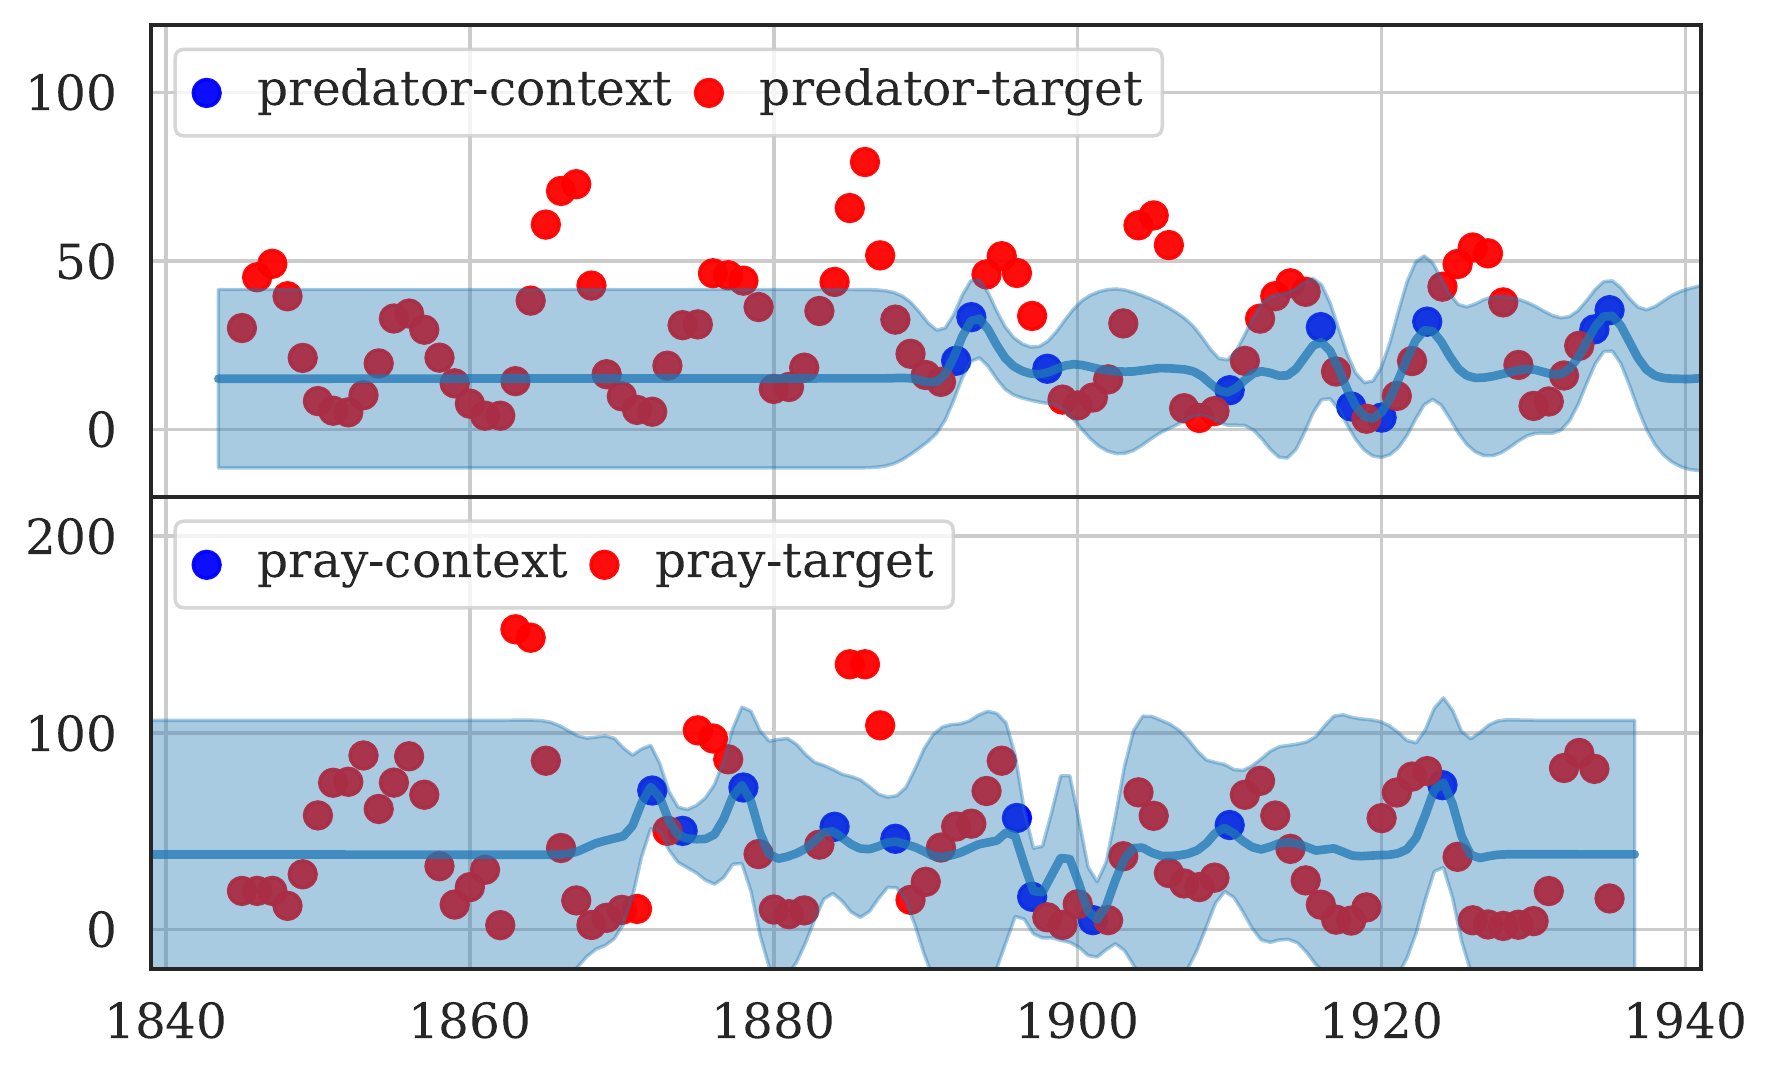}}
\subfloat[ \label{fig:pray-10b} ConvCNP with Task2 ($N^c=10$)]{\includegraphics[width=0.49\linewidth]{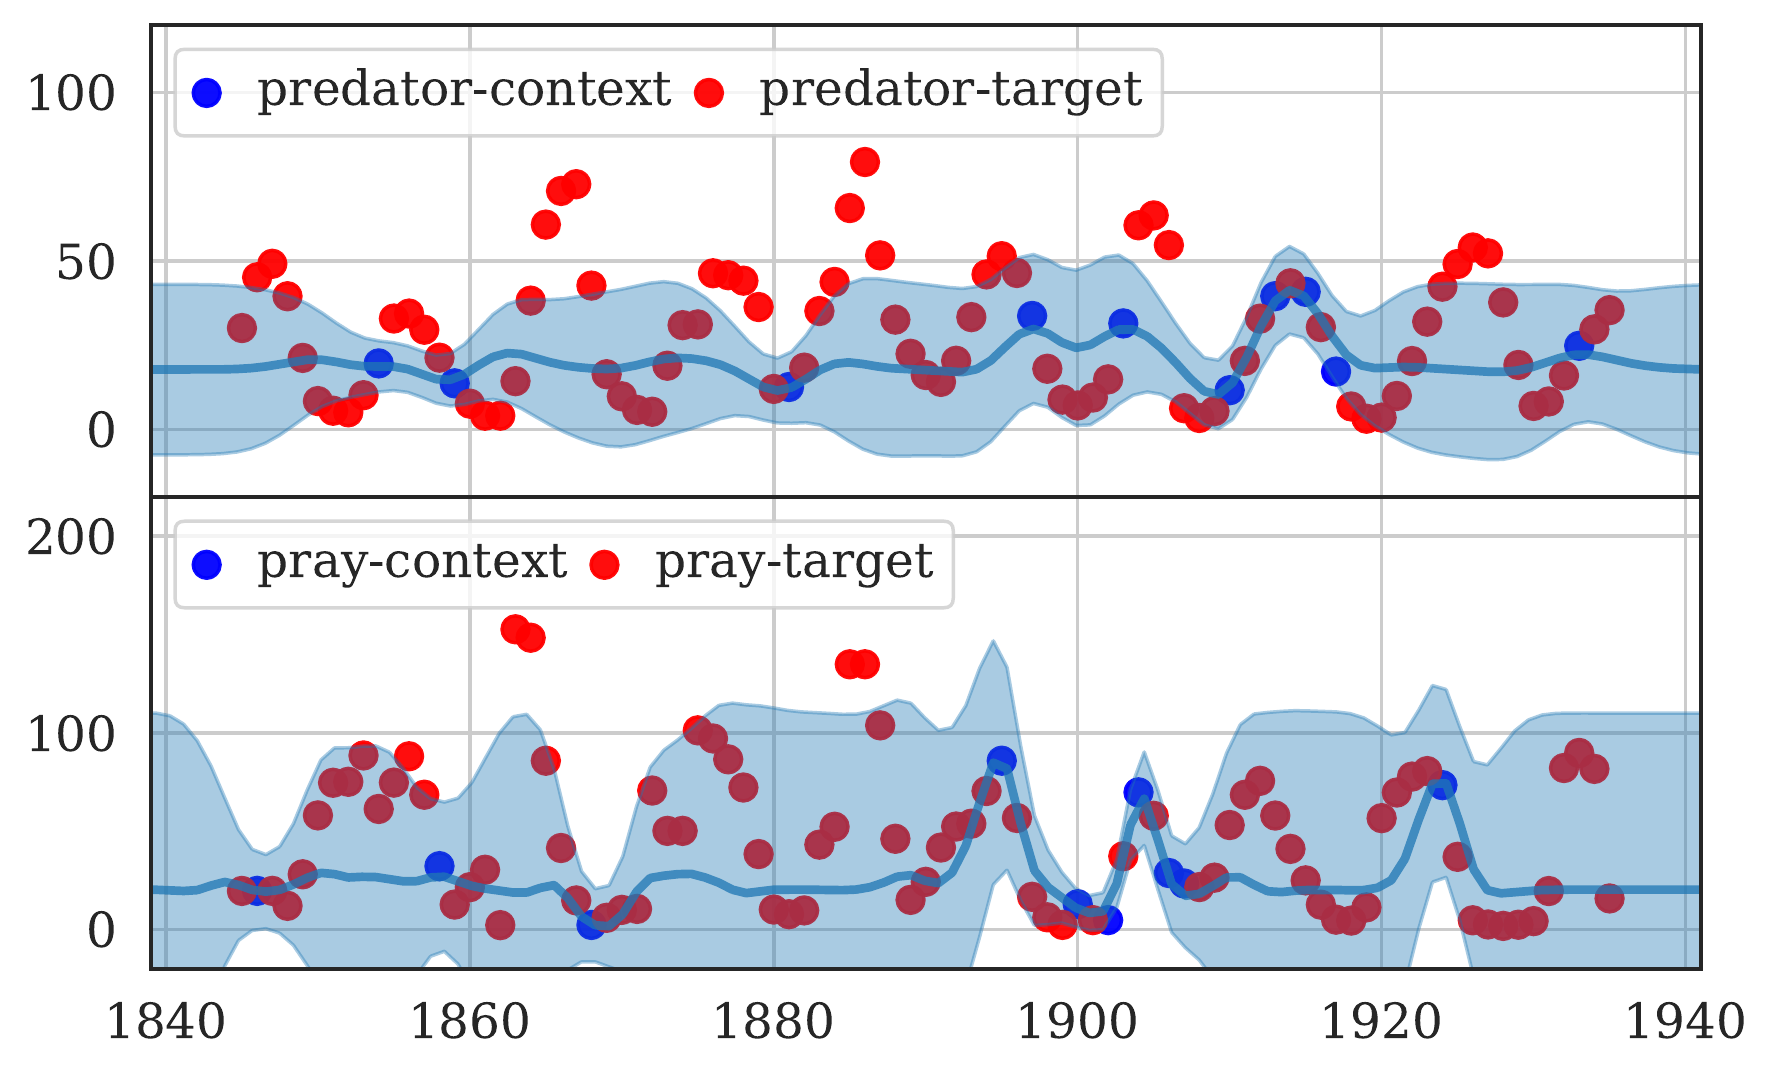}}

 \vspace{4mm}
\subfloat[ \label{fig:pray-10c} GPConvCNP with Task1 ($N^c=10$)]{
 \includegraphics[width=0.49\linewidth]{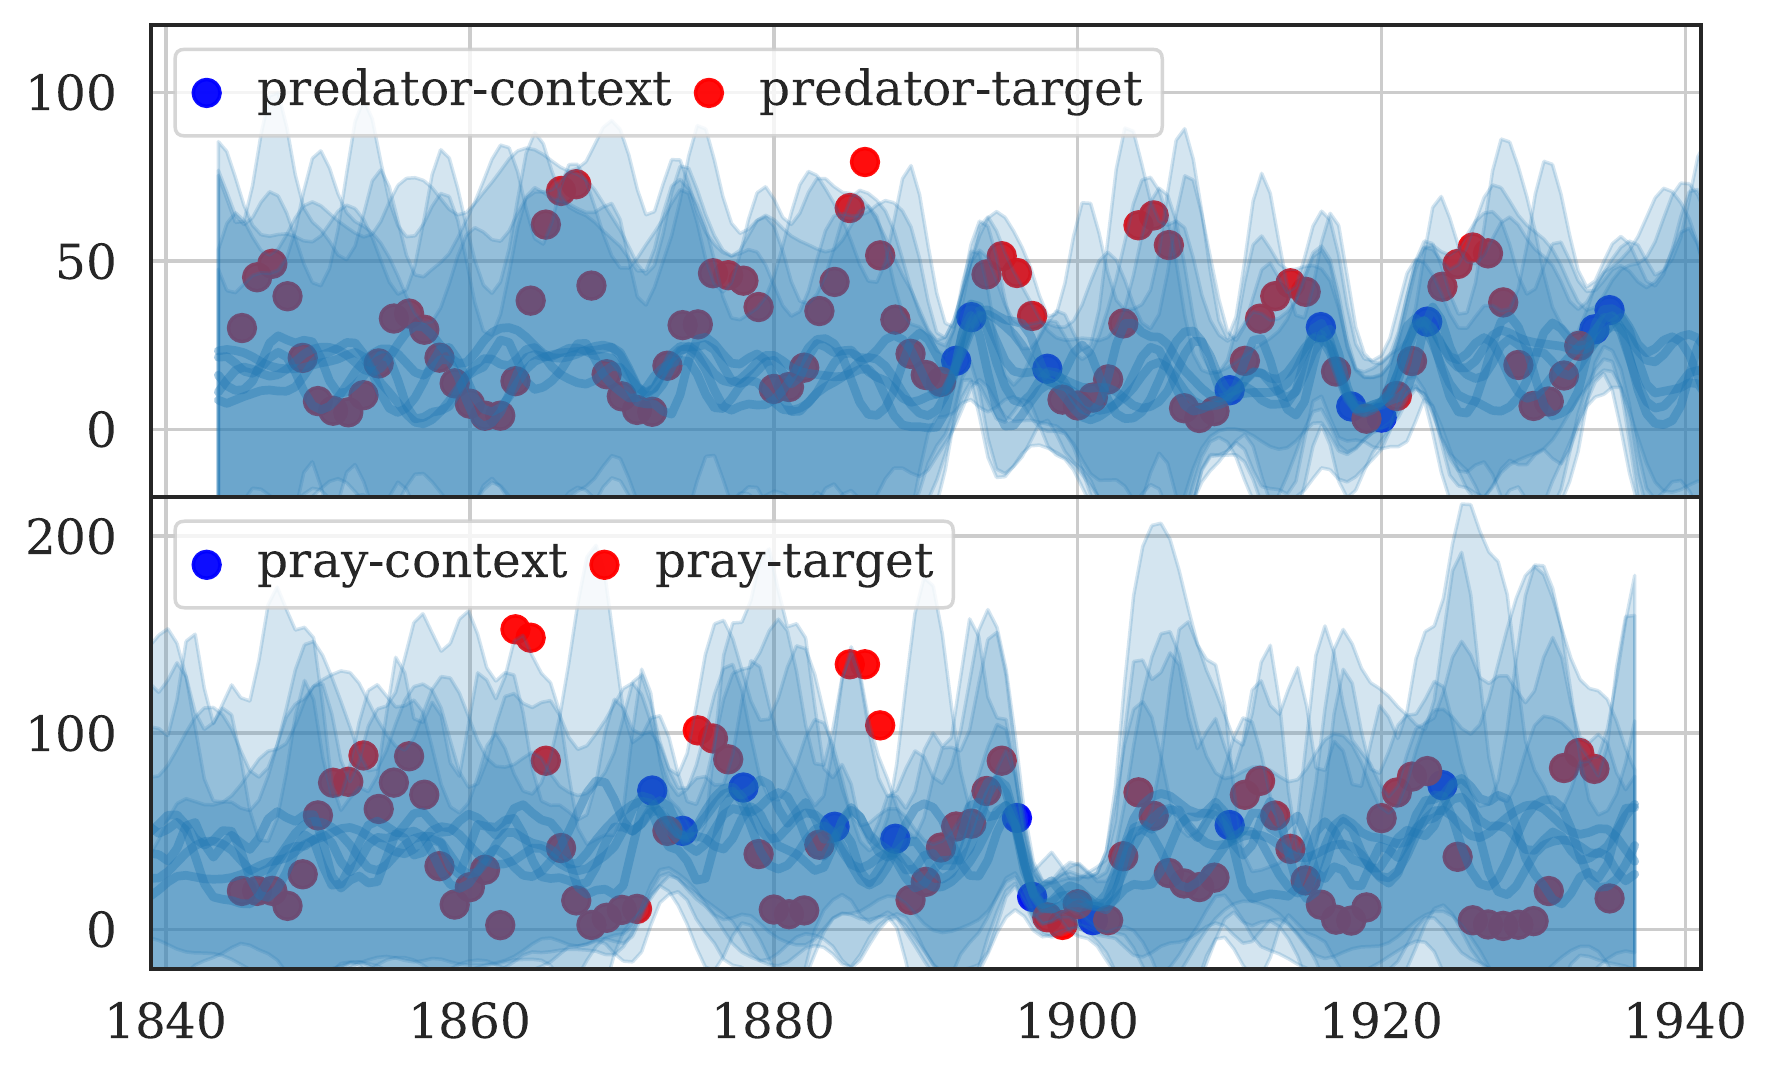}}
\subfloat[\label{fig:pray-10d} GPConvCNP with Task2 ($N^c=10$)]{
 \includegraphics[width=0.49\linewidth]{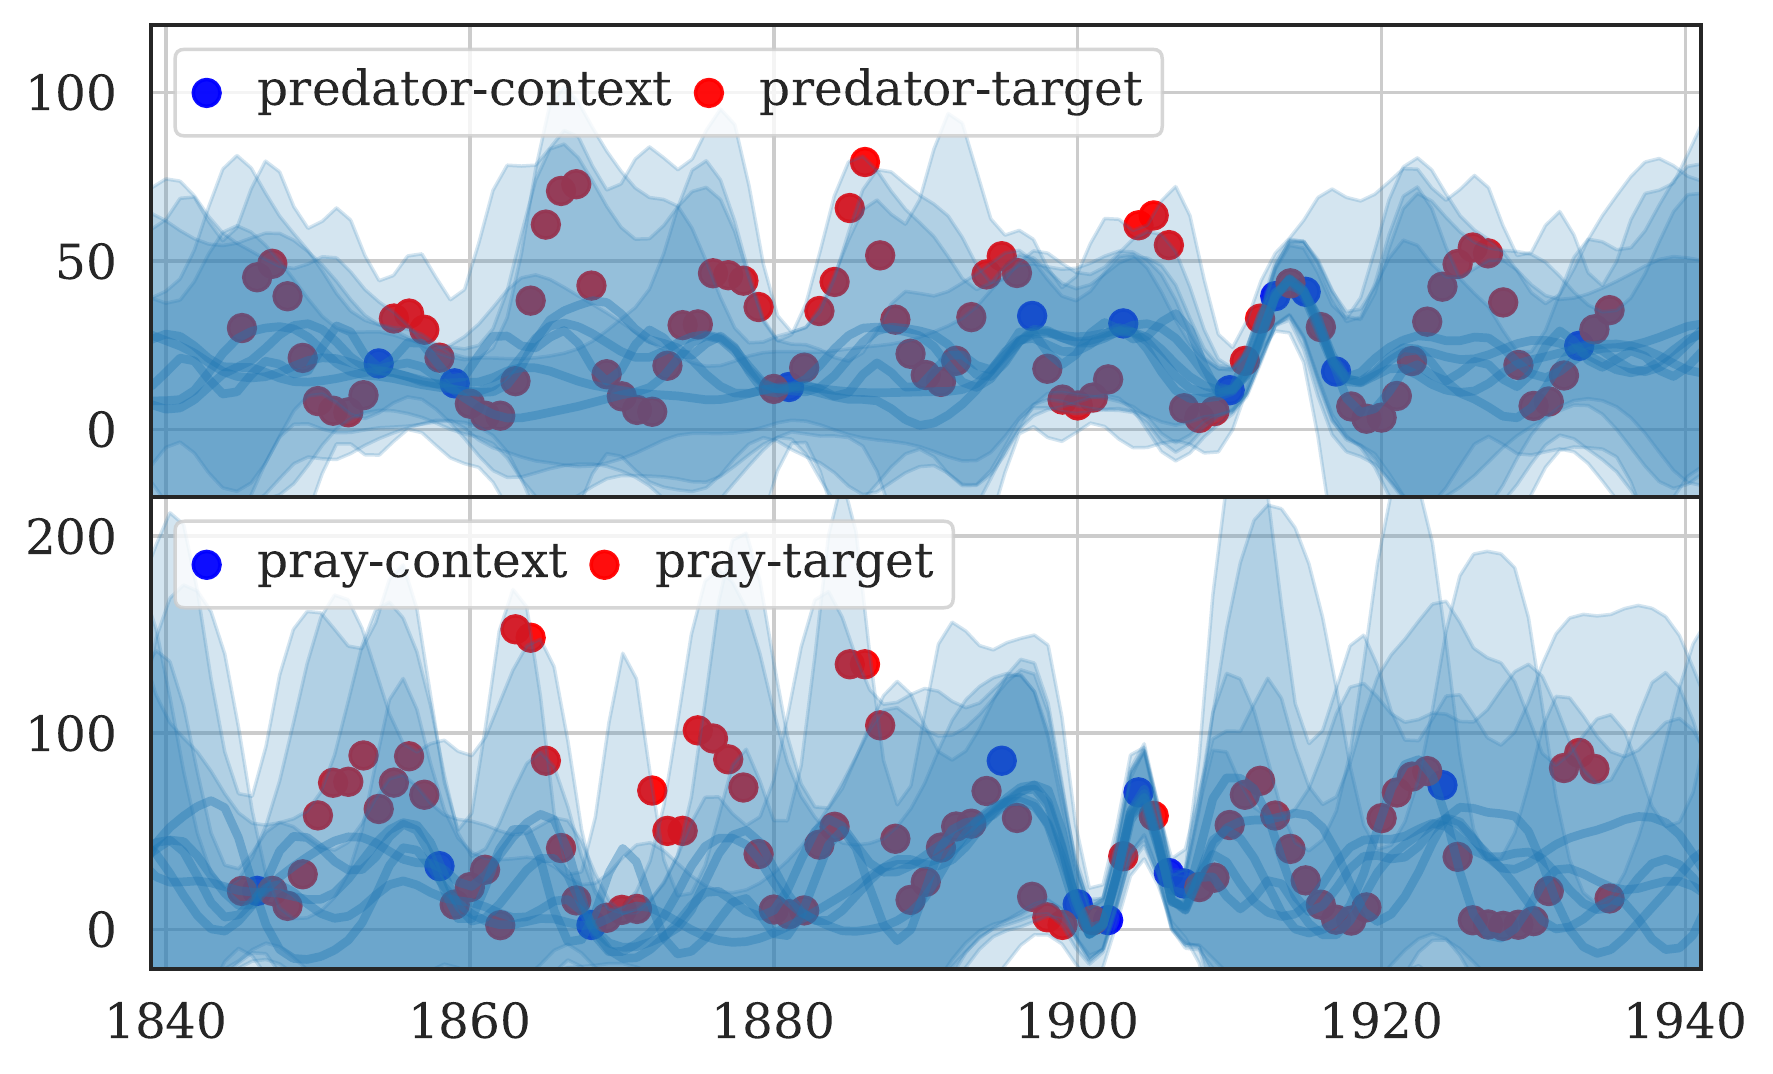}}
 
 \vspace{4mm}
\subfloat[\label{fig:pray-10e} Proposed Model with Task1 ($N^c=10$)]{
 \includegraphics[width=0.49\linewidth]{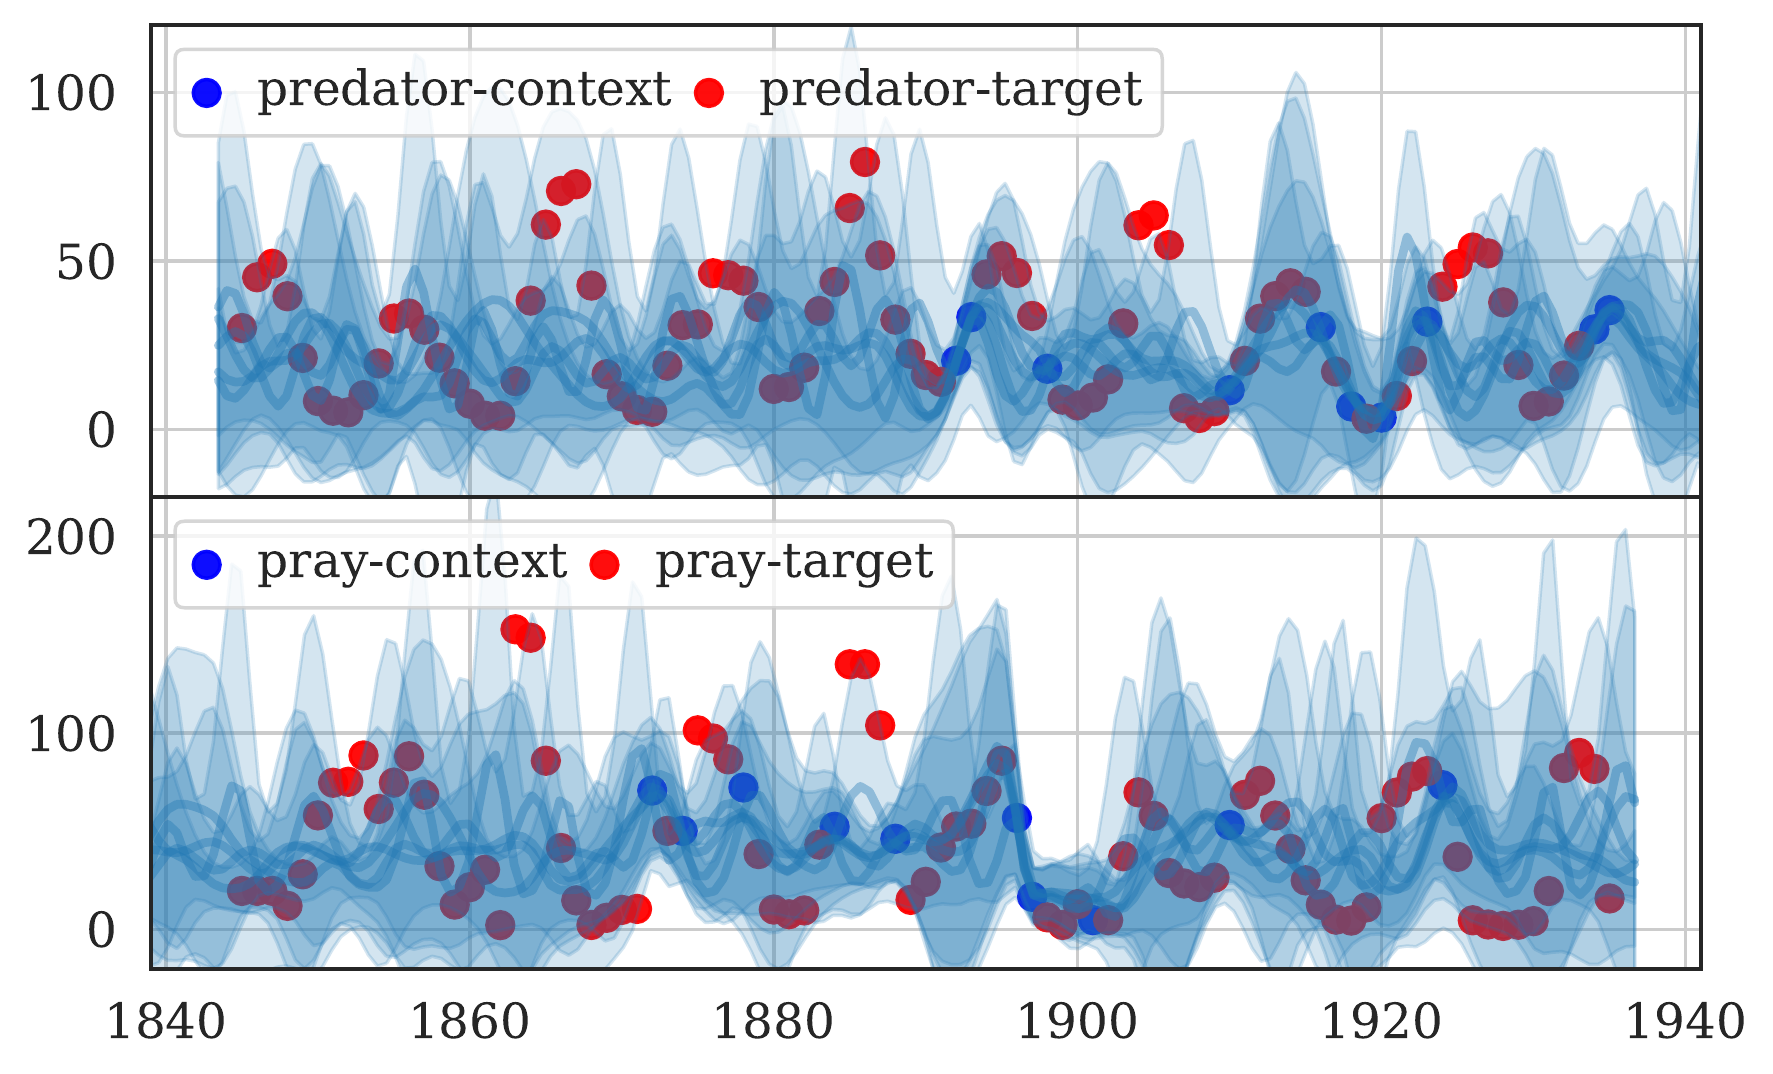}}
\subfloat[\label{fig:pray-10f}Proposed Model with Task2 ($N^c=10$)]{
 \includegraphics[width=0.49\linewidth]{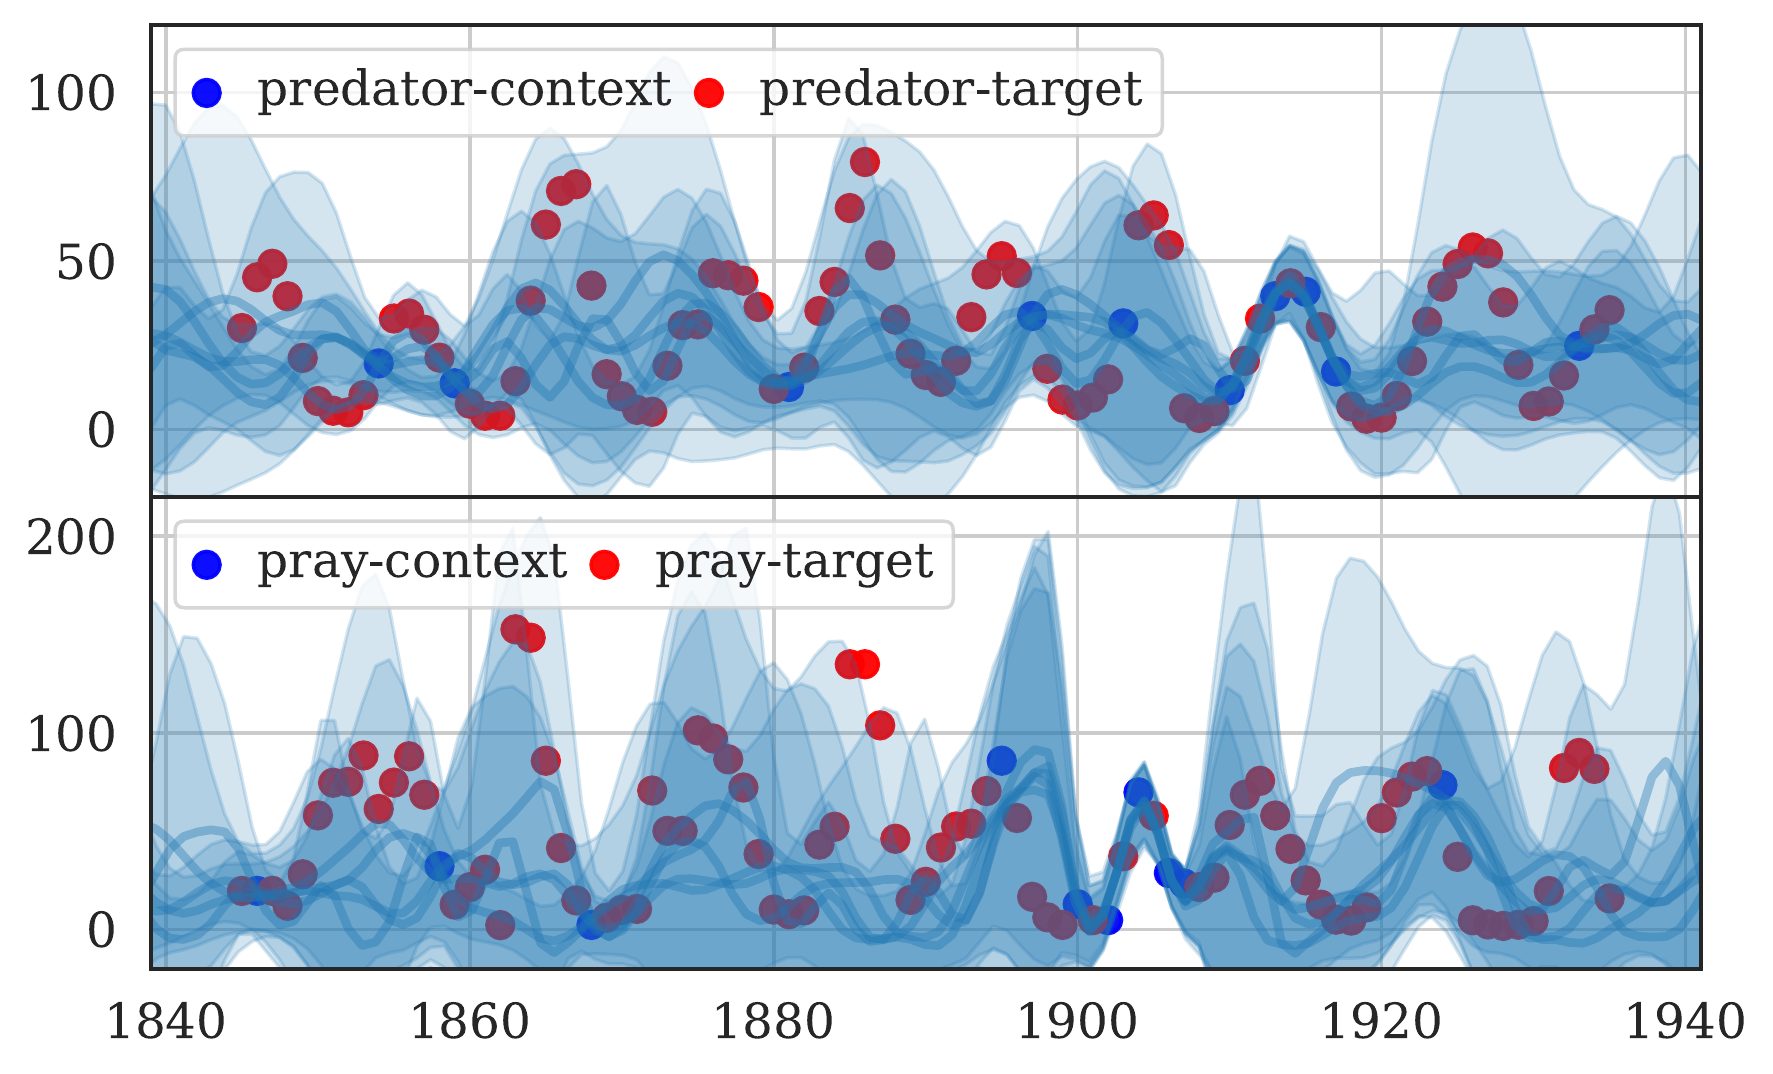}}

\caption{ Prediction results of \textb{Predator-Pray model with 10 context data points ($N^{c}=10$)}; \cref{fig:pray-10a,fig:pray-10b} shows the prediction results of 2 different tasks, respectively. \cref{fig:pray-10c,fig:pray-10d} correspond to the prediction results of GPConvCNP using 5 random functional representations. \cref{fig:pray-10e,fig:pray-10f} correspond to the prediction results of the proposed model using 5 random functional representations. These figures imply that how the random functional representations using prior affect the prediction on target sets when the small number of context data points is given}
\label{fig:predator-pray-10}
\end{figure*}

\vspace{-5mm}
\begin{figure*}[htp!]

% \subfloat[\label{fig:fig-h} \textb{mosm-varying}: $p_{\text{traninv-nn}}(X_c,Y_c)$ ]   
% {\includegraphics[width=0.41\linewidth,height=4.85cm]{Figures/07-appendix-exp2/mosm-varying/mosmvarying_datav11_deptrue_gpdep_weight.pdf}} 
\centering
\subfloat[\label{fig:pray-40a}ConvCNP with Task1 ($N^c=40$)]{
 \includegraphics[width=0.49\linewidth]{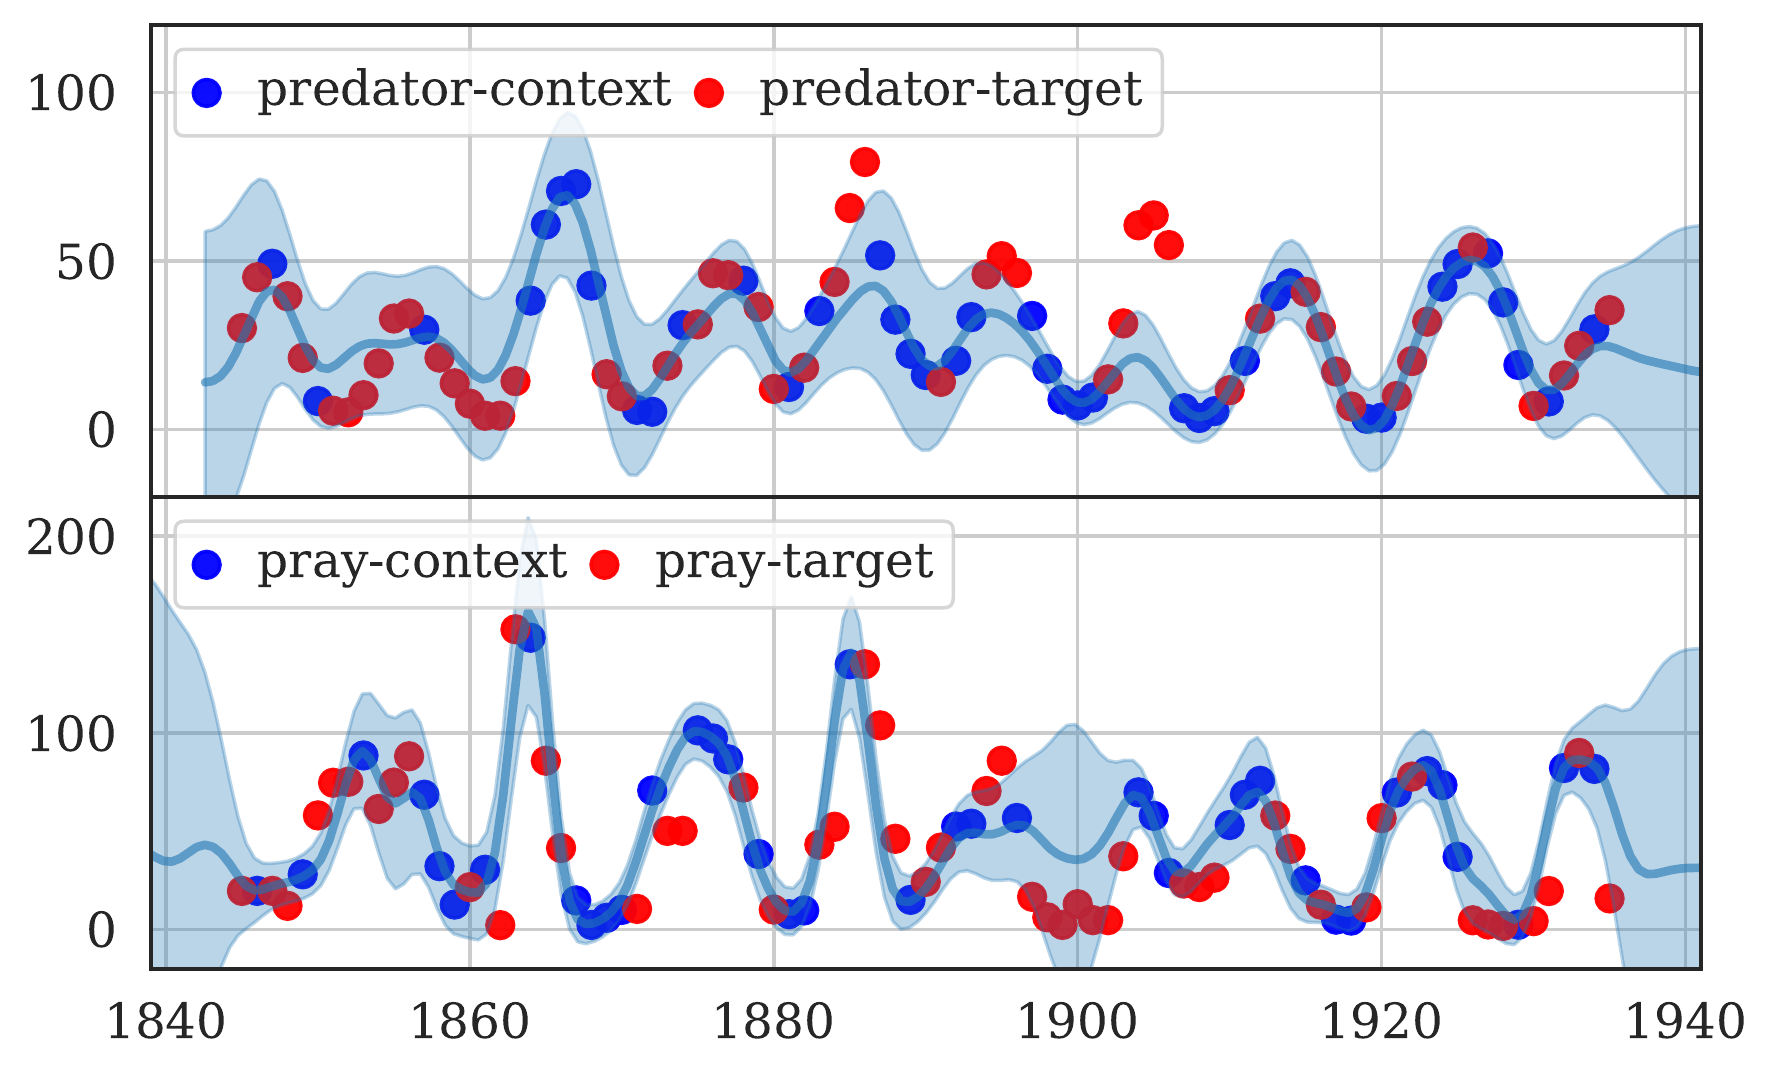}}
\subfloat[\label{fig:pray-40b}ConvCNP with Task2 ($N^c=40$)]{\includegraphics[width=0.49\linewidth]{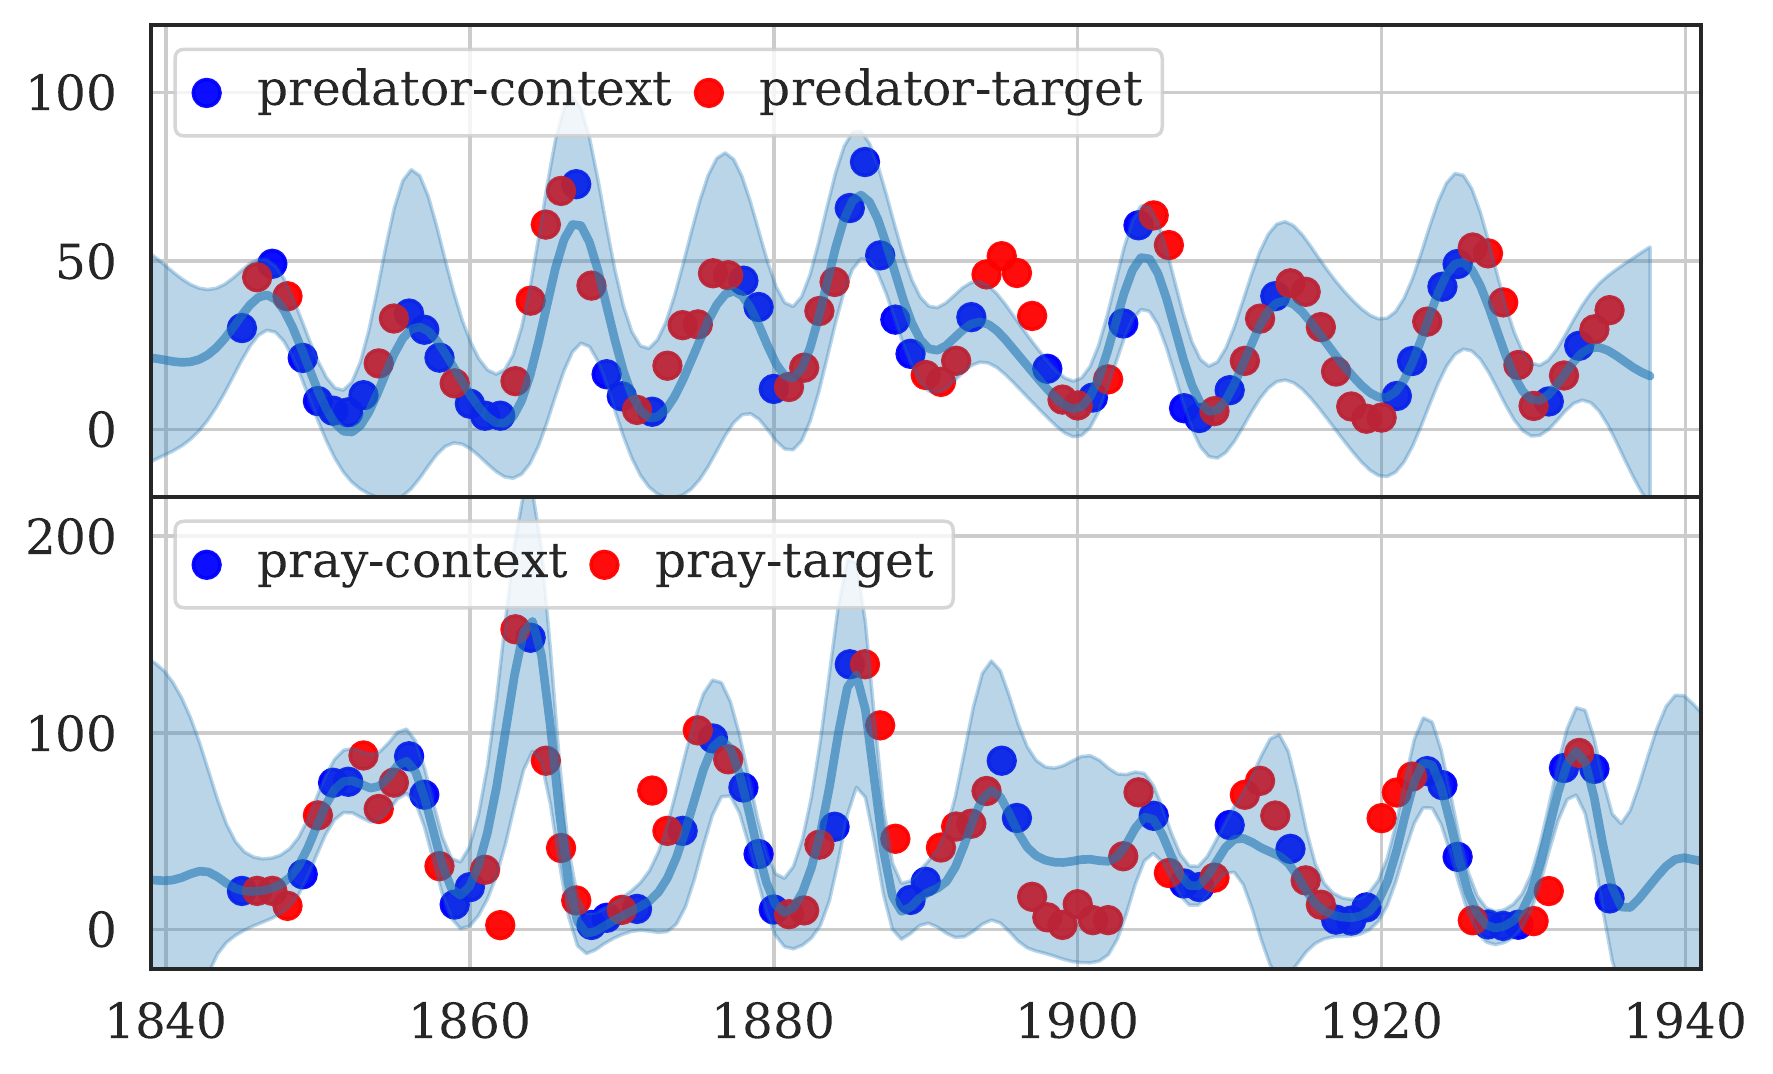}}

 \vspace{4mm}
\subfloat[\label{fig:pray-40c}GPConvCNP with Task1 ($N^c=40$)]{
 \includegraphics[width=0.49\linewidth]{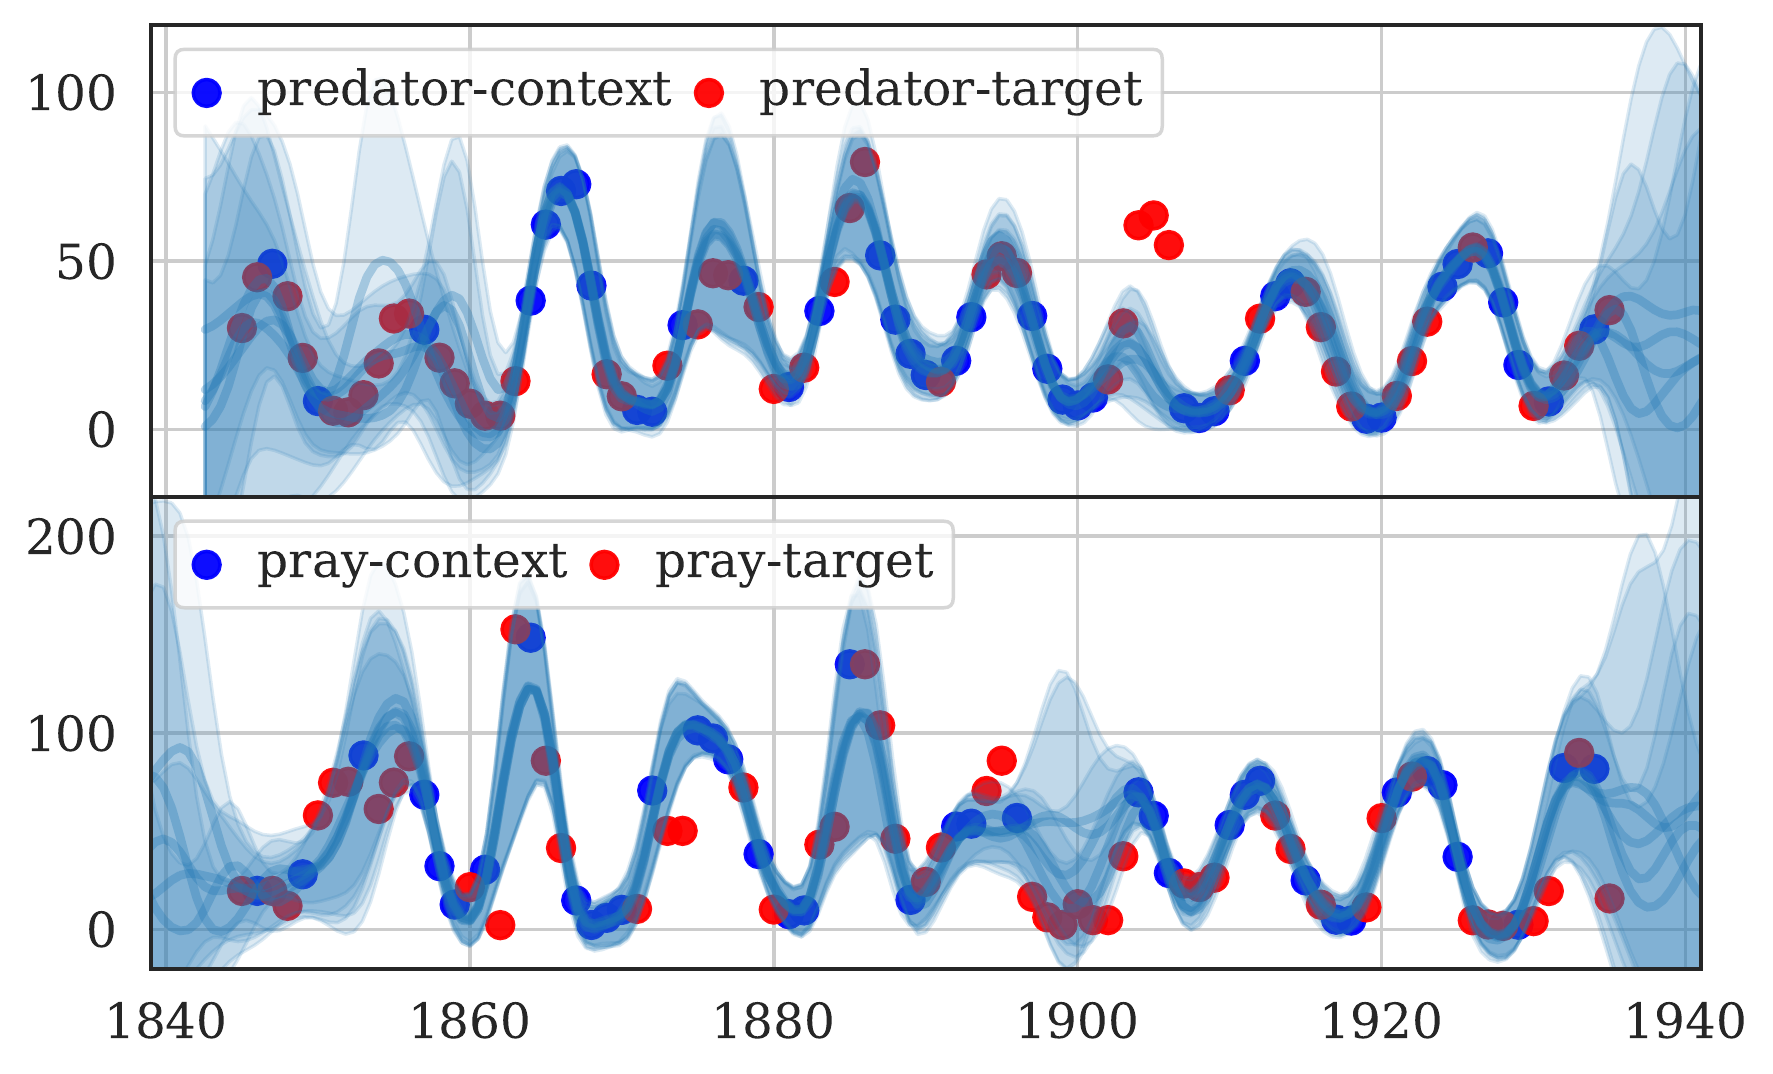}}
\subfloat[\label{fig:pray-40d}GPConvCNP with Task2 ($N^c=40$)]{
 \includegraphics[width=0.49\linewidth]{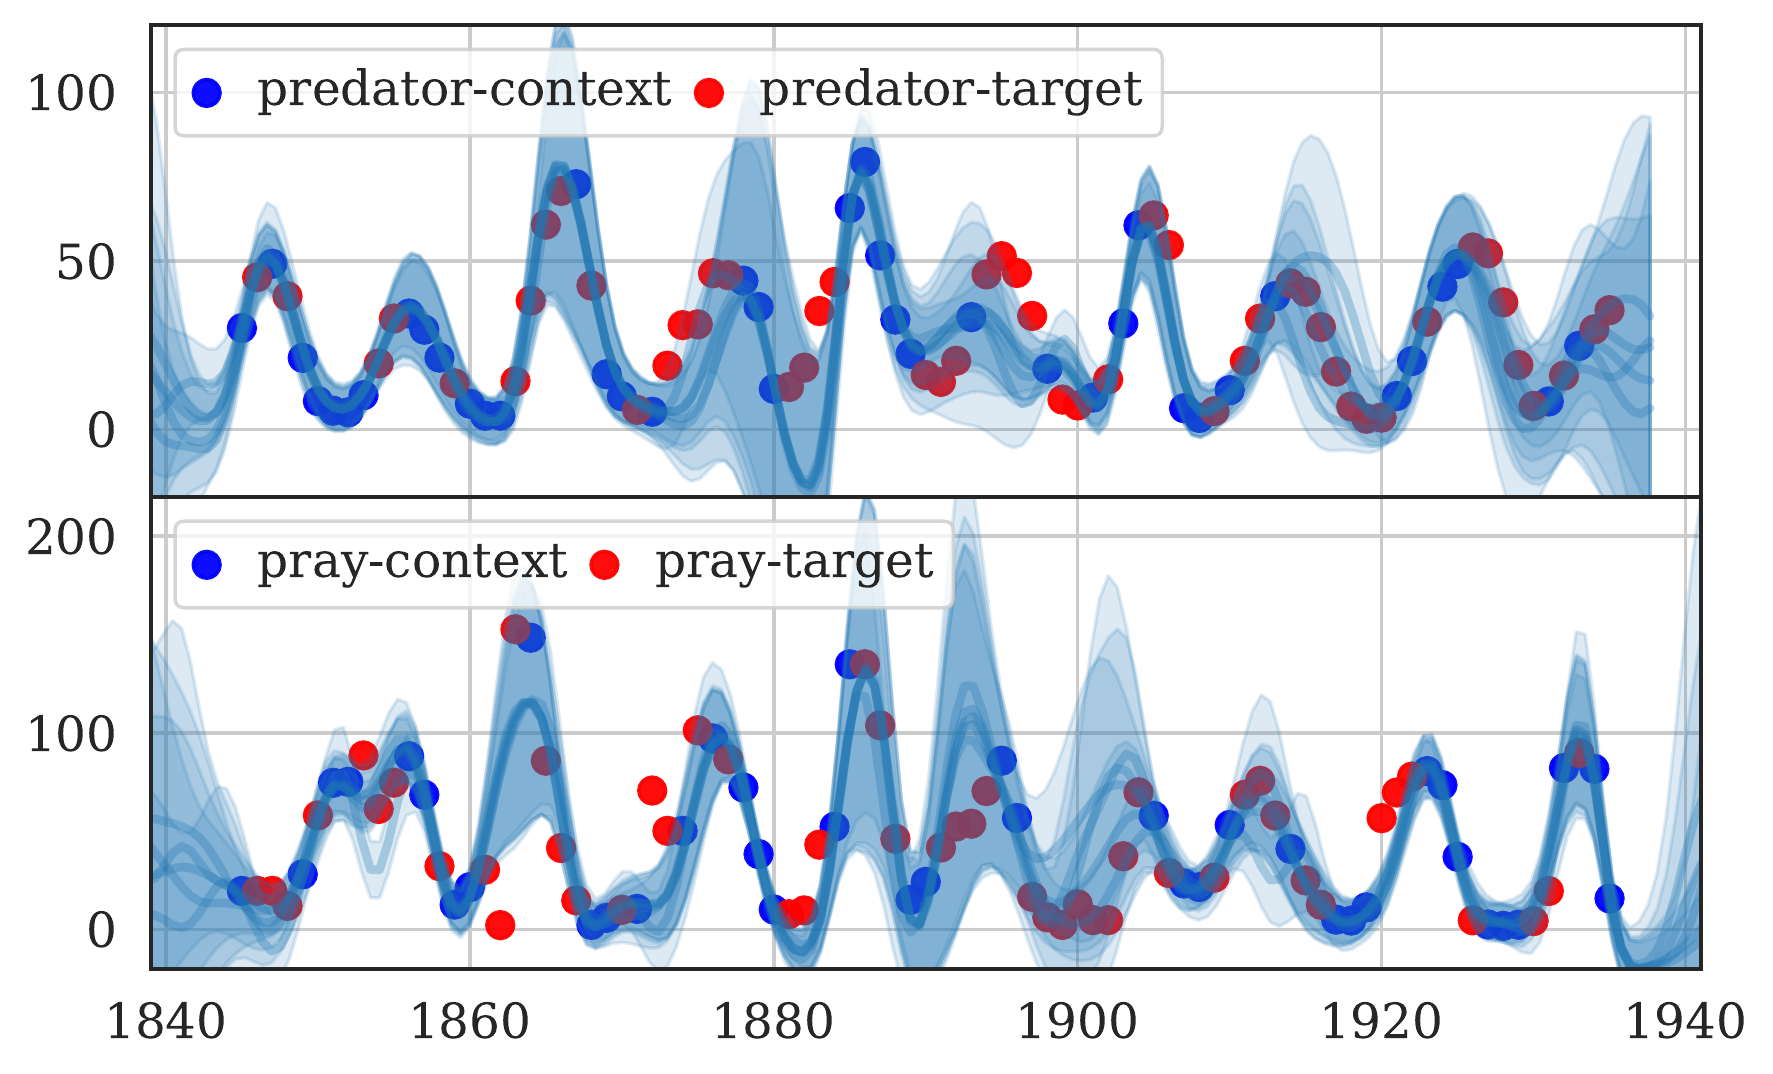}}
 
 \vspace{4mm}
\subfloat[\label{fig:pray-40e}Proposed Model with Task1 ($N^c=40$)]{
 \includegraphics[width=0.49\linewidth]{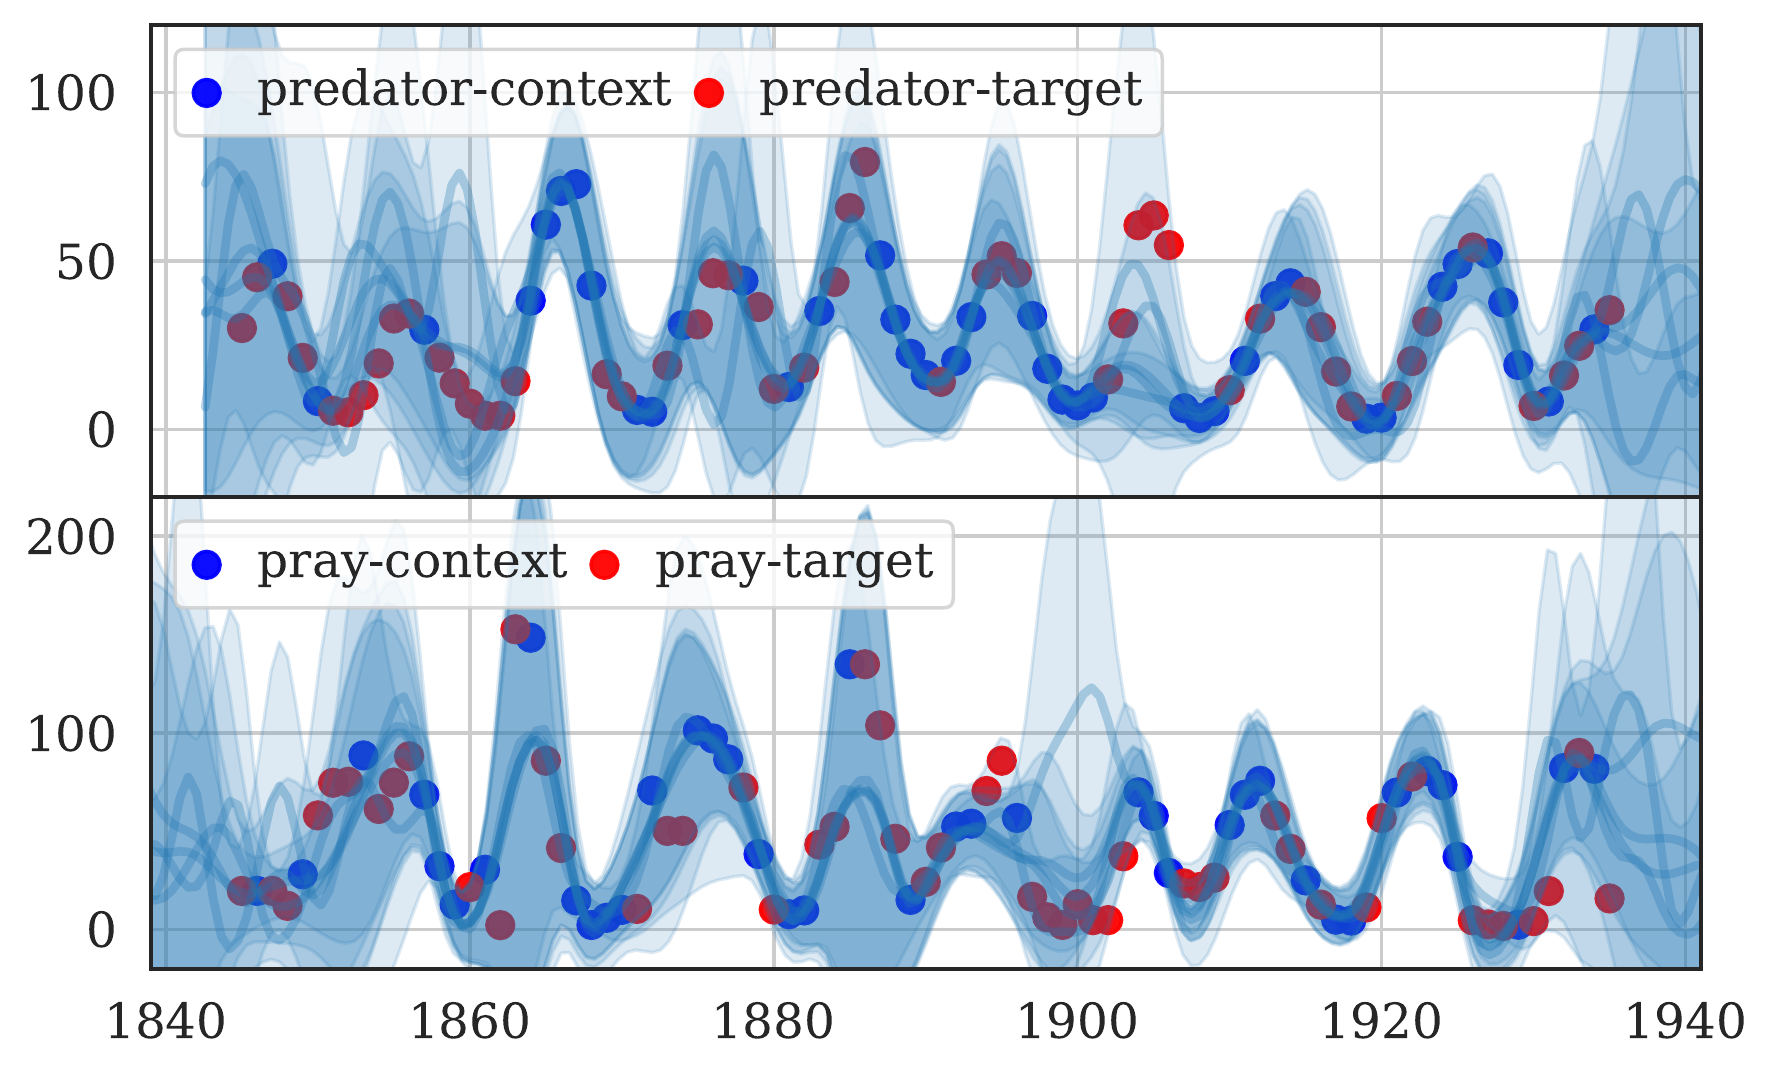}}
\subfloat[\label{fig:pray-40f}Proposed Model with Task2 ($N^c=40$)]{
 \includegraphics[width=0.49\linewidth]{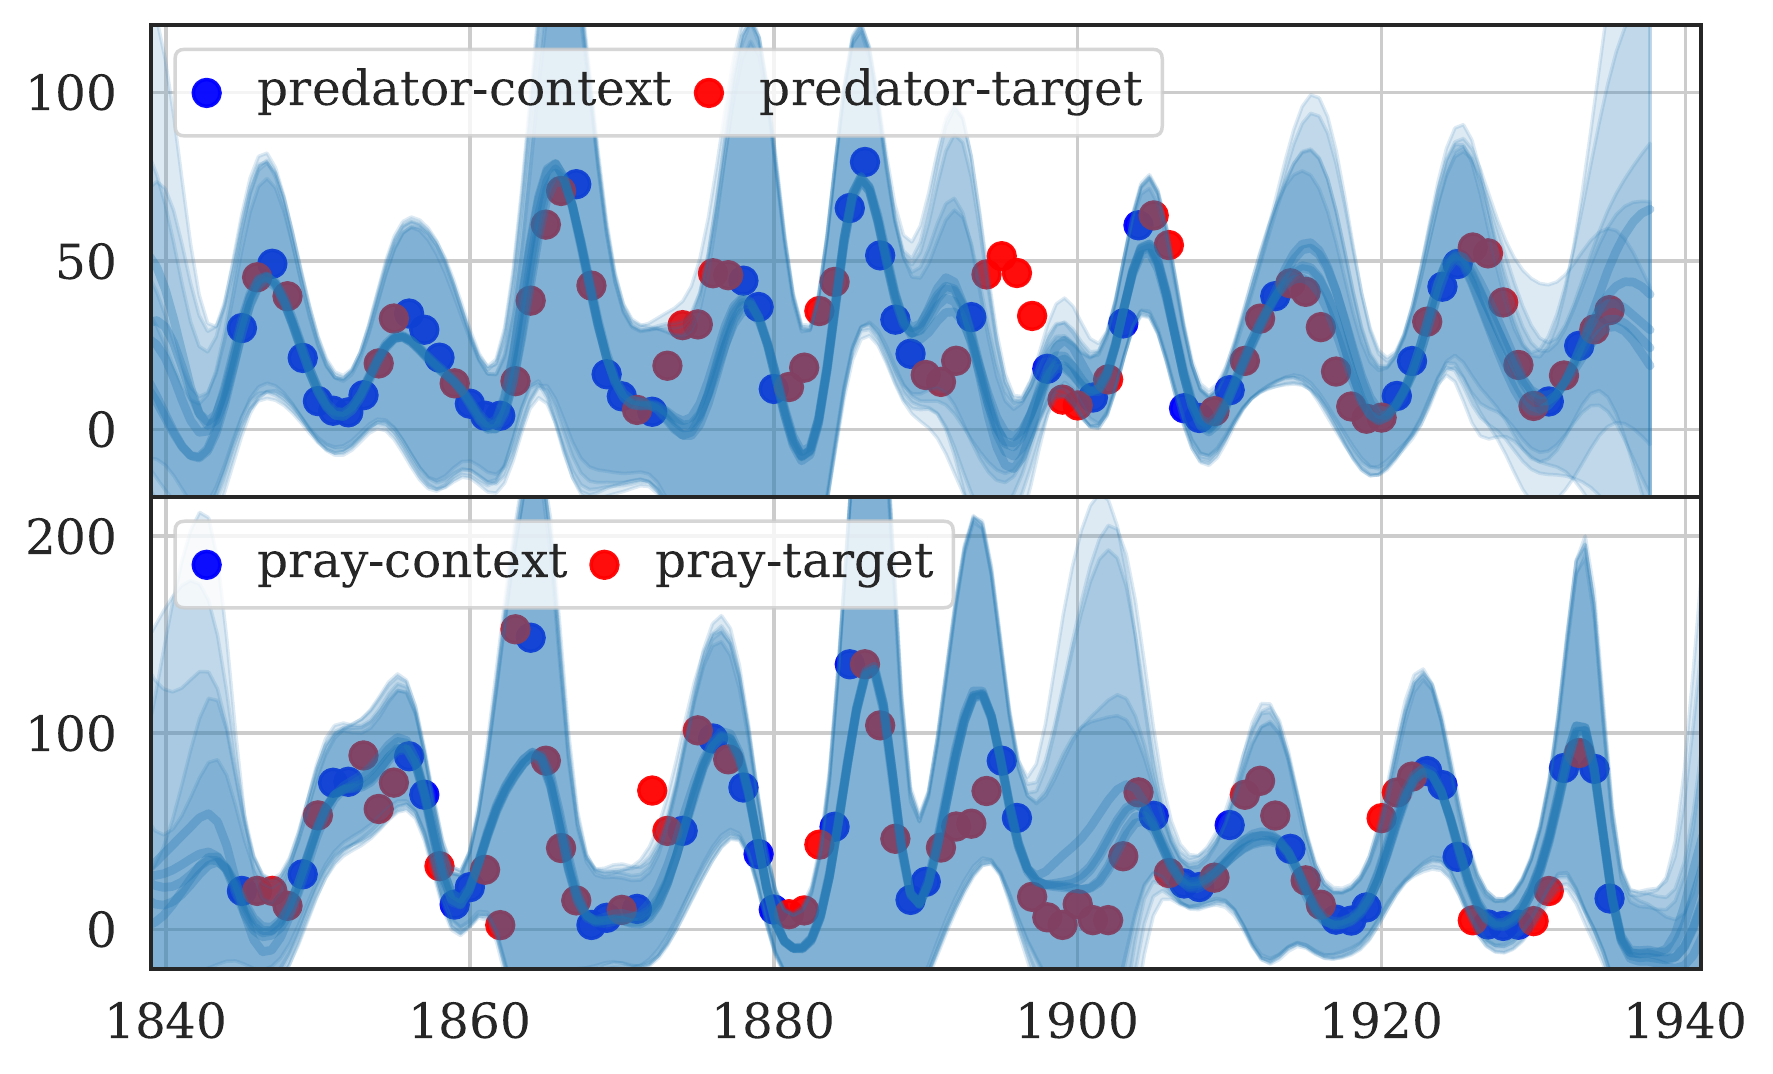}}

\caption{ Prediction results of \textb{Predator-Pray model with 40 context data points ($N^{c}=40$)}; \cref{fig:pray-40a,fig:pray-40b} shows the prediction results of 2 different tasks, respectively. \cref{fig:pray-40c,fig:pray-40d} correspond to the prediction results of GPConvCNP using 5 random functional representations. \cref{fig:pray-40e,fig:pray-40f} correspond to the prediction results of the proposed model using 5 random functional representations. These figures imply the task-dependent prior enables more robust predictions as shown in \cref{fig:pray-40e,fig:pray-40f} compared to GPConvCNP as shown in \cref{fig:pray-40c,fig:pray-40d}}
\label{fig:predator-pray-40}
\end{figure*}

\vspace{-5mm}
\begin{figure*}[htp!]

% \subfloat[\label{fig:fig-h} \textb{mosm-varying}: $p_{\text{traninv-nn}}(X_c,Y_c)$ ]   
% {\includegraphics[width=0.41\linewidth,height=4.85cm]{Figures/07-appendix-exp2/mosm-varying/mosmvarying_datav11_deptrue_gpdep_weight.pdf}} 
\centering
\subfloat[\label{fig:pray-70a} ConvCNP with Task1 ($N^c=70$)]{
 \includegraphics[width=0.49\linewidth]{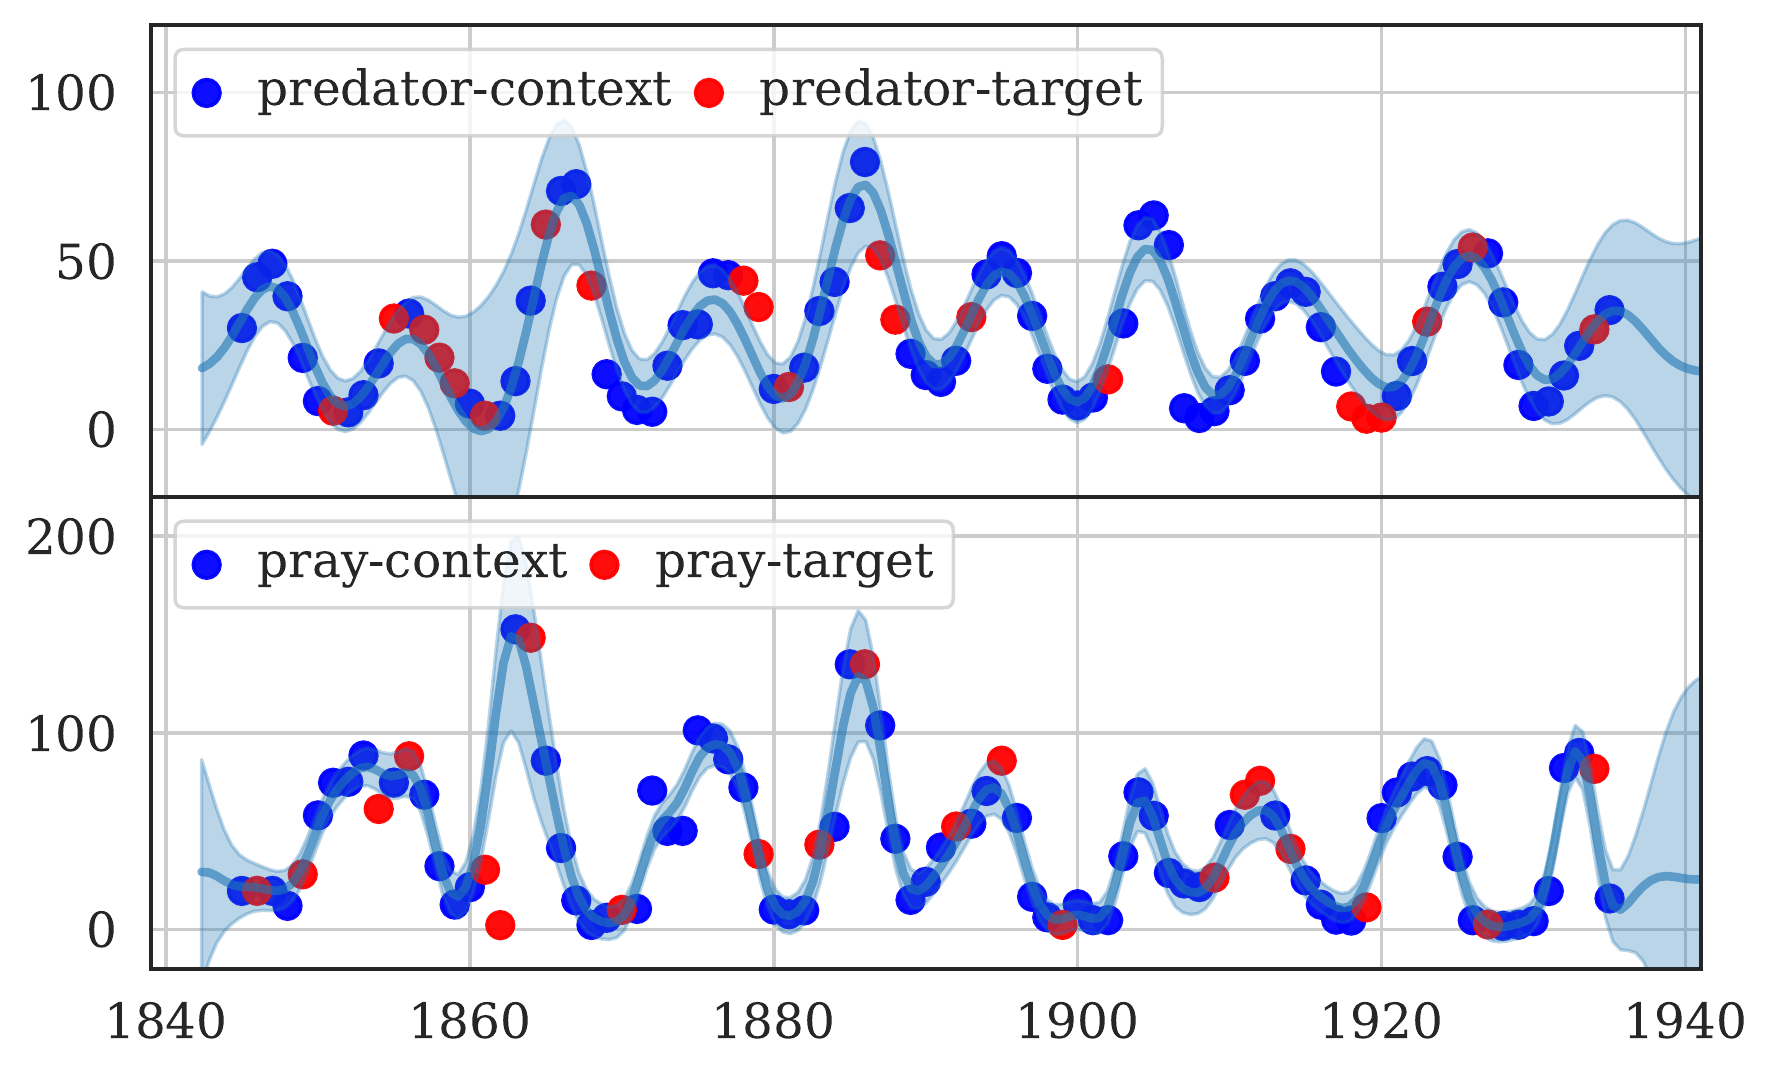}}
\subfloat[\label{fig:pray-70b} ConvCNP with Task2 ($N^c=70$)]{\includegraphics[width=0.49\linewidth]{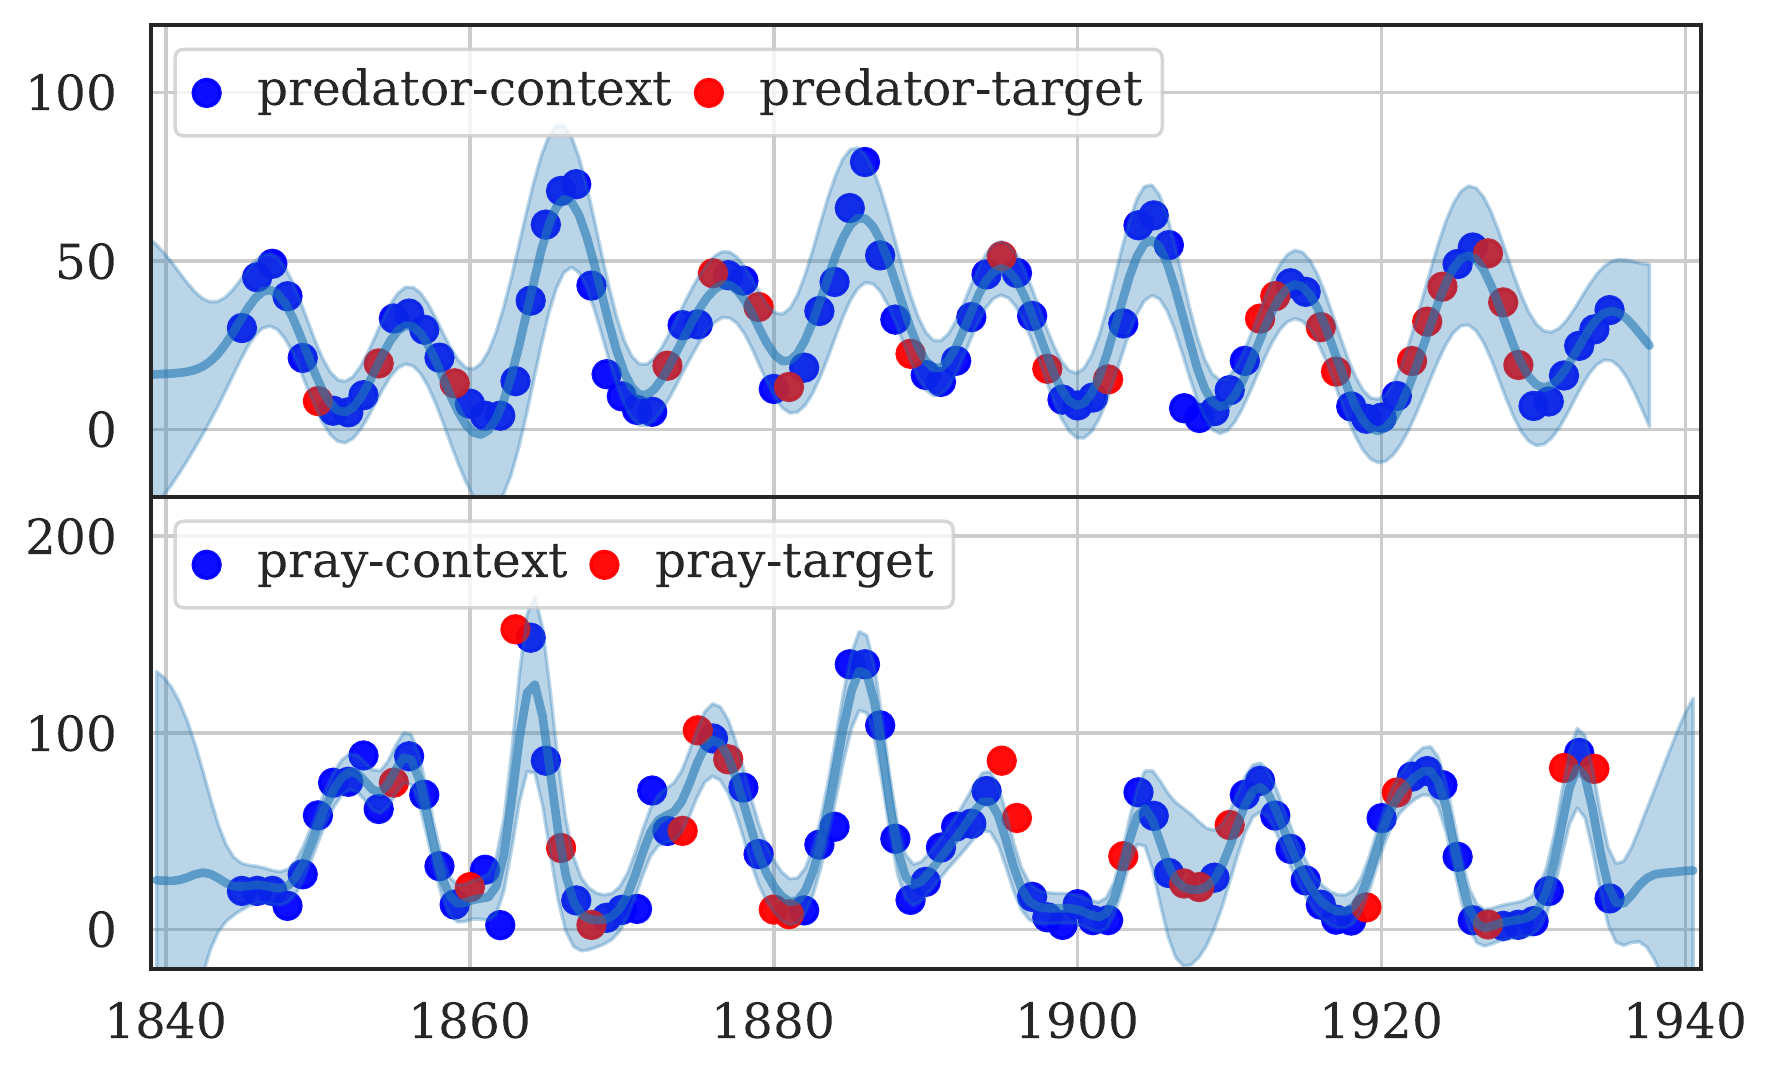}}

 \vspace{4mm}
\subfloat[\label{fig:pray-70c} GPConvCNP with Task1 ($N^c=70$)]{
 \includegraphics[width=0.49\linewidth]{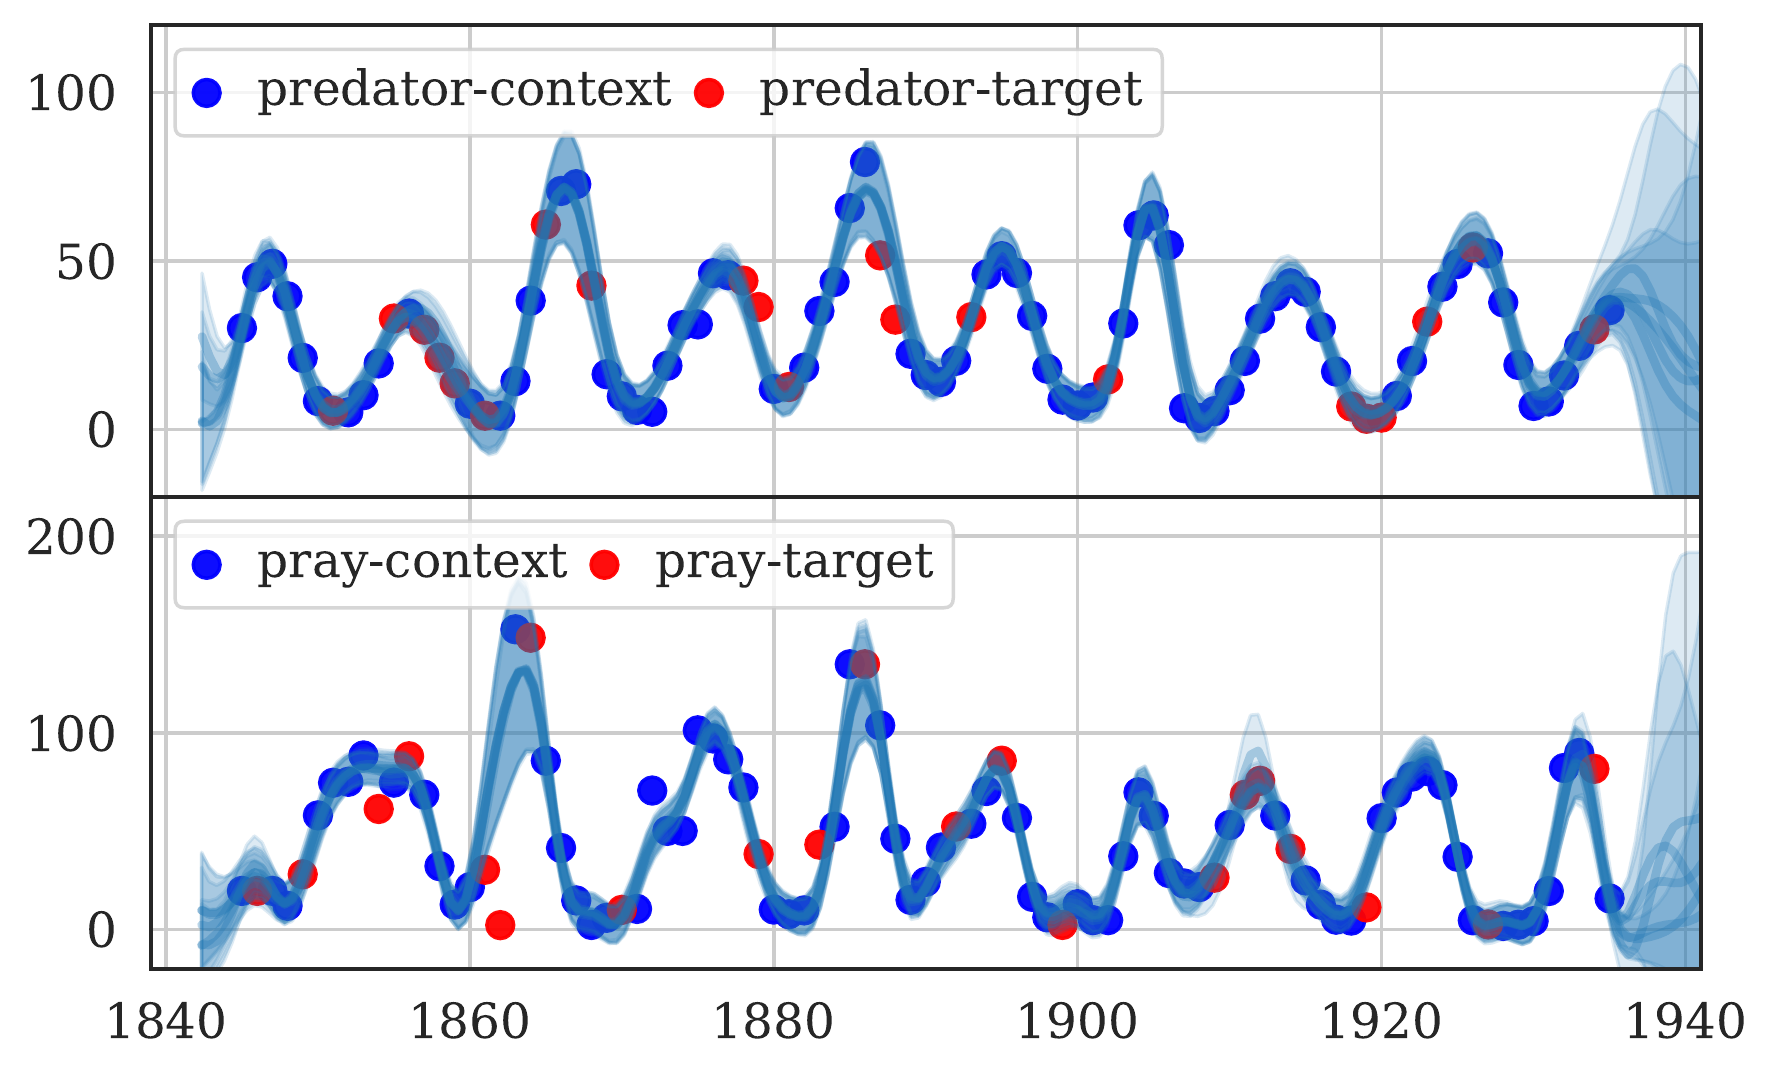}}
\subfloat[\label{fig:pray-70d} GPConvCNP with Task2 ($N^c=70$)]{
 \includegraphics[width=0.49\linewidth]{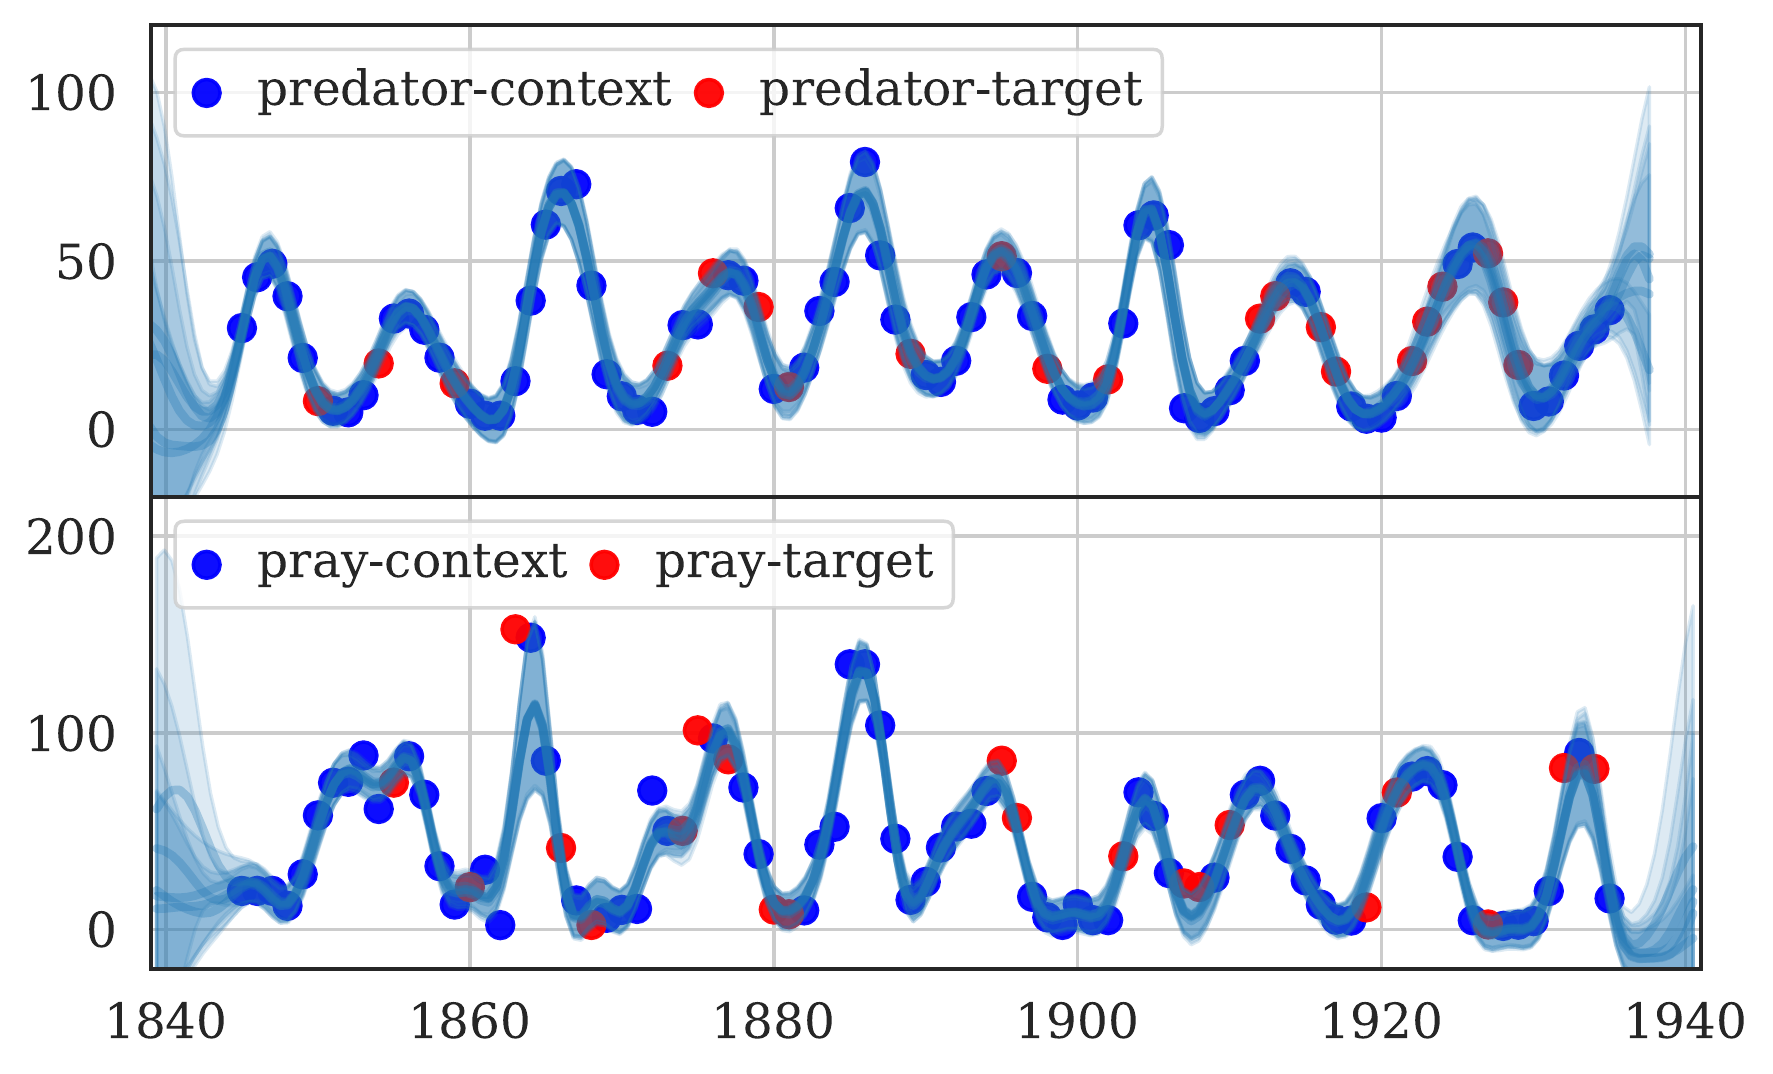}}
 
 \vspace{4mm}
\subfloat[\label{fig:pray-70e}Proposed Model with Task1 ($N^c=70$)]{
 \includegraphics[width=0.49\linewidth]{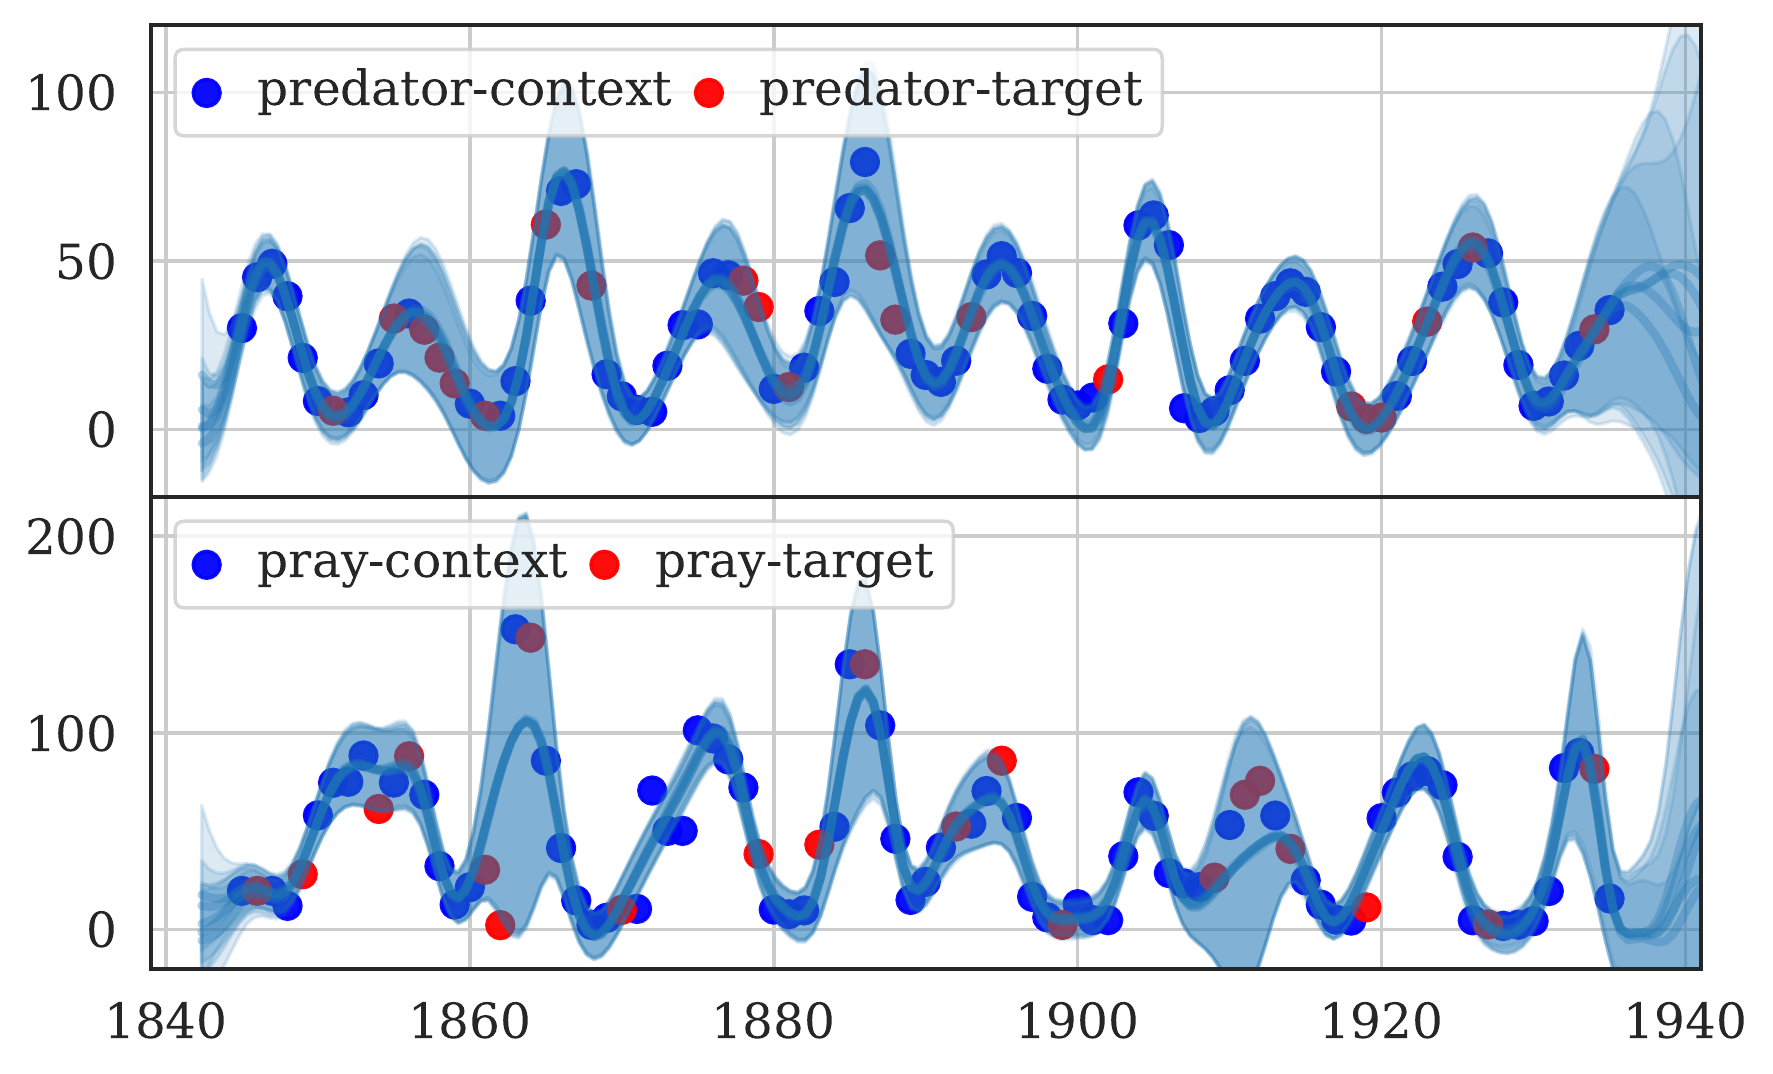}}
\subfloat[\label{fig:pray-70f}Proposed Model with Task2 ($N^c=70$)]{
 \includegraphics[width=0.49\linewidth]{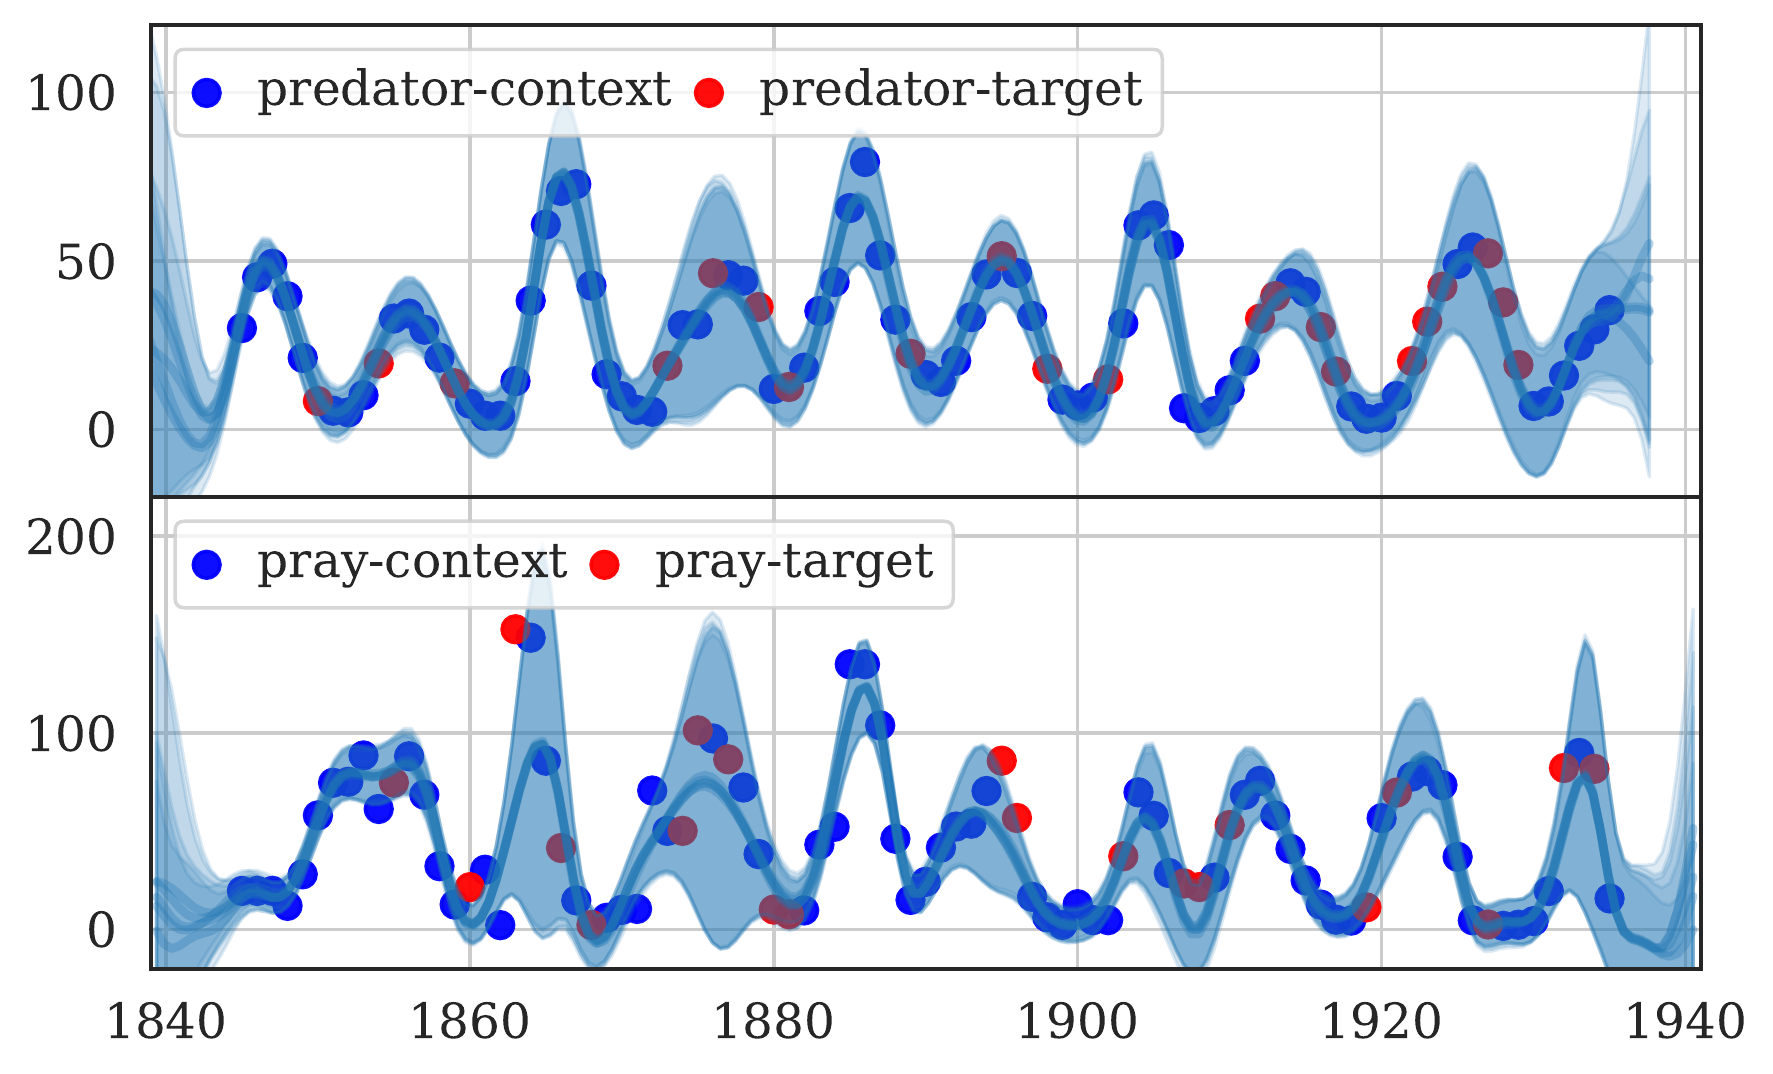}}

\caption{Prediction results of \textb{Predator-Pray model with 70 context data points ($N^{c}=70$)}; \cref{fig:pray-70a,fig:pray-70b} shows the prediction results of 2 different tasks, respectively. \cref{fig:pray-70c,fig:pray-70d} correspond to the prediction results of GPConvCNP using 5 random functional representations. \cref{fig:pray-70e,fig:pray-70f} correspond to the prediction results of the proposed model using 5 random functional representations. These figures imply  that all models obtain similar predictive distribution on target sets when the large number of context data points is given.}
\label{fig:predator-pray-70}
\end{figure*}
