# Supplementary material for: Bayesian Convolutional Deep Sets with Task-Dependent Stationary Prior
Source: arXiv:2210.12363 source file (2022-10-22)
Supplement: Supplementary file 18 [file 07-appendix-v01-chapter5-exp4.tex]

%\subsection{Additional Experimental Results}

%\subsection{Further Details for the Predator-Pray model}
\section{Further Details for Image Completion Task}

\subsection{Details for Datasets}
For image completion task, each task is defined to predict the randomly chosen pixel values of image when using given partial pixel values as context set. To do this, we use a subset of monthly land surface temperature set used in \citeb{remes2017non}. We use the surface temperature of North America ($53{\times}115{\times}3$) and Europe ($78{\times}102{\times}3$).

% For each task, we set that $N^c$ context points and $N^{t}$ target points is proportional to the size of image by choosing a small context rate $p \in \{.01,.05,.10,.20\}$ randomly with probability $[4/10,3/10,2/10,1/10]$. This is indented to investigate how NP models predict the image of temperature when NP models are trained with each context set $D^{c}$ having the the small number $N^{c}$ of context points.

\subsection{Details for Tasks of Training, Validation, and Test }

We use the datasets (2018 - 2020) for the training, and datasets (2021) for the test. 

For training, we randomly sample the context and target set by choosing a small context rate $p \in \{.01,.05,.10,.20\}$ randomly with probability \textb{$[4/10,3/10,2/10,1/10]$}. We use \textb{$2500 \times 5$} tasks for training, and \textb{$256 \times 4$ } tasks as validation set.

For test, we set the varying context rate \textb{$p \in \{.01,.05,.10,.20\}$} as done in training phase, and set target set by choosing a target rate \textb{$p=.5$} We use each \textb{$256$ } tasks per context rate \textb{$p \in \{.01,.05,.10,.20\}$} to evaluate the trained models.

\subsection{Details for Hyperparameters.}

%\paragraph{Hyperparameters of proposed method.}

For stationary kernels, we set $\mu_{1}=[0.0,0.0]$ and $\sigma_{1}=[0.5,0.5]$ for $Q=1$.

For $Q=4$, we set $\mu_{1}=[0.0,0.0],\mu_{2}=[2.0,0.0],\mu_{3}=[0.0,2.0],$ and $\mu_{4}=[2.0,2.0]$ and $\sigma_{q}=[0.5,0.5]$ for $q=1,..,4$.

For the number of spectral points, we use $l=10$ in \textb{Eq. (14)}.

For the number of sample function, we use $N=4$ in \textb{Eq. (19)}.

For the prior hyperparameter of approximate scheme $\alpha$, we use $\alpha \in \{.05,0.1\}$.

For training, we  use ADAM optimizer \citeb{kingma2014adam} with learning rate $5e\text{-}4$ and weight decay $1e\text{-}4$. 

For the regularizer hyperparameter $\beta$ in \textb{Eq. (21)}, we set $\beta=0.1$ for the proposed method.

% \paragraph{Hyperparameters for Training.} We use ADAM optimizer \citeb{kingma2014adam} with learning rate $5e\text{-}4$ and weight decay $1e\text{-}4$. For the regularizer hyperparameter $\beta$ in \textb{Eq. (21)}, we set $\beta=0.1$.

% \subsection{Baseline Implementations}
% For ConvCNP and the proposed model, we use the shallow 2d CNN described in \cref{subsubsec:cnnstructure} for all models

\subsection{Additional Results}
%fig:predator-pray-70

We report additional prediction results for image completion tasks of North America dataset in \cref{fig:image_completion-usa-a}.
\begin{figure*}[h]
\centering
% {\includegraphics[width=0.975\linewidth,height=5cm]{Figures/05-experiments-task03/tempusa_gpdep_Q2_p0.050.2.pdf}}  
{\includegraphics[width=0.95\linewidth,height=4.5cm]{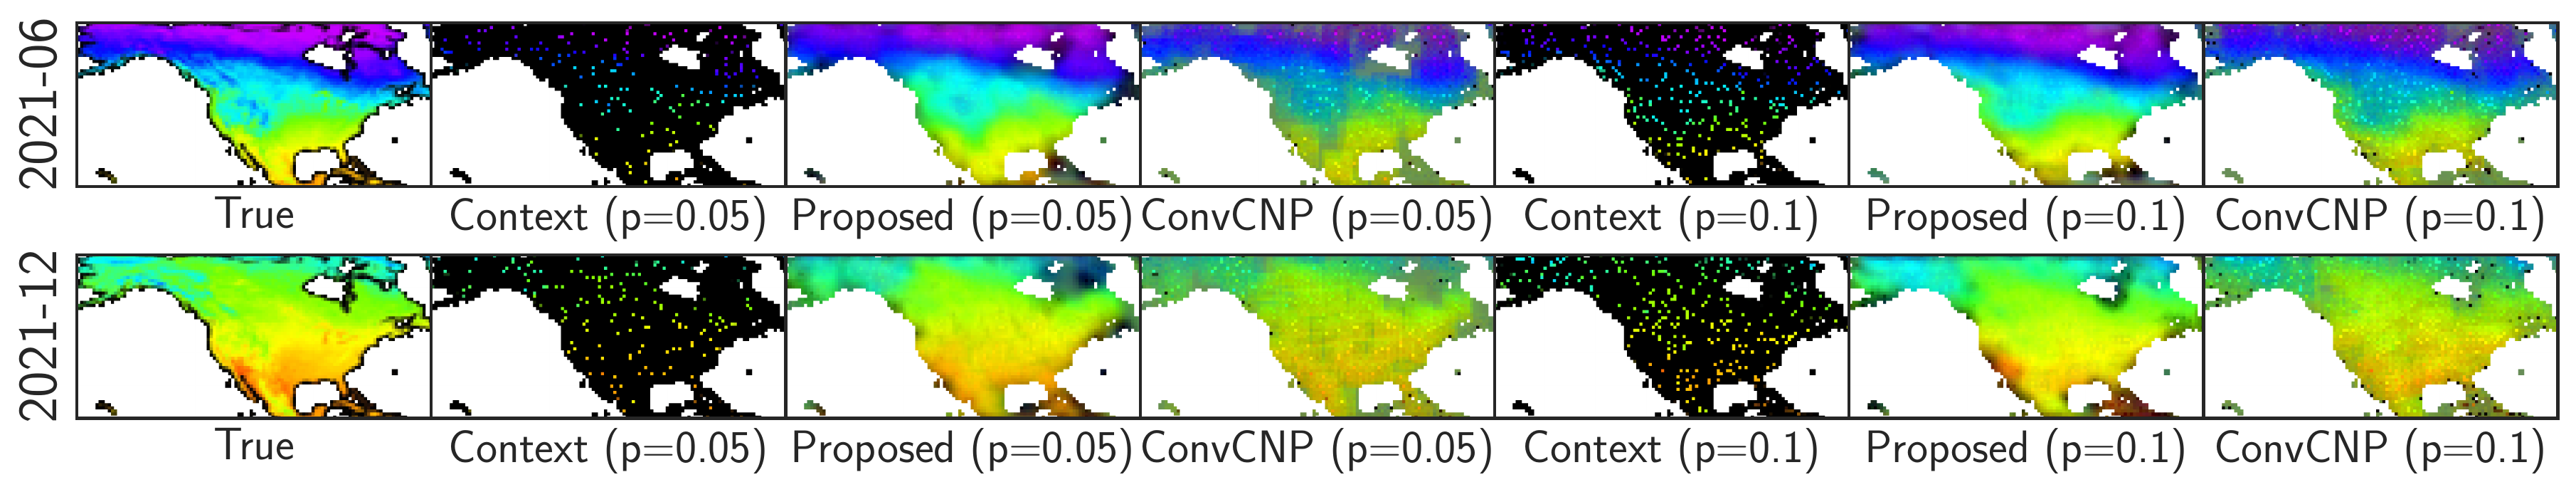}}  
\caption{Prediction results for North America temperatures (June 2021 and December 2021) that are out of training sets.}
\label{fig:image_completion-usa-a}
\end{figure*}

Additionally, we report the progress of the test log likelihood during training phase in \cref{fig:exp5-3:smallset-usa-progress,fig:exp5-3:smallset-eu-progress}. These figures compare the prediction improvement of the models depending on the number of used training tasks.

\cref{fig:exp5-3:small-a,fig:exp5-3:small-b,fig:exp5-3:small-c,fig:exp5-3:small-d} shows the test log likelihood on the dataset of North America (2018-2020) over varying training tasks $\{2500,5000,7500,10000\}$. \cref{fig:exp5-3:small-e,fig:exp5-3:small-f,fig:exp5-3:small-g,fig:exp5-3:small-h} shows the corresponding results on the dataset of North America (2021).

With the same protocol of North America experiment results,  \cref{fig:exp5-3:small-a2,fig:exp5-3:small-b2,fig:exp5-3:small-c2,fig:exp5-3:small-d2} shows the corresponding results on Europe temperature (2018-2020), and \cref{fig:exp5-3:small-e2,fig:exp5-3:small-f2,fig:exp5-3:small-g2,fig:exp5-3:small-h2} shows the corresponding results on Europe temperature (2018-2020),

\vspace{-3mm}
\begin{figure}[H]
%\begin{figure}[htp!]
\centering
\subfloat[ \label{fig:exp5-3:small-a}  2500 tasks (in-train)]
{\includegraphics[width=0.24\linewidth]{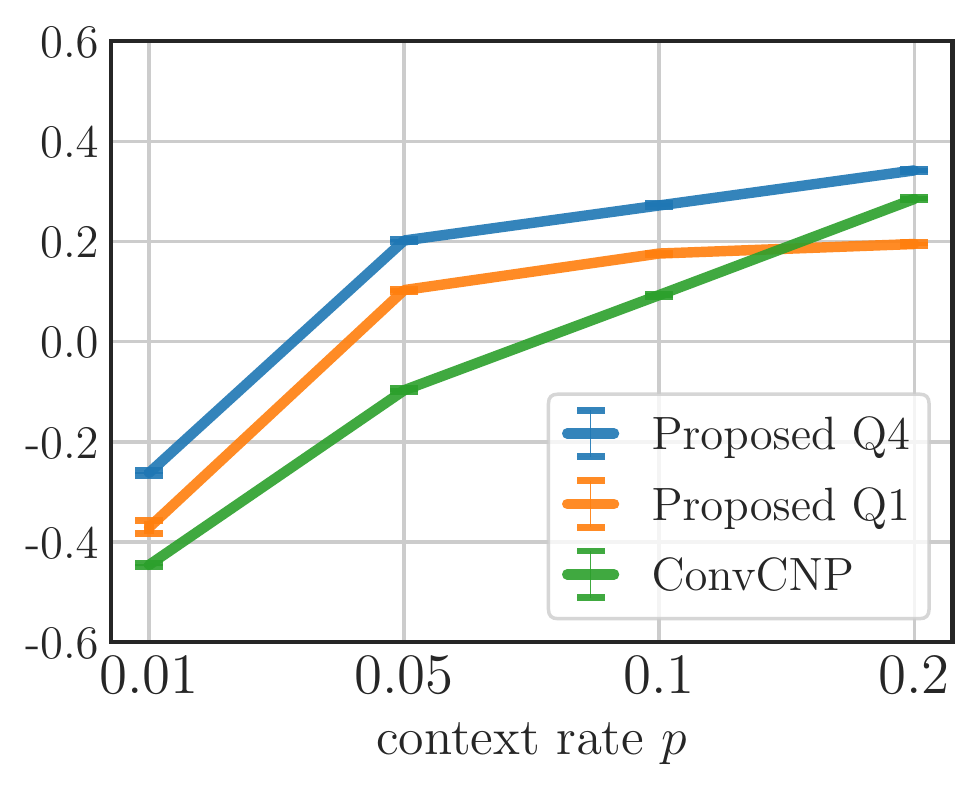}}   \hspace{0.5mm} 
\subfloat[ \label{fig:exp5-3:small-b} 5000 tasks (in-train)] 
{\includegraphics[width=0.24\linewidth]{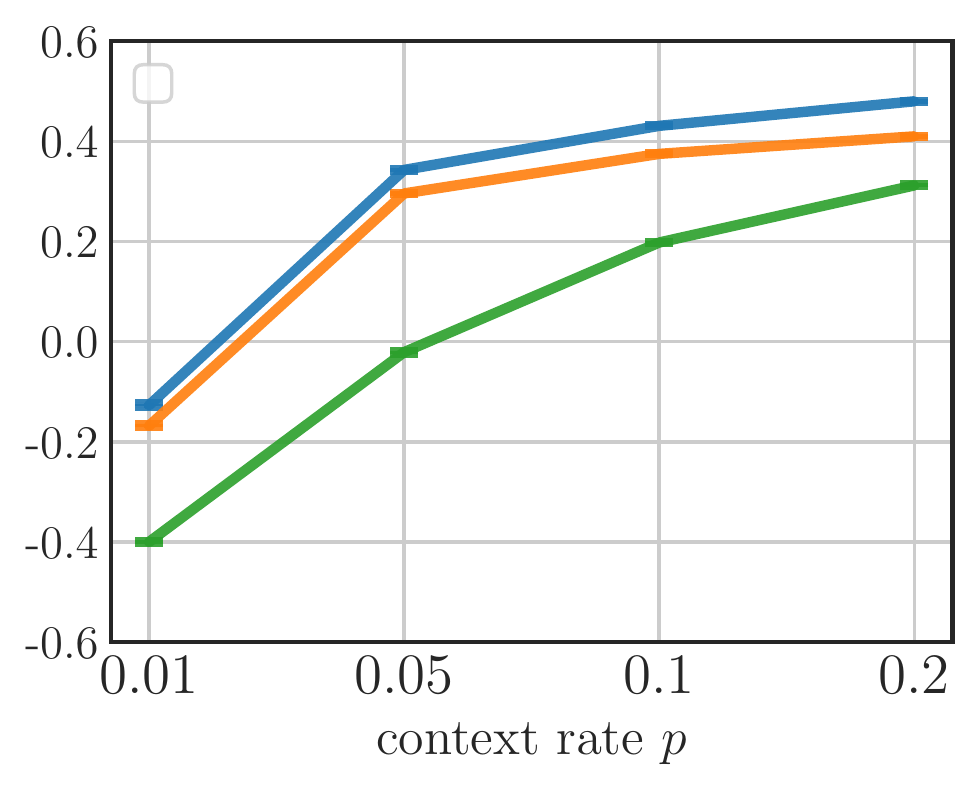}}   \hspace{0.5mm} 
\subfloat[ \label{fig:exp5-3:small-c} 7500 tasks (in-train) ]
{\includegraphics[width=0.24\linewidth]{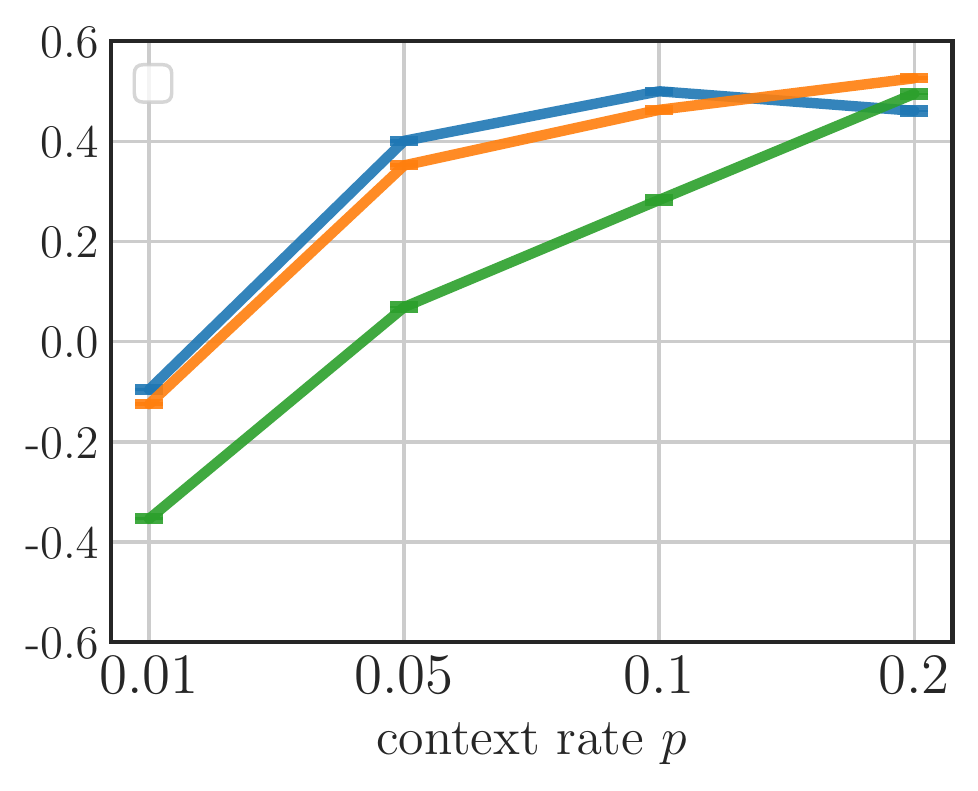}}  \hspace{0.5mm} 
\subfloat[ \label{fig:exp5-3:small-d} 10000 tasks (in-train) ]
{\includegraphics[width=0.24\linewidth]{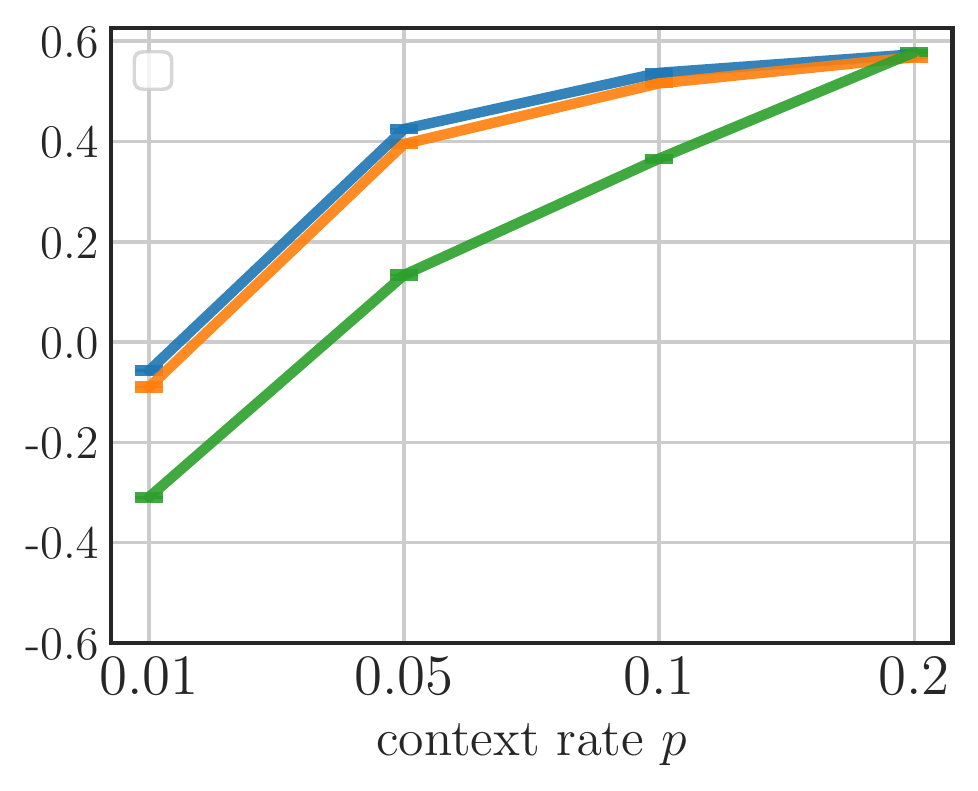}}

\vspace{2mm}
\subfloat[ \label{fig:exp5-3:small-e}  2500 tasks (out-train)]
{\includegraphics[width=0.24\linewidth]{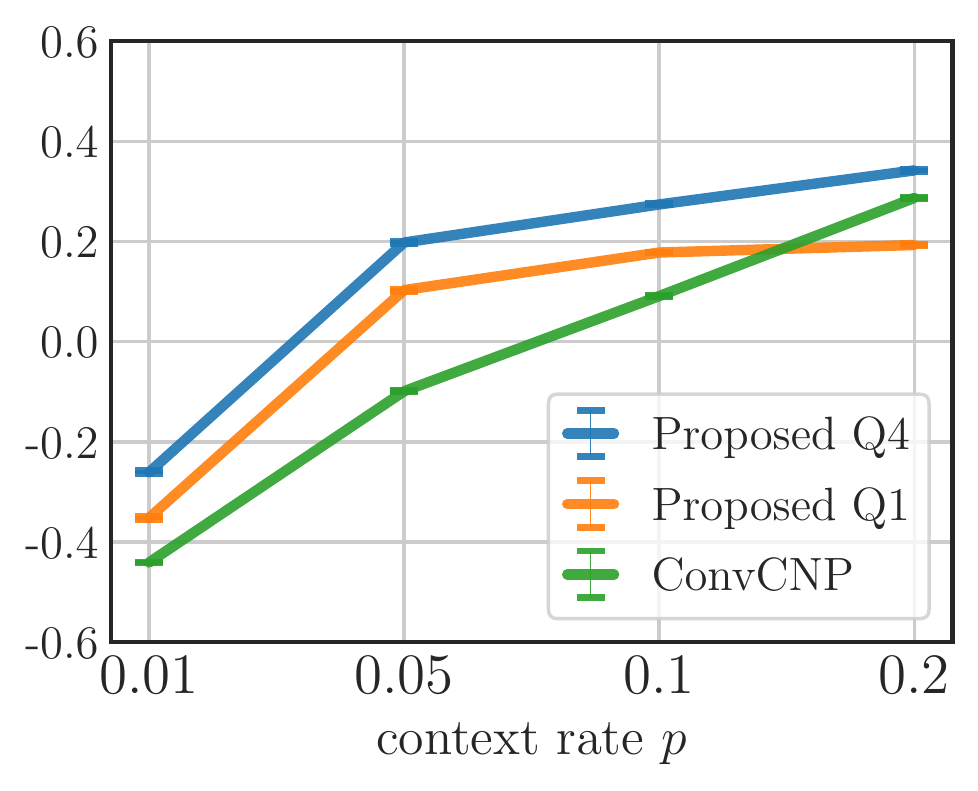}}   \hspace{0.5mm} 
\subfloat[ \label{fig:exp5-3:small-f} 5000 tasks (out-train)] 
{\includegraphics[width=0.24\linewidth]{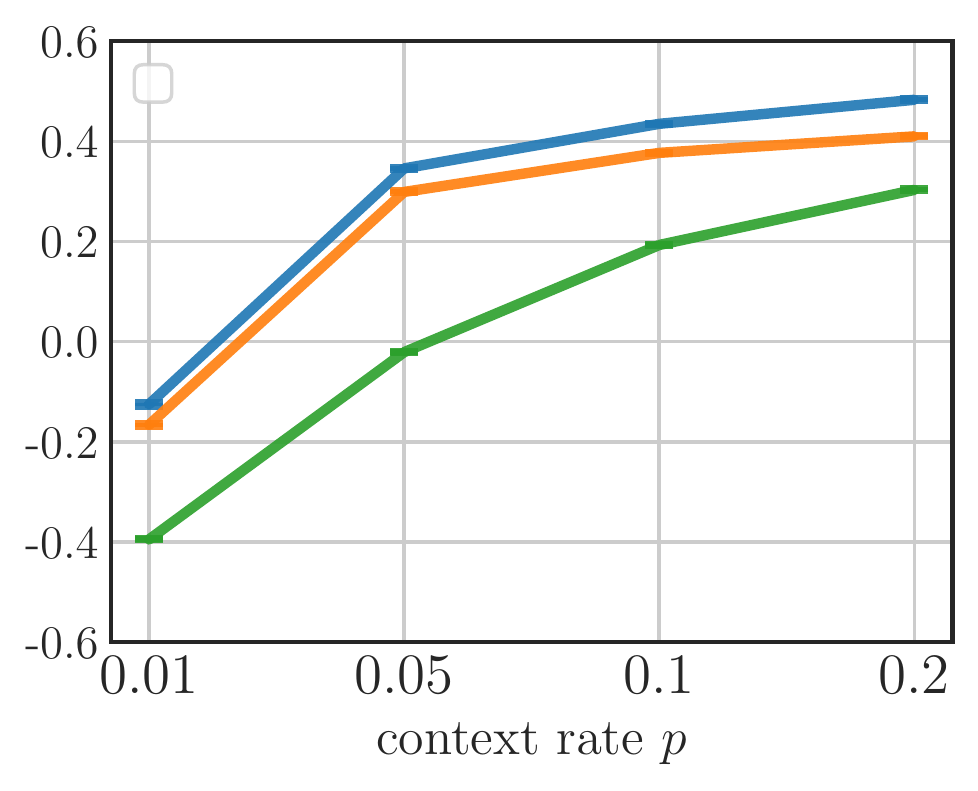}}   \hspace{0.5mm} 
\subfloat[ \label{fig:exp5-3:small-g} 7500 tasks (out-train) ]
{\includegraphics[width=0.24\linewidth]{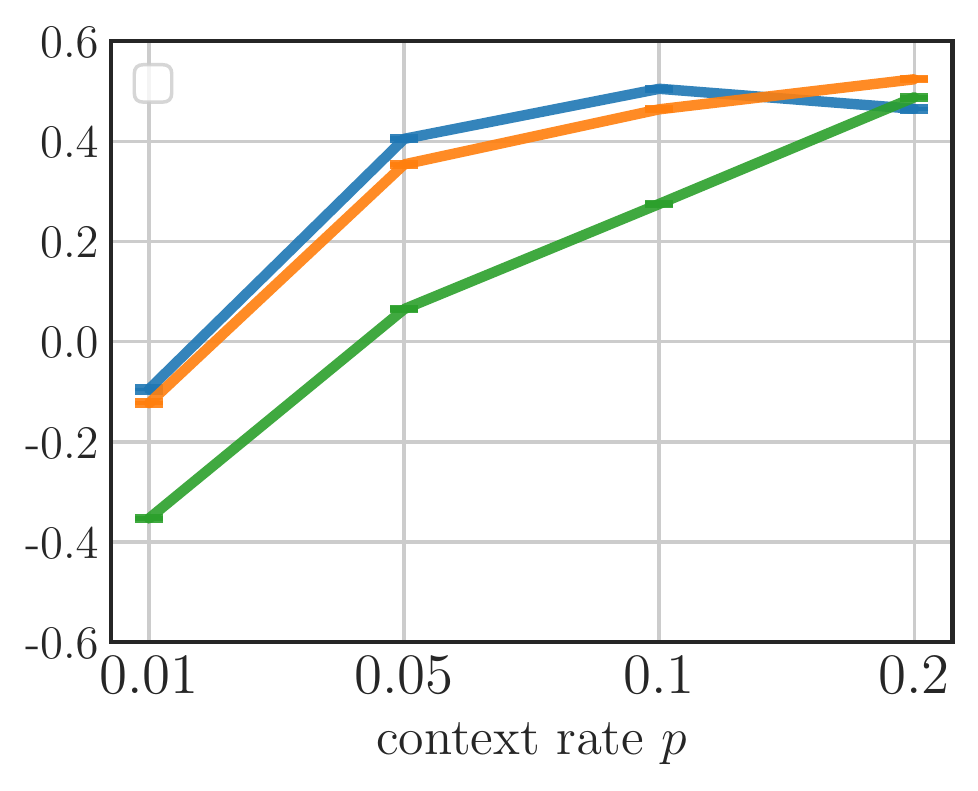}}  \hspace{0.5mm} 
\subfloat[ \label{fig:exp5-3:small-h} 10000 tasks (out-train) ]
{\includegraphics[width=0.24\linewidth]{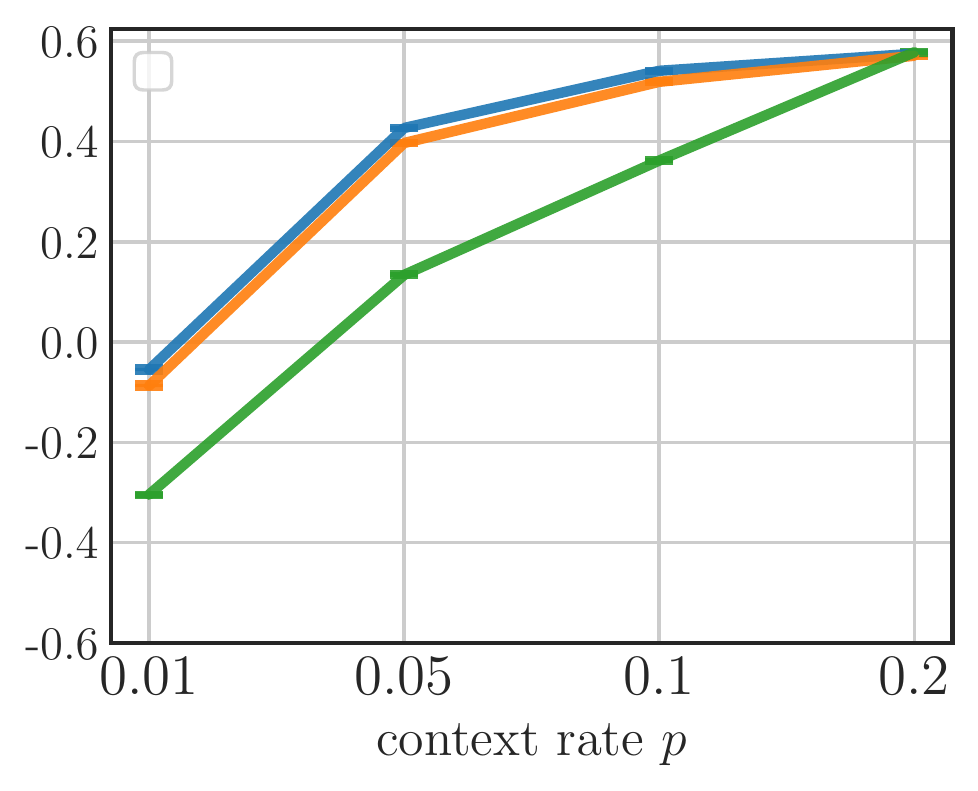}}
\caption{Test log likelihood of \textb{North America} dataset over the varying number of training tasks.}
\label{fig:exp5-3:smallset-usa-progress}
\end{figure}

\vspace{3mm}
\begin{figure}[H]
%\begin{figure}[htp!]
\centering
\subfloat[ \label{fig:exp5-3:small-a2}  2500 tasks (in-train)]
{\includegraphics[width=0.24\linewidth]{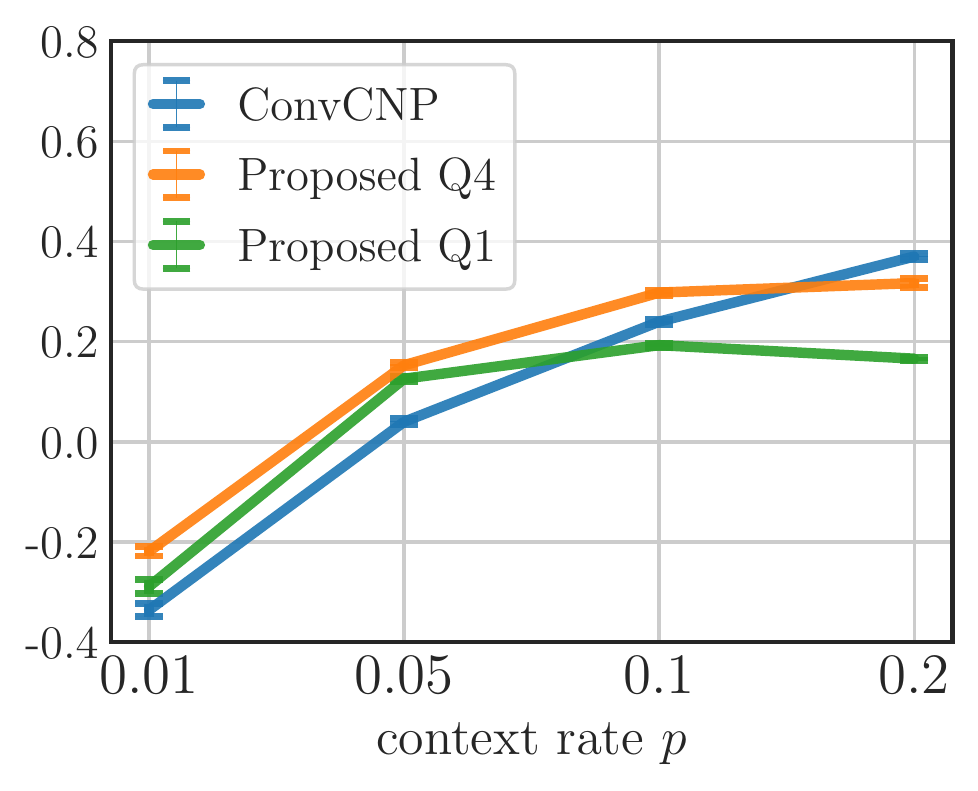}}   \hspace{0.5mm} 
\subfloat[ \label{fig:exp5-3:small-b2} 5000 tasks (in-train)] 
{\includegraphics[width=0.24\linewidth]{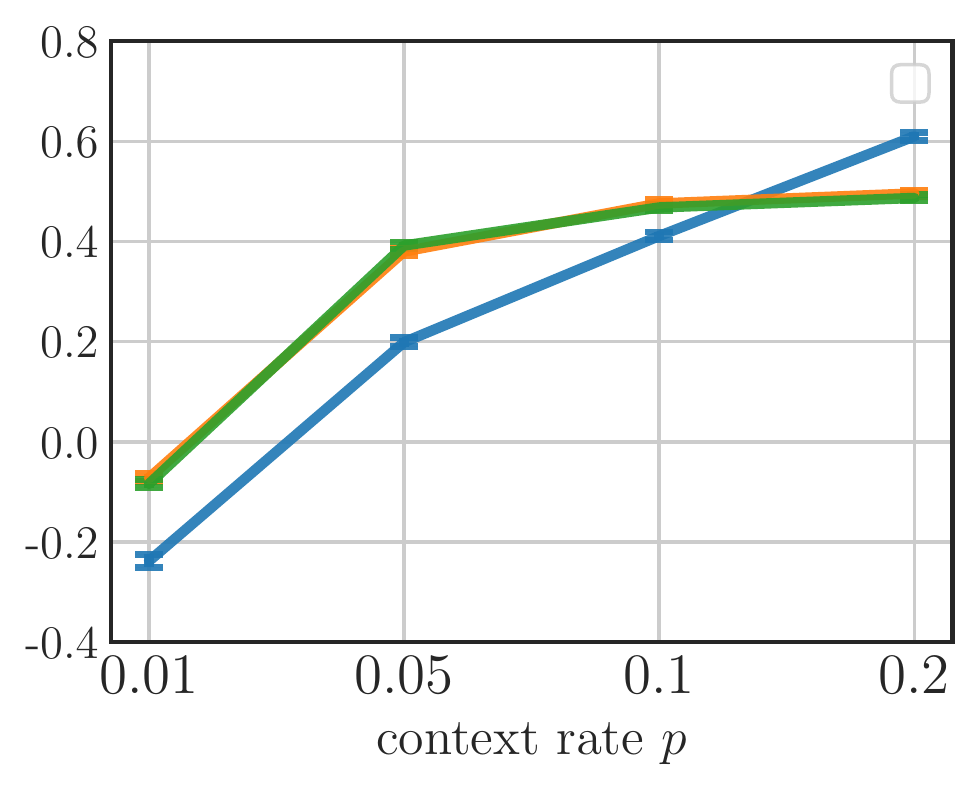}}   \hspace{0.5mm} 
\subfloat[ \label{fig:exp5-3:small-c2} 7500 tasks (in-train) ]
{\includegraphics[width=0.24\linewidth]{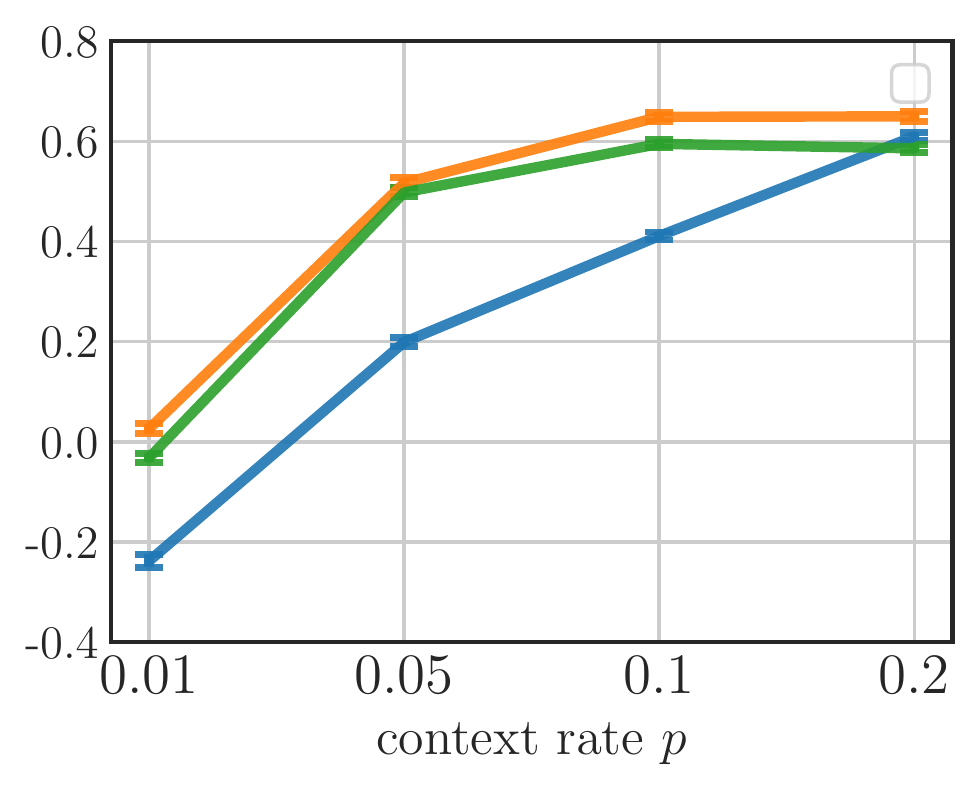}}  \hspace{0.5mm} 
\subfloat[ \label{fig:exp5-3:small-d2} 10000 tasks (in-train) ]
{\includegraphics[width=0.24\linewidth]{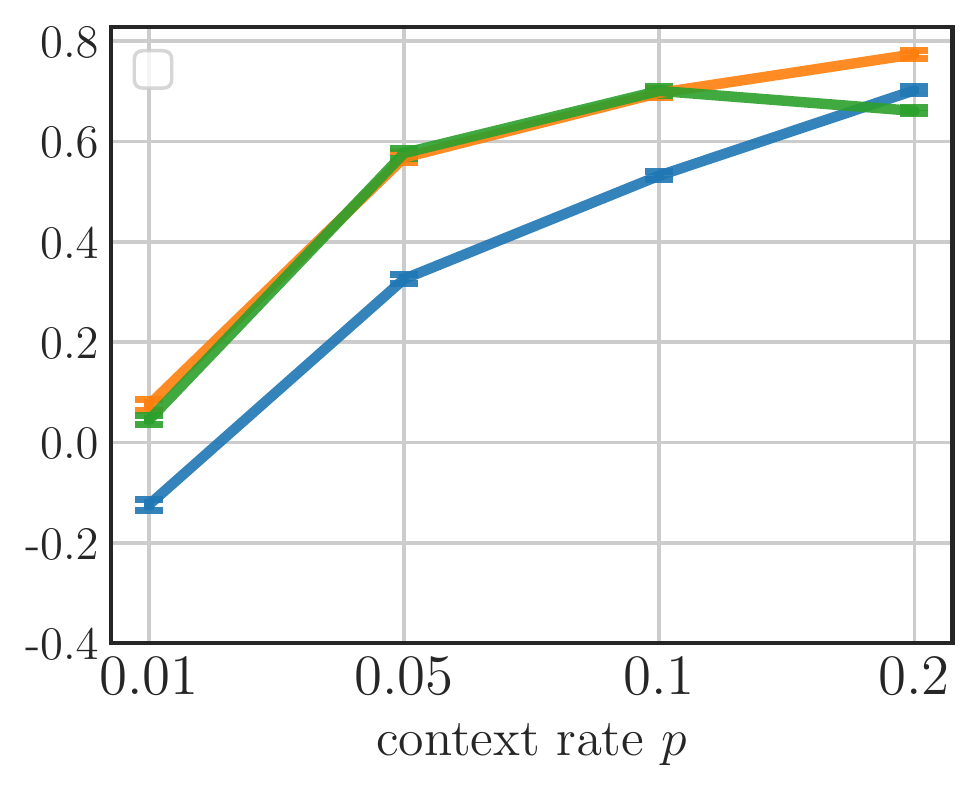}}

\vspace{2mm}
\subfloat[ \label{fig:exp5-3:small-e2}  2500 tasks (out-train)]
{\includegraphics[width=0.24\linewidth]{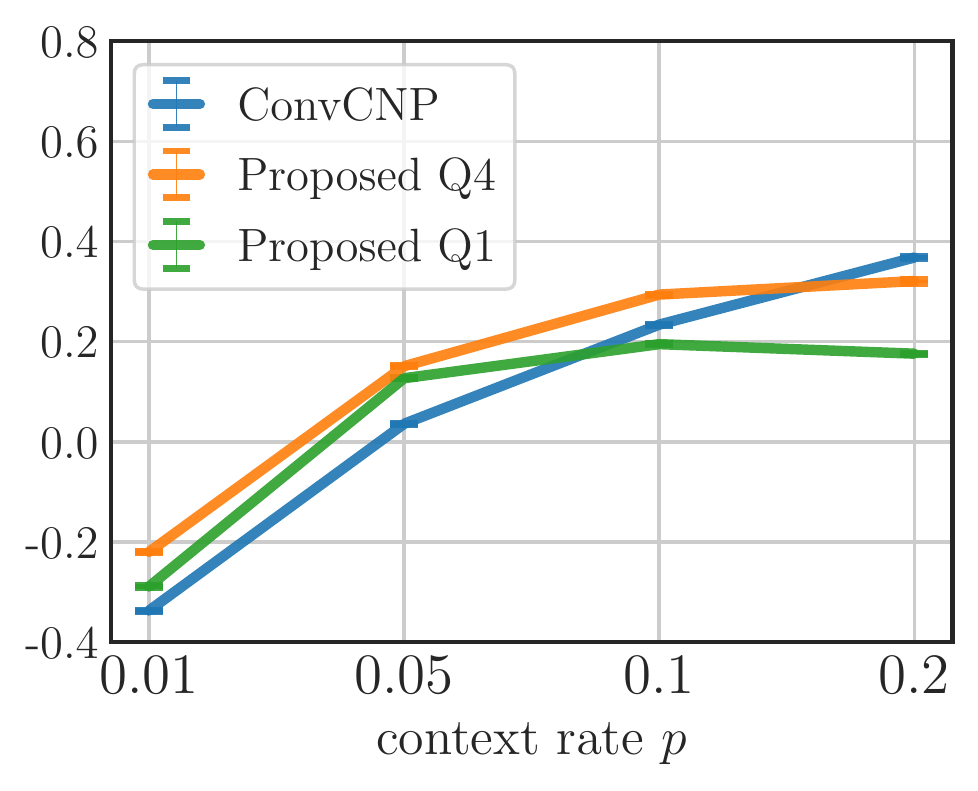}}   \hspace{0.5mm} 
\subfloat[ \label{fig:exp5-3:small-f2} 5000 tasks (out-train)] 
{\includegraphics[width=0.24\linewidth]{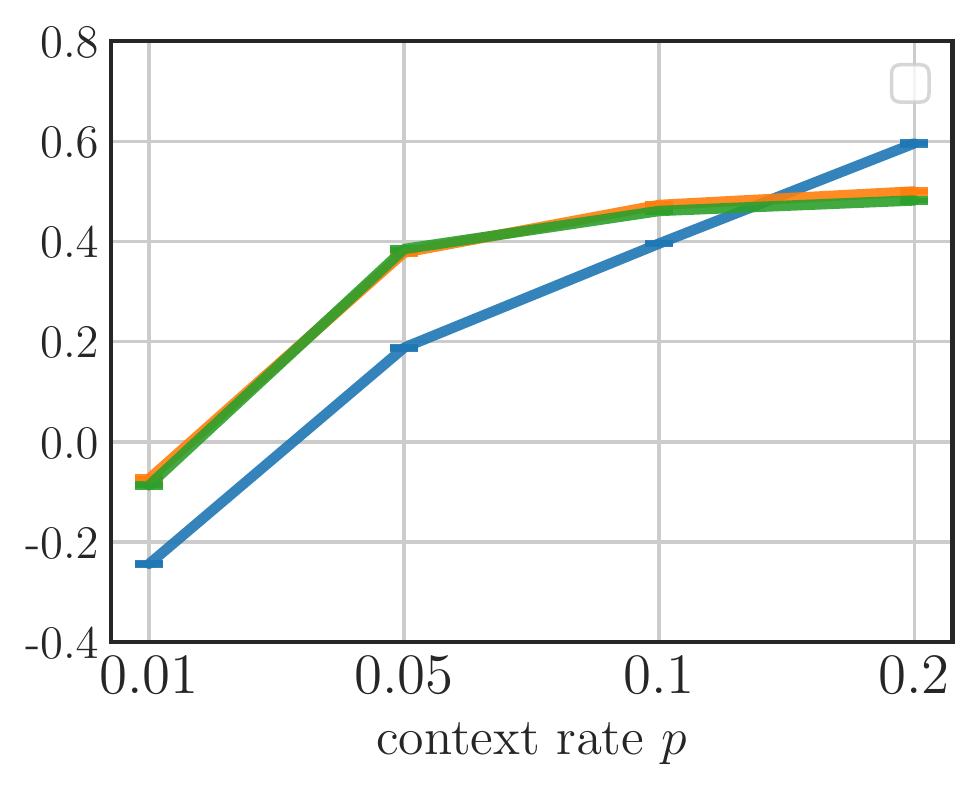}}   \hspace{0.5mm} 
\subfloat[ \label{fig:exp5-3:small-g2} 7500 tasks (out-train) ]
{\includegraphics[width=0.24\linewidth]{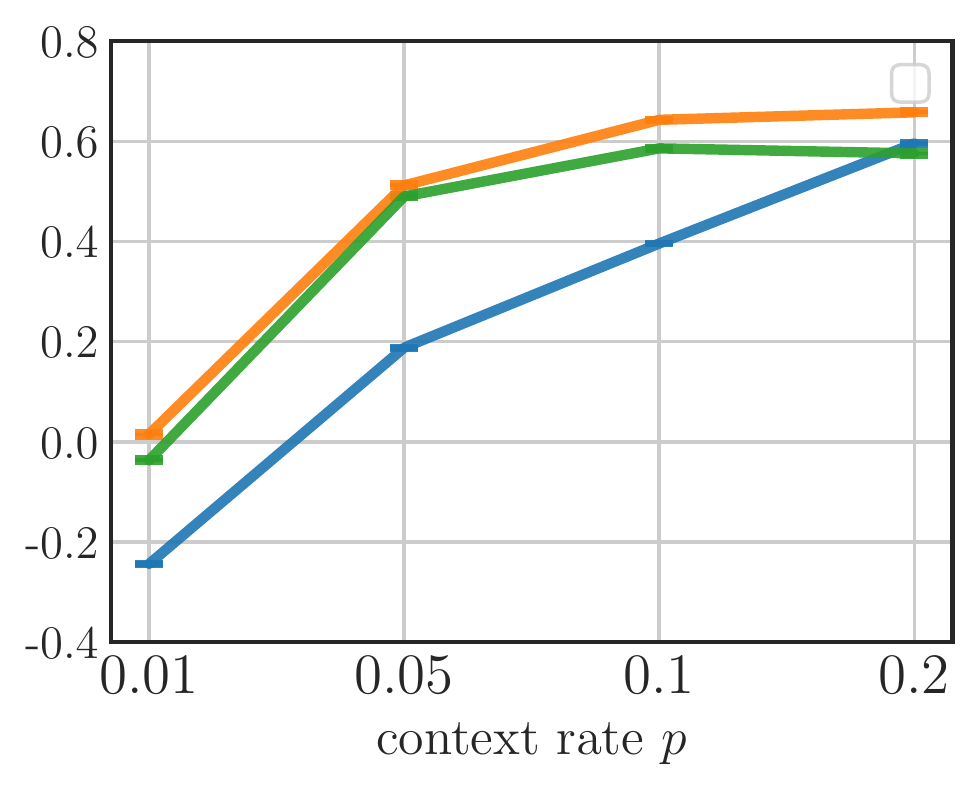}}  \hspace{0.5mm} 
\subfloat[ \label{fig:exp5-3:small-h2} 10000 tasks (out-train) ]
{\includegraphics[width=0.24\linewidth]{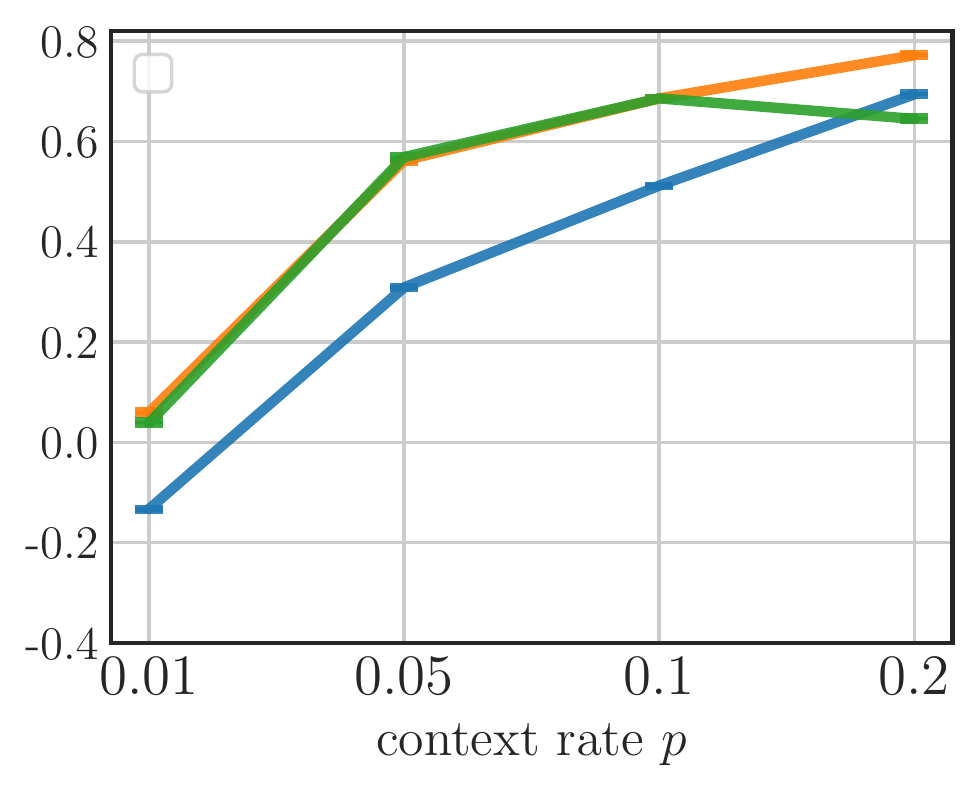}}
\caption{Test log likelihood of \textb{Europe} dataset over the varying number of training tasks.}
\label{fig:exp5-3:smallset-eu-progress}
\end{figure}

% \vspace{5mm}

% \input{07-appendix-v01-chapter4-exp3-figure01}
% \input{07-appendix-v01-chapter4-exp3-figure02}
% \input{07-appendix-v01-chapter4-exp3-figure03}
